# Supplementary material for: PyPhi: A toolbox for integrated information theory
Source: arXiv:1712.09644 ancillary file (2018-06-27)

# Calculating $\Phi$

## A tutorial

William G. P. Mayner<sup>1,2</sup>, William Marshall<sup>2</sup>, Larissa Albantakis<sup>2</sup>,  
Graham Findlay<sup>1,2</sup>, Robert Marchman<sup>2</sup>, and Giulio Tononi<sup>2</sup>

<sup>1</sup>Neuroscience Training Program, University of Wisconsin–Madison

<sup>2</sup>Department of Psychiatry, Wisconsin Institute for Sleep and Consciousness,  
University of Wisconsin–Madison

Cite as:

**PyPhi: A toolbox for integrated information theory,  
supporting information S1: Calculating Phi.** arXiv. 2018.

# Outline

- Elements, states, and the TPM
- Background conditions
- Cause-effect repertoires
- Integrated mechanisms:  $\varphi$
- Concepts and cause-effect structures
- Integrated systems:  $\Phi$
- Complexes

# Outline

- Elements, states, and the TPM
- Background conditions
- Cause-effect repertoires
- Integrated mechanisms:  $\varphi$
- Concepts and cause-effect structures
- Integrated systems:  $\Phi$
- Complexes

Introduction:

## Elements, states, and the TPM

- In integrated information theory, a physical system is represented as a network of interconnected elements
- Elements are in one of at least two **states**
- Each element receives input and provides output
- Each element has an **input-output function** for transitioning from one state to another

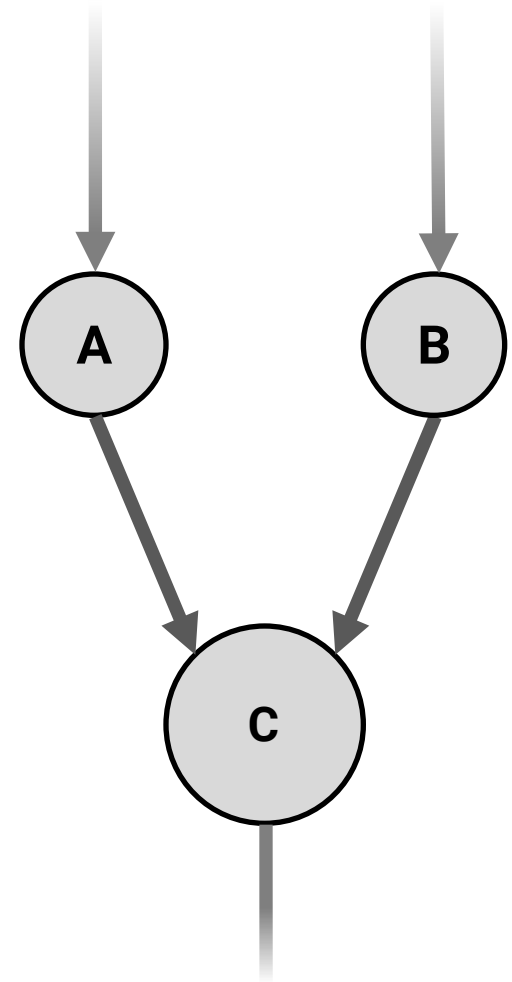

Introduction:

## Elements, states, and the TPM

- An element's input-output function can be fully characterized by a **transition probability matrix** (TPM) that gives the probabilities of each possible state transition
- The TPM can be calculated by perturbing the element's inputs into all possible configurations and recording the results

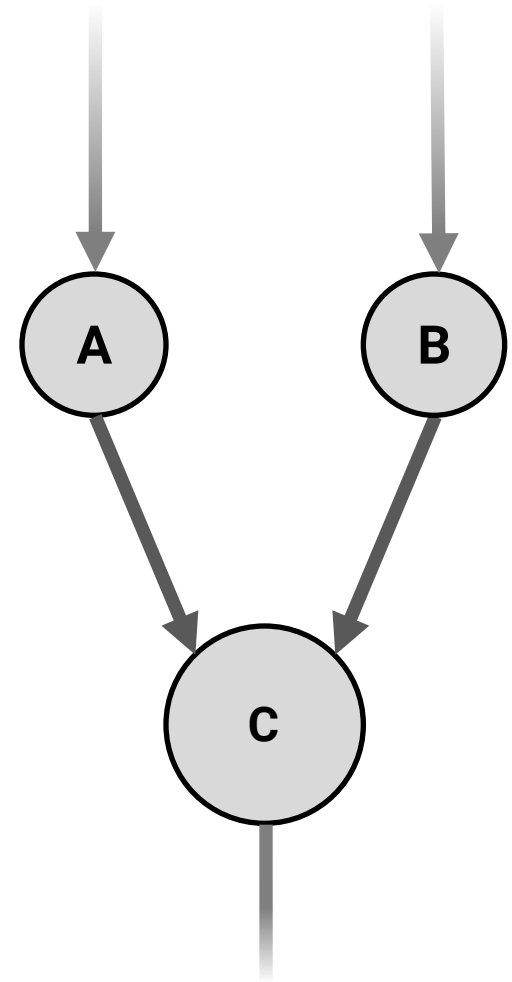

Introduction:

## Elements, states, and the TPM

- We'll do this for element **C**
- We start by setting **A** and **B** to their OFF state in the current timestep,  $t$

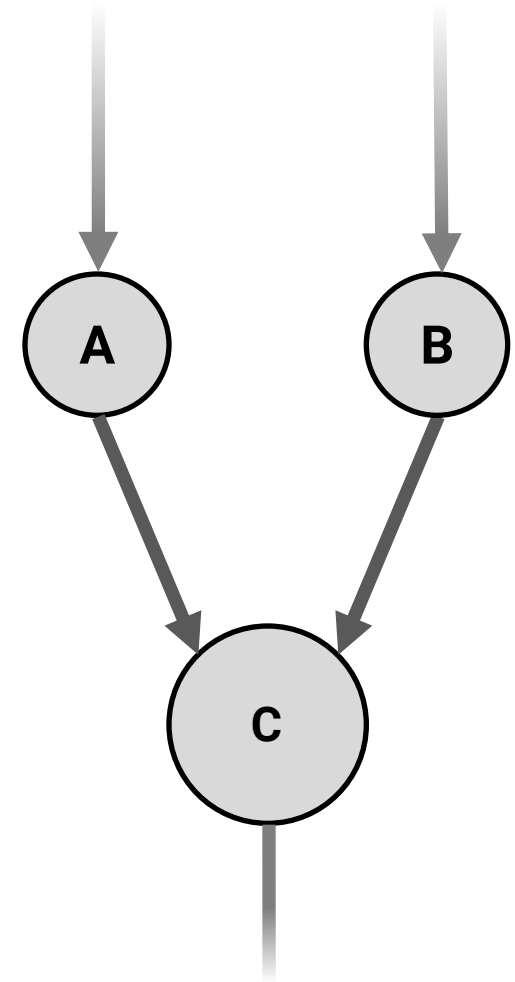

Introduction:

## Elements, states, and the TPM

- We'll do this for element **C**
- We start by setting **A** and **B** to their OFF state in the current timestep,  $t$

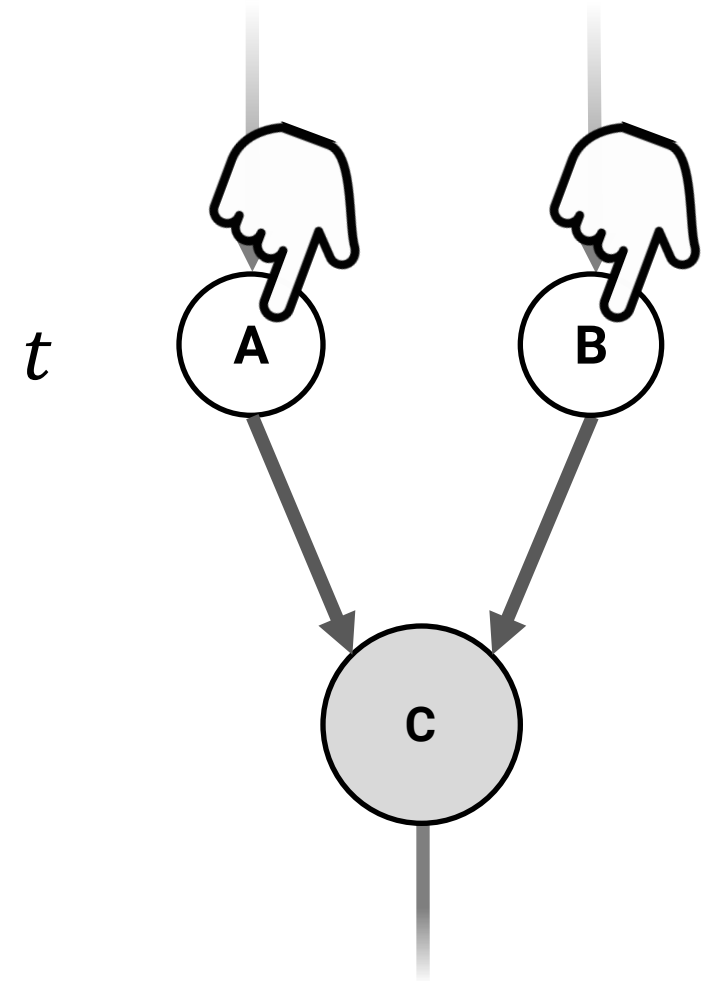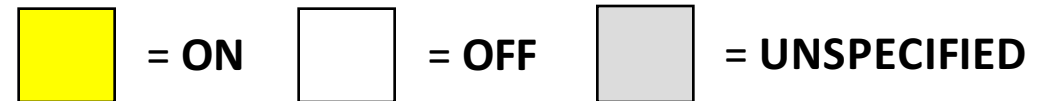

# Introduction:

## Elements, states, and the TPM

|               |                       |                       | Next state            |                                  |
|---------------|-----------------------|-----------------------|-----------------------|----------------------------------|
|               |                       |                       | C                     |                                  |
| Current state | A                     | B                     |                       |                                  |
|               | <input type="radio"/> | <input type="radio"/> | <input type="radio"/> | <input checked="" type="radio"/> |

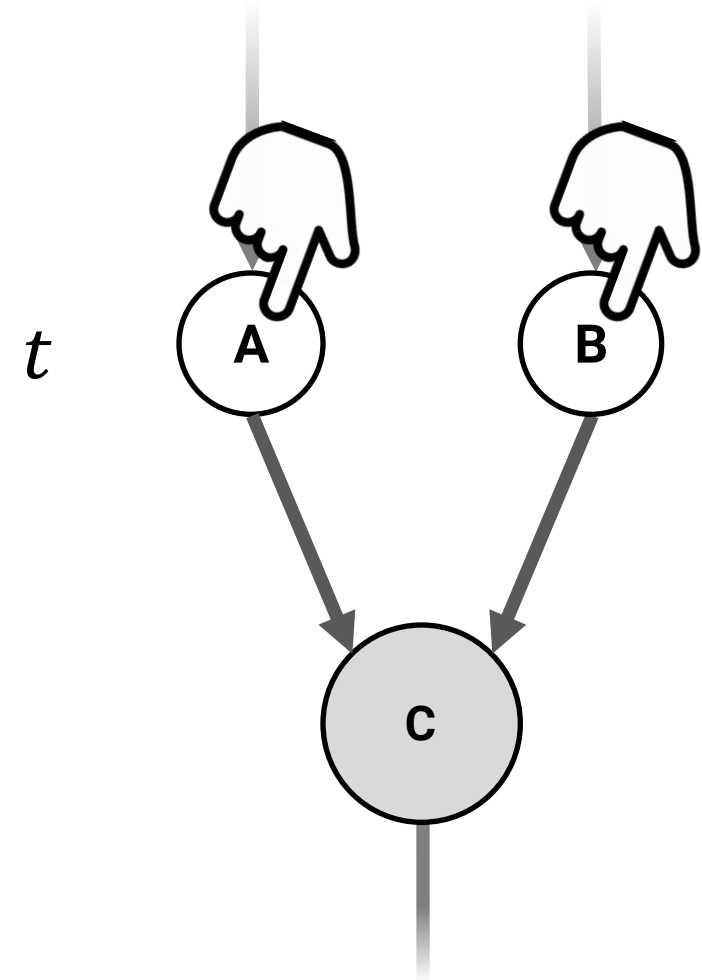

☒ = ON    ☐ = OFF    ☐ = UNSPECIFIED



# Introduction:

## Elements, states, and the TPM

|               |                       |                       | Next state            |                                  |
|---------------|-----------------------|-----------------------|-----------------------|----------------------------------|
| Current state | A                     | B                     | C                     |                                  |
|               | <input type="radio"/> | <input type="radio"/> | <input type="radio"/> | <input checked="" type="radio"/> |
|               | <input type="radio"/> | <input type="radio"/> | 1                     | 0                                |

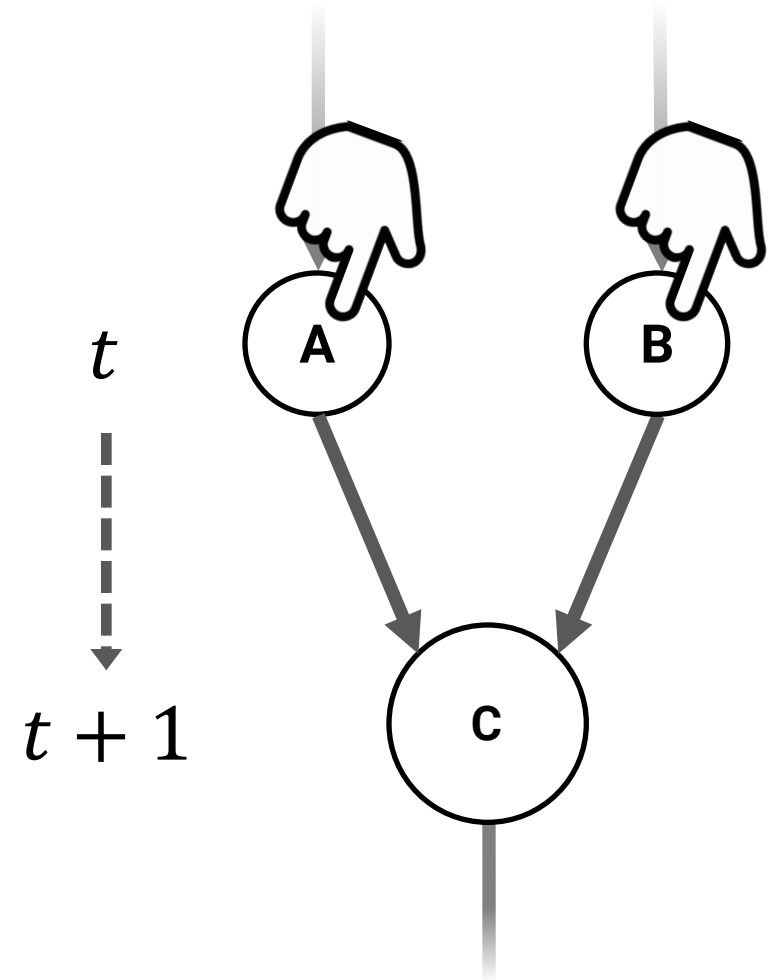

☒ = ON    ☐ = OFF    ☐ = UNSPECIFIED

# Introduction:

## Elements, states, and the TPM

|               |                                                        | Next state            |                                  |
|---------------|--------------------------------------------------------|-----------------------|----------------------------------|
|               |                                                        | C                     |                                  |
| Current state | A B                                                    | <input type="radio"/> | <input checked="" type="radio"/> |
|               | <input type="radio"/> <input type="radio"/>            | 1                     | 0                                |
|               | <input checked="" type="radio"/> <input type="radio"/> |                       |                                  |

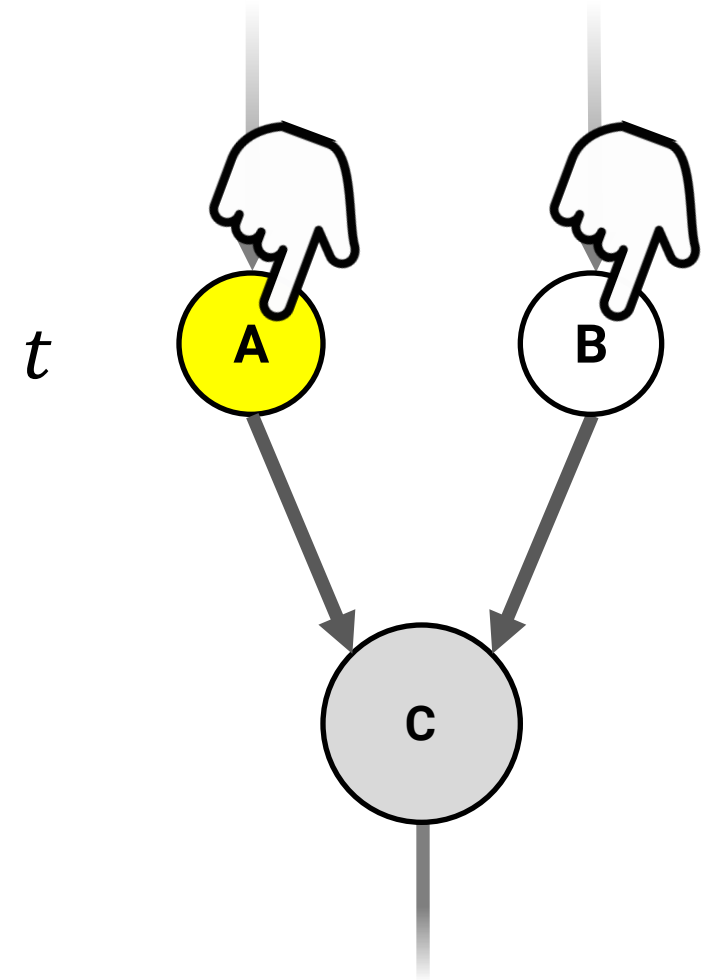

☒ = ON    ☐ = OFF    ☐ = UNSPECIFIED

# Introduction:

## Elements, states, and the TPM

|               |                                  | Next state            |          |
|---------------|----------------------------------|-----------------------|----------|
|               |                                  | <b>C</b>              |          |
| Current state | <b>A</b>                         | <b>B</b>              |          |
|               | <input type="radio"/>            | <input type="radio"/> | <b>1</b> |
|               | <input checked="" type="radio"/> | <input type="radio"/> | <b>1</b> |

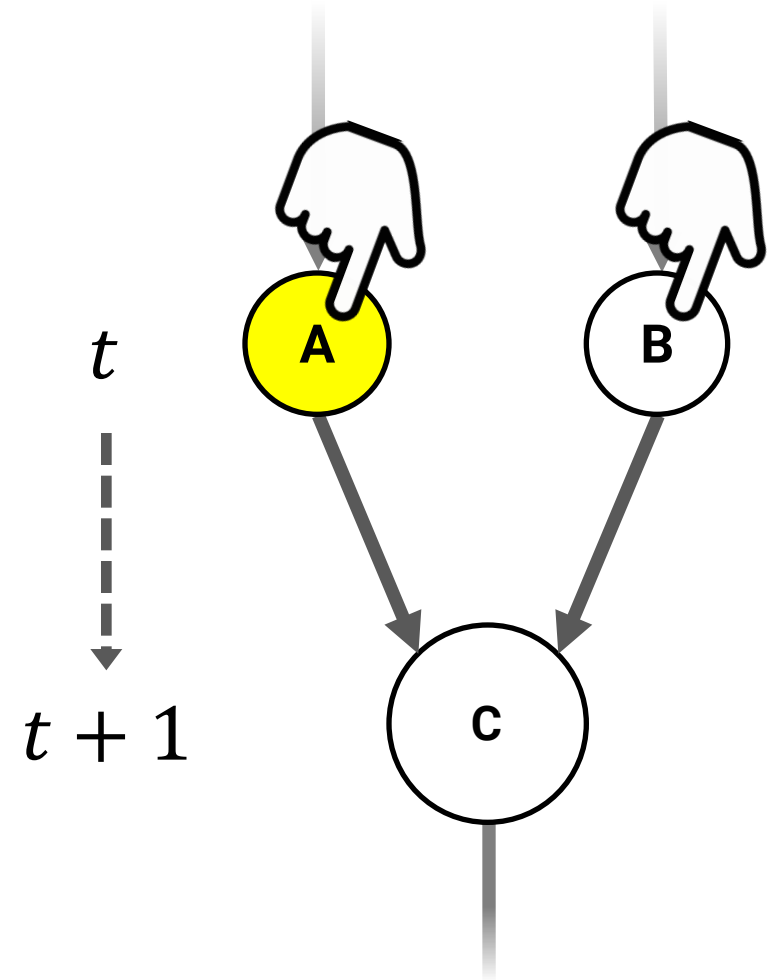

☒ = ON    ☐ = OFF    ☐ = UNSPECIFIED

# Introduction:

## Elements, states, and the TPM

|               |                                  | Next state            |                                  |
|---------------|----------------------------------|-----------------------|----------------------------------|
| Current state |                                  |                       |                                  |
|               | A                                | B                     | C                                |
|               | <input type="radio"/>            | <input type="radio"/> | <input type="radio"/>            |
|               | <input type="radio"/>            | <input type="radio"/> | <input checked="" type="radio"/> |
|               | <input type="radio"/>            | <input type="radio"/> |                                  |
|               | <input checked="" type="radio"/> | <input type="radio"/> |                                  |
|               | <input type="radio"/>            | <input type="radio"/> |                                  |
|               | <input checked="" type="radio"/> | <input type="radio"/> |                                  |

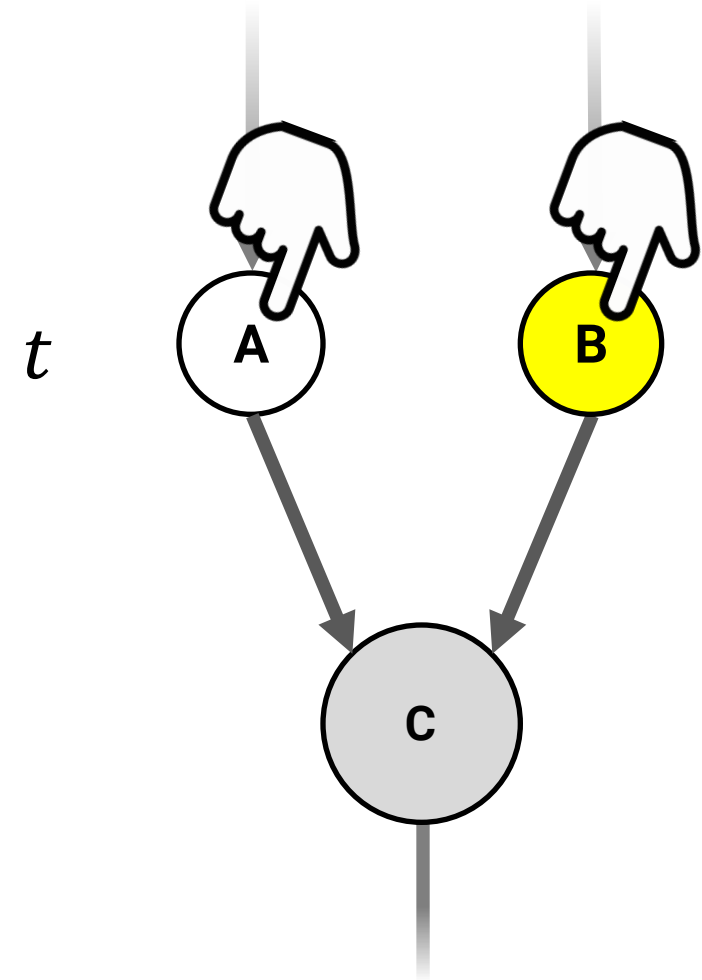

☒ = ON    ☐ = OFF    ☐ = UNSPECIFIED

# Introduction:

## Elements, states, and the TPM

|               |                                  | Next state                       |          |
|---------------|----------------------------------|----------------------------------|----------|
|               |                                  | <b>C</b>                         |          |
| Current state | <b>A</b>                         | <b>B</b>                         |          |
|               | <input type="radio"/>            | <input type="radio"/>            | <b>1</b> |
|               | <input checked="" type="radio"/> | <input type="radio"/>            | <b>1</b> |
|               | <input type="radio"/>            | <input checked="" type="radio"/> | <b>1</b> |

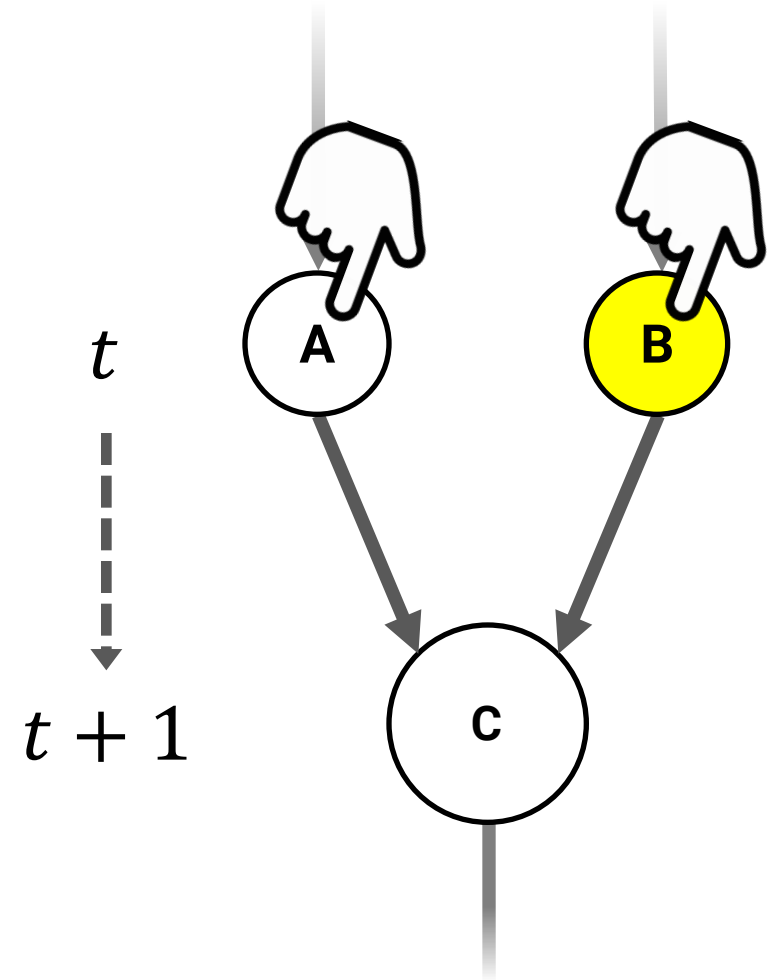

☒ = ON    ☐ = OFF    ☐ = UNSPECIFIED

# Introduction:

## Elements, states, and the TPM

|               |                                                                   | Next state            |                                  |
|---------------|-------------------------------------------------------------------|-----------------------|----------------------------------|
|               |                                                                   | C                     |                                  |
| Current state | A B                                                               | <input type="radio"/> | <input checked="" type="radio"/> |
|               | <input type="radio"/> <input type="radio"/>                       | 1                     | 0                                |
|               | <input checked="" type="radio"/> <input type="radio"/>            | 1                     | 0                                |
|               | <input type="radio"/> <input checked="" type="radio"/>            | 1                     | 0                                |
|               | <input checked="" type="radio"/> <input checked="" type="radio"/> |                       |                                  |

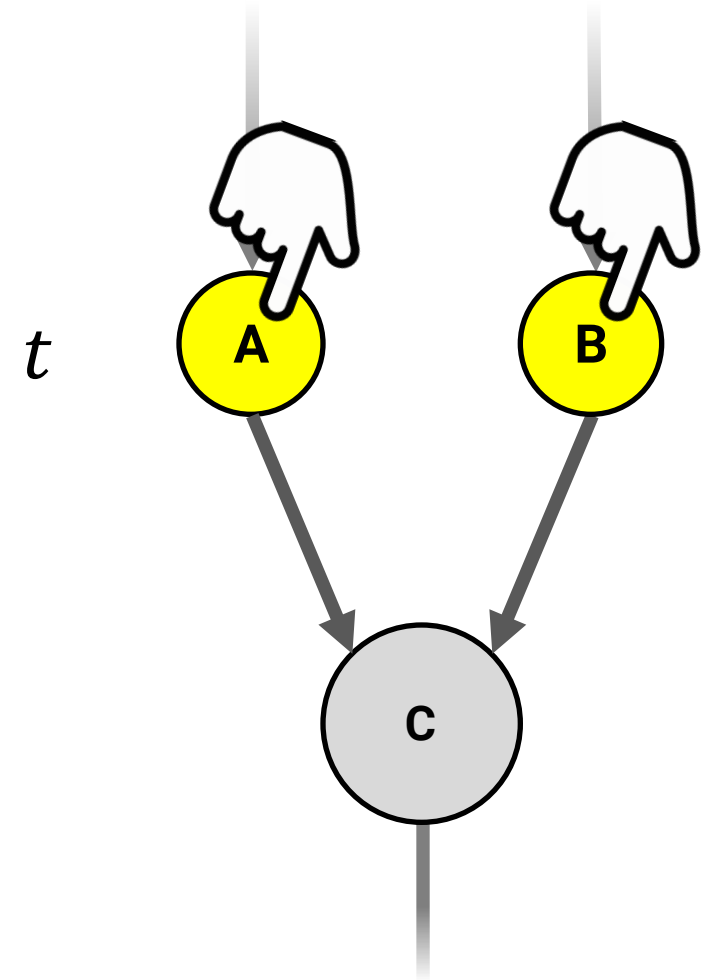

☒ = ON    ☐ = OFF    ☐ = UNSPECIFIED

# Introduction:

## Elements, states, and the TPM

|               |                                                                   | Next state |   |
|---------------|-------------------------------------------------------------------|------------|---|
|               |                                                                   | C          |   |
| Current state | A B                                                               |            |   |
|               | <input type="radio"/> <input type="radio"/>                       | 1          | 0 |
|               | <input checked="" type="radio"/> <input type="radio"/>            | 1          | 0 |
|               | <input type="radio"/> <input checked="" type="radio"/>            | 1          | 0 |
|               | <input checked="" type="radio"/> <input checked="" type="radio"/> | 0          | 1 |

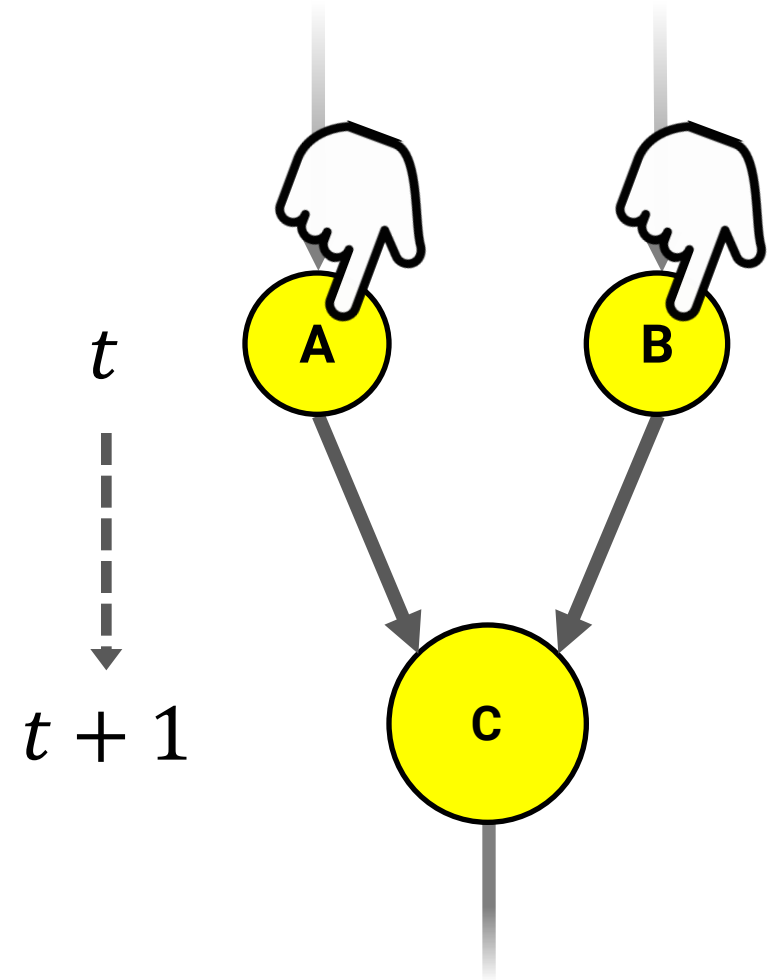

☒ = ON    ☐ = OFF    ☐ = UNSPECIFIED

Introduction:

## Elements, states, and the TPM

|               |                                                                                     |                                                                                     | Next state |   |
|---------------|-------------------------------------------------------------------------------------|-------------------------------------------------------------------------------------|------------|---|
| Current state |                                                                                     |                                                                                     | C          |   |
|               | A                                                                                   | B                                                                                   |            |   |
|               | 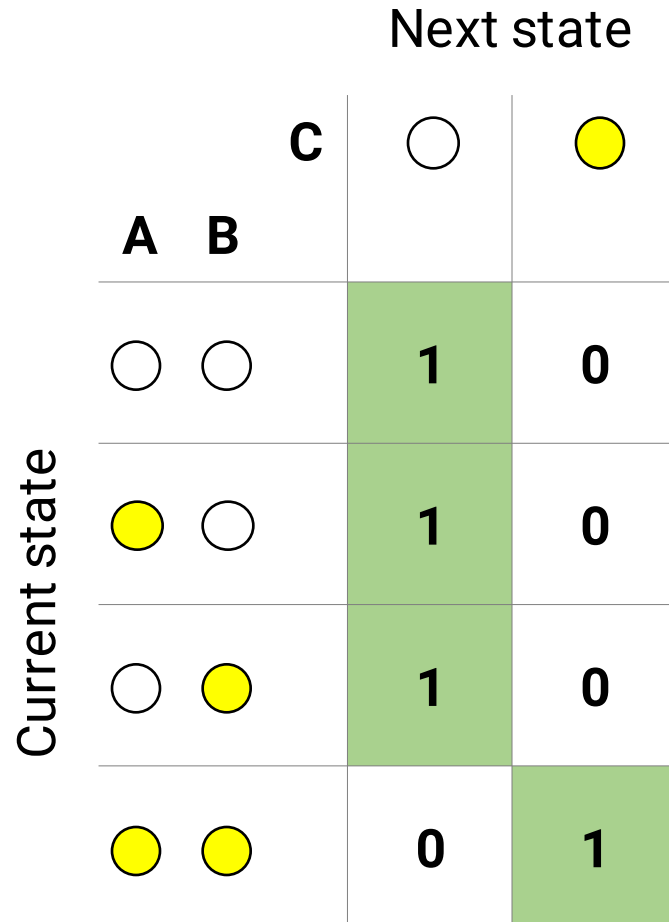   | 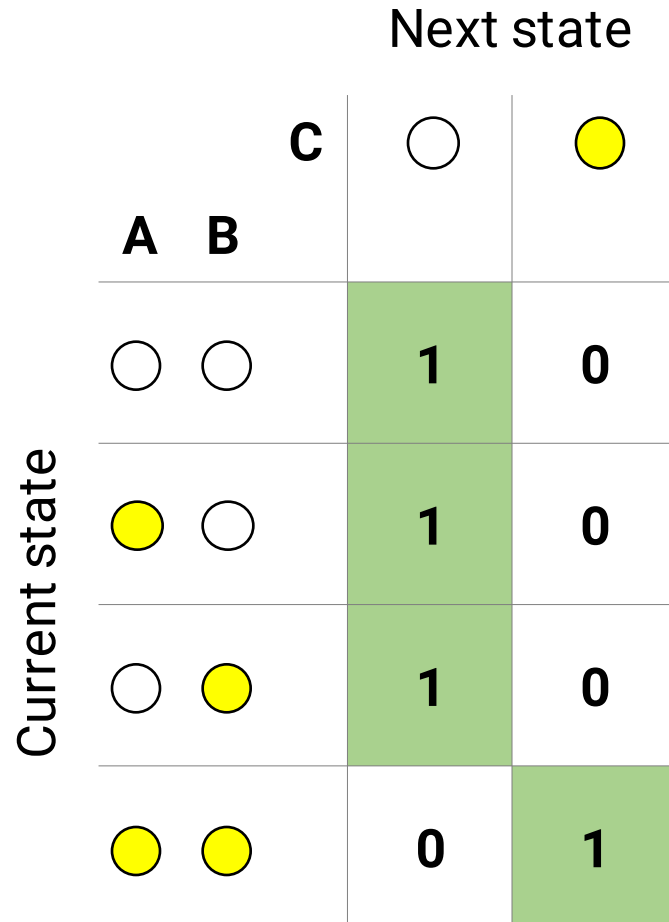   | 1          | 0 |
|               | 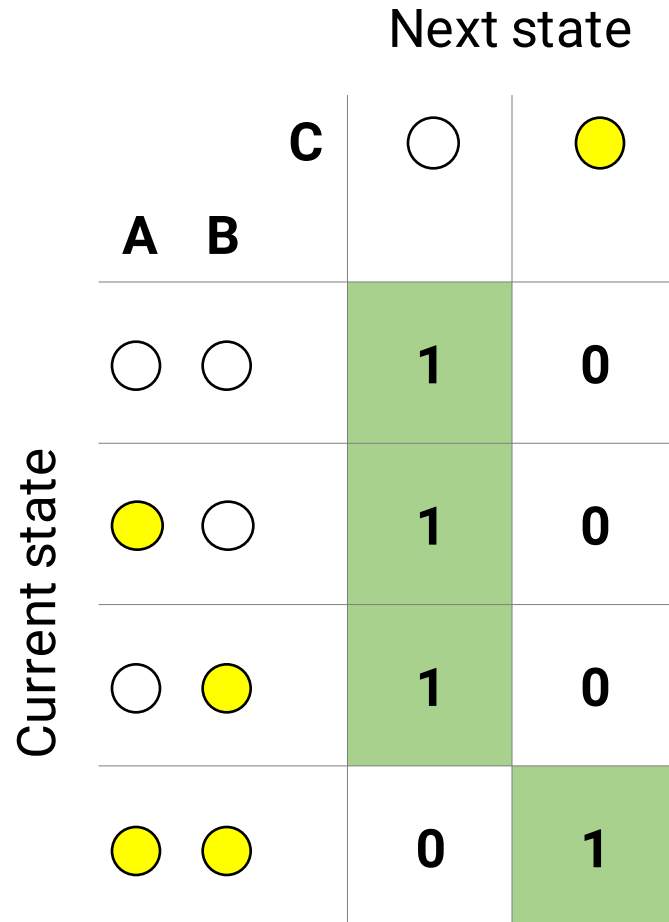   | 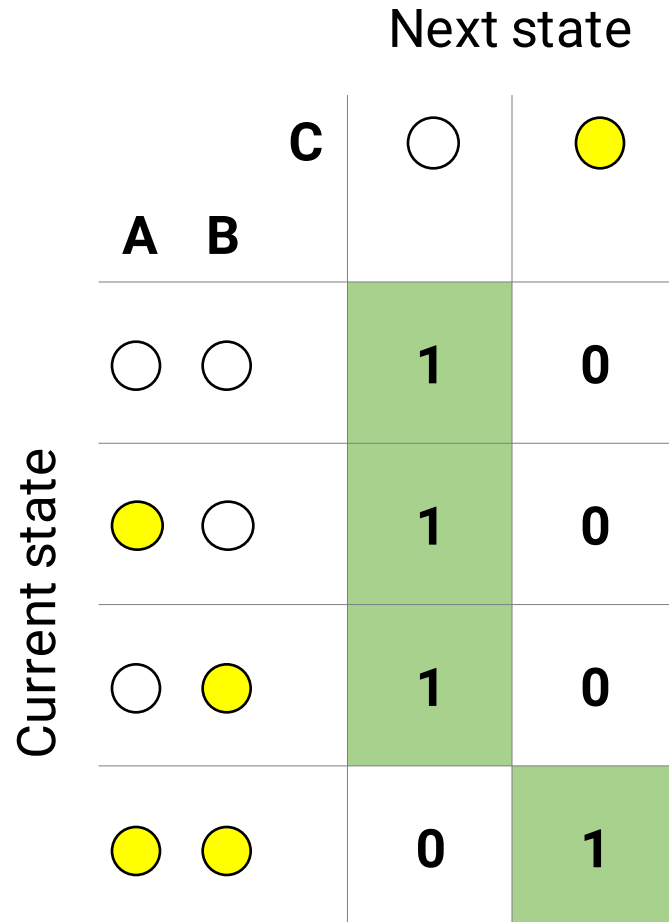   | 1          | 0 |
|               | 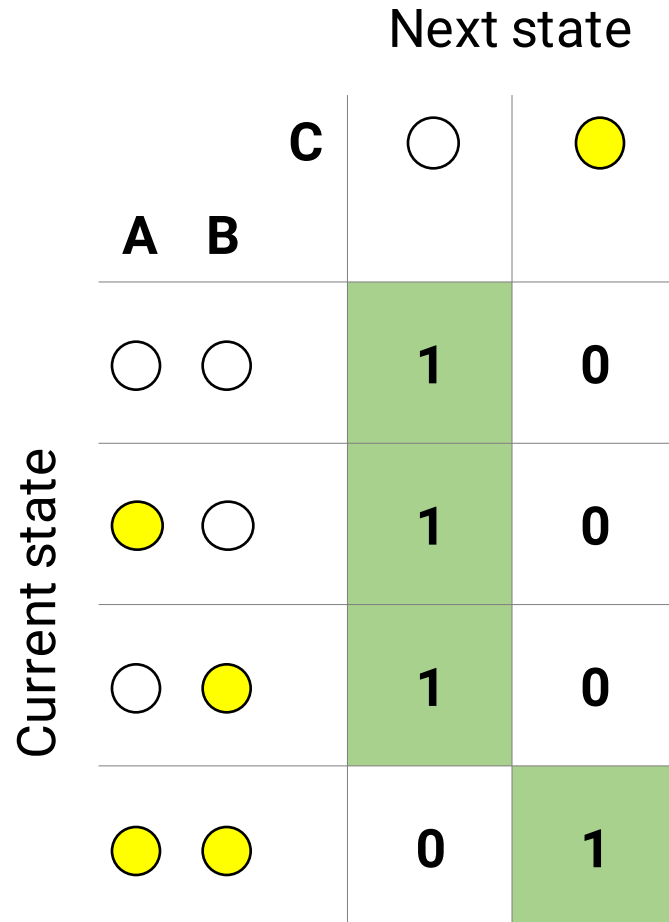 | 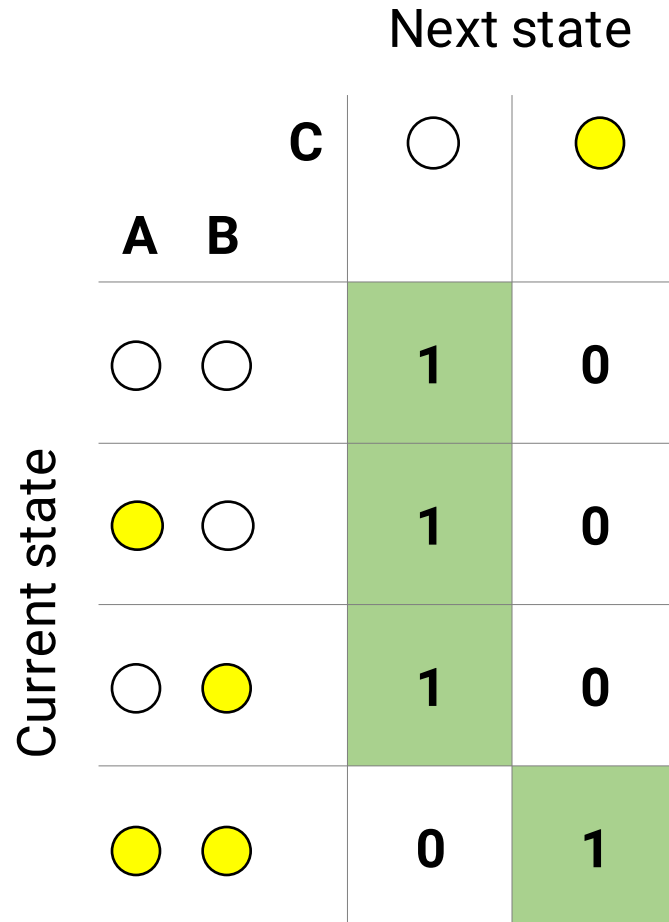 | 1          | 0 |
|               | 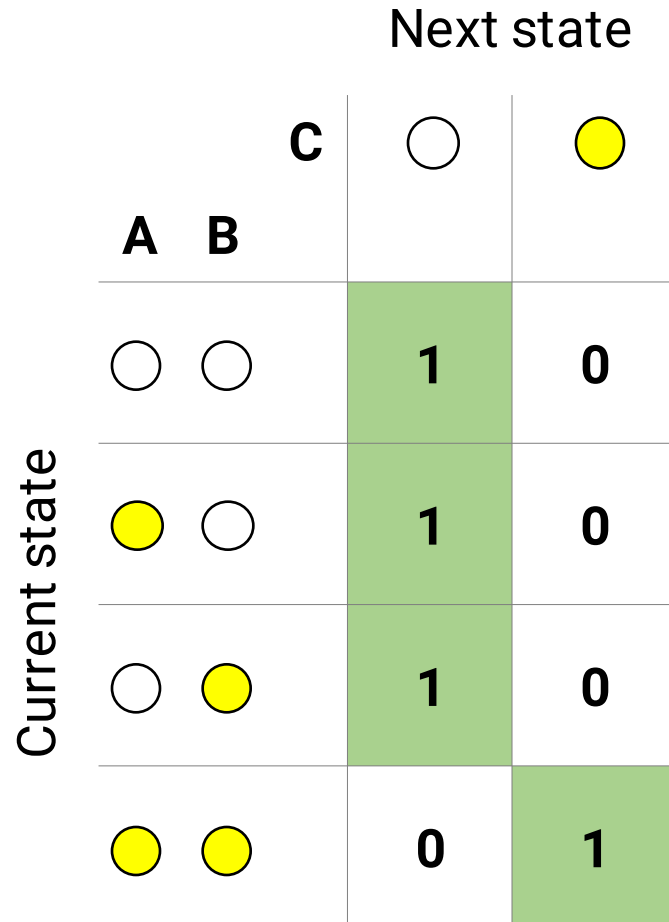 | 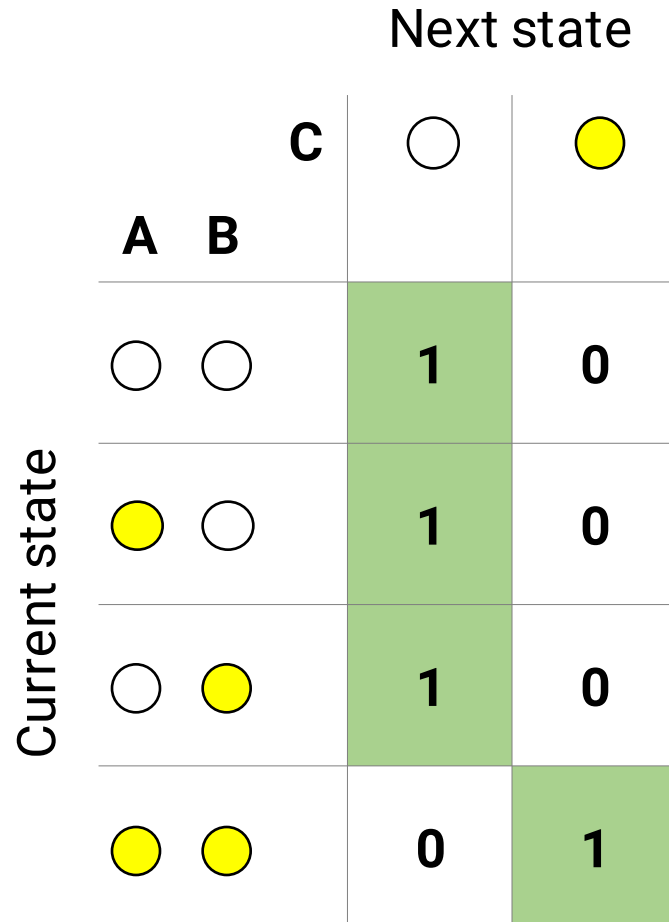 | 0          | 1 |

- Here we can see that **C** is in fact an AND gate
- It is on at  $t + 1$  when its inputs are both on at  $t$ , and off otherwise



# Introduction:

## **Nondeterministic mechanisms**

- In general, input-output functions can be nondeterministic
- For example, we could have an element with this TPM:
- Here, **C** is a noisy AND gate; its next state is somewhat uncertain (so we repeat the perturbations many times)

|                                                                                       |                                                                                       |                                                                                      | Next state                                                                          |                                                                                     |
|---------------------------------------------------------------------------------------|---------------------------------------------------------------------------------------|--------------------------------------------------------------------------------------|-------------------------------------------------------------------------------------|-------------------------------------------------------------------------------------|
|                                                                                       |                                                                                       |                                                                                      | 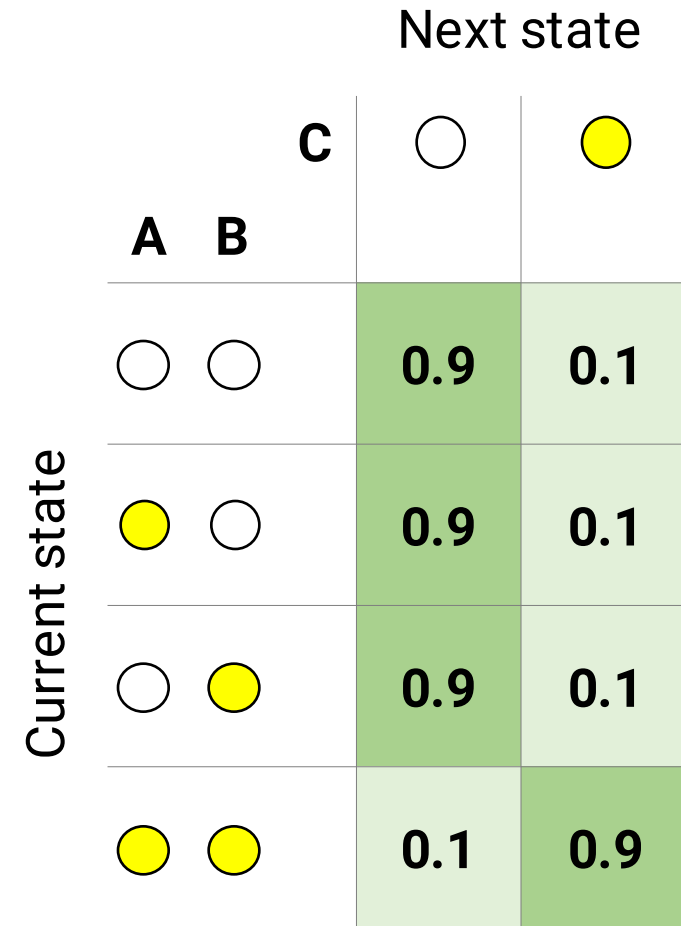 | 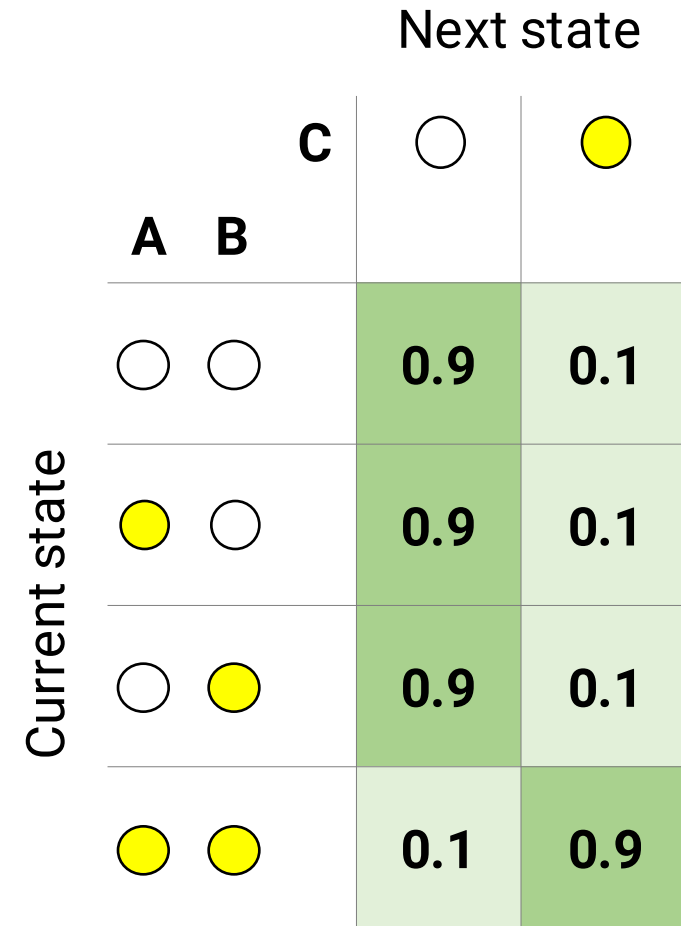 |
| Current state                                                                         | A                                                                                     | B                                                                                    | C                                                                                   |                                                                                     |
|                                                                                       |                                                                                       |                                                                                      |                                                                                     |                                                                                     |
|                                                                                       | 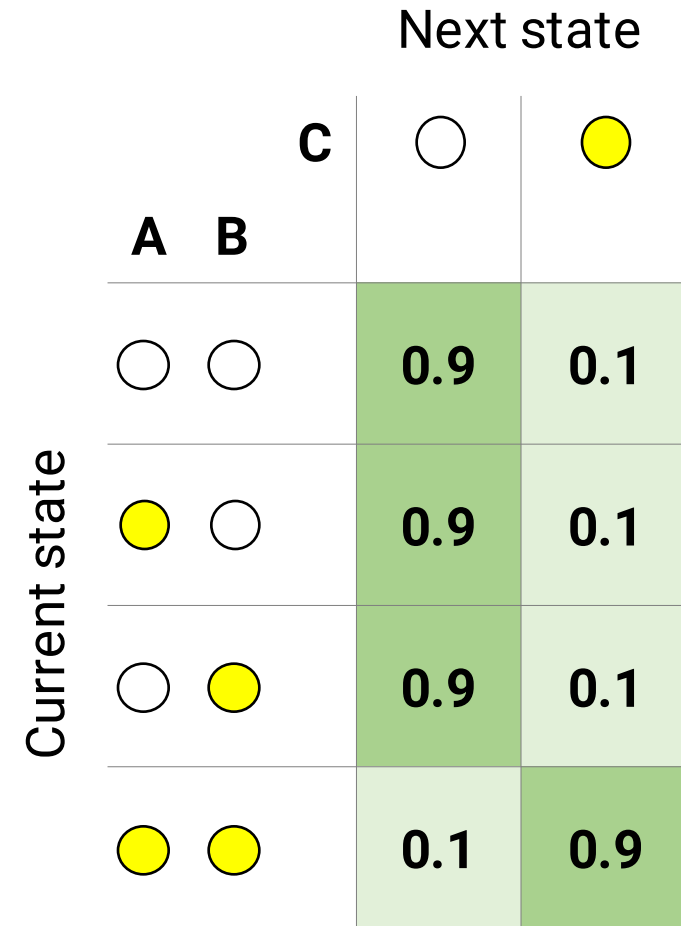   | 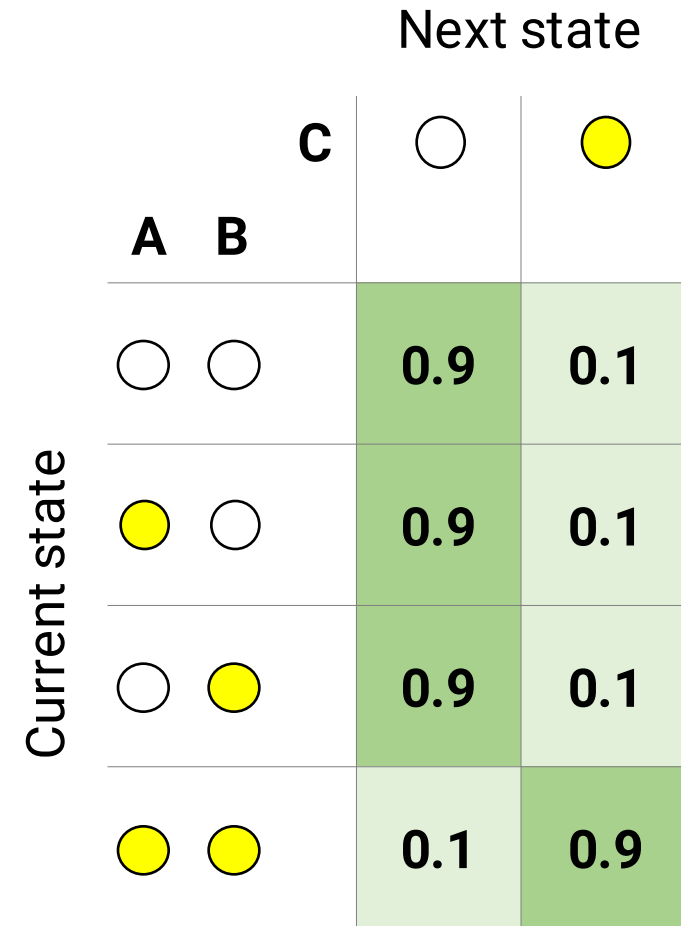  | 0.9                                                                                 | 0.1                                                                                 |
|                                                                                       | 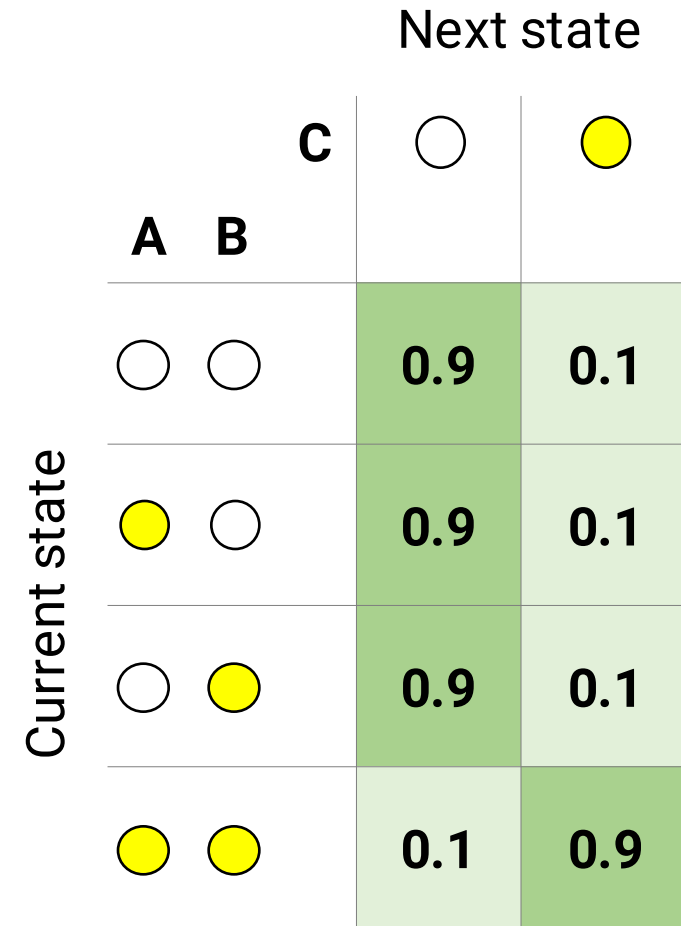   | 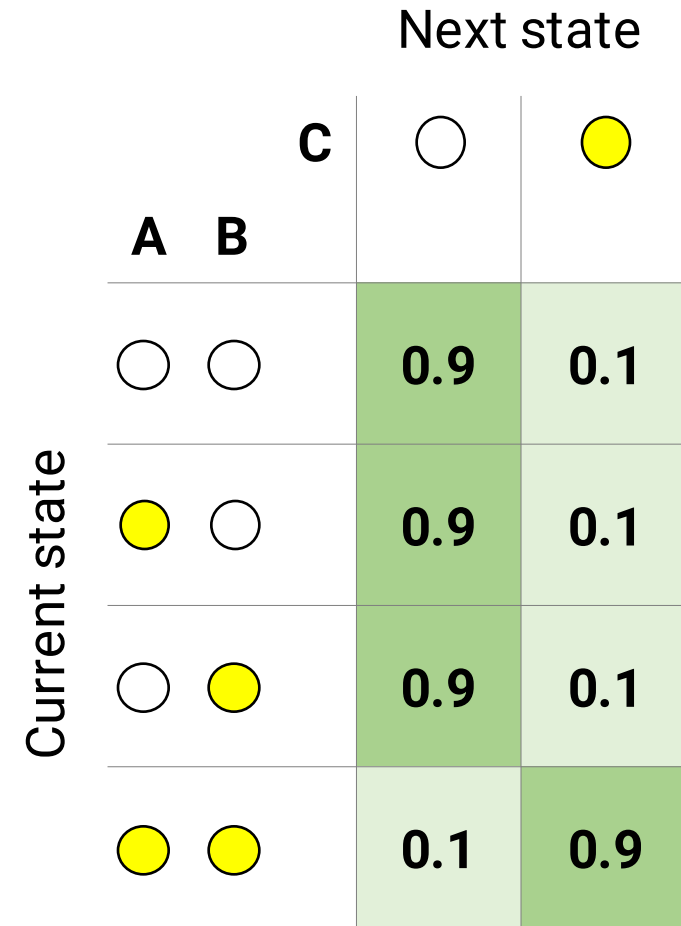  | 0.9                                                                                 | 0.1                                                                                 |
|                                                                                       | 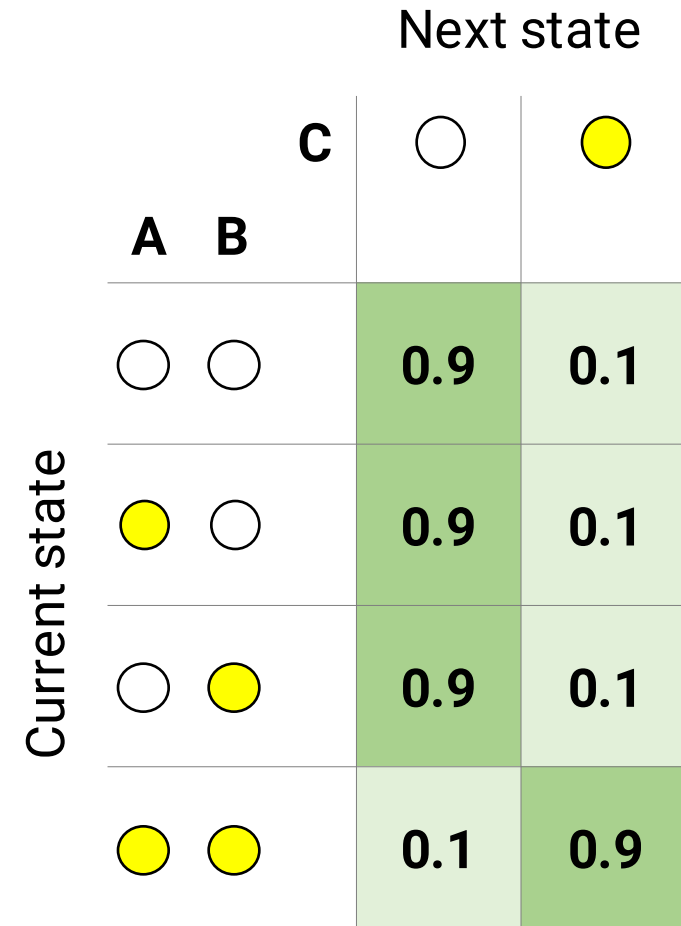  | 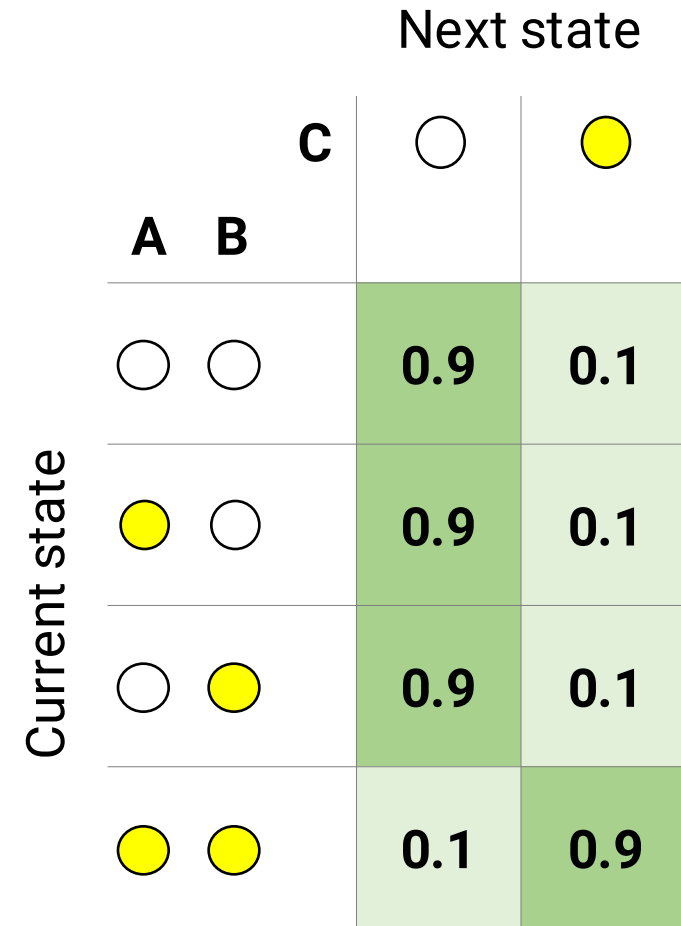 | 0.9                                                                                 | 0.1                                                                                 |
| 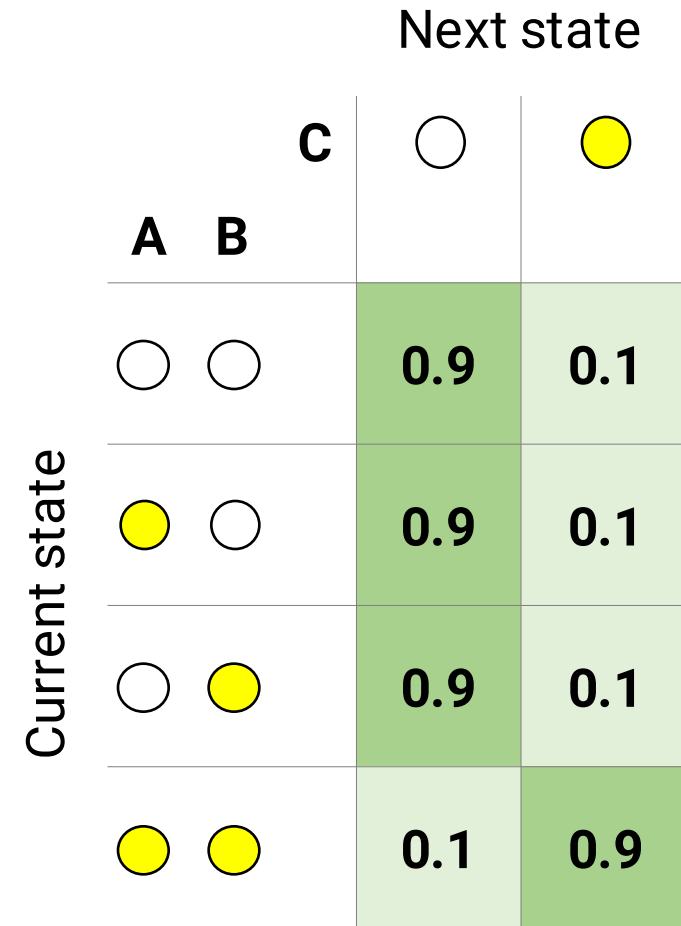 | 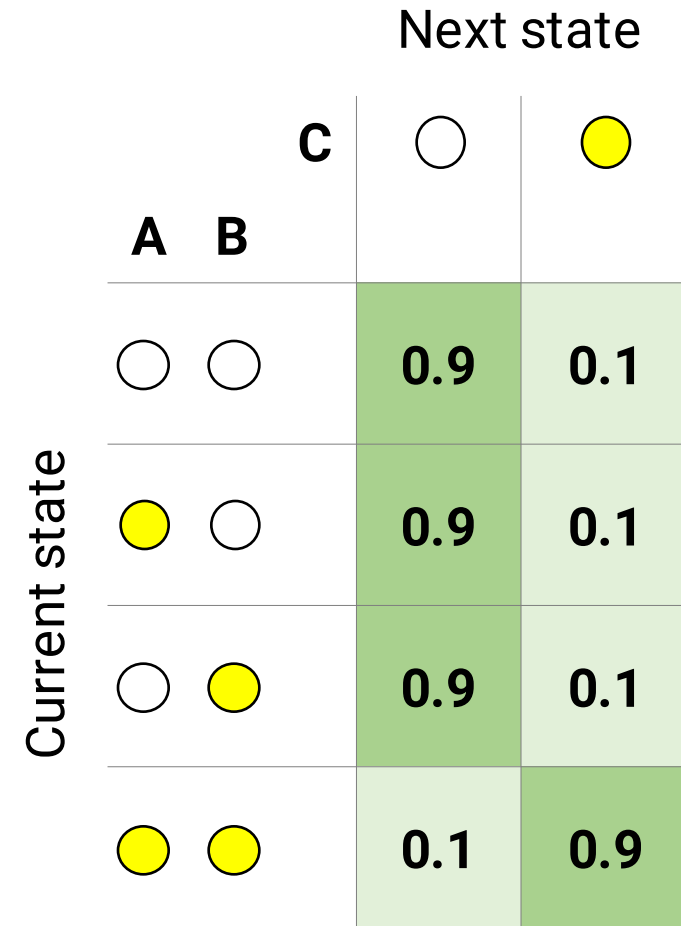 | 0.1                                                                                  | 0.9                                                                                 |                                                                                     |

# An example network

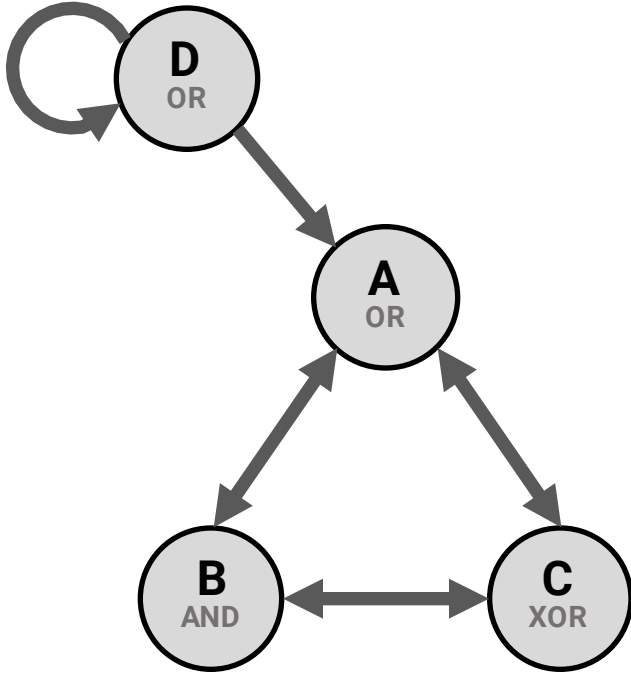

Network with 4 binary elements  
( $2^4 = 16$  possible states)

- Now let's consider a larger network of interconnected elements
- Just as with a single element, we can determine the TPM of the network as a whole
- Again, to do so we perturb the system into each of its possible states and record the results

# An example network

$t$

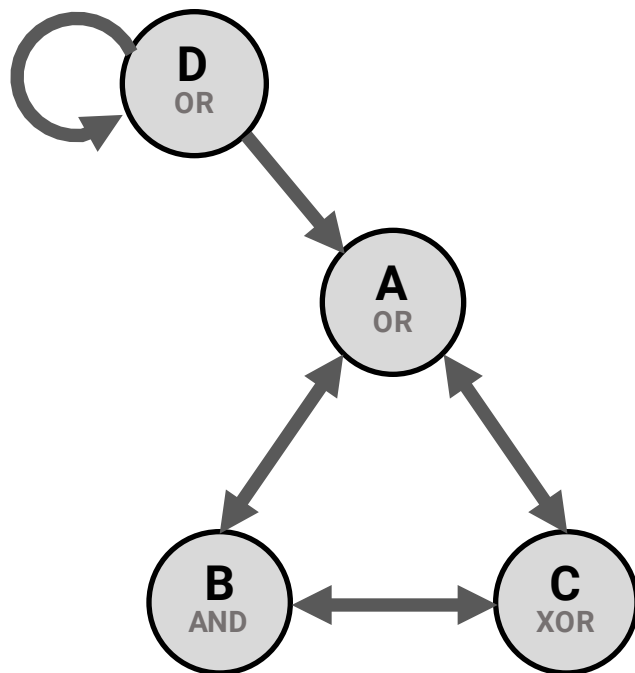

# An example network

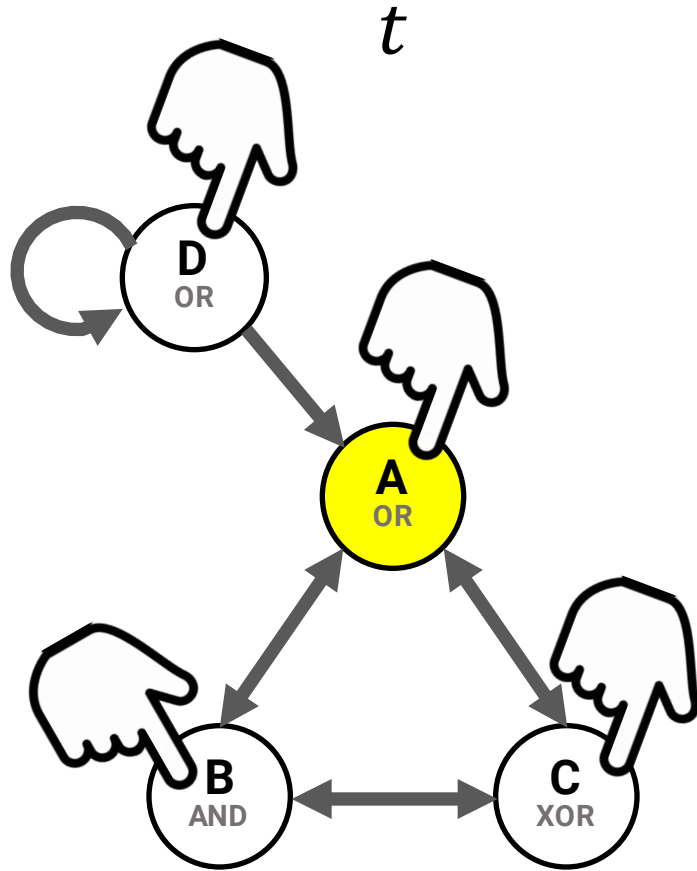

Example perturbation

# An example network

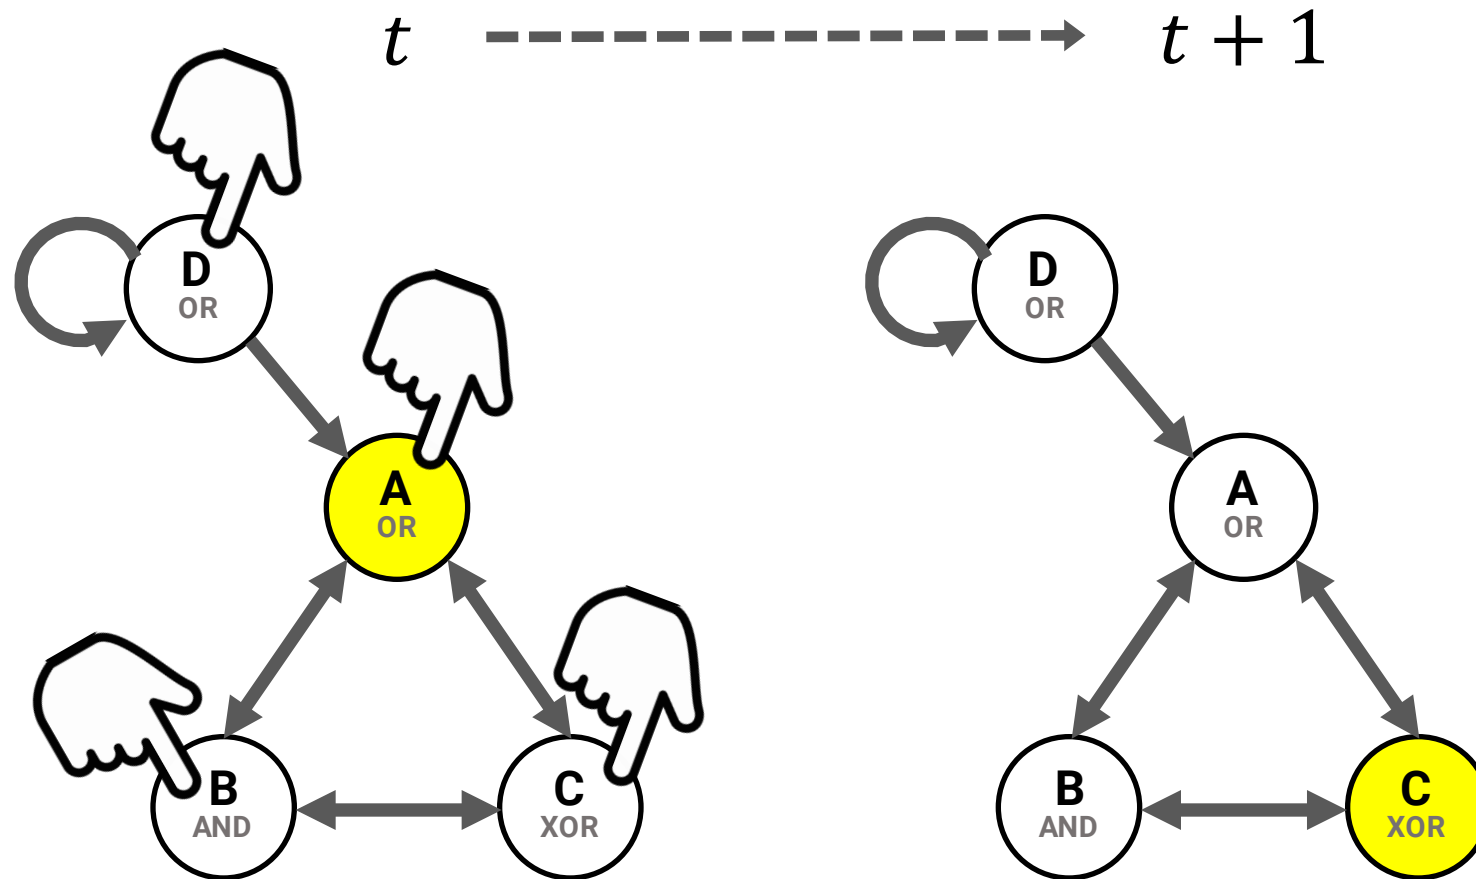

Example perturbation

Result of perturbation

# An example network

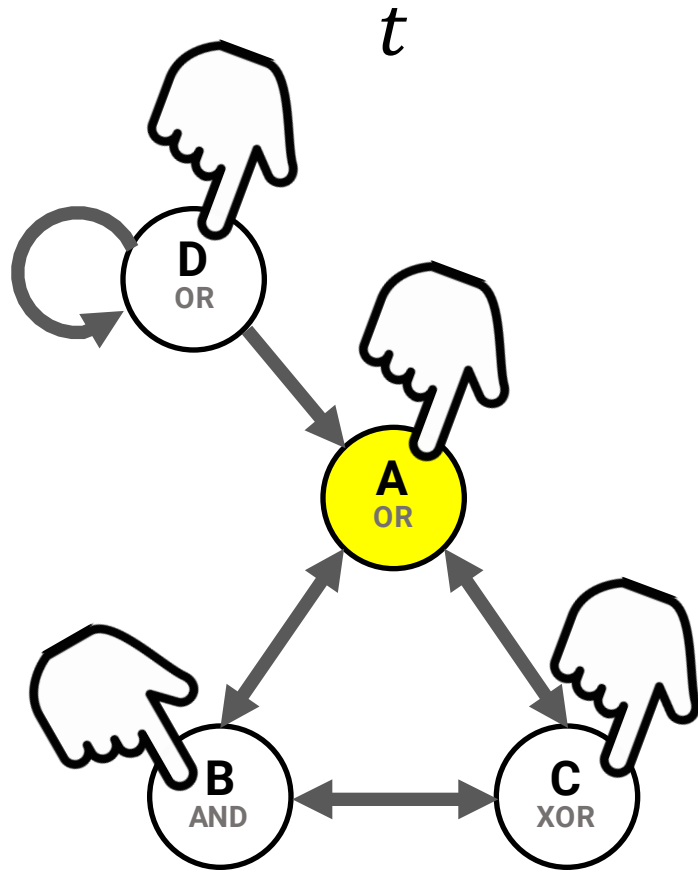

Perturbation

- Note that in this example, we're assuming that the structure of the network is as shown
- In general, we don't know the underlying structure
- Perturbation and observation is what allows the experimenter to determine the TPM

# An example network

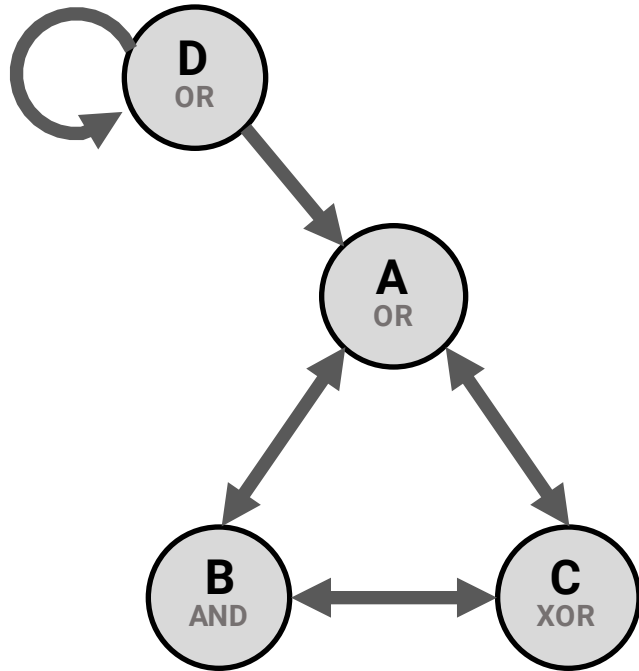

Network with 4 binary elements  
 $(2^4 = 16 \text{ possible states})$

|               |   |   |   | Next state |   |   |   |   |   |   |   |   |   |   |   |   |   |   |   |
|---------------|---|---|---|------------|---|---|---|---|---|---|---|---|---|---|---|---|---|---|---|
|               |   |   |   | A          | B | C | D |   |   |   |   |   |   |   |   |   |   |   |   |
| Current state | A | B | C | D          |   |   |   |   |   |   |   |   |   |   |   |   |   |   |   |
|               | ○ | ○ | ○ | ○          | 1 | 0 | 0 | 0 | 0 | 0 | 0 | 0 | 0 | 0 | 0 | 0 | 0 | 0 | 0 |
|               | ● | ○ | ○ | ○          | 0 | 0 | 0 | 0 | 1 | 0 | 0 | 0 | 0 | 0 | 0 | 0 | 0 | 0 | 0 |
|               | ○ | ● | ○ | ○          | 0 | 0 | 0 | 0 | 0 | 1 | 0 | 0 | 0 | 0 | 0 | 0 | 0 | 0 | 0 |
|               | ● | ● | ○ | ○          | 0 | 1 | 0 | 0 | 0 | 0 | 0 | 0 | 0 | 0 | 0 | 0 | 0 | 0 | 0 |
|               | ○ | ○ | ● | ○          | 0 | 1 | 0 | 0 | 0 | 0 | 0 | 0 | 0 | 0 | 0 | 0 | 0 | 0 | 0 |
|               | ● | ○ | ● | ○          | 0 | 0 | 0 | 0 | 0 | 0 | 0 | 1 | 0 | 0 | 0 | 0 | 0 | 0 | 0 |
|               | ○ | ● | ● | ○          | 0 | 0 | 0 | 0 | 0 | 1 | 0 | 0 | 0 | 0 | 0 | 0 | 0 | 0 | 0 |
|               | ● | ● | ● | ○          | 0 | 0 | 0 | 1 | 0 | 0 | 0 | 0 | 0 | 0 | 0 | 0 | 0 | 0 | 0 |
|               | ○ | ○ | ○ | ●          | 0 | 0 | 0 | 0 | 0 | 0 | 0 | 0 | 0 | 1 | 0 | 0 | 0 | 0 | 0 |
|               | ● | ○ | ○ | ●          | 0 | 0 | 0 | 0 | 0 | 0 | 0 | 0 | 0 | 0 | 0 | 0 | 1 | 0 | 0 |
|               | ○ | ● | ○ | ●          | 0 | 0 | 0 | 0 | 0 | 0 | 0 | 0 | 0 | 0 | 0 | 0 | 1 | 0 | 0 |
|               | ● | ● | ○ | ●          | 0 | 0 | 0 | 0 | 0 | 0 | 0 | 0 | 0 | 1 | 0 | 0 | 0 | 0 | 0 |
|               | ○ | ○ | ● | ●          | 0 | 0 | 0 | 0 | 0 | 0 | 0 | 0 | 0 | 1 | 0 | 0 | 0 | 0 | 0 |
|               | ● | ○ | ● | ●          | 0 | 0 | 0 | 0 | 0 | 0 | 0 | 0 | 0 | 0 | 0 | 0 | 0 | 1 | 0 |
|               | ○ | ● | ● | ●          | 0 | 0 | 0 | 0 | 0 | 0 | 0 | 0 | 0 | 0 | 0 | 1 | 0 | 0 | 0 |
|               | ● | ● | ● | ●          | 0 | 0 | 0 | 0 | 0 | 0 | 0 | 0 | 0 | 0 | 1 | 0 | 0 | 0 | 0 |

Corresponding TPM  $(16 \times 16)$

Deterministic network  $\Leftrightarrow$  single column with  
 1.0 probability in each row

# Outline

- Elements, states, and the TPM
- **Background conditions**
- Cause-effect repertoires
- Integrated mechanisms:  $\varphi$
- Concepts and cause-effect structures
- Integrated systems:  $\Phi$
- Complexes



# Candidate systems and background conditions

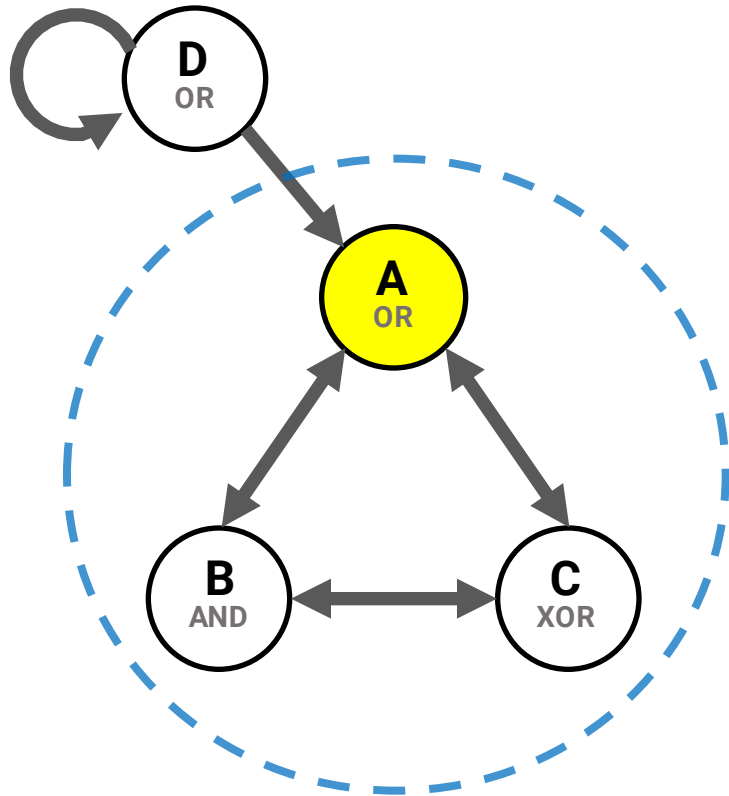

Candidate system **ABC**

- Given a network in some state at some moment in time, we want to evaluate the integrated information of a subset of its elements, called a **candidate system**

# Candidate systems and background conditions

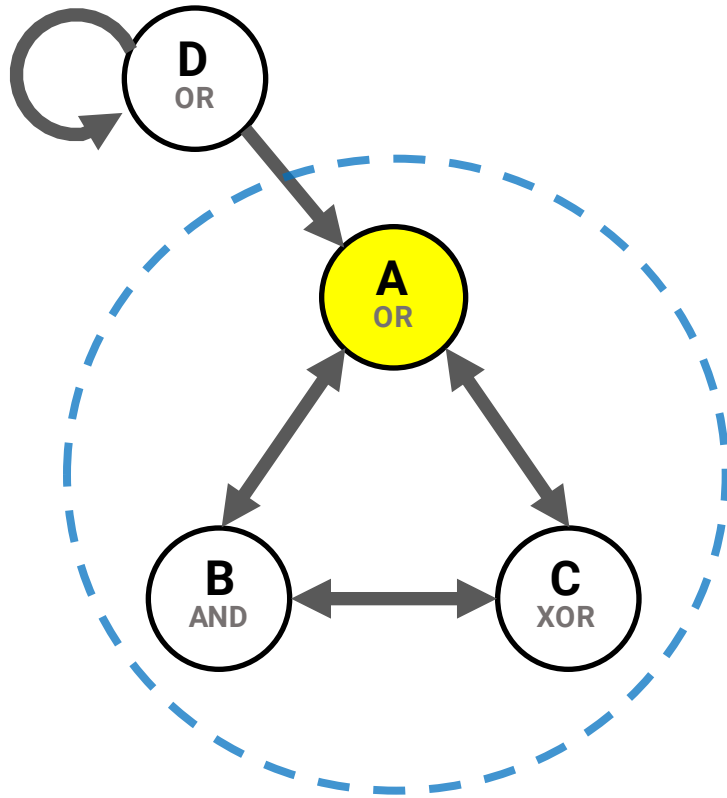

Candidate system **ABC**

- In order to do so, we use the TPM of those elements
- Since the aim is to assess the integrated information of the candidate system *when the network is in a particular state*, we want to determine the TPM of the candidate system by perturbing it while the external elements are **fixed** in that state

# Candidate systems and background conditions

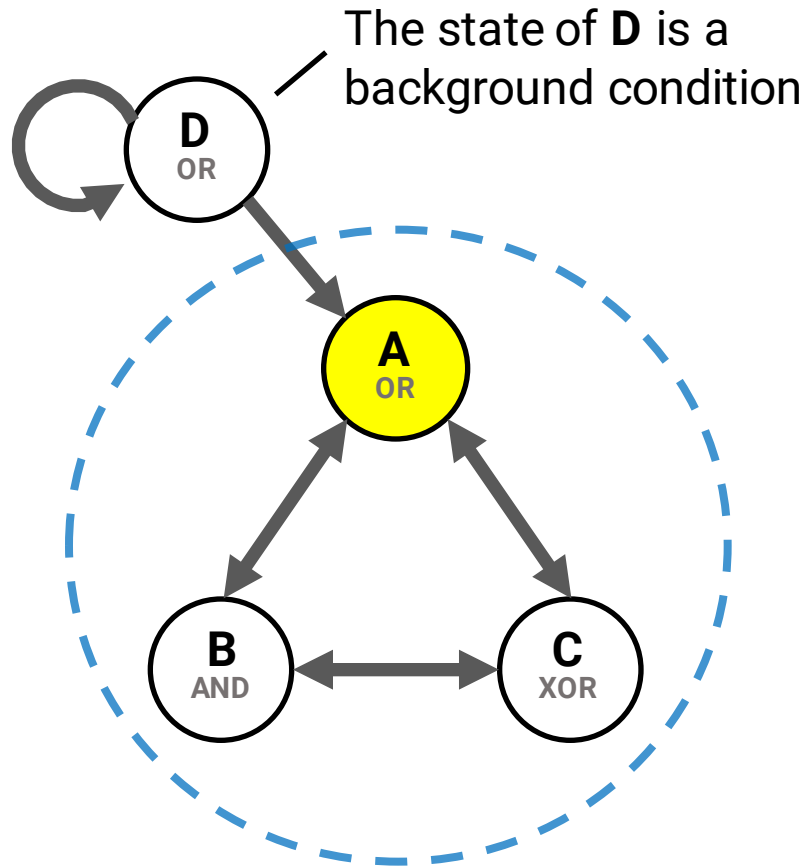

Candidate system **ABC**

- These fixed external elements constitute the **background conditions** for the candidate system
- Calculating the TPM of the candidate system **given** background conditions is a process called **conditioning** on the background conditions

# Fixing background conditions

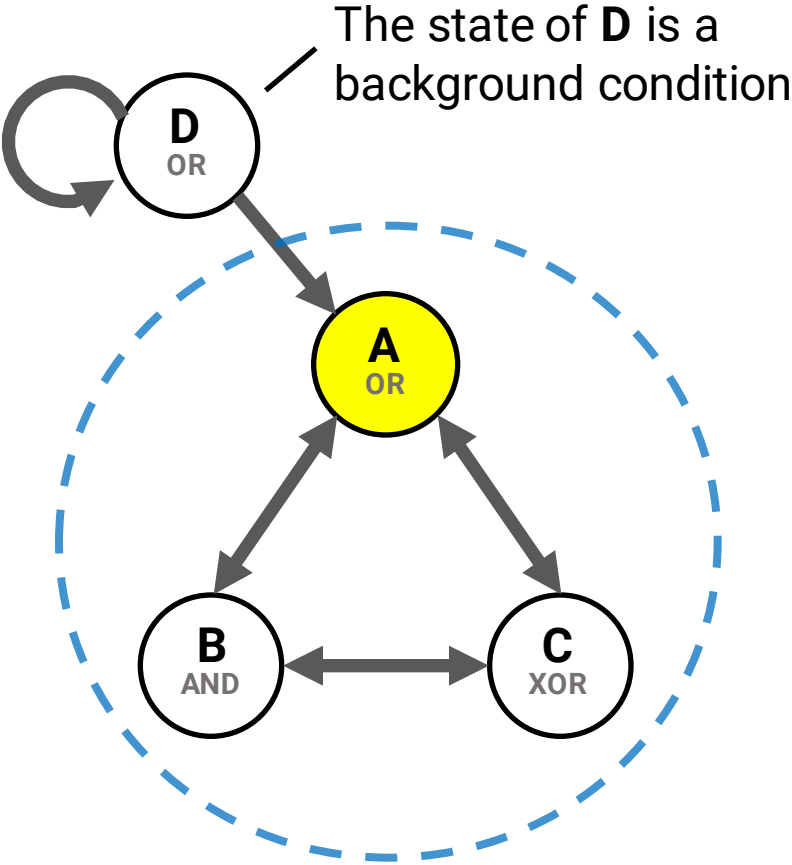

Candidate system **ABC**

|               |   |   |   | Next state |   |   |   |   |   |   |   |   |   |   |   |   |   |   |   |
|---------------|---|---|---|------------|---|---|---|---|---|---|---|---|---|---|---|---|---|---|---|
|               |   |   |   | A          | B | C | D |   |   |   |   |   |   |   |   |   |   |   |   |
| Current state | A | B | C | D          | 1 | 0 | 0 | 0 | 0 | 0 | 0 | 0 | 0 | 0 | 0 | 0 | 0 | 0 | 0 |
|               | 1 | 0 | 0 | 0          | 0 | 0 | 0 | 1 | 0 | 0 | 0 | 0 | 0 | 0 | 0 | 0 | 0 | 0 | 0 |
|               | 0 | 1 | 0 | 0          | 0 | 0 | 0 | 0 | 1 | 0 | 0 | 0 | 0 | 0 | 0 | 0 | 0 | 0 | 0 |
|               | 1 | 1 | 0 | 0          | 0 | 1 | 0 | 0 | 0 | 0 | 0 | 0 | 0 | 0 | 0 | 0 | 0 | 0 | 0 |
|               | 0 | 0 | 1 | 0          | 0 | 1 | 0 | 0 | 0 | 0 | 0 | 0 | 0 | 0 | 0 | 0 | 0 | 0 | 0 |
|               | 1 | 0 | 1 | 0          | 0 | 0 | 0 | 0 | 0 | 1 | 0 | 0 | 0 | 0 | 0 | 0 | 0 | 0 | 0 |
|               | 0 | 1 | 1 | 0          | 0 | 0 | 0 | 1 | 0 | 0 | 0 | 0 | 0 | 0 | 0 | 0 | 0 | 0 | 0 |
|               | 1 | 1 | 1 | 0          | 0 | 0 | 1 | 0 | 0 | 0 | 0 | 0 | 0 | 0 | 0 | 0 | 0 | 0 | 0 |
|               | 0 | 0 | 0 | 1          | 0 | 0 | 0 | 0 | 0 | 0 | 0 | 0 | 1 | 0 | 0 | 0 | 0 | 0 | 0 |
|               | 1 | 0 | 0 | 1          | 0 | 0 | 0 | 0 | 0 | 0 | 0 | 0 | 0 | 0 | 0 | 1 | 0 | 0 | 0 |
|               | 0 | 1 | 0 | 1          | 0 | 0 | 0 | 0 | 0 | 0 | 0 | 0 | 0 | 0 | 0 | 1 | 0 | 0 | 0 |
|               | 1 | 1 | 0 | 1          | 0 | 0 | 0 | 0 | 0 | 0 | 0 | 0 | 1 | 0 | 0 | 0 | 0 | 0 | 0 |
|               | 0 | 0 | 1 | 1          | 0 | 0 | 0 | 0 | 0 | 0 | 0 | 0 | 1 | 0 | 0 | 0 | 0 | 0 | 0 |
|               | 1 | 0 | 1 | 1          | 0 | 0 | 0 | 0 | 0 | 0 | 0 | 0 | 0 | 0 | 0 | 0 | 0 | 1 | 0 |
|               | 0 | 1 | 1 | 1          | 0 | 0 | 0 | 0 | 0 | 0 | 0 | 0 | 0 | 0 | 0 | 1 | 0 | 0 | 0 |
|               | 1 | 1 | 1 | 1          | 0 | 0 | 0 | 0 | 0 | 0 | 0 | 0 | 0 | 1 | 0 | 0 | 0 | 0 | 0 |

Network TPM

# Fixing background conditions

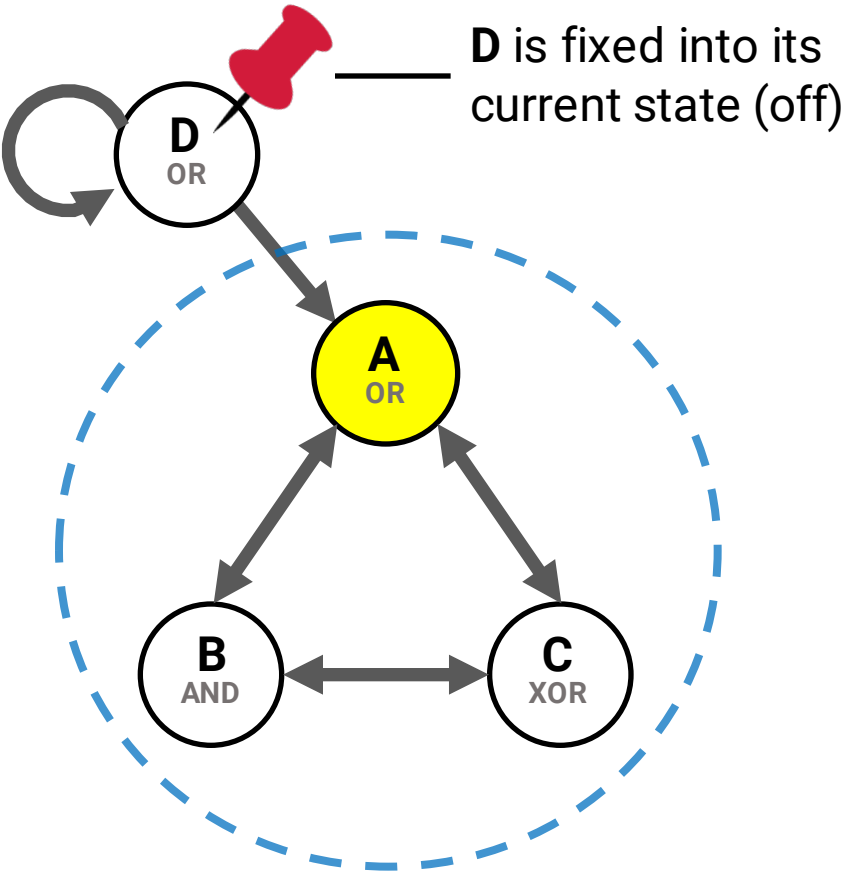

We **fix** the elements outside the candidate system

|               |   |   |   | Next state |   |   |   |   |   |   |   |   |   |   |   |   |   |   |   |
|---------------|---|---|---|------------|---|---|---|---|---|---|---|---|---|---|---|---|---|---|---|
|               |   |   |   | A          | B | C | D | 0 | 1 | 0 | 1 | 0 | 1 | 0 | 1 | 0 | 1 | 0 | 1 |
| Current state | A | B | C | D          | 0 | 1 | 0 | 1 | 0 | 1 | 0 | 1 | 0 | 1 | 0 | 1 | 0 | 1 | 0 |
|               | 0 | 0 | 0 | 0          | 1 | 0 | 0 | 0 | 0 | 0 | 0 | 0 | 0 | 0 | 0 | 0 | 0 | 0 | 0 |
|               | 1 | 0 | 0 | 0          | 0 | 0 | 0 | 0 | 1 | 0 | 0 | 0 | 0 | 0 | 0 | 0 | 0 | 0 | 0 |
|               | 0 | 1 | 0 | 0          | 0 | 0 | 0 | 0 | 1 | 0 | 0 | 0 | 0 | 0 | 0 | 0 | 0 | 0 | 0 |
|               | 1 | 1 | 0 | 0          | 0 | 1 | 0 | 0 | 0 | 0 | 0 | 0 | 0 | 0 | 0 | 0 | 0 | 0 | 0 |
|               | 0 | 0 | 1 | 0          | 0 | 1 | 0 | 0 | 0 | 0 | 0 | 0 | 0 | 0 | 0 | 0 | 0 | 0 | 0 |
|               | 1 | 0 | 1 | 0          | 0 | 0 | 0 | 0 | 0 | 1 | 0 | 0 | 0 | 0 | 0 | 0 | 0 | 0 | 0 |
|               | 0 | 1 | 1 | 0          | 0 | 0 | 0 | 0 | 1 | 0 | 0 | 0 | 0 | 0 | 0 | 0 | 0 | 0 | 0 |
|               | 1 | 1 | 1 | 0          | 0 | 0 | 1 | 0 | 0 | 0 | 0 | 0 | 0 | 0 | 0 | 0 | 0 | 0 | 0 |
|               | 0 | 0 | 0 | 1          | 0 | 0 | 0 | 0 | 0 | 0 | 0 | 0 | 1 | 0 | 0 | 0 | 0 | 0 | 0 |
|               | 1 | 0 | 0 | 1          | 0 | 0 | 0 | 0 | 0 | 0 | 0 | 0 | 0 | 0 | 0 | 1 | 0 | 0 | 0 |
|               | 0 | 1 | 0 | 1          | 0 | 0 | 0 | 0 | 0 | 0 | 0 | 0 | 0 | 0 | 0 | 0 | 1 | 0 | 0 |
|               | 1 | 1 | 0 | 1          | 0 | 0 | 0 | 0 | 0 | 0 | 0 | 0 | 0 | 0 | 0 | 0 | 0 | 1 | 0 |
|               | 0 | 0 | 1 | 1          | 0 | 0 | 0 | 0 | 0 | 0 | 0 | 0 | 0 | 0 | 0 | 0 | 0 | 0 | 1 |
|               | 1 | 0 | 1 | 1          | 0 | 0 | 0 | 0 | 0 | 0 | 0 | 0 | 0 | 0 | 0 | 0 | 0 | 0 | 0 |
|               | 0 | 1 | 1 | 1          | 0 | 0 | 0 | 0 | 0 | 0 | 0 | 0 | 0 | 0 | 0 | 0 | 0 | 0 | 0 |

This corresponds to **conditioning** the TPM on the current state of **D** (off)

# Fixing background conditions

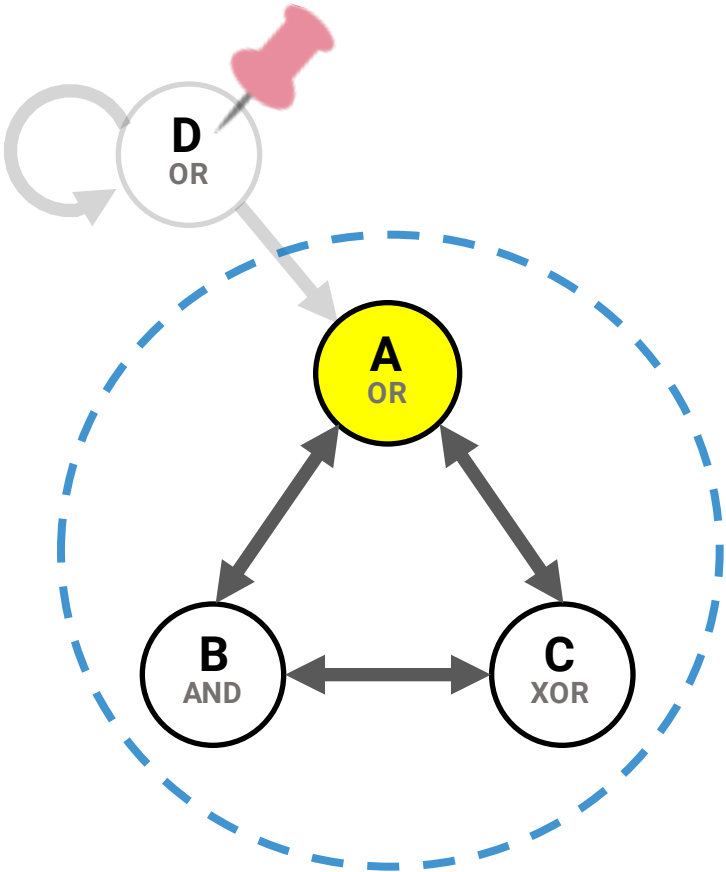

We **fix** the elements outside the candidate system

|               |   |   |   | Next state |   |   |   |   |   |   |   |   |   |   |   |   |   |   |   |
|---------------|---|---|---|------------|---|---|---|---|---|---|---|---|---|---|---|---|---|---|---|
|               |   |   |   | A          | B | C | D | 0 | 1 | 0 | 1 | 0 | 1 | 0 | 1 | 0 | 1 | 0 | 1 |
|               |   |   |   | A          | B | C | D | 0 | 1 | 0 | 1 | 0 | 1 | 0 | 1 | 0 | 1 | 0 | 1 |
| Current state | 0 | 0 | 0 | 0          | 0 | 0 | 0 | 1 | 0 | 0 | 0 | 0 | 0 | 0 | 0 | 0 | 0 | 0 | 0 |
|               | 1 | 0 | 0 | 0          | 0 | 0 | 0 | 0 | 0 | 0 | 0 | 1 | 0 | 0 | 0 | 0 | 0 | 0 | 0 |
|               | 0 | 1 | 0 | 0          | 0 | 0 | 0 | 0 | 0 | 0 | 0 | 0 | 1 | 0 | 0 | 0 | 0 | 0 | 0 |
|               | 1 | 1 | 0 | 0          | 0 | 0 | 0 | 0 | 1 | 0 | 0 | 0 | 0 | 0 | 0 | 0 | 0 | 0 | 0 |
|               | 0 | 0 | 1 | 0          | 0 | 0 | 0 | 0 | 1 | 0 | 0 | 0 | 0 | 0 | 0 | 0 | 0 | 0 | 0 |
|               | 1 | 0 | 1 | 0          | 0 | 0 | 0 | 0 | 0 | 0 | 0 | 0 | 1 | 0 | 0 | 0 | 0 | 0 | 0 |
|               | 0 | 1 | 1 | 0          | 0 | 0 | 0 | 0 | 0 | 0 | 0 | 1 | 0 | 0 | 0 | 0 | 0 | 0 | 0 |
|               | 1 | 1 | 1 | 0          | 0 | 0 | 0 | 0 | 0 | 0 | 1 | 0 | 0 | 0 | 0 | 0 | 0 | 0 | 0 |
|               | 0 | 0 | 0 | 1          | 0 | 0 | 0 | 0 | 0 | 0 | 0 | 0 | 0 | 0 | 0 | 0 | 0 | 0 | 0 |
|               | 1 | 0 | 0 | 1          | 0 | 0 | 0 | 0 | 0 | 0 | 0 | 0 | 0 | 0 | 0 | 0 | 0 | 0 | 0 |
|               | 0 | 1 | 0 | 1          | 0 | 0 | 0 | 0 | 0 | 0 | 0 | 0 | 0 | 0 | 0 | 0 | 0 | 0 | 0 |
|               | 1 | 1 | 0 | 1          | 0 | 0 | 0 | 0 | 0 | 0 | 0 | 0 | 0 | 0 | 0 | 0 | 0 | 0 | 0 |
|               | 0 | 0 | 1 | 1          | 0 | 0 | 0 | 0 | 0 | 0 | 0 | 0 | 0 | 0 | 0 | 0 | 0 | 0 | 0 |
|               | 1 | 0 | 1 | 1          | 0 | 0 | 0 | 0 | 0 | 0 | 0 | 0 | 0 | 0 | 0 | 0 | 0 | 0 | 0 |
|               | 0 | 1 | 1 | 1          | 0 | 0 | 0 | 0 | 0 | 0 | 0 | 0 | 0 | 0 | 0 | 0 | 0 | 0 | 0 |
|               | 1 | 1 | 1 | 1          | 0 | 0 | 0 | 0 | 0 | 0 | 0 | 0 | 0 | 0 | 0 | 0 | 0 | 0 | 0 |

This corresponds to **conditioning** the TPM on the current state of **D** (off)

# Fixing background conditions

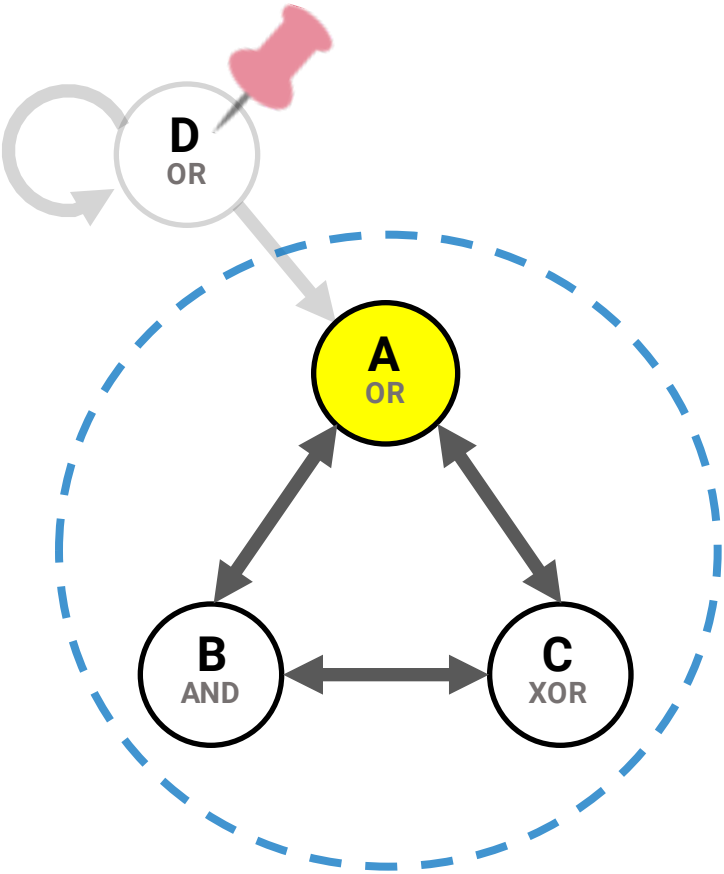

|               |  |  |  | Next state |   |   |   |  |  |  |  |  |  |  |  |  |  |  |  |
|---------------|--|--|--|------------|---|---|---|--|--|--|--|--|--|--|--|--|--|--|--|
|               |  |  |  | A          | B | C | D |  |  |  |  |  |  |  |  |  |  |  |  |
|               |  |  |  | A          | B | C | D |  |  |  |  |  |  |  |  |  |  |  |  |
| Current state |  |  |  |            |   |   |   |  |  |  |  |  |  |  |  |  |  |  |  |
|               |  |  |  |            |   |   |   |  |  |  |  |  |  |  |  |  |  |  |  |
|               |  |  |  |            |   |   |   |  |  |  |  |  |  |  |  |  |  |  |  |
|               |  |  |  |            |   |   |   |  |  |  |  |  |  |  |  |  |  |  |  |
|               |  |  |  |            |   |   |   |  |  |  |  |  |  |  |  |  |  |  |  |
|               |  |  |  |            |   |   |   |  |  |  |  |  |  |  |  |  |  |  |  |
|               |  |  |  |            |   |   |   |  |  |  |  |  |  |  |  |  |  |  |  |
|               |  |  |  |            |   |   |   |  |  |  |  |  |  |  |  |  |  |  |  |
|               |  |  |  |            |   |   |   |  |  |  |  |  |  |  |  |  |  |  |  |
|               |  |  |  |            |   |   |   |  |  |  |  |  |  |  |  |  |  |  |  |
|               |  |  |  |            |   |   |   |  |  |  |  |  |  |  |  |  |  |  |  |
|               |  |  |  |            |   |   |   |  |  |  |  |  |  |  |  |  |  |  |  |
|               |  |  |  |            |   |   |   |  |  |  |  |  |  |  |  |  |  |  |  |
|               |  |  |  |            |   |   |   |  |  |  |  |  |  |  |  |  |  |  |  |
|               |  |  |  |            |   |   |   |  |  |  |  |  |  |  |  |  |  |  |  |
|               |  |  |  |            |   |   |   |  |  |  |  |  |  |  |  |  |  |  |  |

To condition the TPM, we simply take the part of it that corresponds to the current state of **D** being off

# Fixing background conditions

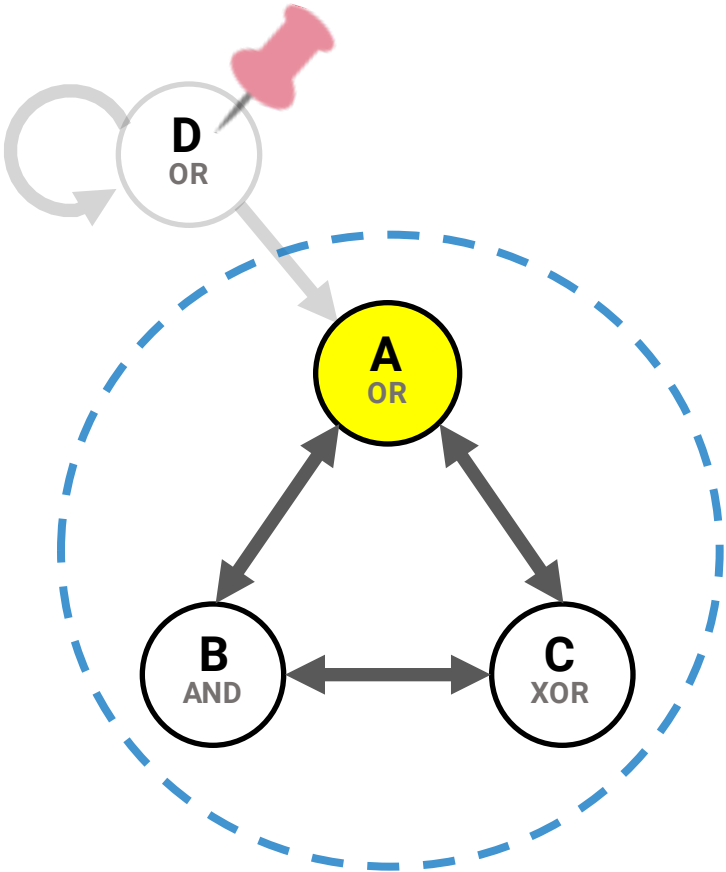

|               |   |   |   | Next state |   |   |   |   |   |   |   |   |   |   |   |   |   |   |   |
|---------------|---|---|---|------------|---|---|---|---|---|---|---|---|---|---|---|---|---|---|---|
|               |   |   |   | A          |   |   |   |   |   |   |   |   |   |   |   |   |   |   |   |
|               |   |   |   | B          |   |   |   |   |   |   |   |   |   |   |   |   |   |   |   |
|               |   |   |   | C          |   |   |   |   |   |   |   |   |   |   |   |   |   |   |   |
|               |   |   |   | D          |   |   |   |   |   |   |   |   |   |   |   |   |   |   |   |
| Current state | A | B | C | D          |   |   |   |   |   |   |   |   |   |   |   |   |   |   |   |
|               | ○ | ○ | ○ | ○          | 1 | 0 | 0 | 0 | 0 | 0 | 0 | 0 | 0 | 0 | 0 | 0 | 0 | 0 | 0 |
|               | ● | ○ | ○ | ○          | 0 | 0 | 0 | 0 | 1 | 0 | 0 | 0 | 0 | 0 | 0 | 0 | 0 | 0 | 0 |
|               | ○ | ● | ○ | ○          | 0 | 0 | 0 | 0 | 0 | 1 | 0 | 0 | 0 | 0 | 0 | 0 | 0 | 0 | 0 |
|               | ● | ● | ○ | ○          | 0 | 1 | 0 | 0 | 0 | 0 | 0 | 0 | 0 | 0 | 0 | 0 | 0 | 0 | 0 |
|               | ○ | ○ | ● | ○          | 0 | 1 | 0 | 0 | 0 | 0 | 0 | 0 | 0 | 0 | 0 | 0 | 0 | 0 | 0 |
|               | ● | ○ | ● | ○          | 0 | 0 | 0 | 0 | 0 | 0 | 0 | 1 | 0 | 0 | 0 | 0 | 0 | 0 | 0 |
|               | ○ | ● | ● | ○          | 0 | 0 | 0 | 0 | 0 | 1 | 0 | 0 | 0 | 0 | 0 | 0 | 0 | 0 | 0 |
|               | ● | ● | ● | ○          | 0 | 0 | 0 | 1 | 0 | 0 | 0 | 0 | 0 | 0 | 0 | 0 | 0 | 0 | 0 |

To condition the TPM, we simply take the part of it that corresponds to the current state of **D** being off



# Fixing background conditions

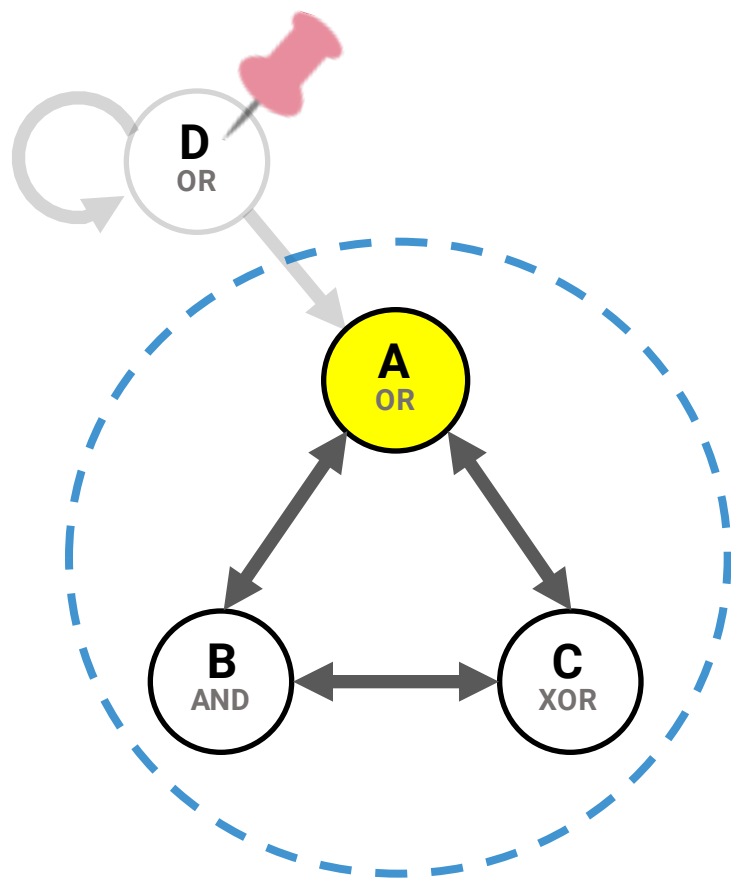

|               |   |   |   | Next state |   |   |   |   |   |   |   |   |   |   |   |   |   |   |   |
|---------------|---|---|---|------------|---|---|---|---|---|---|---|---|---|---|---|---|---|---|---|
|               |   |   |   | A          | B | C | D |   |   |   |   |   |   |   |   |   |   |   |   |
| Current state | A | B | C | D          |   |   |   |   |   |   |   |   |   |   |   |   |   |   |   |
|               | ○ | ○ | ○ | ○          | 1 | 0 | 0 | 0 | 0 | 0 | 0 | 0 | 0 | 0 | 0 | 0 | 0 | 0 | 0 |
|               | ● | ○ | ○ | ○          | 0 | 0 | 0 | 0 | 1 | 0 | 0 | 0 | 0 | 0 | 0 | 0 | 0 | 0 | 0 |
|               | ○ | ● | ○ | ○          | 0 | 0 | 0 | 0 | 0 | 1 | 0 | 0 | 0 | 0 | 0 | 0 | 0 | 0 | 0 |
|               | ● | ● | ○ | ○          | 0 | 1 | 0 | 0 | 0 | 0 | 0 | 0 | 0 | 0 | 0 | 0 | 0 | 0 | 0 |
|               | ○ | ○ | ● | ○          | 0 | 1 | 0 | 0 | 0 | 0 | 0 | 0 | 0 | 0 | 0 | 0 | 0 | 0 | 0 |
|               | ● | ○ | ● | ○          | 0 | 0 | 0 | 0 | 0 | 0 | 1 | 0 | 0 | 0 | 0 | 0 | 0 | 0 | 0 |
|               | ○ | ● | ● | ○          | 0 | 0 | 0 | 0 | 0 | 1 | 0 | 0 | 0 | 0 | 0 | 0 | 0 | 0 | 0 |
|               | ● | ● | ● | ○          | 0 | 0 | 0 | 1 | 0 | 0 | 0 | 0 | 0 | 0 | 0 | 0 | 0 | 0 | 0 |

- However, the states at  $t + 1$  still include **D**, but we're only interested in the probabilities of the states of the candidate system, **ABC**
- We would like to **ignore** the future state of **D**
- This is accomplished by **marginalization**
- We **marginalize-out** element **D** by taking the sum of the probabilities of states that differ only by **D**'s state

Fixing background conditions:  
**Marginalization**

- Note that the first and ninth columns differ only by **D**'s state

|              |              |              |              |              |              |              |              |              |              |              |              |              |              |              |              |              |              |              |
|--------------|--------------|--------------|--------------|--------------|--------------|--------------|--------------|--------------|--------------|--------------|--------------|--------------|--------------|--------------|--------------|--------------|--------------|--------------|
| A            | <div>○</div> | <div>●</div> | <div>○</div> | <div>●</div> | <div>○</div> | <div>●</div> | <div>○</div> | <div>●</div> | <div>○</div> | <div>●</div> | <div>○</div> | <div>●</div> | <div>○</div> | <div>●</div> | <div>○</div> | <div>●</div> | <div>○</div> | <div>●</div> |
| B            | <div>○</div> | <div>○</div> | <div>●</div> | <div>●</div> | <div>○</div> | <div>○</div> | <div>●</div> | <div>●</div> | <div>○</div> | <div>○</div> | <div>●</div> | <div>●</div> | <div>○</div> | <div>○</div> | <div>●</div> | <div>●</div> | <div>○</div> | <div>●</div> |
| C            | <div>○</div> | <div>○</div> | <div>○</div> | <div>○</div> | <div>●</div> | <div>●</div> | <div>●</div> | <div>●</div> | <div>○</div> | <div>○</div> | <div>○</div> | <div>○</div> | <div>●</div> | <div>●</div> | <div>●</div> | <div>●</div> | <div>○</div> | <div>●</div> |
| D            | <div>○</div> | <div>○</div> | <div>○</div> | <div>○</div> | <div>○</div> | <div>○</div> | <div>○</div> | <div>○</div> | <div>○</div> | <div>○</div> | <div>○</div> | <div>○</div> | <div>○</div> | <div>○</div> | <div>○</div> | <div>○</div> | <div>○</div> | <div>○</div> |
| A            | B            | C            |              |              |              |              |              |              |              |              |              |              |              |              |              |              |              |              |
| <div>○</div> | <div>○</div> | <div>○</div> | 1            | 0            | 0            | 0            | 0            | 0            | 0            | 0            | 0            | 0            | 0            | 0            | 0            | 0            | 0            | 0            |
| <div>●</div> | <div>○</div> | <div>○</div> | 0            | 0            | 0            | 0            | 1            | 0            | 0            | 0            | 0            | 0            | 0            | 0            | 0            | 0            | 0            | 0            |
| <div>○</div> | <div>●</div> | <div>○</div> | 0            | 0            | 0            | 0            | 0            | 1            | 0            | 0            | 0            | 0            | 0            | 0            | 0            | 0            | 0            | 0            |
| <div>●</div> | <div>●</div> | <div>○</div> | 0            | 1            | 0            | 0            | 0            | 0            | 0            | 0            | 0            | 0            | 0            | 0            | 0            | 0            | 0            | 0            |
| <div>○</div> | <div>○</div> | <div>●</div> | 0            | 1            | 0            | 0            | 0            | 0            | 0            | 0            | 0            | 0            | 0            | 0            | 0            | 0            | 0            | 0            |
| <div>●</div> | <div>○</div> | <div>●</div> | 0            | 0            | 0            | 0            | 0            | 0            | 0            | 1            | 0            | 0            | 0            | 0            | 0            | 0            | 0            | 0            |
| <div>○</div> | <div>●</div> | <div>●</div> | 0            | 0            | 0            | 0            | 0            | 1            | 0            | 0            | 0            | 0            | 0            | 0            | 0            | 0            | 0            | 0            |
| <div>●</div> | <div>●</div> | <div>●</div> | 0            | 0            | 0            | 1            | 0            | 0            | 0            | 0            | 0            | 0            | 0            | 0            | 0            | 0            | 0            | 0            |

|              |              |              |   |              |
|--------------|--------------|--------------|---|--------------|
|              |              |              | A | <div>○</div> |
|              |              |              | B | <div>○</div> |
|              |              |              | C | <div>○</div> |
| A            | B            | C            |   |              |
| <div>○</div> | <div>○</div> | <div>○</div> |   |              |
| <div>●</div> | <div>○</div> | <div>○</div> |   |              |
| <div>○</div> | <div>●</div> | <div>○</div> |   |              |
| <div>●</div> | <div>●</div> | <div>○</div> |   |              |
| <div>○</div> | <div>○</div> | <div>●</div> |   |              |
| <div>●</div> | <div>○</div> | <div>●</div> |   |              |
| <div>○</div> | <div>●</div> | <div>●</div> |   |              |
| <div>●</div> | <div>●</div> | <div>●</div> |   |              |

Fixing background conditions:

## Marginalization

- Note that the first and ninth columns differ only by **D**'s state
- We sum those columns together to get the probabilities of transitioning to state **ABC** = (0, 0, 0), **ignoring the state of D**, from each previous state

|                                  |                                  |                                  |                                  |                                  |                                  |                                  |                                  |                                  |                                  |                                  |                                  |                                  |                                  |                                  |                                  |                                  |                                  |                                  |                                  |
|----------------------------------|----------------------------------|----------------------------------|----------------------------------|----------------------------------|----------------------------------|----------------------------------|----------------------------------|----------------------------------|----------------------------------|----------------------------------|----------------------------------|----------------------------------|----------------------------------|----------------------------------|----------------------------------|----------------------------------|----------------------------------|----------------------------------|----------------------------------|
|                                  | A                                | <input type="radio"/>            | <input checked="" type="radio"/> | <input type="radio"/>            | <input checked="" type="radio"/> | <input type="radio"/>            | <input checked="" type="radio"/> | <input type="radio"/>            | <input checked="" type="radio"/> | <input type="radio"/>            | <input checked="" type="radio"/> | <input type="radio"/>            | <input checked="" type="radio"/> | <input type="radio"/>            | <input checked="" type="radio"/> | <input type="radio"/>            | <input checked="" type="radio"/> | <input type="radio"/>            | <input checked="" type="radio"/> |
|                                  | B                                | <input type="radio"/>            | <input type="radio"/>            | <input checked="" type="radio"/> | <input checked="" type="radio"/> | <input type="radio"/>            | <input type="radio"/>            | <input checked="" type="radio"/> | <input checked="" type="radio"/> | <input type="radio"/>            | <input type="radio"/>            | <input checked="" type="radio"/> | <input checked="" type="radio"/> | <input type="radio"/>            | <input type="radio"/>            | <input checked="" type="radio"/> | <input checked="" type="radio"/> | <input type="radio"/>            | <input checked="" type="radio"/> |
|                                  | C                                | <input type="radio"/>            | <input type="radio"/>            | <input type="radio"/>            | <input type="radio"/>            | <input checked="" type="radio"/> | <input checked="" type="radio"/> | <input checked="" type="radio"/> | <input checked="" type="radio"/> | <input type="radio"/>            | <input type="radio"/>            | <input type="radio"/>            | <input type="radio"/>            | <input checked="" type="radio"/> | <input checked="" type="radio"/> | <input checked="" type="radio"/> | <input checked="" type="radio"/> | <input checked="" type="radio"/> | <input checked="" type="radio"/> |
|                                  | D                                | <input type="radio"/>            | <input type="radio"/>            | <input type="radio"/>            | <input type="radio"/>            | <input type="radio"/>            | <input type="radio"/>            | <input type="radio"/>            | <input type="radio"/>            | <input checked="" type="radio"/> | <input checked="" type="radio"/> | <input checked="" type="radio"/> | <input checked="" type="radio"/> | <input checked="" type="radio"/> | <input checked="" type="radio"/> | <input checked="" type="radio"/> | <input checked="" type="radio"/> | <input checked="" type="radio"/> | <input checked="" type="radio"/> |
| A                                | B                                | C                                |                                  |                                  |                                  |                                  |                                  |                                  |                                  |                                  |                                  |                                  |                                  |                                  |                                  |                                  |                                  |                                  |                                  |
| <input type="radio"/>            | <input type="radio"/>            | <input type="radio"/>            | 1                                | 0                                | 0                                | 0                                | 0                                | 0                                | 0                                | 0                                | 0                                | 0                                | 0                                | 0                                | 0                                | 0                                | 0                                | 0                                | 0                                |
| <input checked="" type="radio"/> | <input type="radio"/>            | <input type="radio"/>            | 0                                | 0                                | 0                                | 0                                | 1                                | 0                                | 0                                | 0                                | 0                                | 0                                | 0                                | 0                                | 0                                | 0                                | 0                                | 0                                | 0                                |
| <input type="radio"/>            | <input checked="" type="radio"/> | <input type="radio"/>            | 0                                | 0                                | 0                                | 0                                | 0                                | 1                                | 0                                | 0                                | 0                                | 0                                | 0                                | 0                                | 0                                | 0                                | 0                                | 0                                | 0                                |
| <input checked="" type="radio"/> | <input checked="" type="radio"/> | <input type="radio"/>            | 0                                | 1                                | 0                                | 0                                | 0                                | 0                                | 0                                | 0                                | 0                                | 0                                | 0                                | 0                                | 0                                | 0                                | 0                                | 0                                | 0                                |
| <input type="radio"/>            | <input type="radio"/>            | <input checked="" type="radio"/> | 0                                | 1                                | 0                                | 0                                | 0                                | 0                                | 0                                | 0                                | 0                                | 0                                | 0                                | 0                                | 0                                | 0                                | 0                                | 0                                | 0                                |
| <input checked="" type="radio"/> | <input type="radio"/>            | <input checked="" type="radio"/> | 0                                | 0                                | 0                                | 0                                | 0                                | 0                                | 0                                | 1                                | 0                                | 0                                | 0                                | 0                                | 0                                | 0                                | 0                                | 0                                | 0                                |
| <input type="radio"/>            | <input checked="" type="radio"/> | <input checked="" type="radio"/> | 0                                | 0                                | 0                                | 0                                | 0                                | 1                                | 0                                | 0                                | 0                                | 0                                | 0                                | 0                                | 0                                | 0                                | 0                                | 0                                | 0                                |
| <input checked="" type="radio"/> | <input checked="" type="radio"/> | <input checked="" type="radio"/> | 0                                | 0                                | 0                                | 1                                | 0                                | 0                                | 0                                | 0                                | 0                                | 0                                | 0                                | 0                                | 0                                | 0                                | 0                                | 0                                | 0                                |

A☐

B☐

C☐

A

B

C

☐

1

0

0

0

0

0

0

0

0

0

0

0

0

0

0

0

0

0

0

0

0

0

0

0

0

0

0

0

0

0

0

0

0

0

0

0

0

0

0

0

0

0

0

0

0

0

0

0

0

0

0

0

0

0

0

0

0

0

0

0

0

0

0

0

0

0

0

0

0

0

0

0

0

0

0

0

0

0

0

0

0

0

0

0

0

0

0

0

0

0

0

0

0

0

0

0

0

0

0

0

0

0

0

0

0

0

0

0

0

0

0

0

0

0

0

0

0

0

0

0

0

0

0

0

0

0

0

0

0

0

0

0

0

0

0

0

0

0

0

0

0

0

0

0

0

0

0

0

0

0

0

0

0

0

0

0

0

0

0

0

0

0

0

0

0

0

0

0

0

0

0

0

0

0

0

0

0

0

0

0

0

0

0

0

0

0

0

0

0

0

0

0

0

0

0

0

0

0

0

0

0

0

0

0

0

0

0

0

0

0

0

0

0

0

0

0

0

0

0

0

0

0

0

0

0

0

0

0

0

0

0

0

0

0

0

0

0

0

0

0

0

0

0

0

0

0

0

0

0

0

0

0

0

0

0

0

0

0

0

0

0

0

0

0

0

0

0

0

0

0

0

0

0

0

0

0

0

0

0

0

0

0

0

0

0

0

0

0

0

0

0

0

0

0

0

0

0

0

0

0

0

0

0

0

0

0

0

0

0

0

0

0

0

0

0

0

0

0

0

0

0

0

0

0

0

0

0

0

0

0

0

0

0

0

0

0

0

0

0

0

0

0

0

0

0

0

0

0

0

0

Fixing background conditions:

## Marginalization

- Note that the first and ninth columns differ only by **D**'s state
- We sum those columns together to get the probabilities of transitioning to state **ABC** = (0, 0, 0), **ignoring the state of D**, from each previous state
- We repeat this for **ABC** = (1, 0, 0)...

|   |   |   |   |   |   |   |   |   |   |   |   |   |   |   |   |   |
|---|---|---|---|---|---|---|---|---|---|---|---|---|---|---|---|---|
| A | ○ | ● | ○ | ● | ○ | ● | ○ | ● | ○ | ● | ○ | ● | ○ | ● | ○ | ● |
| B | ○ | ○ | ● | ● | ○ | ○ | ● | ● | ○ | ○ | ● | ● | ○ | ○ | ● | ● |
| C | ○ | ○ | ○ | ○ | ● | ● | ● | ● | ○ | ○ | ○ | ○ | ● | ● | ● | ● |
| D | ○ | ○ | ○ | ○ | ○ | ○ | ○ | ○ | ● | ○ | ● | ● | ● | ● | ● | ● |

  

| A | B | C | 1 | 0 | 0 | 0 | 0 | 0 | 0 | 0 | 0 | 0 | 0 | 0 | 0 | 0 |
|---|---|---|---|---|---|---|---|---|---|---|---|---|---|---|---|---|
| ○ | ○ | ○ | 1 | 0 | 0 | 0 | 0 | 0 | 0 | 0 | 0 | 0 | 0 | 0 | 0 | 0 |
| ● | ○ | ○ | 0 | 0 | 0 | 0 | 1 | 0 | 0 | 0 | 0 | 0 | 0 | 0 | 0 | 0 |
| ○ | ● | ○ | 0 | 0 | 0 | 0 | 0 | 1 | 0 | 0 | 0 | 0 | 0 | 0 | 0 | 0 |
| ● | ● | ○ | 0 | 1 | 0 | 0 | 0 | 0 | 0 | 0 | 0 | 0 | 0 | 0 | 0 | 0 |
| ○ | ○ | ● | 0 | 1 | 0 | 0 | 0 | 0 | 0 | 0 | 0 | 0 | 0 | 0 | 0 | 0 |
| ● | ○ | ● | 0 | 0 | 0 | 0 | 0 | 0 | 0 | 1 | 0 | 0 | 0 | 0 | 0 | 0 |
| ○ | ● | ● | 0 | 0 | 0 | 0 | 0 | 1 | 0 | 0 | 0 | 0 | 0 | 0 | 0 | 0 |
| ● | ● | ● | 0 | 0 | 0 | 1 | 0 | 0 | 0 | 0 | 0 | 0 | 0 | 0 | 0 | 0 |

  

| A | B | C | 1 | 0 |
|---|---|---|---|---|
| ○ | ○ | ○ | 1 | 0 |
| ● | ○ | ○ | 0 | 0 |
| ○ | ● | ○ | 0 | 0 |
| ● | ● | ○ | 0 | 1 |
| ○ | ○ | ● | 0 | 1 |
| ● | ○ | ● | 0 | 0 |
| ○ | ● | ● | 0 | 0 |
| ● | ● | ● | 0 | 0 |

# Marginalization

- 

|                                                                                       |                                                                                       |                                                                                       |          |                                                                                     |                                                                                     |                                                                                     |                                                                                     |                                                                                     |                                                                                     |                                                                                     |                                                                                     |
|---------------------------------------------------------------------------------------|---------------------------------------------------------------------------------------|---------------------------------------------------------------------------------------|----------|-------------------------------------------------------------------------------------|-------------------------------------------------------------------------------------|-------------------------------------------------------------------------------------|-------------------------------------------------------------------------------------|-------------------------------------------------------------------------------------|-------------------------------------------------------------------------------------|-------------------------------------------------------------------------------------|-------------------------------------------------------------------------------------|
|                                                                                       |                                                                                       |                                                                                       | <b>A</b> | 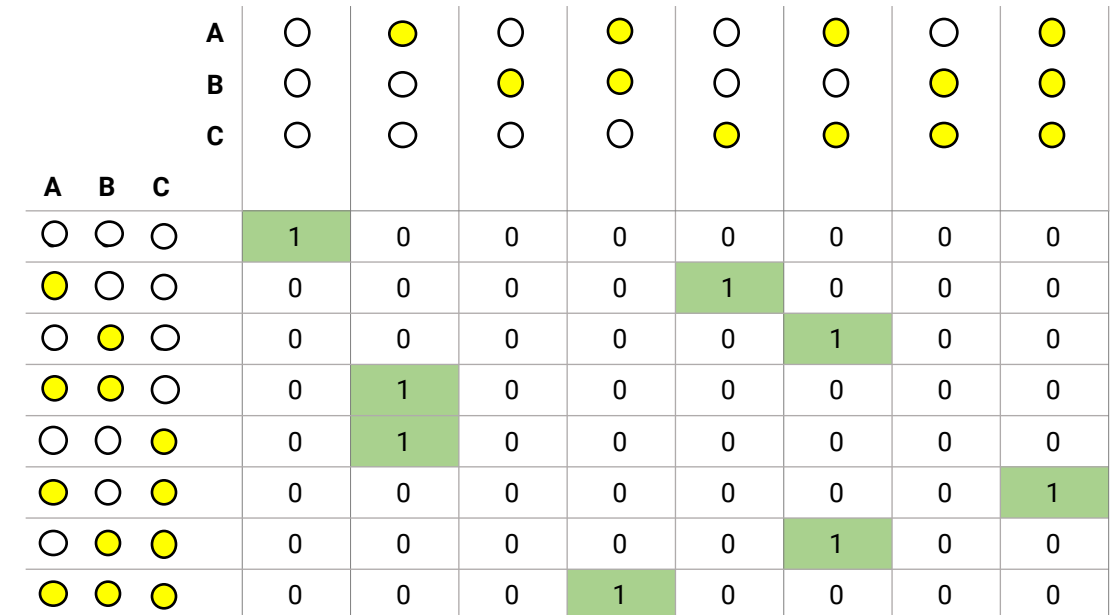 | 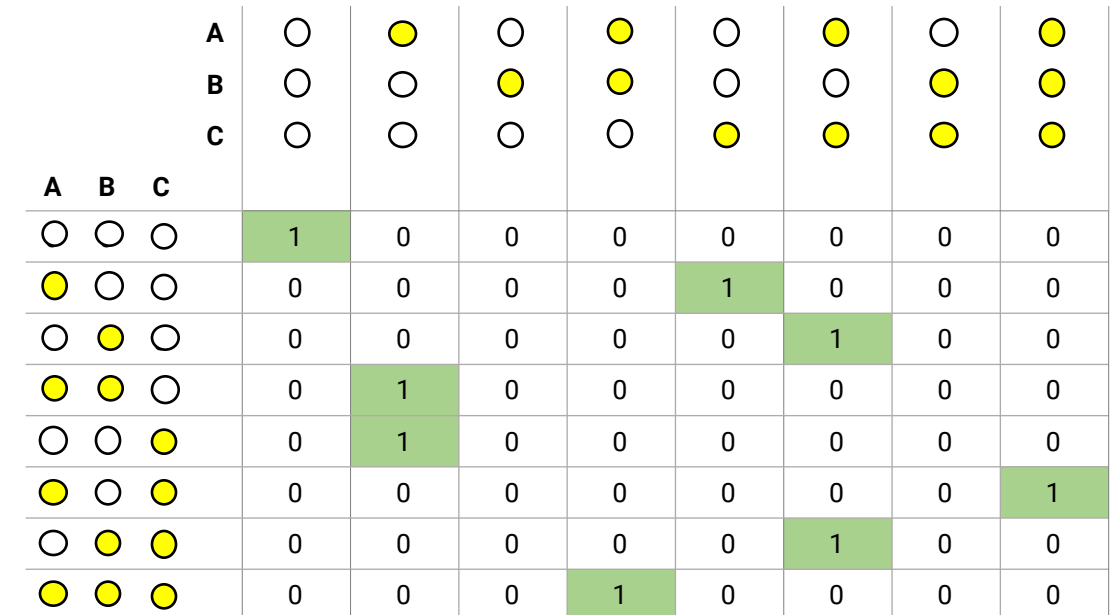 | 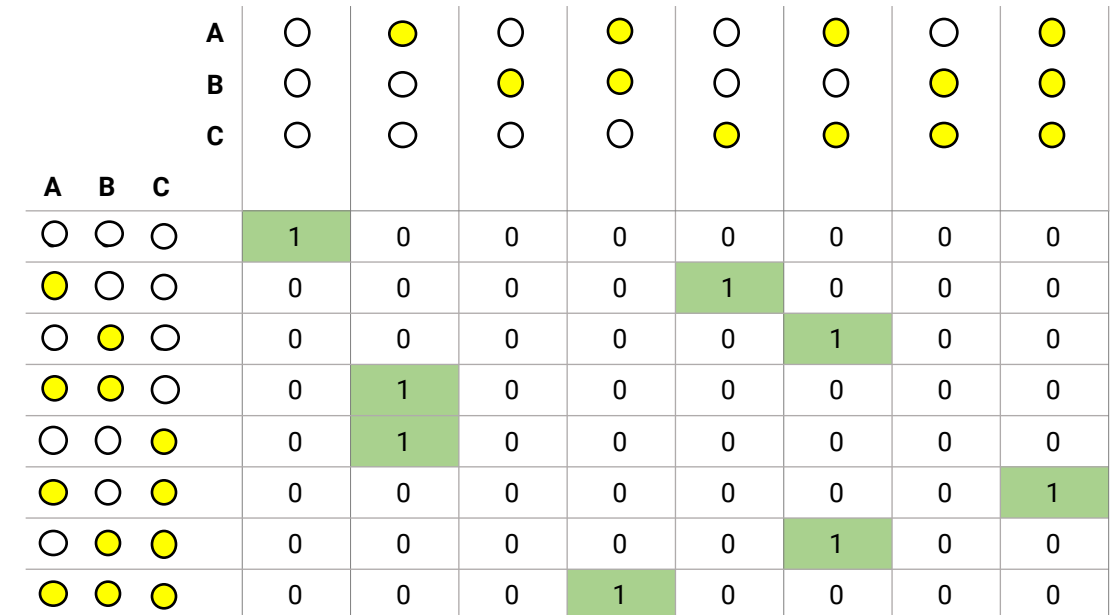 | 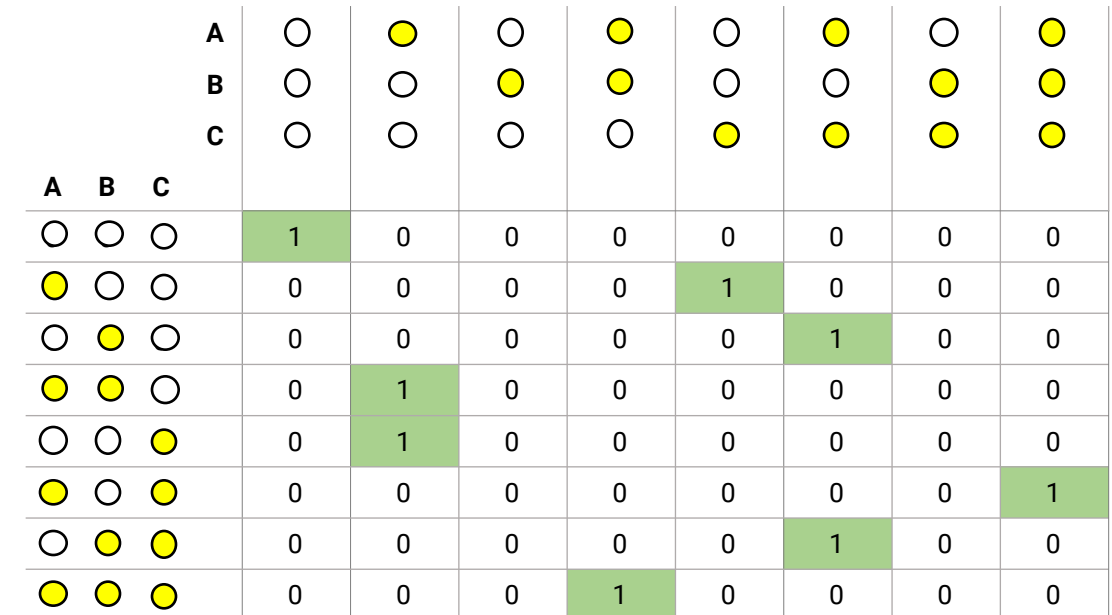 | 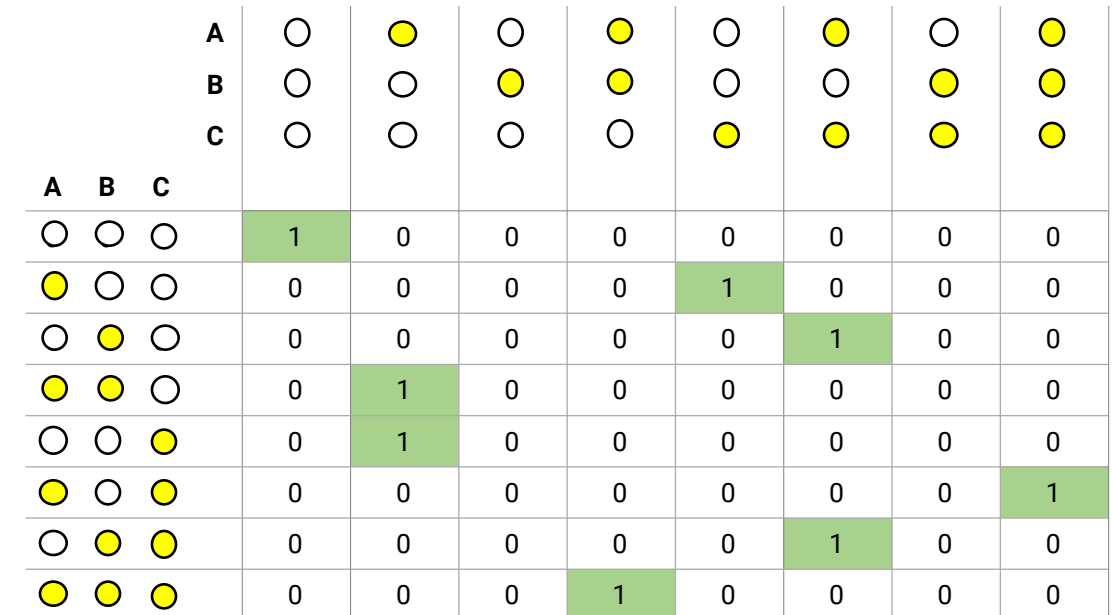 | 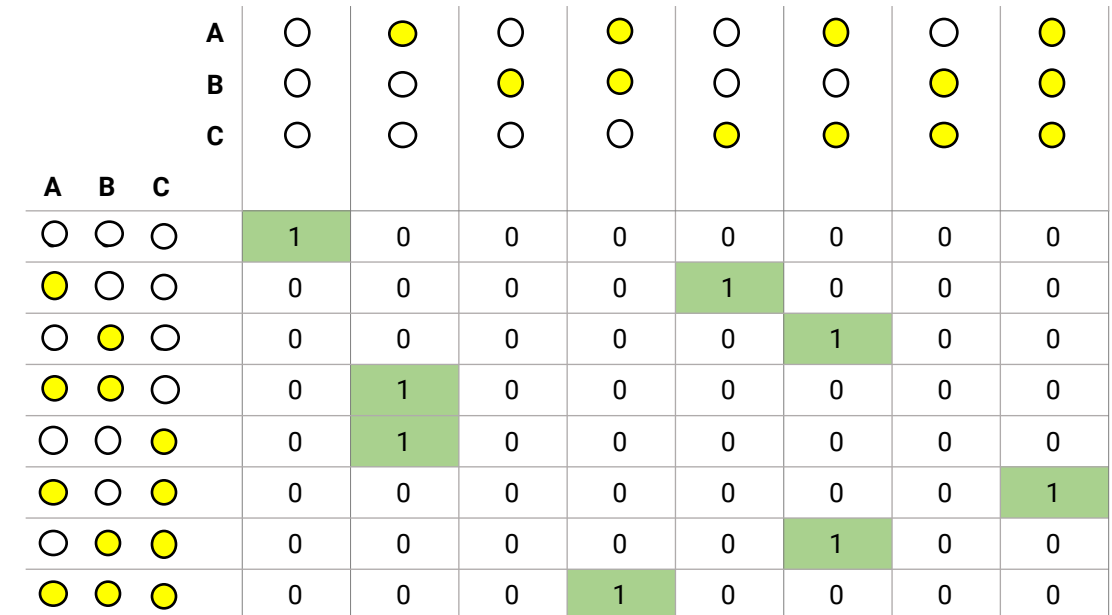 | 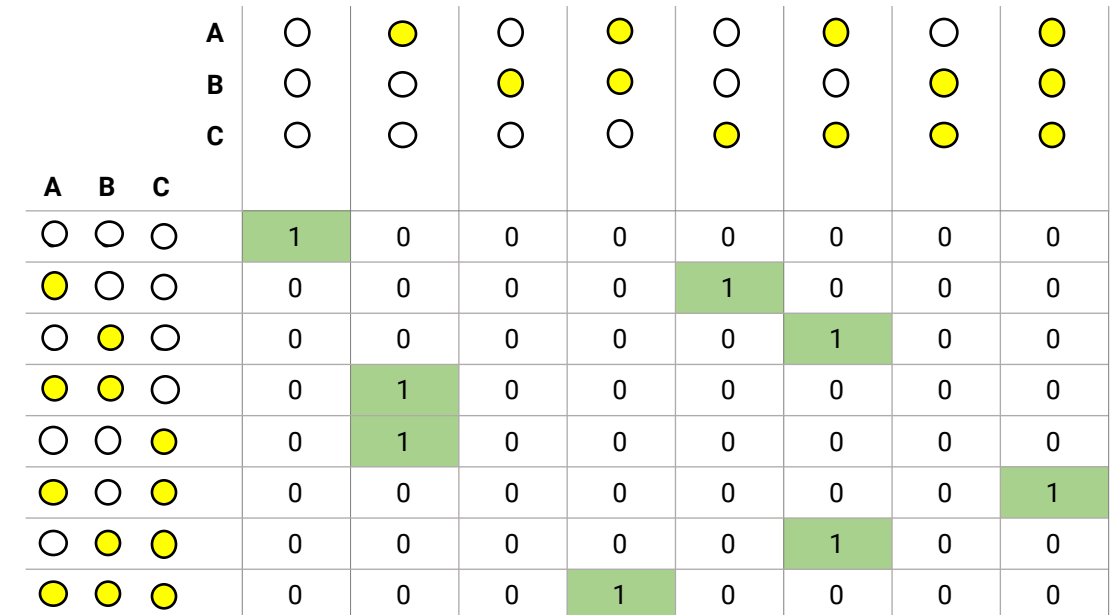 | 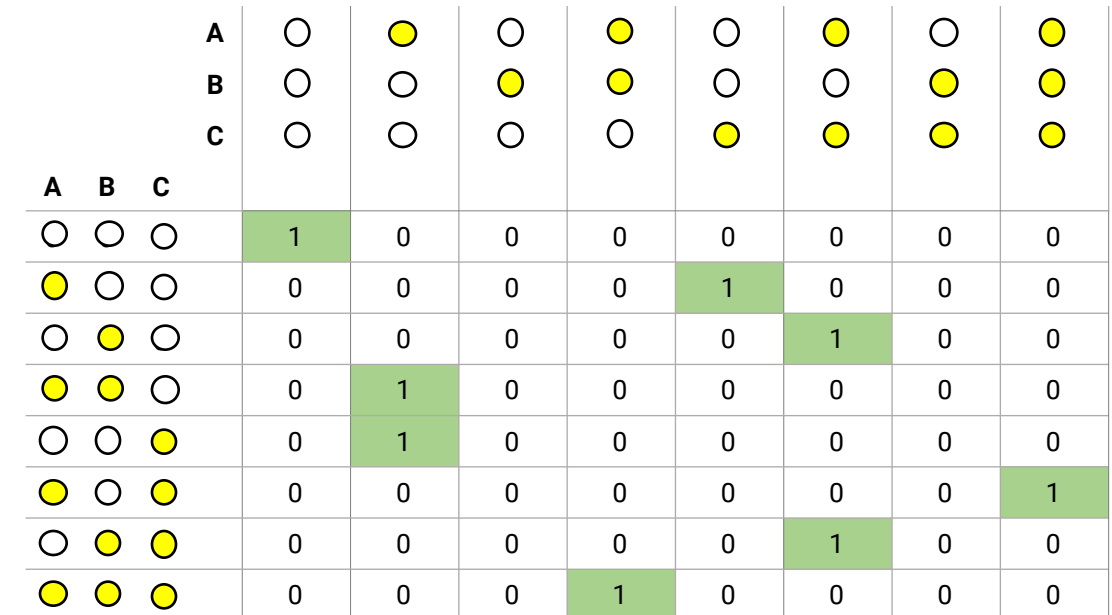 |
|                                                                                       |                                                                                       |                                                                                       | <b>B</b> | 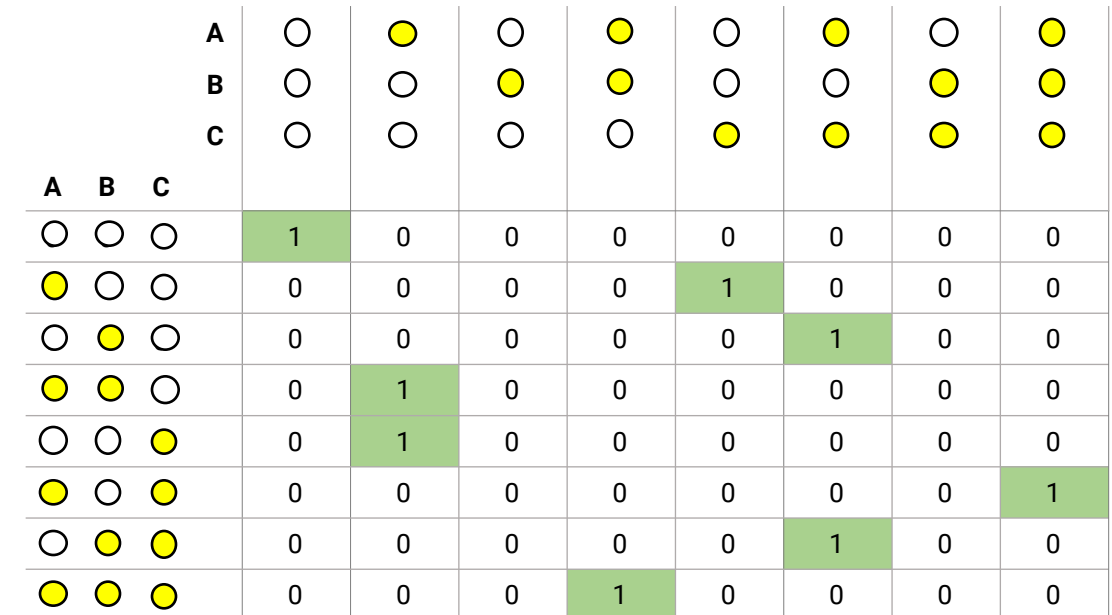 | 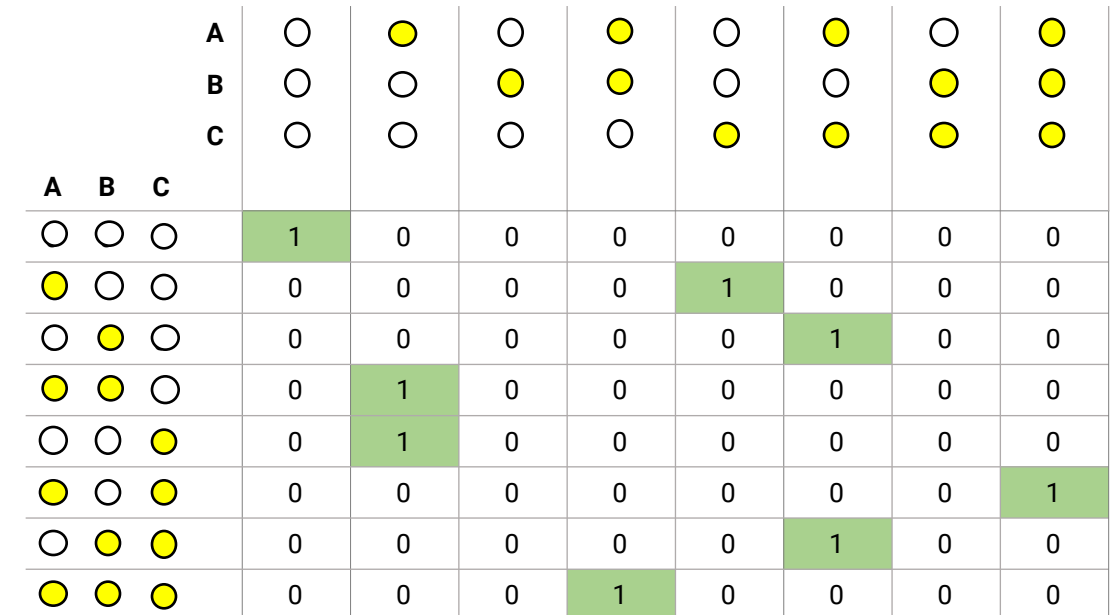 | 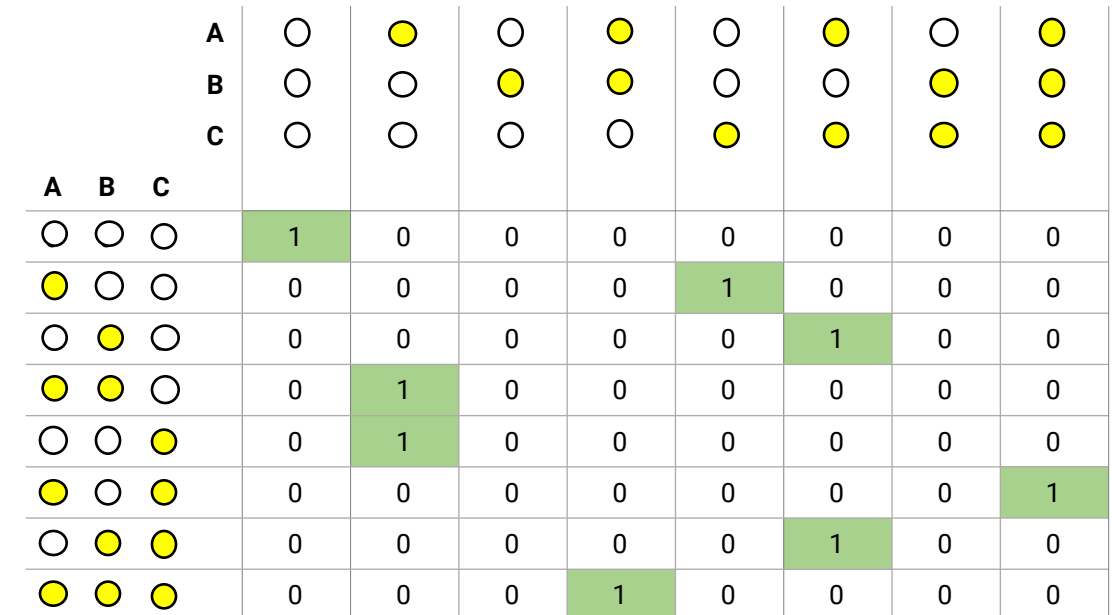 | 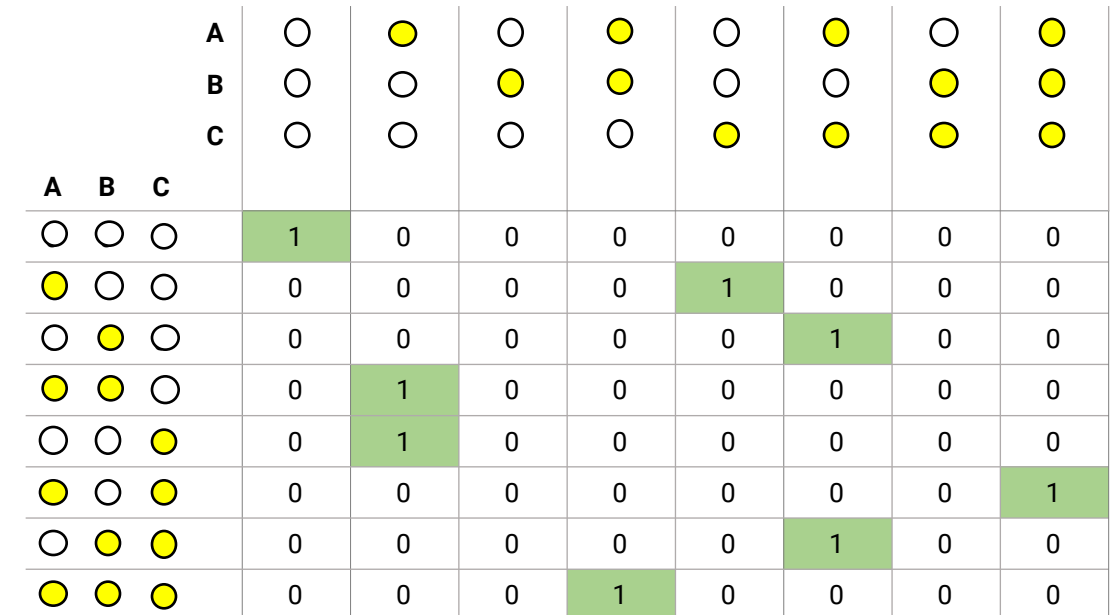 | 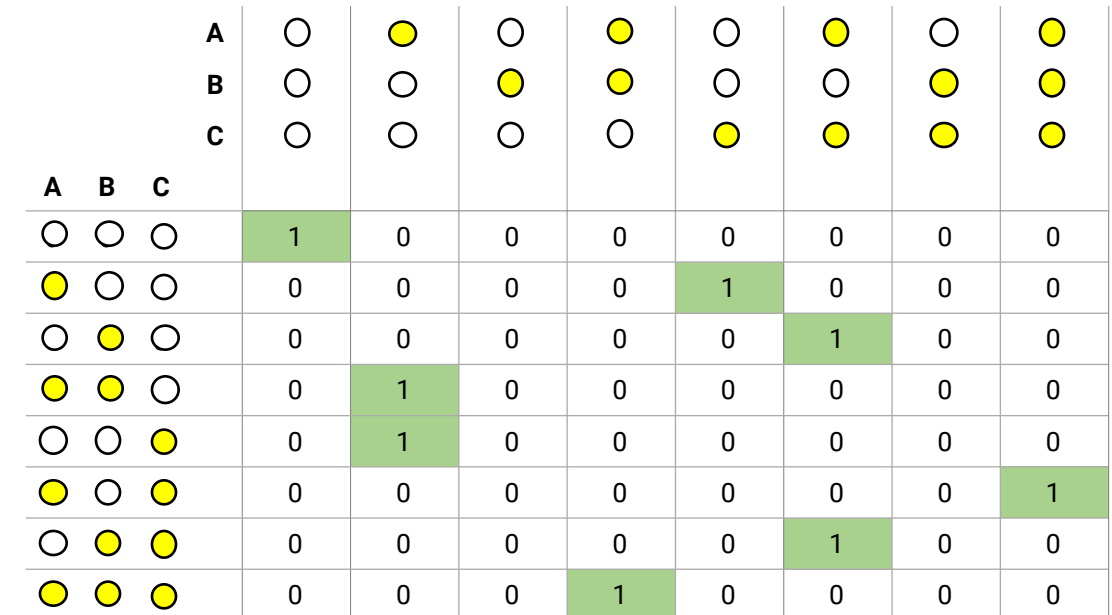 | 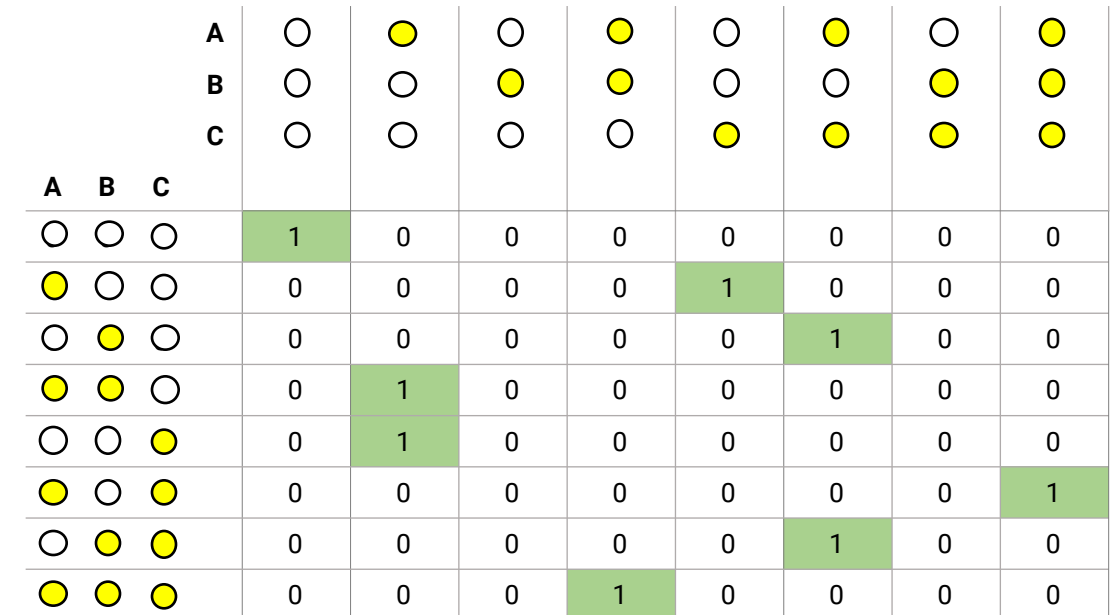 | 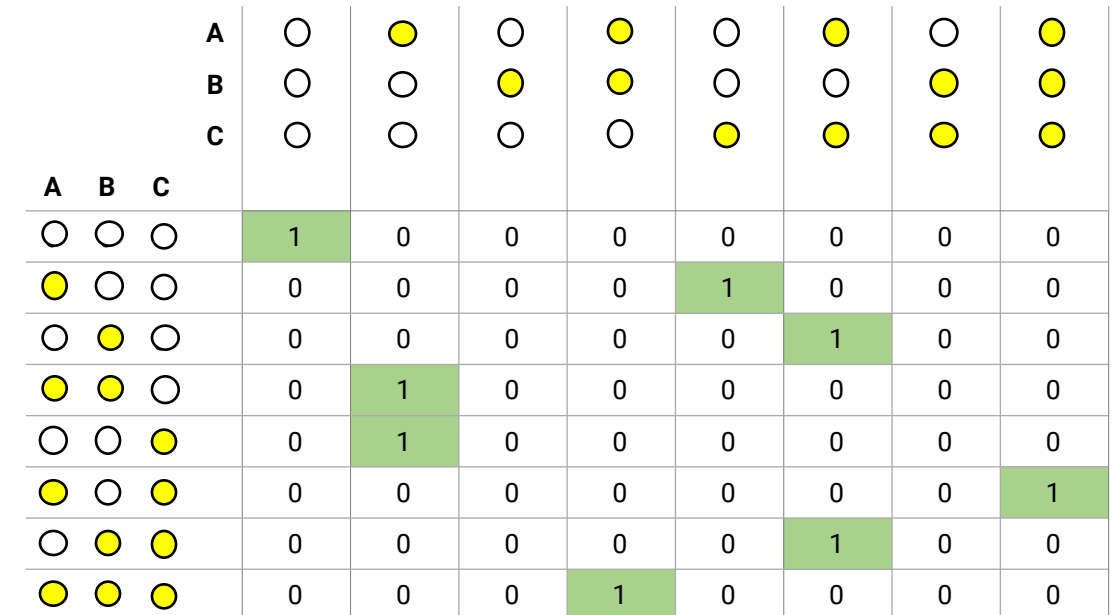 | 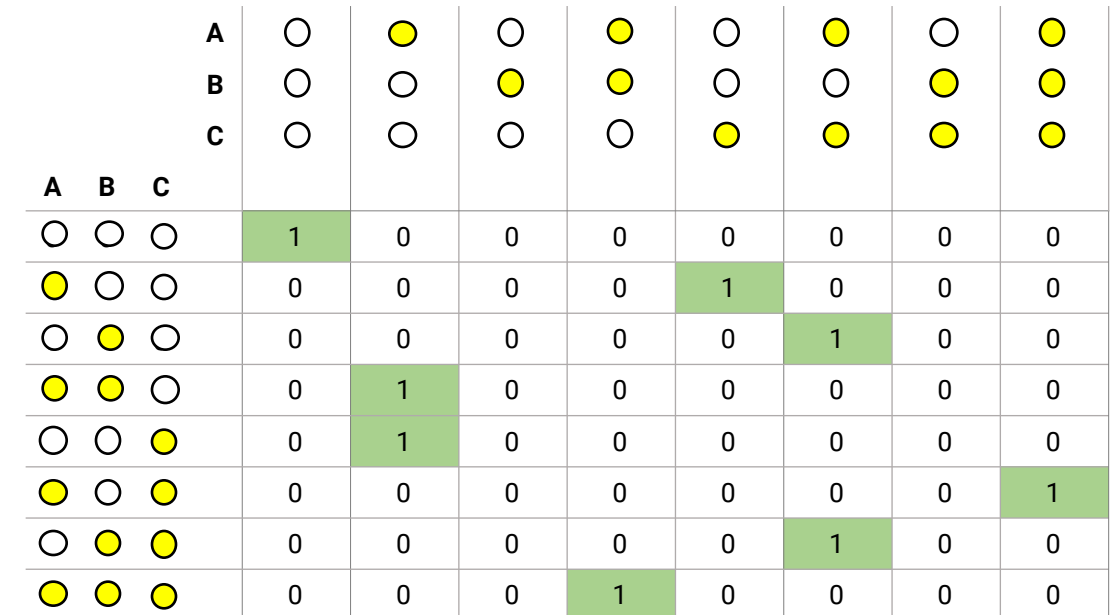 |
|                                                                                       |                                                                                       |                                                                                       | <b>C</b> | 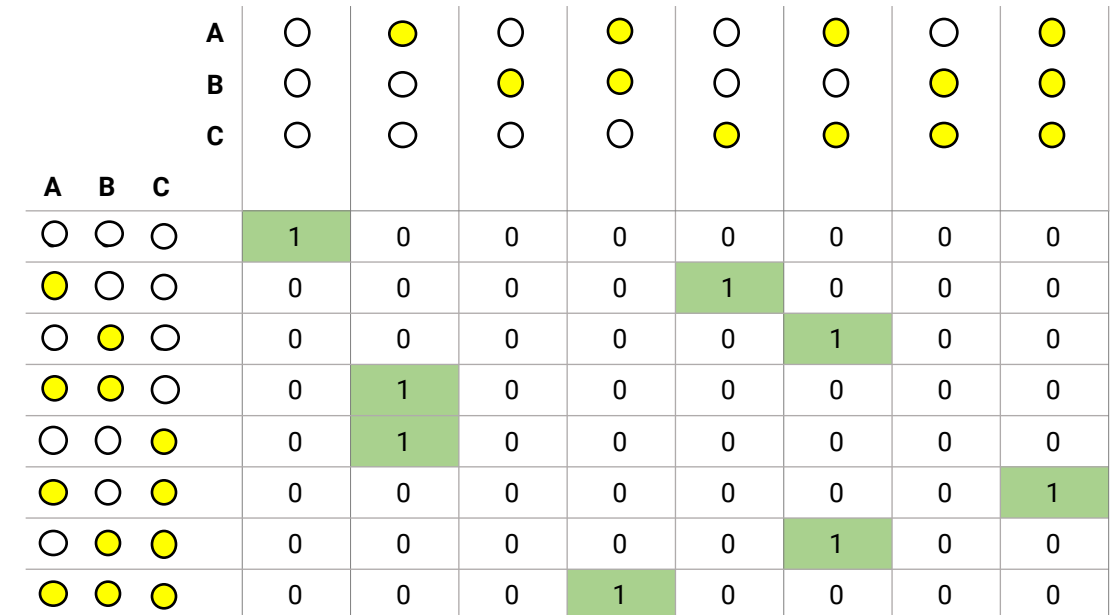 | 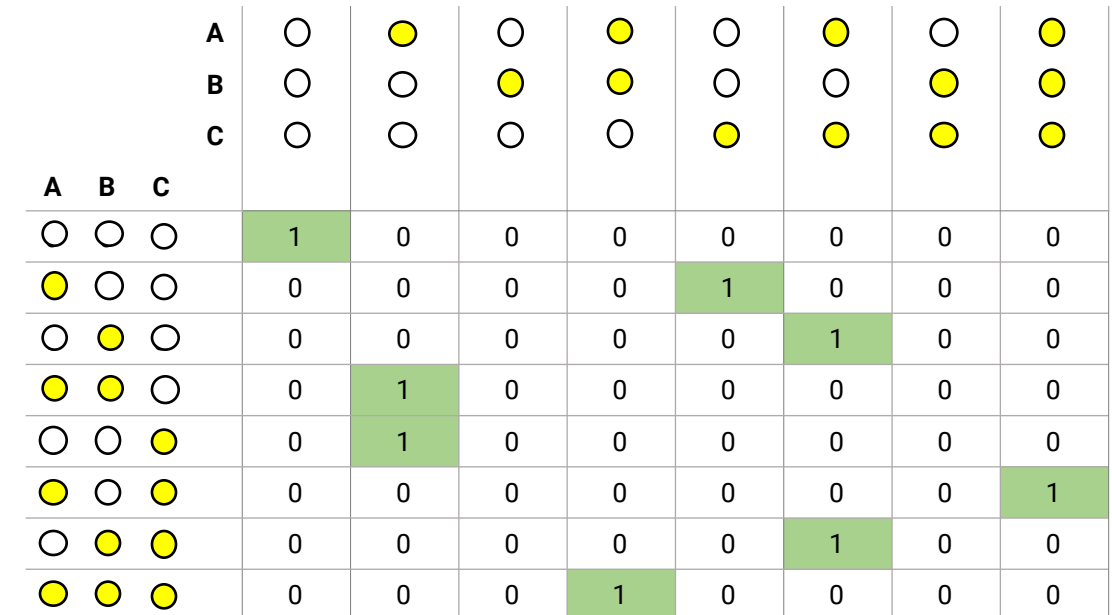 | 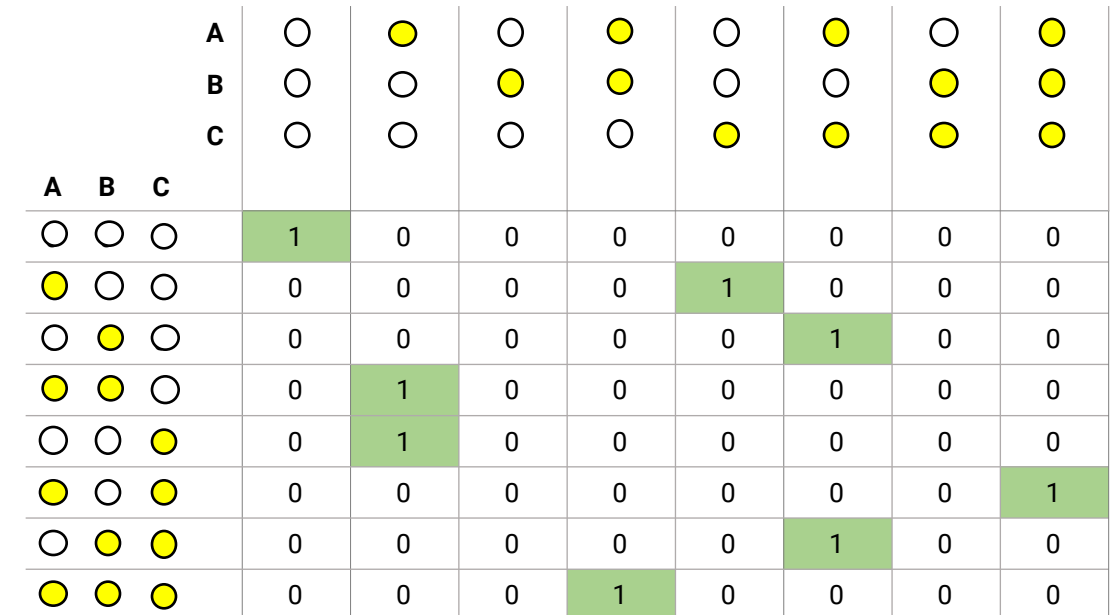 | 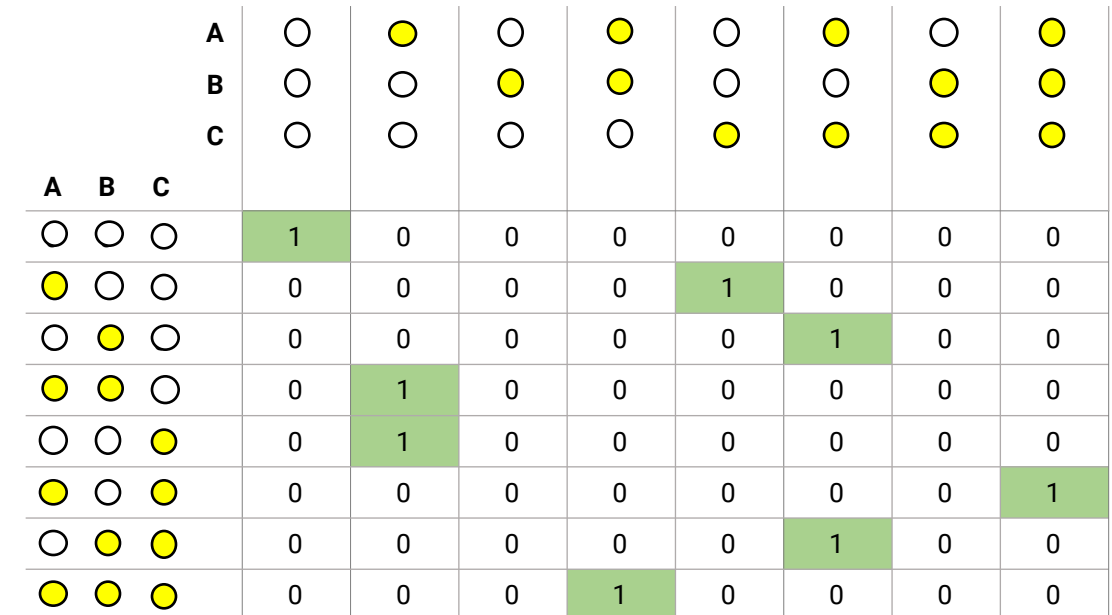 | 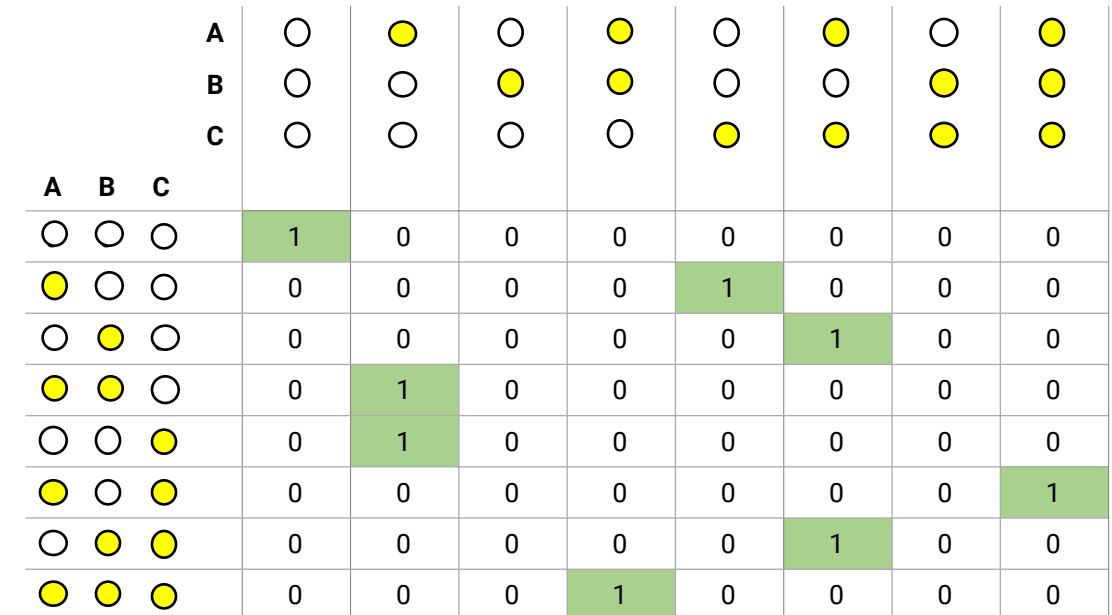 | 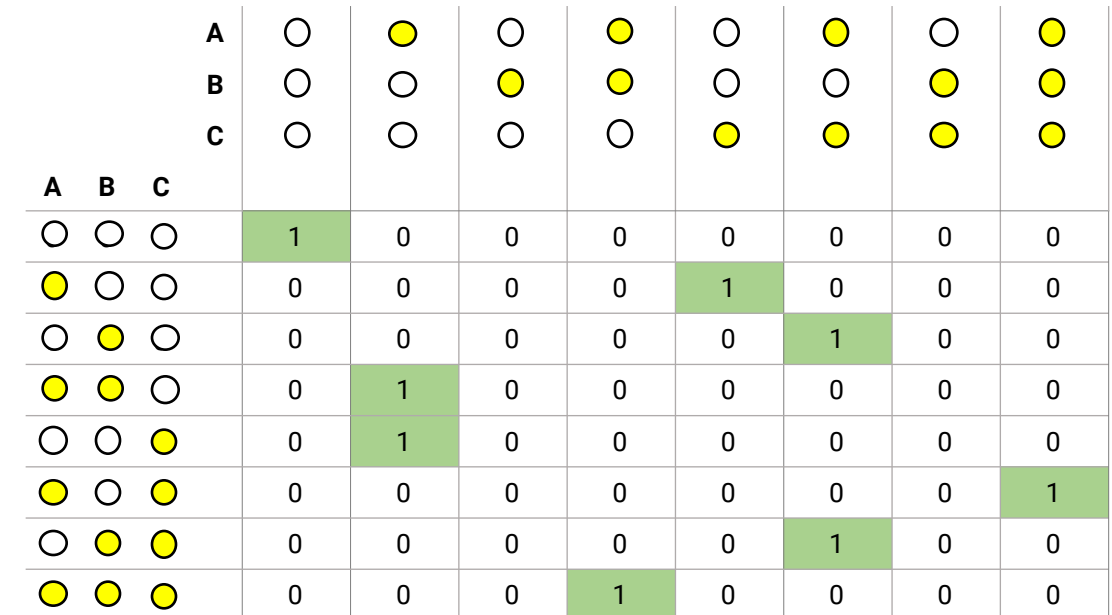 | 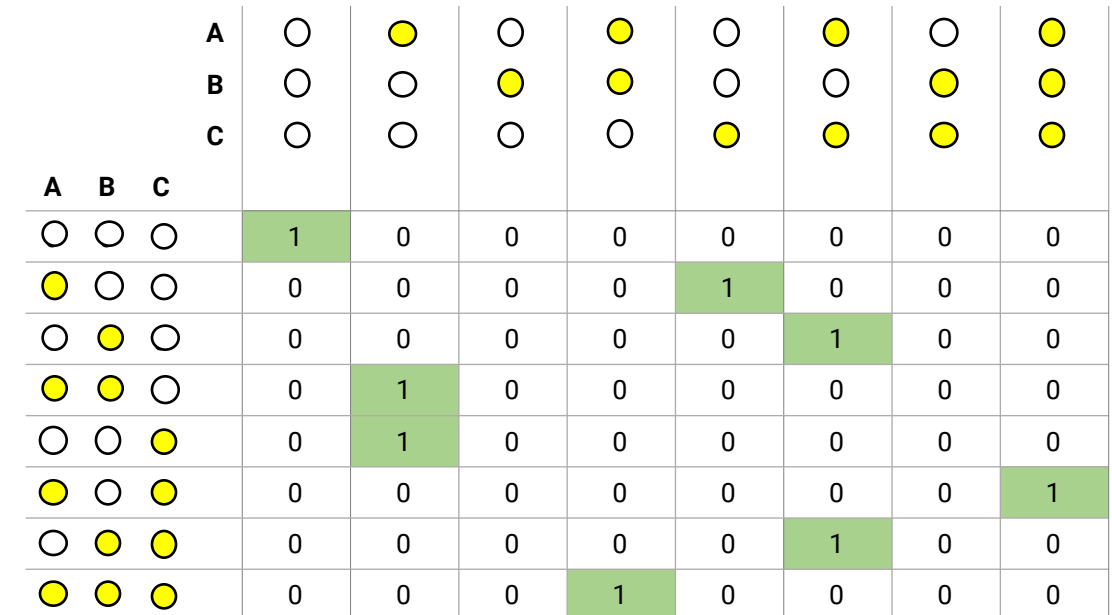 | 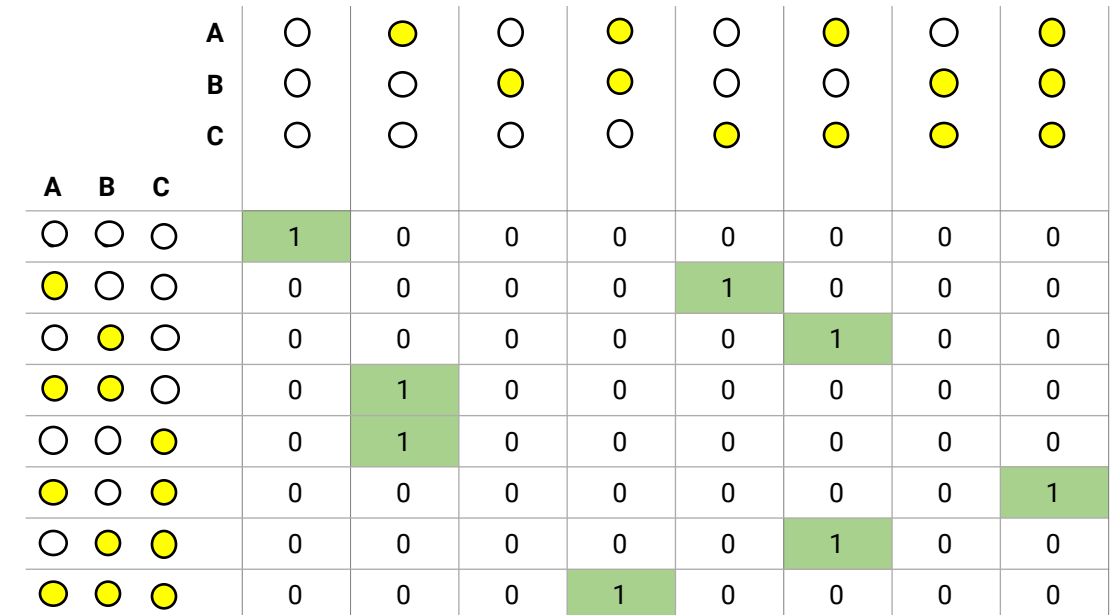 |
| <b>A</b>                                                                              | <b>B</b>                                                                              | <b>C</b>                                                                              |          |                                                                                     |                                                                                     |                                                                                     |                                                                                     |                                                                                     |                                                                                     |                                                                                     |                                                                                     |
| 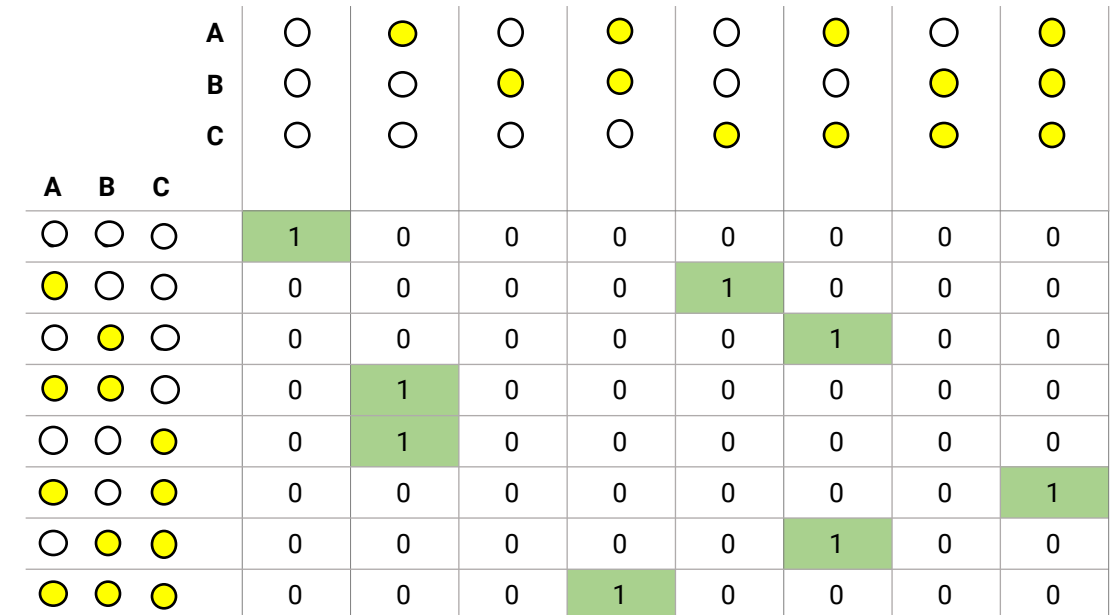  | 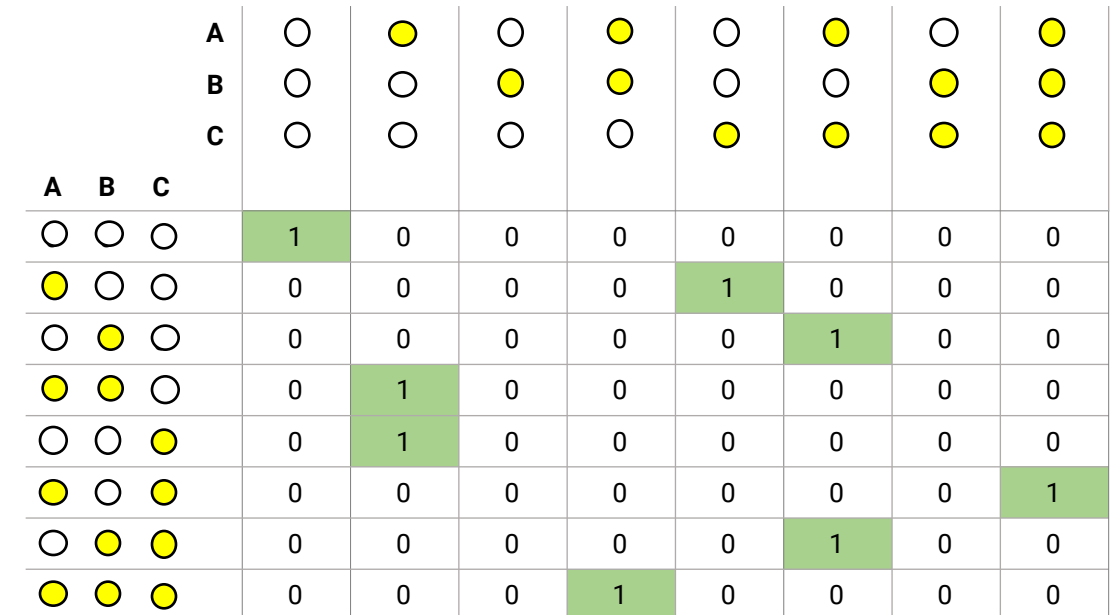  | 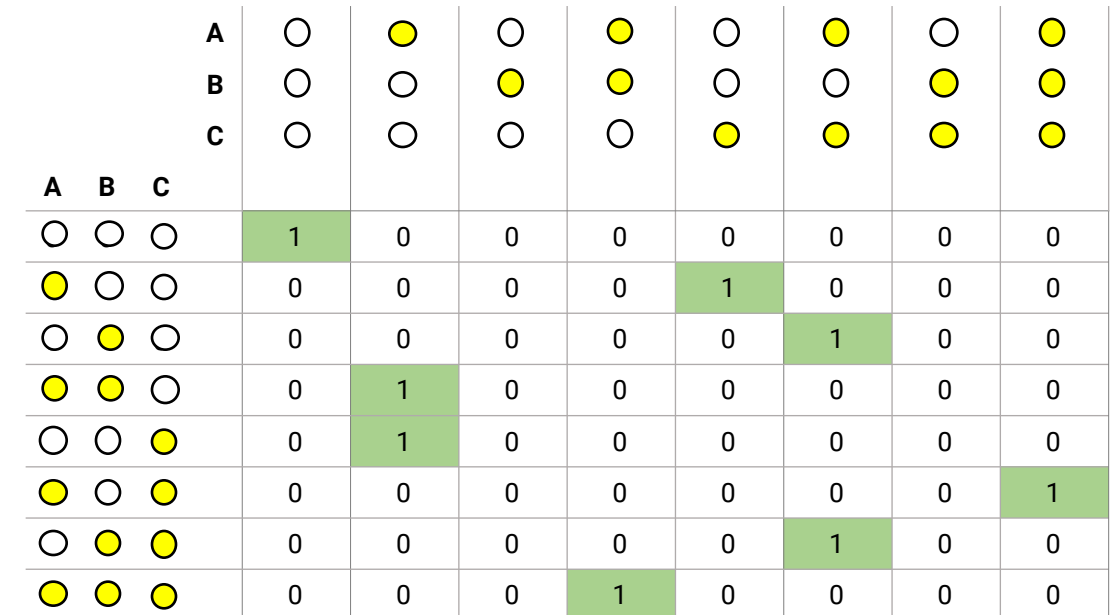  |          | 1                                                                                   | 0                                                                                   | 0                                                                                   | 0                                                                                   | 0                                                                                   | 0                                                                                   | 0                                                                                   | 0                                                                                   |
| 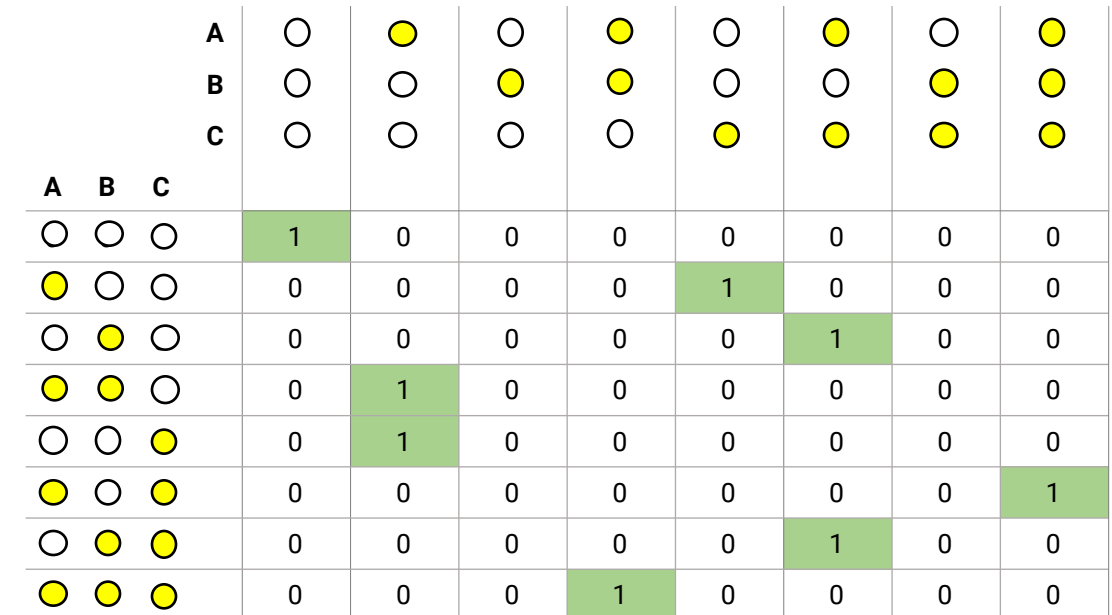 | 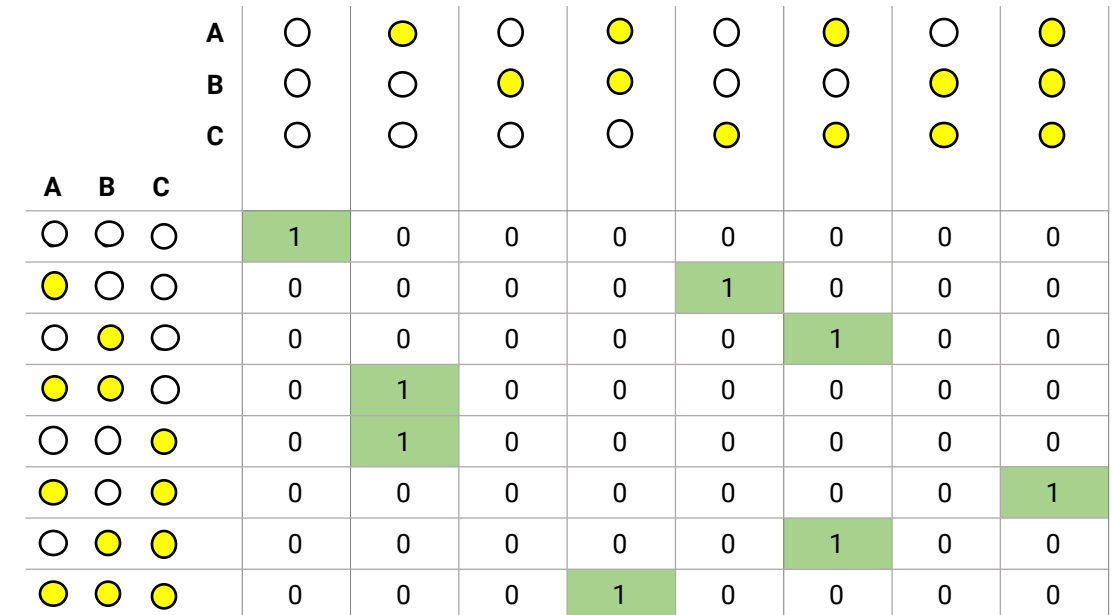 | 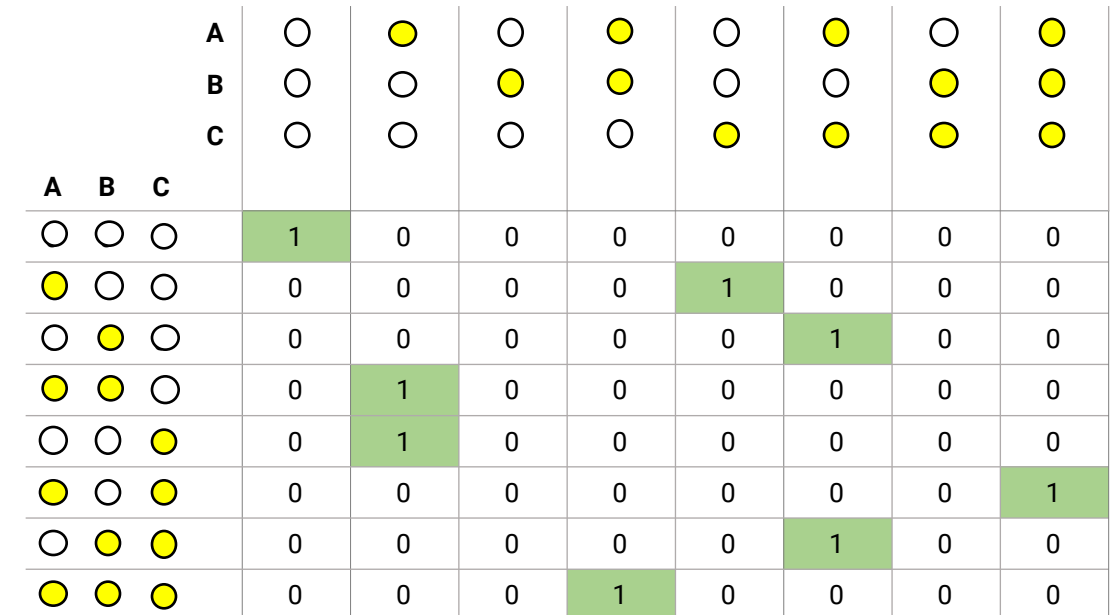 |          | 0                                                                                   | 0                                                                                   | 0                                                                                   | 0                                                                                   | 1                                                                                   | 0                                                                                   | 0                                                                                   | 0                                                                                   |
| 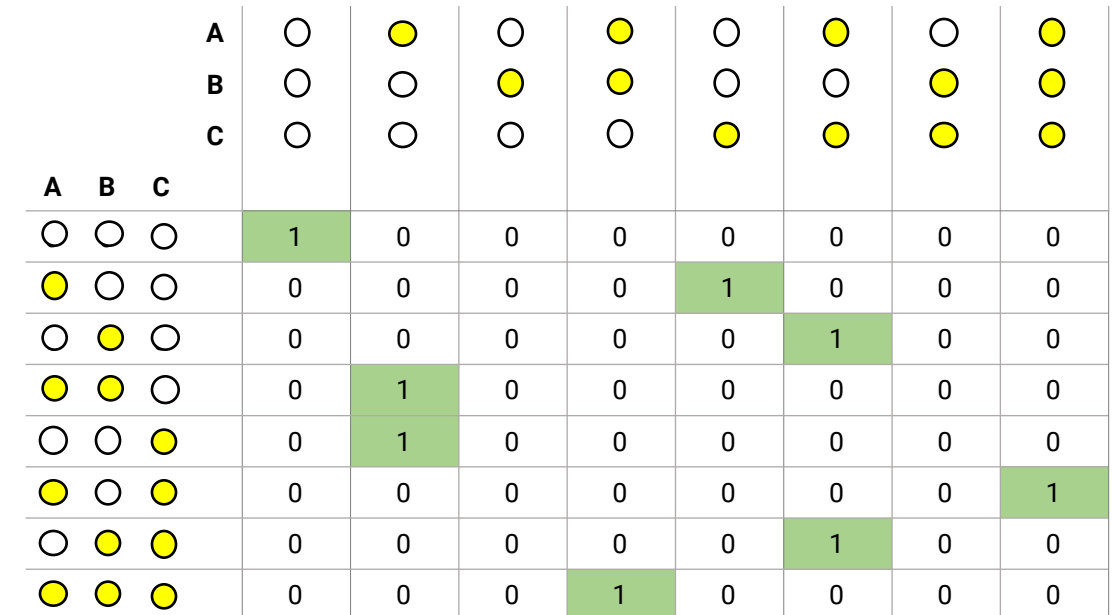 | 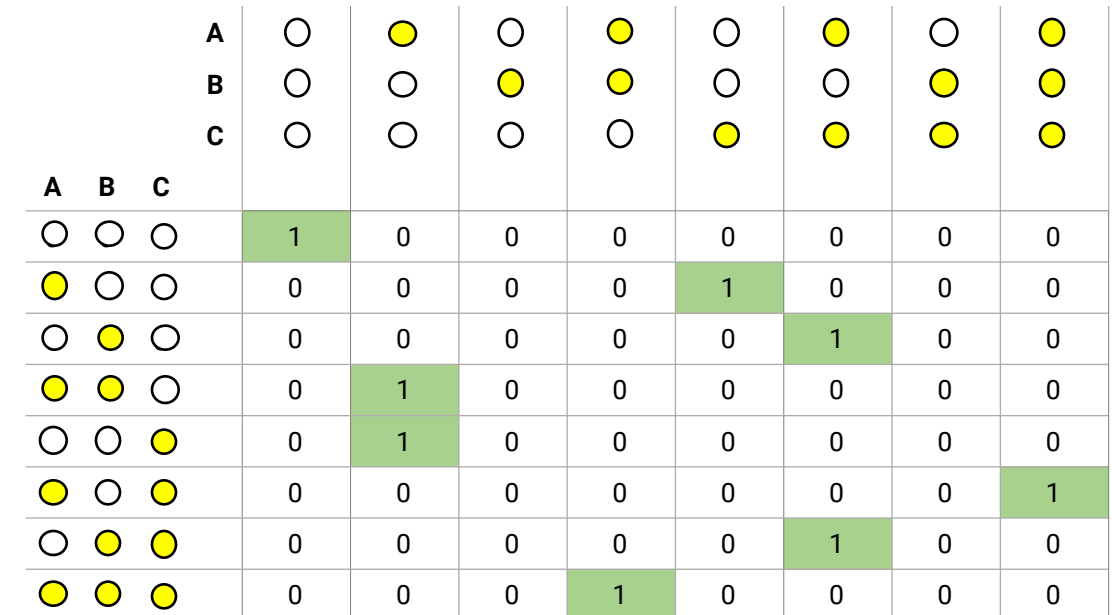 | 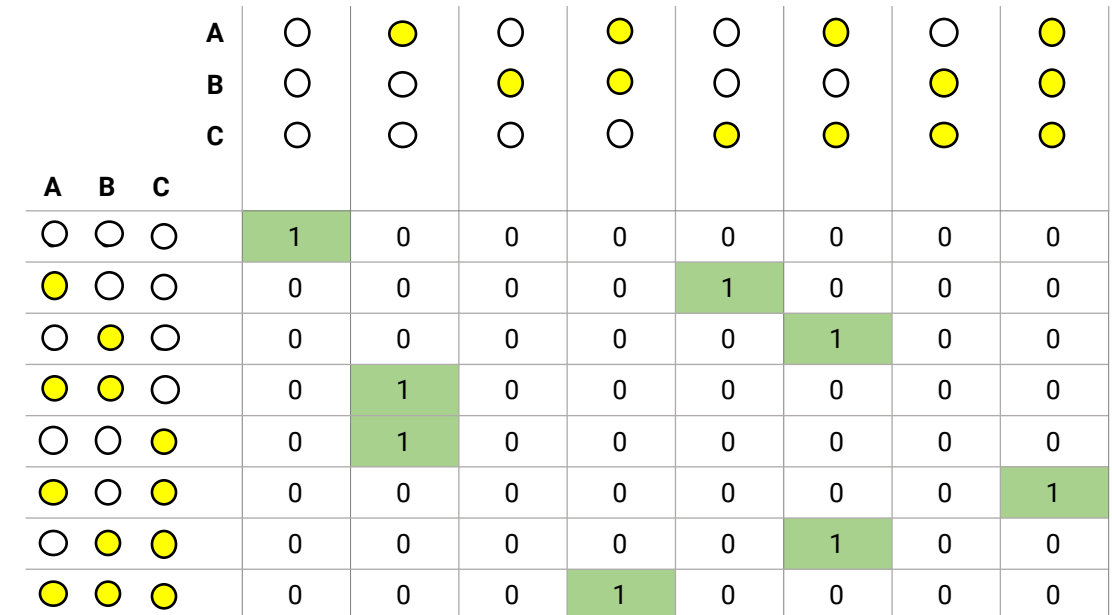 |          | 0                                                                                   | 0                                                                                   | 0                                                                                   | 0                                                                                   | 0                                                                                   | 1                                                                                   | 0                                                                                   | 0                                                                                   |
| 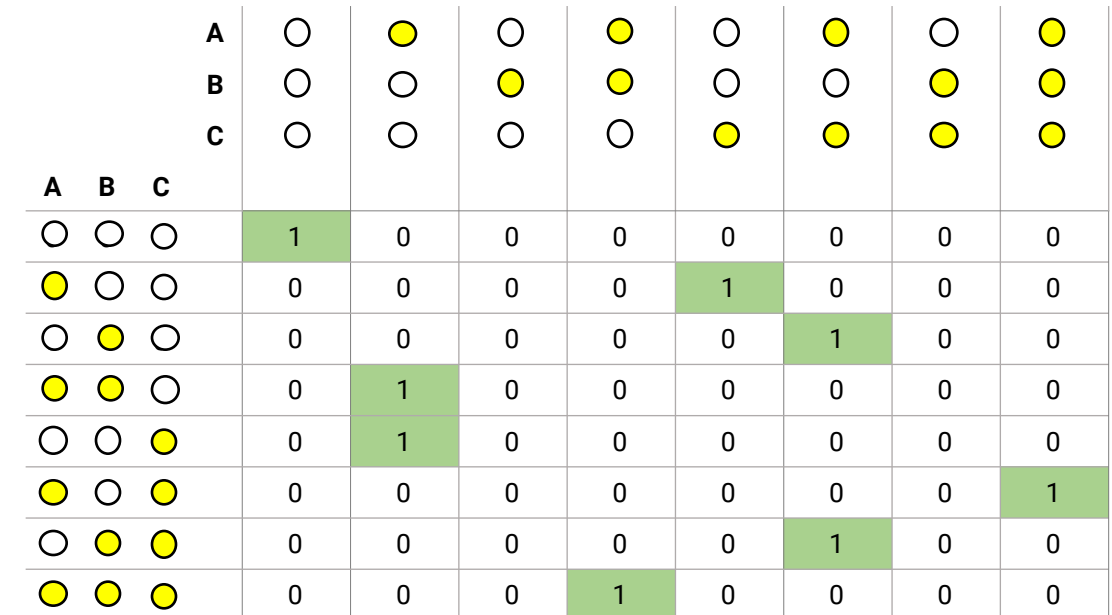 | 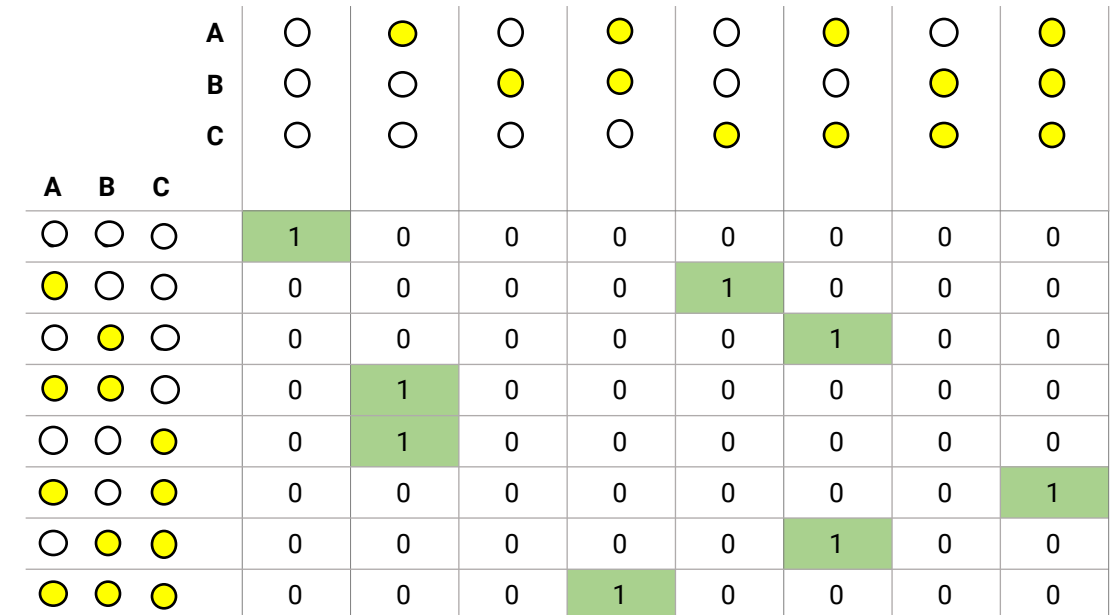 | 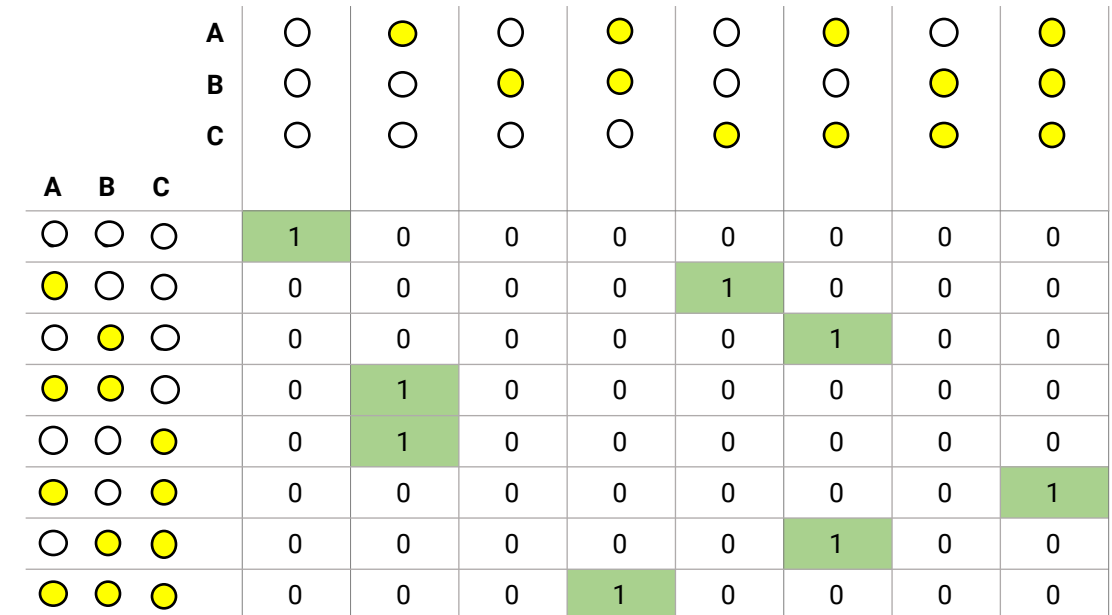 |          | 0                                                                                   | 1                                                                                   | 0                                                                                   | 0                                                                                   | 0                                                                                   | 0                                                                                   | 0                                                                                   | 0                                                                                   |
| 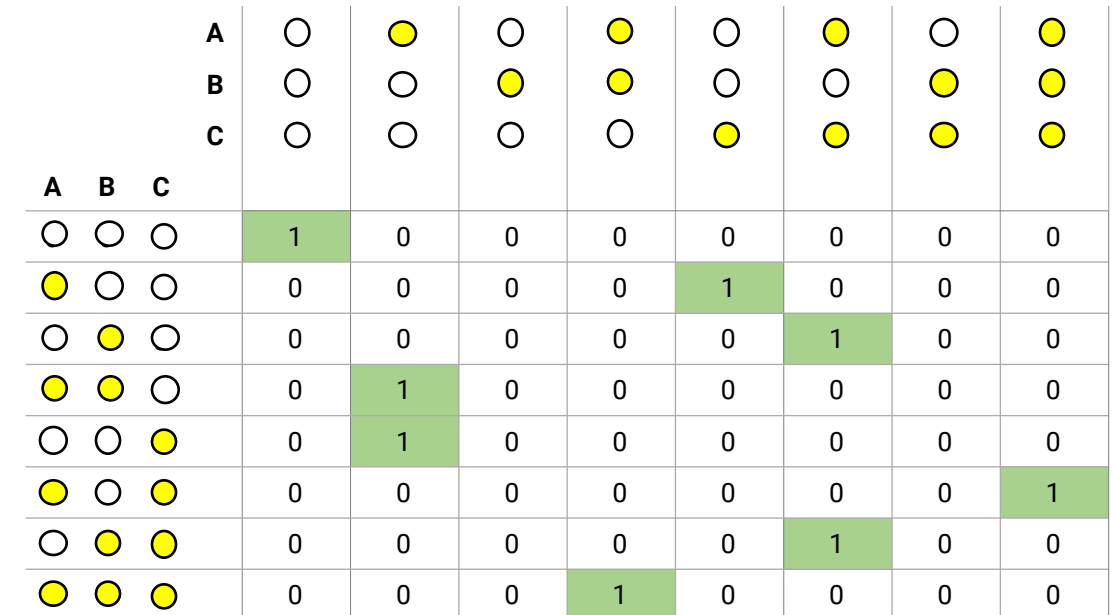 | 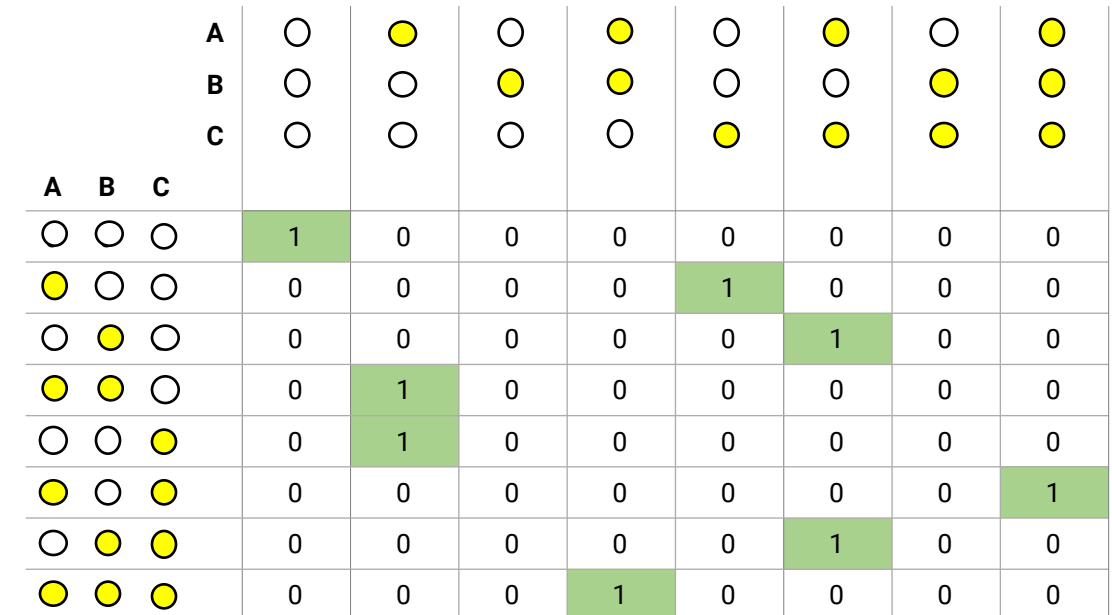 | 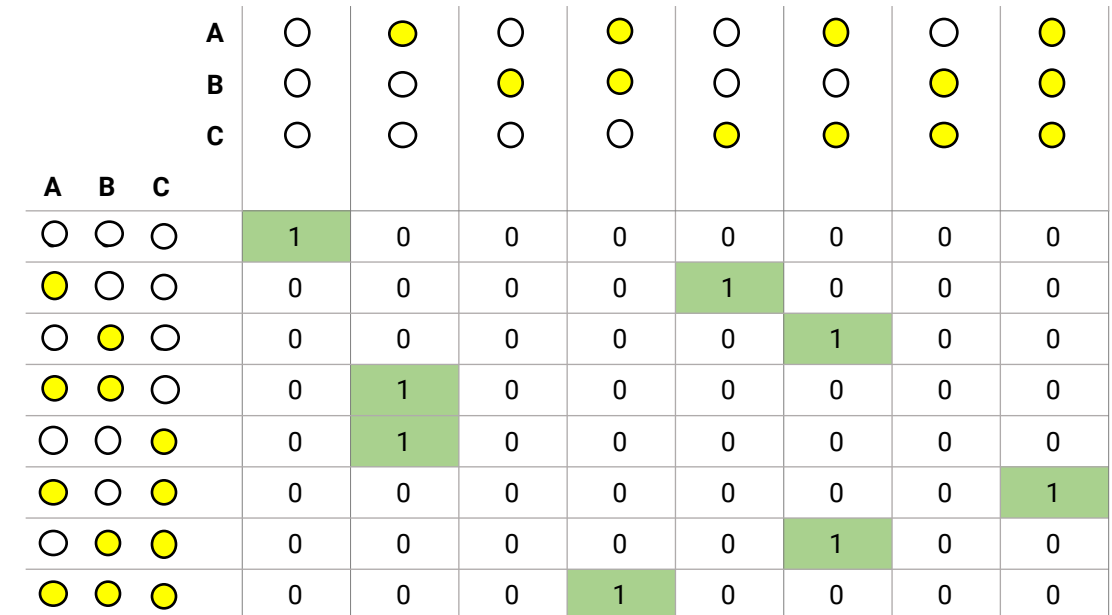 |          | 0                                                                                   | 1                                                                                   | 0                                                                                   | 0                                                                                   | 0                                                                                   | 0                                                                                   | 0                                                                                   | 0                                                                                   |
| 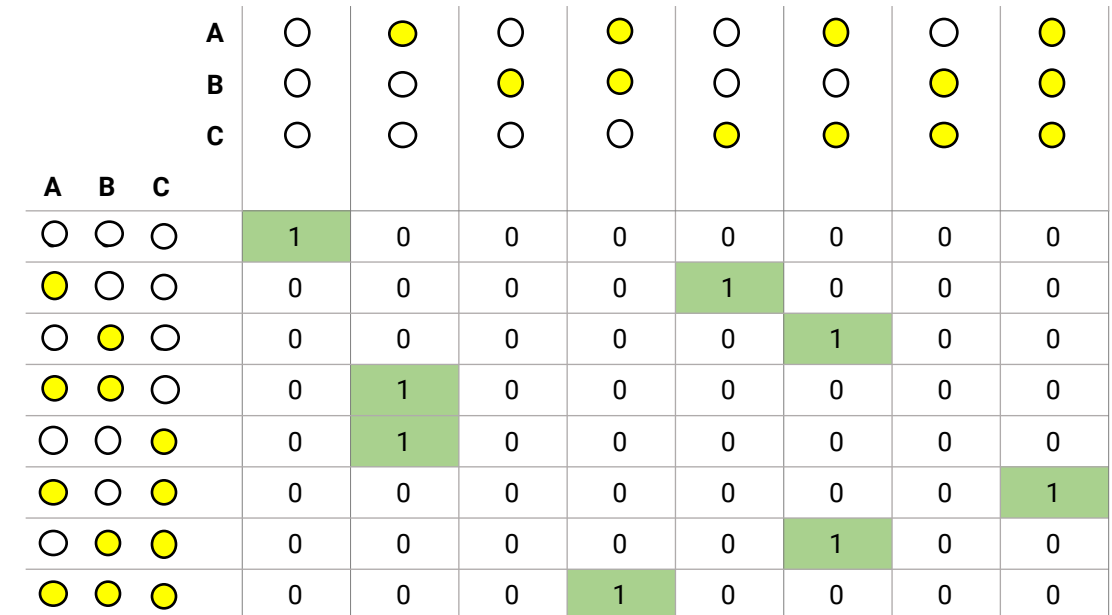 | 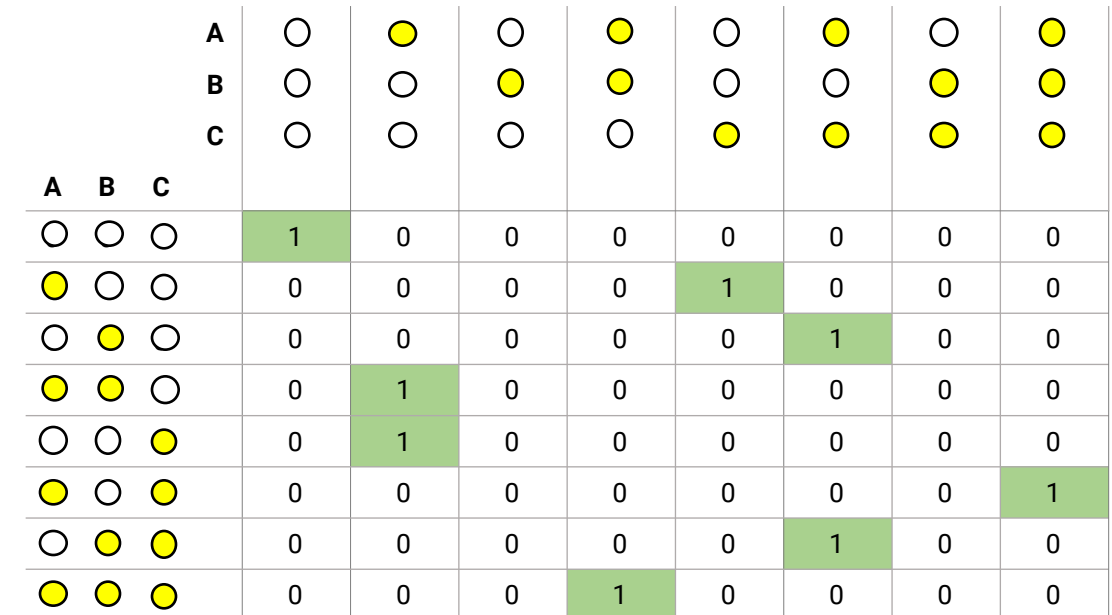 | 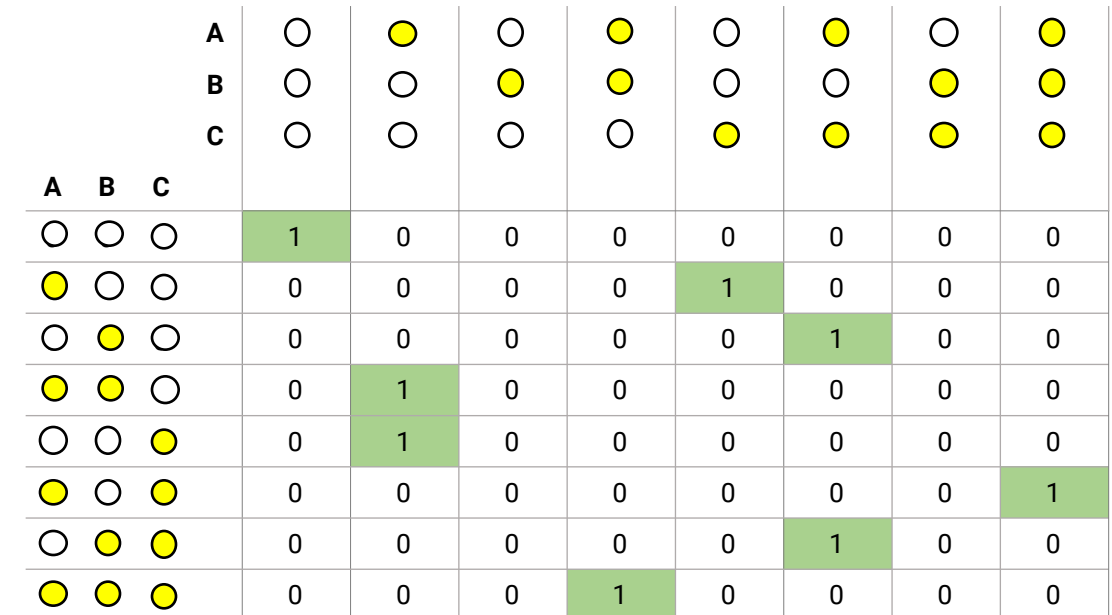 |          | 0                                                                                   | 0                                                                                   | 0                                                                                   | 0                                                                                   | 0                                                                                   | 0                                                                                   | 0                                                                                   | 1                                                                                   |
| 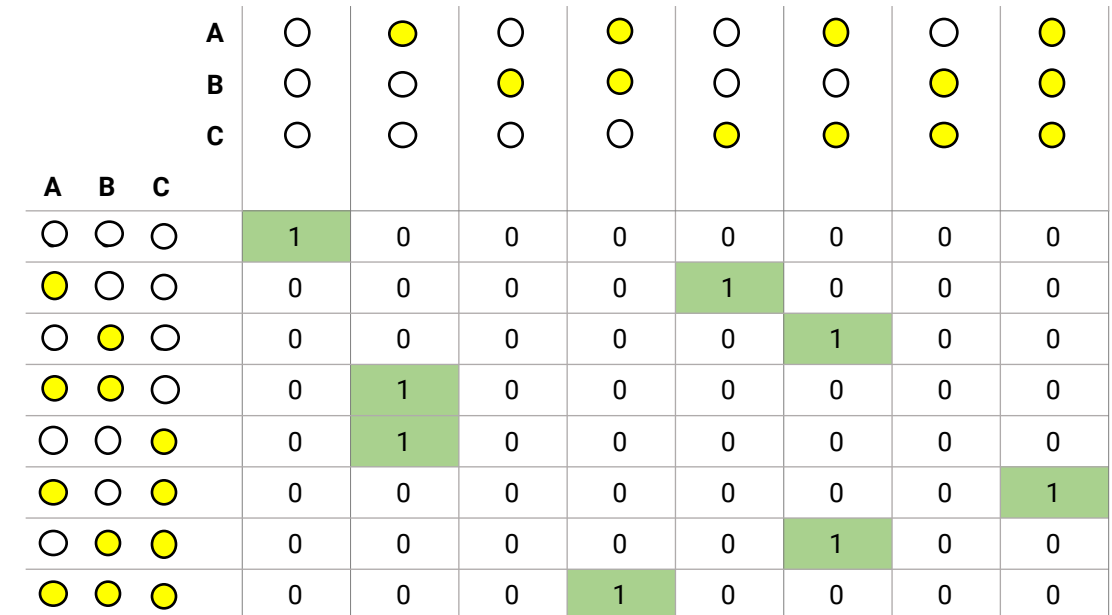 | 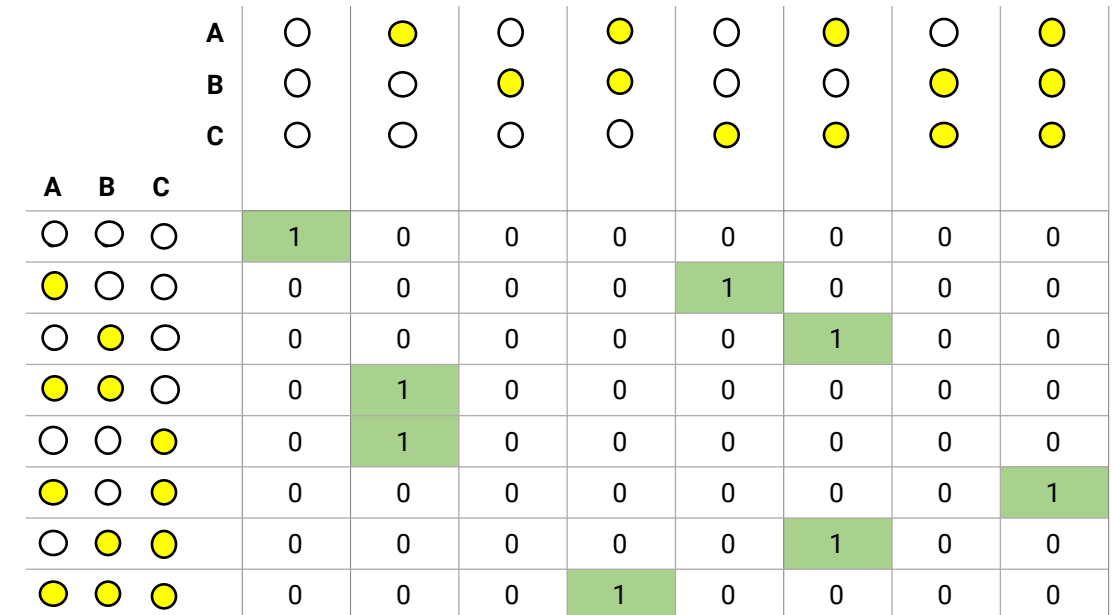 | 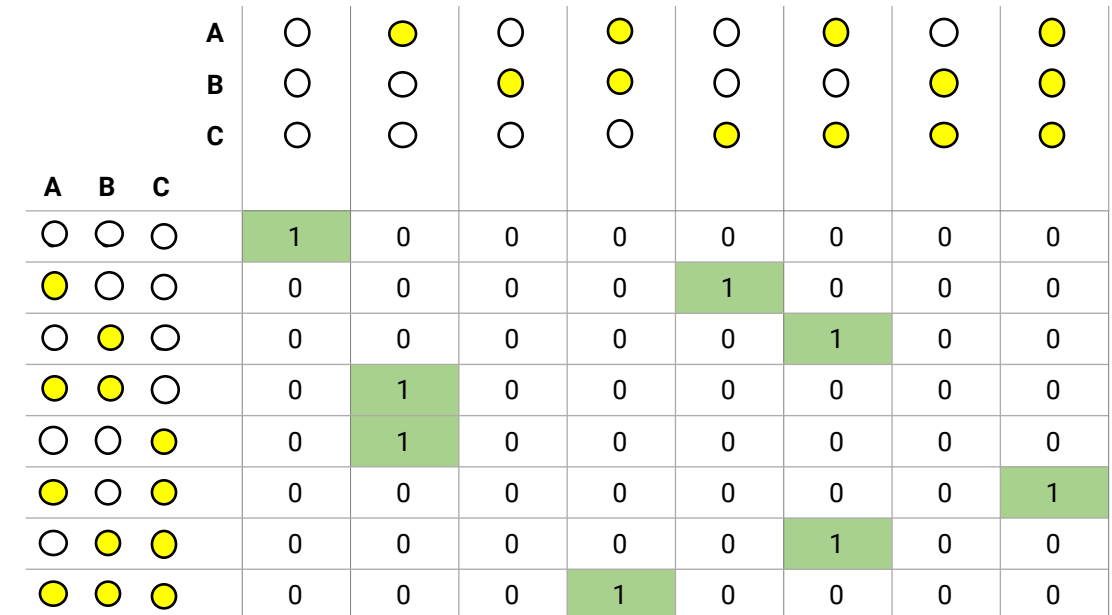 |          | 0                                                                                   | 0                                                                                   | 0                                                                                   | 0                                                                                   | 0                                                                                   | 1                                                                                   | 0                                                                                   | 0                                                                                   |
| 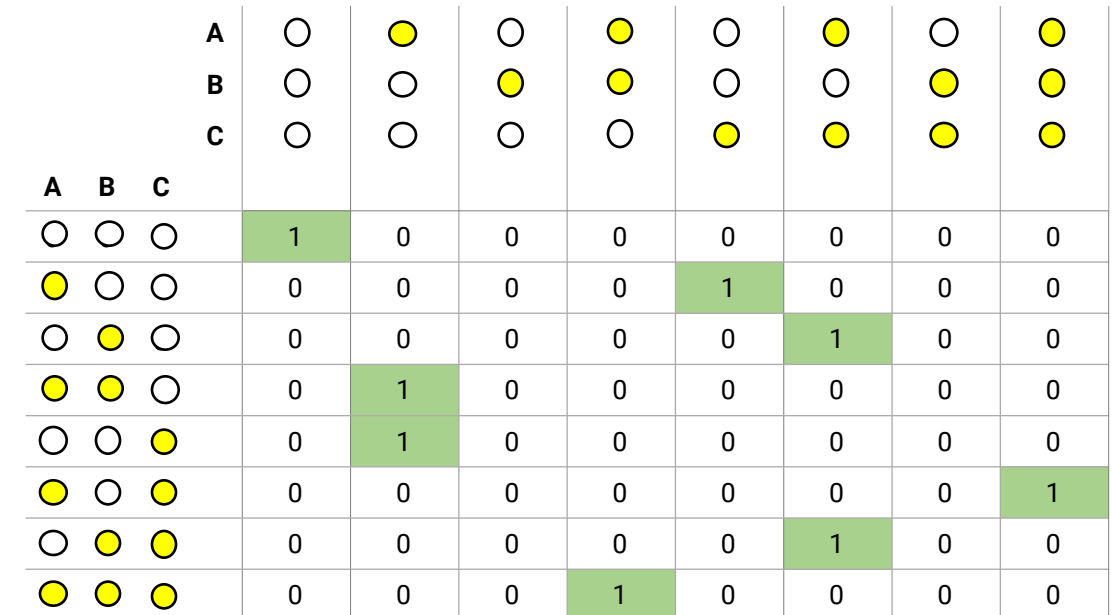 | 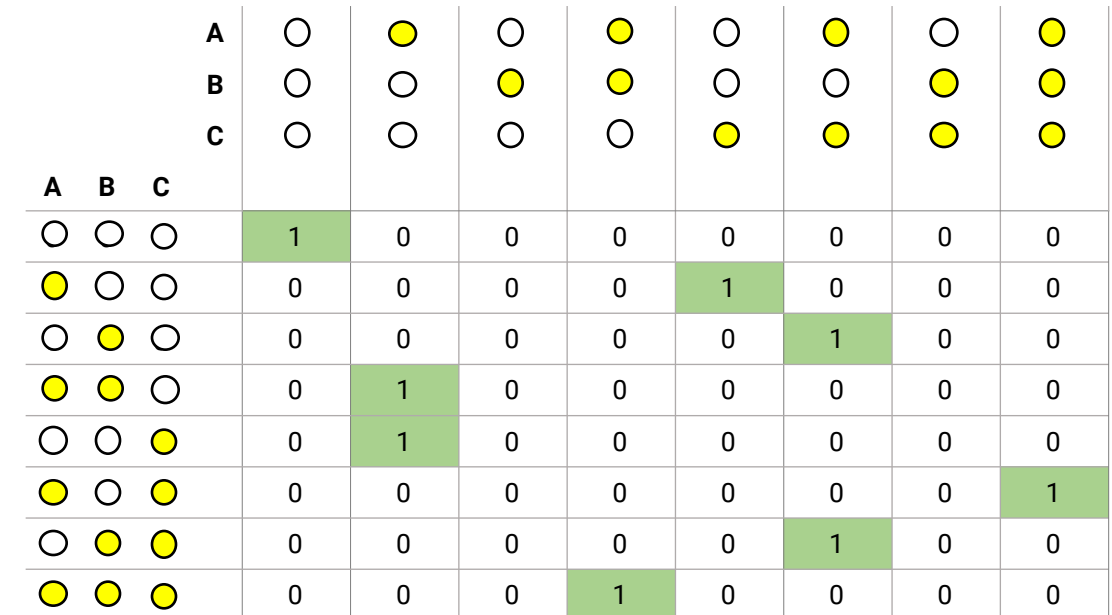 | 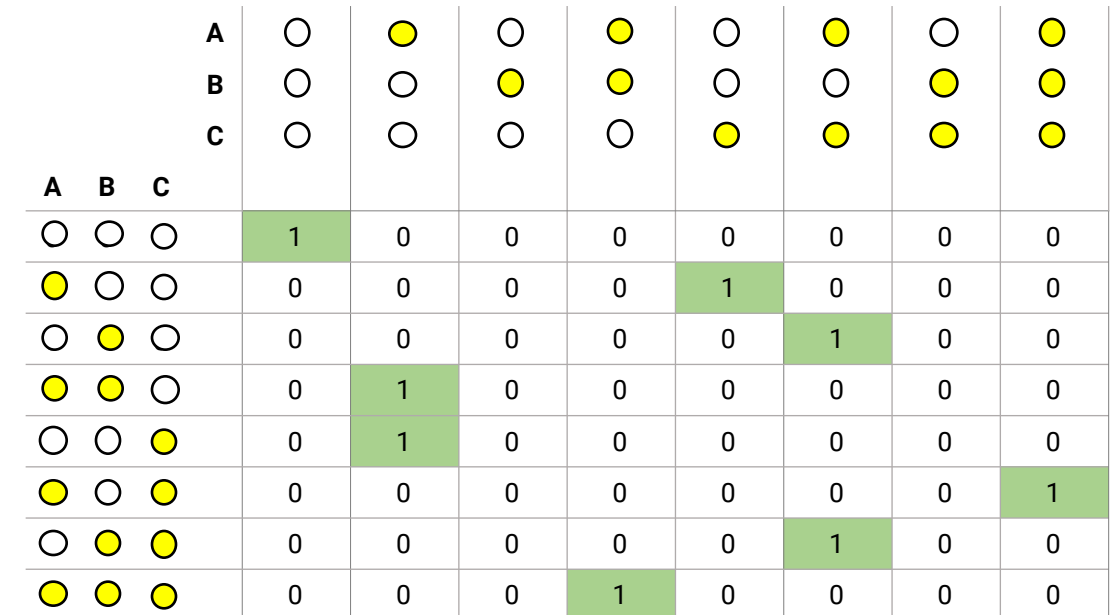 |          | 0                                                                                   | 0                                                                                   | 0                                                                                   | 1                                                                                   | 0                                                                                   | 0                                                                                   | 0                                                                                   | 0                                                                                   |

# Marginalization

- [illegible]

|                                                                                       |                                                                                       |                                                                                       |          |                                                                                     |                                                                                     |                                                                                     |                                                                                     |                                                                                     |                                                                                     |                                                                                     |                                                                                     |
|---------------------------------------------------------------------------------------|---------------------------------------------------------------------------------------|---------------------------------------------------------------------------------------|----------|-------------------------------------------------------------------------------------|-------------------------------------------------------------------------------------|-------------------------------------------------------------------------------------|-------------------------------------------------------------------------------------|-------------------------------------------------------------------------------------|-------------------------------------------------------------------------------------|-------------------------------------------------------------------------------------|-------------------------------------------------------------------------------------|
|                                                                                       |                                                                                       |                                                                                       | <b>A</b> | 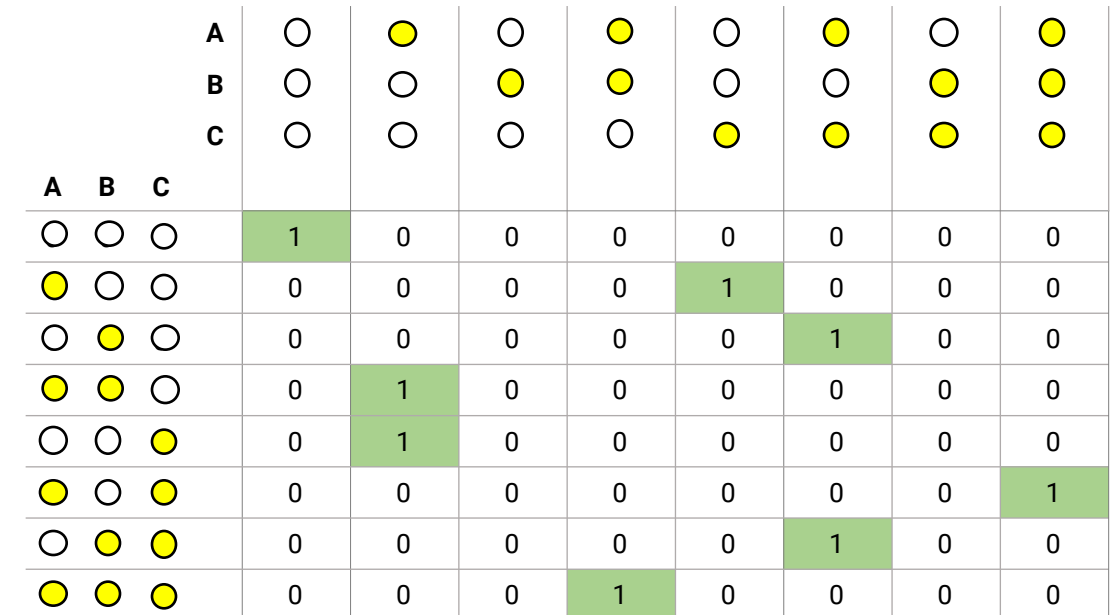 | 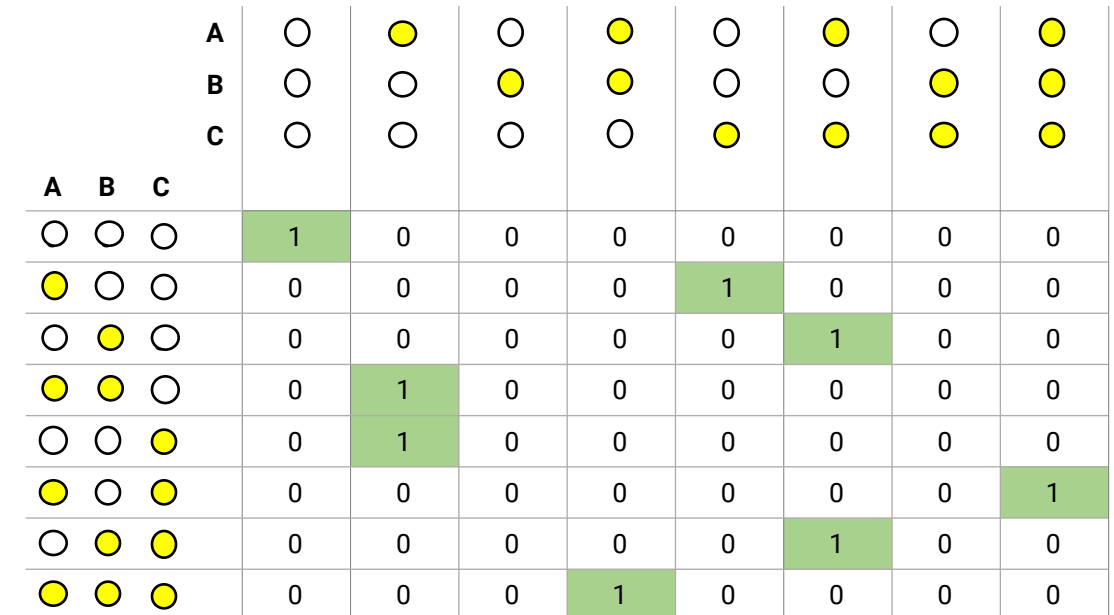 | 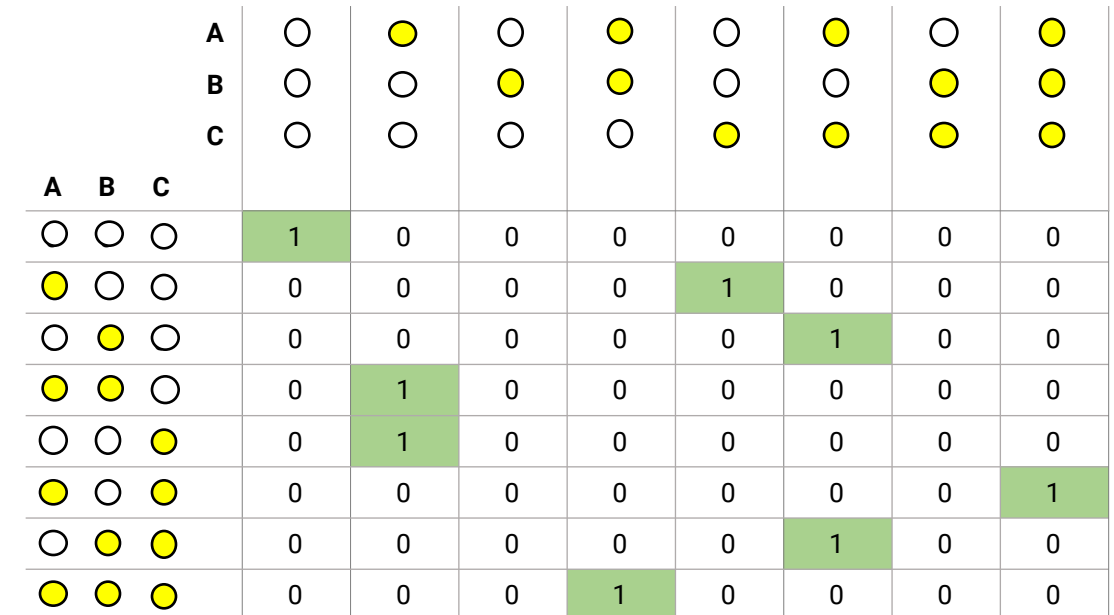 | 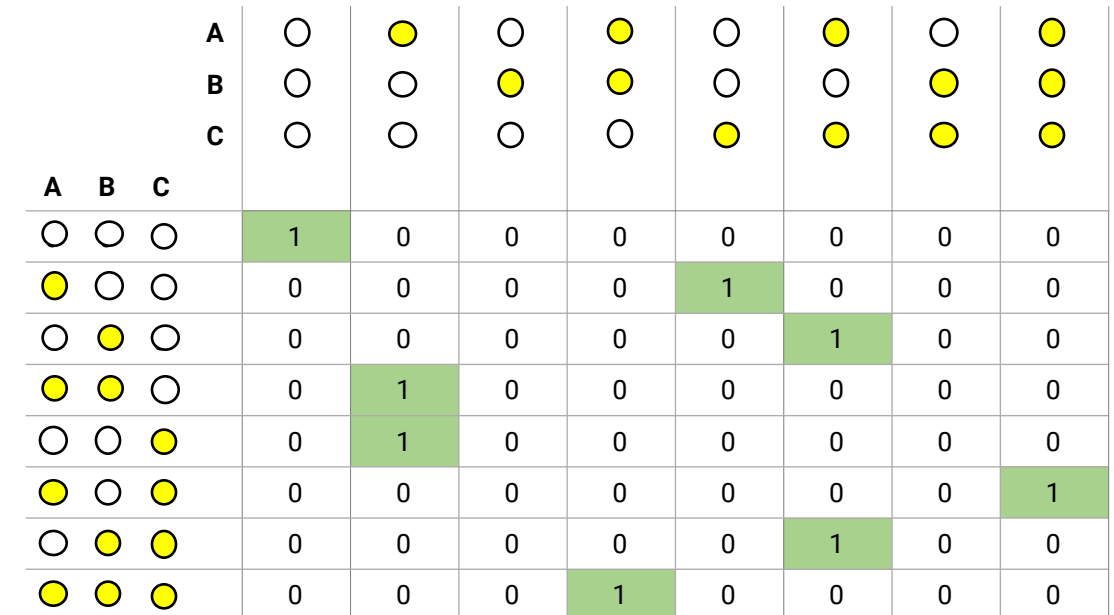 | 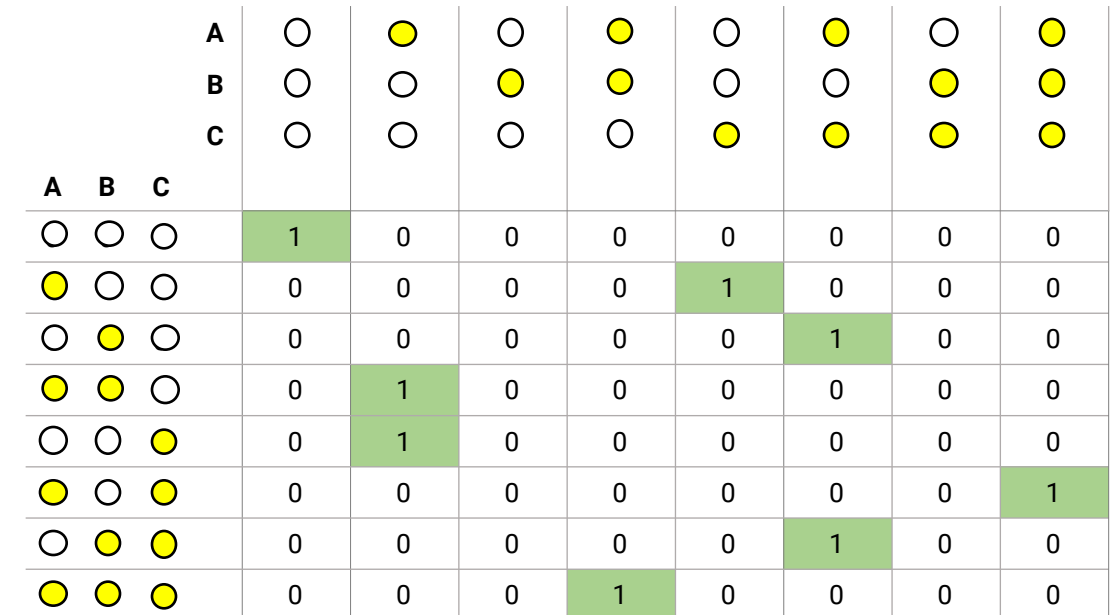 | 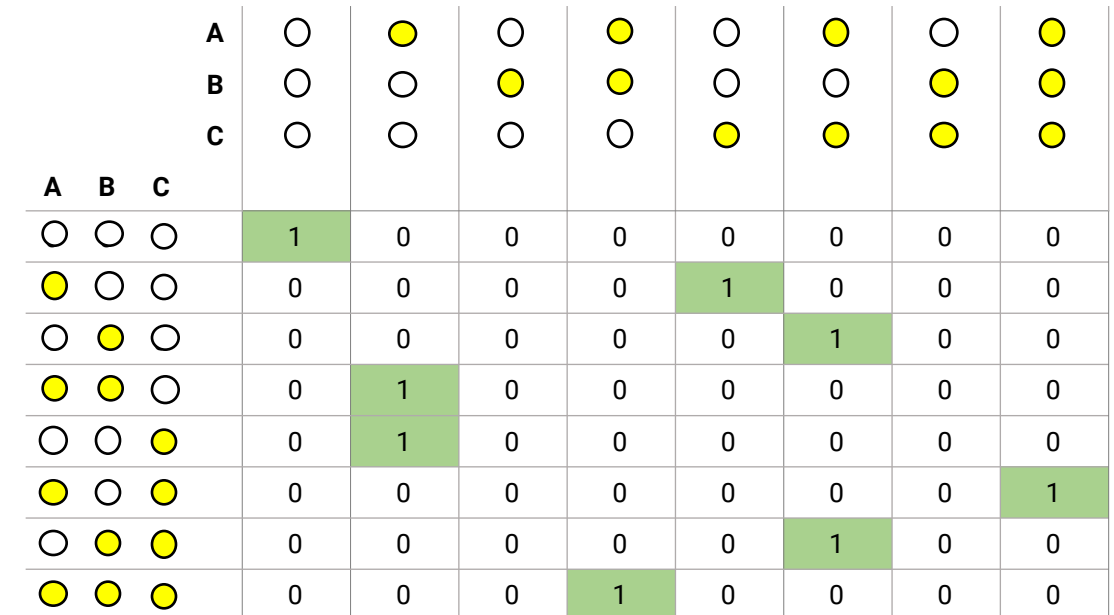 | 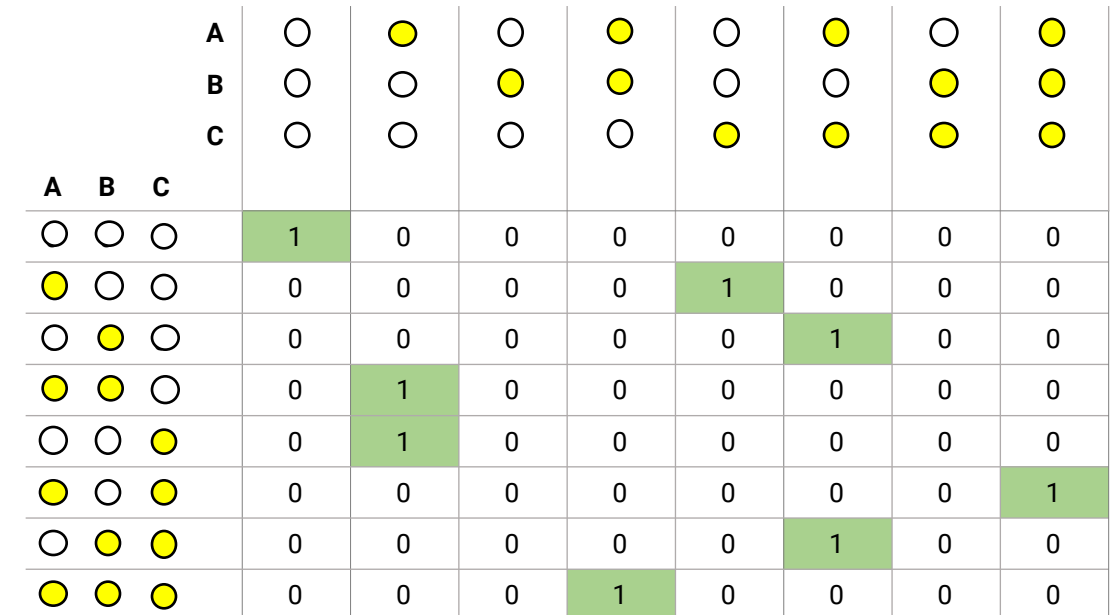 | 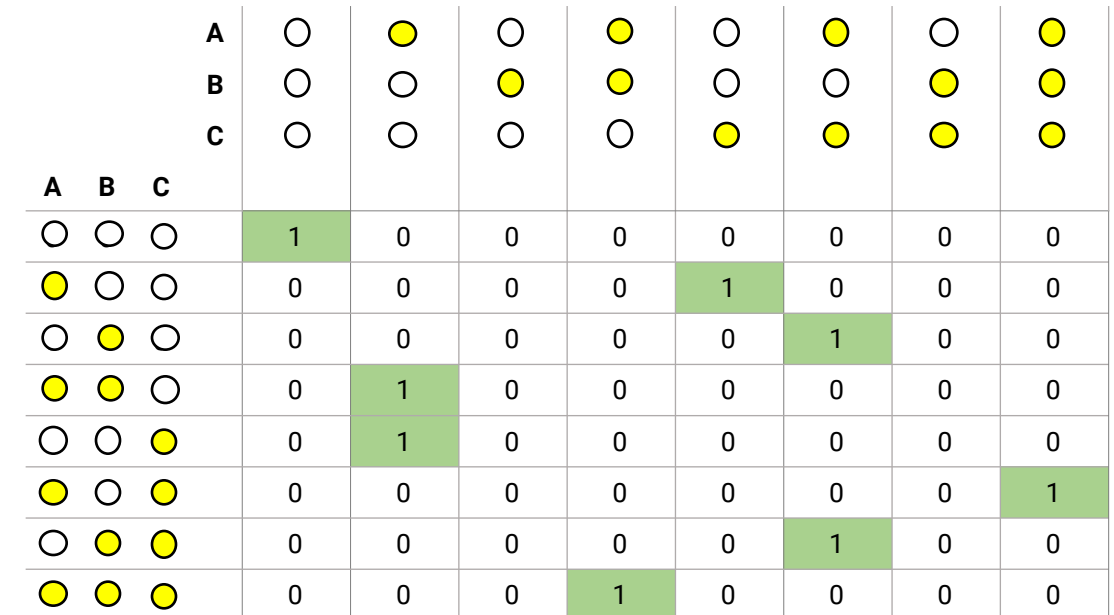 |
|                                                                                       |                                                                                       |                                                                                       | <b>B</b> | 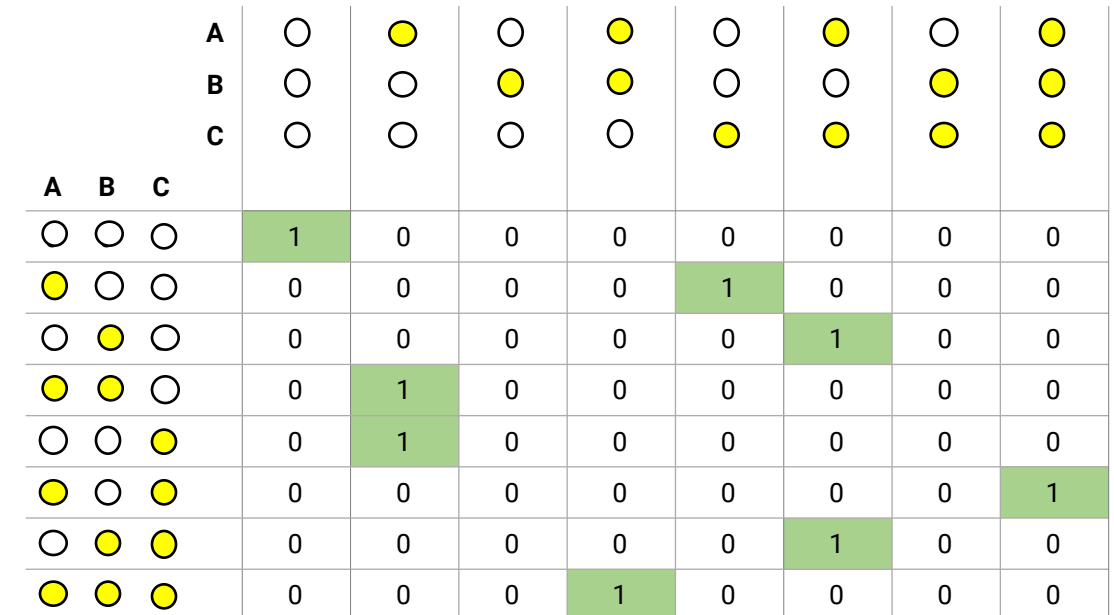 | 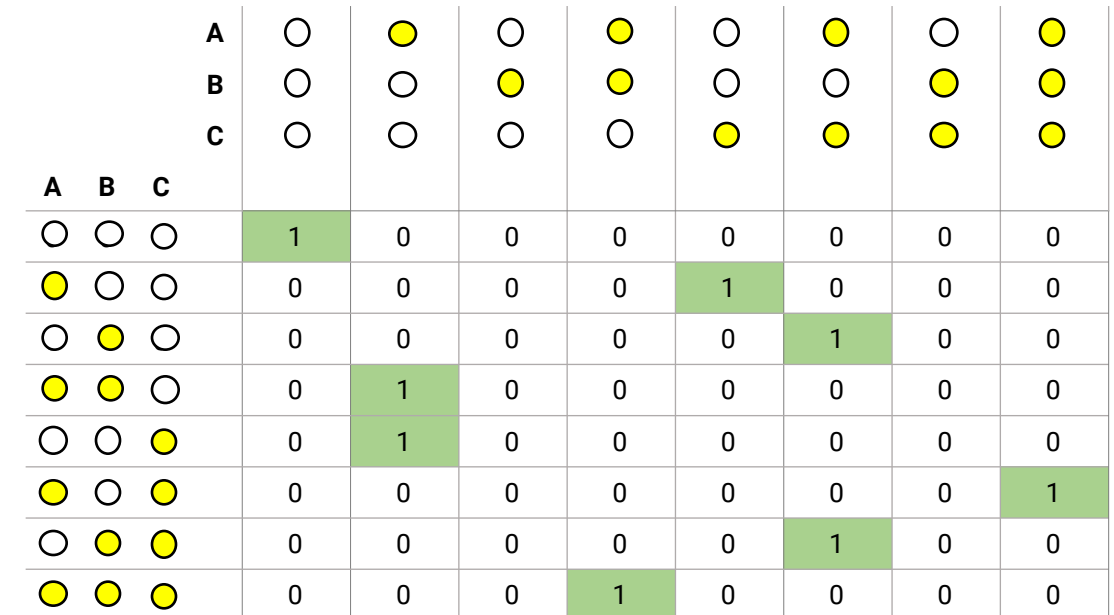 | 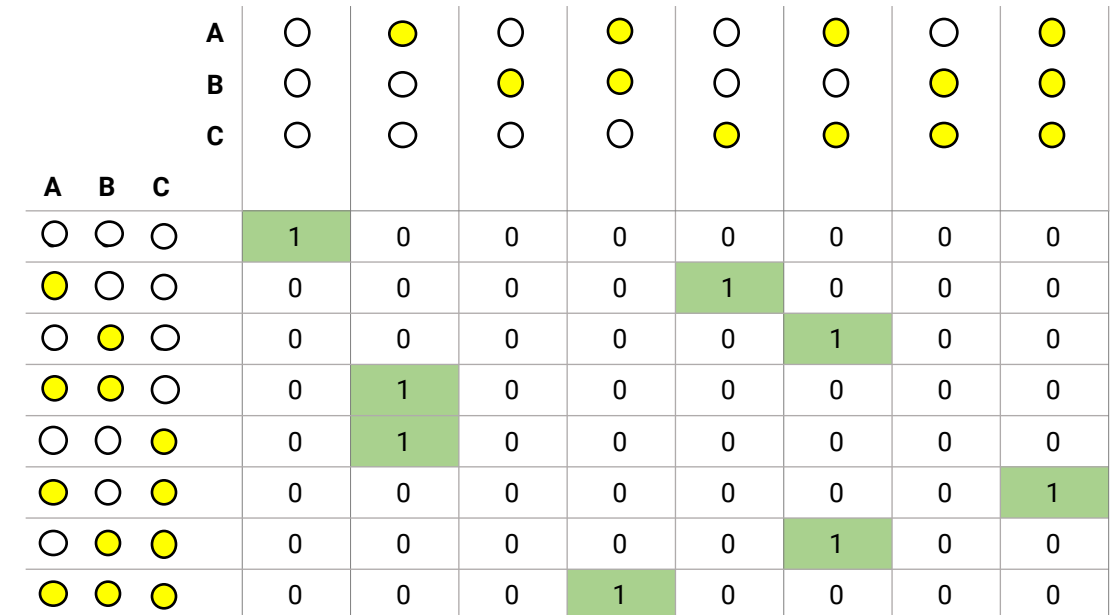 | 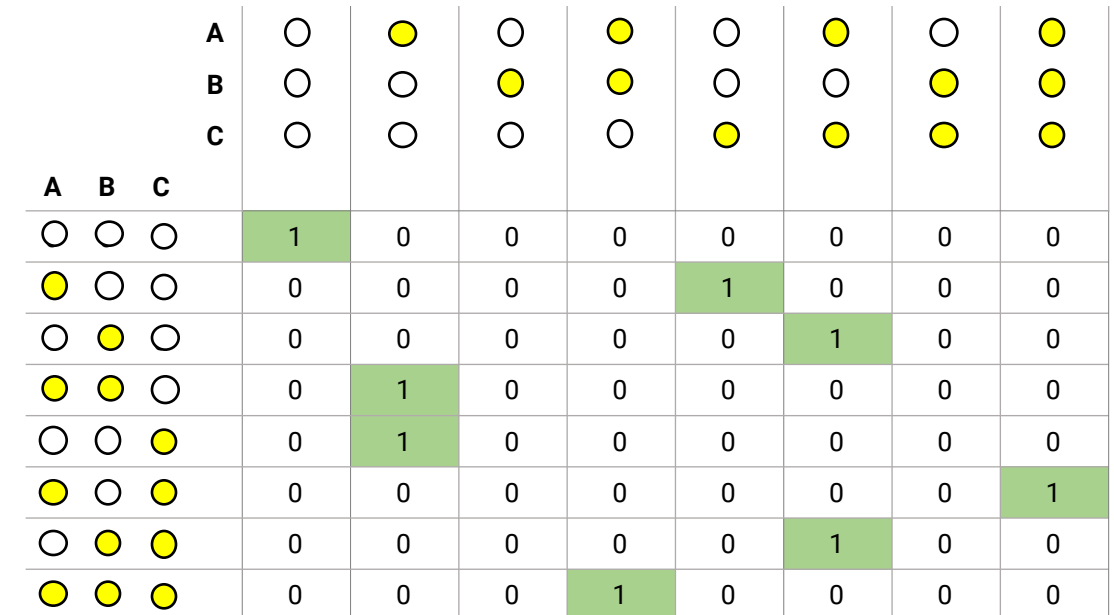 | 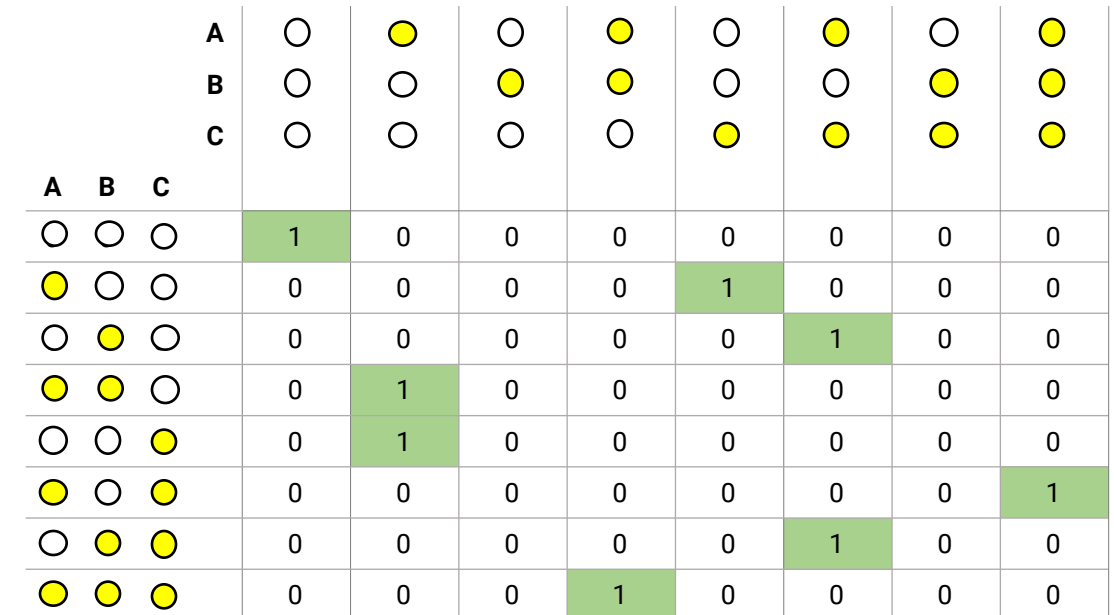 | 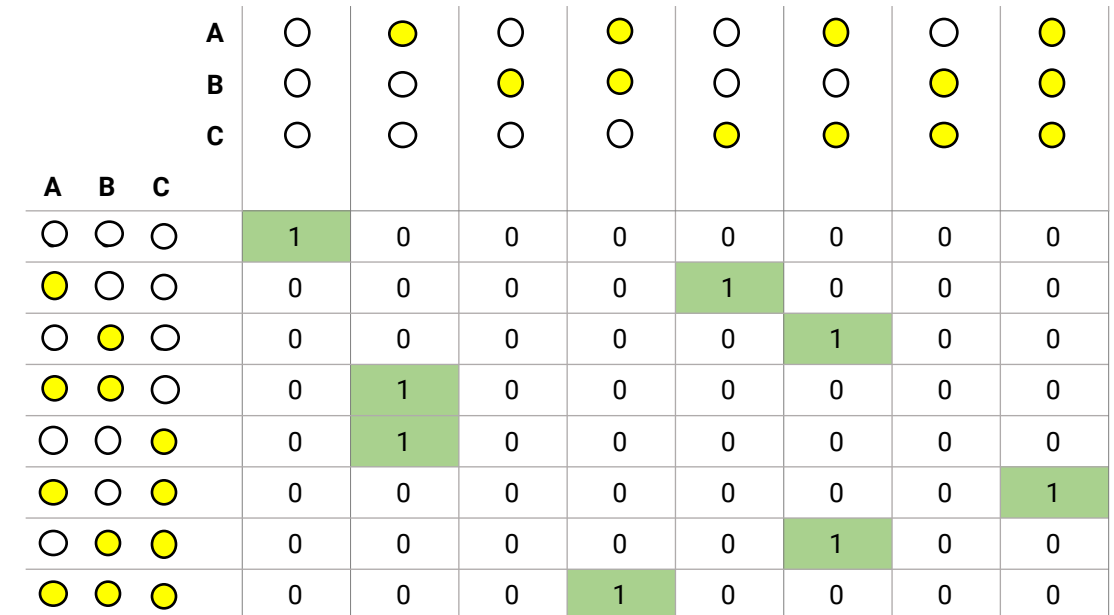 | 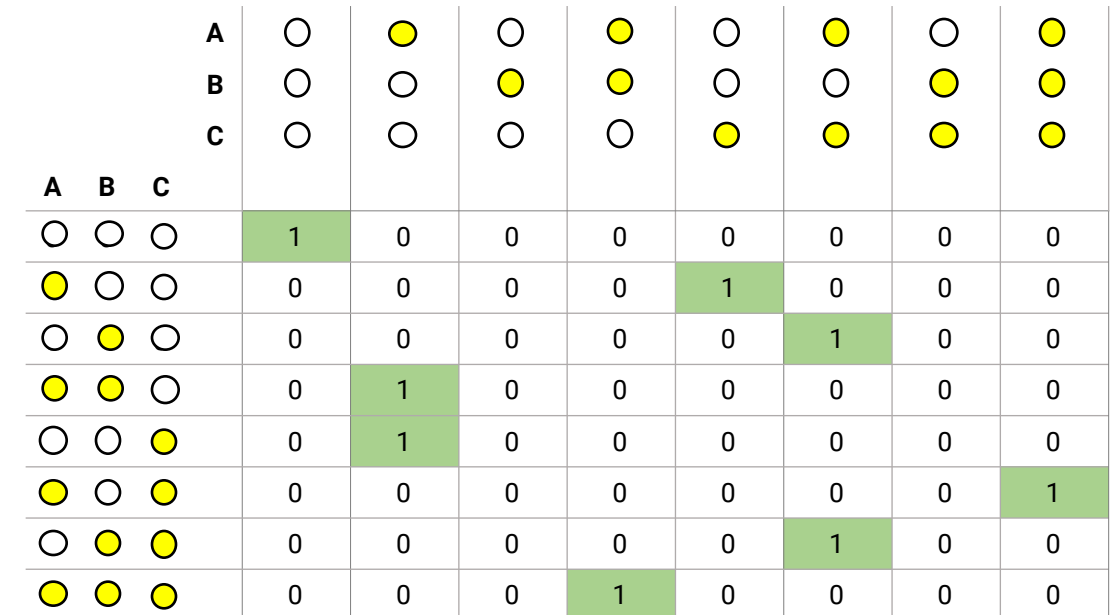 | 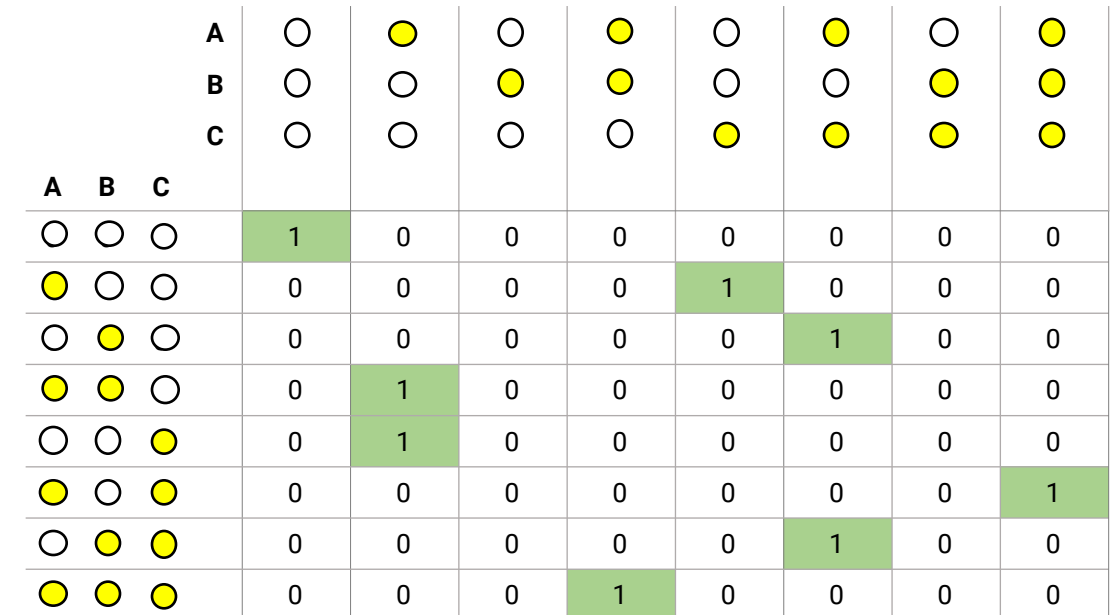 |
|                                                                                       |                                                                                       |                                                                                       | <b>C</b> | 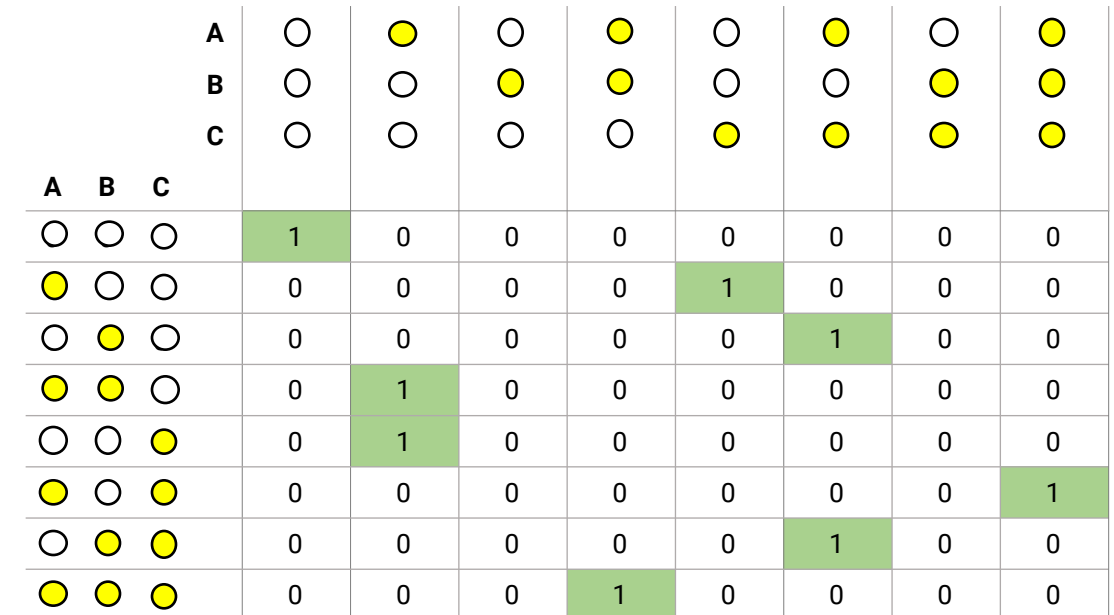 | 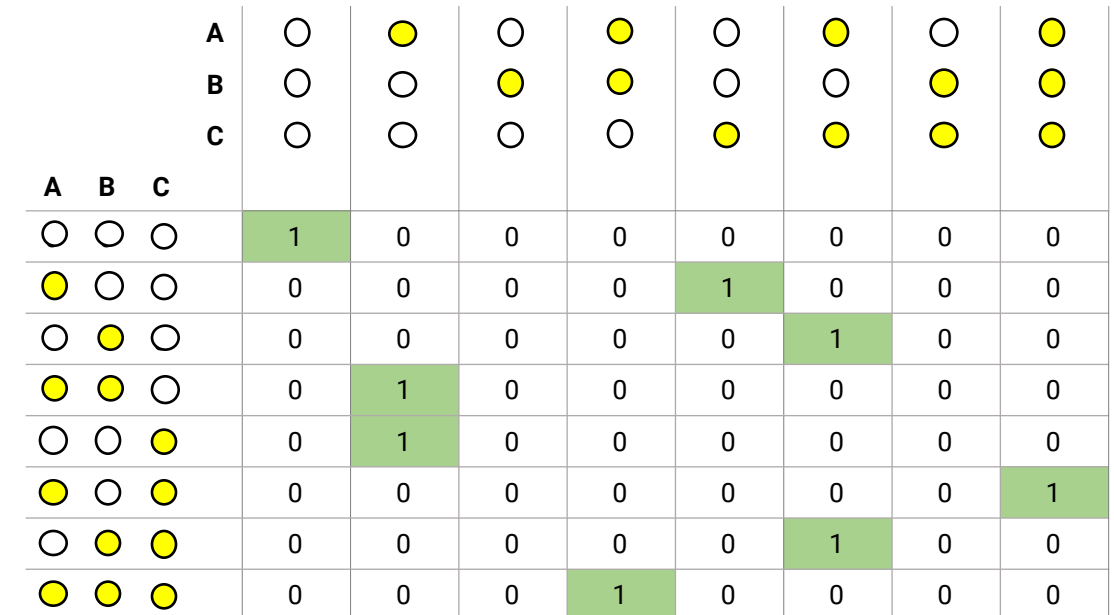 | 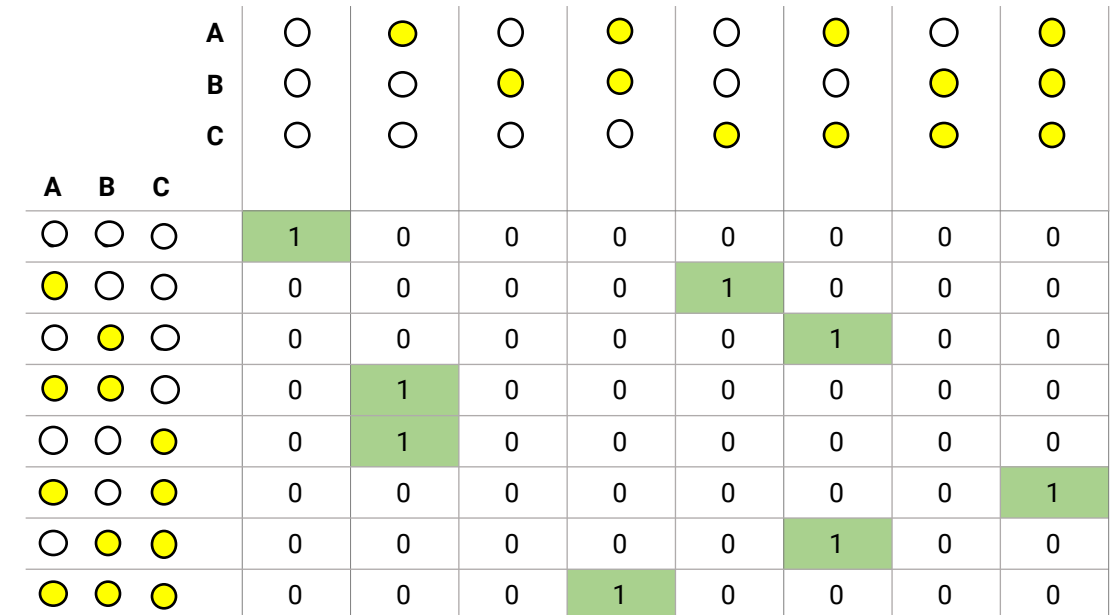 | 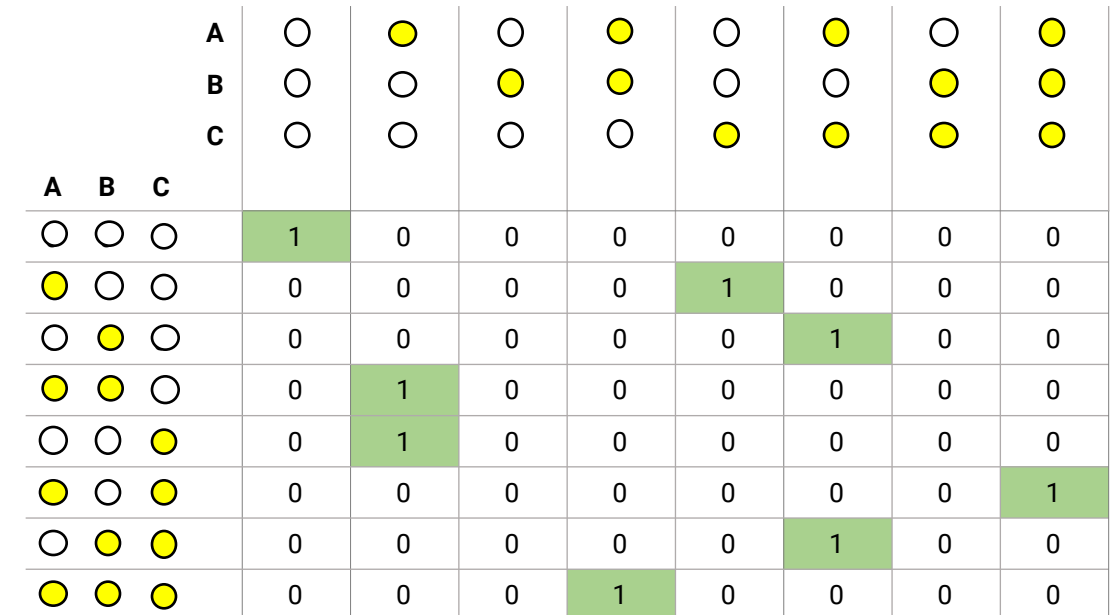 | 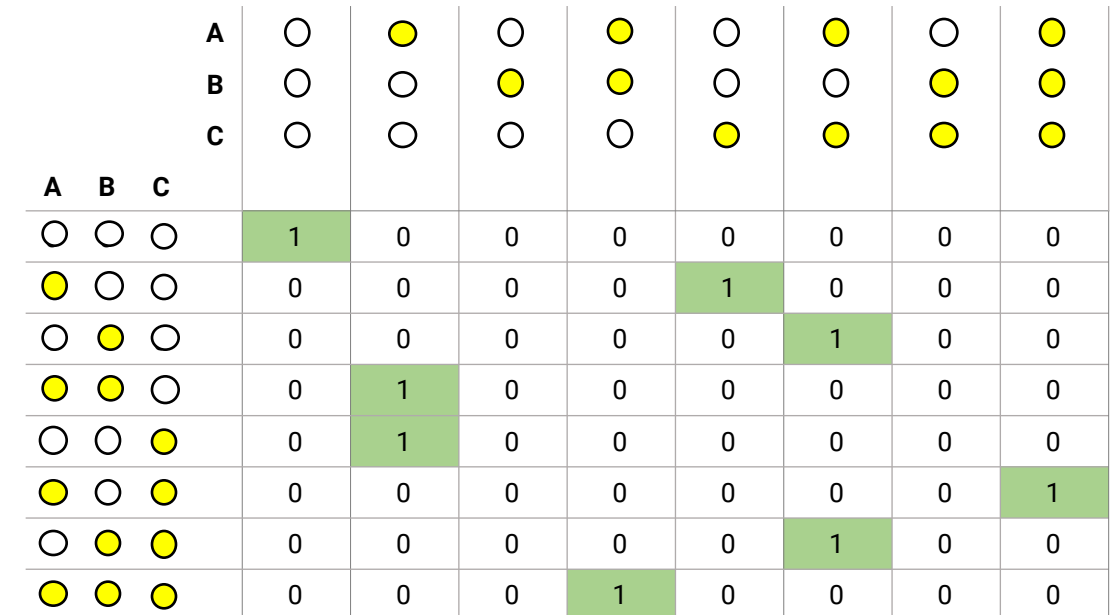 | 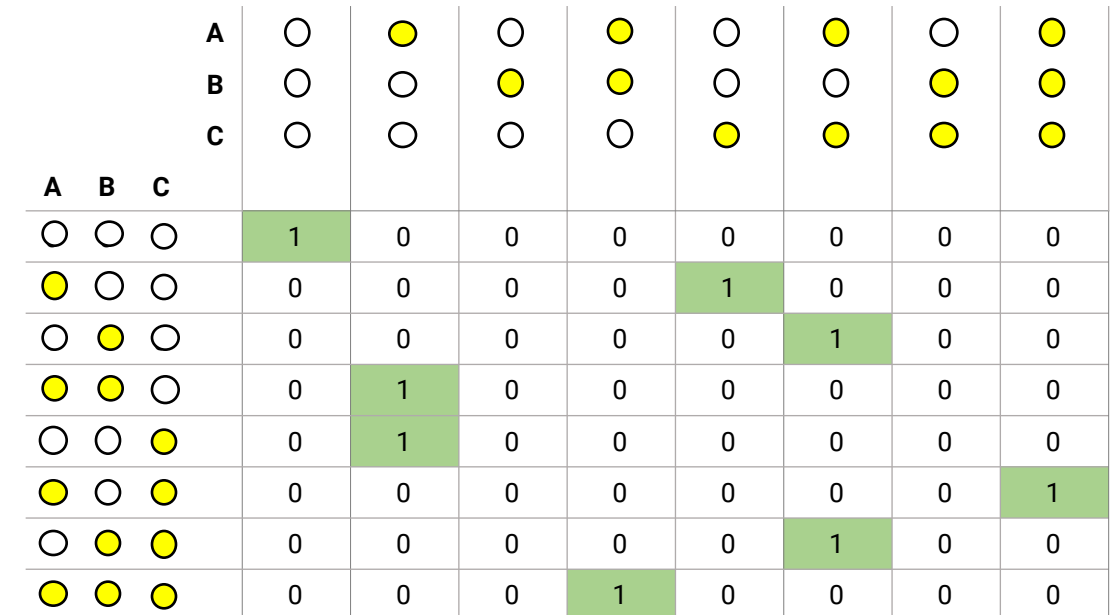 | 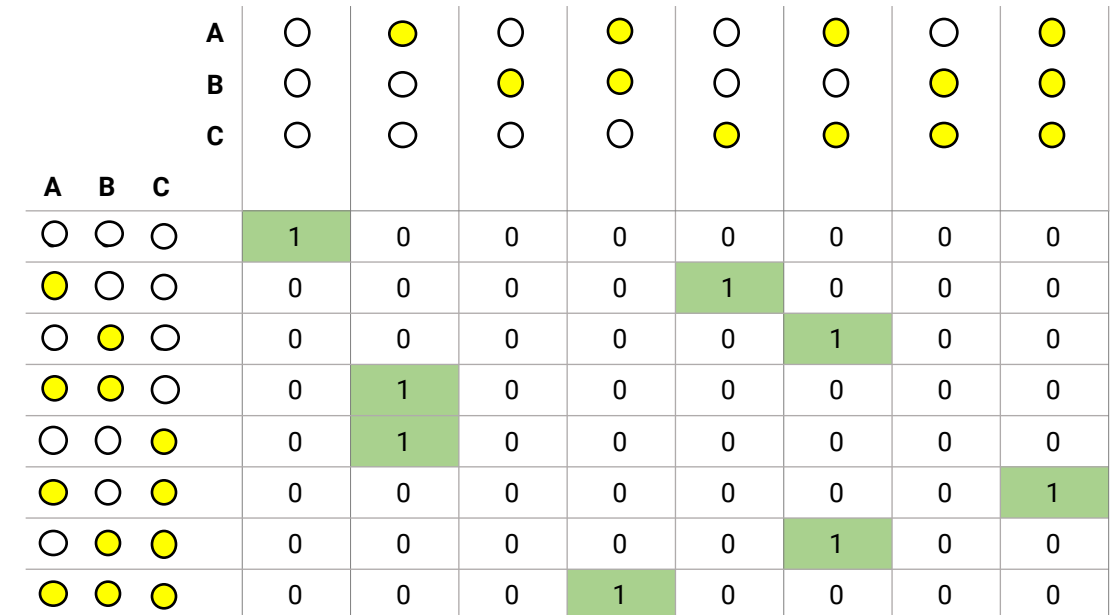 | 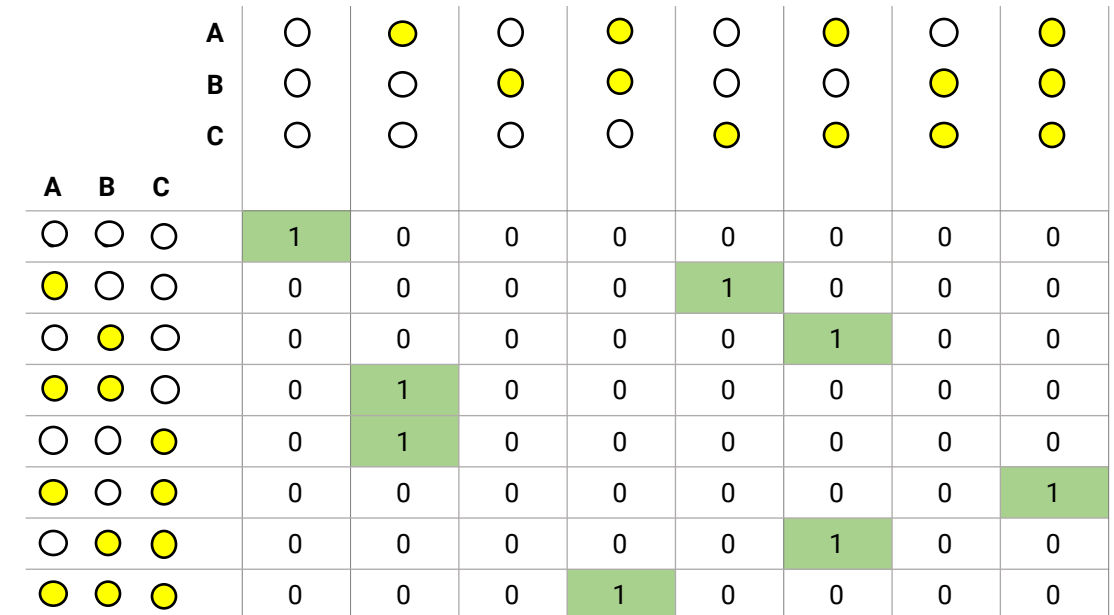 |
| <b>A</b>                                                                              | <b>B</b>                                                                              | <b>C</b>                                                                              |          |                                                                                     |                                                                                     |                                                                                     |                                                                                     |                                                                                     |                                                                                     |                                                                                     |                                                                                     |
| 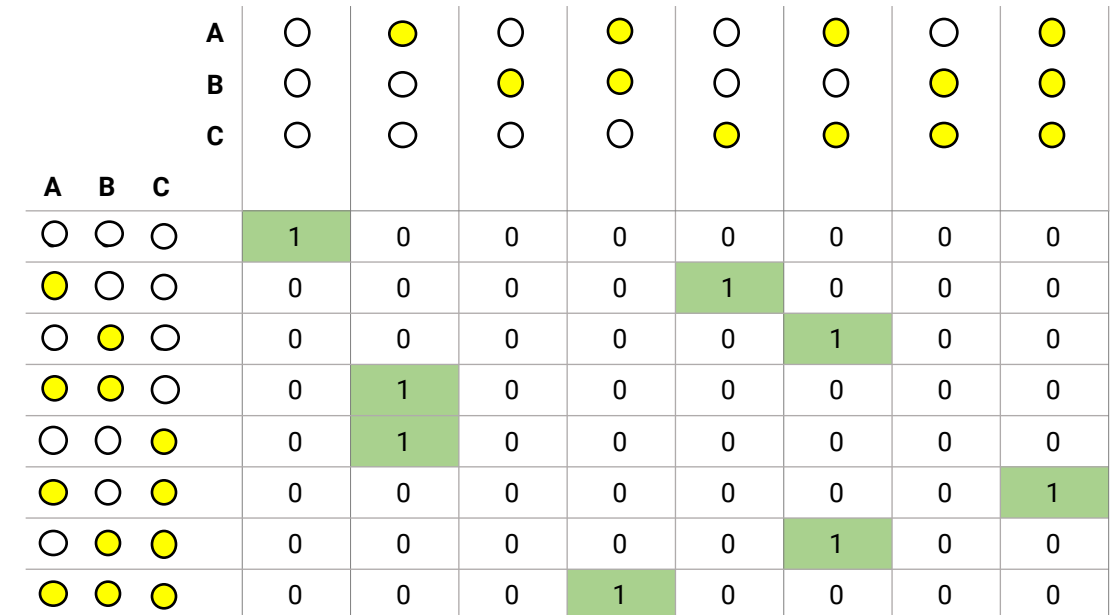  | 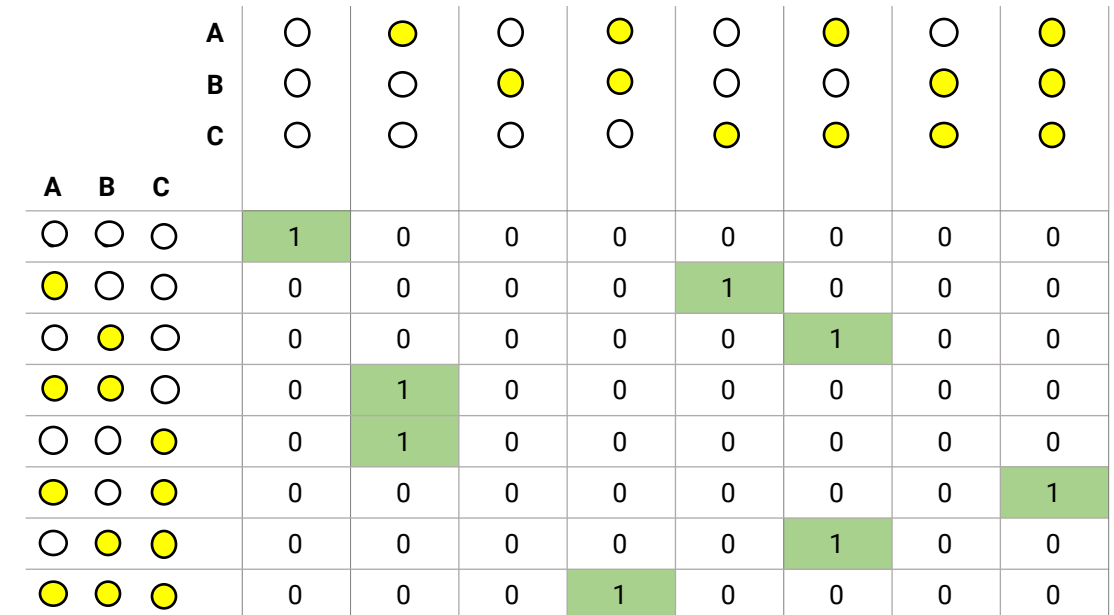  | 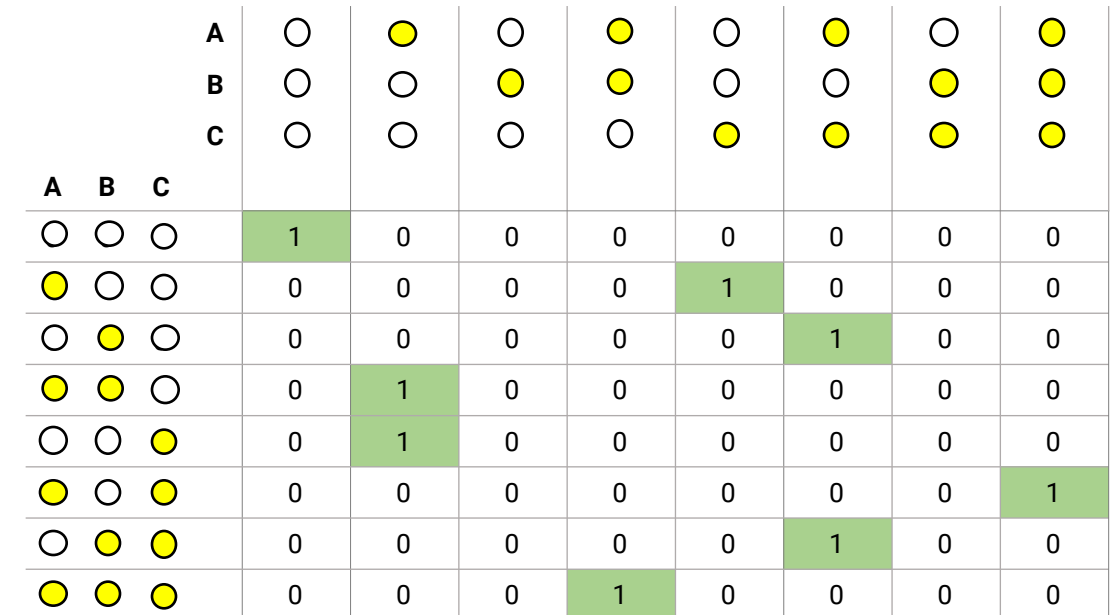  |          | 1                                                                                   | 0                                                                                   | 0                                                                                   | 0                                                                                   | 0                                                                                   | 0                                                                                   | 0                                                                                   | 0                                                                                   |
| 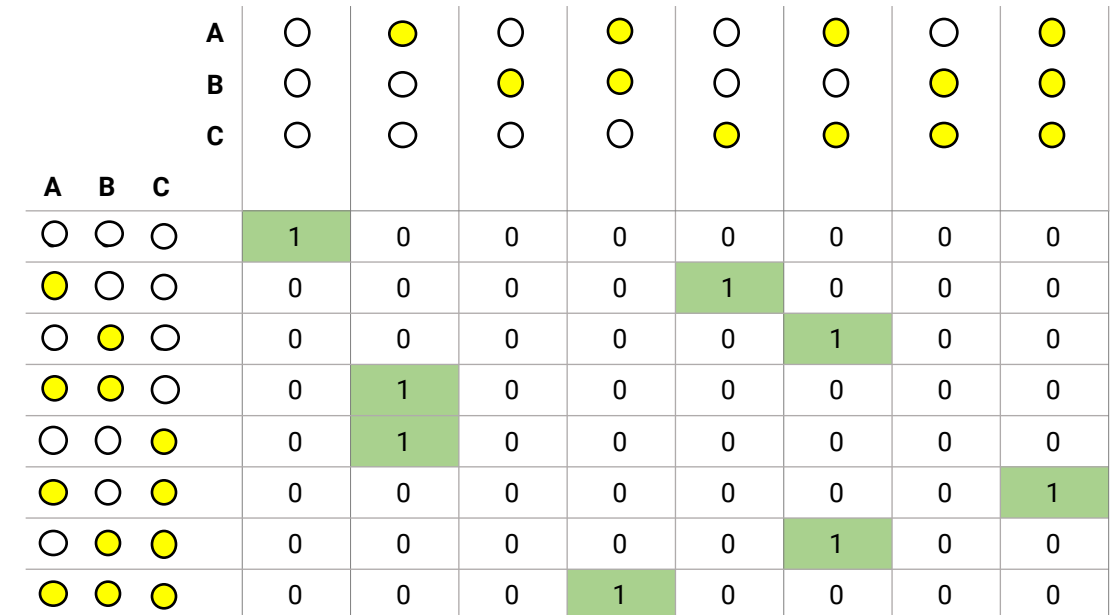 | 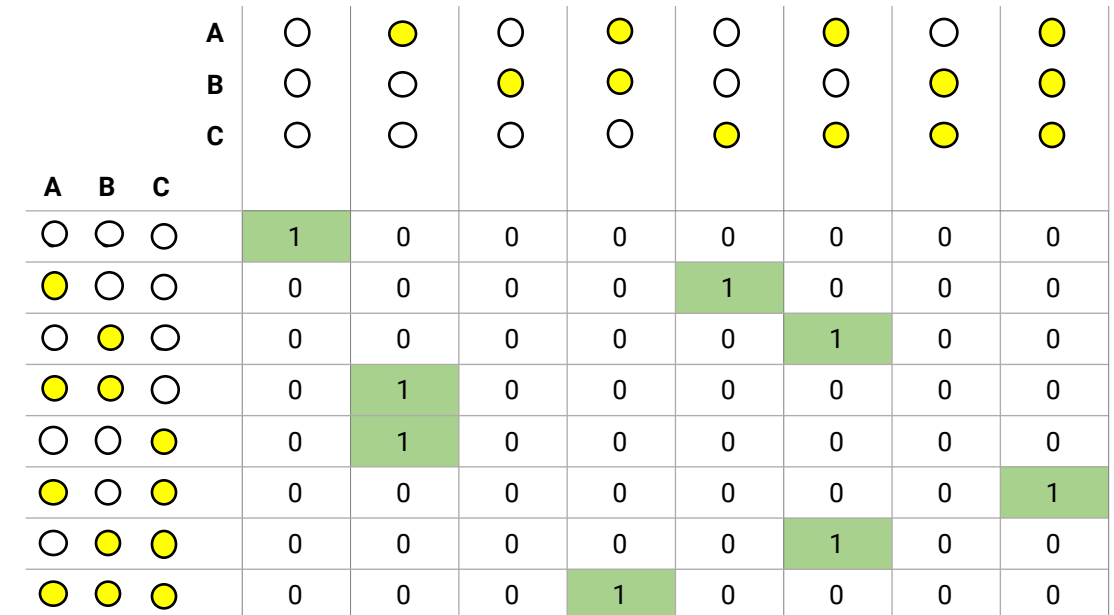 | 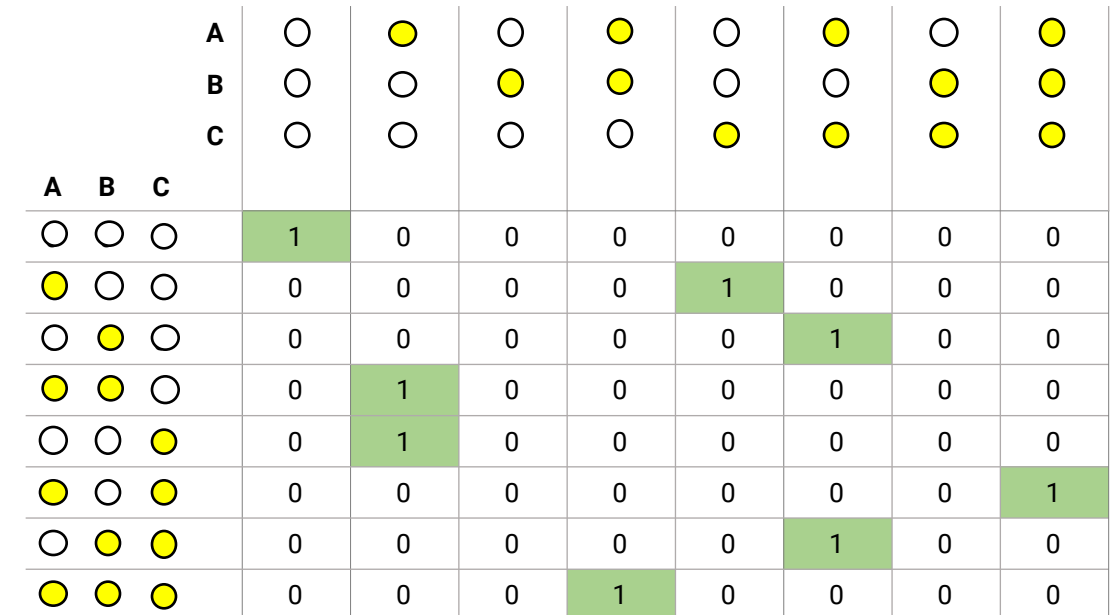 |          | 0                                                                                   | 0                                                                                   | 0                                                                                   | 0                                                                                   | 1                                                                                   | 0                                                                                   | 0                                                                                   | 0                                                                                   |
| 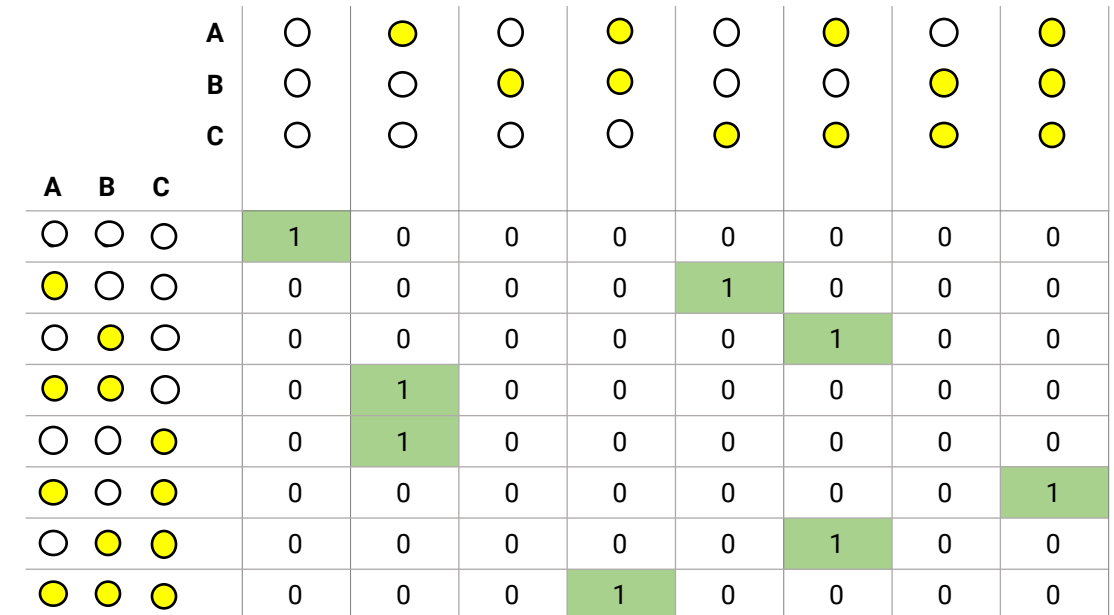 | 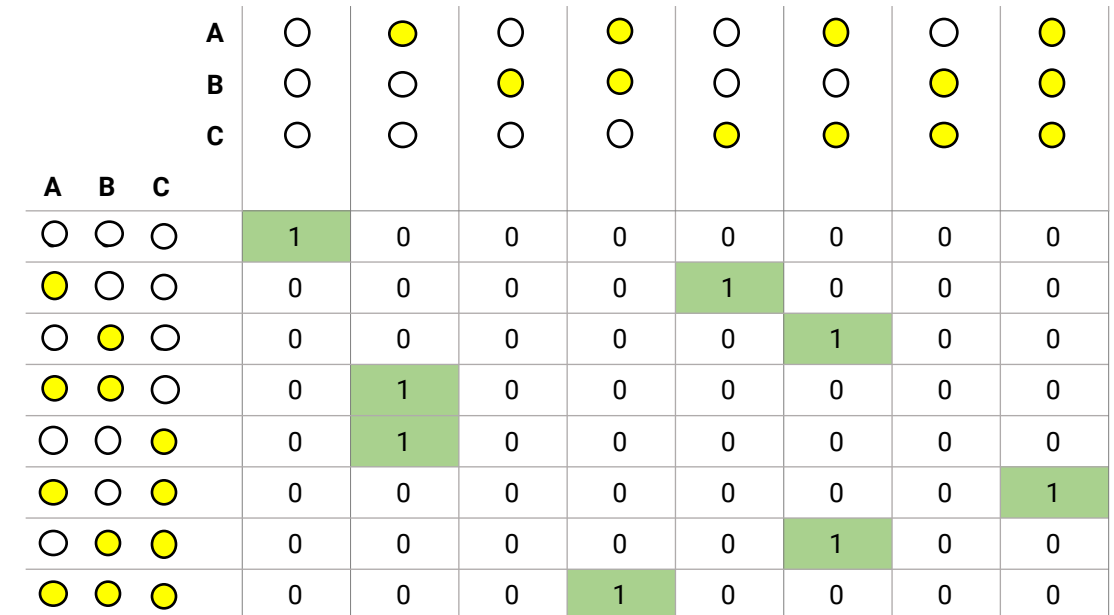 | 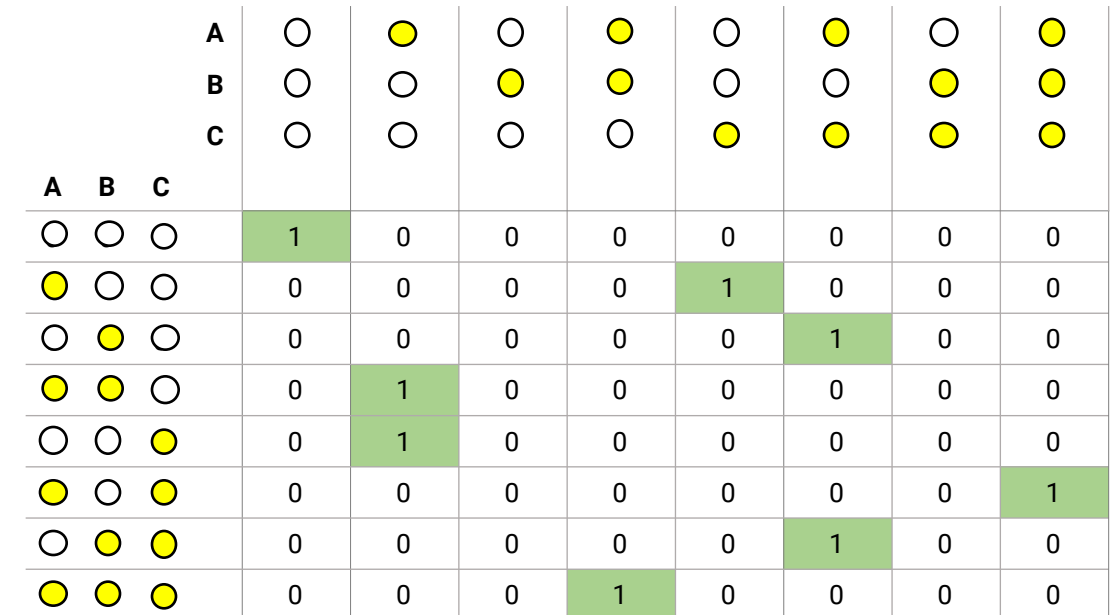 |          | 0                                                                                   | 0                                                                                   | 0                                                                                   | 0                                                                                   | 0                                                                                   | 1                                                                                   | 0                                                                                   | 0                                                                                   |
| 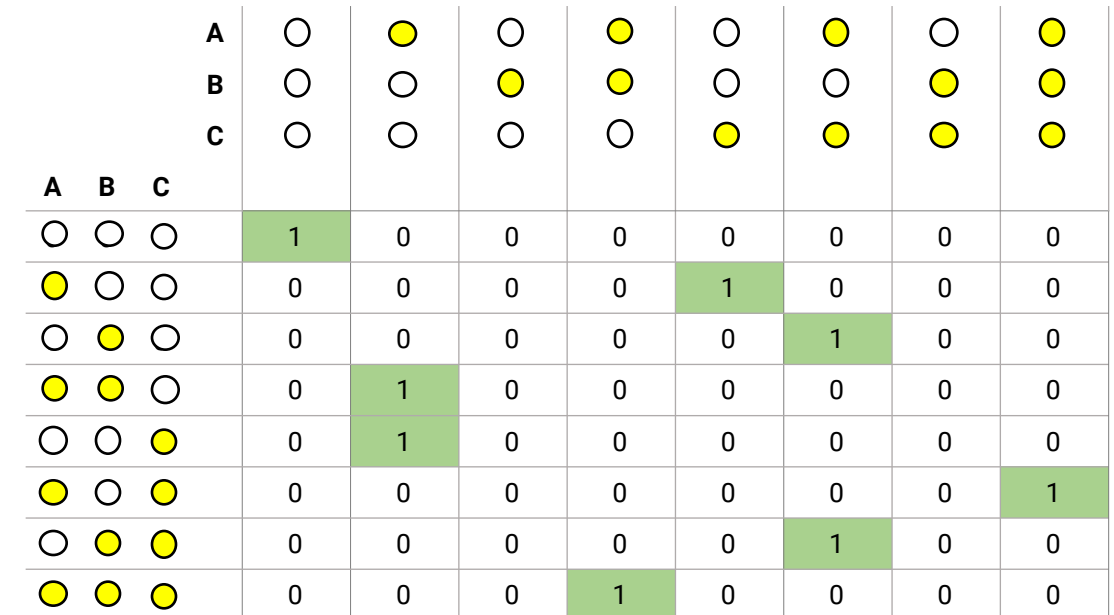 | 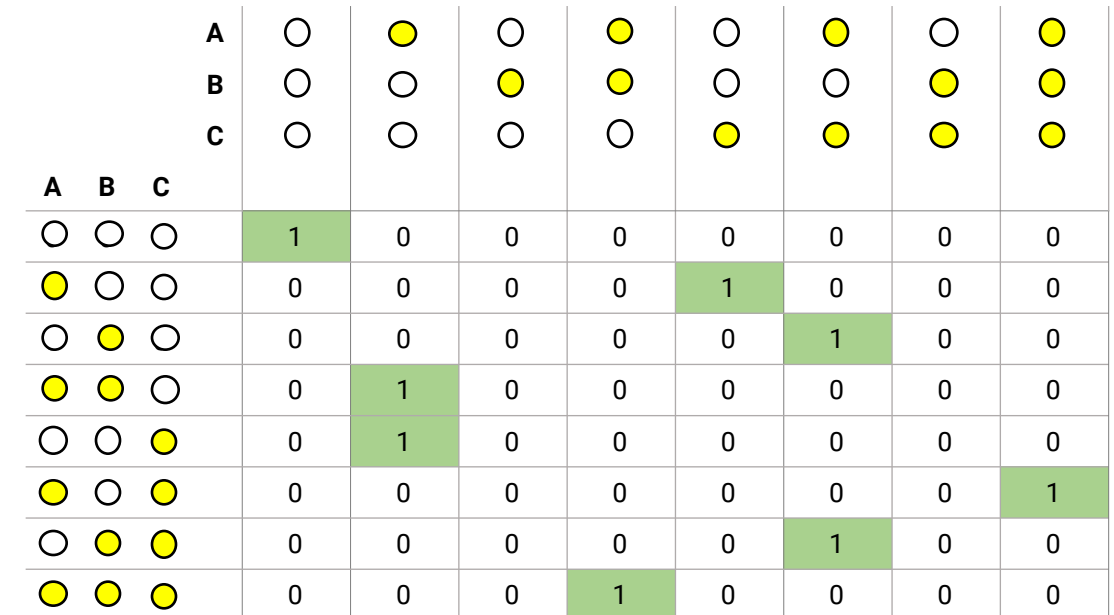 | 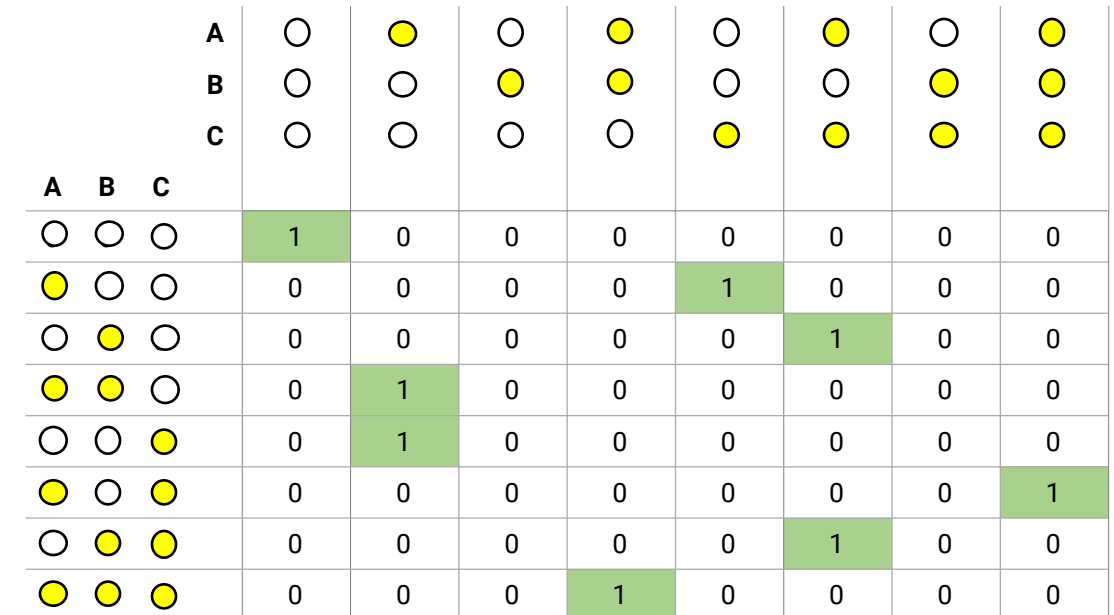 |          | 0                                                                                   | 1                                                                                   | 0                                                                                   | 0                                                                                   | 0                                                                                   | 0                                                                                   | 0                                                                                   | 0                                                                                   |
| 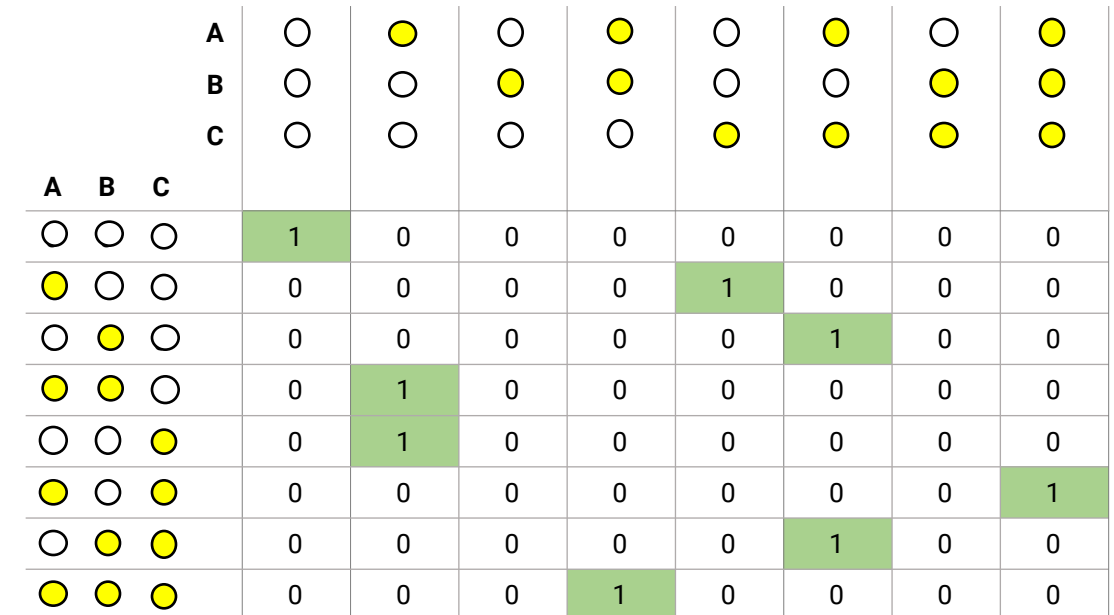 | 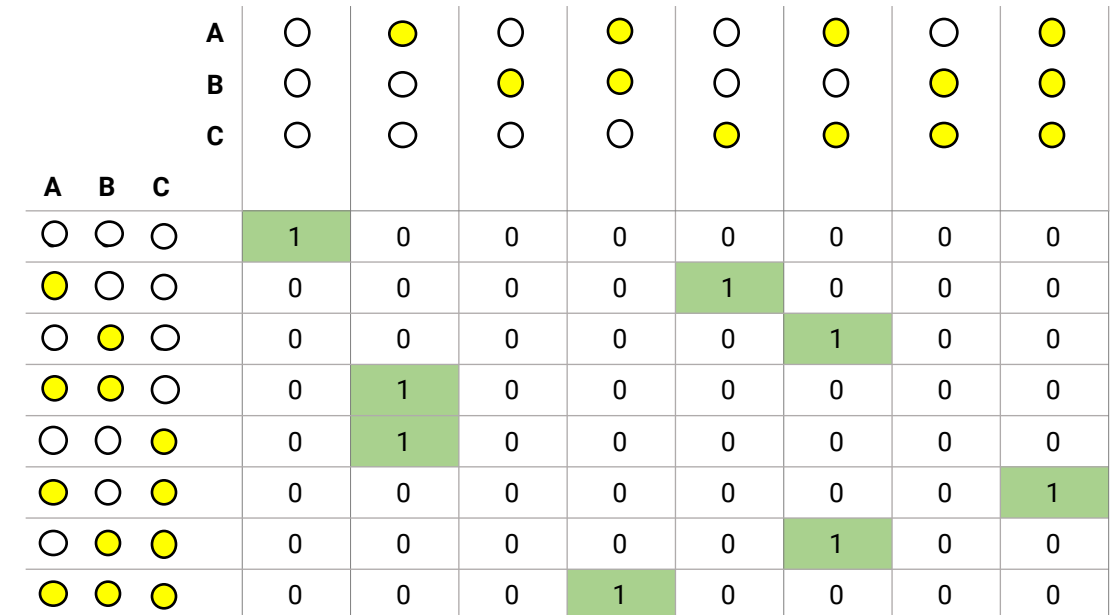 | 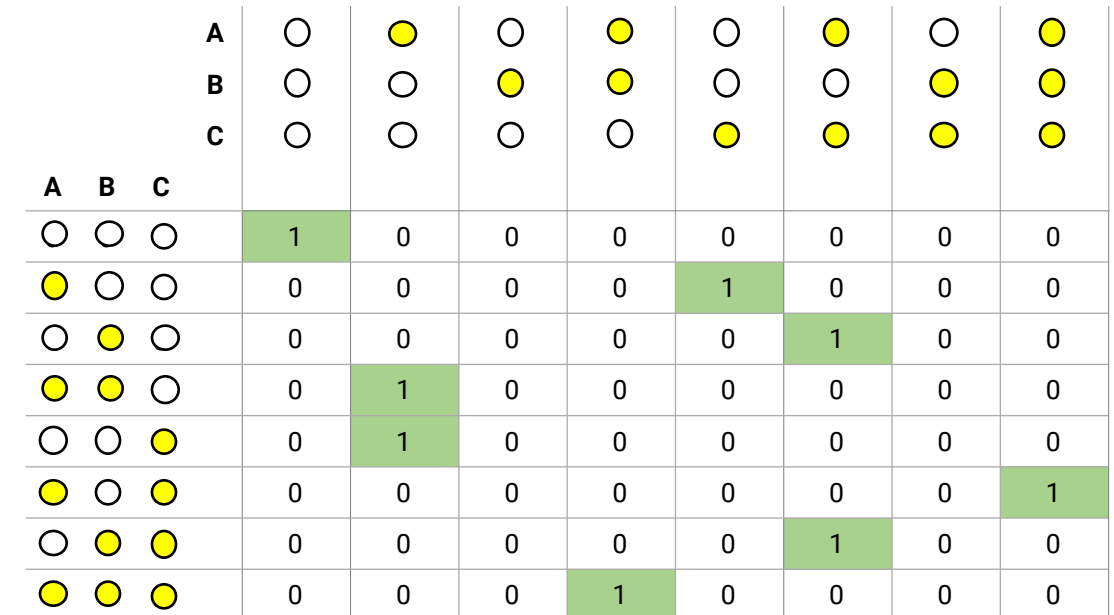 |          | 0                                                                                   | 1                                                                                   | 0                                                                                   | 0                                                                                   | 0                                                                                   | 0                                                                                   | 0                                                                                   | 0                                                                                   |
| 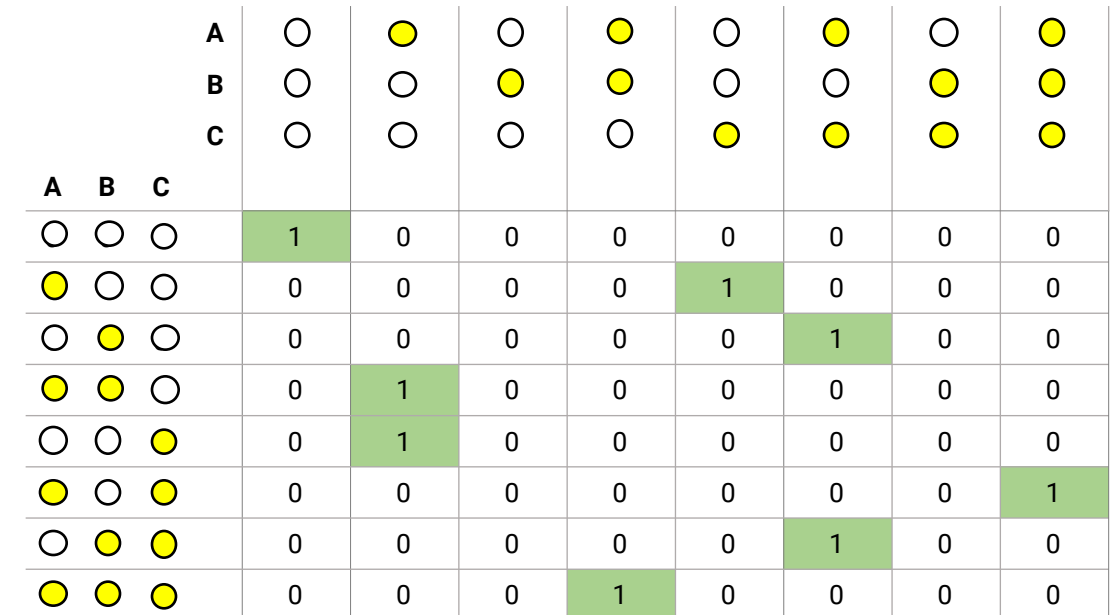 | 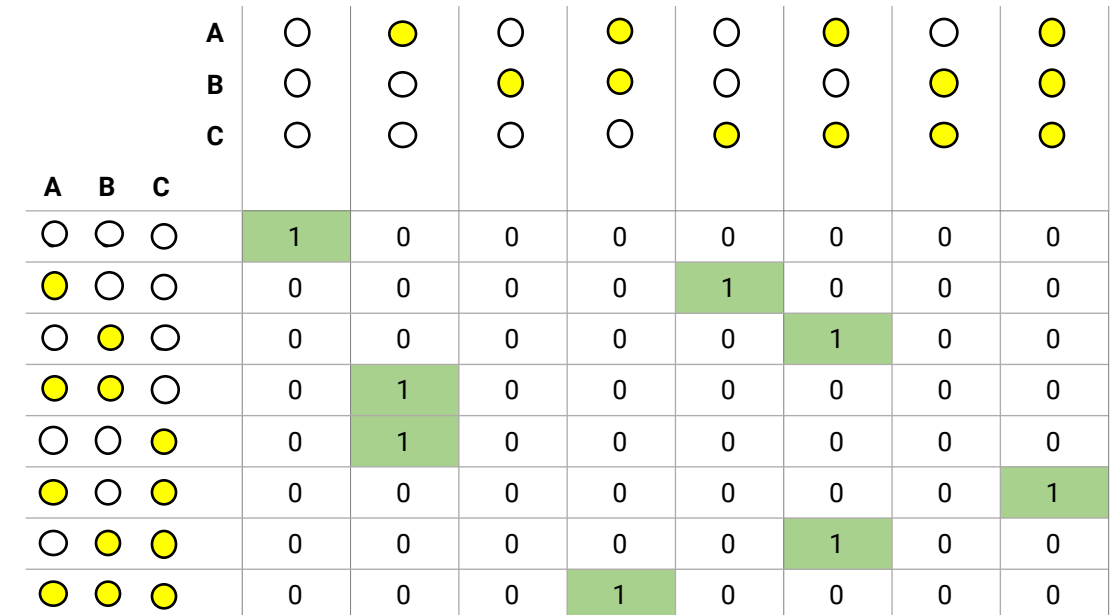 | 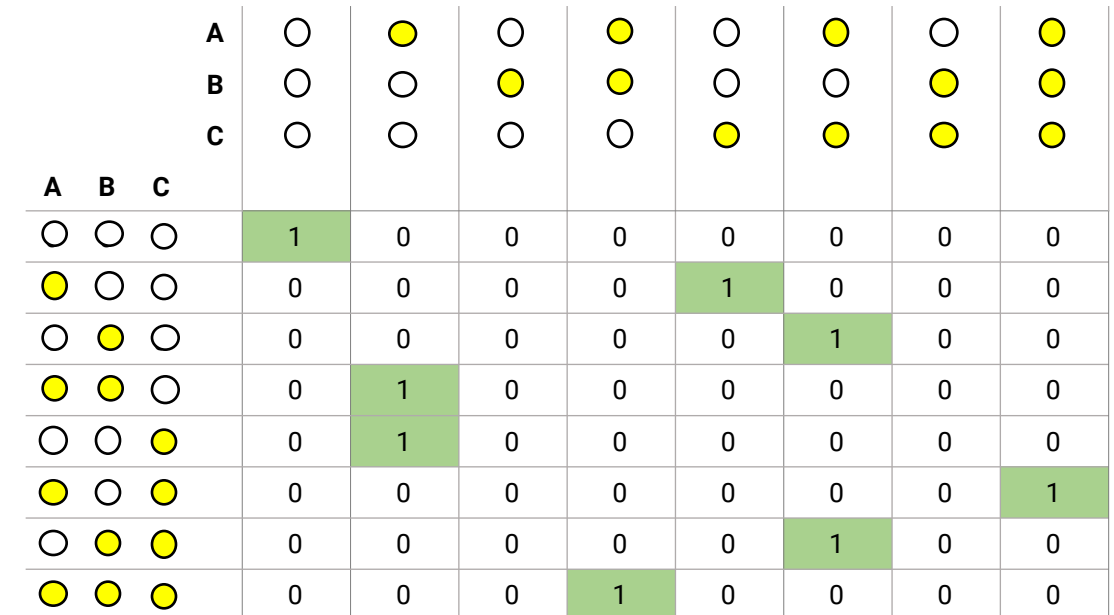 |          | 0                                                                                   | 0                                                                                   | 0                                                                                   | 0                                                                                   | 0                                                                                   | 0                                                                                   | 0                                                                                   | 1                                                                                   |
| 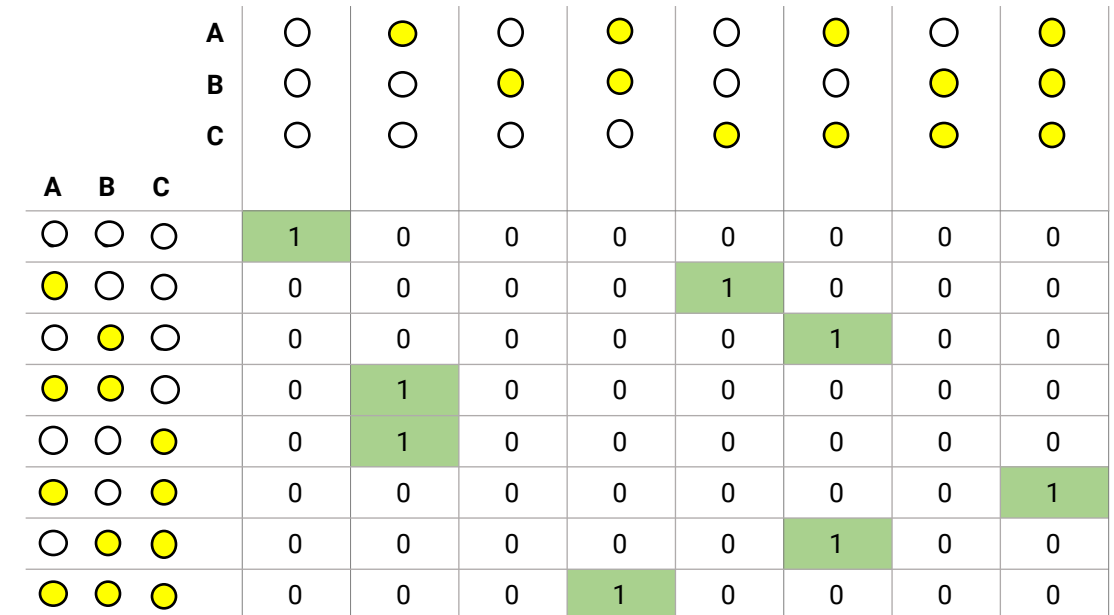 | 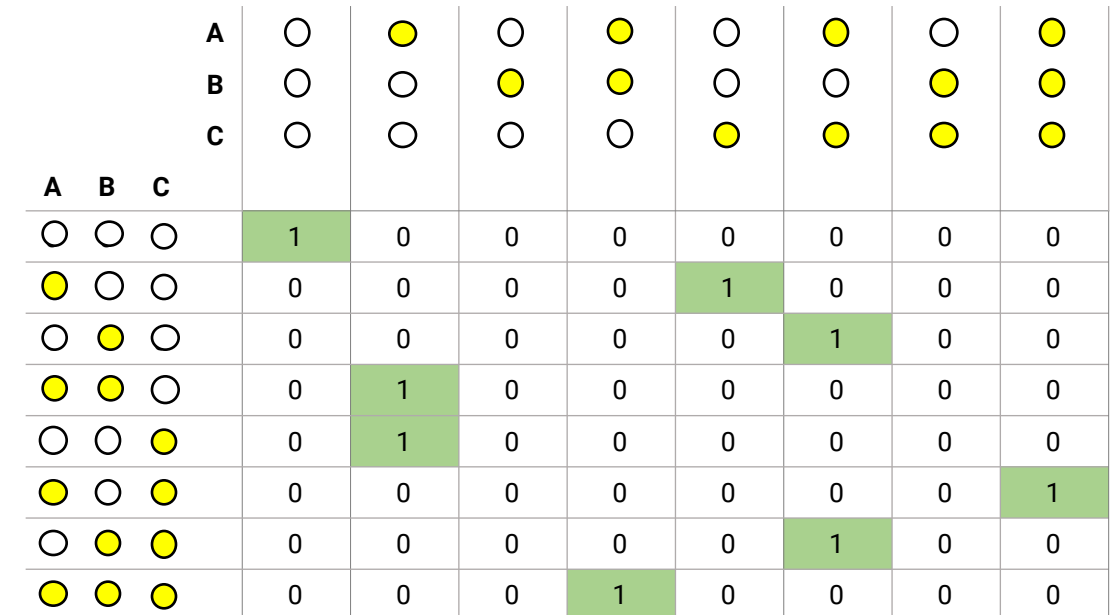 | 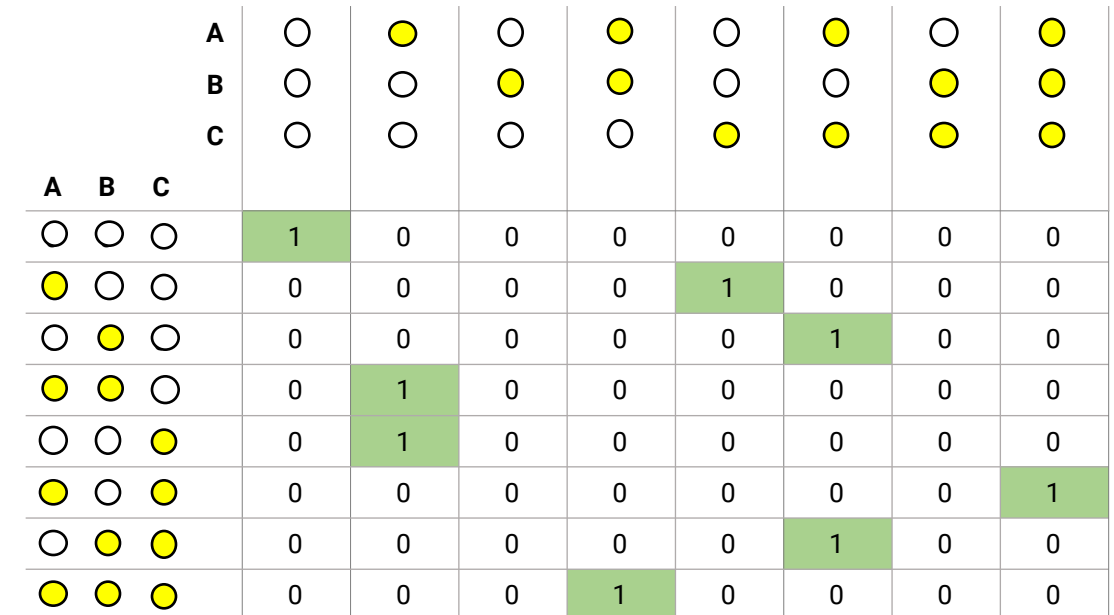 |          | 0                                                                                   | 0                                                                                   | 0                                                                                   | 0                                                                                   | 0                                                                                   | 1                                                                                   | 0                                                                                   | 0                                                                                   |
| 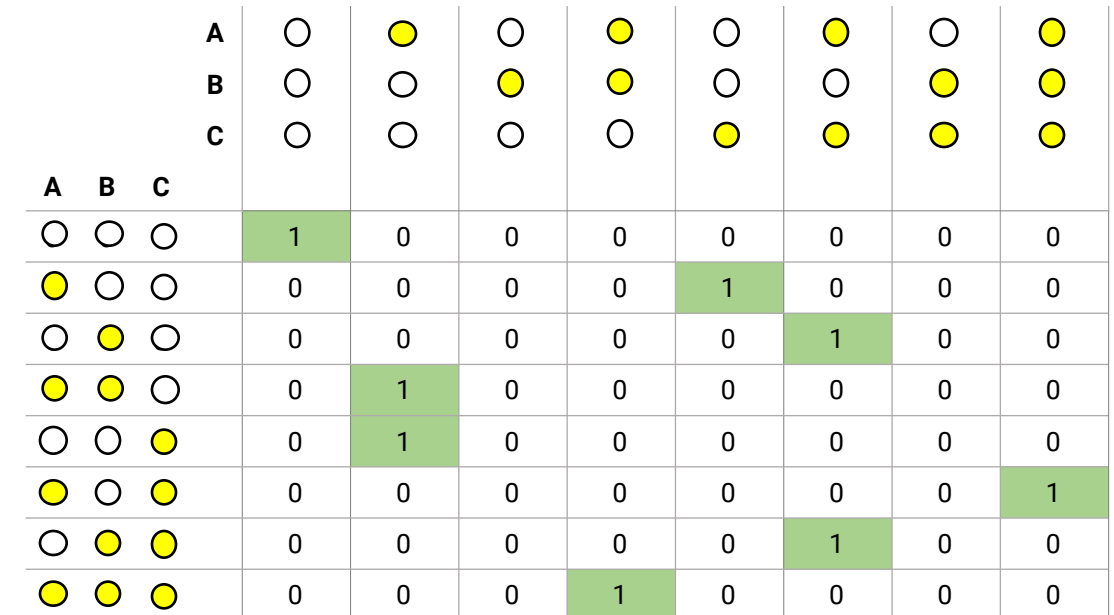 | 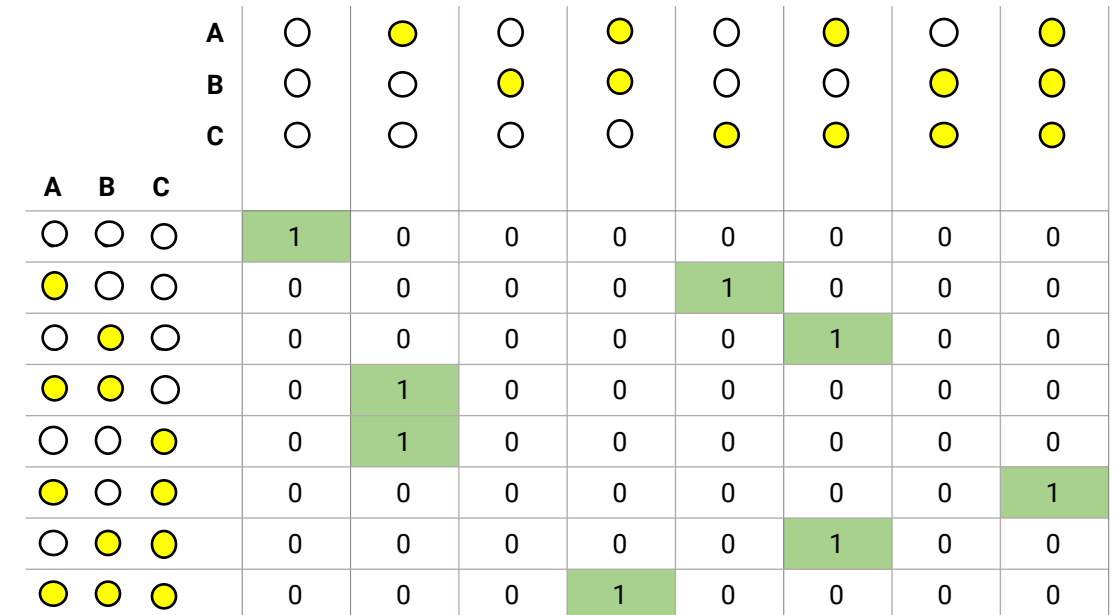 | 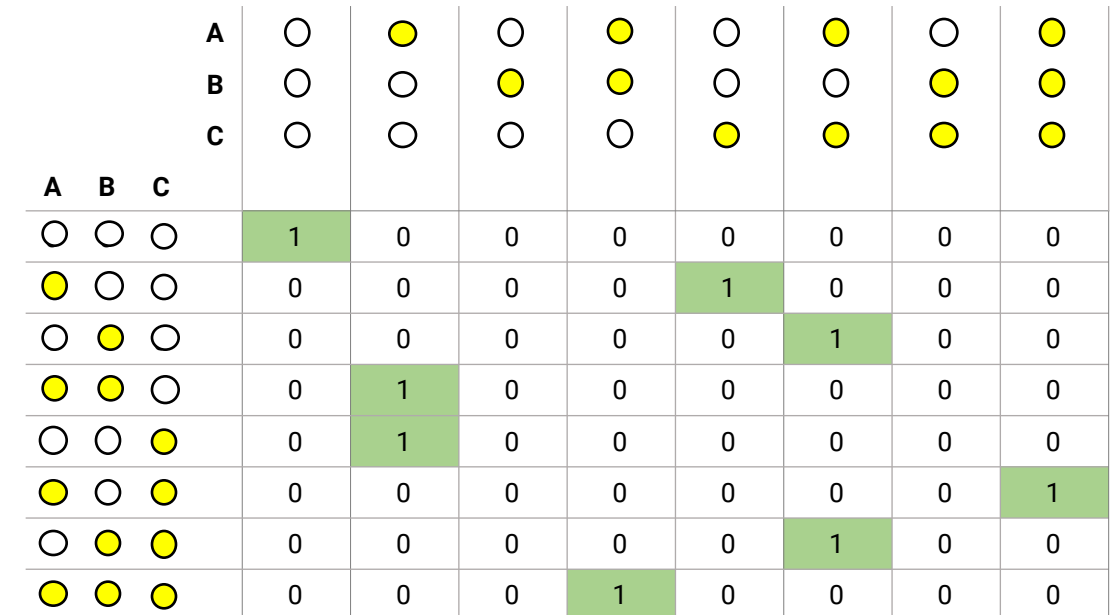 |          | 0                                                                                   | 0                                                                                   | 0                                                                                   | 1                                                                                   | 0                                                                                   | 0                                                                                   | 0                                                                                   | 0                                                                                   |



Fixing background conditions:  
**Updated from IIT 3.0**

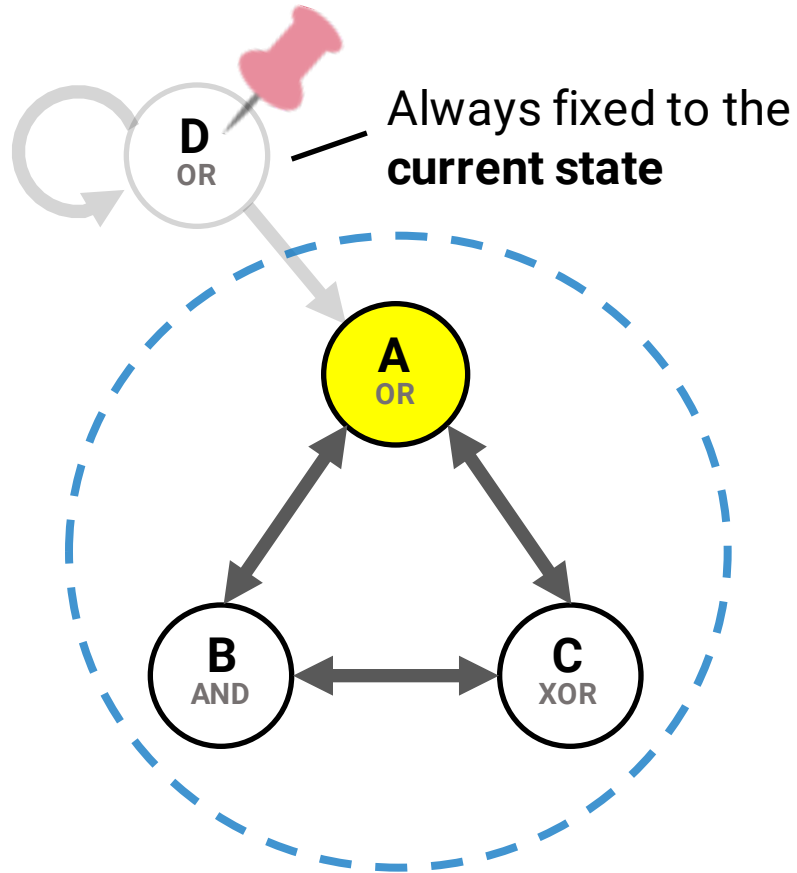

- Note that the external elements are fixed in their *current* state throughout the analysis
- This is an update to the formalism compared to IIT 3.0, where the previous state was used instead of the current state in certain parts of the analysis



# Outline

- Elements, states, and the TPM
- Background conditions
- **Cause-effect repertoires**
- Integrated mechanisms:  $\varphi$
- Concepts and cause-effect structures
- Integrated systems:  $\Phi$
- Complexes

# Cause-effect repertoires

- Having chosen a candidate system and conditioned on the state of external, background elements, we now consider all subsets of the candidate system
- We call these subsets of elements **candidate mechanisms**
- We would like to evaluate the causal properties of each candidate mechanism

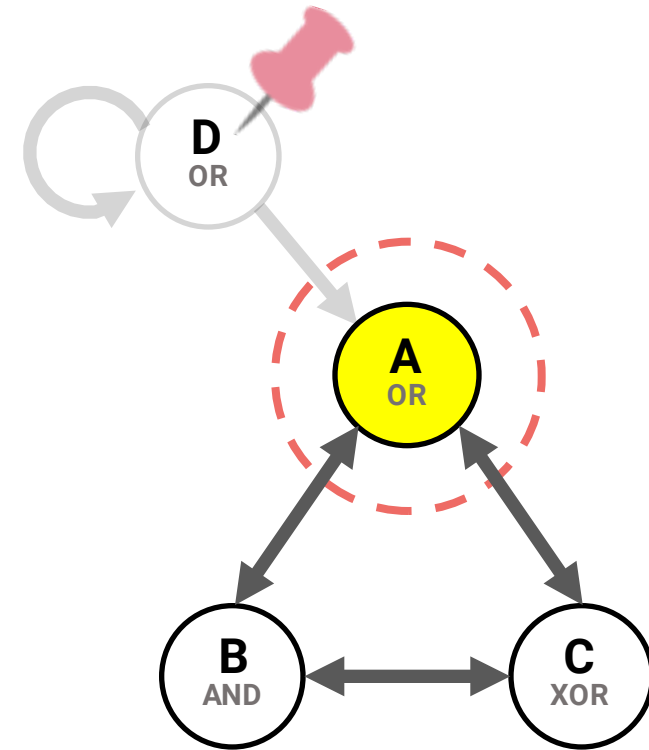

Candidate mechanism **A**

# Cause-effect repertoires

- Having chosen a candidate system and conditioned on the state of external, background elements, we now consider all subsets of the candidate system
- We call these subsets of elements **candidate mechanisms**
- We would like to evaluate the causal properties of each candidate mechanism

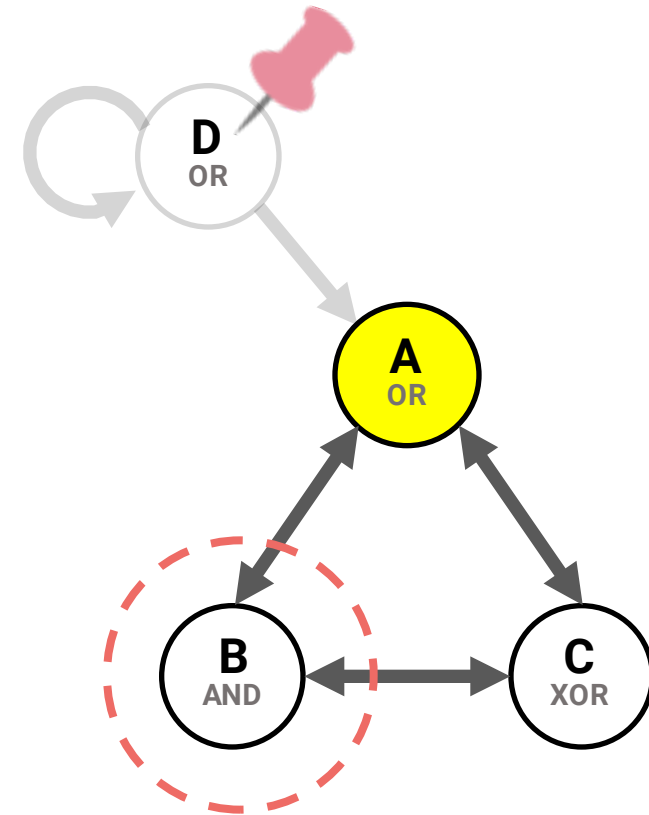

Candidate mechanism **B**

# Cause-effect repertoires

- Having chosen a candidate system and conditioned on the state of external, background elements, we now consider all subsets of the candidate system
- We call these subsets of elements **candidate mechanisms**
- We would like to evaluate the causal properties of each candidate mechanism

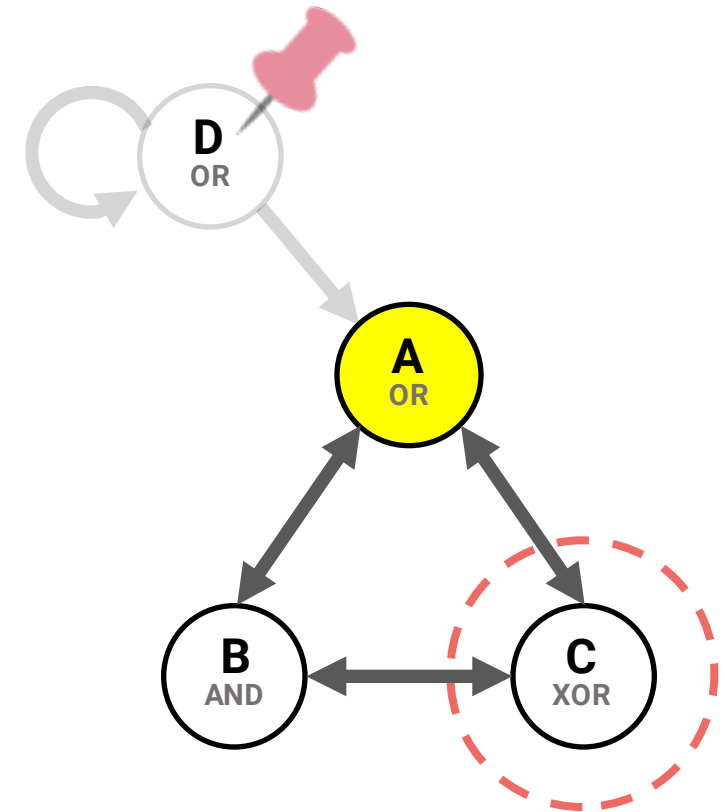

Candidate mechanism **C**

# Cause-effect repertoires

- Having chosen a candidate system and conditioned on the state of external, background elements, we now consider all subsets of the candidate system
- We call these subsets of elements **candidate mechanisms**
- We would like to evaluate the causal properties of each candidate mechanism

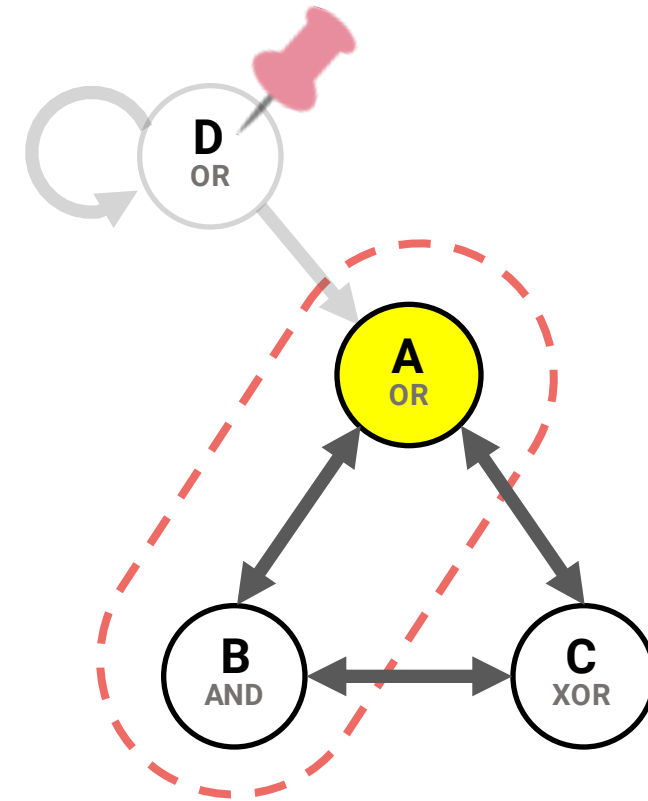

Candidate mechanism **AB**

# Cause-effect repertoires

- Having chosen a candidate system and conditioned on the state of external, background elements, we now consider all subsets of the candidate system
- We call these subsets of elements **candidate mechanisms**
- We would like to evaluate the causal properties of each candidate mechanism

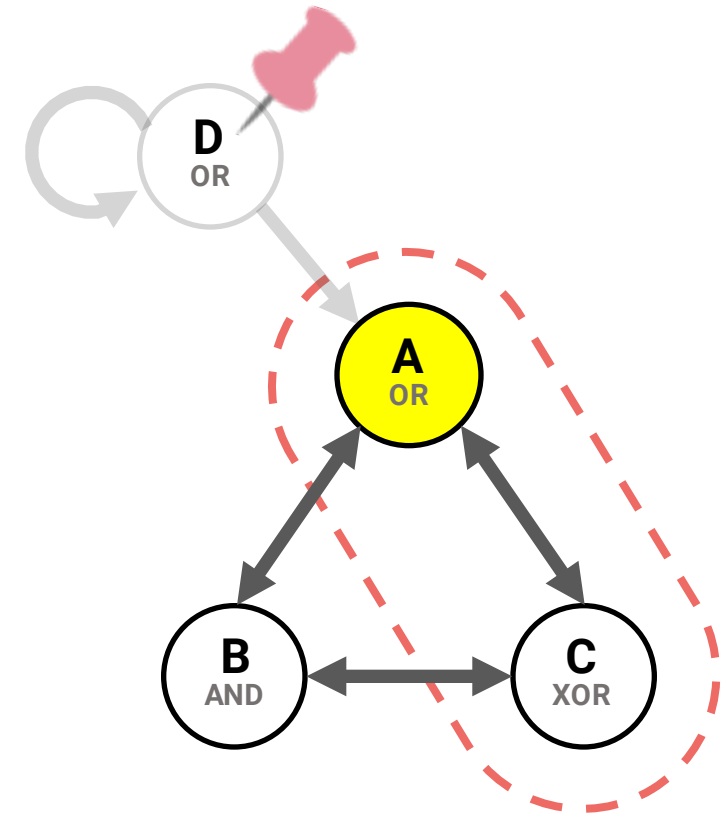

Candidate mechanism **AC**

# Cause-effect repertoires

- Having chosen a candidate system and conditioned on the state of external, background elements, we now consider all subsets of the candidate system
- We call these subsets of elements **candidate mechanisms**
- We would like to evaluate the causal properties of each candidate mechanism

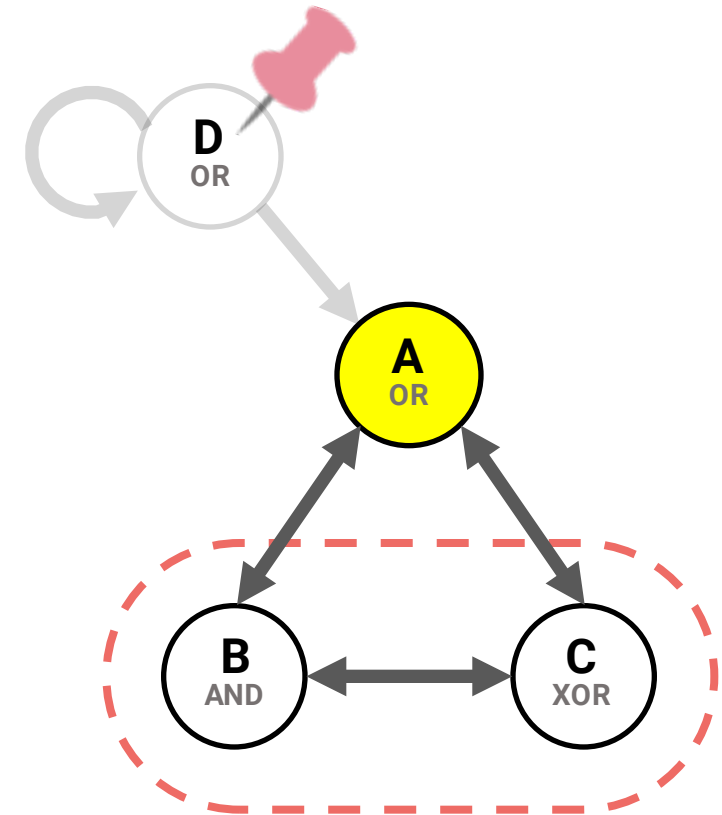

Candidate mechanism **BC**

# Cause-effect repertoires

- Having chosen a candidate system and conditioned on the state of external, background elements, we now consider all subsets of the candidate system
- We call these subsets of elements **candidate mechanisms**
- We would like to evaluate the causal properties of each candidate mechanism

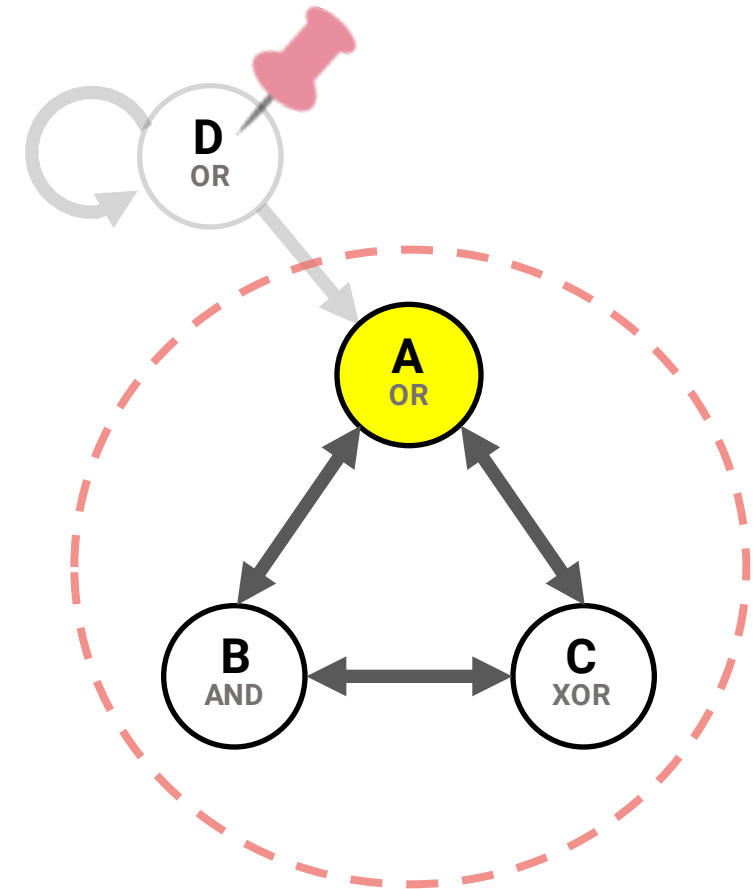

Candidate mechanism **ABC**



# Cause-effect repertoires

- The notion of “causal properties” is made precise with the **cause repertoire and effect repertoire** of a candidate mechanism
- These repertoires are probability distributions over states of the system at  $t - 1$  and  $t + 1$ , respectively
- They describe how the mechanism in its current state at  $t$  causally constrains the other elements
- First we'll focus on the effect repertoire

# Calculating an effect repertoire: Conditioning on the mechanism **ABC**

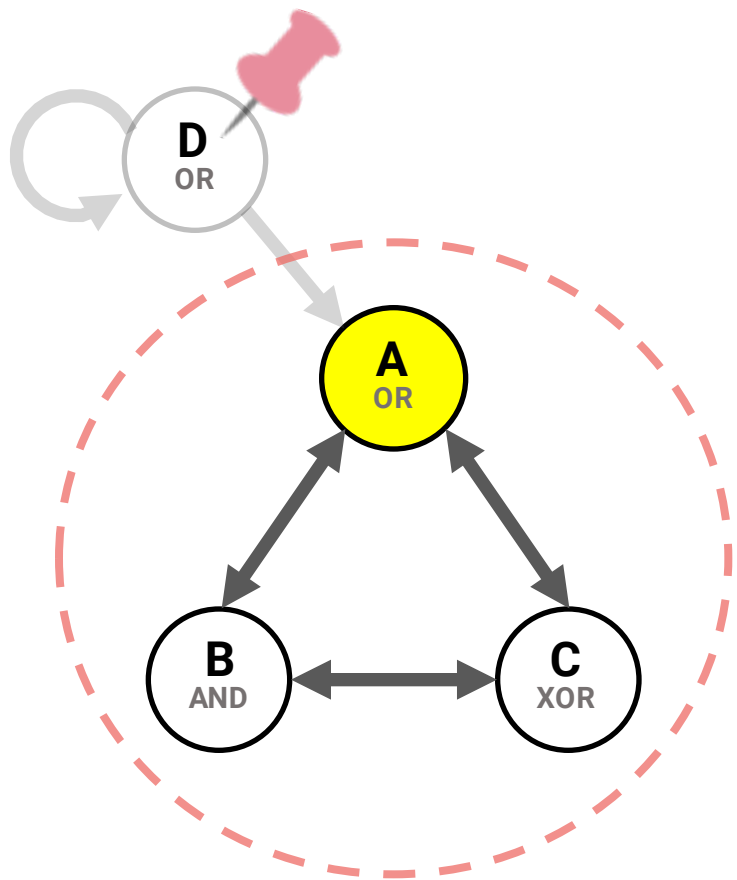

For example, let’s calculate the effect repertoire of the candidate mechanism **ABC**

|               |   |   |   | Next state |   |   |   |   |   |   |   |
|---------------|---|---|---|------------|---|---|---|---|---|---|---|
|               |   |   |   | A          |   |   |   |   |   |   |   |
|               |   |   |   | B          |   |   |   |   |   |   |   |
|               |   |   |   | C          |   |   |   |   |   |   |   |
| Current state | A | B | C |            |   |   |   |   |   |   |   |
|               |   |   |   | 1          | 0 | 0 | 0 | 0 | 0 | 0 | 0 |
|               |   |   |   | 0          | 0 | 0 | 0 | 1 | 0 | 0 | 0 |
|               |   |   |   | 0          | 0 | 0 | 0 | 0 | 1 | 0 | 0 |
|               |   |   |   | 0          | 1 | 0 | 0 | 0 | 0 | 0 | 0 |
|               |   |   |   | 0          | 1 | 0 | 0 | 0 | 0 | 0 | 0 |
|               |   |   |   | 0          | 0 | 0 | 0 | 0 | 0 | 0 | 1 |
|               |   |   |   | 0          | 0 | 0 | 0 | 0 | 1 | 0 | 0 |
|               |   |   |   | 0          | 0 | 0 | 1 | 0 | 0 | 0 | 0 |

# Calculating an effect repertoire: Conditioning on the mechanism **ABC**

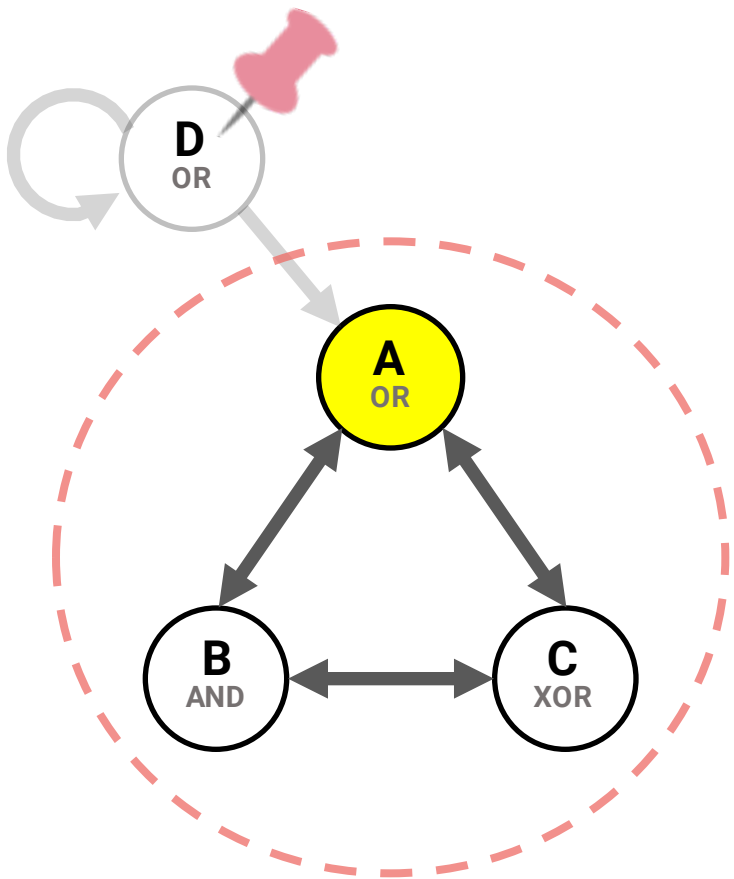

We want to determine how the current state of **ABC** constrains the next state...

|               |   |   | Next state |   |   |   |   |   |   |   |
|---------------|---|---|------------|---|---|---|---|---|---|---|
|               |   |   | A          |   |   |   |   |   |   |   |
|               |   |   | B          |   |   |   |   |   |   |   |
|               |   |   | C          |   |   |   |   |   |   |   |
| Current state | A | B | C          |   |   |   |   |   |   |   |
|               |   |   |            | 1 | 0 | 0 | 0 | 0 | 0 | 0 |
|               |   |   |            | 0 | 0 | 0 | 0 | 1 | 0 | 0 |
|               |   |   |            | 0 | 0 | 0 | 0 | 0 | 1 | 0 |
|               |   |   |            | 0 | 1 | 0 | 0 | 0 | 0 | 0 |
|               |   |   |            | 0 | 1 | 0 | 0 | 0 | 0 | 0 |
|               |   |   |            | 0 | 0 | 0 | 0 | 0 | 0 | 1 |
|               |   |   |            | 0 | 0 | 0 | 0 | 1 | 0 | 0 |
|               |   |   |            | 0 | 0 | 0 | 1 | 0 | 0 | 0 |

# Calculating an effect repertoire: Conditioning on the mechanism ABC

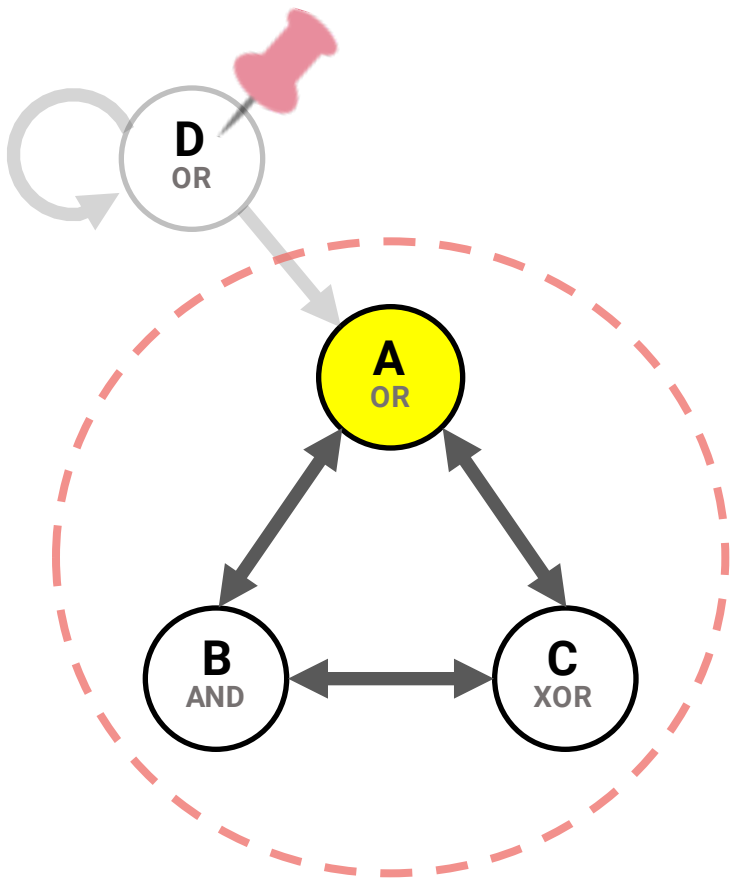

We want to determine how the current state of **ABC** constrains the next state...

|               |   |   | Next state |   |   |   |   |   |   |   |
|---------------|---|---|------------|---|---|---|---|---|---|---|
|               |   |   | A          |   |   |   |   |   |   |   |
|               |   |   | B          |   |   |   |   |   |   |   |
|               |   |   | C          |   |   |   |   |   |   |   |
| Current state | A | B | C          |   |   |   |   |   |   |   |
|               |   |   |            | 1 | 0 | 0 | 0 | 0 | 0 | 0 |
|               |   |   |            | 0 | 0 | 0 | 0 | 1 | 0 | 0 |
|               |   |   |            | 0 | 0 | 0 | 0 | 0 | 1 | 0 |
|               |   |   |            | 0 | 1 | 0 | 0 | 0 | 0 | 0 |
|               |   |   |            | 0 | 1 | 0 | 0 | 0 | 0 | 0 |
|               |   |   |            | 0 | 0 | 0 | 0 | 0 | 0 | 1 |
|               |   |   |            | 0 | 0 | 0 | 0 | 1 | 0 | 0 |
|               |   |   |            | 0 | 0 | 0 | 1 | 0 | 0 | 0 |

...so, as with background conditions, we condition on the current state by looking at the rows of the TPM that correspond to it

# Calculating an effect repertoire: Conditioning on the mechanism ABC

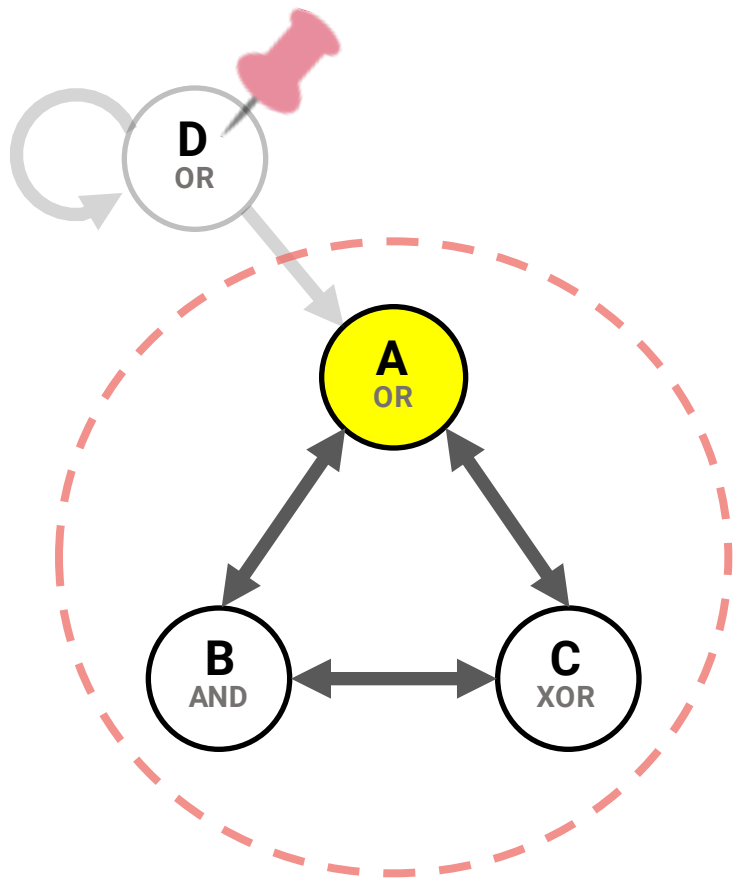

We want to determine how the current state of **ABC** constrains the next state...

|               |   |   | Next state |   |   |   |   |   |   |   |
|---------------|---|---|------------|---|---|---|---|---|---|---|
|               |   |   | A          |   |   |   |   |   |   |   |
|               |   |   | B          |   |   |   |   |   |   |   |
|               |   |   | C          |   |   |   |   |   |   |   |
| Current state | A | B | C          |   |   |   |   |   |   |   |
|               |   |   |            | 1 | 0 | 0 | 0 | 0 | 0 | 0 |
|               |   |   |            | 0 | 0 | 0 | 0 | 1 | 0 | 0 |
|               |   |   |            | 0 | 0 | 0 | 0 | 0 | 1 | 0 |
|               |   |   |            | 0 | 1 | 0 | 0 | 0 | 0 | 0 |
|               |   |   |            | 0 | 1 | 0 | 0 | 0 | 0 | 0 |
|               |   |   |            | 0 | 0 | 0 | 0 | 0 | 0 | 1 |
|               |   |   |            | 0 | 0 | 0 | 0 | 1 | 0 | 0 |
|               |   |   |            | 0 | 0 | 0 | 1 | 0 | 0 | 0 |

...so, as with background conditions, we condition on the current state by looking at the rows of the TPM that correspond to it

# Calculating an effect repertoire: Conditioning on the mechanism ABC

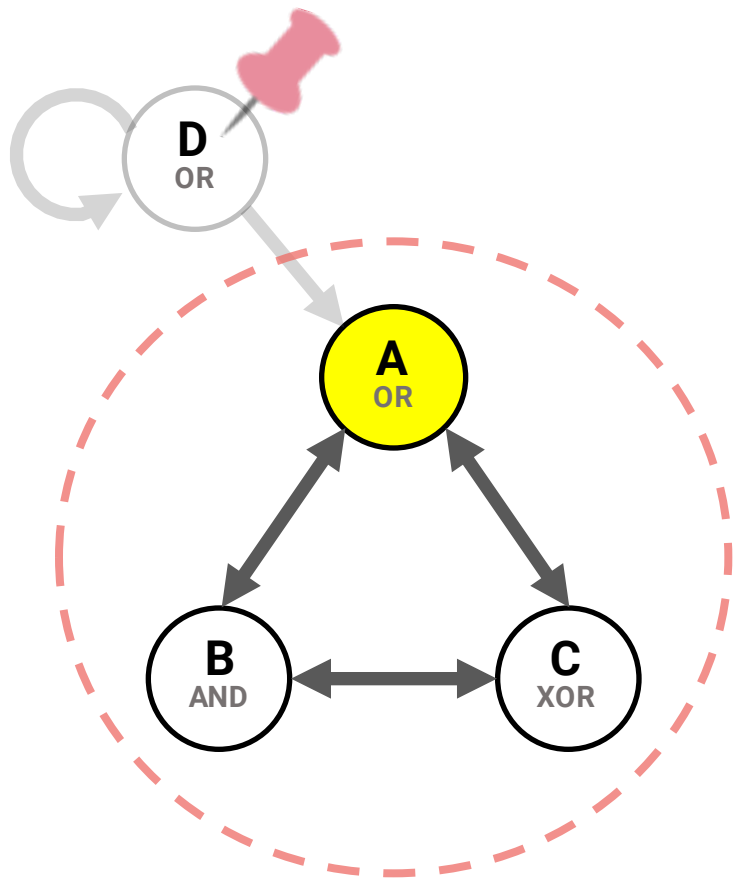

We want to determine how the current state of **ABC** constrains the next state...

|               |   |   |   | Next state |   |   |   |   |   |   |   |
|---------------|---|---|---|------------|---|---|---|---|---|---|---|
|               |   |   |   | A          |   |   |   |   |   |   |   |
|               |   |   |   | B          |   |   |   |   |   |   |   |
|               |   |   |   | C          |   |   |   |   |   |   |   |
| Current state | A | B | C |            |   |   |   |   |   |   |   |
|               |   |   |   | 1          | 0 | 0 | 0 | 0 | 0 | 0 | 0 |
|               |   |   |   | 0          | 0 | 0 | 0 | 1 | 0 | 0 | 0 |
|               |   |   |   | 0          | 0 | 0 | 0 | 0 | 1 | 0 | 0 |
|               |   |   |   | 0          | 1 | 0 | 0 | 0 | 0 | 0 | 0 |
|               |   |   |   | 0          | 1 | 0 | 0 | 0 | 0 | 0 | 0 |
|               |   |   |   | 0          | 0 | 0 | 0 | 0 | 0 | 0 | 1 |
|               |   |   |   | 0          | 0 | 0 | 0 | 0 | 1 | 0 | 0 |
|               |   |   |   | 0          | 0 | 0 | 1 | 0 | 0 | 0 | 0 |

...so, as with background conditions, we condition on the current state by looking at the rows of the TPM that correspond to it

# Calculating an effect repertoire: Conditioning on the mechanism ABC

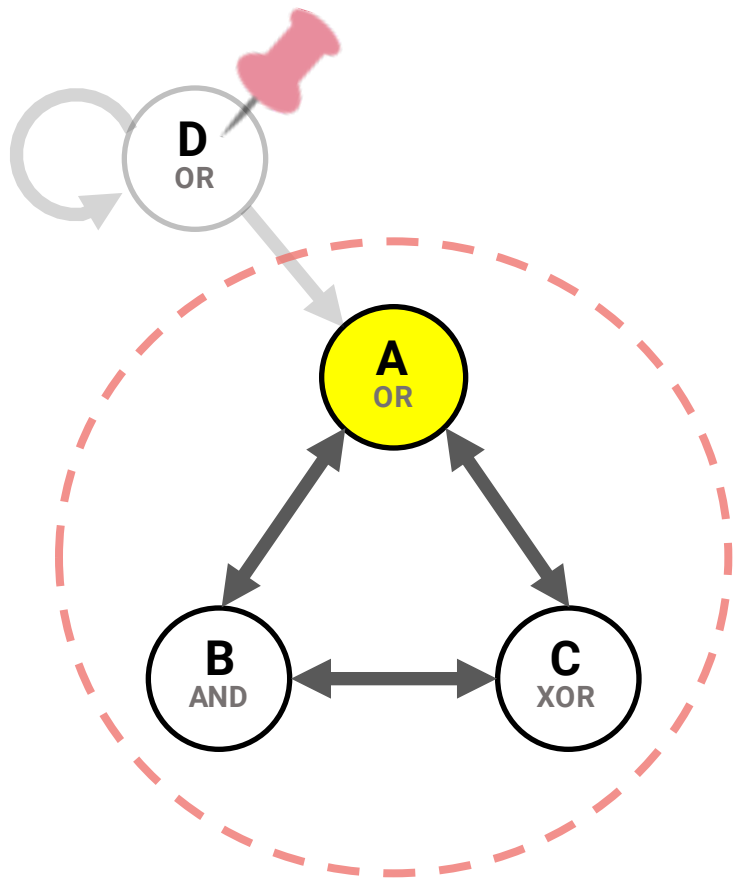

We want to determine how the current state of **ABC** constrains the next state...

|               |   |   |   | Next state |   |   |   |   |   |   |   |
|---------------|---|---|---|------------|---|---|---|---|---|---|---|
|               |   |   |   | A          |   |   |   |   |   |   |   |
|               |   |   |   | B          |   |   |   |   |   |   |   |
|               |   |   |   | C          |   |   |   |   |   |   |   |
| Current state | A | B | C |            |   |   |   |   |   |   |   |
|               |   |   |   | 1          | 0 | 0 | 0 | 0 | 0 | 0 | 0 |
|               |   |   |   | 0          | 0 | 0 | 0 | 1 | 0 | 0 | 0 |
|               |   |   |   | 0          | 0 | 0 | 0 | 0 | 1 | 0 | 0 |
|               |   |   |   | 0          | 1 | 0 | 0 | 0 | 0 | 0 | 0 |
|               |   |   |   | 0          | 1 | 0 | 0 | 0 | 0 | 0 | 0 |
|               |   |   |   | 0          | 0 | 0 | 0 | 0 | 0 | 0 | 1 |
|               |   |   |   | 0          | 0 | 0 | 0 | 0 | 1 | 0 | 0 |
|               |   |   |   | 0          | 0 | 0 | 1 | 0 | 0 | 0 | 0 |

...so, as with background conditions, we condition on the current state by looking at the rows of the TPM that correspond to it

# Calculating an effect repertoire: Conditioning on the mechanism ABC

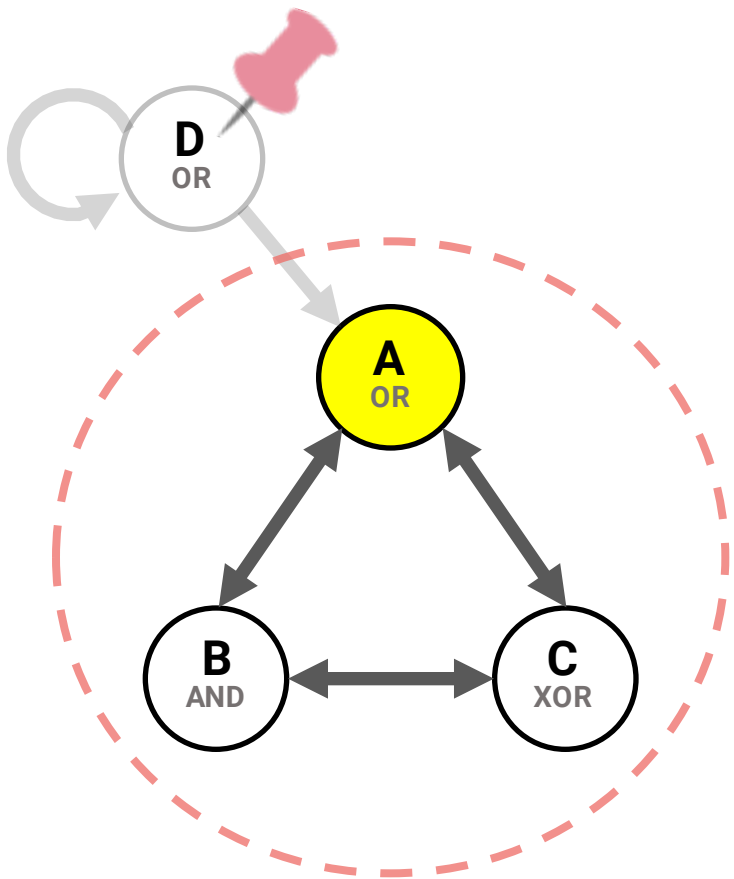

|               |   |   |   | Next state |   |   |   |   |   |   |   |
|---------------|---|---|---|------------|---|---|---|---|---|---|---|
|               |   |   |   | A          |   |   |   |   |   |   |   |
|               |   |   |   | B          |   |   |   |   |   |   |   |
|               |   |   |   | C          |   |   |   |   |   |   |   |
| Current state | A | B | C |            |   |   |   |   |   |   |   |
|               |   |   |   | 1          | 0 | 0 | 0 | 0 | 0 | 0 | 0 |
|               |   |   |   | 0          | 0 | 0 | 0 | 1 | 0 | 0 | 0 |
|               |   |   |   | 0          | 0 | 0 | 0 | 0 | 1 | 0 | 0 |
|               |   |   |   | 0          | 1 | 0 | 0 | 0 | 0 | 0 | 0 |
|               |   |   |   | 0          | 1 | 0 | 0 | 0 | 0 | 0 | 0 |
|               |   |   |   | 0          | 0 | 0 | 0 | 0 | 0 | 0 | 1 |
|               |   |   |   | 0          | 0 | 0 | 0 | 0 | 1 | 0 | 0 |
|               |   |   |   | 0          | 0 | 0 | 1 | 0 | 0 | 0 | 0 |

This row in the TPM is a distribution over the states at  $t + 1$  (and since this is a deterministic system, the next state is fully specified by the current state)



Calculating an effect repertoire:  
**Conditioning on the mechanism ABC**

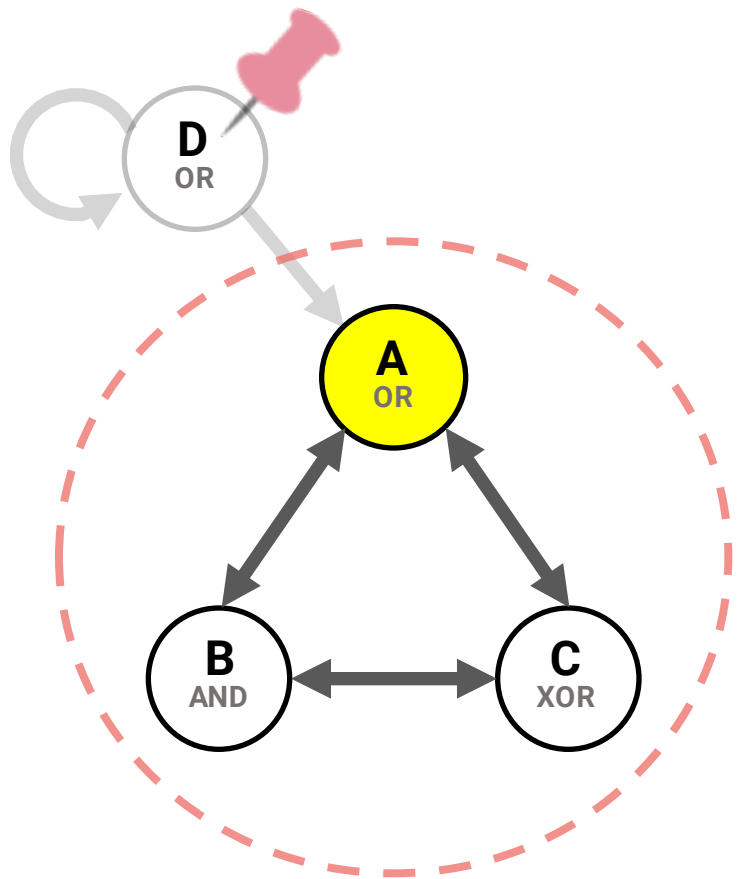

|               |   |   | Next state |   |   |   |   |   |   |   |
|---------------|---|---|------------|---|---|---|---|---|---|---|
|               |   |   | A          |   |   |   |   |   |   |   |
|               |   |   | B          |   |   |   |   |   |   |   |
|               |   |   | C          |   |   |   |   |   |   |   |
| Current state | A | B | C          |   |   |   |   |   |   |   |
|               |   |   |            | 1 | 0 | 0 | 0 | 0 | 0 | 0 |
|               |   |   |            | 0 | 0 | 0 | 0 | 1 | 0 | 0 |
|               |   |   |            | 0 | 0 | 0 | 0 | 0 | 1 | 0 |
|               |   |   |            | 0 | 1 | 0 | 0 | 0 | 0 | 0 |
|               |   |   |            | 0 | 1 | 0 | 0 | 0 | 0 | 0 |
|               |   |   |            | 0 | 0 | 0 | 0 | 0 | 0 | 1 |
|               |   |   |            | 0 | 0 | 0 | 0 | 0 | 1 | 0 |
|               |   |   |            | 0 | 0 | 0 | 1 | 0 | 0 | 0 |

This is the effect repertoire of **ABC** when the system is in state (1, 0, 0)

# Calculating an effect repertoire: Conditioning on the mechanism ABC

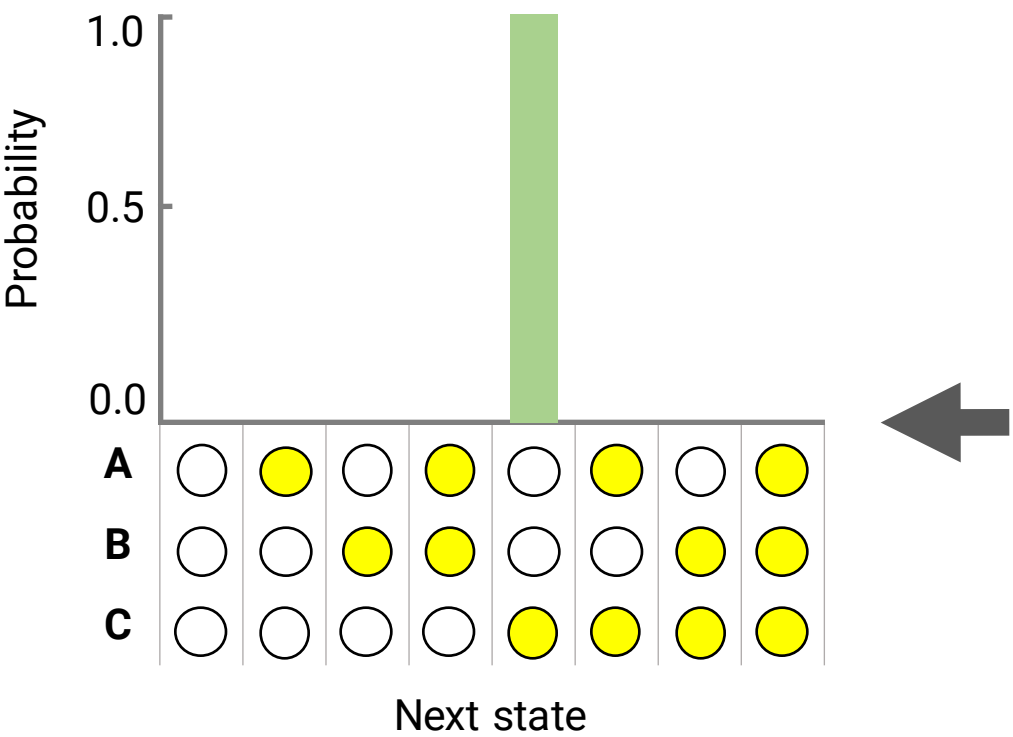

|               |   |   | Next state |   |   |   |   |   |   |   |
|---------------|---|---|------------|---|---|---|---|---|---|---|
| A             | B | C |            |   |   |   |   |   |   |   |
|               |   |   |            |   |   |   |   |   |   |   |
|               |   |   |            |   |   |   |   |   |   |   |
| Current state | A | B | C          |   |   |   |   |   |   |   |
|               |   |   |            | 1 | 0 | 0 | 0 | 0 | 0 | 0 |
|               |   |   |            | 0 | 0 | 0 | 0 | 1 | 0 | 0 |
|               |   |   |            | 0 | 0 | 0 | 0 | 0 | 1 | 0 |
|               |   |   |            | 0 | 1 | 0 | 0 | 0 | 0 | 0 |
|               |   |   |            | 0 | 1 | 0 | 0 | 0 | 0 | 0 |
|               |   |   |            | 0 | 0 | 0 | 0 | 0 | 0 | 1 |
|               |   |   |            | 0 | 0 | 0 | 0 | 0 | 1 | 0 |
|               |   |   |            | 0 | 0 | 0 | 1 | 0 | 0 | 0 |

This is the effect repertoire of **ABC** when the system is in state (1, 0, 0)

# Calculating an effect repertoire: Purviews

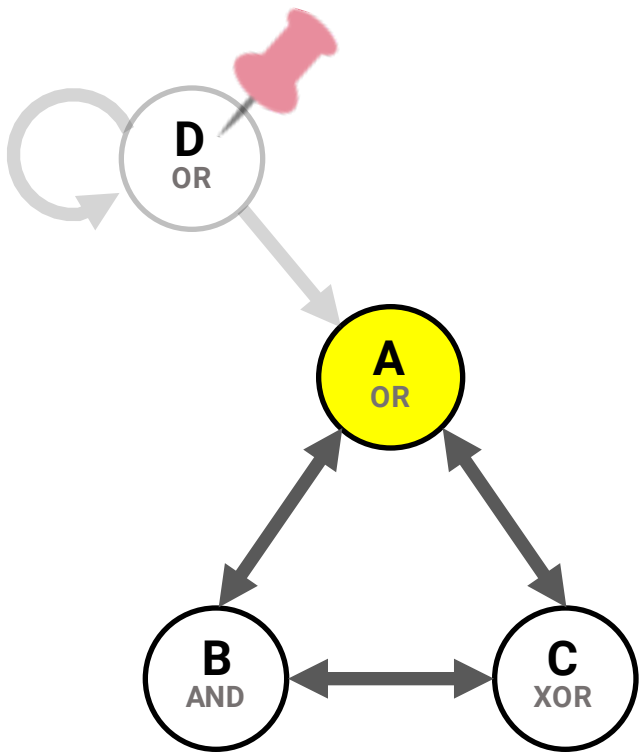

|               |   |   | Next state |   |   |   |   |   |   |   |
|---------------|---|---|------------|---|---|---|---|---|---|---|
|               |   |   | A          |   |   |   |   |   |   |   |
|               |   |   | B          |   |   |   |   |   |   |   |
|               |   |   | C          |   |   |   |   |   |   |   |
| Current state | A | B | C          |   |   |   |   |   |   |   |
|               |   |   |            | 1 | 0 | 0 | 0 | 0 | 0 | 0 |
|               |   |   |            | 0 | 0 | 0 | 0 | 1 | 0 | 0 |
|               |   |   |            | 0 | 0 | 0 | 0 | 0 | 1 | 0 |
|               |   |   |            | 0 | 1 | 0 | 0 | 0 | 0 | 0 |
|               |   |   |            | 0 | 1 | 0 | 0 | 0 | 0 | 0 |
|               |   |   |            | 0 | 0 | 0 | 0 | 0 | 0 | 1 |
|               |   |   |            | 0 | 0 | 0 | 0 | 1 | 0 | 0 |
|               |   |   |            | 0 | 0 | 0 | 1 | 0 | 0 | 0 |

But in general, we can determine how knowing the current state constrains the next state of a *subset* of elements, rather than that of the whole system

# Calculating an effect repertoire: Purviews

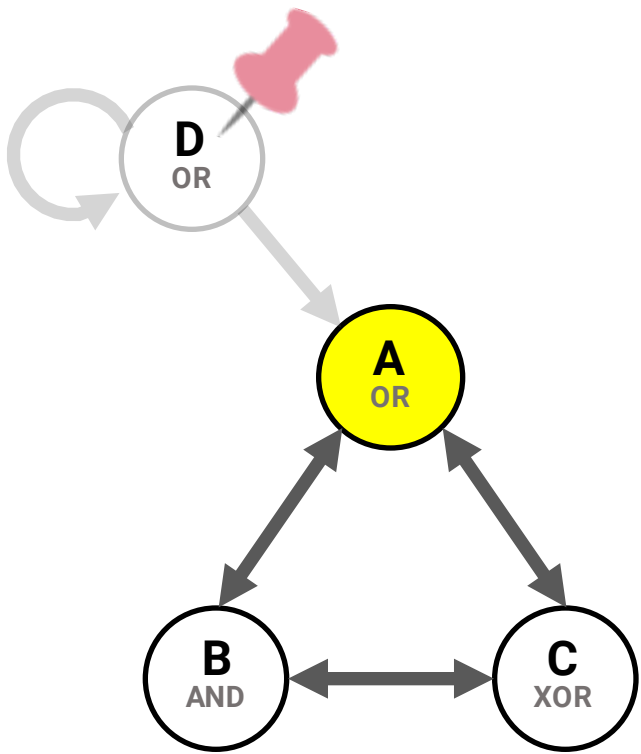

|               |   |   | Next state |   |   |   |   |   |   |   |
|---------------|---|---|------------|---|---|---|---|---|---|---|
|               |   |   | A          |   |   |   |   |   |   |   |
|               |   |   | B          |   |   |   |   |   |   |   |
|               |   |   | C          |   |   |   |   |   |   |   |
| Current state | A | B | C          |   |   |   |   |   |   |   |
|               |   |   |            | 1 | 0 | 0 | 0 | 0 | 0 | 0 |
|               |   |   |            | 0 | 0 | 0 | 0 | 1 | 0 | 0 |
|               |   |   |            | 0 | 0 | 0 | 0 | 0 | 1 | 0 |
|               |   |   |            | 0 | 1 | 0 | 0 | 0 | 0 | 0 |
|               |   |   |            | 0 | 1 | 0 | 0 | 0 | 0 | 0 |
|               |   |   |            | 0 | 0 | 0 | 0 | 0 | 0 | 1 |
|               |   |   |            | 0 | 0 | 0 | 0 | 1 | 0 | 0 |
|               |   |   |            | 0 | 0 | 0 | 1 | 0 | 0 | 0 |

The subset of elements whose next state we’re interested in is called the **purview**

# Calculating an effect repertoire: ABC over purview BC

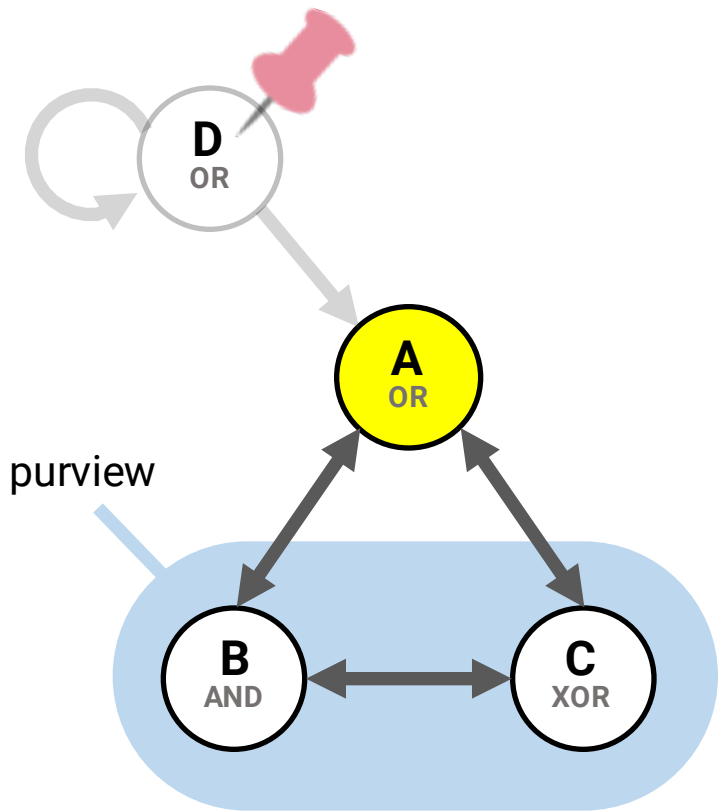

|               |                        |                        | Next state             |                        |                        |                        |                        |                        |                        |                        |
|---------------|------------------------|------------------------|------------------------|------------------------|------------------------|------------------------|------------------------|------------------------|------------------------|------------------------|
|               |                        |                        | A                      |                        |                        |                        |                        |                        |                        |                        |
|               |                        |                        | B                      |                        |                        |                        |                        |                        |                        |                        |
|               |                        |                        | C                      |                        |                        |                        |                        |                        |                        |                        |
| Current state | A                      | B                      | C                      | <div><div></div></div> | <div><div></div></div> | <div><div></div></div> | <div><div></div></div> | <div><div></div></div> | <div><div></div></div> | <div><div></div></div> |
|               | <div><div></div></div> | <div><div></div></div> | <div><div></div></div> | 1                      | 0                      | 0                      | 0                      | 0                      | 0                      | 0                      |
|               | <div><div></div></div> | <div><div></div></div> | <div><div></div></div> | 0                      | 0                      | 0                      | 0                      | 1                      | 0                      | 0                      |
|               | <div><div></div></div> | <div><div></div></div> | <div><div></div></div> | 0                      | 0                      | 0                      | 0                      | 0                      | 1                      | 0                      |
|               | <div><div></div></div> | <div><div></div></div> | <div><div></div></div> | 0                      | 1                      | 0                      | 0                      | 0                      | 0                      | 0                      |
|               | <div><div></div></div> | <div><div></div></div> | <div><div></div></div> | 0                      | 1                      | 0                      | 0                      | 0                      | 0                      | 0                      |
|               | <div><div></div></div> | <div><div></div></div> | <div><div></div></div> | 0                      | 0                      | 0                      | 0                      | 0                      | 0                      | 1                      |
|               | <div><div></div></div> | <div><div></div></div> | <div><div></div></div> | 0                      | 0                      | 0                      | 0                      | 1                      | 0                      | 0                      |
|               | <div><div></div></div> | <div><div></div></div> | <div><div></div></div> | 0                      | 0                      | 0                      | 1                      | 0                      | 0                      | 0                      |

For example, let’s calculate how knowing the current state of **ABC** constrains the next state of the purview **BC**

Calculating an effect repertoire:  
**ABC over purview BC**

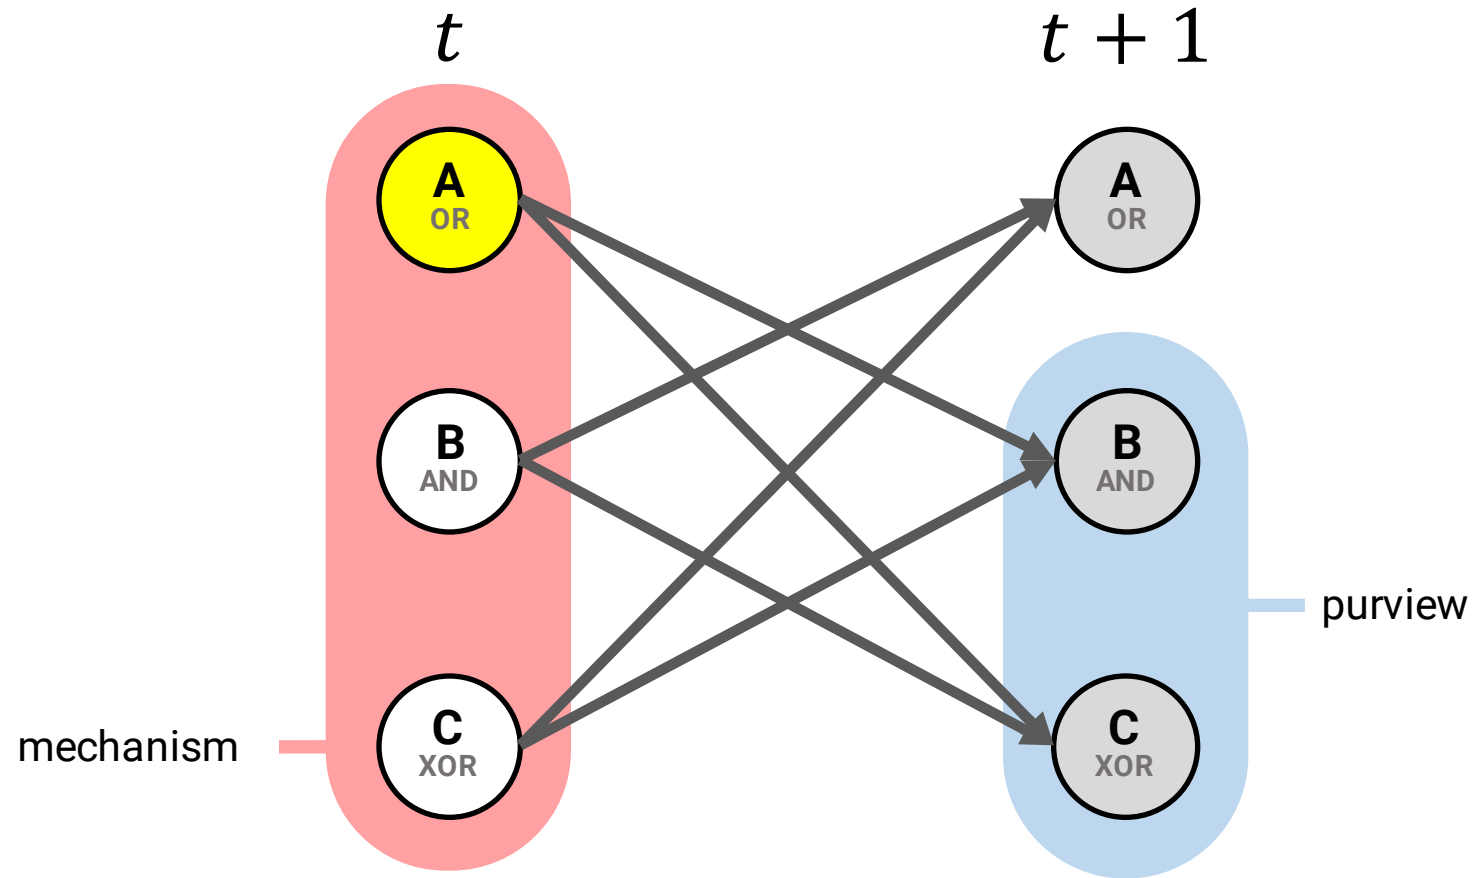

Let's unfold the graph in time between the current and next timestep

# Calculating an effect repertoire: ABC over purview BC

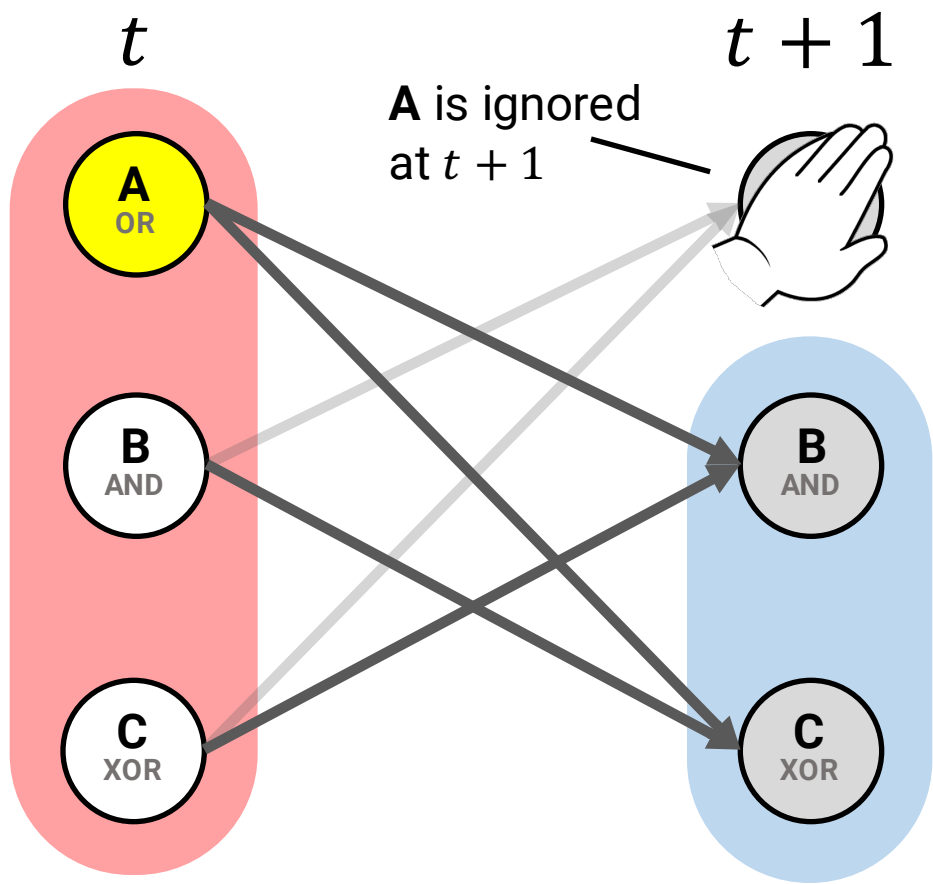

|               |   |   |   | Next state |   |   |   |   |   |   |   |   |   |   |   |   |
|---------------|---|---|---|------------|---|---|---|---|---|---|---|---|---|---|---|---|
|               |   |   |   | A          |   |   |   | B |   |   |   | C |   |   |   |   |
|               |   |   |   |            |   |   |   |   |   |   |   |   |   |   |   |   |
| Current state | A | B | C |            |   |   |   |   |   |   |   |   |   |   |   |   |
|               |   |   |   | 1          | 0 | 0 | 0 | 0 | 0 | 0 | 0 | 0 | 0 | 0 | 0 | 0 |
|               |   |   |   | 0          | 0 | 0 | 0 | 1 | 0 | 0 | 0 | 0 | 0 | 0 | 0 | 0 |
|               |   |   |   | 0          | 0 | 0 | 0 | 0 | 1 | 0 | 0 | 0 | 0 | 0 | 0 | 0 |
|               |   |   |   | 0          | 1 | 0 | 0 | 0 | 0 | 0 | 0 | 0 | 0 | 0 | 0 | 0 |
|               |   |   |   | 0          | 1 | 0 | 0 | 0 | 0 | 0 | 0 | 0 | 0 | 0 | 0 | 0 |
|               |   |   |   | 0          | 0 | 0 | 0 | 0 | 0 | 0 | 0 | 0 | 1 | 0 | 0 | 0 |
|               |   |   |   | 0          | 0 | 0 | 0 | 0 | 1 | 0 | 0 | 0 | 0 | 0 | 0 | 0 |
|               |   |   | 0 | 0          | 0 | 1 | 0 | 0 | 0 | 0 | 0 | 0 | 0 | 0 | 0 | 0 |

Since we’re only interested in the next state of the purview **BC**, we want to **ignore** the next state of **A**

# Calculating an effect repertoire: ABC over purview BC

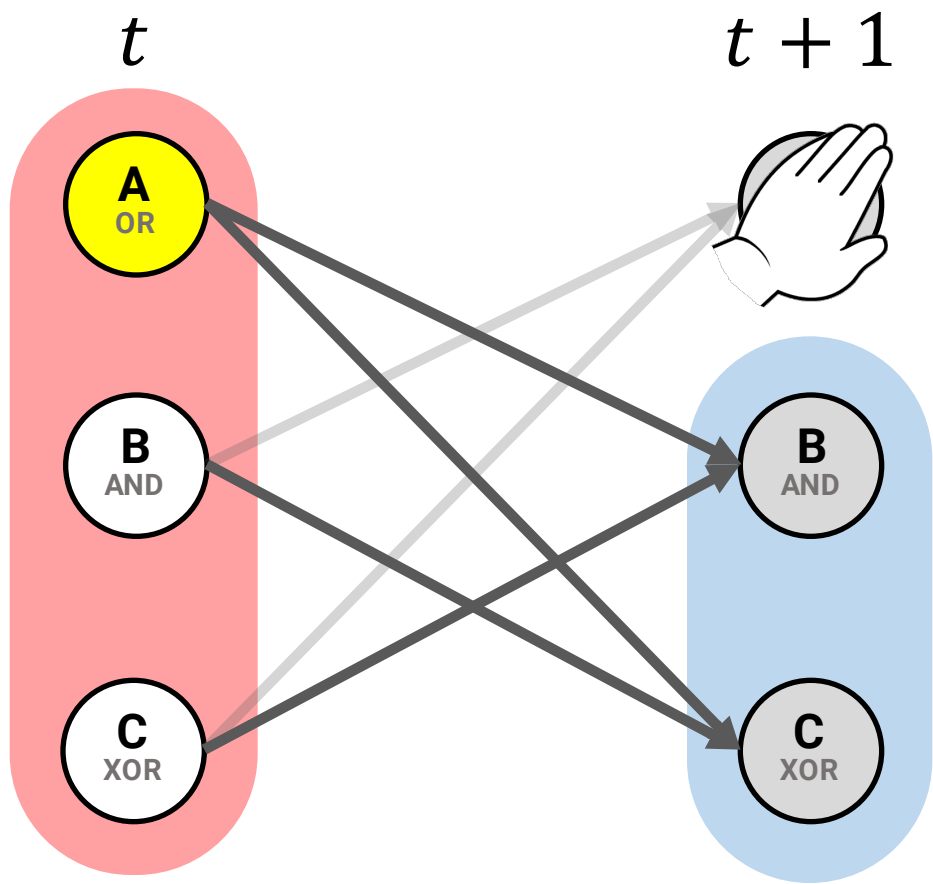

|               |   |   | Next state |   |   |   |   |  |  |  |
|---------------|---|---|------------|---|---|---|---|--|--|--|
|               |   |   | A          |   |   |   |   |  |  |  |
|               |   |   |            |   |   |   |   |  |  |  |
|               |   |   | B          |   |   |   |   |  |  |  |
|               |   |   | C          |   |   |   |   |  |  |  |
| Current state | A | B | C          |   |   |   |   |  |  |  |
|               |   |   |            | 1 | 0 | 0 | 0 |  |  |  |
|               |   |   |            | 0 | 0 | 1 | 0 |  |  |  |
|               |   |   |            | 0 | 0 | 1 | 0 |  |  |  |
|               |   |   |            | 1 | 0 | 0 | 0 |  |  |  |
|               |   |   |            | 1 | 0 | 0 | 0 |  |  |  |
|               |   |   |            | 0 | 0 | 0 | 1 |  |  |  |
|               |   |   |            | 0 | 0 | 1 | 0 |  |  |  |
|               |   |   |            | 0 | 1 | 0 | 0 |  |  |  |

So, we marginalize the next state of **A** out of the TPM



Calculating an effect repertoire:  
**ABC over purview BC**

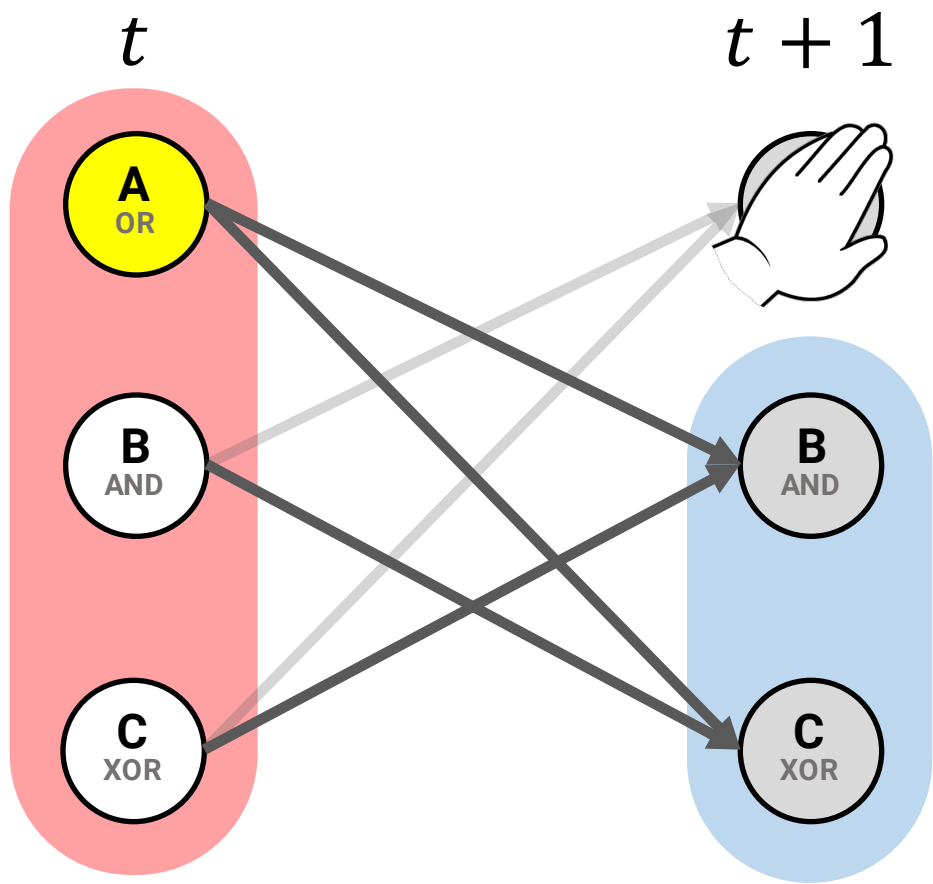

|   |   |   | Next state |   |   |   |
|---|---|---|------------|---|---|---|
|   |   |   | B          |   |   |   |
|   |   |   | C          |   |   |   |
| A | B | C |            |   |   |   |
|   |   |   | 1          | 0 | 0 | 0 |
|   |   |   | 0          | 0 | 1 | 0 |
|   |   |   | 0          | 0 | 1 | 0 |
|   |   |   | 1          | 0 | 0 | 0 |
|   |   |   | 1          | 0 | 0 | 0 |
|   |   |   | 0          | 0 | 0 | 1 |
|   |   |   | 0          | 0 | 1 | 0 |
|   |   |   | 0          | 1 | 0 | 0 |

So, we marginalize the next state of **A** out of the TPM

Calculating an effect repertoire:  
**ABC over purview BC**

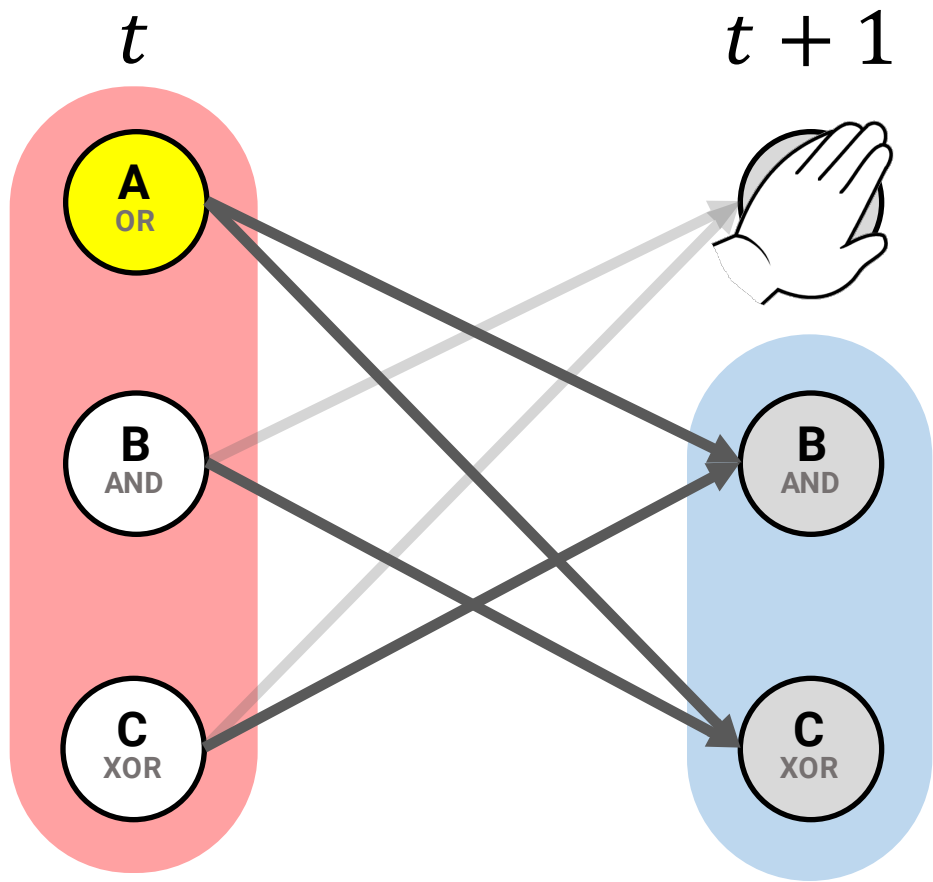

|          |          |          | Next state |  |  |  |
|----------|----------|----------|------------|--|--|--|
|          |          |          | <b>B</b>   |  |  |  |
|          |          |          | <b>C</b>   |  |  |  |
| <b>A</b> | <b>B</b> | <b>C</b> |            |  |  |  |
|          |          |          |            |  |  |  |
|          |          |          |            |  |  |  |
|          |          |          |            |  |  |  |
|          |          |          |            |  |  |  |
|          |          |          |            |  |  |  |
|          |          |          |            |  |  |  |
|          |          |          |            |  |  |  |
|          |          |          |            |  |  |  |

Now we have a TPM that just gives the probabilities of the next states of **B** and **C**

# Calculating an effect repertoire: **ABC over purview BC**

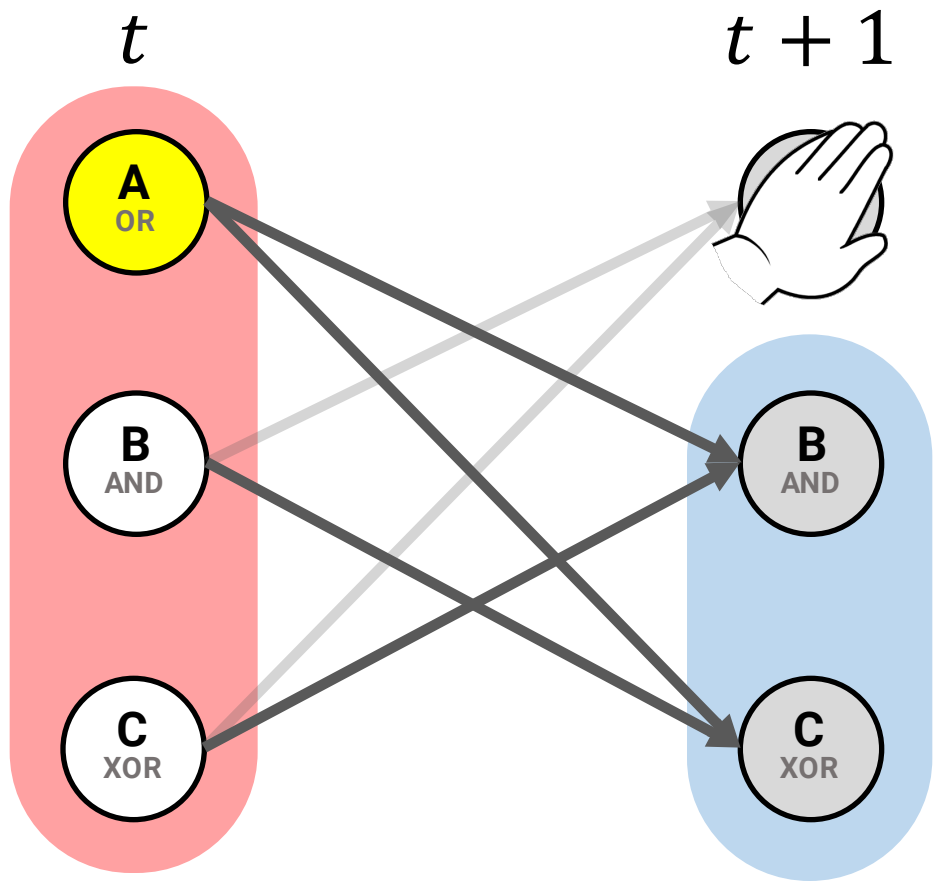

|   |   |   | Next state |   |   |   |
|---|---|---|------------|---|---|---|
|   |   |   | B          |   |   |   |
|   |   |   | C          |   |   |   |
| A | B | C |            |   |   |   |
|   |   |   | 1          | 0 | 0 | 0 |
|   |   |   | 0          | 0 | 1 | 0 |
|   |   |   | 0          | 0 | 1 | 0 |
|   |   |   | 1          | 0 | 0 | 0 |
|   |   |   | 1          | 0 | 0 | 0 |
|   |   |   | 0          | 0 | 0 | 1 |
|   |   |   | 0          | 0 | 1 | 0 |
|   |   |   | 0          | 1 | 0 | 0 |

So we can condition on the current state of the mechanism to get the effect repertoire of mechanism **ABC** over purview **BC** when the system is in state (1, 0, 0)

# Calculating an effect repertoire: **ABC over purview BC**

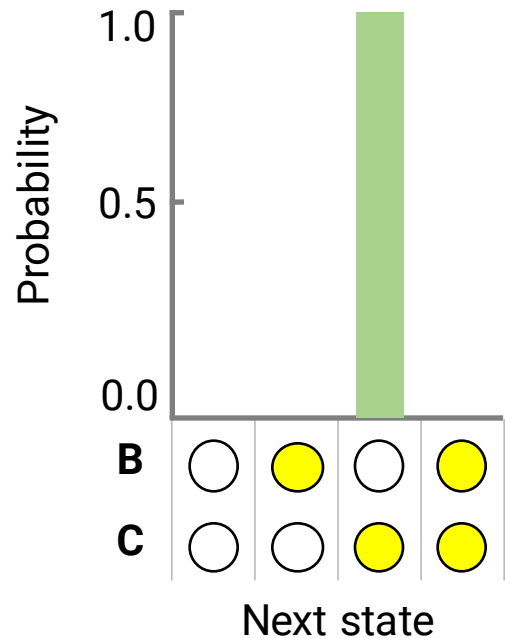

|   |   |   | Next state |   |   |   |
|---|---|---|------------|---|---|---|
|   |   |   | B          |   |   |   |
|   |   |   | C          |   |   |   |
| A | B | C |            |   |   |   |
| 0 | 0 | 0 | 1          | 0 | 0 | 0 |
| 1 | 0 | 0 | 0          | 0 | 1 | 0 |
| 0 | 1 | 0 | 0          | 0 | 1 | 0 |
| 1 | 1 | 0 | 1          | 0 | 0 | 0 |
| 0 | 0 | 1 | 1          | 0 | 0 | 0 |
| 1 | 0 | 1 | 0          | 0 | 0 | 1 |
| 0 | 1 | 1 | 0          | 0 | 1 | 0 |
| 1 | 1 | 1 | 0          | 1 | 0 | 0 |

So we can condition on the current state of the mechanism to get the effect repertoire of mechanism **ABC** over purview **BC** when the system is in state (1, 0, 0)

# Calculating an effect repertoire: Mechanism C over purview BC

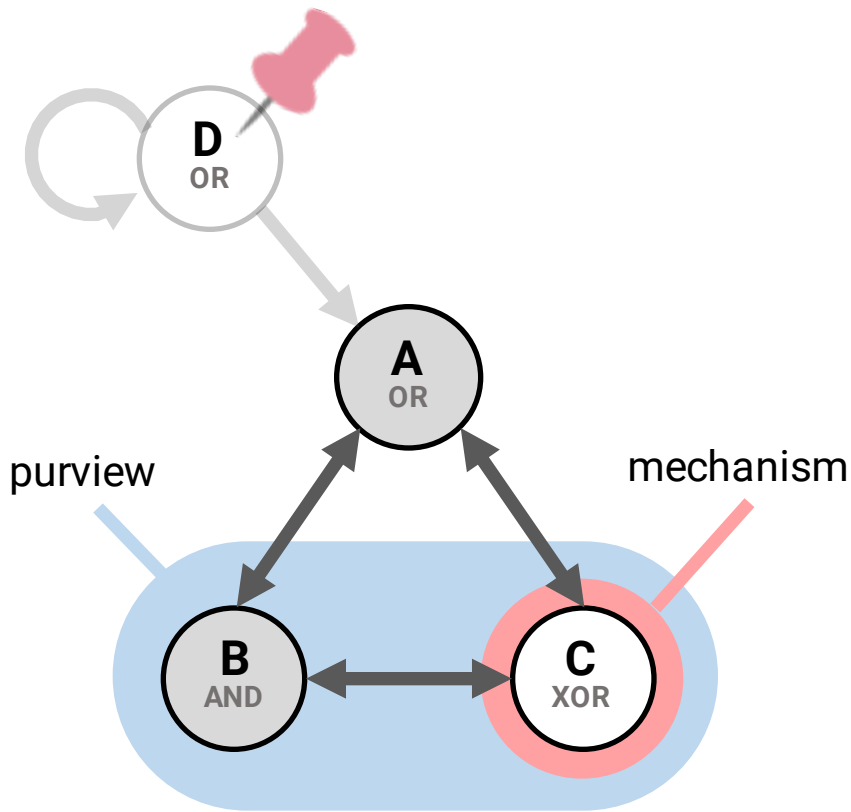

|               |                        |                        | Next state             |                        |                        |                        |                        |                        |                        |                        |
|---------------|------------------------|------------------------|------------------------|------------------------|------------------------|------------------------|------------------------|------------------------|------------------------|------------------------|
|               |                        |                        | A                      |                        |                        |                        |                        |                        |                        |                        |
|               |                        |                        | B                      |                        |                        |                        |                        |                        |                        |                        |
|               |                        |                        | C                      |                        |                        |                        |                        |                        |                        |                        |
| Current state | A                      | B                      | C                      | <div><div></div></div> | <div><div></div></div> | <div><div></div></div> | <div><div></div></div> | <div><div></div></div> | <div><div></div></div> | <div><div></div></div> |
|               | <div><div></div></div> | <div><div></div></div> | <div><div></div></div> | 1                      | 0                      | 0                      | 0                      | 0                      | 0                      | 0                      |
|               | <div><div></div></div> | <div><div></div></div> | <div><div></div></div> | 0                      | 0                      | 0                      | 0                      | 1                      | 0                      | 0                      |
|               | <div><div></div></div> | <div><div></div></div> | <div><div></div></div> | 0                      | 0                      | 0                      | 0                      | 0                      | 1                      | 0                      |
|               | <div><div></div></div> | <div><div></div></div> | <div><div></div></div> | 0                      | 1                      | 0                      | 0                      | 0                      | 0                      | 0                      |
|               | <div><div></div></div> | <div><div></div></div> | <div><div></div></div> | 0                      | 1                      | 0                      | 0                      | 0                      | 0                      | 0                      |
|               | <div><div></div></div> | <div><div></div></div> | <div><div></div></div> | 0                      | 0                      | 0                      | 0                      | 0                      | 0                      | 1                      |
|               | <div><div></div></div> | <div><div></div></div> | <div><div></div></div> | 0                      | 0                      | 0                      | 0                      | 1                      | 0                      | 0                      |
|               | <div><div></div></div> | <div><div></div></div> | <div><div></div></div> | 0                      | 0                      | 0                      | 1                      | 0                      | 0                      | 0                      |

Now let’s consider an example of both a limited mechanism and a limited purview:  
The effect repertoire of candidate mechanism **C** (red) over the purview **BC** (blue)

# Calculating an effect repertoire: Mechanism C over purview BC

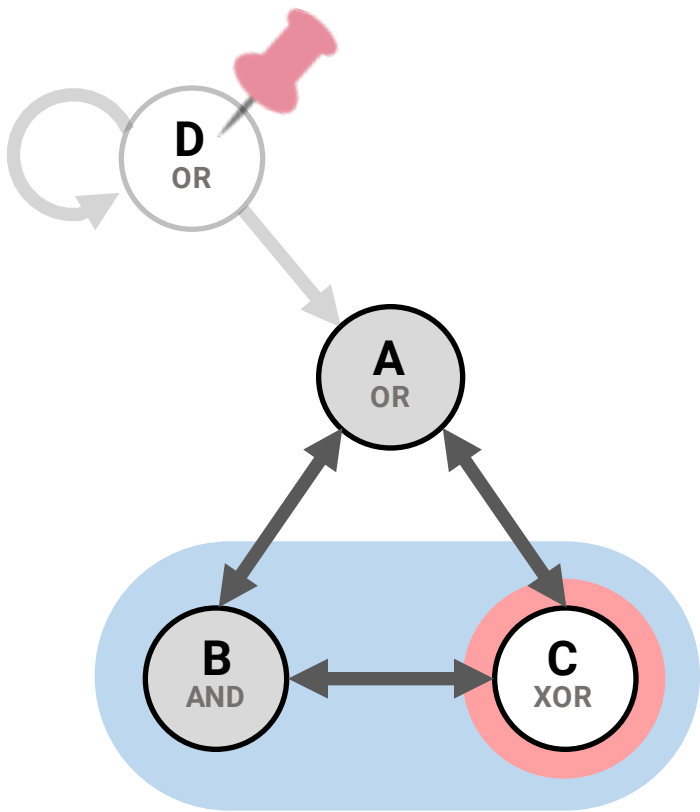

|               |   |   | Next state |   |   |   |   |   |   |   |
|---------------|---|---|------------|---|---|---|---|---|---|---|
|               |   |   | A          |   |   |   |   |   |   |   |
|               |   |   | B          |   |   |   |   |   |   |   |
|               |   |   | C          |   |   |   |   |   |   |   |
| Current state | A | B | C          |   |   |   |   |   |   |   |
|               |   |   |            | 1 | 0 | 0 | 0 | 0 | 0 | 0 |
|               |   |   |            | 0 | 0 | 0 | 0 | 1 | 0 | 0 |
|               |   |   |            | 0 | 0 | 0 | 0 | 0 | 1 | 0 |
|               |   |   |            | 0 | 1 | 0 | 0 | 0 | 0 | 0 |
|               |   |   |            | 0 | 1 | 0 | 0 | 0 | 0 | 0 |
|               |   |   |            | 0 | 0 | 0 | 0 | 0 | 0 | 1 |
|               |   |   |            | 0 | 0 | 0 | 0 | 1 | 0 | 0 |
|               |   |   |            | 0 | 0 | 0 | 1 | 0 | 0 | 0 |

The idea is to fix the current state of the mechanism **C** and perturb the other, unconstrained elements **A** and **B** into all their possible states (with equal likelihood) and observe the effects on the purview, **B** and **C**

# Calculating an effect repertoire: Mechanism C over purview BC

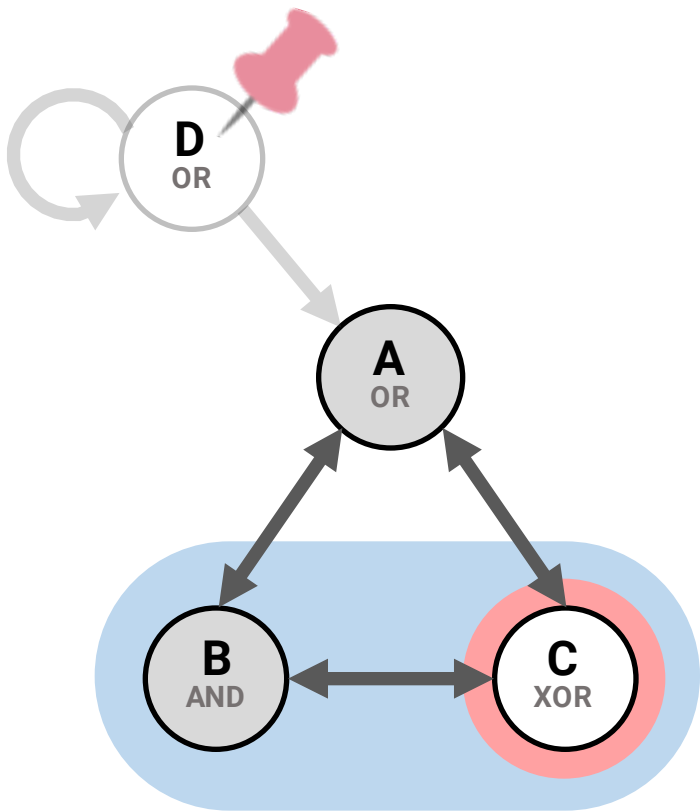

|               |                        |                        | Next state             |                        |                        |                        |                        |                        |                        |                        |
|---------------|------------------------|------------------------|------------------------|------------------------|------------------------|------------------------|------------------------|------------------------|------------------------|------------------------|
|               |                        |                        | A                      |                        |                        |                        |                        |                        |                        |                        |
|               |                        |                        | B                      |                        |                        |                        |                        |                        |                        |                        |
|               |                        |                        | C                      |                        |                        |                        |                        |                        |                        |                        |
| Current state | A                      | B                      | C                      | <div><div></div></div> | <div><div></div></div> | <div><div></div></div> | <div><div></div></div> | <div><div></div></div> | <div><div></div></div> | <div><div></div></div> |
|               | <div><div></div></div> | <div><div></div></div> | <div><div></div></div> | 1                      | 0                      | 0                      | 0                      | 0                      | 0                      | 0                      |
|               | <div><div></div></div> | <div><div></div></div> | <div><div></div></div> | 0                      | 0                      | 0                      | 0                      | 1                      | 0                      | 0                      |
|               | <div><div></div></div> | <div><div></div></div> | <div><div></div></div> | 0                      | 0                      | 0                      | 0                      | 0                      | 1                      | 0                      |
|               | <div><div></div></div> | <div><div></div></div> | <div><div></div></div> | 0                      | 1                      | 0                      | 0                      | 0                      | 0                      | 0                      |
|               | <div><div></div></div> | <div><div></div></div> | <div><div></div></div> | 0                      | 1                      | 0                      | 0                      | 0                      | 0                      | 0                      |
|               | <div><div></div></div> | <div><div></div></div> | <div><div></div></div> | 0                      | 0                      | 0                      | 0                      | 0                      | 0                      | 1                      |
|               | <div><div></div></div> | <div><div></div></div> | <div><div></div></div> | 0                      | 0                      | 0                      | 0                      | 1                      | 0                      | 0                      |
|               | <div><div></div></div> | <div><div></div></div> | <div><div></div></div> | 0                      | 0                      | 0                      | 1                      | 0                      | 0                      | 0                      |

However, note that the two purview elements **B** and **C** share common input from **A**

# Calculating an effect repertoire: Mechanism C over purview BC

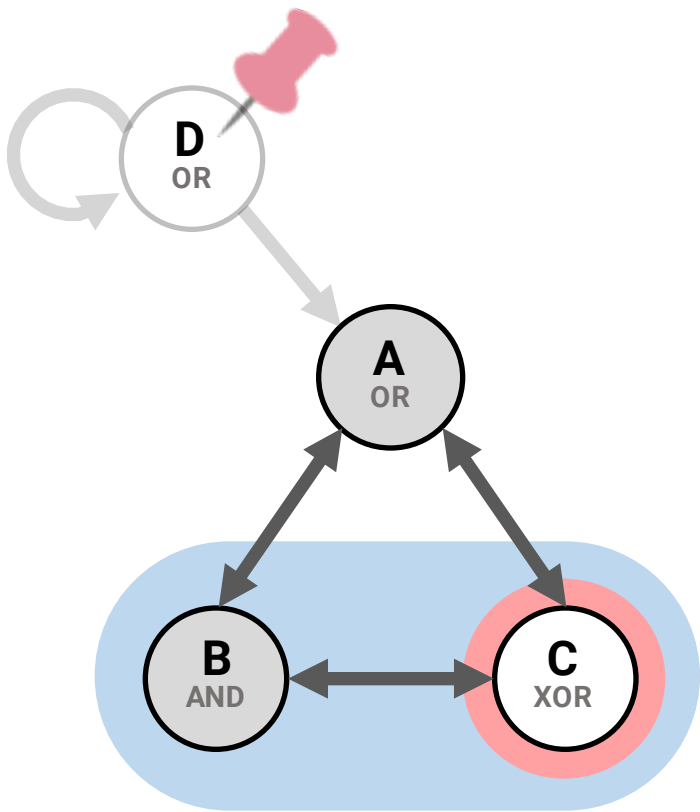

|               |   |   |   | Next state |   |   |   |   |   |   |   |
|---------------|---|---|---|------------|---|---|---|---|---|---|---|
|               |   |   |   | A          |   |   |   |   |   |   |   |
|               |   |   |   | B          |   |   |   |   |   |   |   |
|               |   |   |   | C          |   |   |   |   |   |   |   |
| Current state | A | B | C |            |   |   |   |   |   |   |   |
|               |   |   |   | 1          | 0 | 0 | 0 | 0 | 0 | 0 | 0 |
|               | 1 |   |   | 0          | 0 | 0 | 0 | 1 | 0 | 0 | 0 |
|               |   | 1 |   | 0          | 0 | 0 | 0 | 0 | 1 | 0 | 0 |
|               | 1 | 1 |   | 0          | 1 | 0 | 0 | 0 | 0 | 0 | 0 |
|               |   |   | 1 | 0          | 1 | 0 | 0 | 0 | 0 | 0 | 0 |
|               | 1 |   | 1 | 0          | 0 | 0 | 0 | 0 | 0 | 0 | 1 |
|               |   | 1 | 1 | 0          | 0 | 0 | 0 | 1 | 0 | 0 | 0 |
|               | 1 | 1 | 1 | 0          | 0 | 0 | 1 | 0 | 0 | 0 | 0 |

This means that when we set **A**’s state during the perturbation, the observed effects on **B** and **C** might depend in part on correlations due to this common input, rather than depending only on the current state of the mechanism **C**



# Calculating an effect repertoire: Virtual elements

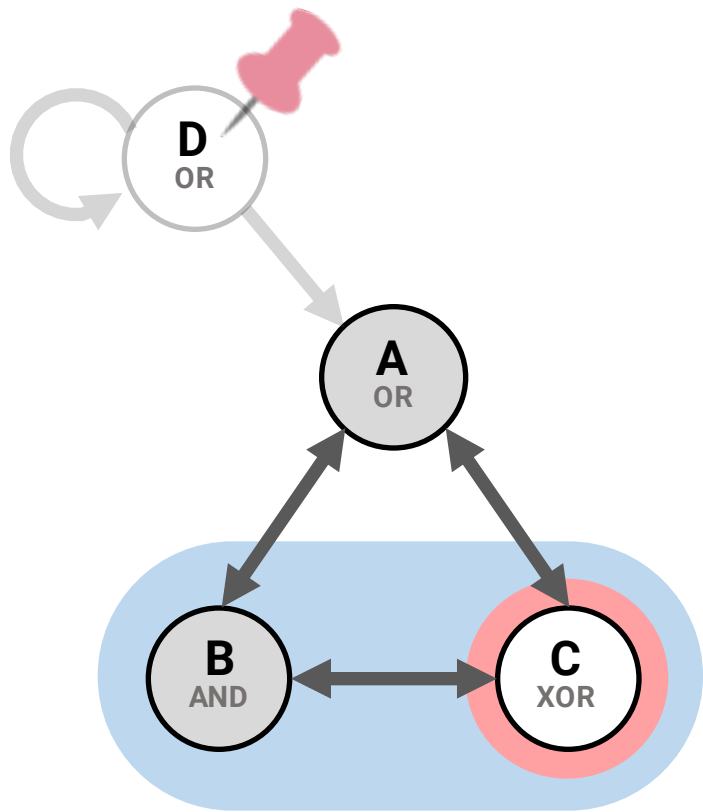

|               |   |   | Next state |   |   |   |   |   |   |   |
|---------------|---|---|------------|---|---|---|---|---|---|---|
|               |   |   | A          |   |   |   |   |   |   |   |
|               |   |   | B          |   |   |   |   |   |   |   |
|               |   |   | C          |   |   |   |   |   |   |   |
| Current state | A | B | C          |   |   |   |   |   |   |   |
|               |   |   |            | 1 | 0 | 0 | 0 | 0 | 0 | 0 |
|               |   |   |            | 0 | 0 | 0 | 0 | 1 | 0 | 0 |
|               |   |   |            | 0 | 0 | 0 | 0 | 0 | 1 | 0 |
|               |   |   |            | 0 | 1 | 0 | 0 | 0 | 0 | 0 |
|               |   |   |            | 0 | 1 | 0 | 0 | 0 | 0 | 0 |
|               |   |   |            | 0 | 0 | 0 | 0 | 0 | 0 | 1 |
|               |   |   |            | 0 | 0 | 0 | 0 | 1 | 0 | 0 |
|               |   |   |            | 0 | 0 | 0 | 1 | 0 | 0 | 0 |

To remove the unwanted effects of correlations due to common input, we introduce **virtual elements** that we can perturb independently

Calculating an effect repertoire:  
**Virtual elements**

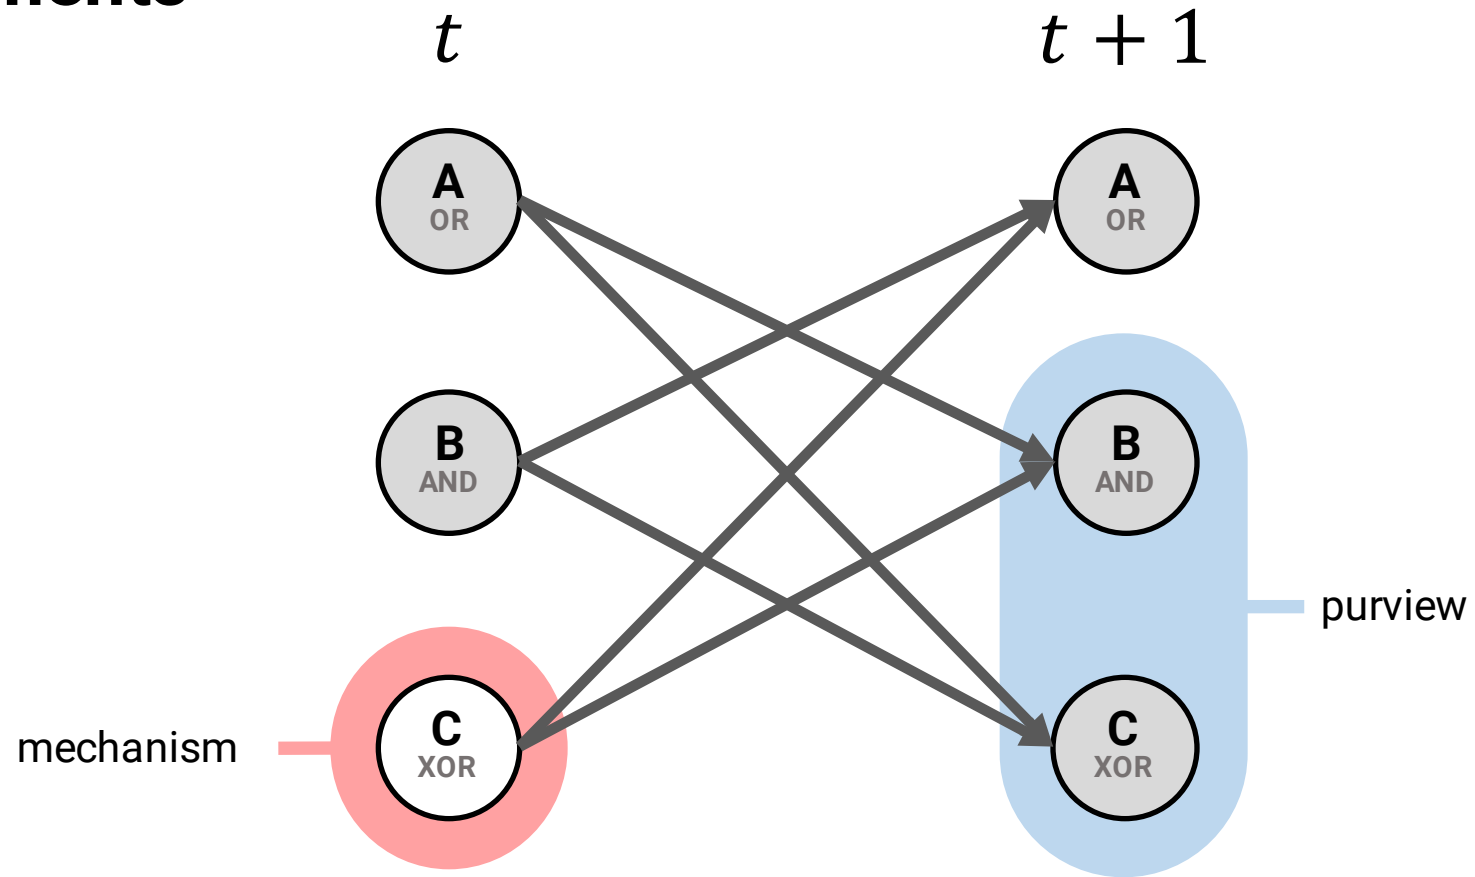

Let's unfold the graph in time between  $t$  and  $t + 1$  again

Calculating an effect repertoire:  
**Virtual elements**

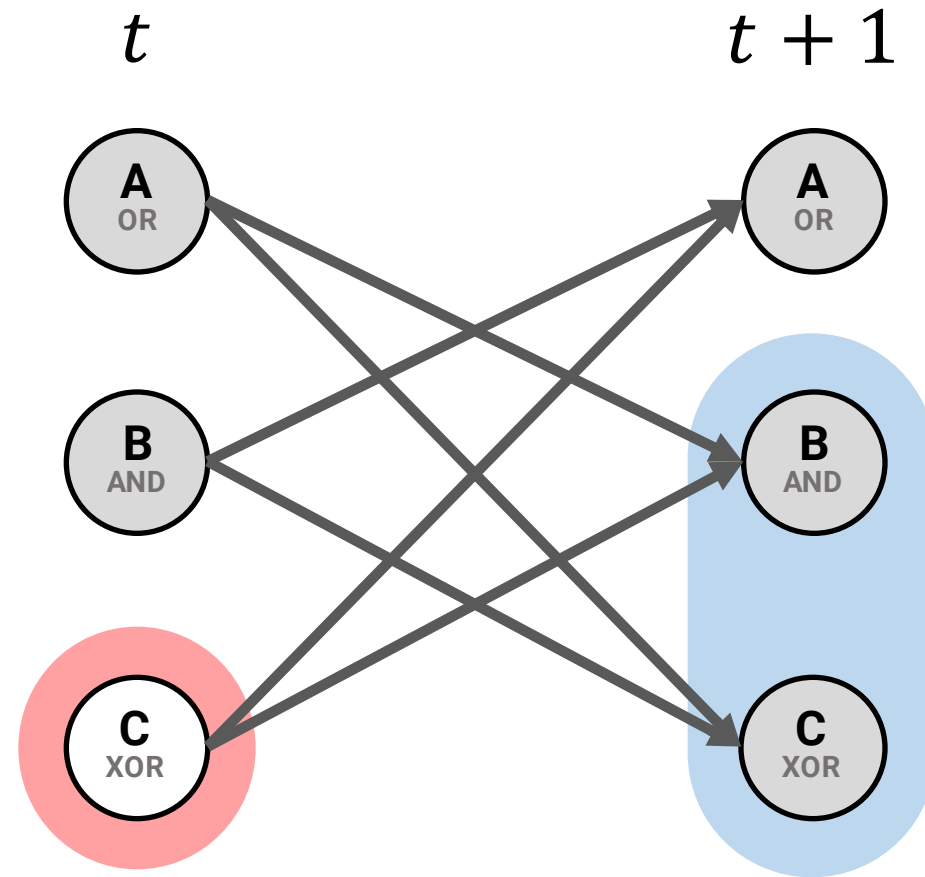

Since **A** is outside the mechanism (and thus will be perturbed) and it outputs to more than one purview element, we introduce virtual elements **A<sub>B</sub>** and **A<sub>C</sub>** at time  $t$  that independently provide input to **B** and **C**

Calculating an effect repertoire:  
**Virtual elements**

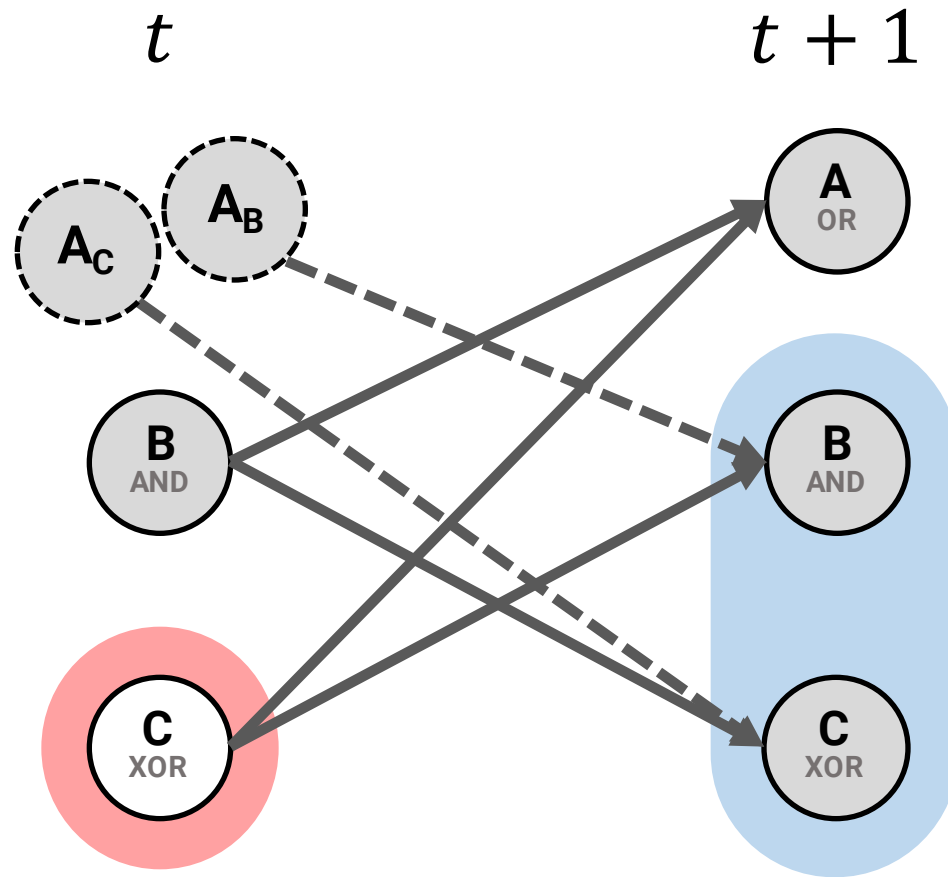

Since **A** is outside the mechanism (and thus will be perturbed) and it outputs to more than one purview element, we introduce virtual elements **A<sub>B</sub>** and **A<sub>C</sub>** at time  $t$  that independently provide input to **B** and **C**

Calculating an effect repertoire:  
**Virtual elements**

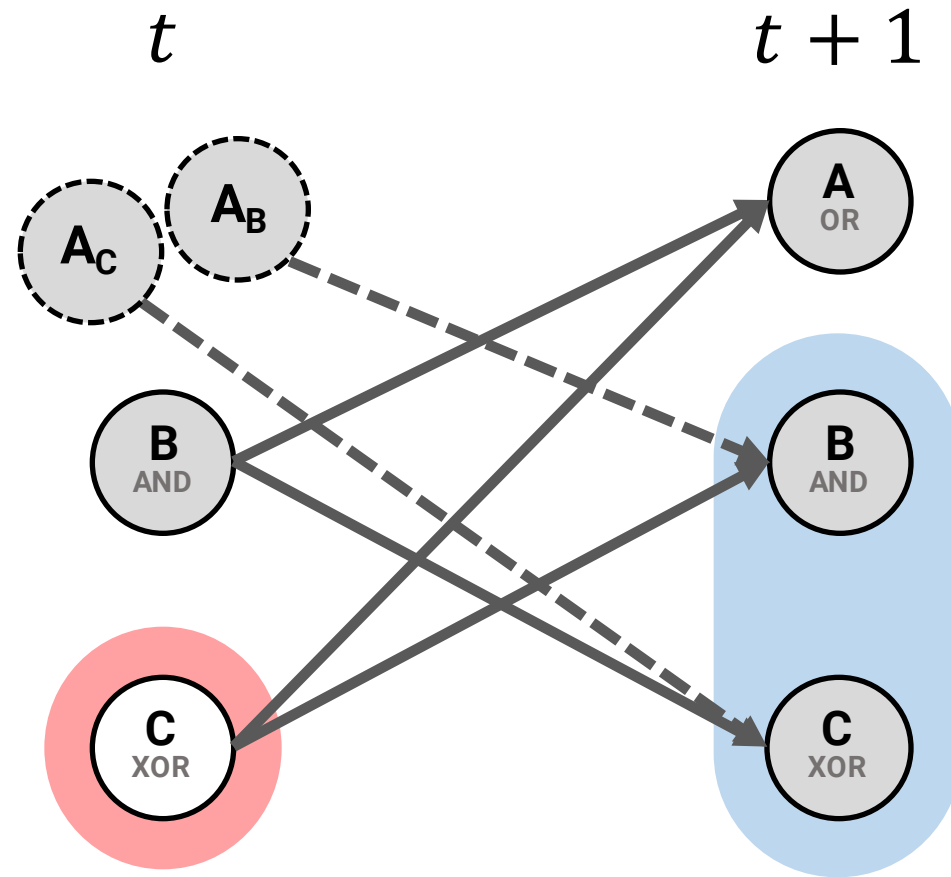

We can now perturb the non-mechanism elements into all their possible states at  $t$  to get a “virtual TPM” that doesn’t contain correlations due to common input

# Calculating an effect repertoire: Virtual elements

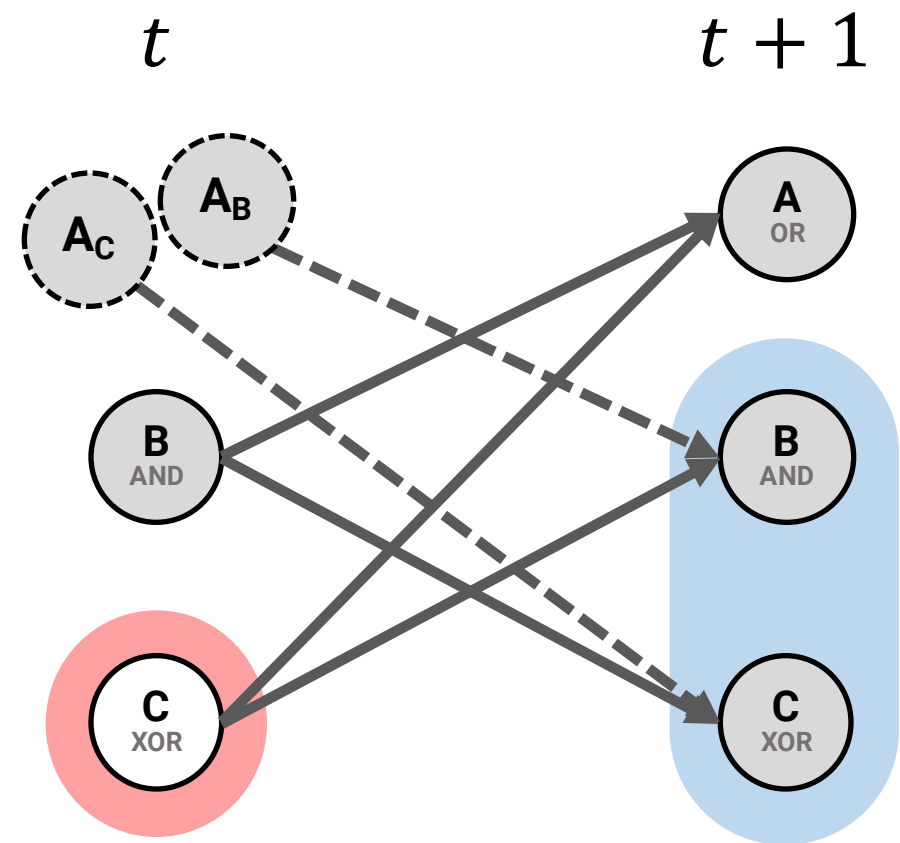

|               |                |                |   |   | Next state |   |   |   |   |   |   |   |
|---------------|----------------|----------------|---|---|------------|---|---|---|---|---|---|---|
|               |                |                |   |   | A          |   |   |   |   |   |   |   |
|               |                |                |   |   | B          |   |   |   |   |   |   |   |
|               |                |                |   |   | C          |   |   |   |   |   |   |   |
| Current state | A <sub>B</sub> | A <sub>C</sub> | B | C |            |   |   |   |   |   |   |   |
|               | ○              | ○              | ○ | ○ | 1          | 0 | 0 | 0 | 0 | 0 | 0 | 0 |
|               | ●              | ○              | ○ | ○ | 1          | 0 | 0 | 0 | 0 | 0 | 0 | 0 |
|               | ○              | ●              | ○ | ○ | 0          | 0 | 0 | 0 | 1 | 0 | 0 | 0 |
|               | ●              | ●              | ○ | ○ | 0          | 0 | 0 | 0 | 1 | 0 | 0 | 0 |
|               | ○              | ○              | ● | ○ | 0          | 0 | 0 | 0 | 0 | 1 | 0 | 0 |
|               | ●              | ○              | ● | ○ | 0          | 0 | 0 | 0 | 0 | 1 | 0 | 0 |
|               | ○              | ●              | ● | ○ | 0          | 1 | 0 | 0 | 0 | 0 | 0 | 0 |
|               | ●              | ●              | ● | ○ | 0          | 1 | 0 | 0 | 0 | 0 | 0 | 0 |
|               | ○              | ○              | ○ | ● | 0          | 1 | 0 | 0 | 0 | 0 | 0 | 0 |
|               | ●              | ○              | ○ | ● | 0          | 0 | 0 | 1 | 0 | 0 | 0 | 0 |
|               | ○              | ●              | ○ | ● | 0          | 0 | 0 | 0 | 0 | 1 | 0 | 0 |
|               | ●              | ●              | ○ | ● | 0          | 0 | 0 | 0 | 0 | 0 | 0 | 1 |
|               | ○              | ○              | ● | ● | 0          | 0 | 0 | 0 | 0 | 1 | 0 | 0 |
|               | ●              | ○              | ● | ● | 0          | 0 | 0 | 0 | 0 | 0 | 0 | 1 |
|               | ○              | ●              | ● | ● | 0          | 1 | 0 | 0 | 0 | 0 | 0 | 0 |
|               | ●              | ●              | ● | ● | 0          | 0 | 0 | 1 | 0 | 0 | 0 | 0 |

We can now perturb the non-mechanism elements into all their possible states at  $t$  to get a “virtual TPM” that doesn’t contain correlations due to common input

# Calculating an effect repertoire: Virtual elements

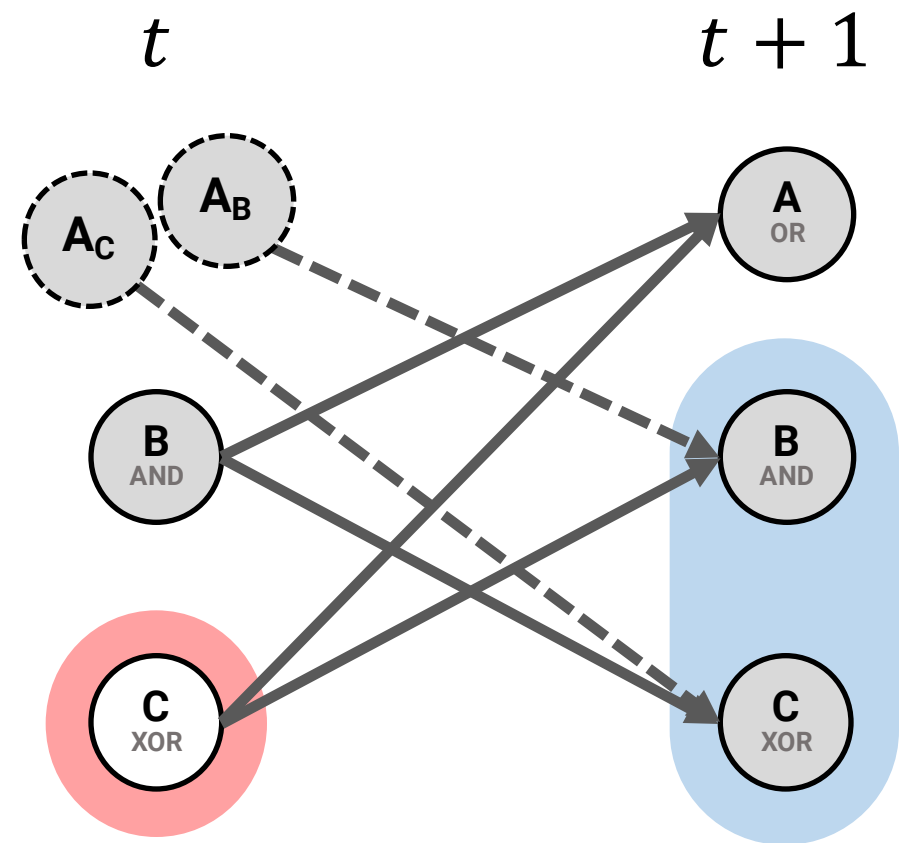

|               |                |                |   | Next state |   |   |   |   |   |   |   |
|---------------|----------------|----------------|---|------------|---|---|---|---|---|---|---|
|               |                |                |   | A          |   |   |   |   |   |   |   |
|               |                |                |   | B          |   |   |   |   |   |   |   |
|               |                |                |   | C          |   |   |   |   |   |   |   |
| Current state | A <sub>B</sub> | A <sub>C</sub> | B | C          |   |   |   |   |   |   |   |
|               |                |                |   |            | 1 | 0 | 0 | 0 | 0 | 0 | 0 |
|               |                |                |   |            | 1 | 0 | 0 | 0 | 0 | 0 | 0 |
|               |                |                |   |            | 0 | 0 | 0 | 0 | 1 | 0 | 0 |
|               |                |                |   |            | 0 | 0 | 0 | 0 | 1 | 0 | 0 |
|               |                |                |   |            | 0 | 0 | 0 | 0 | 0 | 1 | 0 |
|               |                |                |   |            | 0 | 0 | 0 | 0 | 0 | 1 | 0 |
|               |                |                |   |            | 0 | 1 | 0 | 0 | 0 | 0 | 0 |
|               |                |                |   |            | 0 | 1 | 0 | 0 | 0 | 0 | 0 |
|               |                |                |   |            | 0 | 1 | 0 | 0 | 0 | 0 | 0 |
|               |                |                |   |            | 0 | 0 | 0 | 1 | 0 | 0 | 0 |
|               |                |                |   |            | 0 | 0 | 0 | 0 | 0 | 1 | 0 |
|               |                |                |   |            | 0 | 0 | 0 | 0 | 0 | 0 | 1 |
|               |                |                |   |            | 0 | 0 | 0 | 0 | 0 | 1 | 0 |
|               |                |                |   |            | 0 | 0 | 0 | 0 | 0 | 0 | 1 |

Now, since we’re only interested in how the current state of **C** constrains the next state of the purview **BC**, rather than the whole system, we want to **ignore** the next state of **A**

# Calculating an effect repertoire: Virtual elements

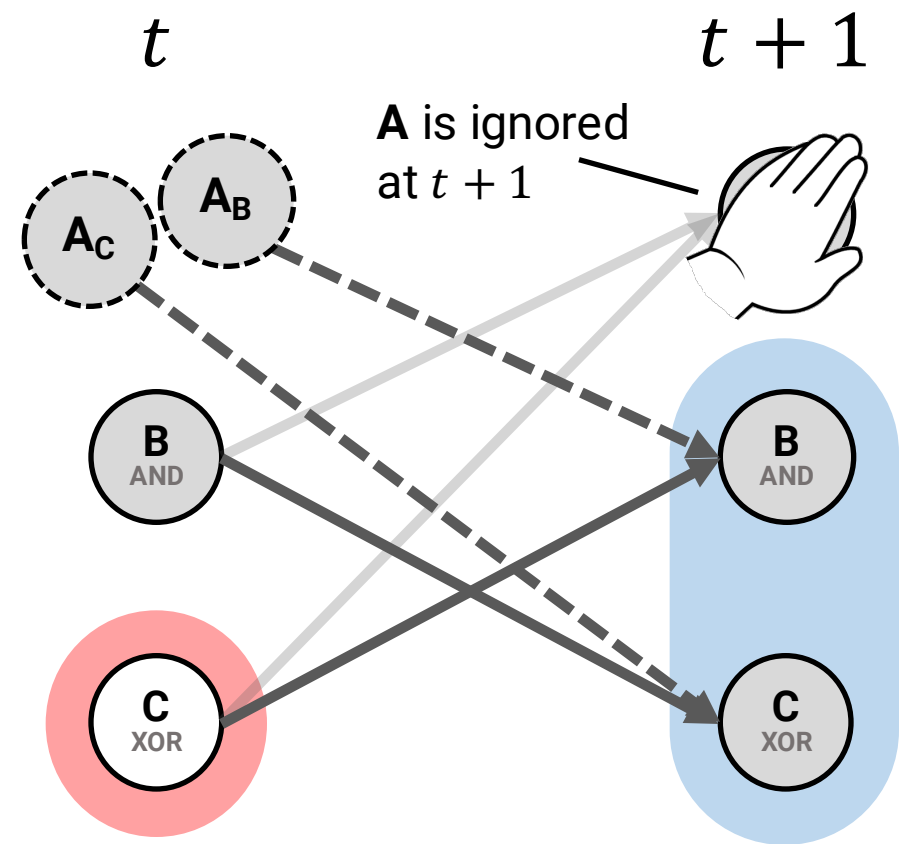

|               |       |       |   | Next state |   |   |   |   |   |   |   |
|---------------|-------|-------|---|------------|---|---|---|---|---|---|---|
|               |       |       |   | A          |   |   |   |   |   |   |   |
|               |       |       |   | B          |   |   |   |   |   |   |   |
|               |       |       |   | C          |   |   |   |   |   |   |   |
| Current state | $A_B$ | $A_C$ | B | C          |   |   |   |   |   |   |   |
|               | ○     | ○     | ○ | ○          | 1 | 0 | 0 | 0 | 0 | 0 | 0 |
|               | ●     | ○     | ○ | ○          | 1 | 0 | 0 | 0 | 0 | 0 | 0 |
|               | ○     | ●     | ○ | ○          | 0 | 0 | 0 | 0 | 1 | 0 | 0 |
|               | ●     | ●     | ○ | ○          | 0 | 0 | 0 | 0 | 1 | 0 | 0 |
|               | ○     | ○     | ● | ○          | 0 | 0 | 0 | 0 | 0 | 1 | 0 |
|               | ●     | ○     | ● | ○          | 0 | 0 | 0 | 0 | 0 | 1 | 0 |
|               | ○     | ●     | ● | ○          | 0 | 1 | 0 | 0 | 0 | 0 | 0 |
|               | ●     | ●     | ● | ○          | 0 | 1 | 0 | 0 | 0 | 0 | 0 |
|               | ○     | ○     | ○ | ●          | 0 | 1 | 0 | 0 | 0 | 0 | 0 |
|               | ●     | ○     | ○ | ●          | 0 | 0 | 0 | 1 | 0 | 0 | 0 |
|               | ○     | ●     | ○ | ●          | 0 | 0 | 0 | 0 | 0 | 1 | 0 |
|               | ●     | ●     | ○ | ●          | 0 | 0 | 0 | 0 | 0 | 0 | 1 |
|               | ○     | ○     | ● | ●          | 0 | 0 | 0 | 0 | 0 | 1 | 0 |
|               | ●     | ○     | ● | ●          | 0 | 0 | 0 | 0 | 0 | 0 | 1 |
|               | ○     | ●     | ● | ●          | 0 | 1 | 0 | 0 | 0 | 0 | 0 |
|               | ●     | ●     | ● | ●          | 0 | 0 | 0 | 1 | 0 | 0 | 0 |

Now, since we’re only interested in how the current state of **C** constrains the next state of the purview **BC**, rather than the whole system, we want to **ignore** the next state of **A**



# Calculating an effect repertoire: Marginalizing-out non-purview elements

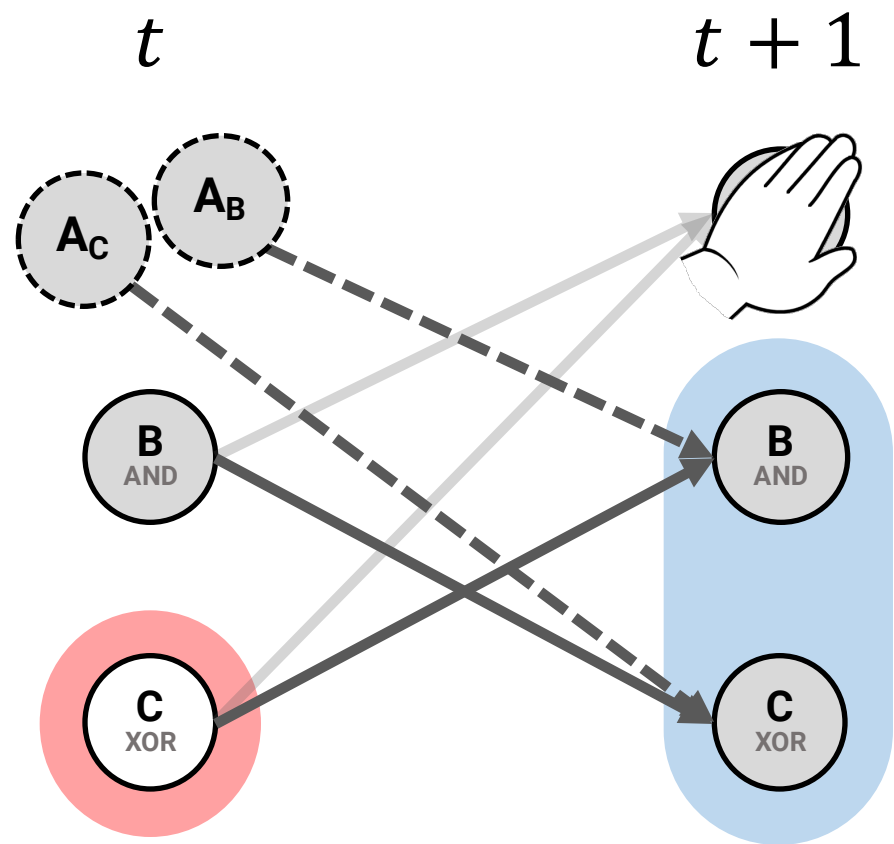

|               |                |                |   | Next state |   |   |   |   |   |   |   |
|---------------|----------------|----------------|---|------------|---|---|---|---|---|---|---|
|               |                |                |   | A          |   |   |   |   |   |   |   |
|               |                |                |   | B          |   |   |   |   |   |   |   |
|               |                |                |   | C          |   |   |   |   |   |   |   |
| Current state | A <sub>B</sub> | A <sub>C</sub> | B | C          |   |   |   |   |   |   |   |
|               | ○              | ○              | ○ | ○          | 1 | 0 | 0 | 0 | 0 | 0 | 0 |
|               | ●              | ○              | ○ | ○          | 1 | 0 | 0 | 0 | 0 | 0 | 0 |
|               | ○              | ●              | ○ | ○          | 0 | 0 | 0 | 0 | 1 | 0 | 0 |
|               | ●              | ●              | ○ | ○          | 0 | 0 | 0 | 0 | 1 | 0 | 0 |
|               | ○              | ○              | ● | ○          | 0 | 0 | 0 | 0 | 0 | 1 | 0 |
|               | ●              | ○              | ● | ○          | 0 | 0 | 0 | 0 | 0 | 1 | 0 |
|               | ○              | ●              | ● | ○          | 0 | 1 | 0 | 0 | 0 | 0 | 0 |
|               | ●              | ●              | ● | ○          | 0 | 1 | 0 | 0 | 0 | 0 | 0 |
|               | ○              | ○              | ○ | ●          | 0 | 1 | 0 | 0 | 0 | 0 | 0 |
|               | ●              | ○              | ○ | ●          | 0 | 0 | 0 | 1 | 0 | 0 | 0 |
|               | ○              | ●              | ○ | ●          | 0 | 0 | 0 | 0 | 0 | 1 | 0 |
|               | ●              | ●              | ○ | ●          | 0 | 0 | 0 | 0 | 0 | 0 | 1 |
|               | ○              | ○              | ● | ●          | 0 | 0 | 0 | 0 | 0 | 1 | 0 |
|               | ●              | ○              | ● | ●          | 0 | 0 | 0 | 0 | 0 | 0 | 1 |
|               | ○              | ●              | ● | ●          | 0 | 1 | 0 | 0 | 0 | 0 | 0 |
|               | ●              | ●              | ● | ●          | 0 | 0 | 0 | 1 | 0 | 0 | 0 |

As usual, ignoring the next state of **A** corresponds to **marginalizing it out** of the TPM

# Calculating an effect repertoire: Marginalizing-out non-purview elements

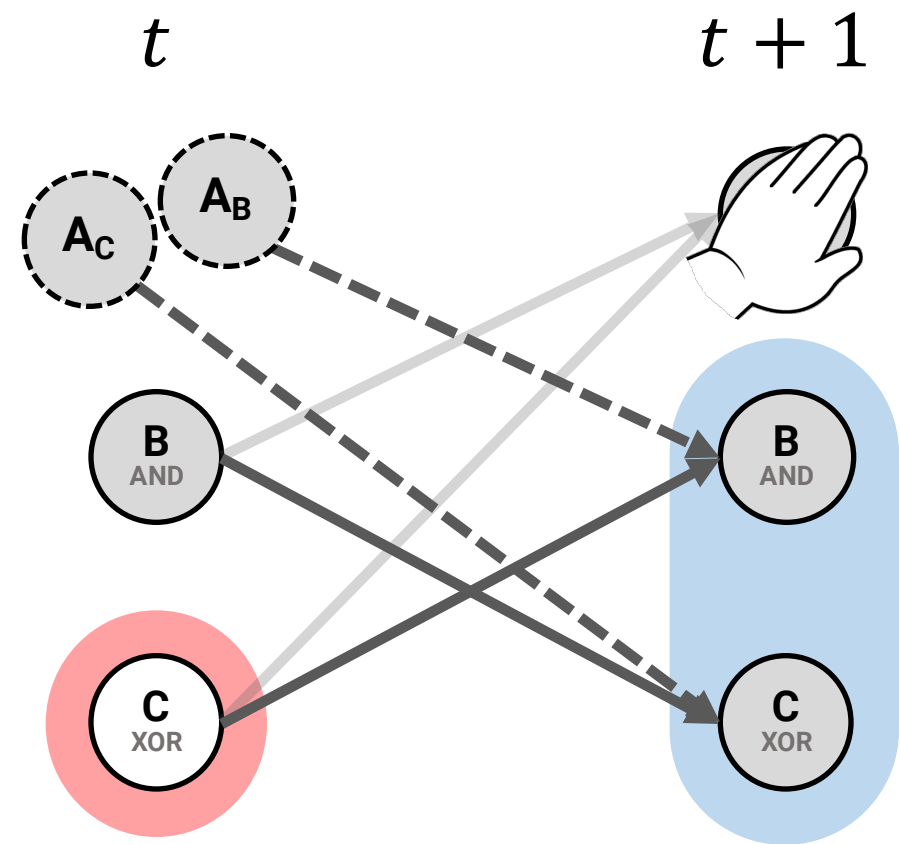

|               |                |                |   | Next state |   |   |   |   |   |   |   |
|---------------|----------------|----------------|---|------------|---|---|---|---|---|---|---|
|               |                |                |   | A          |   |   |   |   |   |   |   |
|               |                |                |   | B          |   |   |   |   |   |   |   |
|               |                |                |   | C          |   |   |   |   |   |   |   |
| Current state | A <sub>B</sub> | A <sub>C</sub> | B | C          |   |   |   |   |   |   |   |
|               | ○              | ○              | ○ | ○          | 1 | 0 | 0 | 0 | 0 | 0 | 0 |
|               | ●              | ○              | ○ | ○          | 1 | 0 | 0 | 0 | 0 | 0 | 0 |
|               | ○              | ●              | ○ | ○          | 0 | 0 | 0 | 0 | 1 | 0 | 0 |
|               | ●              | ●              | ○ | ○          | 0 | 0 | 0 | 0 | 1 | 0 | 0 |
|               | ○              | ○              | ● | ○          | 0 | 0 | 0 | 0 | 0 | 1 | 0 |
|               | ●              | ○              | ● | ○          | 0 | 0 | 0 | 0 | 0 | 1 | 0 |
|               | ○              | ●              | ● | ○          | 0 | 1 | 0 | 0 | 0 | 0 | 0 |
|               | ●              | ●              | ● | ○          | 0 | 1 | 0 | 0 | 0 | 0 | 0 |
|               | ○              | ○              | ○ | ●          | 0 | 1 | 0 | 0 | 0 | 0 | 0 |
|               | ●              | ○              | ○ | ●          | 0 | 0 | 0 | 1 | 0 | 0 | 0 |
|               | ○              | ●              | ○ | ●          | 0 | 0 | 0 | 0 | 0 | 1 | 0 |
|               | ●              | ●              | ○ | ●          | 0 | 0 | 0 | 0 | 0 | 0 | 1 |
|               | ○              | ○              | ● | ●          | 0 | 0 | 0 | 0 | 0 | 1 | 0 |
|               | ●              | ○              | ● | ●          | 0 | 0 | 0 | 0 | 0 | 0 | 1 |
|               | ○              | ●              | ● | ●          | 0 | 1 | 0 | 0 | 0 | 0 | 0 |
|               | ●              | ●              | ● | ●          | 0 | 0 | 0 | 1 | 0 | 0 | 0 |

The process is the same as when we marginalized-out **D** as a background condition:  
We sum pairs of columns whose corresponding states differ only by **A**'s state

# Calculating an effect repertoire: Marginalizing-out non-purview elements

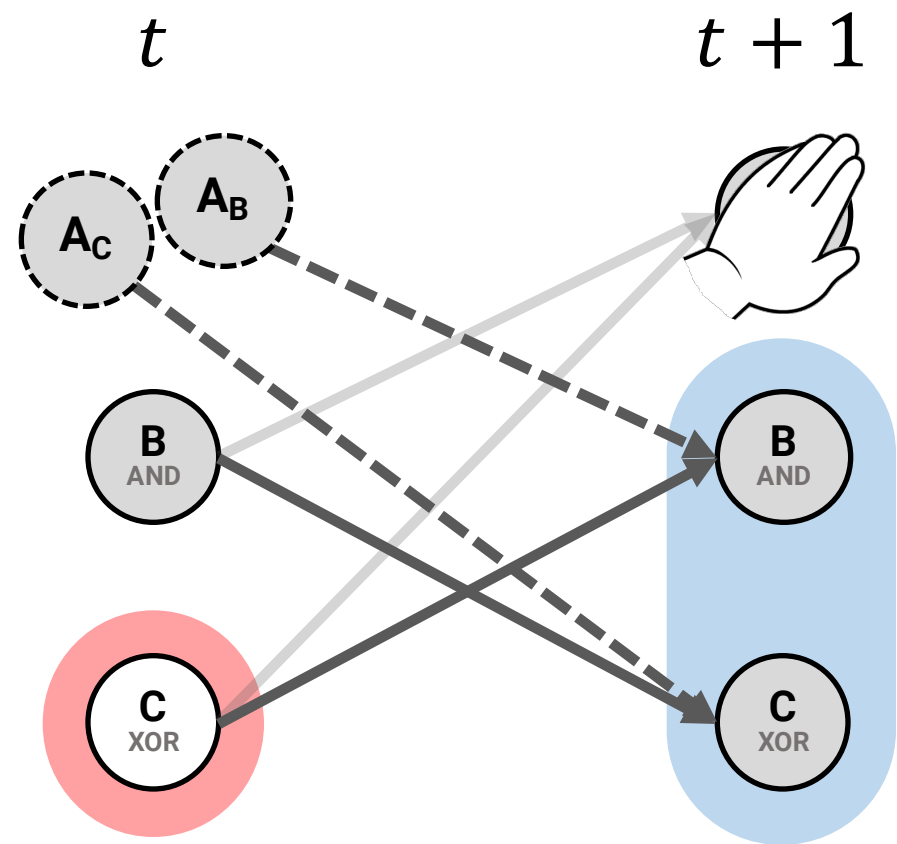

|               |                |                |   | Next state |   |   |   |   |   |   |   |
|---------------|----------------|----------------|---|------------|---|---|---|---|---|---|---|
|               |                |                |   | A          |   |   |   |   |   |   |   |
|               |                |                |   | B          |   |   |   |   |   |   |   |
|               |                |                |   | C          |   |   |   |   |   |   |   |
| Current state | A <sub>B</sub> | A <sub>C</sub> | B | C          |   |   |   |   |   |   |   |
|               | ○              | ○              | ○ | ○          | 1 | 0 | 0 | 0 | 0 | 0 | 0 |
|               | ●              | ○              | ○ | ○          | 1 | 0 | 0 | 0 | 0 | 0 | 0 |
|               | ○              | ●              | ○ | ○          | 0 | 0 | 0 | 0 | 1 | 0 | 0 |
|               | ●              | ●              | ○ | ○          | 0 | 0 | 0 | 0 | 1 | 0 | 0 |
|               | ○              | ○              | ● | ○          | 0 | 0 | 0 | 0 | 0 | 1 | 0 |
|               | ●              | ○              | ● | ○          | 0 | 0 | 0 | 0 | 0 | 1 | 0 |
|               | ○              | ●              | ● | ○          | 0 | 1 | 0 | 0 | 0 | 0 | 0 |
|               | ●              | ●              | ● | ○          | 0 | 1 | 0 | 0 | 0 | 0 | 0 |
|               | ○              | ○              | ○ | ●          | 0 | 1 | 0 | 0 | 0 | 0 | 0 |
|               | ●              | ○              | ○ | ●          | 0 | 0 | 0 | 1 | 0 | 0 | 0 |
|               | ○              | ●              | ○ | ●          | 0 | 0 | 0 | 0 | 0 | 1 | 0 |
|               | ●              | ●              | ○ | ●          | 0 | 0 | 0 | 0 | 0 | 0 | 1 |
|               | ○              | ○              | ● | ●          | 0 | 0 | 0 | 0 | 0 | 1 | 0 |
|               | ●              | ○              | ● | ●          | 0 | 0 | 0 | 0 | 0 | 0 | 1 |
|               | ○              | ●              | ● | ●          | 0 | 1 | 0 | 0 | 0 | 0 | 0 |
|               | ●              | ●              | ● | ●          | 0 | 0 | 0 | 1 | 0 | 0 | 0 |

The process is the same as when we marginalized-out **D** as a background condition:  
We sum pairs of columns whose corresponding states differ only by **A**'s state

# Calculating an effect repertoire: Marginalizing-out non-purview elements

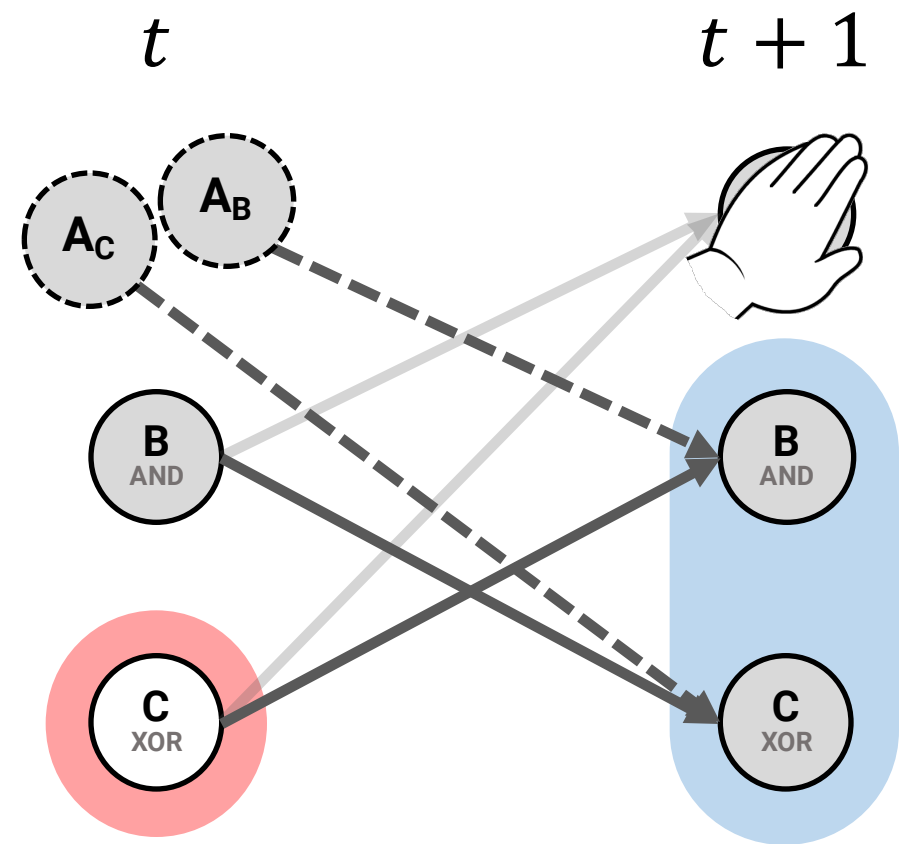

|               |                |                |   | Next state |   |   |   |
|---------------|----------------|----------------|---|------------|---|---|---|
|               |                |                |   | A          |   |   |   |
|               |                |                |   | B          |   |   |   |
|               |                |                |   | C          |   |   |   |
| Current state | A <sub>B</sub> | A <sub>C</sub> | B | C          |   |   |   |
|               | ○              | ○              | ○ | ○          | 1 | 0 | 0 |
|               | ●              | ○              | ○ | ○          | 1 | 0 | 0 |
|               | ○              | ●              | ○ | ○          | 0 | 0 | 1 |
|               | ●              | ●              | ○ | ○          | 0 | 0 | 1 |
|               | ○              | ○              | ● | ○          | 0 | 0 | 1 |
|               | ●              | ○              | ● | ○          | 0 | 0 | 1 |
|               | ○              | ●              | ● | ○          | 1 | 0 | 0 |
|               | ●              | ●              | ● | ○          | 1 | 0 | 0 |
|               | ○              | ○              | ○ | ●          | 1 | 0 | 0 |
|               | ●              | ○              | ○ | ●          | 0 | 1 | 0 |
|               | ○              | ●              | ○ | ●          | 0 | 0 | 1 |
|               | ●              | ●              | ○ | ●          | 0 | 0 | 0 |
|               | ○              | ○              | ● | ●          | 0 | 0 | 1 |
|               | ●              | ○              | ● | ●          | 0 | 0 | 1 |
|               | ○              | ●              | ● | ●          | 1 | 0 | 0 |
|               | ●              | ●              | ● | ●          | 0 | 1 | 0 |

The process is the same as when we marginalized-out **D** as a background condition:  
We sum pairs of columns whose corresponding states differ only by **A**'s state

# Calculating an effect repertoire: Marginalizing-out non-purview elements

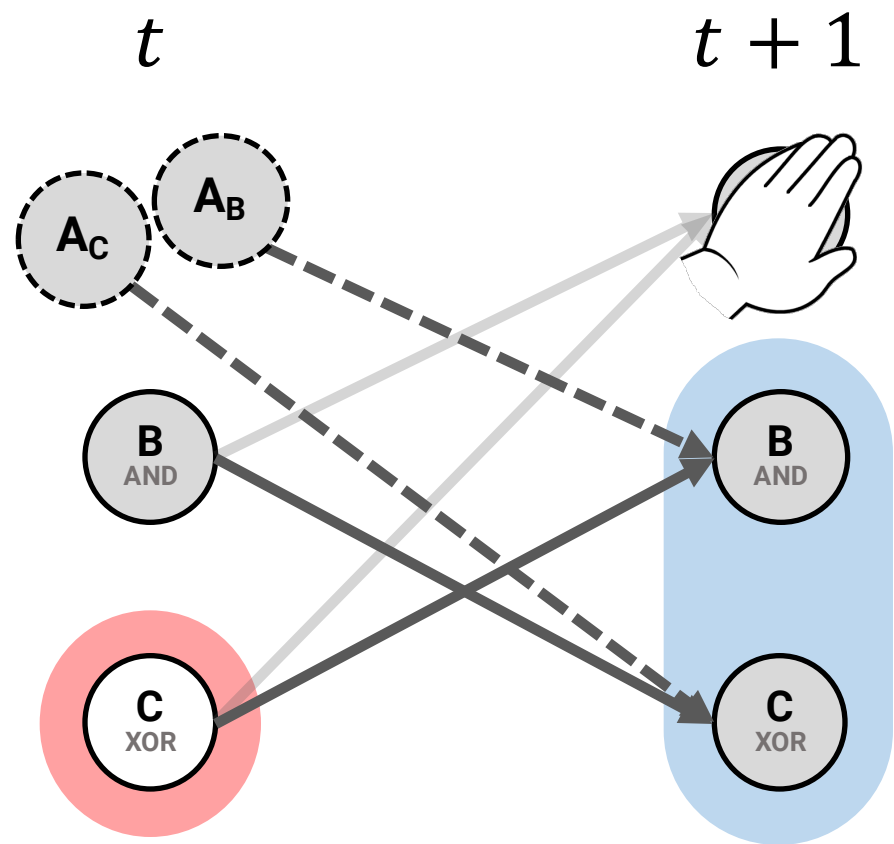

|               |                |                |              |              | Next state |   |   |   |
|---------------|----------------|----------------|--------------|--------------|------------|---|---|---|
| Current state |                |                |              |              | B          |   |   |   |
|               |                |                |              |              | C          |   |   |   |
|               | A <sub>B</sub> | A <sub>C</sub> | B            | C            |            |   |   |   |
|               | <div>○</div>   | <div>○</div>   | <div>○</div> | <div>○</div> | 1          | 0 | 0 | 0 |
|               | <div>●</div>   | <div>○</div>   | <div>○</div> | <div>○</div> | 1          | 0 | 0 | 0 |
|               | <div>○</div>   | <div>●</div>   | <div>○</div> | <div>○</div> | 0          | 0 | 1 | 0 |
|               | <div>●</div>   | <div>●</div>   | <div>○</div> | <div>○</div> | 0          | 0 | 1 | 0 |
|               | <div>○</div>   | <div>○</div>   | <div>●</div> | <div>○</div> | 0          | 0 | 1 | 0 |
|               | <div>●</div>   | <div>○</div>   | <div>●</div> | <div>○</div> | 0          | 0 | 1 | 0 |
|               | <div>○</div>   | <div>●</div>   | <div>●</div> | <div>○</div> | 1          | 0 | 0 | 0 |
|               | <div>●</div>   | <div>●</div>   | <div>●</div> | <div>○</div> | 1          | 0 | 0 | 0 |
|               | <div>○</div>   | <div>○</div>   | <div>○</div> | <div>●</div> | 1          | 0 | 0 | 0 |
|               | <div>●</div>   | <div>○</div>   | <div>○</div> | <div>●</div> | 0          | 1 | 0 | 0 |
|               | <div>○</div>   | <div>●</div>   | <div>○</div> | <div>●</div> | 0          | 0 | 1 | 0 |
|               | <div>●</div>   | <div>●</div>   | <div>○</div> | <div>●</div> | 0          | 0 | 0 | 1 |
|               | <div>○</div>   | <div>○</div>   | <div>●</div> | <div>●</div> | 0          | 0 | 1 | 0 |
|               | <div>●</div>   | <div>○</div>   | <div>●</div> | <div>●</div> | 0          | 0 | 0 | 1 |
| <div>○</div>  | <div>●</div>   | <div>●</div>   | <div>●</div> | 1            | 0          | 0 | 0 |   |
| <div>●</div>  | <div>●</div>   | <div>●</div>   | <div>●</div> | 0            | 1          | 0 | 0 |   |

The process is the same as when we marginalized-out **D** as a background condition:  
We sum pairs of columns whose corresponding states differ only by **A**'s state

# Calculating an effect repertoire: Marginalizing-out non-purview elements

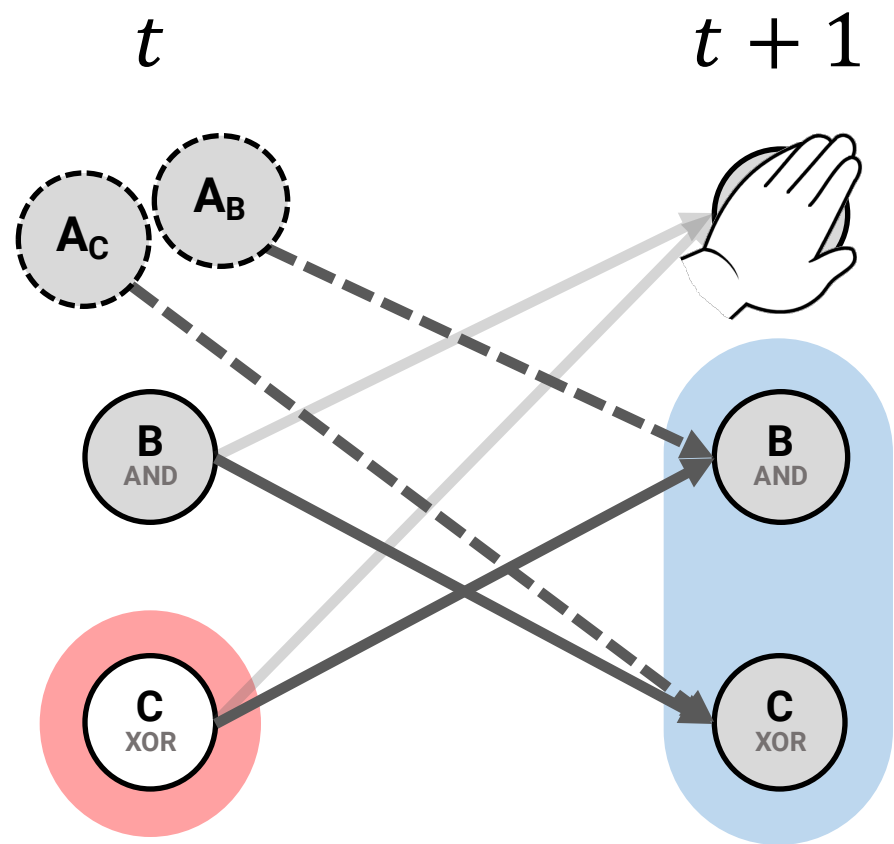

|               |                |                |   | Next state |   |   |   |
|---------------|----------------|----------------|---|------------|---|---|---|
|               |                |                |   | B          |   |   |   |
|               |                |                |   | C          |   |   |   |
| Current state | A <sub>B</sub> | A <sub>C</sub> | B | C          |   |   |   |
|               | ○              | ○              | ○ | ○          | 1 | 0 | 0 |
|               | ●              | ○              | ○ | ○          | 1 | 0 | 0 |
|               | ○              | ●              | ○ | ○          | 0 | 0 | 1 |
|               | ●              | ●              | ○ | ○          | 0 | 0 | 1 |
|               | ○              | ○              | ● | ○          | 0 | 0 | 1 |
|               | ●              | ○              | ● | ○          | 0 | 0 | 1 |
|               | ○              | ●              | ● | ○          | 1 | 0 | 0 |
|               | ●              | ●              | ● | ○          | 1 | 0 | 0 |
|               | ○              | ○              | ○ | ●          | 1 | 0 | 0 |
|               | ●              | ○              | ○ | ●          | 0 | 1 | 0 |
|               | ○              | ●              | ○ | ●          | 0 | 0 | 1 |
|               | ●              | ●              | ○ | ●          | 0 | 0 | 0 |
|               | ○              | ○              | ● | ●          | 0 | 0 | 1 |
|               | ●              | ○              | ● | ●          | 0 | 0 | 1 |
|               | ○              | ●              | ● | ●          | 1 | 0 | 0 |
|               | ●              | ●              | ● | ●          | 0 | 1 | 0 |

The process is the same as when we marginalized-out **D** as a background condition:  
We sum pairs of columns whose corresponding states differ only by **A**'s state

# Calculating an effect repertoire: Marginalizing-out non-mechanism elements

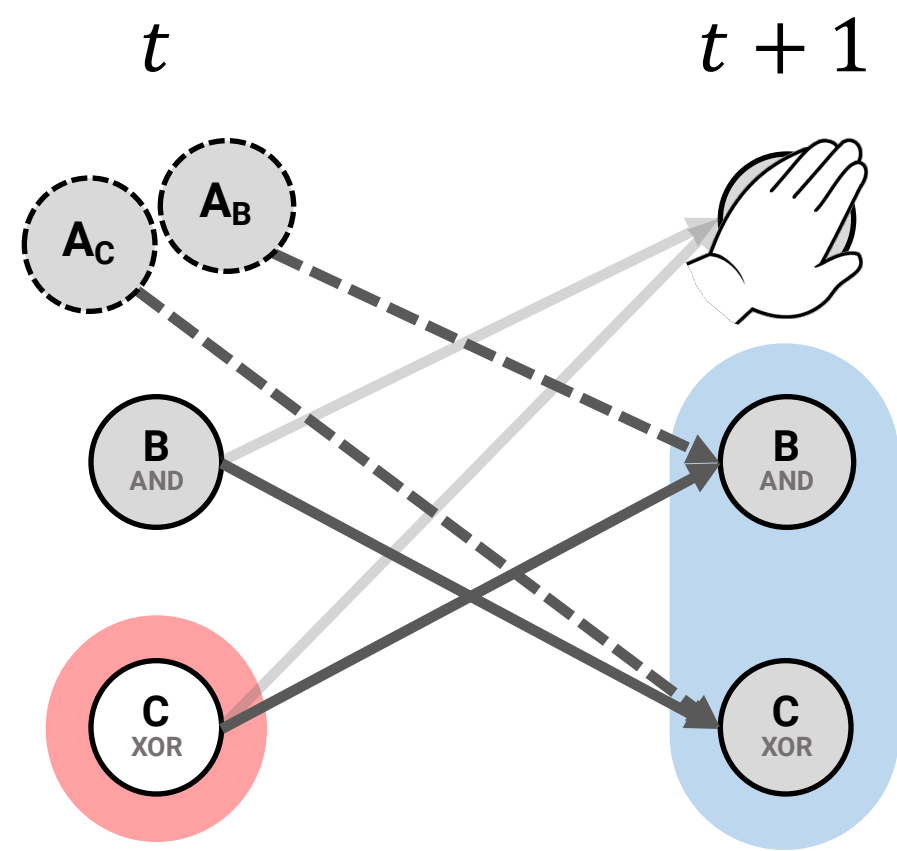

|               |                |                |   | Next state |   |   |   |
|---------------|----------------|----------------|---|------------|---|---|---|
|               |                |                |   | B          |   |   |   |
|               |                |                |   | C          |   |   |   |
| Current state | A <sub>B</sub> | A <sub>C</sub> | B | C          |   |   |   |
|               | ○              | ○              | ○ | ○          | 1 | 0 | 0 |
|               | ●              | ○              | ○ | ○          | 1 | 0 | 0 |
|               | ○              | ●              | ○ | ○          | 0 | 0 | 1 |
|               | ●              | ●              | ○ | ○          | 0 | 0 | 1 |
|               | ○              | ○              | ● | ○          | 0 | 0 | 1 |
|               | ●              | ○              | ● | ○          | 0 | 0 | 1 |
|               | ○              | ●              | ● | ○          | 1 | 0 | 0 |
|               | ●              | ●              | ● | ○          | 1 | 0 | 0 |
|               | ○              | ○              | ○ | ●          | 1 | 0 | 0 |
|               | ●              | ○              | ○ | ●          | 0 | 1 | 0 |
|               | ○              | ●              | ○ | ●          | 0 | 0 | 1 |
|               | ●              | ●              | ○ | ●          | 0 | 0 | 0 |
|               | ○              | ○              | ● | ●          | 0 | 0 | 1 |
|               | ●              | ○              | ● | ●          | 0 | 0 | 1 |
|               | ○              | ●              | ● | ●          | 1 | 0 | 0 |
|               | ●              | ●              | ● | ●          | 0 | 1 | 0 |

Now, to find the effect repertoire of the mechanism, **C**, as before, we want a TPM that gives the probabilities of next purview states given **only** the current state of **C**

# Calculating an effect repertoire: Marginalizing-out non-mechanism elements

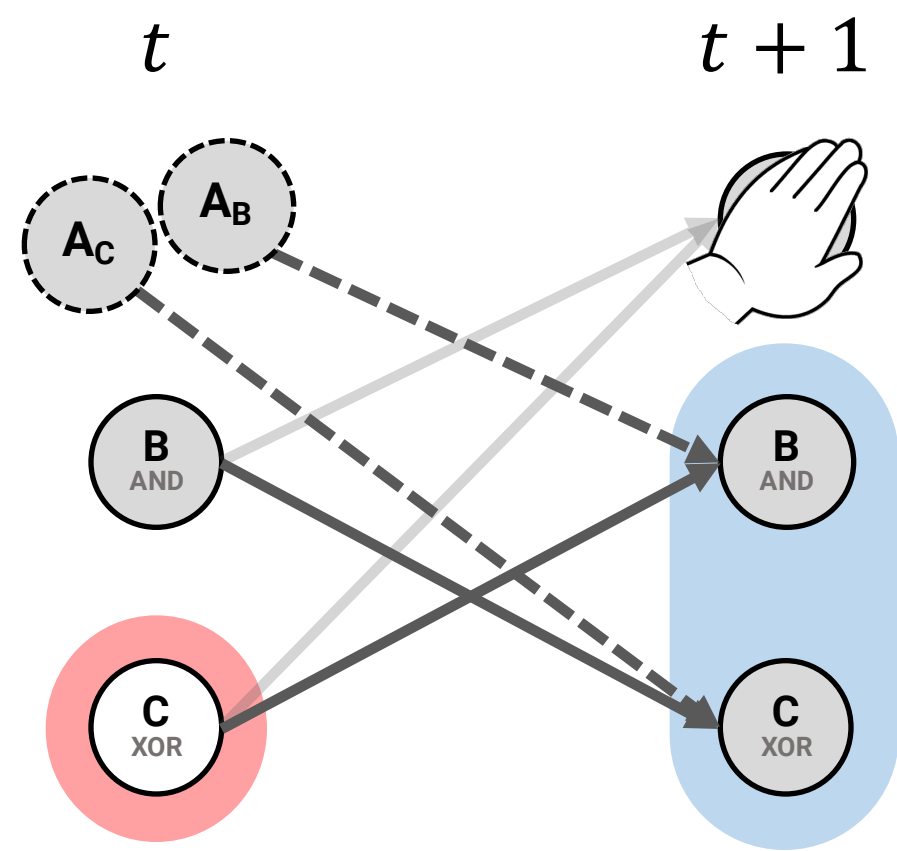

|               |                |                |   | Next state |   |   |   |
|---------------|----------------|----------------|---|------------|---|---|---|
|               |                |                |   | B          |   |   |   |
|               |                |                |   | C          |   |   |   |
| Current state | A <sub>B</sub> | A <sub>C</sub> | B | C          |   |   |   |
|               | ○              | ○              | ○ | ○          | 1 | 0 | 0 |
|               | ●              | ○              | ○ | ○          | 1 | 0 | 0 |
|               | ○              | ●              | ○ | ○          | 0 | 0 | 1 |
|               | ●              | ●              | ○ | ○          | 0 | 0 | 1 |
|               | ○              | ○              | ● | ○          | 0 | 0 | 1 |
|               | ●              | ○              | ● | ○          | 0 | 0 | 1 |
|               | ○              | ●              | ● | ○          | 1 | 0 | 0 |
|               | ●              | ●              | ● | ○          | 1 | 0 | 0 |
|               | ○              | ○              | ○ | ●          | 1 | 0 | 0 |
|               | ●              | ○              | ○ | ●          | 0 | 1 | 0 |
|               | ○              | ●              | ○ | ●          | 0 | 0 | 1 |
|               | ●              | ●              | ○ | ●          | 0 | 0 | 0 |
|               | ○              | ○              | ● | ●          | 0 | 0 | 1 |
|               | ●              | ○              | ● | ●          | 0 | 0 | 1 |
|               | ○              | ●              | ● | ●          | 1 | 0 | 0 |
|               | ●              | ●              | ● | ●          | 0 | 1 | 0 |

In other words, we want to ignore the current state of the non-mechanism elements—so we marginalize them out of the TPM



# Calculating an effect repertoire: Marginalizing-out non-mechanism elements

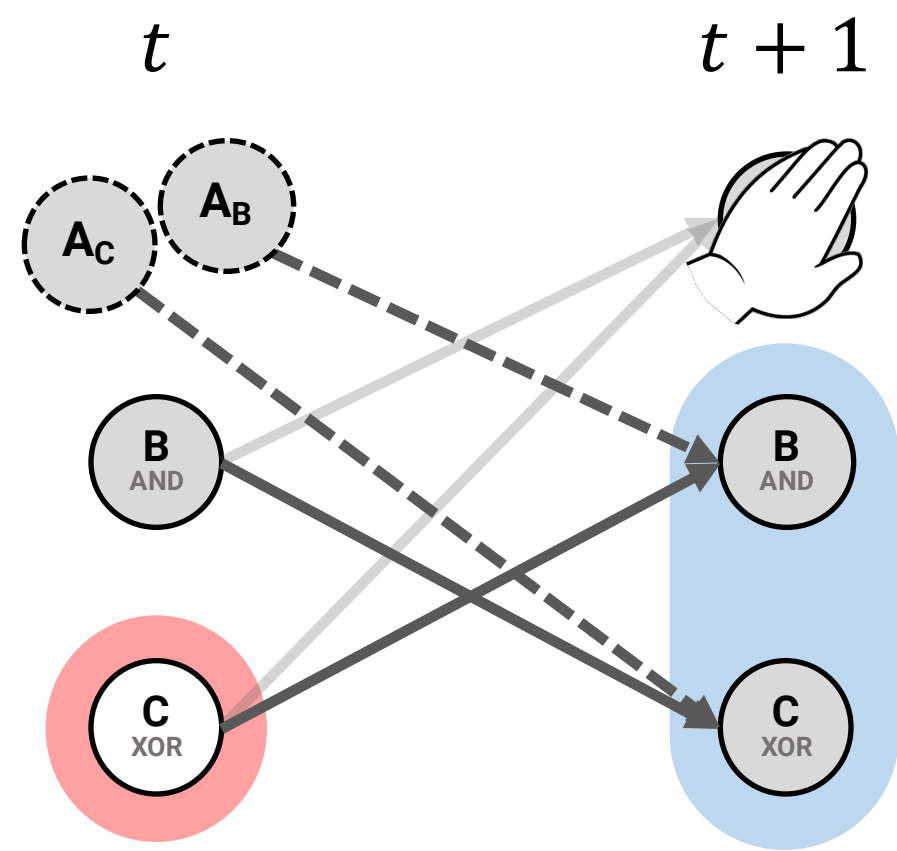

|               |       |       |   | Next state |   |   |   |
|---------------|-------|-------|---|------------|---|---|---|
|               |       |       |   | B          |   |   |   |
|               |       |       |   | C          |   |   |   |
| Current state | $A_B$ | $A_C$ | B | C          |   |   |   |
|               | ○     | ○     | ○ | ○          | 1 | 0 | 0 |
|               | ●     | ○     | ○ | ○          | 1 | 0 | 0 |
|               | ○     | ●     | ○ | ○          | 0 | 0 | 1 |
|               | ●     | ●     | ○ | ○          | 0 | 0 | 1 |
|               | ○     | ○     | ● | ○          | 0 | 0 | 1 |
|               | ●     | ○     | ● | ○          | 0 | 0 | 1 |
|               | ○     | ●     | ● | ○          | 1 | 0 | 0 |
|               | ●     | ●     | ● | ○          | 1 | 0 | 0 |
|               | ○     | ○     | ○ | ●          | 1 | 0 | 0 |
|               | ●     | ○     | ○ | ●          | 0 | 1 | 0 |
|               | ○     | ●     | ○ | ●          | 0 | 0 | 1 |
|               | ●     | ●     | ○ | ●          | 0 | 0 | 0 |
|               | ○     | ○     | ● | ●          | 0 | 0 | 1 |
|               | ●     | ○     | ● | ●          | 0 | 0 | 1 |
|               | ○     | ●     | ● | ●          | 1 | 0 | 0 |
|               | ●     | ●     | ● | ●          | 0 | 1 | 0 |

As with the previous example, marginalizing over the current states of elements means we sum over rows, rather than columns (and renormalize the resulting rows)

# Calculating an effect repertoire: Marginalizing-out non-mechanism elements

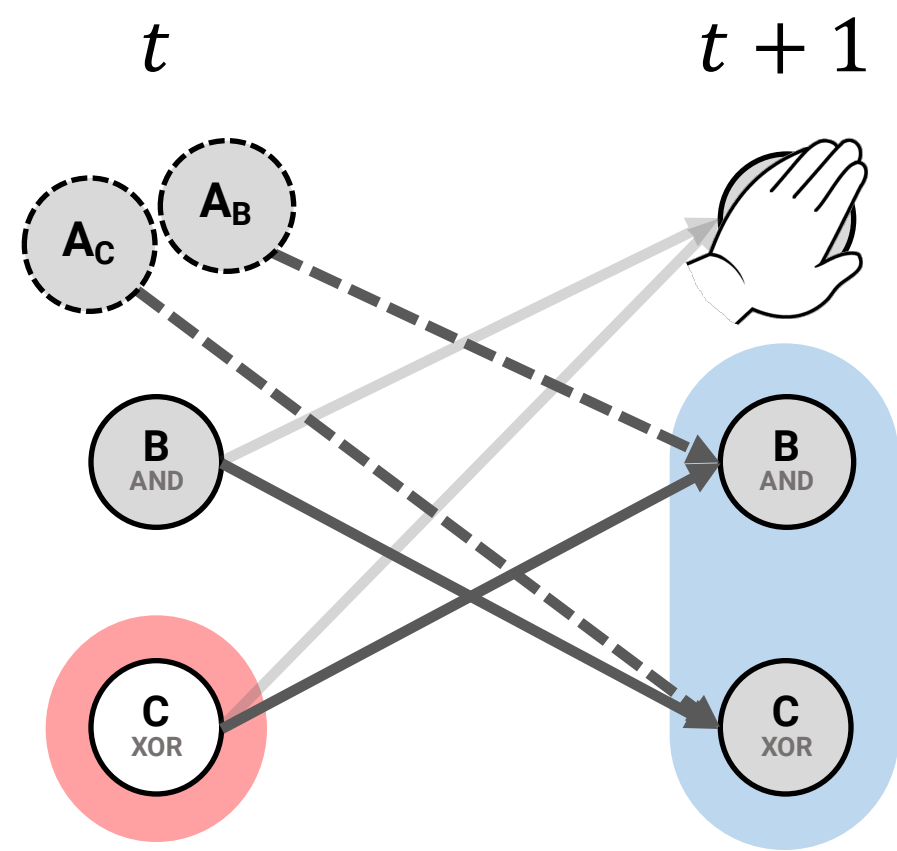

First we'll marginalize-out  $A_B$

|               |       |       |   | Next state |   |   |   |
|---------------|-------|-------|---|------------|---|---|---|
|               |       |       |   | B          |   |   |   |
|               |       |       |   | C          |   |   |   |
| Current state | $A_B$ | $A_C$ | B | C          |   |   |   |
|               | ○     | ○     | ○ | ○          | 1 | 0 | 0 |
|               | ●     | ○     | ○ | ○          | 1 | 0 | 0 |
|               | ○     | ●     | ○ | ○          | 0 | 0 | 1 |
|               | ●     | ●     | ○ | ○          | 0 | 0 | 1 |
|               | ○     | ○     | ● | ○          | 0 | 0 | 1 |
|               | ●     | ○     | ● | ○          | 0 | 0 | 1 |
|               | ○     | ●     | ● | ○          | 1 | 0 | 0 |
|               | ●     | ●     | ● | ○          | 1 | 0 | 0 |
|               | ○     | ○     | ○ | ●          | 1 | 0 | 0 |
|               | ●     | ○     | ○ | ●          | 0 | 1 | 0 |
|               | ○     | ●     | ○ | ●          | 0 | 0 | 1 |
|               | ●     | ●     | ○ | ●          | 0 | 0 | 0 |
|               | ○     | ○     | ● | ●          | 0 | 0 | 1 |
|               | ●     | ○     | ● | ●          | 0 | 0 | 1 |
|               | ○     | ●     | ● | ●          | 1 | 0 | 0 |
|               | ●     | ●     | ● | ●          | 0 | 1 | 0 |

# Calculating an effect repertoire: Marginalizing-out non-mechanism elements

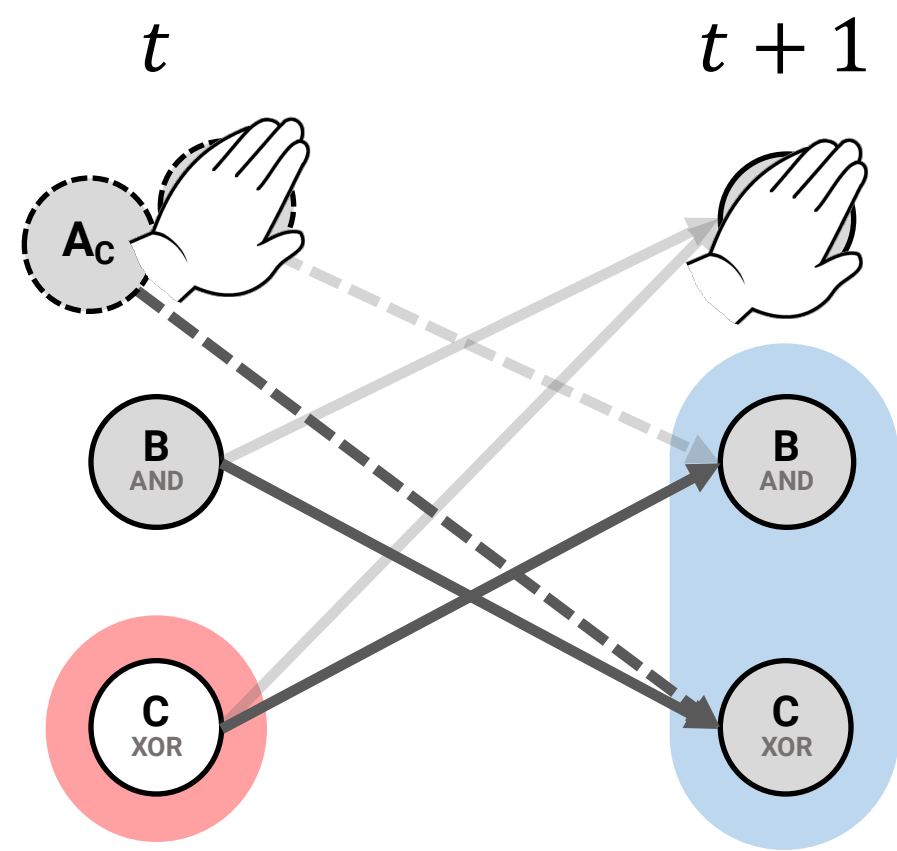

First we'll marginalize-out  $A_B$

|               |                |                |   |   | Next state |   |   |   |   |
|---------------|----------------|----------------|---|---|------------|---|---|---|---|
|               |                |                |   |   | B          | ○ | ● | ○ | ● |
|               |                |                |   |   | C          | ○ | ○ | ● | ● |
| Current state | A <sub>B</sub> | A <sub>C</sub> | B | C |            |   |   |   |   |
|               | ○              | ○              | ○ | ○ | 1          | 0 | 0 | 0 | 0 |
|               | ●              | ○              | ○ | ○ | 1          | 0 | 0 | 0 | 0 |
|               | ○              | ●              | ○ | ○ | 0          | 0 | 1 | 0 | 0 |
|               | ●              | ●              | ○ | ○ | 0          | 0 | 1 | 0 | 0 |
|               | ○              | ○              | ● | ○ | 0          | 0 | 1 | 0 | 0 |
|               | ●              | ○              | ● | ○ | 0          | 0 | 1 | 0 | 0 |
|               | ○              | ●              | ● | ○ | 1          | 0 | 0 | 0 | 0 |
|               | ●              | ●              | ● | ○ | 1          | 0 | 0 | 0 | 0 |
|               | ○              | ○              | ○ | ● | 1          | 0 | 0 | 0 | 0 |
|               | ●              | ○              | ○ | ● | 0          | 1 | 0 | 0 | 0 |
|               | ○              | ●              | ○ | ● | 0          | 0 | 1 | 0 | 0 |
|               | ●              | ●              | ○ | ● | 0          | 0 | 0 | 1 | 0 |
|               | ○              | ○              | ● | ● | 0          | 0 | 1 | 0 | 0 |
|               | ●              | ○              | ● | ● | 0          | 0 | 0 | 1 | 0 |
|               | ○              | ●              | ● | ● | 1          | 0 | 0 | 0 | 0 |
|               | ●              | ●              | ● | ● | 0          | 1 | 0 | 0 | 0 |

# Calculating an effect repertoire: Marginalizing-out non-mechanism elements

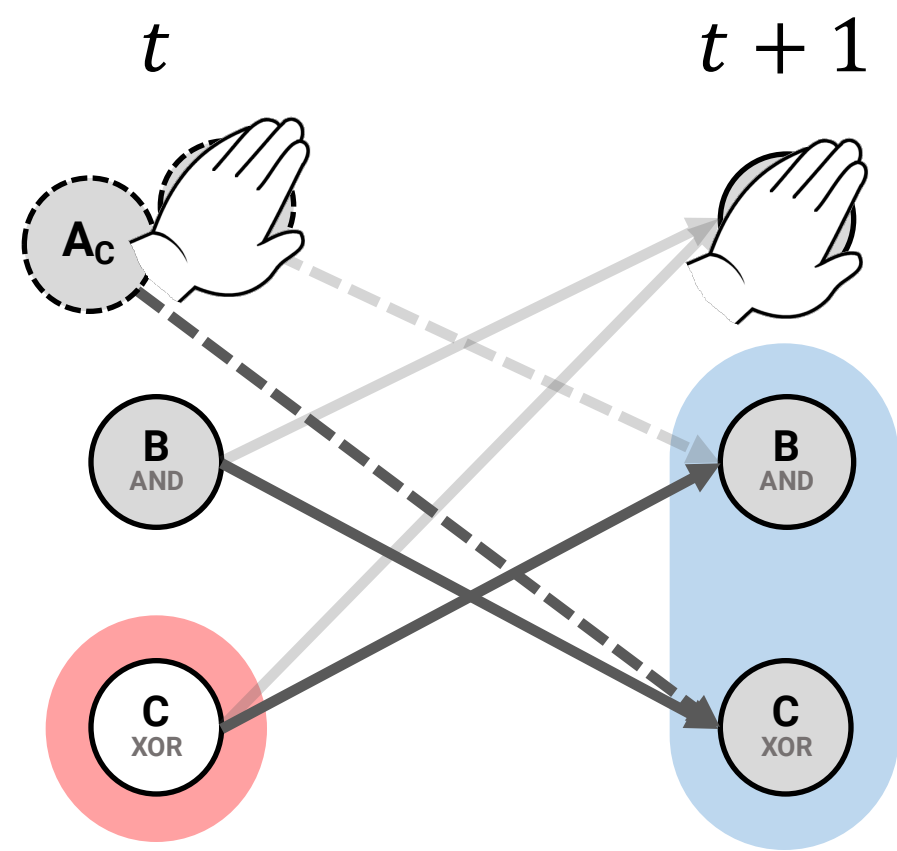

First we'll marginalize-out  $A_B$

|               |                |                |   |   | Next state |   |   |   |   |
|---------------|----------------|----------------|---|---|------------|---|---|---|---|
|               |                |                |   |   | B          | ○ | ● | ○ | ● |
|               |                |                |   |   | C          | ○ | ○ | ● | ● |
| Current state | A <sub>B</sub> | A <sub>C</sub> | B | C |            |   |   |   |   |
|               | ○              | ○              | ○ | ○ | 1          | 0 | 0 | 0 | 0 |
|               | ●              | ○              | ○ | ○ | 1          | 0 | 0 | 0 | 0 |
|               | ○              | ●              | ○ | ○ | 0          | 0 | 1 | 0 | 0 |
|               | ●              | ●              | ○ | ○ | 0          | 0 | 1 | 0 | 0 |
|               | ○              | ○              | ● | ○ | 0          | 0 | 1 | 0 | 0 |
|               | ●              | ○              | ● | ○ | 0          | 0 | 1 | 0 | 0 |
|               | ○              | ●              | ● | ○ | 1          | 0 | 0 | 0 | 0 |
|               | ●              | ●              | ● | ○ | 1          | 0 | 0 | 0 | 0 |
|               | ○              | ○              | ○ | ● | 1          | 0 | 0 | 0 | 0 |
|               | ●              | ○              | ○ | ● | 0          | 1 | 0 | 0 | 0 |
|               | ○              | ●              | ○ | ● | 0          | 0 | 1 | 0 | 0 |
|               | ●              | ●              | ○ | ● | 0          | 0 | 0 | 1 | 0 |
|               | ○              | ○              | ● | ● | 0          | 0 | 1 | 0 | 0 |
|               | ●              | ○              | ● | ● | 0          | 0 | 0 | 1 | 0 |
|               | ○              | ●              | ● | ● | 1          | 0 | 0 | 0 | 0 |
|               | ●              | ●              | ● | ● | 0          | 1 | 0 | 0 | 0 |

# Calculating an effect repertoire: Marginalizing-out non-mechanism elements

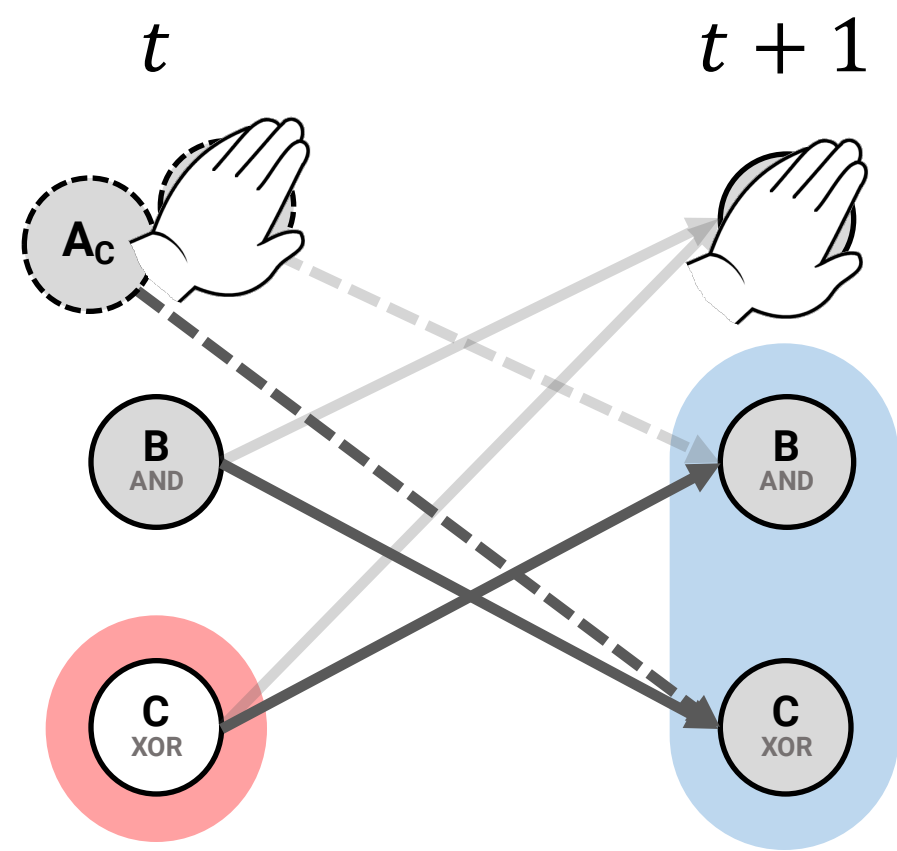

First we'll marginalize-out **A<sub>B</sub>**

|               |                |   | Next state |   |   |   |   |
|---------------|----------------|---|------------|---|---|---|---|
|               |                |   | B<br>C     |   |   |   |   |
| Current state | A <sub>c</sub> | B | C          |   |   |   |   |
|               |                |   |            | 1 | 0 | 0 | 0 |
|               |                |   |            | 1 | 0 | 0 | 0 |
|               |                |   |            | 0 | 0 | 1 | 0 |
|               |                |   |            | 0 | 0 | 1 | 0 |
|               |                |   |            | 0 | 0 | 1 | 0 |
|               |                |   |            | 0 | 0 | 1 | 0 |
|               |                |   |            | 1 | 0 | 0 | 0 |
|               |                |   |            | 1 | 0 | 0 | 0 |
|               |                |   |            | 1 | 0 | 0 | 0 |
|               |                |   |            | 0 | 1 | 0 | 0 |
|               |                |   |            | 0 | 0 | 1 | 0 |
|               |                |   |            | 0 | 0 | 0 | 1 |
|               |                |   |            | 0 | 0 | 1 | 0 |
|               |                |   |            | 0 | 0 | 0 | 1 |
|               |                |   |            | 1 | 0 | 0 | 0 |
|               |                |   |            | 0 | 1 | 0 | 0 |

# Calculating an effect repertoire: Marginalizing-out non-mechanism elements

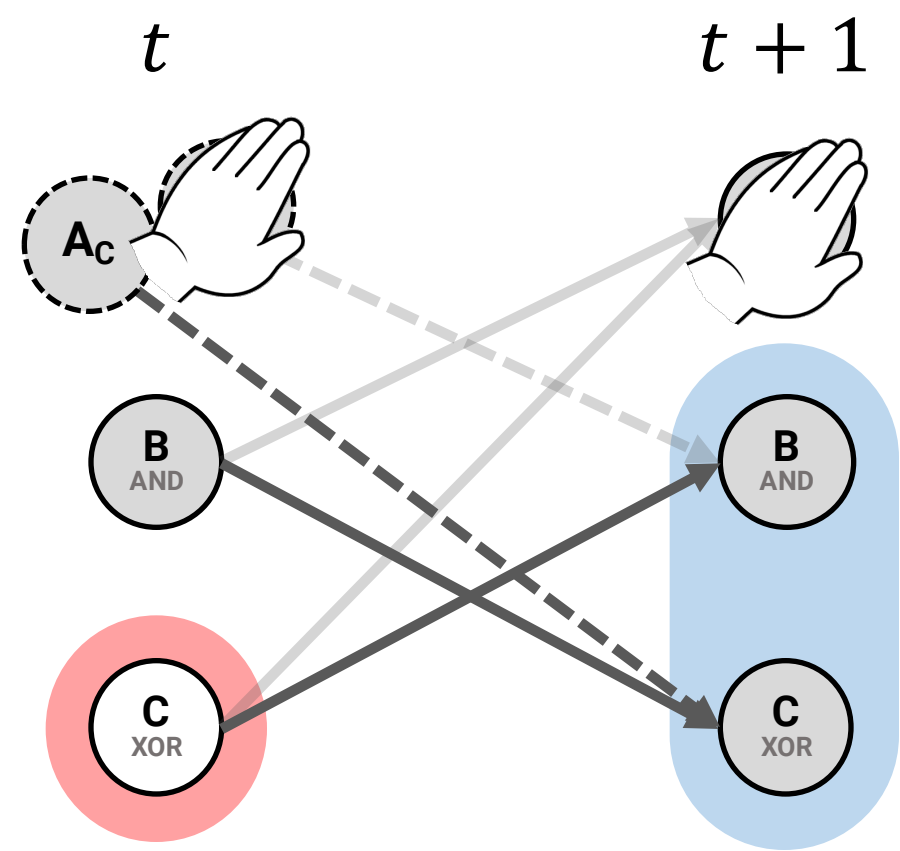

First we'll marginalize-out  $A_B$

|               |       |   | Next state |   |   |   |
|---------------|-------|---|------------|---|---|---|
|               |       |   | B          |   |   |   |
|               |       |   | C          |   |   |   |
| Current state | $A_c$ | B | C          |   |   |   |
|               |       |   |            | 2 | 0 | 0 |
|               |       |   |            | 0 | 0 | 2 |
|               |       |   |            | 0 | 0 | 2 |
|               |       |   |            | 2 | 0 | 0 |
|               |       |   |            | 1 | 1 | 0 |
|               |       |   |            | 0 | 0 | 1 |
|               |       |   |            | 0 | 0 | 1 |
|               |       |   |            | 1 | 1 | 0 |

# Calculating an effect repertoire: Marginalizing-out non-mechanism elements

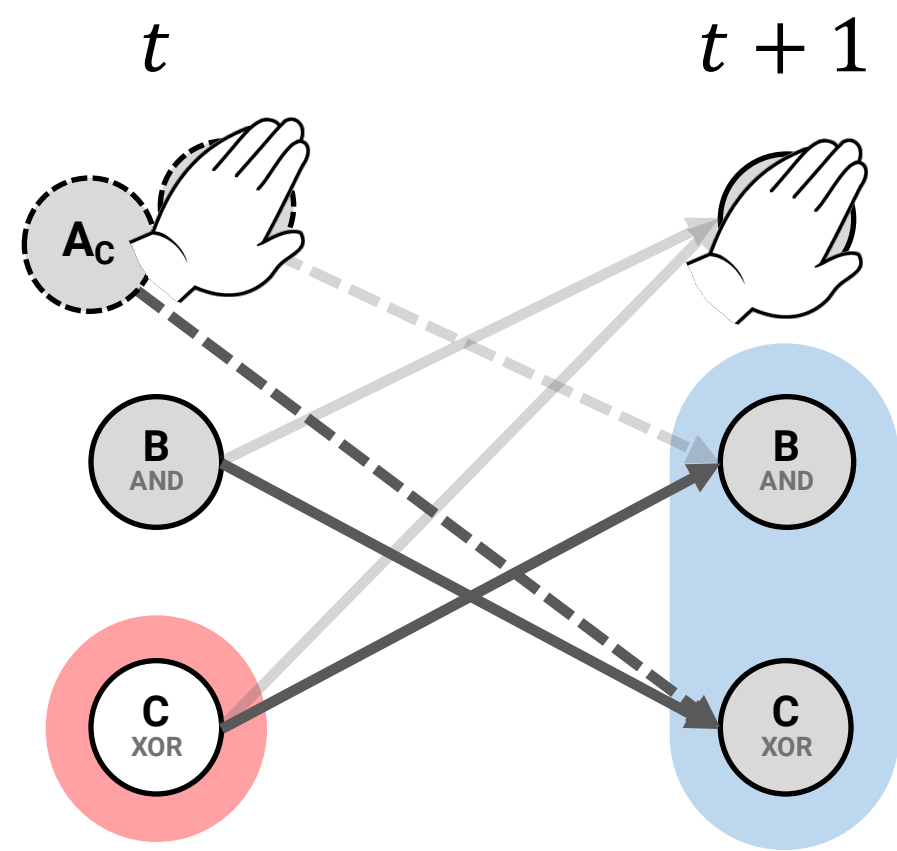

First we'll marginalize-out  $A_B$

|               |                        |                        | Next state             |                        |                        |                        |
|---------------|------------------------|------------------------|------------------------|------------------------|------------------------|------------------------|
|               |                        |                        | B                      |                        |                        |                        |
|               |                        |                        | C                      |                        |                        |                        |
| Current state | $A_c$                  | B                      | C                      | <div><div></div></div> | <div><div></div></div> | <div><div></div></div> |
|               | <div><div></div></div> | <div><div></div></div> | <div><div></div></div> | 1                      | 0                      | 0                      |
|               | <div><div></div></div> | <div><div></div></div> | <div><div></div></div> | 0                      | 0                      | 1                      |
|               | <div><div></div></div> | <div><div></div></div> | <div><div></div></div> | 0                      | 0                      | 1                      |
|               | <div><div></div></div> | <div><div></div></div> | <div><div></div></div> | 1                      | 0                      | 0                      |
|               | <div><div></div></div> | <div><div></div></div> | <div><div></div></div> | 1/2                    | 1/2                    | 0                      |
|               | <div><div></div></div> | <div><div></div></div> | <div><div></div></div> | 0                      | 0                      | 1/2                    |
|               | <div><div></div></div> | <div><div></div></div> | <div><div></div></div> | 0                      | 0                      | 1/2                    |
|               | <div><div></div></div> | <div><div></div></div> | <div><div></div></div> | 1/2                    | 1/2                    | 0                      |

# Calculating an effect repertoire: Marginalizing-out non-mechanism elements

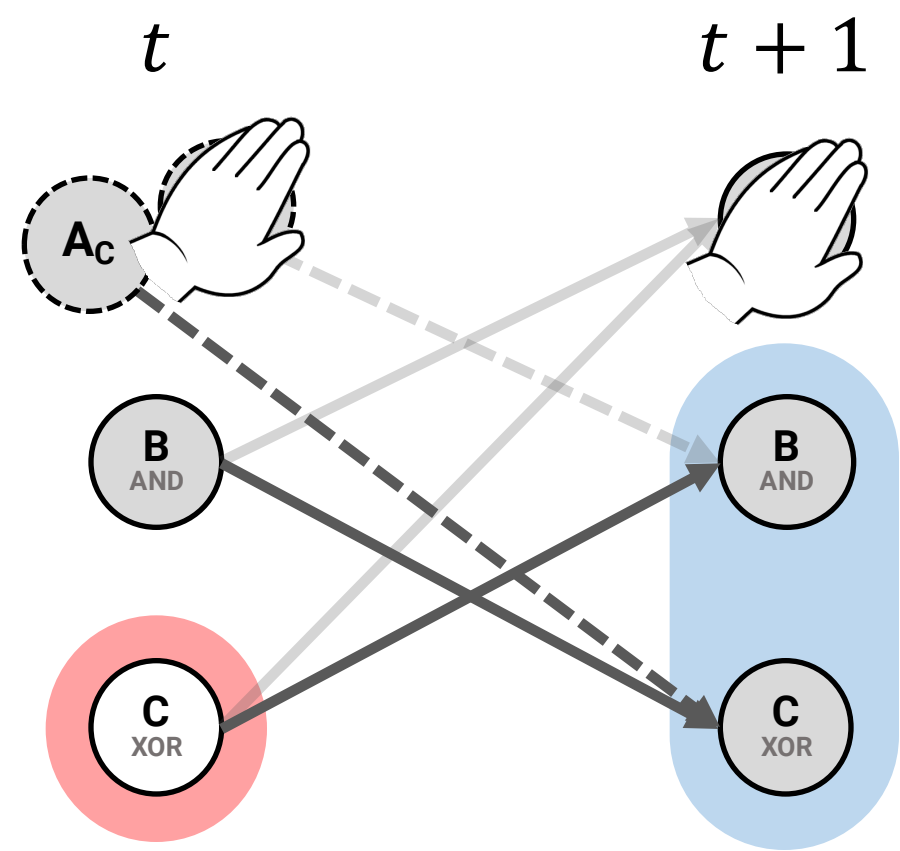

Now we'll marginalize-out  $A_c$

|               |       |   | Next state |     |     |     |
|---------------|-------|---|------------|-----|-----|-----|
|               |       |   | B          |     |     |     |
|               |       |   | C          |     |     |     |
| Current state | $A_c$ | B | C          |     |     |     |
|               |       |   |            |     |     |     |
|               |       |   |            |     |     |     |
|               |       |   |            |     |     |     |
|               |       |   |            |     |     |     |
|               |       |   |            |     |     |     |
|               |       |   |            |     |     |     |
|               |       |   |            |     |     |     |
|               |       |   |            |     |     |     |
|               |       |   |            | 1   | 0   | 0   |
|               |       |   |            | 0   | 0   | 1   |
|               |       |   |            | 0   | 0   | 1   |
|               |       |   |            | 1   | 0   | 0   |
|               |       |   |            | 1/2 | 1/2 | 0   |
|               |       |   |            | 0   | 0   | 1/2 |
|               |       |   |            | 0   | 0   | 1/2 |
|               |       |   |            | 1/2 | 1/2 | 0   |



# Calculating an effect repertoire: Marginalizing-out non-mechanism elements

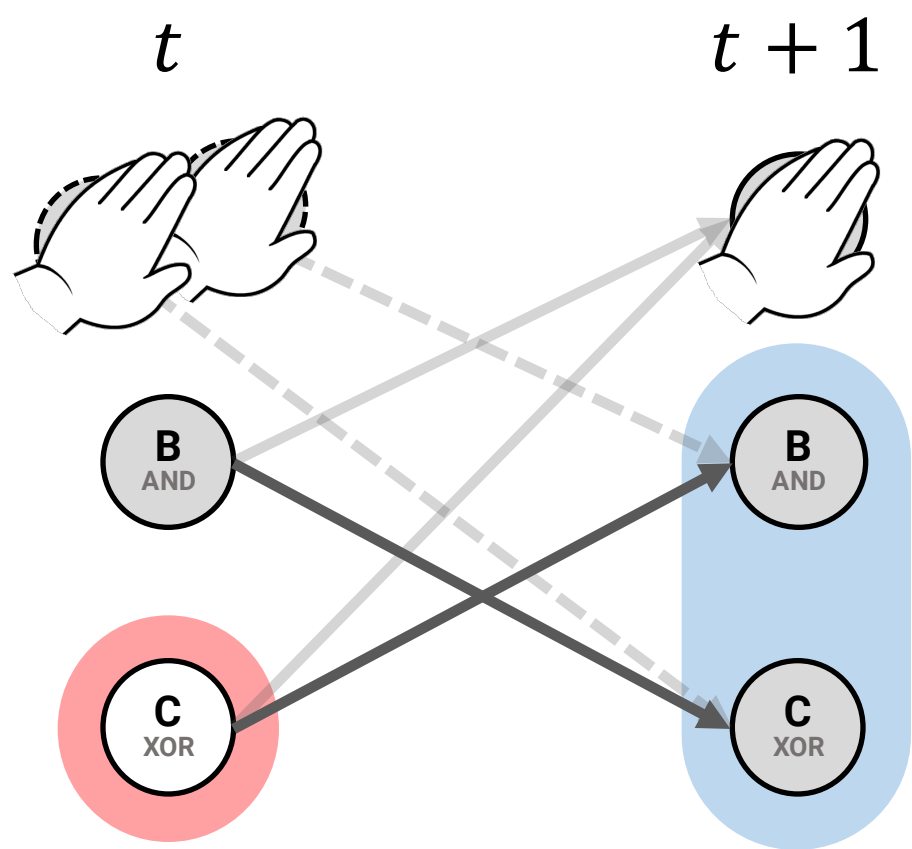

Now we'll marginalize-out  $A_c$

|               |                        |                        | Next state             |                        |                        |                        |
|---------------|------------------------|------------------------|------------------------|------------------------|------------------------|------------------------|
|               |                        |                        | B                      |                        |                        |                        |
|               |                        |                        | C                      |                        |                        |                        |
| Current state | $A_c$                  | B                      | C                      | <div><div></div></div> | <div><div></div></div> | <div><div></div></div> |
|               | <div><div></div></div> | <div><div></div></div> | <div><div></div></div> | 1                      | 0                      | 0                      |
|               | <div><div></div></div> | <div><div></div></div> | <div><div></div></div> | 0                      | 0                      | 1                      |
|               | <div><div></div></div> | <div><div></div></div> | <div><div></div></div> | 0                      | 0                      | 1                      |
|               | <div><div></div></div> | <div><div></div></div> | <div><div></div></div> | 1                      | 0                      | 0                      |
|               | <div><div></div></div> | <div><div></div></div> | <div><div></div></div> | $\frac{1}{2}$          | $\frac{1}{2}$          | 0                      |
|               | <div><div></div></div> | <div><div></div></div> | <div><div></div></div> | 0                      | 0                      | $\frac{1}{2}$          |
|               | <div><div></div></div> | <div><div></div></div> | <div><div></div></div> | 0                      | 0                      | $\frac{1}{2}$          |
|               | <div><div></div></div> | <div><div></div></div> | <div><div></div></div> | $\frac{1}{2}$          | $\frac{1}{2}$          | 0                      |

# Calculating an effect repertoire: Marginalizing-out non-mechanism elements

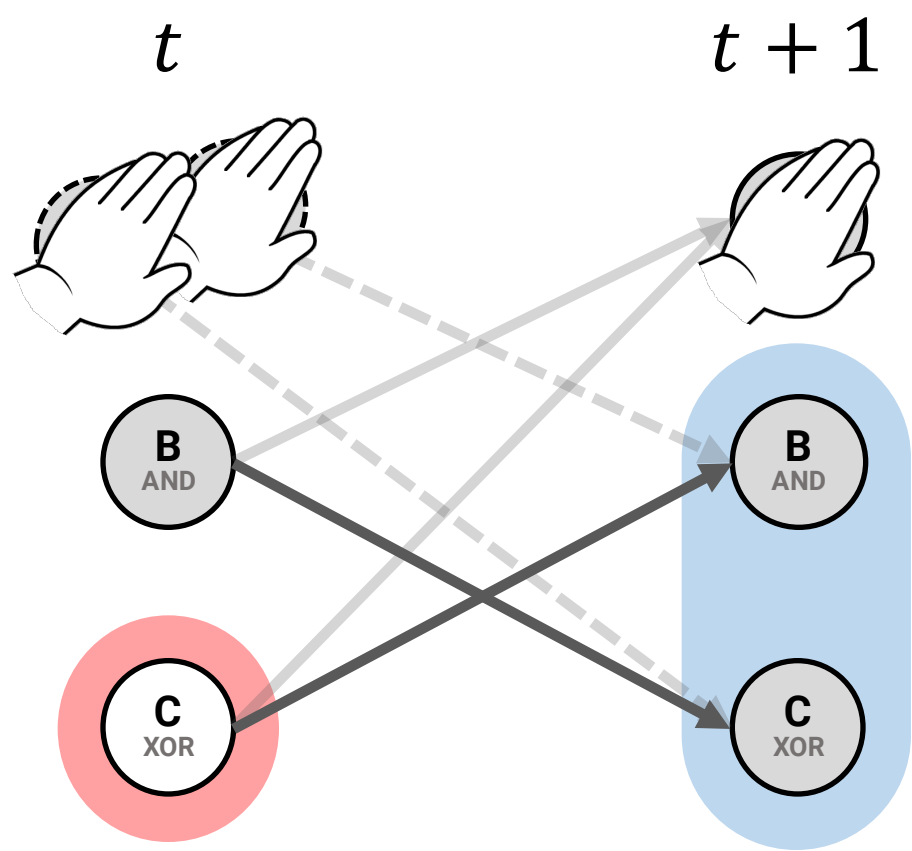

Now we'll marginalize-out  $A_c$

|               |                |   | Next state |     |     |     |     |
|---------------|----------------|---|------------|-----|-----|-----|-----|
|               |                |   | B          |     |     |     |     |
|               |                |   | C          |     |     |     |     |
| Current state | A <sub>c</sub> | B | C          |     |     |     |     |
|               |                |   |            | 1   | 0   | 0   | 0   |
|               |                |   |            | 0   | 0   | 1   | 0   |
|               |                |   |            | 0   | 0   | 1   | 0   |
|               |                |   |            | 1   | 0   | 0   | 0   |
|               |                |   |            | 1/2 | 1/2 | 0   | 0   |
|               |                |   |            | 0   | 0   | 1/2 | 1/2 |
|               |                |   |            | 0   | 0   | 1/2 | 1/2 |
|               |                |   |            | 1/2 | 1/2 | 0   | 0   |

# Calculating an effect repertoire: Marginalizing-out non-mechanism elements

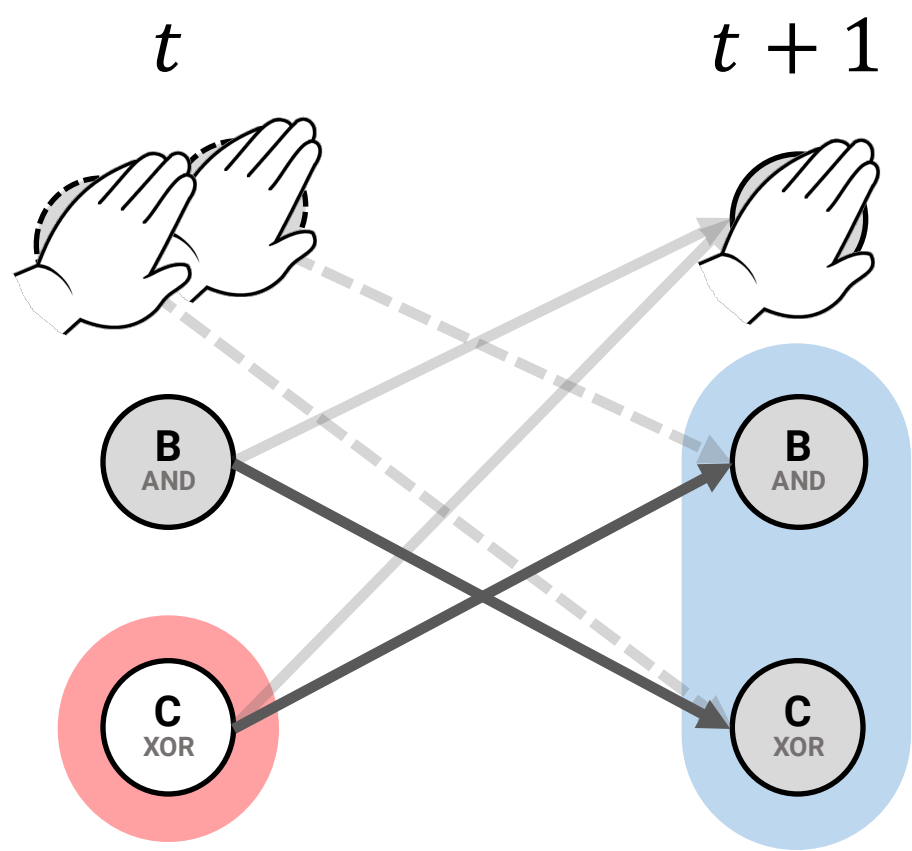

Now we'll marginalize-out  $A_c$

|               |                                   | Next state                        |                                   |                                   |                                   |                                   |
|---------------|-----------------------------------|-----------------------------------|-----------------------------------|-----------------------------------|-----------------------------------|-----------------------------------|
|               |                                   | B                                 | C                                 | B                                 | C                                 |                                   |
| Current state | B                                 | C                                 | <div><div></div><div></div></div> | <div><div></div><div></div></div> | <div><div></div><div></div></div> | <div><div></div><div></div></div> |
|               | <div><div></div><div></div></div> | <div><div></div><div></div></div> | 1                                 | 0                                 | 1                                 | 0                                 |
|               | <div><div></div><div></div></div> | <div><div></div><div></div></div> | 1                                 | 0                                 | 1                                 | 0                                 |
|               | <div><div></div><div></div></div> | <div><div></div><div></div></div> | $\frac{1}{2}$                     | $\frac{1}{2}$                     | $\frac{1}{2}$                     | $\frac{1}{2}$                     |
|               | <div><div></div><div></div></div> | <div><div></div><div></div></div> | $\frac{1}{2}$                     | $\frac{1}{2}$                     | $\frac{1}{2}$                     | $\frac{1}{2}$                     |

## Calculating an effect repertoire: Marginalizing-out non-mechanism elements

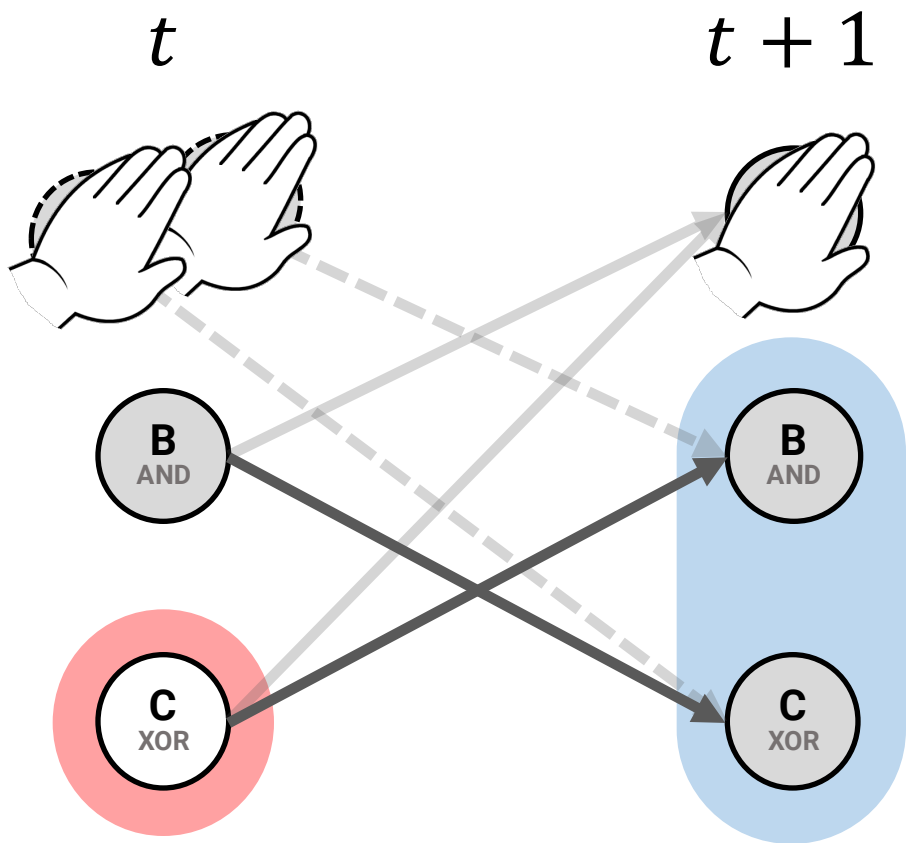

Now we'll marginalize-out  $\mathbf{A}_c$

|               |   |   | Next state    |               |               |               |
|---------------|---|---|---------------|---------------|---------------|---------------|
|               |   |   | B             | C             | ⊙             | ⊙             |
| Current state | B | C | ⊙             | ⊙             | ⊙             | ⊙             |
|               | ⊙ | ⊙ | $\frac{1}{2}$ | 0             | $\frac{1}{2}$ | 0             |
|               | ⊙ | ⊙ | $\frac{1}{2}$ | 0             | $\frac{1}{2}$ | 0             |
|               | ⊙ | ⊙ | $\frac{1}{4}$ | $\frac{1}{4}$ | $\frac{1}{4}$ | $\frac{1}{4}$ |
|               | ⊙ | ⊙ | $\frac{1}{4}$ | $\frac{1}{4}$ | $\frac{1}{4}$ | $\frac{1}{4}$ |

# Calculating an effect repertoire: Marginalizing-out non-mechanism elements

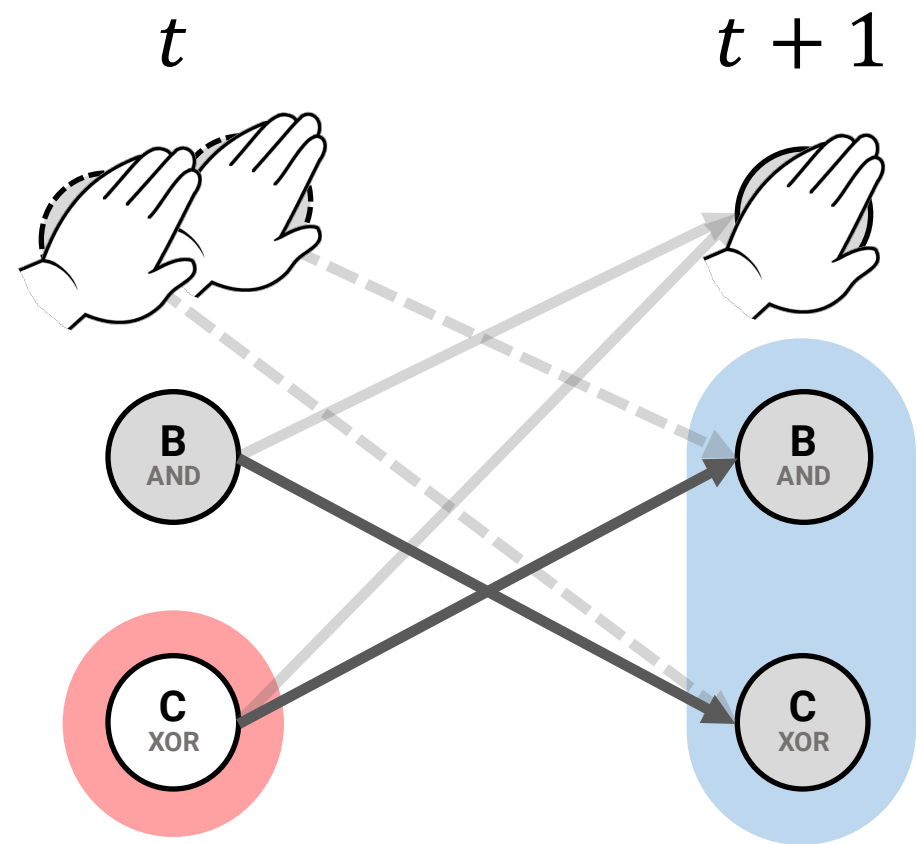

And finally we'll marginalize-out **B**

|               |                                   | Next state                        |                                   |                                   |                                   |
|---------------|-----------------------------------|-----------------------------------|-----------------------------------|-----------------------------------|-----------------------------------|
| Current state | B                                 | C                                 | <div><div></div><div></div></div> | <div><div></div><div></div></div> | <div><div></div><div></div></div> |
|               | <div><div></div><div></div></div> | <div><div></div><div></div></div> | <div><div></div><div></div></div> | <div><div></div><div></div></div> | <div><div></div><div></div></div> |
|               | <div><div></div><div></div></div> | <div><div></div><div></div></div> | $\frac{1}{2}$                     | 0                                 | $\frac{1}{2}$                     |
|               | <div><div></div><div></div></div> | <div><div></div><div></div></div> | $\frac{1}{2}$                     | 0                                 | $\frac{1}{2}$                     |
|               | <div><div></div><div></div></div> | <div><div></div><div></div></div> | $\frac{1}{4}$                     | $\frac{1}{4}$                     | $\frac{1}{4}$                     |
|               | <div><div></div><div></div></div> | <div><div></div><div></div></div> | $\frac{1}{4}$                     | $\frac{1}{4}$                     | $\frac{1}{4}$                     |

# Calculating an effect repertoire: Marginalizing-out non-mechanism elements

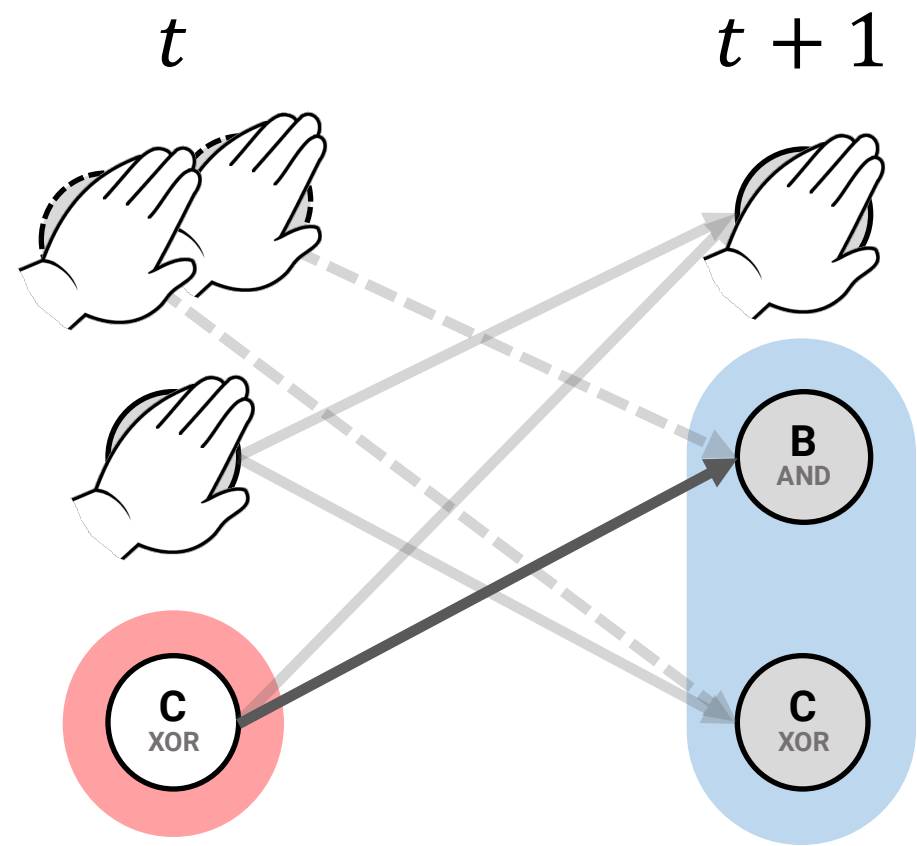

And finally we'll marginalize-out **B**

|               |                                   | Next state                        |                                   |                                   |                                   |                                   |
|---------------|-----------------------------------|-----------------------------------|-----------------------------------|-----------------------------------|-----------------------------------|-----------------------------------|
|               |                                   | B                                 | C                                 |                                   |                                   |                                   |
| Current state | B                                 | C                                 | <div><div></div><div></div></div> | <div><div></div><div></div></div> | <div><div></div><div></div></div> | <div><div></div><div></div></div> |
|               | <div><div></div><div></div></div> | <div><div></div><div></div></div> | $\frac{1}{2}$                     | 0                                 | $\frac{1}{2}$                     | 0                                 |
|               | <div><div></div><div></div></div> | <div><div></div><div></div></div> | $\frac{1}{2}$                     | 0                                 | $\frac{1}{2}$                     | 0                                 |
|               | <div><div></div><div></div></div> | <div><div></div><div></div></div> | $\frac{1}{4}$                     | $\frac{1}{4}$                     | $\frac{1}{4}$                     | $\frac{1}{4}$                     |
|               | <div><div></div><div></div></div> | <div><div></div><div></div></div> | $\frac{1}{4}$                     | $\frac{1}{4}$                     | $\frac{1}{4}$                     | $\frac{1}{4}$                     |

Calculating an effect repertoire:  
**Marginalizing-out non-mechanism elements**

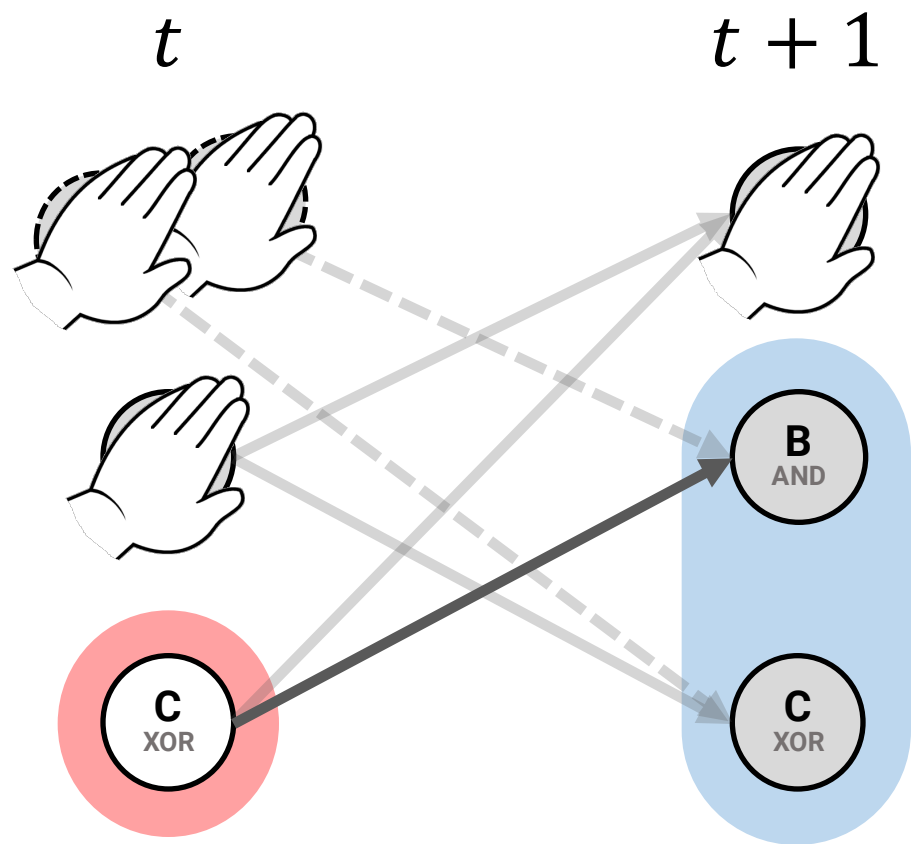

And finally we'll marginalize-out **B**

|               |                                   | Next state                        |                                   |                                   |                                   |                                   |
|---------------|-----------------------------------|-----------------------------------|-----------------------------------|-----------------------------------|-----------------------------------|-----------------------------------|
|               |                                   | B                                 | C                                 |                                   |                                   |                                   |
| Current state | B                                 | C                                 | <div><div></div><div></div></div> | <div><div></div><div></div></div> | <div><div></div><div></div></div> | <div><div></div><div></div></div> |
|               | <div><div></div><div></div></div> | <div><div></div><div></div></div> | $\frac{1}{2}$                     | 0                                 | $\frac{1}{2}$                     | 0                                 |
|               | <div><div></div><div></div></div> | <div><div></div><div></div></div> | $\frac{1}{2}$                     | 0                                 | $\frac{1}{2}$                     | 0                                 |
|               | <div><div></div><div></div></div> | <div><div></div><div></div></div> | $\frac{1}{4}$                     | $\frac{1}{4}$                     | $\frac{1}{4}$                     | $\frac{1}{4}$                     |
|               | <div><div></div><div></div></div> | <div><div></div><div></div></div> | $\frac{1}{4}$                     | $\frac{1}{4}$                     | $\frac{1}{4}$                     | $\frac{1}{4}$                     |

Calculating an effect repertoire:  
**Marginalizing-out non-mechanism elements**

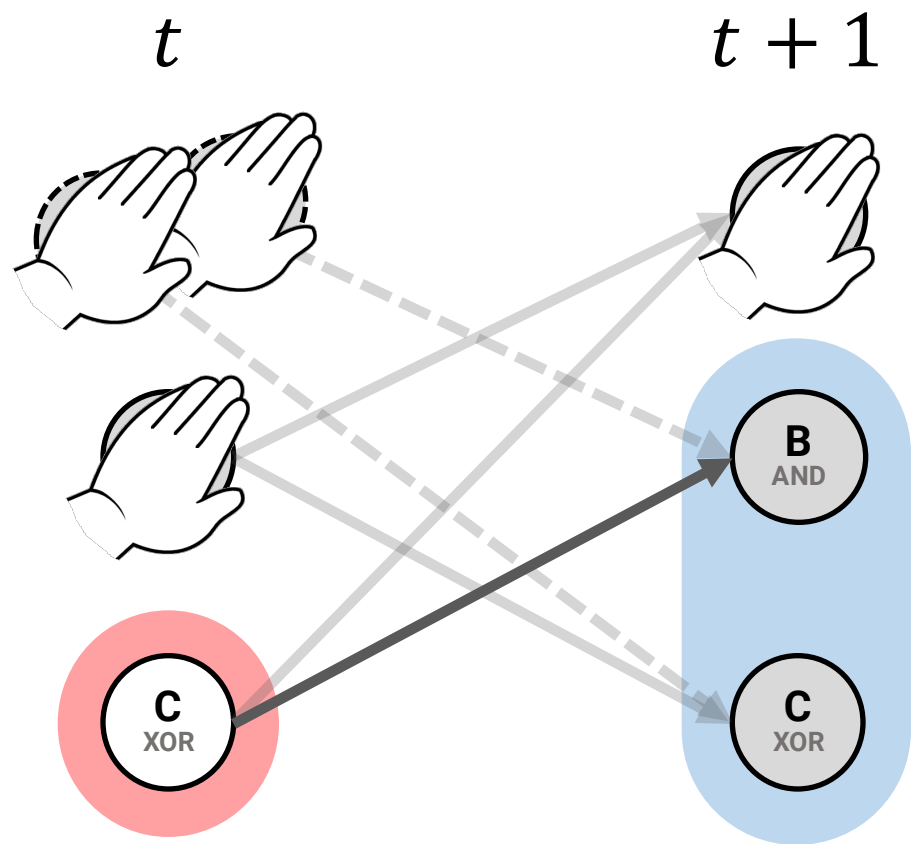

And finally we'll marginalize-out **B**

|               |                                   | Next state                        |                                   |                                   |                                   |
|---------------|-----------------------------------|-----------------------------------|-----------------------------------|-----------------------------------|-----------------------------------|
|               |                                   | B                                 |                                   |                                   |                                   |
|               |                                   | C                                 |                                   |                                   |                                   |
| Current state | C                                 | <div><div></div><div></div></div> | <div><div></div><div></div></div> | <div><div></div><div></div></div> | <div><div></div><div></div></div> |
|               | <div><div></div><div></div></div> | $\frac{1}{2}$                     | 0                                 | $\frac{1}{2}$                     | 0                                 |
|               | <div><div></div><div></div></div> | $\frac{1}{2}$                     | 0                                 | $\frac{1}{2}$                     | 0                                 |
|               | <div><div></div><div></div></div> | $\frac{1}{4}$                     | $\frac{1}{4}$                     | $\frac{1}{4}$                     | $\frac{1}{4}$                     |
|               | <div><div></div><div></div></div> | $\frac{1}{4}$                     | $\frac{1}{4}$                     | $\frac{1}{4}$                     | $\frac{1}{4}$                     |



Calculating an effect repertoire:  
**Marginalizing-out non-mechanism elements**

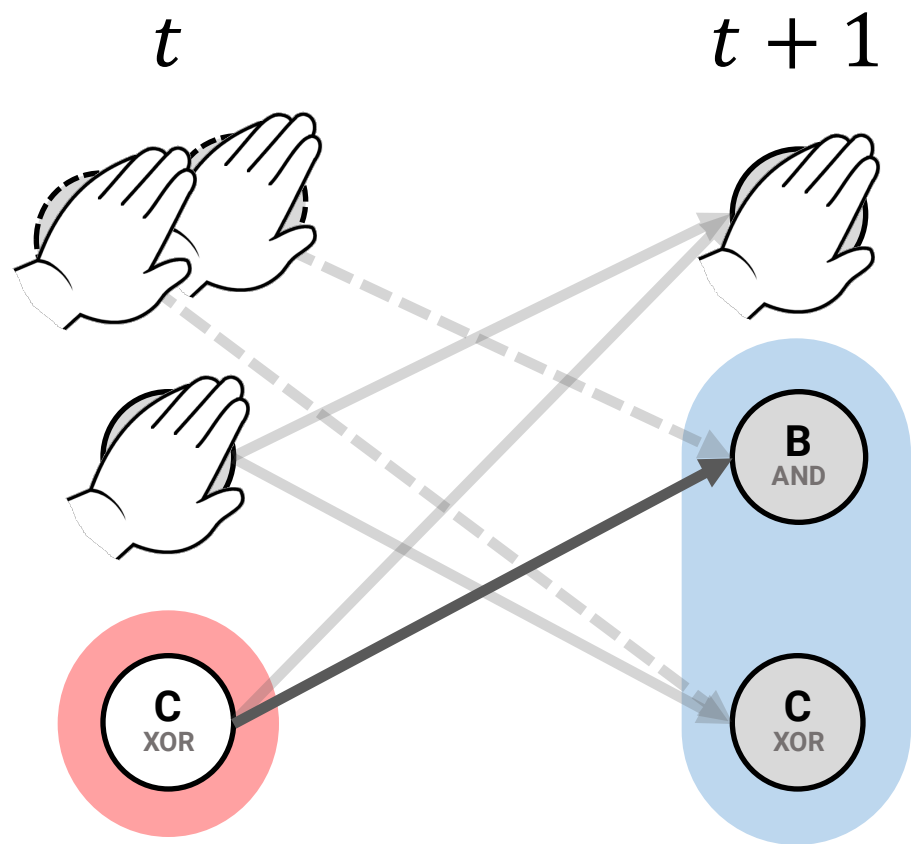

And finally we'll marginalize-out **B**

|               |                                   | Next state                        |                                   |                                   |                                   |
|---------------|-----------------------------------|-----------------------------------|-----------------------------------|-----------------------------------|-----------------------------------|
|               |                                   | B                                 |                                   |                                   |                                   |
|               |                                   | C                                 |                                   |                                   |                                   |
| Current state | C                                 | <div><div></div><div></div></div> | <div><div></div><div></div></div> | <div><div></div><div></div></div> | <div><div></div><div></div></div> |
|               |                                   | <div><div></div><div></div></div> | <div><div></div><div></div></div> | <div><div></div><div></div></div> | <div><div></div><div></div></div> |
|               | <div><div></div><div></div></div> | 1                                 | 0                                 | 1                                 | 0                                 |
|               | <div><div></div><div></div></div> | $\frac{1}{2}$                     | $\frac{1}{2}$                     | $\frac{1}{2}$                     | $\frac{1}{2}$                     |

Calculating an effect repertoire:  
**Marginalizing-out non-mechanism elements**

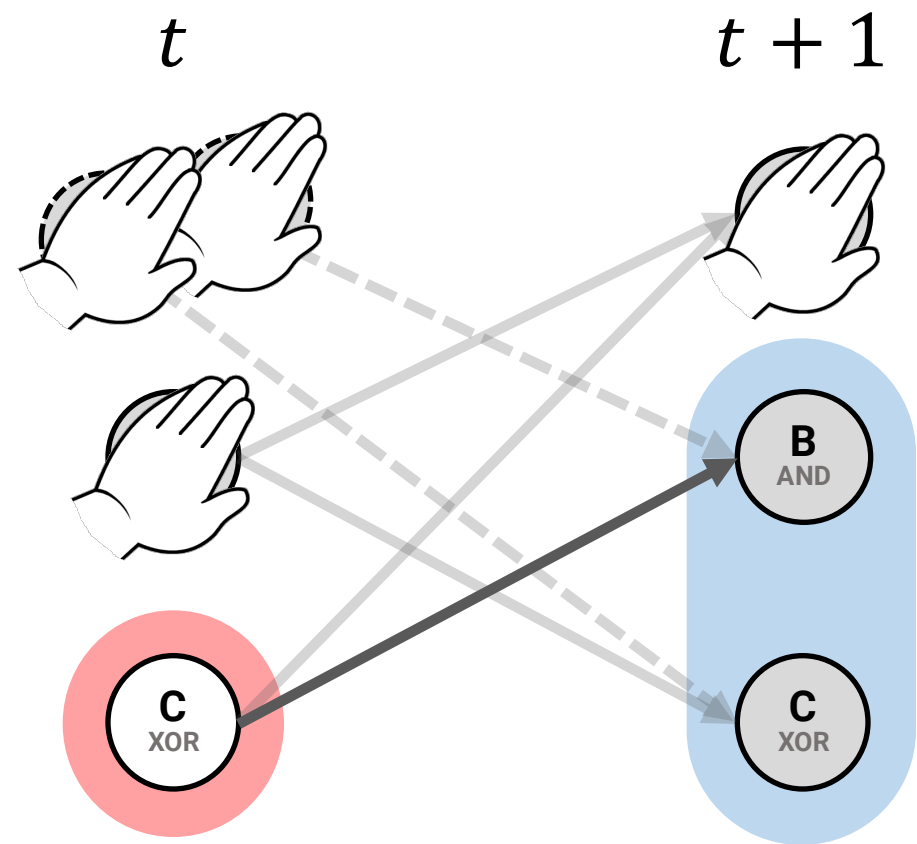

And finally we'll marginalize-out **B**

|               |                        | Next state                        |                                   |                                   |                                   |
|---------------|------------------------|-----------------------------------|-----------------------------------|-----------------------------------|-----------------------------------|
|               |                        | B                                 |                                   |                                   |                                   |
|               |                        | C                                 |                                   |                                   |                                   |
| Current state | C                      | <div><div></div><div></div></div> | <div><div></div><div></div></div> | <div><div></div><div></div></div> | <div><div></div><div></div></div> |
|               |                        | <div><div></div><div></div></div> | <div><div></div><div></div></div> | <div><div></div><div></div></div> | <div><div></div><div></div></div> |
|               | <div><div></div></div> | $\frac{1}{2}$                     | 0                                 | $\frac{1}{2}$                     | 0                                 |
|               | <div><div></div></div> | $\frac{1}{4}$                     | $\frac{1}{4}$                     | $\frac{1}{4}$                     | $\frac{1}{4}$                     |

## Calculating an effect repertoire: Marginalizing-out non-mechanism elements

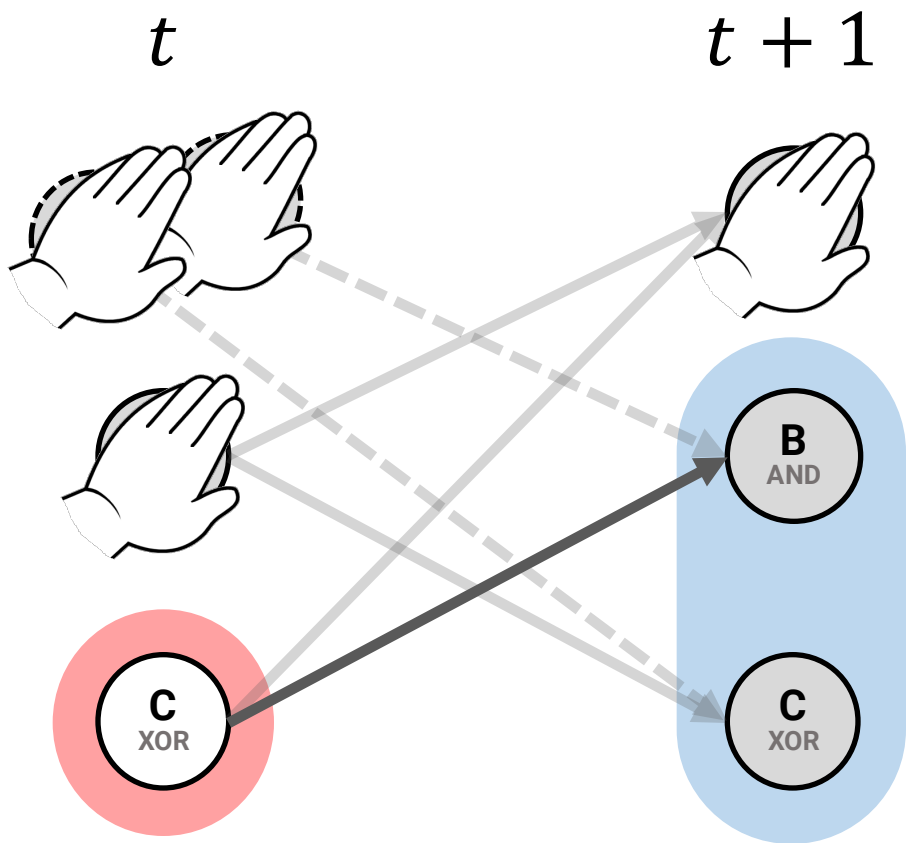

And finally we'll marginalize-out **B**

|               |   | Next state                |                           |                           |                           |
|---------------|---|---------------------------|---------------------------|---------------------------|---------------------------|
|               |   | B                         | C                         |                           |                           |
| Current state | C | <div>○</div> <div>○</div> | <div>●</div> <div>○</div> | <div>○</div> <div>●</div> | <div>●</div> <div>●</div> |
|               | ○ | $\frac{1}{2}$             | 0                         | $\frac{1}{2}$             | 0                         |
|               | ● | $\frac{1}{4}$             | $\frac{1}{4}$             | $\frac{1}{4}$             | $\frac{1}{4}$             |

## Calculating an effect repertoire: Marginalizing-out non-mechanism elements

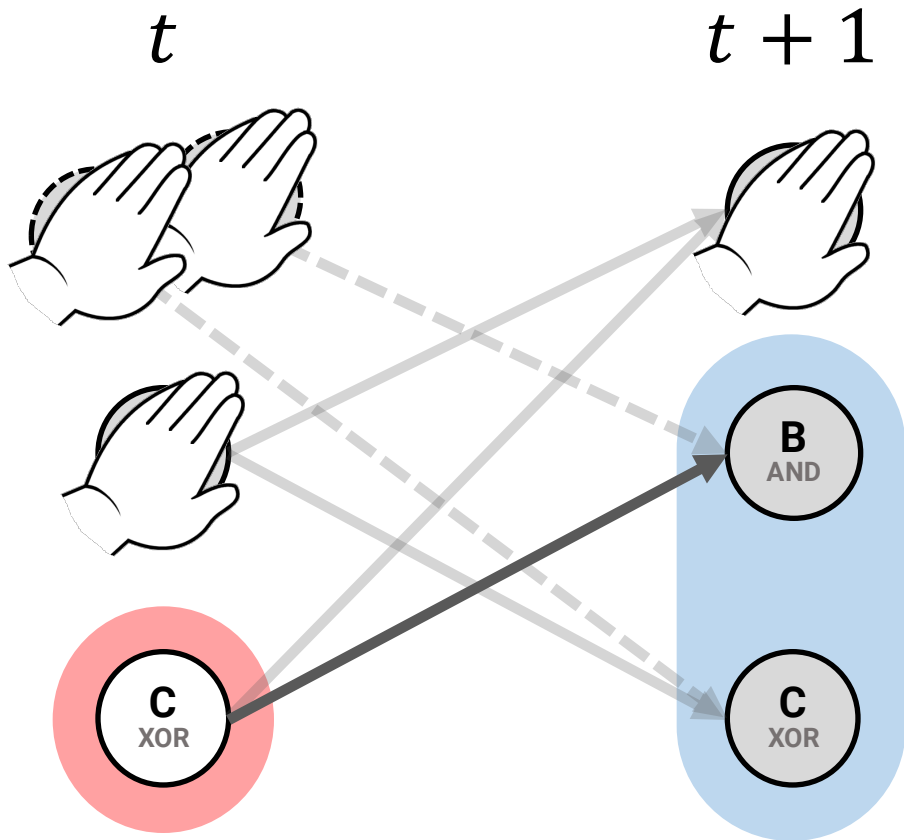

|               |   | Next state    |               |               |               |
|---------------|---|---------------|---------------|---------------|---------------|
| Current state | B |               |               |               |               |
|               | C |               |               |               |               |
|               | C |               |               |               |               |
|               |   | $\frac{1}{2}$ | 0             | $\frac{1}{2}$ | 0             |
|               |   | $\frac{1}{4}$ | $\frac{1}{4}$ | $\frac{1}{4}$ | $\frac{1}{4}$ |

Now we have a table of probabilities of next purview states given each possible current state of **C**

Calculating an effect repertoire:  
**Marginalizing-out non-mechanism elements**

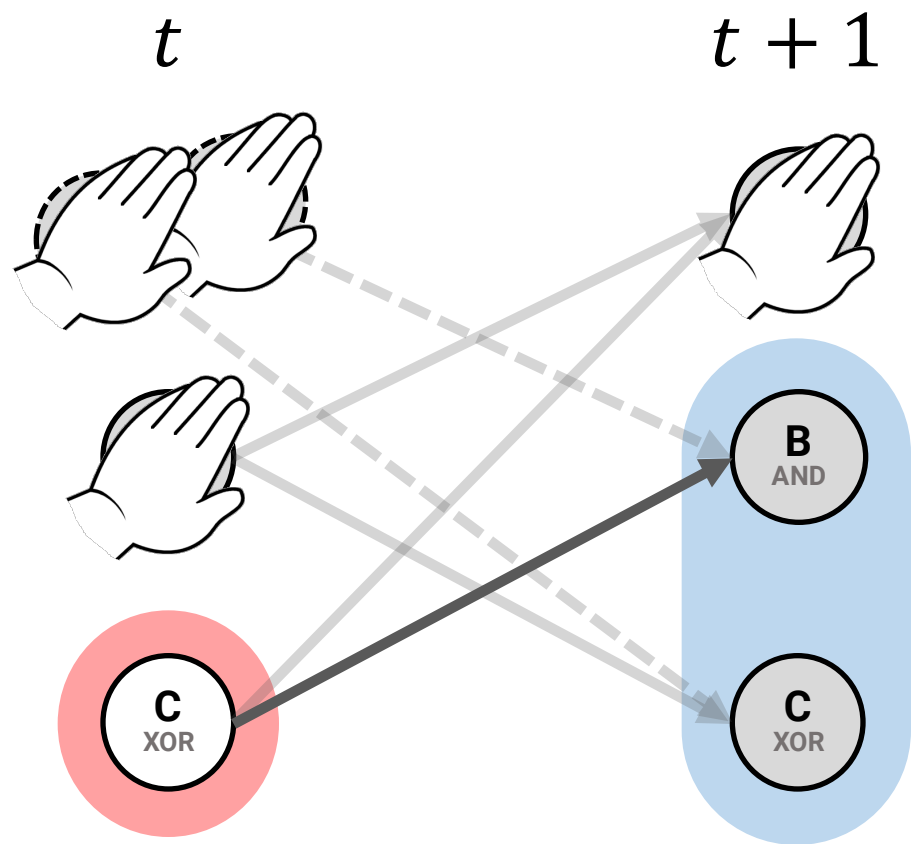

|               |                        | Next state                        |                                   |                                   |                                   |
|---------------|------------------------|-----------------------------------|-----------------------------------|-----------------------------------|-----------------------------------|
|               |                        | B                                 |                                   |                                   |                                   |
|               |                        | C                                 |                                   |                                   |                                   |
| Current state | C                      | <div><div></div><div></div></div> | <div><div></div><div></div></div> | <div><div></div><div></div></div> | <div><div></div><div></div></div> |
|               | <div><div></div></div> | $\frac{1}{2}$                     | 0                                 | $\frac{1}{2}$                     | 0                                 |
|               | <div><div></div></div> | $\frac{1}{4}$                     | $\frac{1}{4}$                     | $\frac{1}{4}$                     | $\frac{1}{4}$                     |

With this TPM, we can now simply look up the effect repertoire, by conditioning on **C**'s current state (taking the row that corresponds to it)

# Calculating an effect repertoire: Marginalizing-out non-mechanism elements

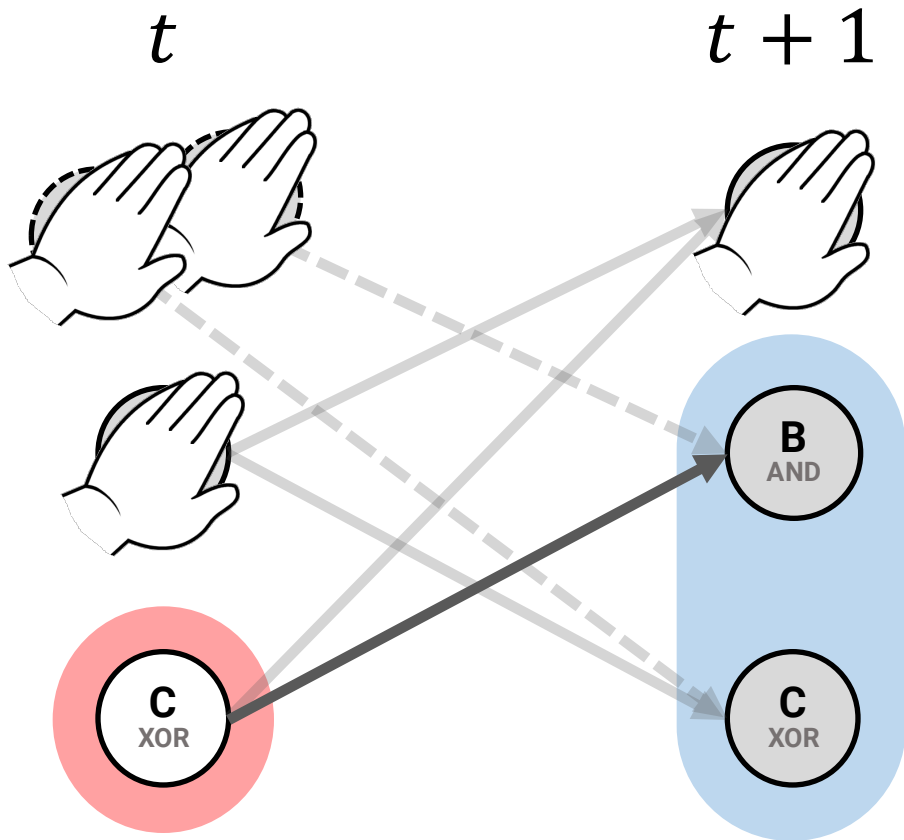

|               |   | Next state    |               |               |               |
|---------------|---|---------------|---------------|---------------|---------------|
|               |   | B             |               |               |               |
|               |   | C             |               |               |               |
| Current state | C |               |               |               |               |
|               |   |               |               |               |               |
|               |   | $\frac{1}{2}$ | 0             | $\frac{1}{2}$ | 0             |
|               |   | $\frac{1}{4}$ | $\frac{1}{4}$ | $\frac{1}{4}$ | $\frac{1}{4}$ |

With this TPM, we can now simply look up the effect repertoire, by conditioning on **C**'s current state (taking the row that corresponds to it)



# Calculating an effect repertoire: Marginalizing-out non-mechanism elements

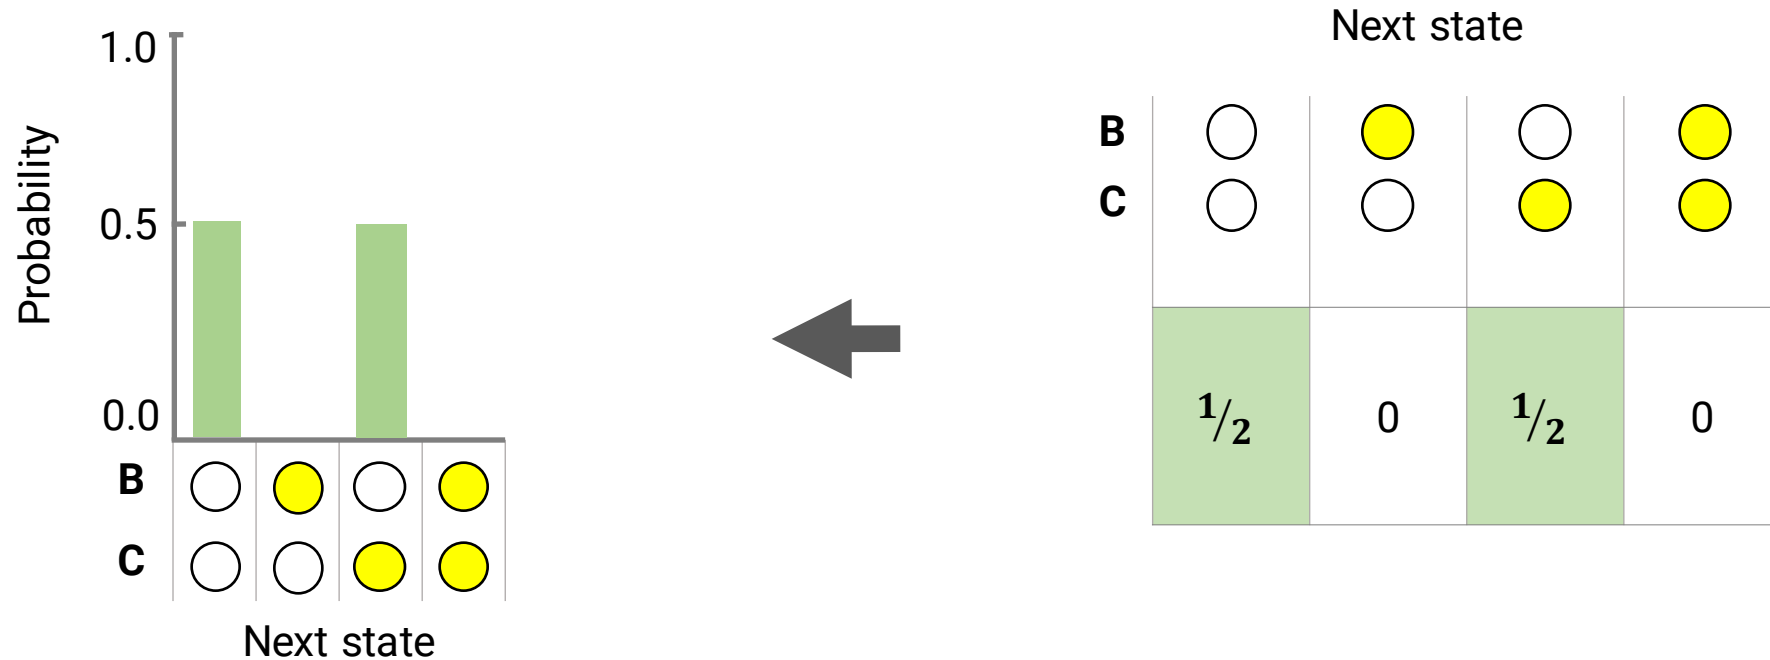

And this is the effect repertoire of mechanism **C** over purview **BC** when the system is in state (1, 0, 0)



Calculating an effect repertoire:

## Recap

We've shown how to determine the effect repertoire by:

### SYSTEM

- Introducing **virtual elements** to remove effects due to common input
- **Ignoring** the elements outside the purview
- **Ignoring** the elements outside the mechanism
- **Fixing** the current state of the mechanism

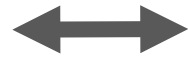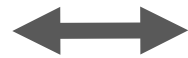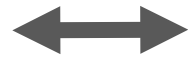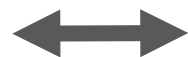

### TPM

- Finding the **virtual TPM** via perturbation
- **Marginalizing-out** the elements outside the purview
- **Marginalizing-out** the elements outside the mechanism
- **Conditioning** the TPM on the state of the mechanism

## Calculating an effect repertoire: Expanding to the full state-space

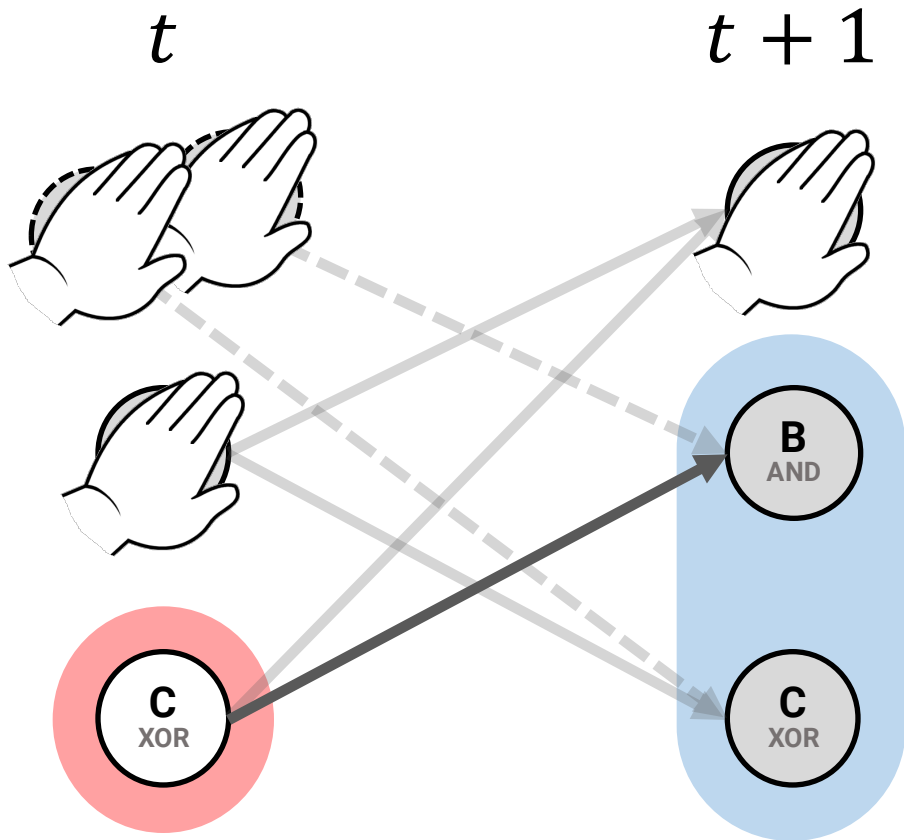

|               |   | Next state                                                                          |                                                                                     |                                                                                     |                                                                                     |
|---------------|---|-------------------------------------------------------------------------------------|-------------------------------------------------------------------------------------|-------------------------------------------------------------------------------------|-------------------------------------------------------------------------------------|
| B             | C | 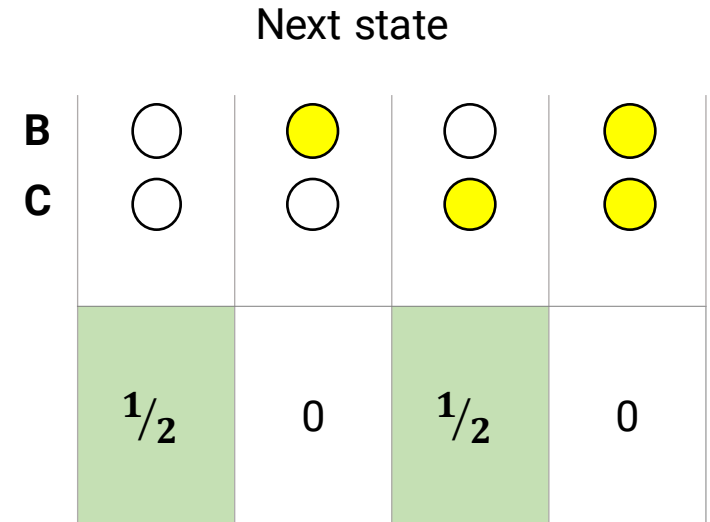 | 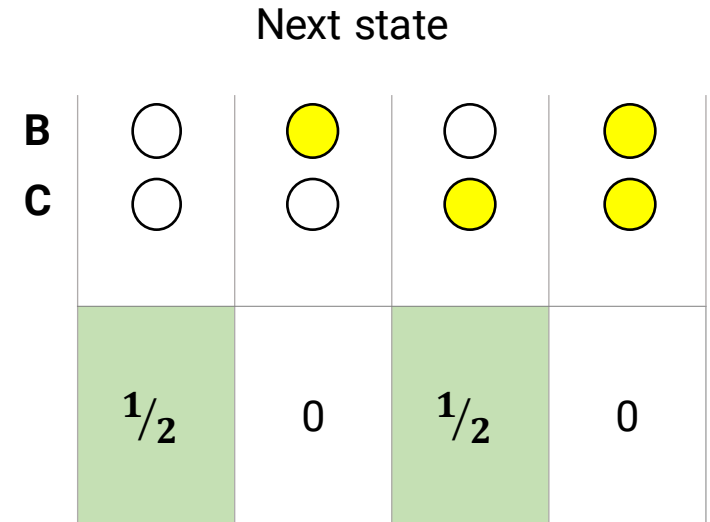 | 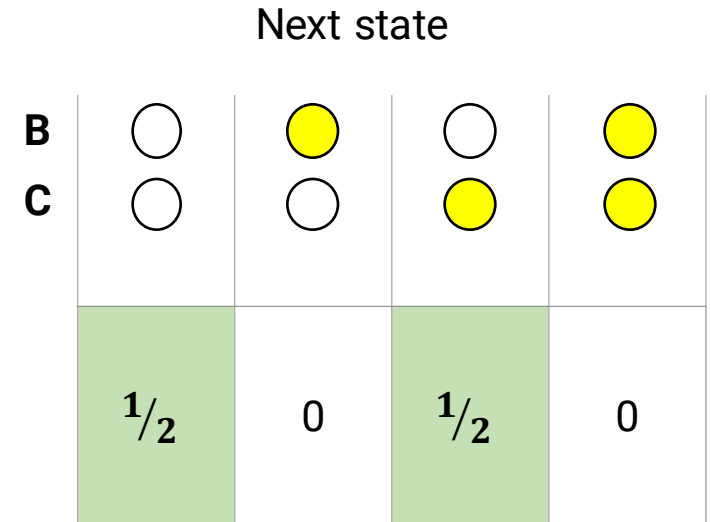 | 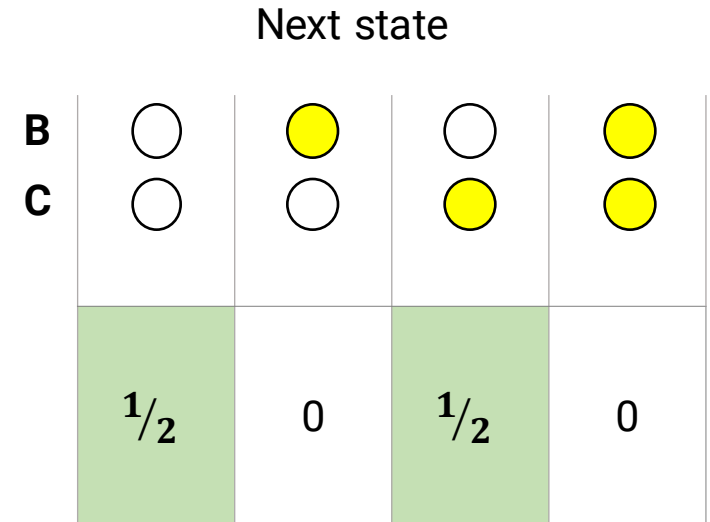 |
|               |   | 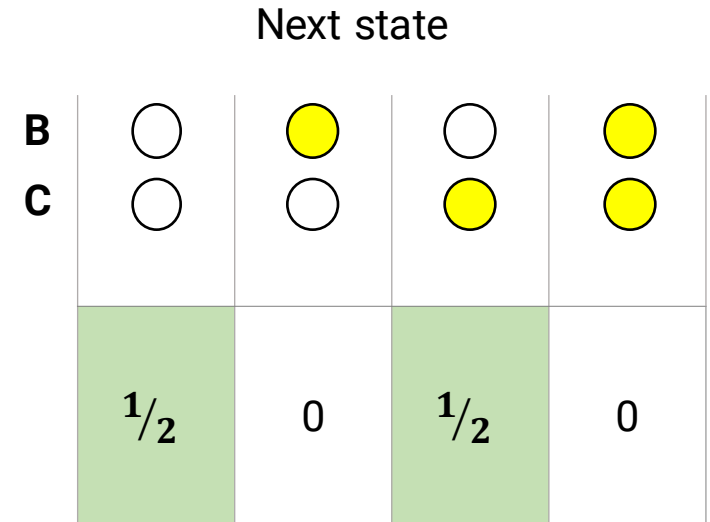 | 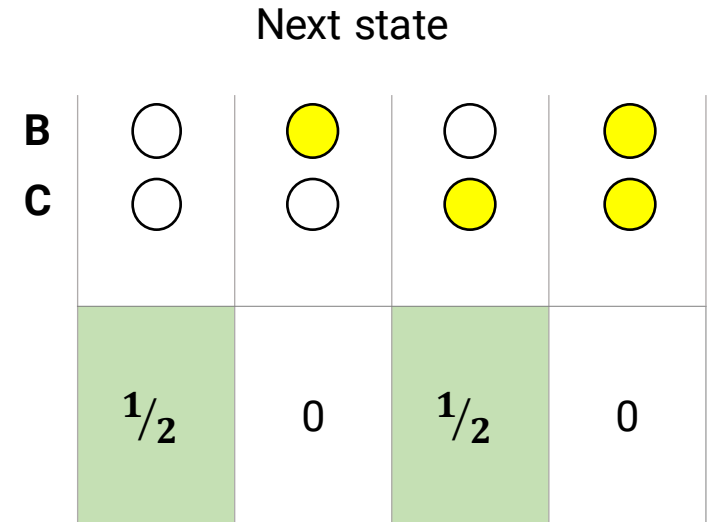 | 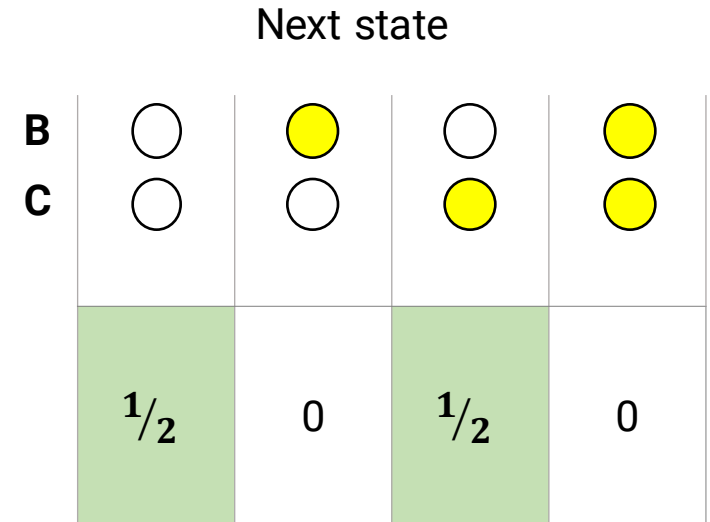 | 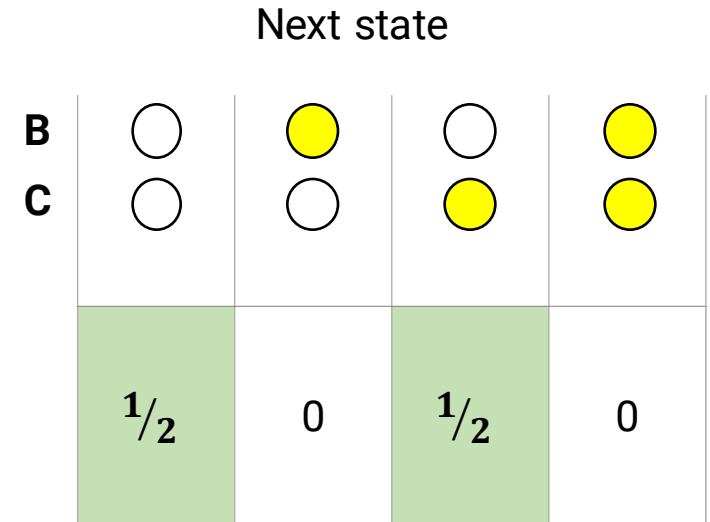 |
| $\frac{1}{2}$ |   | 0                                                                                   | $\frac{1}{2}$                                                                       | 0                                                                                   |                                                                                     |

Note that we can expand this repertoire into a distribution over states of the entire system by multiplying it by the **unconstrained distribution** over non-purview elements

## Calculating an effect repertoire: Expanding to the full state-space

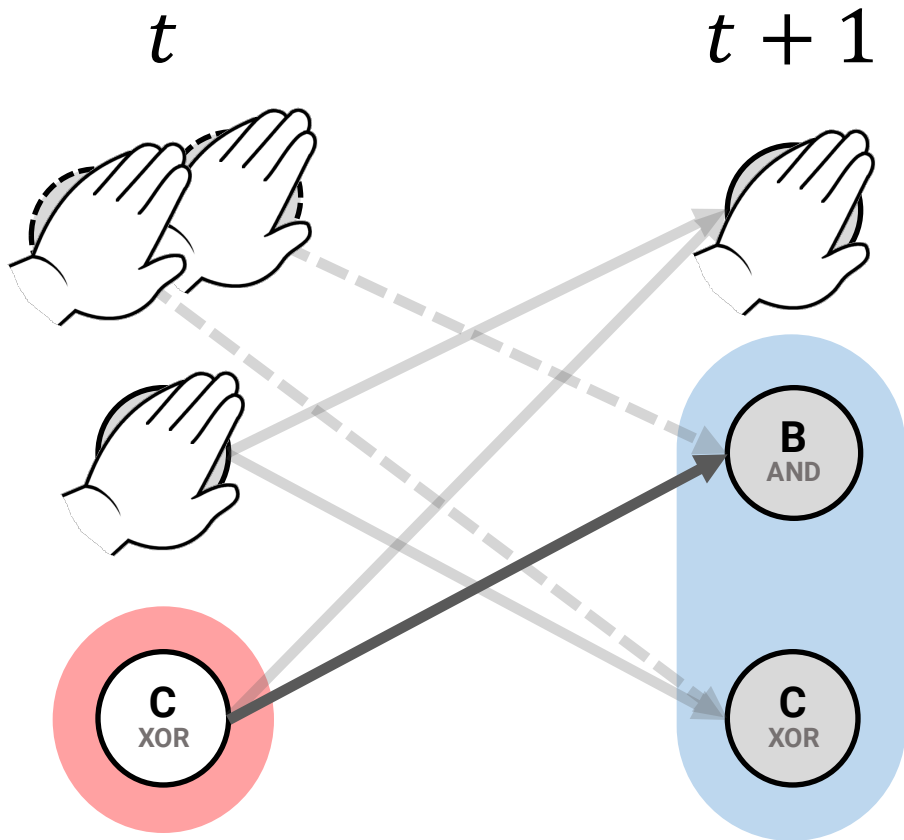

|               |   | Next state                                                                          |                                                                                     |                                                                                     |                                                                                     |
|---------------|---|-------------------------------------------------------------------------------------|-------------------------------------------------------------------------------------|-------------------------------------------------------------------------------------|-------------------------------------------------------------------------------------|
| B             | C | 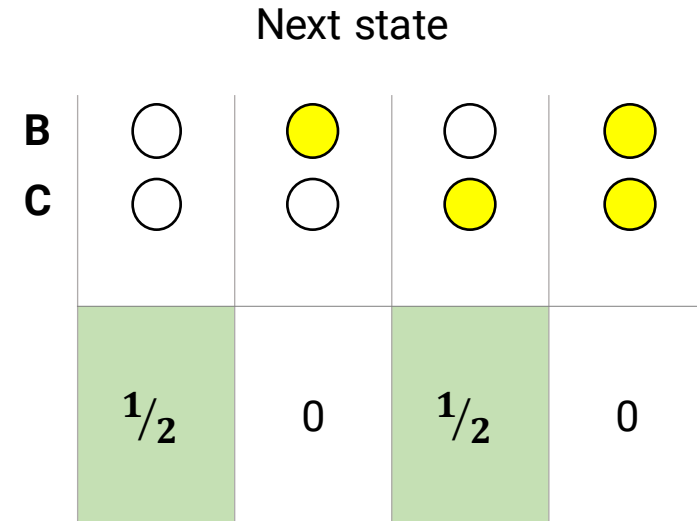 | 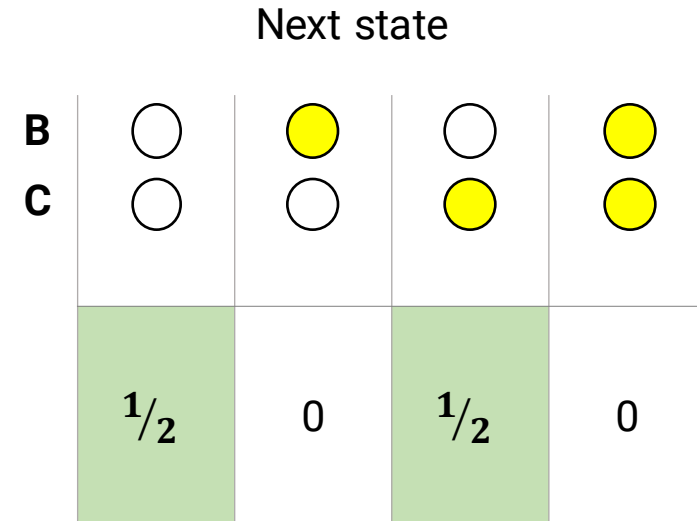 | 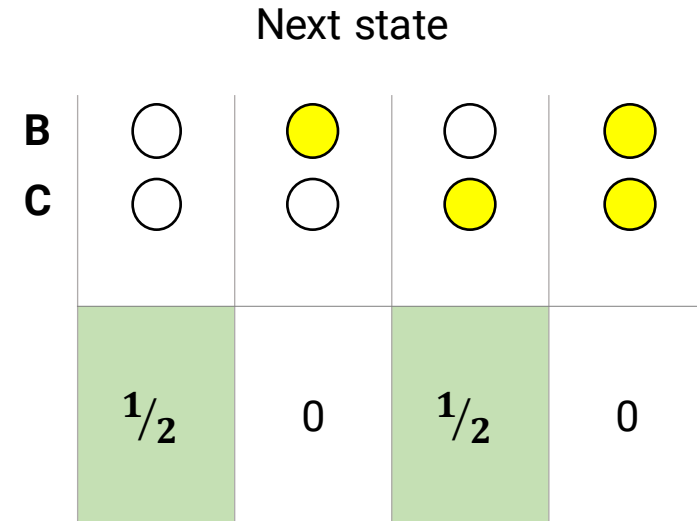 | 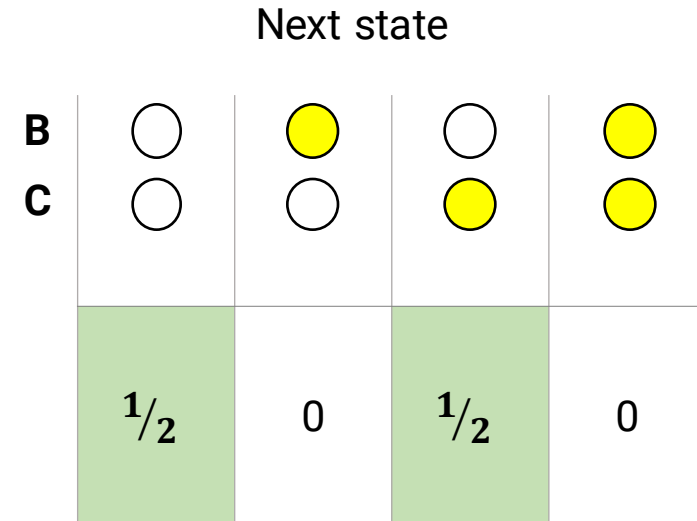 |
|               |   | 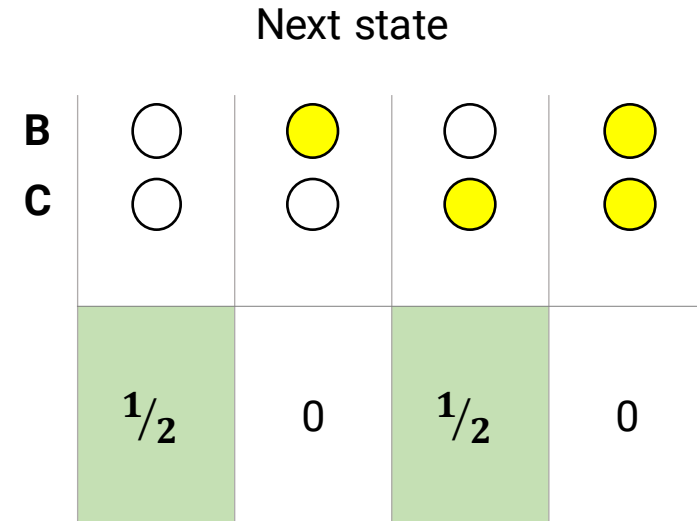 | 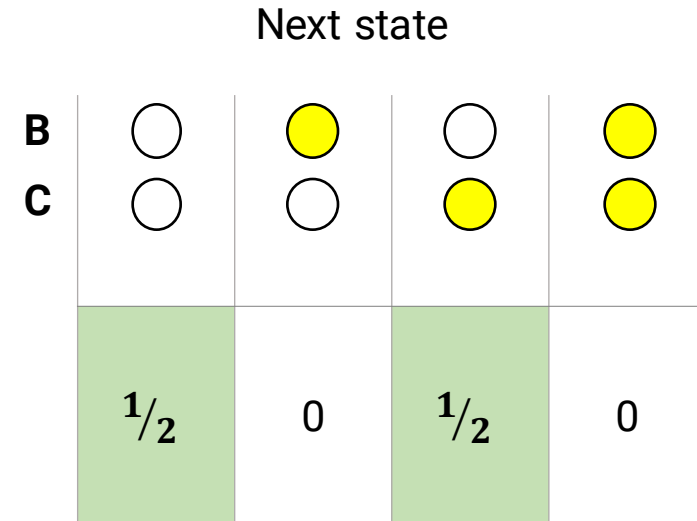 | 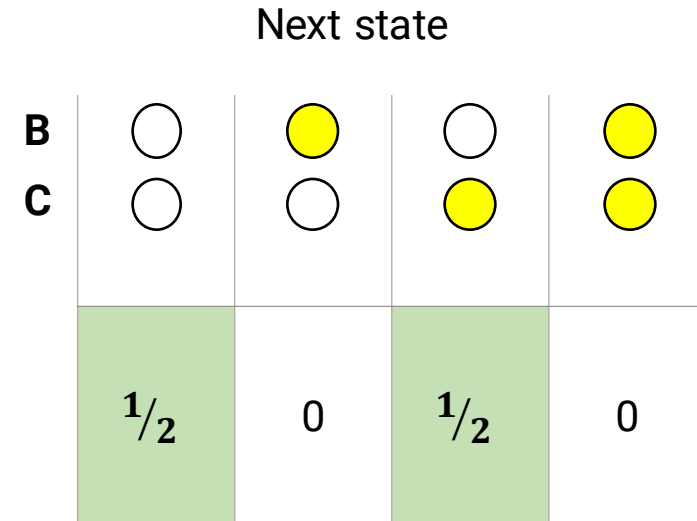 | 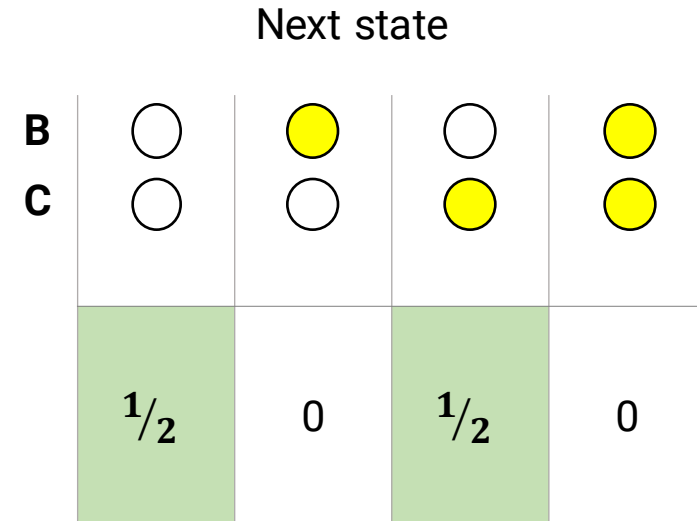 |
| $\frac{1}{2}$ |   | 0                                                                                   | $\frac{1}{2}$                                                                       | 0                                                                                   |                                                                                     |

To calculate the **unconstrained distribution**, we use the same method that we just did but **without conditioning on any mechanism**

Calculating an effect repertoire:  
**Expanding to the full state-space**

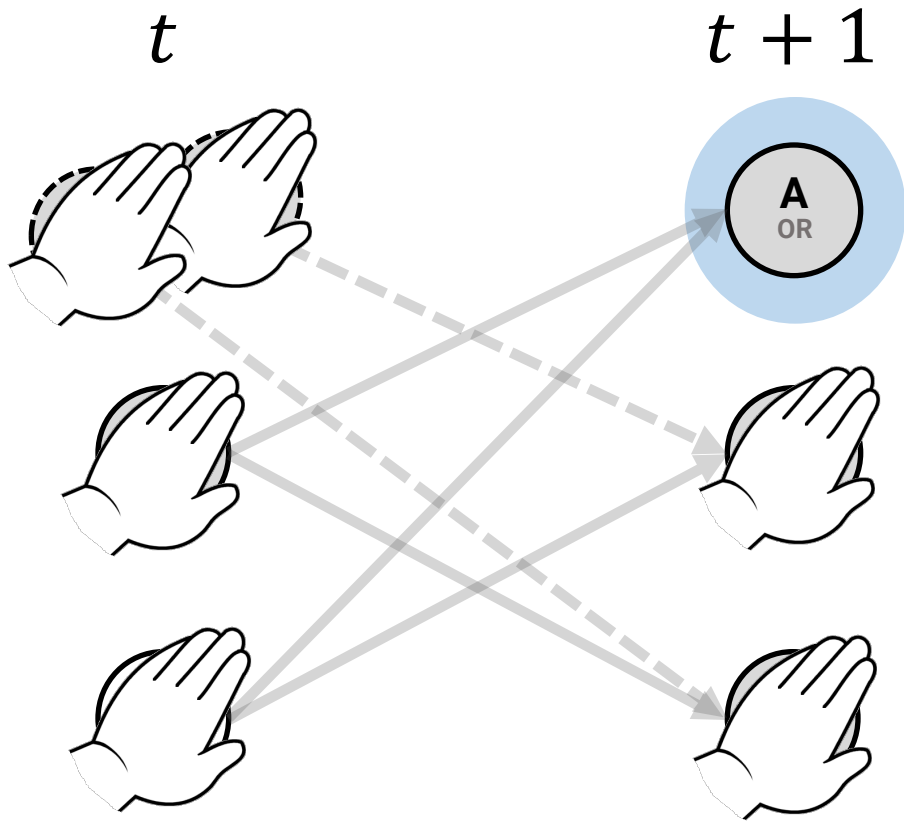

To calculate the **unconstrained distribution**, we use the same method that we just did but **without conditioning on any mechanism**

## Calculating an effect repertoire: Expanding to the full state-space

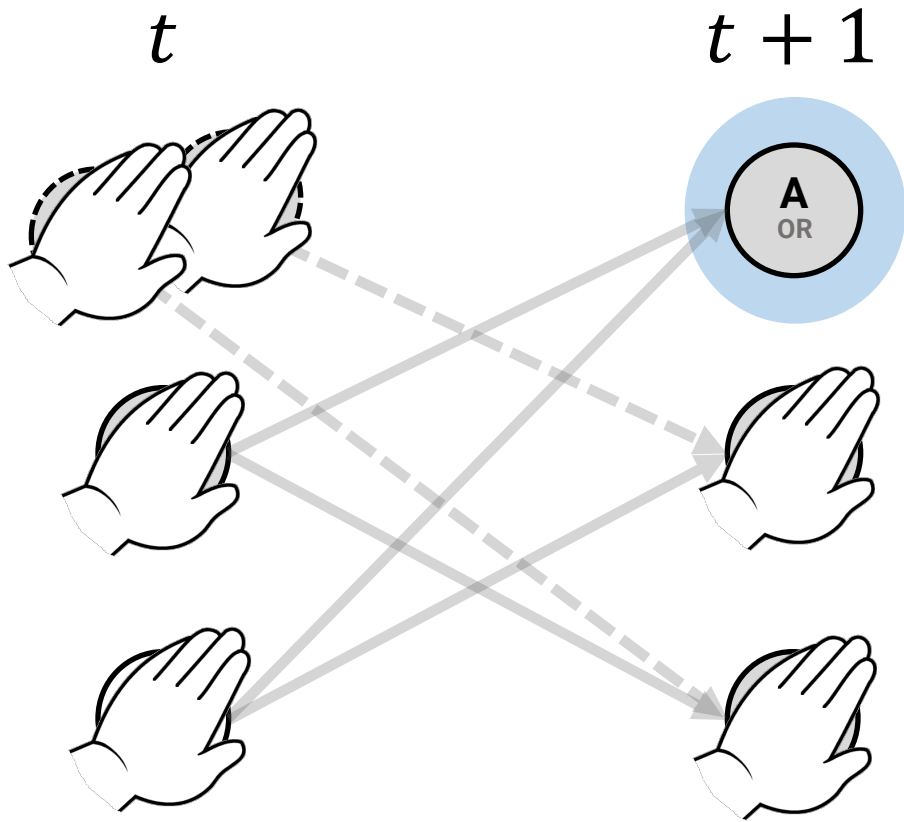

| Next state |                                                                                     |                                                                                     |
|------------|-------------------------------------------------------------------------------------|-------------------------------------------------------------------------------------|
| A          | 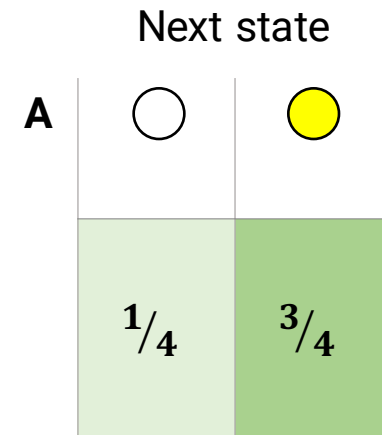 | 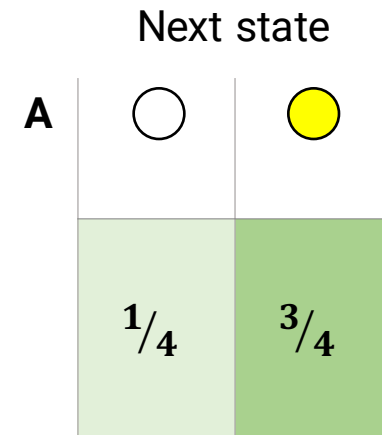 |
|            | $\frac{1}{4}$                                                                       | $\frac{3}{4}$                                                                       |

In this example, this is the unconstrained distribution over **A**'s next states (here this can be obtained immediately by observing that **A** is an OR gate)

# Calculating an effect repertoire: Expanding to the full state-space

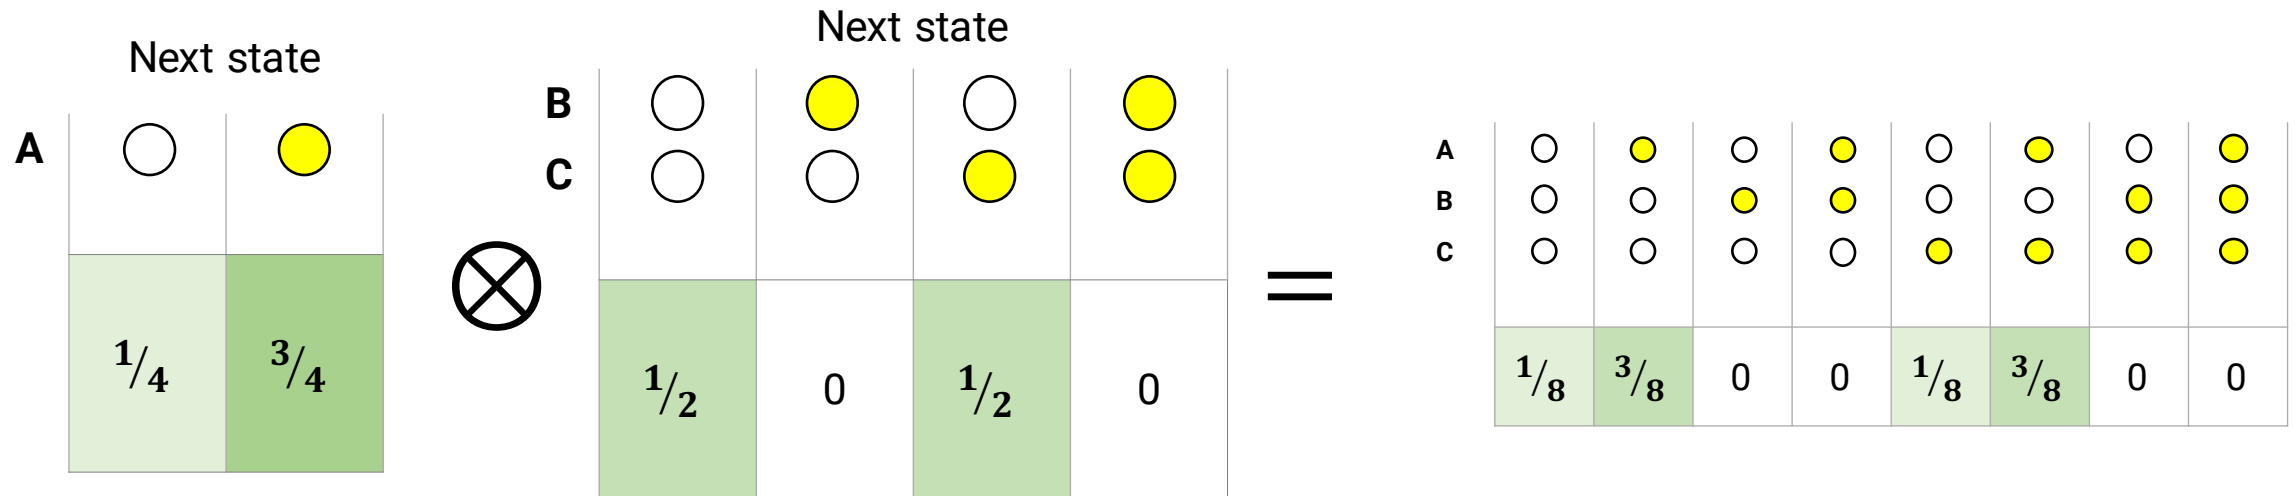

Taking the tensor product yields the final effect repertoire over the whole system

# Calculating an effect repertoire: Expanding to the full state-space

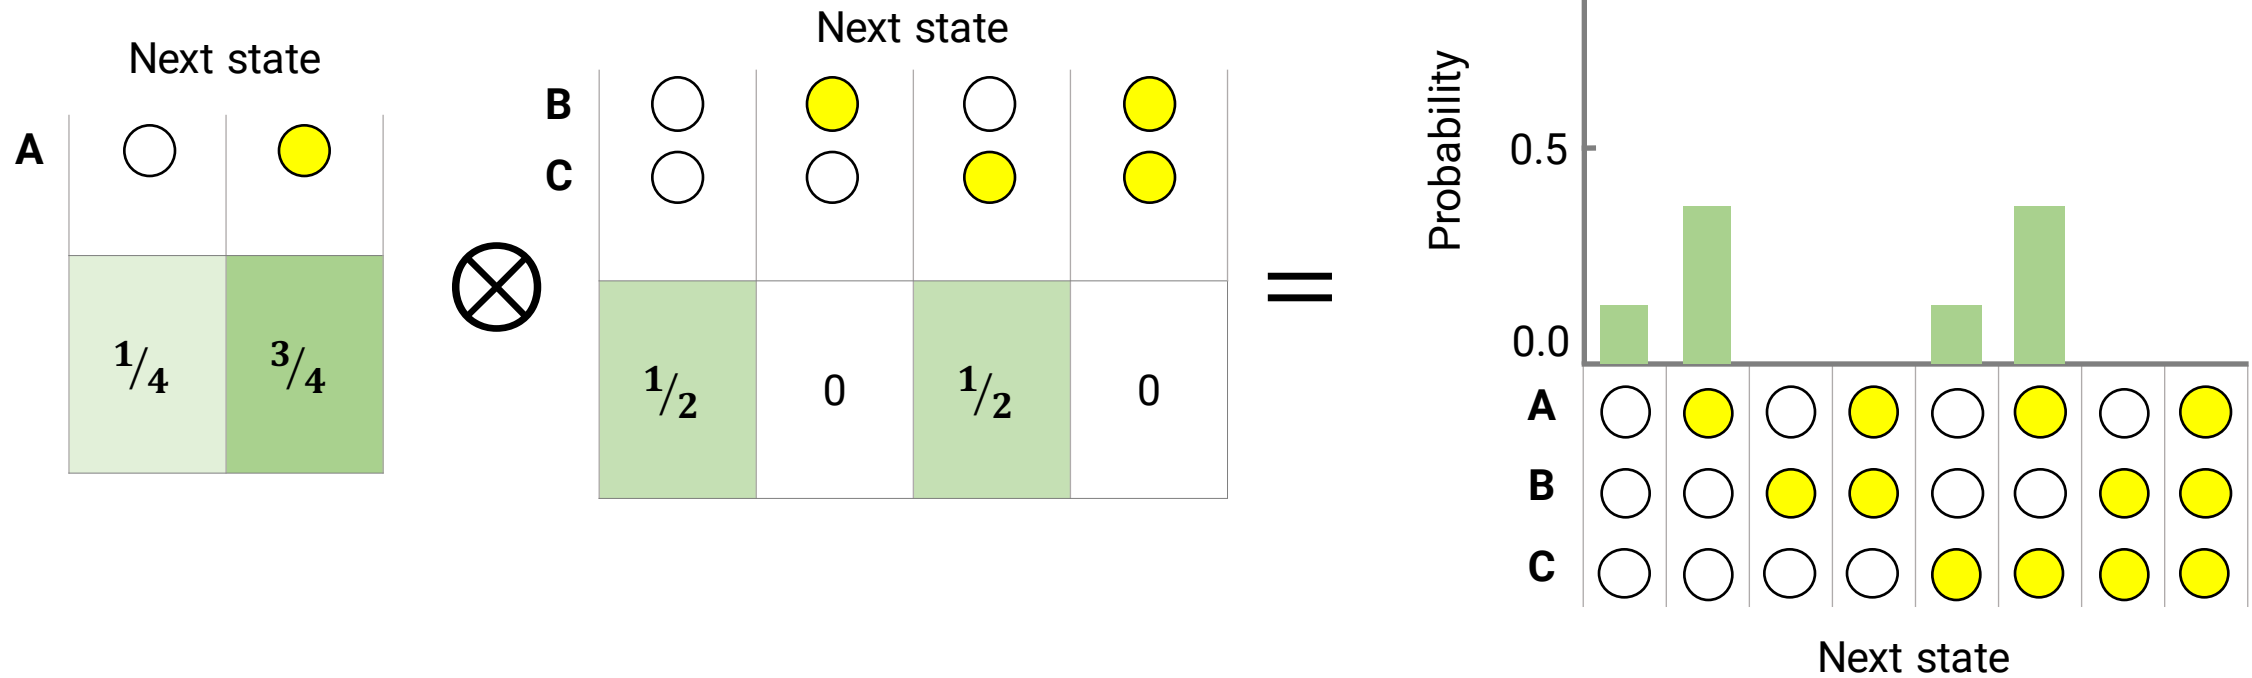

Taking the tensor product yields the final effect repertoire over the whole system

Calculating an effect repertoire:

## **A more practical method**

- In practice, calculations can be made simpler than described so far
- One trick we can use to simplify things stems from the fact that in our model of physical systems, we rule out instantaneous causation
- This is captured by the requirement that elements be conditionally independent
- That is, each element's state at  $t + 1$  depends only the system's state at  $t$  and not on other elements' states at  $t + 1$



Calculating an effect repertoire:

## **A more practical method**

- Conditional independence implies that if  $p$  is a distribution over the states of an element  $\mathbf{X}$  and  $q$  is the distribution over the states of  $\mathbf{Y}$ , then the **joint distribution** of  $\mathbf{X}$  and  $\mathbf{Y}$  is the product  $pq$
- So, when we calculate an effect repertoire over some purview, we can simply take the product of all the purview elements' individual effect repertoires
- This holds for the cause repertoires as well, though in that case the repertoires are over the individual mechanism elements
- This way we only ever need to calculate the effect repertoire over single-element purviews—so there can be no common input, and thus there's no need to actually implement virtual elements

Calculating an effect repertoire:

## **A note on computational techniques**

- For binary elements, the TPM can be more compactly stored and more easily manipulated for the purposes of calculating cause-effect repertoires when it is represented in **state-by-node form**
- In this form, columns correspond to nodes (elements), rather than states
- An entry  $(i, j)$  gives the probability that the element corresponding to  $j$  will be in state “ON” given the previous state  $i$

# Calculating a cause repertoire

- Now we'll discuss the cause repertoire
- The goal is again to obtain a distribution over purview states given the mechanism's current state
- Now, however, the distribution is over previous states of the purview
- The idea remains the same: use perturbation to determine how the mechanism in its current state constrains the purview

# Calculating a cause repertoire

- This entails perturbing the input of each mechanism element independently
- Again, however, there is the issue of common input
- For example, suppose we want to find the cause repertoire of **XY** over the purview **Z** in this system

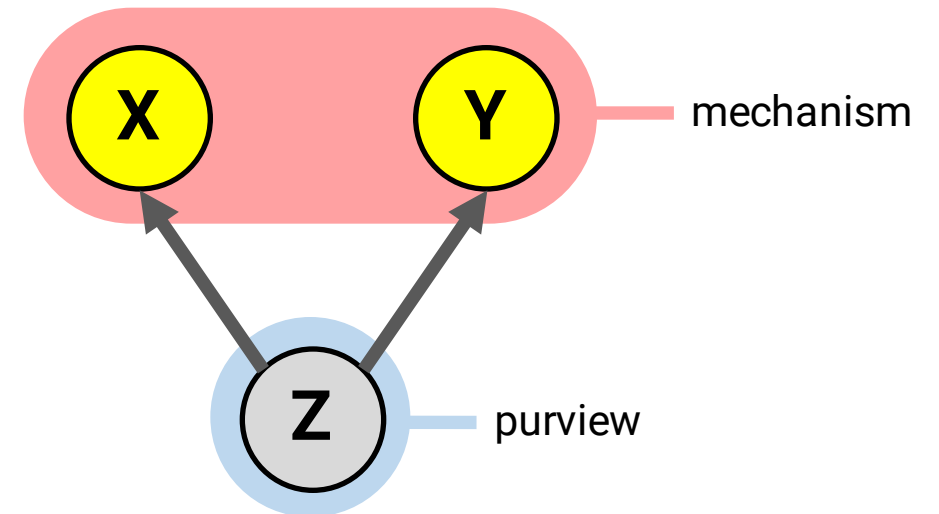

# Calculating a cause repertoire

- We want to independently provide each element in the mechanism with all its possible inputs
- That is, we want to provide **XY** with inputs (0, 0), (0, 1), (1, 0), and (1, 1)
- We can't do this by simply perturbing **Z**, because setting **Z** to 0 and 1 will only provide **X** and **Y** with inputs (0, 0) and (1, 1)

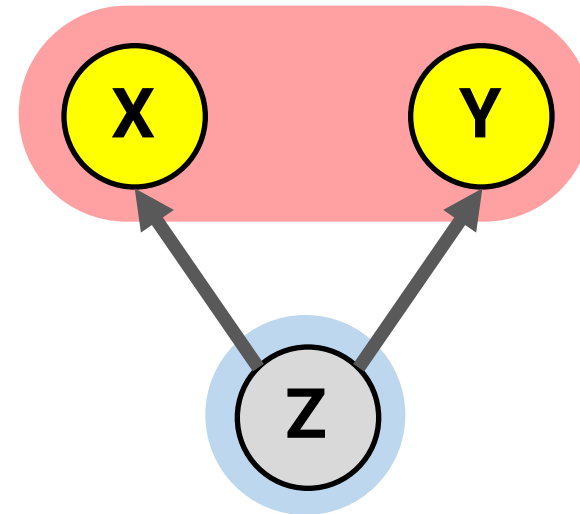

# Calculating a cause repertoire

- So we need to introduce virtual elements that we can perturb independently

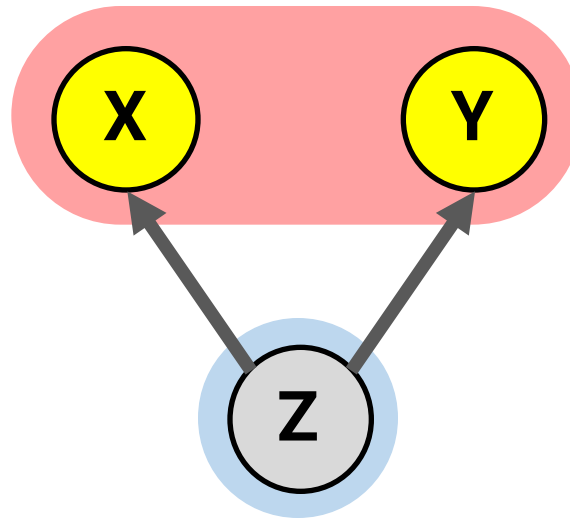

# Calculating a cause repertoire

- So we need to introduce virtual elements that we can perturb independently

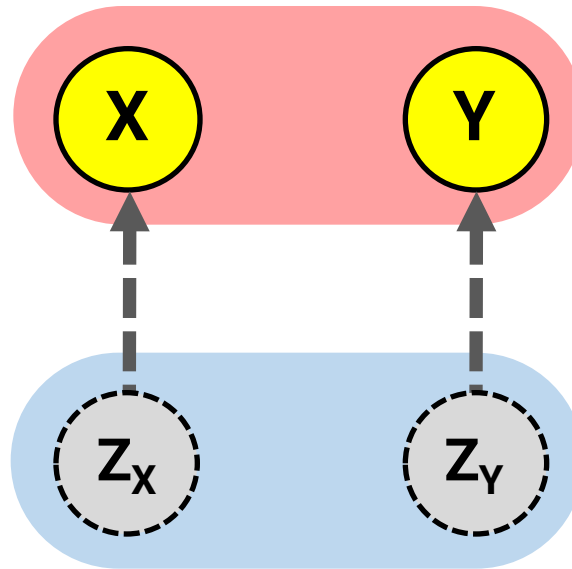

# Calculating a cause repertoire

- So we need to introduce virtual elements that we can perturb independently
- When we virtualize and perturb the elements at  $t - 1$  with equal likelihood, the unconstrained distribution over previous states is uniform
- This is consistent with the intuition that no previous state is *a priori* more likely than another

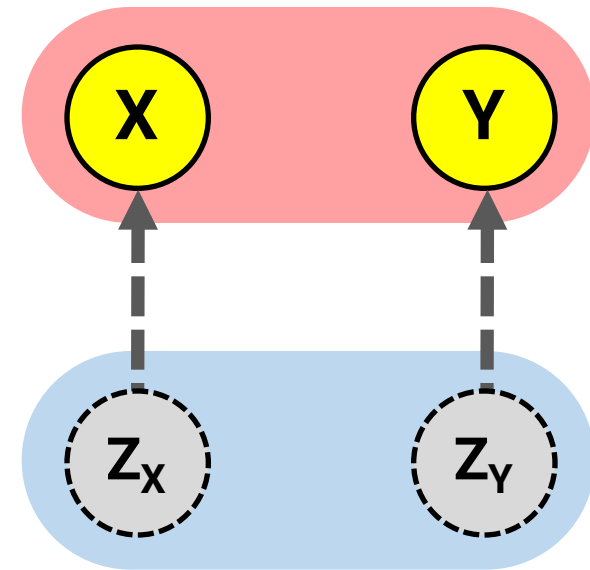



# Calculating a cause repertoire

- Conditional independence implies that cause repertoires of higher-order mechanisms can be calculated by simply taking the product of the repertoires of individual mechanism elements
- So in practice, there is no common input
- So virtual elements are implicit in the cause repertoire, but don't actually have to be implemented

# Calculating a cause repertoire

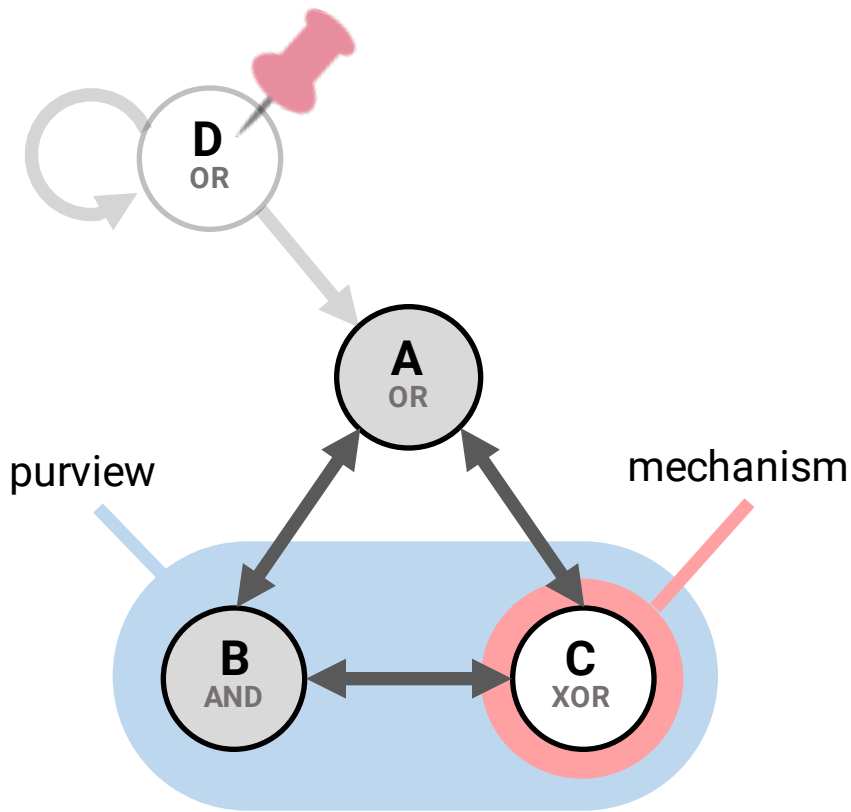

|               |   |   | Next state |   |   |   |   |   |   |   |
|---------------|---|---|------------|---|---|---|---|---|---|---|
|               |   |   | A          |   |   |   |   |   |   |   |
|               |   |   | B          |   |   |   |   |   |   |   |
|               |   |   | C          |   |   |   |   |   |   |   |
| Current state | A | B | C          |   |   |   |   |   |   |   |
|               |   |   |            | 1 | 0 | 0 | 0 | 0 | 0 | 0 |
|               |   |   |            | 0 | 0 | 0 | 0 | 1 | 0 | 0 |
|               |   |   |            | 0 | 0 | 0 | 0 | 0 | 1 | 0 |
|               |   |   |            | 0 | 1 | 0 | 0 | 0 | 0 | 0 |
|               |   |   |            | 0 | 1 | 0 | 0 | 0 | 0 | 0 |
|               |   |   |            | 0 | 0 | 0 | 0 | 0 | 0 | 1 |
|               |   |   |            | 0 | 0 | 0 | 0 | 1 | 0 | 0 |
|               |   |   |            | 0 | 0 | 0 | 1 | 0 | 0 | 0 |

Now we’ll calculate the cause repertoire of **C** over the purview **BC** in our example system

# Calculating a cause repertoire

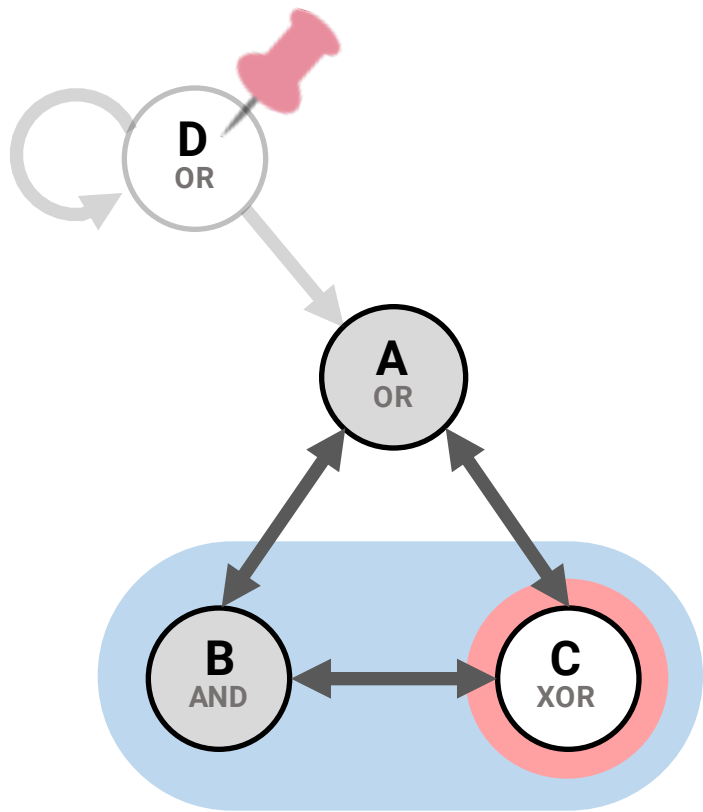

|               |                        |                        | Next state             |                        |                        |                        |                        |                        |                        |                        |
|---------------|------------------------|------------------------|------------------------|------------------------|------------------------|------------------------|------------------------|------------------------|------------------------|------------------------|
|               |                        |                        | A                      |                        |                        |                        |                        |                        |                        |                        |
|               |                        |                        | B                      |                        |                        |                        |                        |                        |                        |                        |
|               |                        |                        | C                      |                        |                        |                        |                        |                        |                        |                        |
| Current state | A                      | B                      | C                      | <div><div></div></div> | <div><div></div></div> | <div><div></div></div> | <div><div></div></div> | <div><div></div></div> | <div><div></div></div> | <div><div></div></div> |
|               | <div><div></div></div> | <div><div></div></div> | <div><div></div></div> | 1                      | 0                      | 0                      | 0                      | 0                      | 0                      | 0                      |
|               | <div><div></div></div> | <div><div></div></div> | <div><div></div></div> | 0                      | 0                      | 0                      | 0                      | 1                      | 0                      | 0                      |
|               | <div><div></div></div> | <div><div></div></div> | <div><div></div></div> | 0                      | 0                      | 0                      | 0                      | 0                      | 1                      | 0                      |
|               | <div><div></div></div> | <div><div></div></div> | <div><div></div></div> | 0                      | 1                      | 0                      | 0                      | 0                      | 0                      | 0                      |
|               | <div><div></div></div> | <div><div></div></div> | <div><div></div></div> | 0                      | 1                      | 0                      | 0                      | 0                      | 0                      | 0                      |
|               | <div><div></div></div> | <div><div></div></div> | <div><div></div></div> | 0                      | 0                      | 0                      | 0                      | 0                      | 0                      | 1                      |
|               | <div><div></div></div> | <div><div></div></div> | <div><div></div></div> | 0                      | 0                      | 0                      | 0                      | 1                      | 0                      | 0                      |
|               | <div><div></div></div> | <div><div></div></div> | <div><div></div></div> | 0                      | 0                      | 0                      | 1                      | 0                      | 0                      | 0                      |

We start by interpreting the TPM as giving the transition probabilities from the state at  $t - 1$  to  $t$

# Calculating a cause repertoire

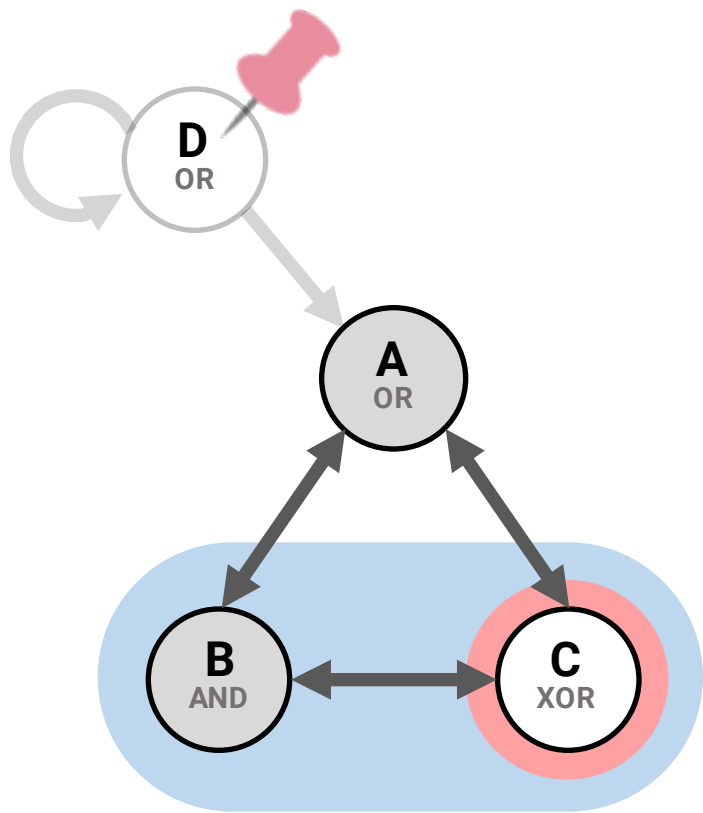

|                |                        |                        | Current state          |                        |                        |                        |                        |                        |                        |                        |
|----------------|------------------------|------------------------|------------------------|------------------------|------------------------|------------------------|------------------------|------------------------|------------------------|------------------------|
|                |                        |                        | A                      |                        |                        |                        |                        |                        |                        |                        |
|                |                        |                        | B                      |                        |                        |                        |                        |                        |                        |                        |
|                |                        |                        | C                      |                        |                        |                        |                        |                        |                        |                        |
| Previous state | A                      | B                      | C                      | <div><div></div></div> | <div><div></div></div> | <div><div></div></div> | <div><div></div></div> | <div><div></div></div> | <div><div></div></div> | <div><div></div></div> |
|                | <div><div></div></div> | <div><div></div></div> | <div><div></div></div> | 1                      | 0                      | 0                      | 0                      | 0                      | 0                      | 0                      |
|                | <div><div></div></div> | <div><div></div></div> | <div><div></div></div> | 0                      | 0                      | 0                      | 0                      | 1                      | 0                      | 0                      |
|                | <div><div></div></div> | <div><div></div></div> | <div><div></div></div> | 0                      | 0                      | 0                      | 0                      | 0                      | 1                      | 0                      |
|                | <div><div></div></div> | <div><div></div></div> | <div><div></div></div> | 0                      | 1                      | 0                      | 0                      | 0                      | 0                      | 0                      |
|                | <div><div></div></div> | <div><div></div></div> | <div><div></div></div> | 0                      | 1                      | 0                      | 0                      | 0                      | 0                      | 0                      |
|                | <div><div></div></div> | <div><div></div></div> | <div><div></div></div> | 0                      | 0                      | 0                      | 0                      | 0                      | 0                      | 1                      |
|                | <div><div></div></div> | <div><div></div></div> | <div><div></div></div> | 0                      | 0                      | 0                      | 0                      | 0                      | 1                      | 0                      |
|                | <div><div></div></div> | <div><div></div></div> | <div><div></div></div> | 0                      | 0                      | 0                      | 1                      | 0                      | 0                      | 0                      |

We start by interpreting the TPM as giving the transition probabilities from the state at  $t - 1$  to  $t$

# Calculating a cause repertoire

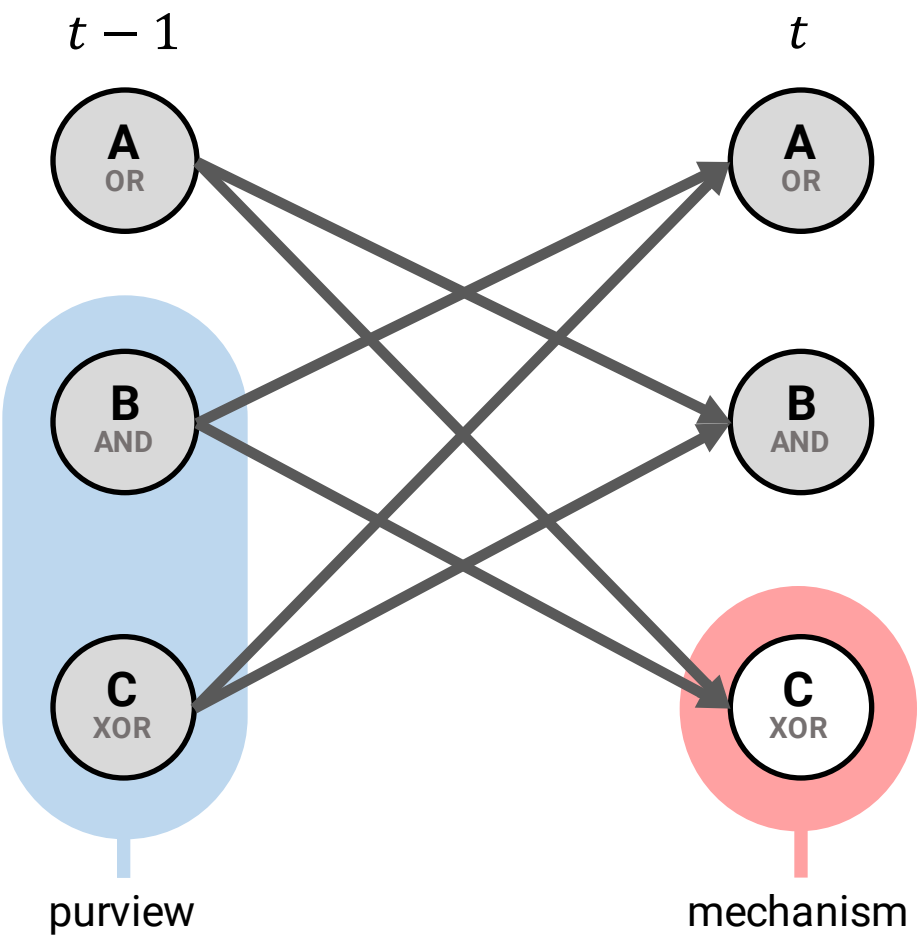

Now we'll unfold the graph in time again

|                |                                  |                                  | Current state                    |   |   |   |   |   |   |   |
|----------------|----------------------------------|----------------------------------|----------------------------------|---|---|---|---|---|---|---|
|                |                                  |                                  | A                                |   |   |   |   |   |   |   |
|                |                                  |                                  | B                                |   |   |   |   |   |   |   |
|                |                                  |                                  | C                                |   |   |   |   |   |   |   |
| Previous state | A                                | B                                | C                                |   |   |   |   |   |   |   |
|                | <input type="radio"/>            | <input type="radio"/>            | <input type="radio"/>            | 1 | 0 | 0 | 0 | 0 | 0 | 0 |
|                | <input checked="" type="radio"/> | <input type="radio"/>            | <input type="radio"/>            | 0 | 0 | 0 | 0 | 1 | 0 | 0 |
|                | <input type="radio"/>            | <input checked="" type="radio"/> | <input type="radio"/>            | 0 | 0 | 0 | 0 | 0 | 1 | 0 |
|                | <input checked="" type="radio"/> | <input checked="" type="radio"/> | <input type="radio"/>            | 0 | 1 | 0 | 0 | 0 | 0 | 0 |
|                | <input type="radio"/>            | <input type="radio"/>            | <input checked="" type="radio"/> | 0 | 1 | 0 | 0 | 0 | 0 | 0 |
|                | <input checked="" type="radio"/> | <input type="radio"/>            | <input checked="" type="radio"/> | 0 | 0 | 0 | 0 | 0 | 0 | 1 |
|                | <input type="radio"/>            | <input checked="" type="radio"/> | <input checked="" type="radio"/> | 0 | 0 | 0 | 0 | 0 | 1 | 0 |
|                | <input checked="" type="radio"/> | <input checked="" type="radio"/> | <input checked="" type="radio"/> | 0 | 0 | 0 | 1 | 0 | 0 | 0 |

# Calculating a cause repertoire: Virtual elements

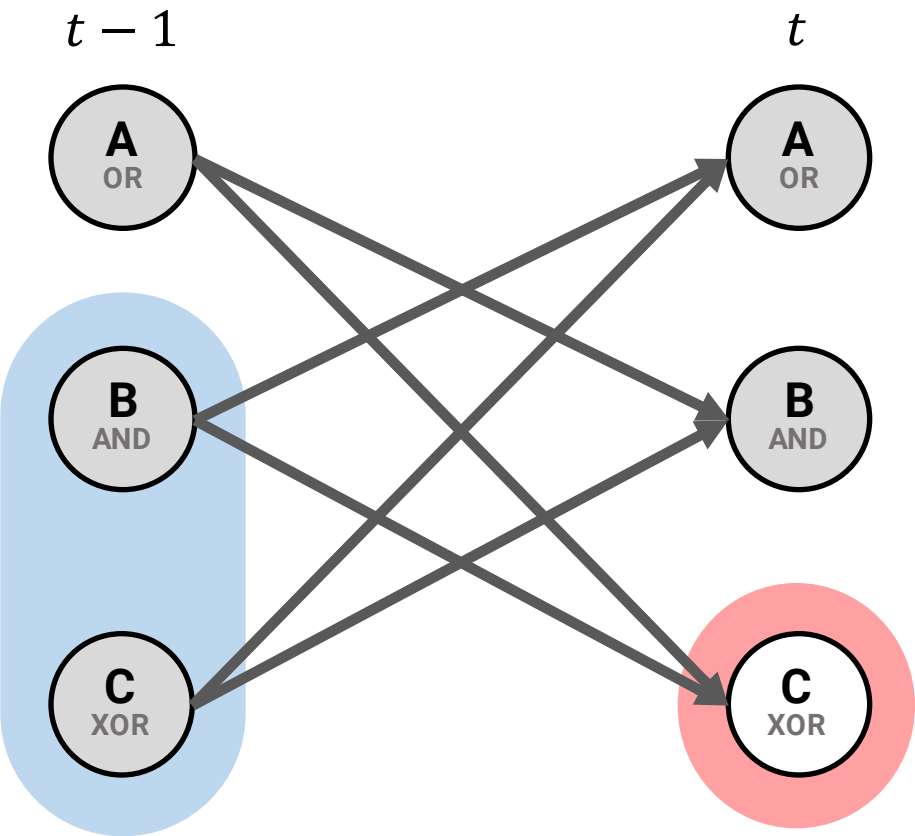

|                |                                  |                                  | Current state                    |   |   |   |   |   |   |   |
|----------------|----------------------------------|----------------------------------|----------------------------------|---|---|---|---|---|---|---|
|                |                                  |                                  | A                                |   |   |   |   |   |   |   |
|                |                                  |                                  | B                                |   |   |   |   |   |   |   |
|                |                                  |                                  | C                                |   |   |   |   |   |   |   |
| Previous state | A                                | B                                | C                                |   |   |   |   |   |   |   |
|                | <input type="radio"/>            | <input type="radio"/>            | <input type="radio"/>            | 1 | 0 | 0 | 0 | 0 | 0 | 0 |
|                | <input checked="" type="radio"/> | <input type="radio"/>            | <input type="radio"/>            | 0 | 0 | 0 | 0 | 1 | 0 | 0 |
|                | <input type="radio"/>            | <input checked="" type="radio"/> | <input type="radio"/>            | 0 | 0 | 0 | 0 | 0 | 1 | 0 |
|                | <input checked="" type="radio"/> | <input checked="" type="radio"/> | <input type="radio"/>            | 0 | 1 | 0 | 0 | 0 | 0 | 0 |
|                | <input type="radio"/>            | <input type="radio"/>            | <input checked="" type="radio"/> | 0 | 1 | 0 | 0 | 0 | 0 | 0 |
|                | <input checked="" type="radio"/> | <input type="radio"/>            | <input checked="" type="radio"/> | 0 | 0 | 0 | 0 | 0 | 0 | 1 |
|                | <input type="radio"/>            | <input checked="" type="radio"/> | <input checked="" type="radio"/> | 0 | 0 | 0 | 0 | 0 | 1 | 0 |
|                | <input checked="" type="radio"/> | <input checked="" type="radio"/> | <input checked="" type="radio"/> | 0 | 0 | 0 | 1 | 0 | 0 | 0 |

Here we would introduce virtual elements and calculate the virtualized TPM, as with the effect repertoire, but in this example we can omit that step since the mechanism consists of only one element (so there can be no common input)

Calculating a cause repertoire:  
**Marginalizing-out non-purview elements**

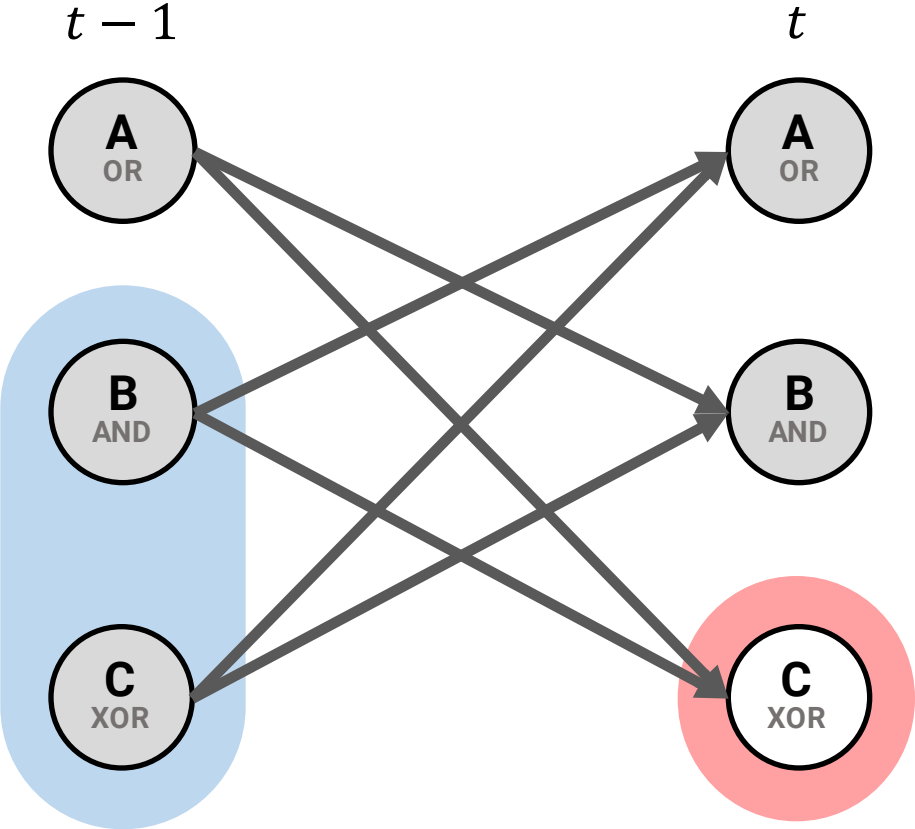

|                |                                  |                                  | Current state                    |   |   |   |   |   |   |   |
|----------------|----------------------------------|----------------------------------|----------------------------------|---|---|---|---|---|---|---|
|                |                                  |                                  | A                                |   |   |   |   |   |   |   |
|                |                                  |                                  | B                                |   |   |   |   |   |   |   |
|                |                                  |                                  | C                                |   |   |   |   |   |   |   |
| Previous state | A                                | B                                | C                                |   |   |   |   |   |   |   |
|                | <input type="radio"/>            | <input type="radio"/>            | <input type="radio"/>            | 1 | 0 | 0 | 0 | 0 | 0 | 0 |
|                | <input checked="" type="radio"/> | <input type="radio"/>            | <input type="radio"/>            | 0 | 0 | 0 | 0 | 1 | 0 | 0 |
|                | <input type="radio"/>            | <input checked="" type="radio"/> | <input type="radio"/>            | 0 | 0 | 0 | 0 | 0 | 1 | 0 |
|                | <input checked="" type="radio"/> | <input checked="" type="radio"/> | <input type="radio"/>            | 0 | 1 | 0 | 0 | 0 | 0 | 0 |
|                | <input type="radio"/>            | <input type="radio"/>            | <input checked="" type="radio"/> | 0 | 1 | 0 | 0 | 0 | 0 | 0 |
|                | <input checked="" type="radio"/> | <input type="radio"/>            | <input checked="" type="radio"/> | 0 | 0 | 0 | 0 | 0 | 0 | 1 |
|                | <input type="radio"/>            | <input checked="" type="radio"/> | <input checked="" type="radio"/> | 0 | 0 | 0 | 0 | 0 | 1 | 0 |
|                | <input checked="" type="radio"/> | <input checked="" type="radio"/> | <input checked="" type="radio"/> | 0 | 0 | 0 | 1 | 0 | 0 | 0 |

The first step is then to ignore the elements outside the purview (in this case **A**) and marginalize them out of the TPM

Calculating a cause repertoire:  
**Marginalizing-out non-purview elements**

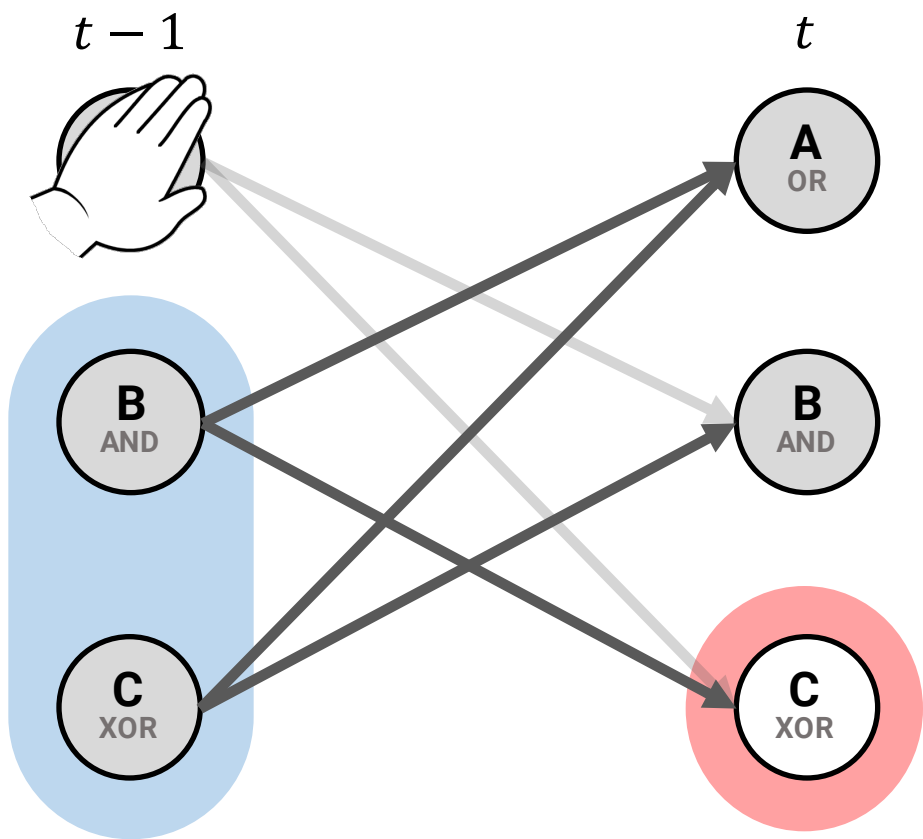

|                |   |   | Current state |   |   |   |   |   |   |   |
|----------------|---|---|---------------|---|---|---|---|---|---|---|
|                |   |   | A             |   |   |   |   |   |   |   |
|                |   |   | B             |   |   |   |   |   |   |   |
|                |   |   | C             |   |   |   |   |   |   |   |
| Previous state | A | B | C             |   |   |   |   |   |   |   |
|                |   |   |               | 1 | 0 | 0 | 0 | 0 | 0 | 0 |
|                |   |   |               | 0 | 0 | 0 | 0 | 1 | 0 | 0 |
|                |   |   |               | 0 | 0 | 0 | 0 | 0 | 1 | 0 |
|                |   |   |               | 0 | 1 | 0 | 0 | 0 | 0 | 0 |
|                |   |   |               | 0 | 1 | 0 | 0 | 0 | 0 | 0 |
|                |   |   |               | 0 | 0 | 0 | 0 | 0 | 0 | 1 |
|                |   |   |               | 0 | 0 | 0 | 0 | 1 | 0 | 0 |
|                |   |   |               | 0 | 0 | 0 | 1 | 0 | 0 | 0 |

The first step is then to ignore the elements outside the purview (in this case **A**) and marginalize them out of the TPM



# Calculating a cause repertoire: Marginalizing-out non-purview elements

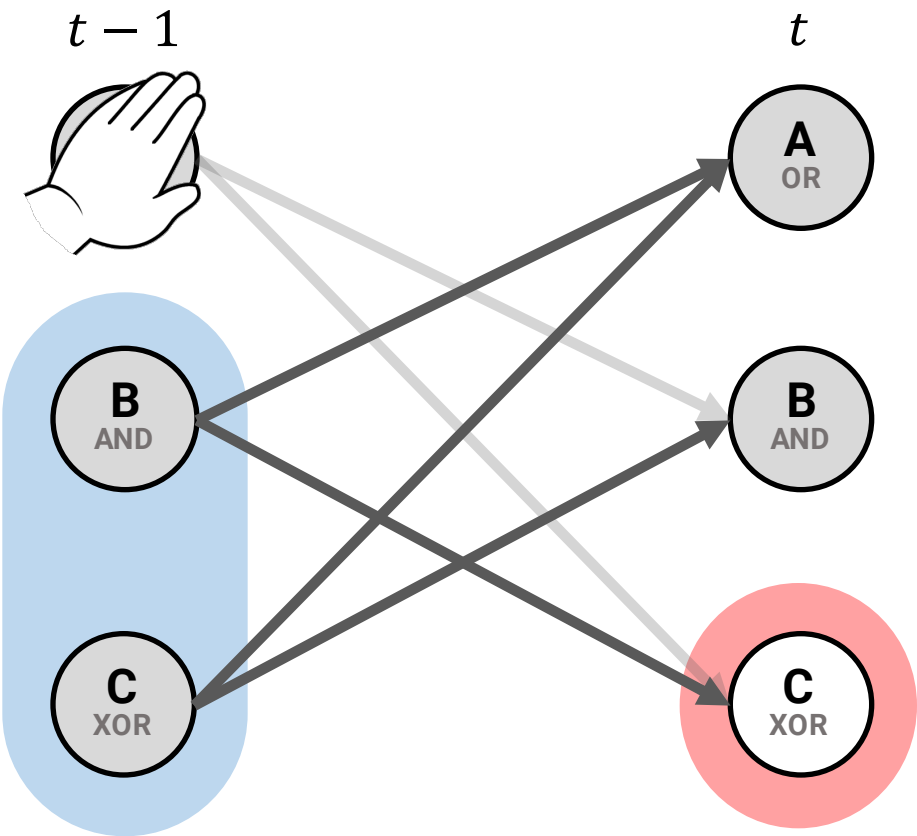

|                |   |   | Current state |   |   |   |   |   |   |   |
|----------------|---|---|---------------|---|---|---|---|---|---|---|
|                |   |   | A             |   |   |   |   |   |   |   |
|                |   |   | B             |   |   |   |   |   |   |   |
|                |   |   | C             |   |   |   |   |   |   |   |
| Previous state | A | B | C             |   |   |   |   |   |   |   |
|                |   |   |               | 1 | 0 | 0 | 0 | 0 | 0 | 0 |
|                |   |   |               | 0 | 0 | 0 | 0 | 1 | 0 | 0 |
|                |   |   |               | 0 | 0 | 0 | 0 | 0 | 1 | 0 |
|                |   |   |               | 0 | 1 | 0 | 0 | 0 | 0 | 0 |
|                |   |   |               | 0 | 1 | 0 | 0 | 0 | 0 | 0 |
|                |   |   |               | 0 | 0 | 0 | 0 | 0 | 0 | 1 |
|                |   |   |               | 0 | 0 | 0 | 0 | 1 | 0 | 0 |
|                |   |   |               | 0 | 0 | 0 | 1 | 0 | 0 | 0 |

Note that since the purview is now at  $t - 1$ , the roles of columns and rows in the TPM have switched

Calculating a cause repertoire:  
**Marginalizing-out non-purview elements**

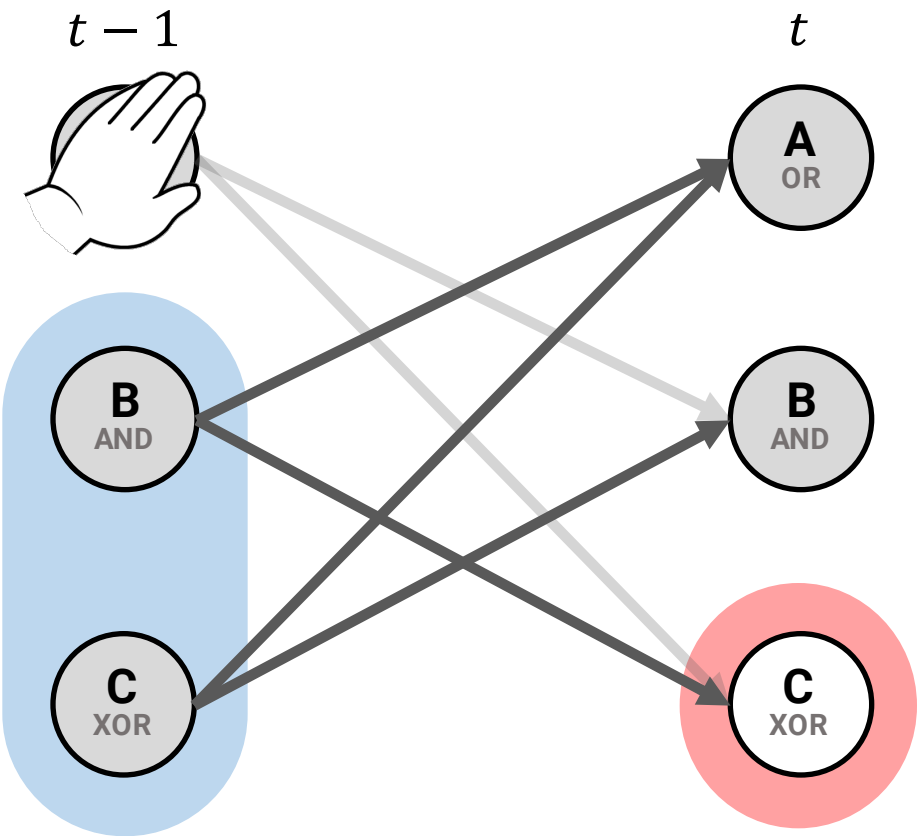

|                |   |   | Current state |   |   |   |   |   |   |   |
|----------------|---|---|---------------|---|---|---|---|---|---|---|
|                |   |   | A             |   |   |   |   |   |   |   |
|                |   |   | B             |   |   |   |   |   |   |   |
|                |   |   | C             |   |   |   |   |   |   |   |
| Previous state | A | B | C             |   |   |   |   |   |   |   |
|                |   |   |               | 1 | 0 | 0 | 0 | 0 | 0 | 0 |
|                |   |   |               | 0 | 0 | 0 | 0 | 1 | 0 | 0 |
|                |   |   |               | 0 | 0 | 0 | 0 | 0 | 1 | 0 |
|                |   |   |               | 0 | 1 | 0 | 0 | 0 | 0 | 0 |
|                |   |   |               | 0 | 1 | 0 | 0 | 0 | 0 | 0 |
|                |   |   |               | 0 | 0 | 0 | 0 | 0 | 0 | 1 |
|                |   |   |               | 0 | 0 | 0 | 0 | 0 | 1 | 0 |
|                |   |   |               | 0 | 0 | 0 | 1 | 0 | 0 | 0 |

We now sum and renormalize pairs of **rows** corresponding to states at  $t - 1$  that differ only by **A**'s state

Calculating a cause repertoire:  
**Marginalizing-out non-purview elements**

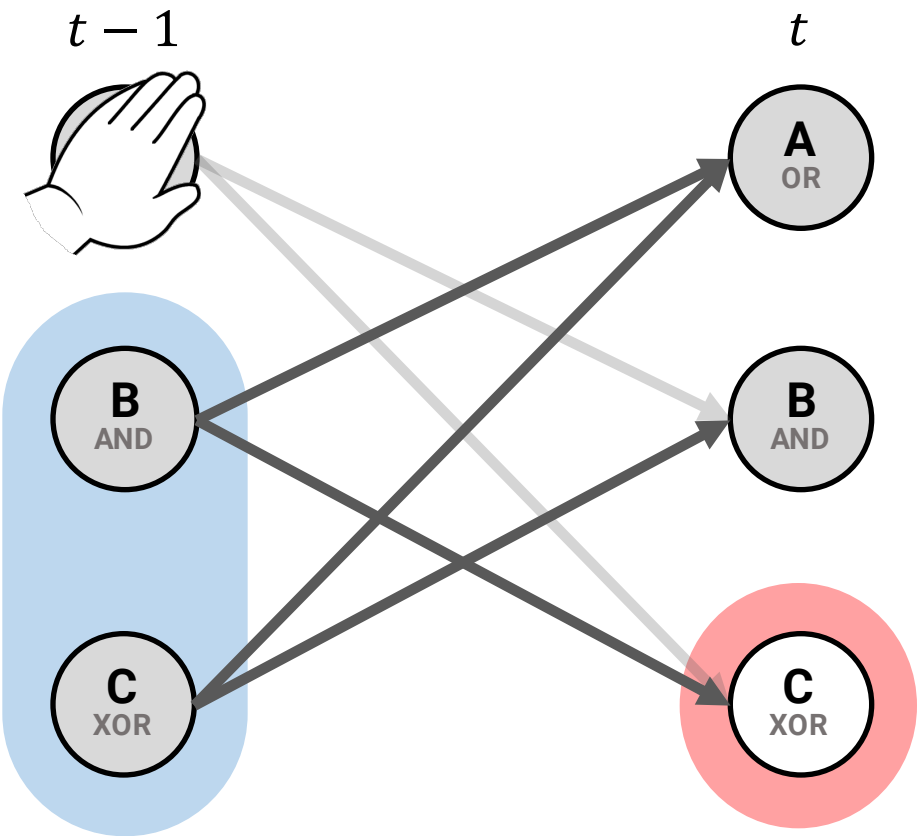

|                |   |   | Current state |   |   |   |   |   |   |   |
|----------------|---|---|---------------|---|---|---|---|---|---|---|
|                |   |   | A             |   |   |   |   |   |   |   |
|                |   |   | B             |   |   |   |   |   |   |   |
|                |   |   | C             |   |   |   |   |   |   |   |
| Previous state | A | B | C             |   |   |   |   |   |   |   |
|                |   |   |               | 1 | 0 | 0 | 0 | 0 | 0 | 0 |
|                |   |   |               | 0 | 0 | 0 | 0 | 1 | 0 | 0 |
|                |   |   |               | 0 | 0 | 0 | 0 | 0 | 1 | 0 |
|                |   |   |               | 0 | 1 | 0 | 0 | 0 | 0 | 0 |
|                |   |   |               | 0 | 1 | 0 | 0 | 0 | 0 | 0 |
|                |   |   |               | 0 | 0 | 0 | 0 | 0 | 0 | 1 |
|                |   |   |               | 0 | 0 | 0 | 0 | 0 | 1 | 0 |
|                |   |   |               | 0 | 0 | 0 | 1 | 0 | 0 | 0 |

We now sum and renormalize pairs of **rows** corresponding to states at  $t - 1$  that differ only by **A**'s state

Calculating a cause repertoire:  
**Marginalizing-out non-purview elements**

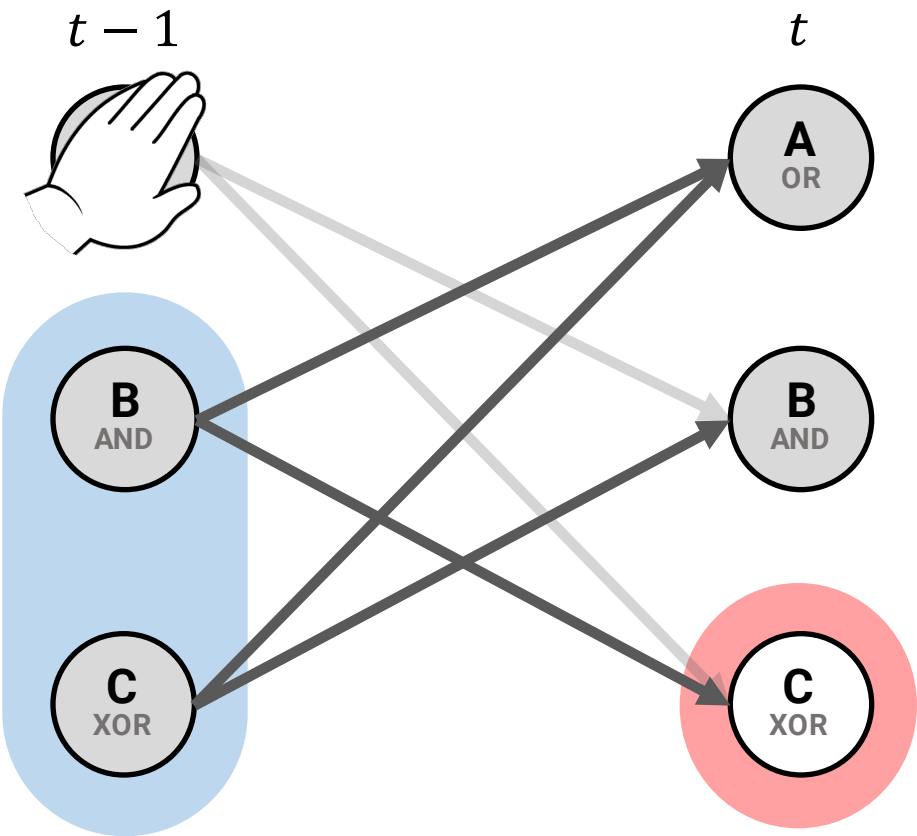

|                |                                  |                                  | Current state                    |   |   |   |   |   |   |   |
|----------------|----------------------------------|----------------------------------|----------------------------------|---|---|---|---|---|---|---|
|                |                                  |                                  | A                                |   |   |   |   |   |   |   |
|                |                                  |                                  | A                                |   |   |   |   |   |   |   |
|                |                                  |                                  | B                                |   |   |   |   |   |   |   |
|                |                                  |                                  | C                                |   |   |   |   |   |   |   |
| Previous state | A                                | B                                | C                                |   |   |   |   |   |   |   |
|                | <input type="radio"/>            | <input type="radio"/>            | <input type="radio"/>            | 1 | 0 | 0 | 0 | 0 | 0 | 0 |
|                | <input checked="" type="radio"/> | <input type="radio"/>            | <input type="radio"/>            | 0 | 0 | 0 | 0 | 1 | 0 | 0 |
|                | <input type="radio"/>            | <input checked="" type="radio"/> | <input type="radio"/>            | 0 | 0 | 0 | 0 | 0 | 1 | 0 |
|                | <input checked="" type="radio"/> | <input checked="" type="radio"/> | <input type="radio"/>            | 0 | 1 | 0 | 0 | 0 | 0 | 0 |
|                | <input type="radio"/>            | <input type="radio"/>            | <input checked="" type="radio"/> | 0 | 1 | 0 | 0 | 0 | 0 | 0 |
|                | <input checked="" type="radio"/> | <input type="radio"/>            | <input checked="" type="radio"/> | 0 | 0 | 0 | 0 | 0 | 0 | 1 |
|                | <input type="radio"/>            | <input checked="" type="radio"/> | <input checked="" type="radio"/> | 0 | 0 | 0 | 0 | 0 | 1 | 0 |
|                | <input checked="" type="radio"/> | <input checked="" type="radio"/> | <input checked="" type="radio"/> | 0 | 0 | 0 | 1 | 0 | 0 | 0 |

We now sum and renormalize pairs of **rows** corresponding to states at  $t - 1$  that differ only by **A**'s state

Calculating a cause repertoire:  
**Marginalizing-out non-purview elements**

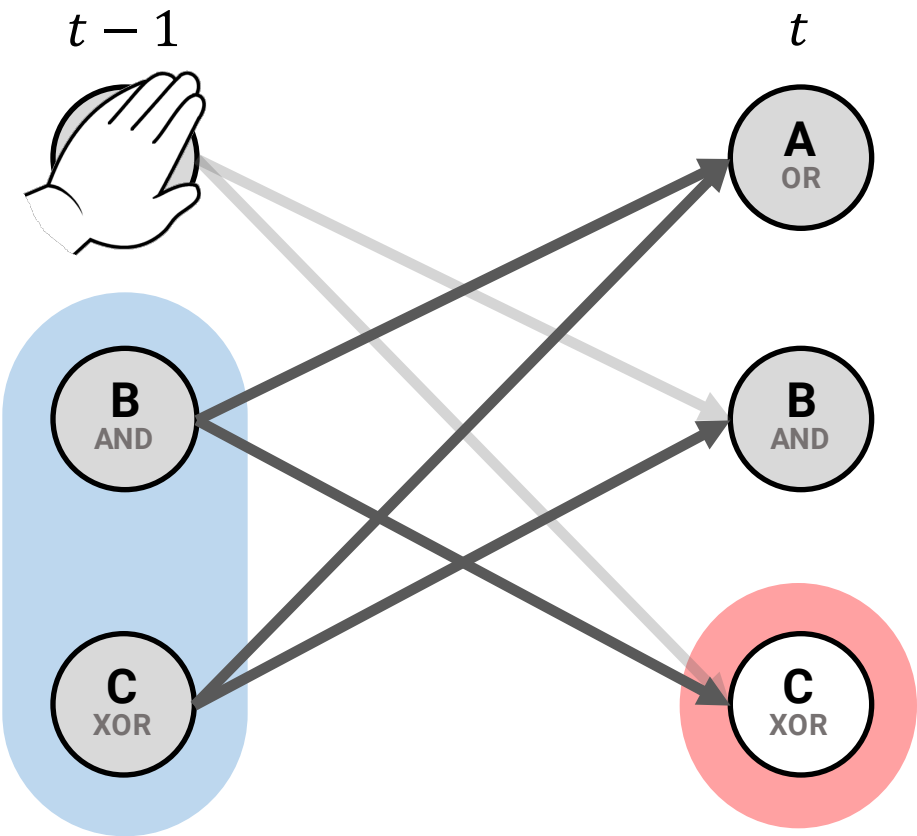

|                |                                  | Current state                    |   |   |   |   |   |   |   |
|----------------|----------------------------------|----------------------------------|---|---|---|---|---|---|---|
|                |                                  | A                                |   |   |   |   |   |   |   |
|                |                                  | B                                | C |   |   |   |   |   |   |
| Previous state | <input type="radio"/>            | <input type="radio"/>            |   | 1 | 0 | 0 | 0 | 0 | 0 |
|                | <input type="radio"/>            | <input type="radio"/>            |   | 0 | 0 | 0 | 0 | 1 | 0 |
|                | <input checked="" type="radio"/> | <input type="radio"/>            |   | 0 | 0 | 0 | 0 | 0 | 1 |
|                | <input checked="" type="radio"/> | <input type="radio"/>            |   | 0 | 1 | 0 | 0 | 0 | 0 |
|                | <input type="radio"/>            | <input checked="" type="radio"/> |   | 0 | 1 | 0 | 0 | 0 | 0 |
|                | <input type="radio"/>            | <input checked="" type="radio"/> |   | 0 | 0 | 0 | 0 | 0 | 0 |
|                | <input checked="" type="radio"/> | <input checked="" type="radio"/> |   | 0 | 0 | 0 | 0 | 1 | 0 |
|                | <input checked="" type="radio"/> | <input checked="" type="radio"/> |   | 0 | 0 | 0 | 1 | 0 | 0 |

We now sum and renormalize pairs of **rows** corresponding to states at  $t - 1$  that differ only by **A**'s state

Calculating a cause repertoire:  
**Marginalizing-out non-purview elements**

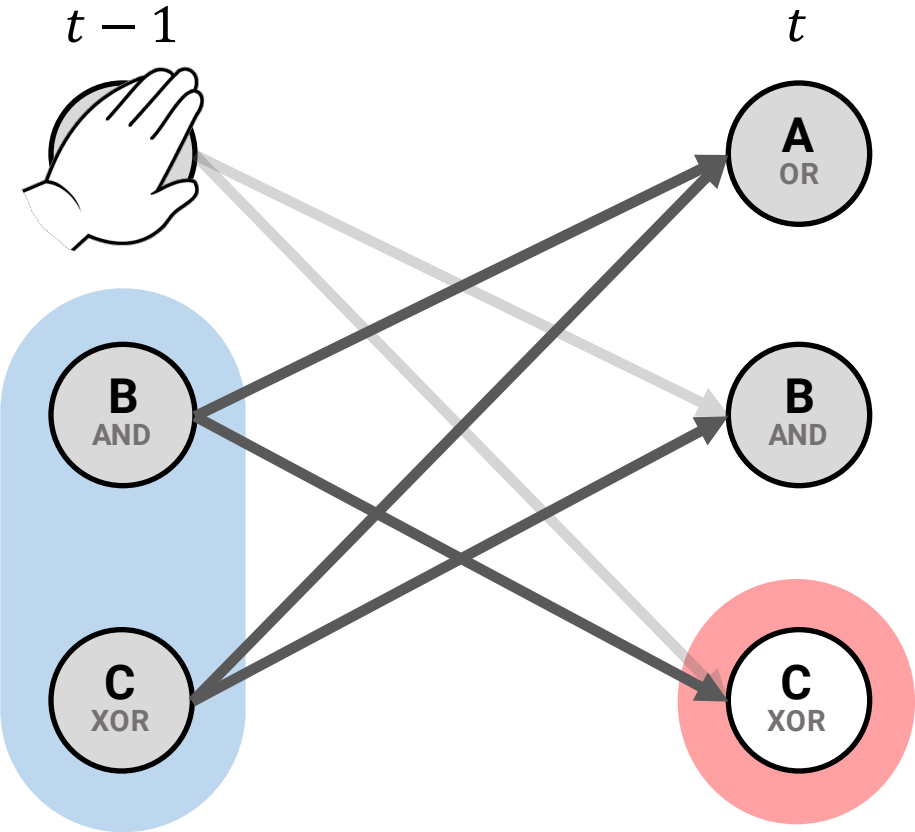

|                |                                   | Current state                     |   |   |   |   |   |   |   |
|----------------|-----------------------------------|-----------------------------------|---|---|---|---|---|---|---|
|                |                                   | A                                 |   |   |   |   |   |   |   |
|                |                                   | B                                 |   |   |   |   |   |   |   |
|                |                                   | C                                 |   |   |   |   |   |   |   |
| Previous state | B C                               | <div><div></div><div></div></div> |   |   |   |   |   |   |   |
|                | <div><div></div><div></div></div> | 1                                 | 0 | 0 | 0 | 1 | 0 | 0 | 0 |
|                | <div><div></div><div></div></div> | 0                                 | 1 | 0 | 0 | 0 | 1 | 0 | 0 |
|                | <div><div></div><div></div></div> | 0                                 | 1 | 0 | 0 | 0 | 0 | 0 | 1 |
| Previous state | B C                               | <div><div></div><div></div></div> |   |   |   |   |   |   |   |
|                | <div><div></div><div></div></div> | 0                                 | 0 | 0 | 1 | 0 | 1 | 0 | 0 |

We now sum and renormalize pairs of **rows** corresponding to states at  $t-1$  that differ only by **A**'s state

Calculating a cause repertoire:  
**Marginalizing-out non-purview elements**

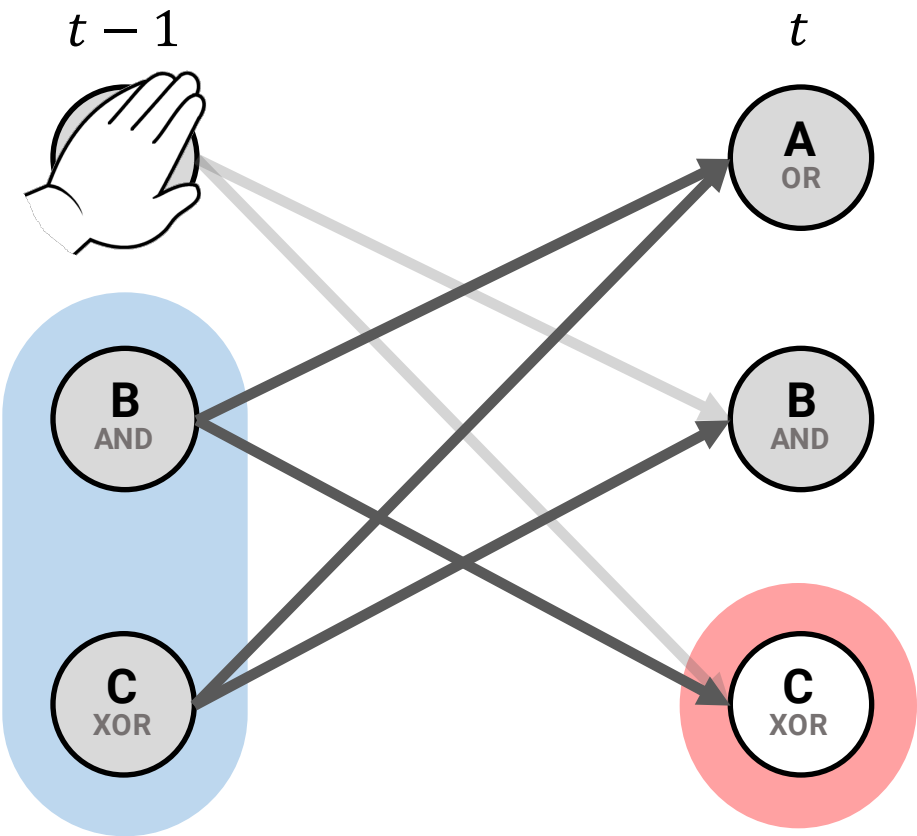

|                |     | Current state |     |     |   |     |     |     |     |
|----------------|-----|---------------|-----|-----|---|-----|-----|-----|-----|
|                |     | A             |     |     |   |     |     |     |     |
|                |     | A             |     |     |   |     |     |     |     |
|                |     | B             |     |     |   |     |     |     |     |
|                |     | C             |     |     |   |     |     |     |     |
| Previous state | B C |               |     |     |   |     |     |     |     |
|                |     |               |     |     |   |     |     |     |     |
|                |     |               |     |     |   |     |     |     |     |
|                |     |               |     |     |   |     |     |     |     |
|                |     |               |     |     |   |     |     |     |     |
|                |     |               | 1/2 | 0   | 0 | 0   | 1/2 | 0   | 0   |
|                |     |               | 0   | 1/2 | 0 | 0   | 0   | 1/2 | 0   |
|                |     |               | 0   | 1/2 | 0 | 0   | 0   | 0   | 1/2 |
|                |     |               | 0   | 0   | 0 | 1/2 | 0   | 1/2 | 0   |

We now sum and renormalize pairs of **rows** corresponding to states at  $t - 1$  that differ only by **A**'s state

Calculating a cause repertoire:  
**Marginalizing-out non-purview elements**

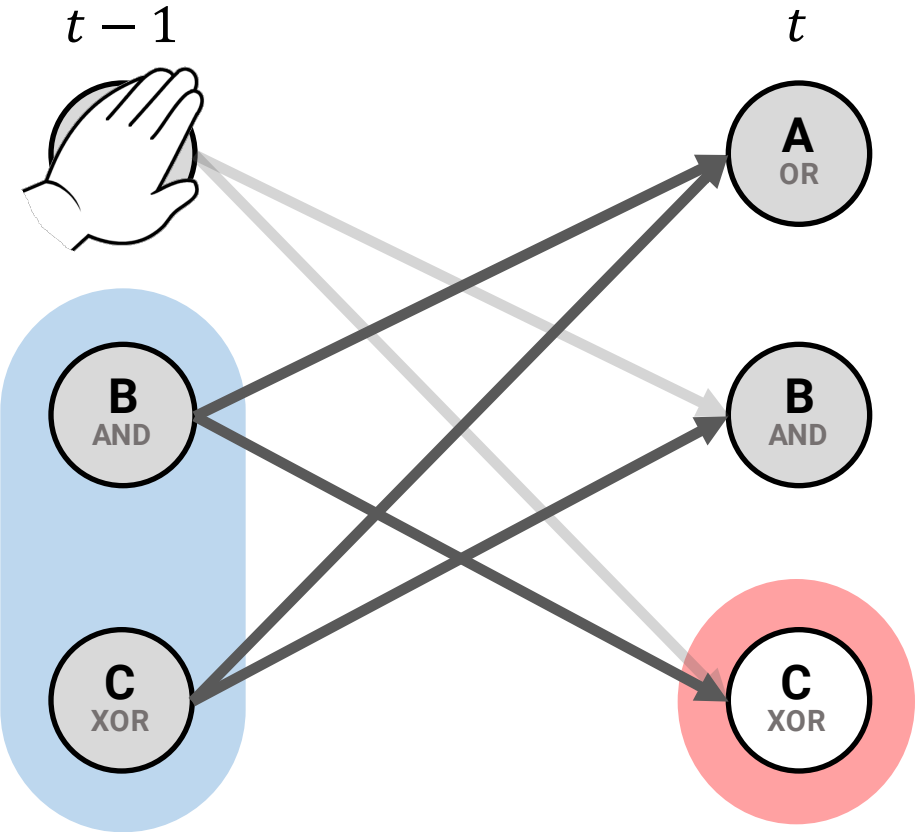

|                |                   | Current state |               |   |               |               |               |   |               |
|----------------|-------------------|---------------|---------------|---|---------------|---------------|---------------|---|---------------|
|                |                   | A             |               |   |               |               |               |   |               |
|                |                   | B             | C             |   |               |               |               |   |               |
| Previous state | <b>B</b> <b>C</b> |               |               |   |               |               |               |   |               |
|                | <b>○ ○</b>        | $\frac{1}{2}$ | 0             | 0 | 0             | $\frac{1}{2}$ | 0             | 0 | 0             |
|                | <b>● ○</b>        | 0             | $\frac{1}{2}$ | 0 | 0             | 0             | $\frac{1}{2}$ | 0 | 0             |
|                | <b>○ ●</b>        | 0             | $\frac{1}{2}$ | 0 | 0             | 0             | 0             | 0 | $\frac{1}{2}$ |
|                | <b>● ●</b>        | 0             | 0             | 0 | $\frac{1}{2}$ | 0             | $\frac{1}{2}$ | 0 | 0             |

We now sum and renormalize pairs of **rows** corresponding to states at  $t - 1$  that differ only by **A**'s state



Calculating a cause repertoire:  
**Marginalizing-out non-mechanism elements**

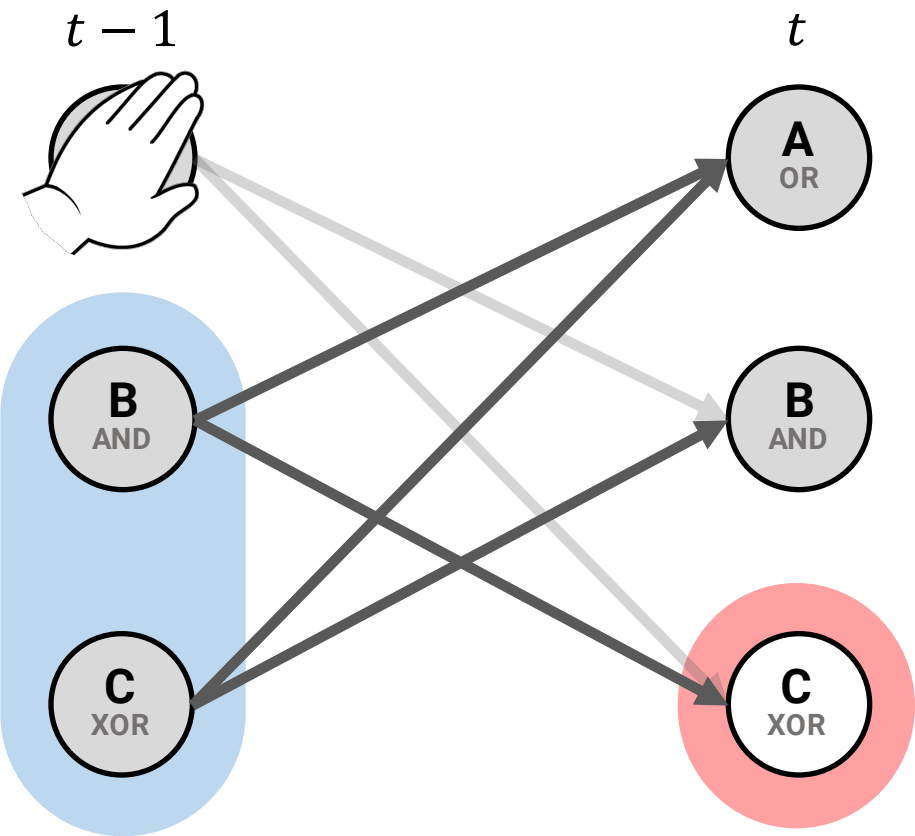

|                |                                  | Current state                    |               |               |   |               |               |               |               |
|----------------|----------------------------------|----------------------------------|---------------|---------------|---|---------------|---------------|---------------|---------------|
|                |                                  | A                                |               |               |   |               |               |               |               |
|                |                                  | B                                | C             |               |   |               |               |               |               |
| Previous state | <b>B</b>                         | <b>C</b>                         |               |               |   |               |               |               |               |
|                | <input type="radio"/>            | <input type="radio"/>            | $\frac{1}{2}$ | 0             | 0 | 0             | $\frac{1}{2}$ | 0             | 0             |
|                | <input checked="" type="radio"/> | <input type="radio"/>            | 0             | $\frac{1}{2}$ | 0 | 0             | 0             | $\frac{1}{2}$ | 0             |
|                | <input type="radio"/>            | <input checked="" type="radio"/> | 0             | $\frac{1}{2}$ | 0 | 0             | 0             | 0             | $\frac{1}{2}$ |
|                | <input checked="" type="radio"/> | <input checked="" type="radio"/> | 0             | 0             | 0 | $\frac{1}{2}$ | 0             | $\frac{1}{2}$ | 0             |

Now we marginalize over the current states of elements outside the mechanism (**A** and **B**)

Calculating a cause repertoire:  
**Marginalizing-out non-mechanism elements**

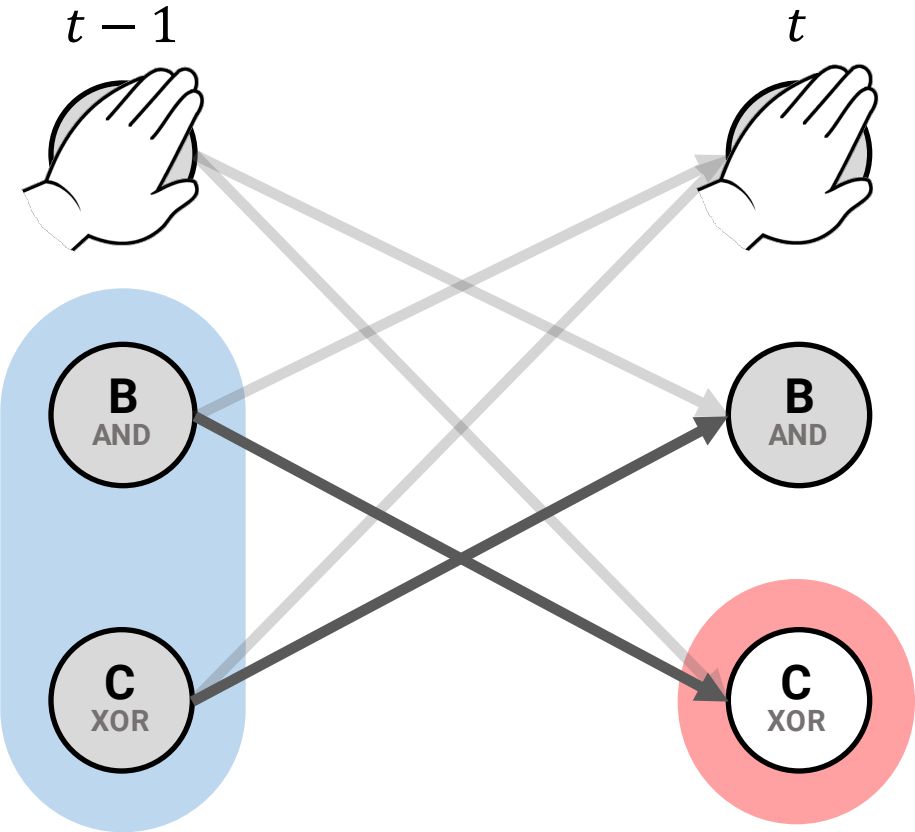

|                |     | Current state |               |   |               |               |               |   |               |
|----------------|-----|---------------|---------------|---|---------------|---------------|---------------|---|---------------|
| Previous state | A   |               |               |   |               |               |               |   |               |
|                | B   |               |               |   |               |               |               |   |               |
|                | C   |               |               |   |               |               |               |   |               |
|                | B C |               |               |   |               |               |               |   |               |
|                |     | $\frac{1}{2}$ | 0             | 0 | 0             | $\frac{1}{2}$ | 0             | 0 | 0             |
|                |     | 0             | $\frac{1}{2}$ | 0 | 0             | 0             | $\frac{1}{2}$ | 0 | 0             |
|                |     | 0             | $\frac{1}{2}$ | 0 | 0             | 0             | 0             | 0 | $\frac{1}{2}$ |
|                |     | 0             | 0             | 0 | $\frac{1}{2}$ | 0             | $\frac{1}{2}$ | 0 | 0             |

Now we marginalize over the current states of elements outside the mechanism (**A** and **B**)

Calculating a cause repertoire:  
**Marginalizing-out non-mechanism elements**

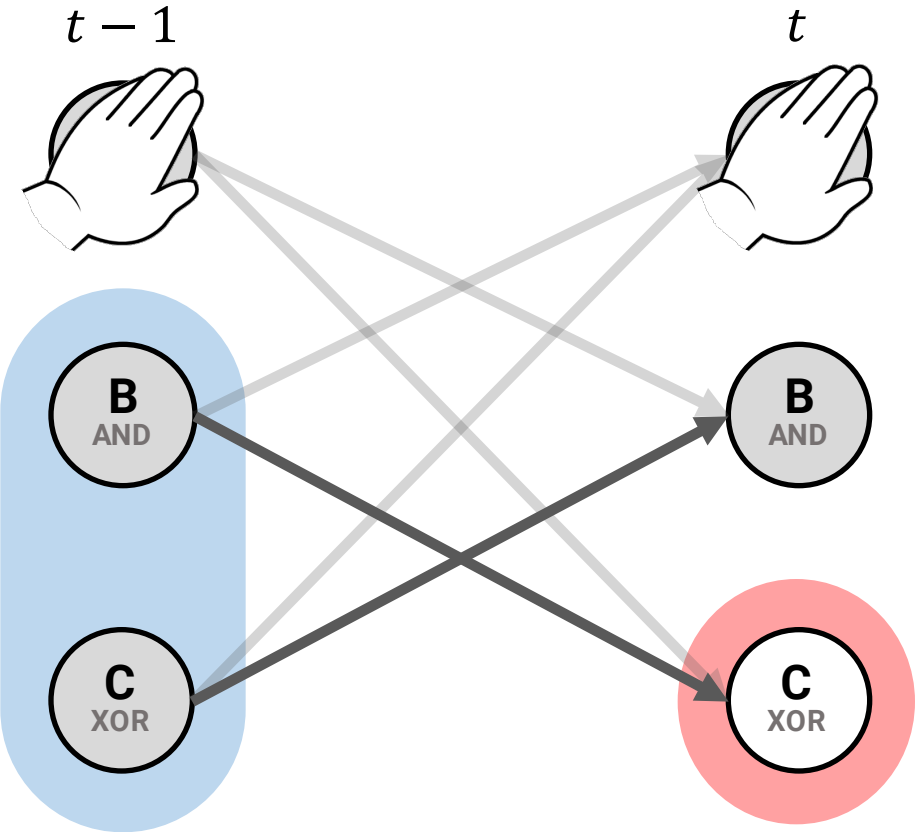

Now we marginalize over the current states of elements outside the mechanism (**A** and **B**)

|                |   |   | Current state |     |   |     |     |     |   |     |
|----------------|---|---|---------------|-----|---|-----|-----|-----|---|-----|
| Previous state |   |   | A             |     |   |     |     |     |   |     |
|                |   |   | B             |     |   |     |     |     |   |     |
|                |   |   | C             |     |   |     |     |     |   |     |
|                | B | C |               |     |   |     |     |     |   |     |
|                |   |   |               |     |   |     |     |     |   |     |
|                | ○ | ○ | 1/2           | 0   | 0 | 0   | 1/2 | 0   | 0 | 0   |
|                | ● | ○ | 0             | 1/2 | 0 | 0   | 0   | 1/2 | 0 | 0   |
|                | ○ | ● | 0             | 1/2 | 0 | 0   | 0   | 0   | 0 | 1/2 |
|                | ● | ● | 0             | 0   | 0 | 1/2 | 0   | 1/2 | 0 | 0   |



## Calculating a cause repertoire:

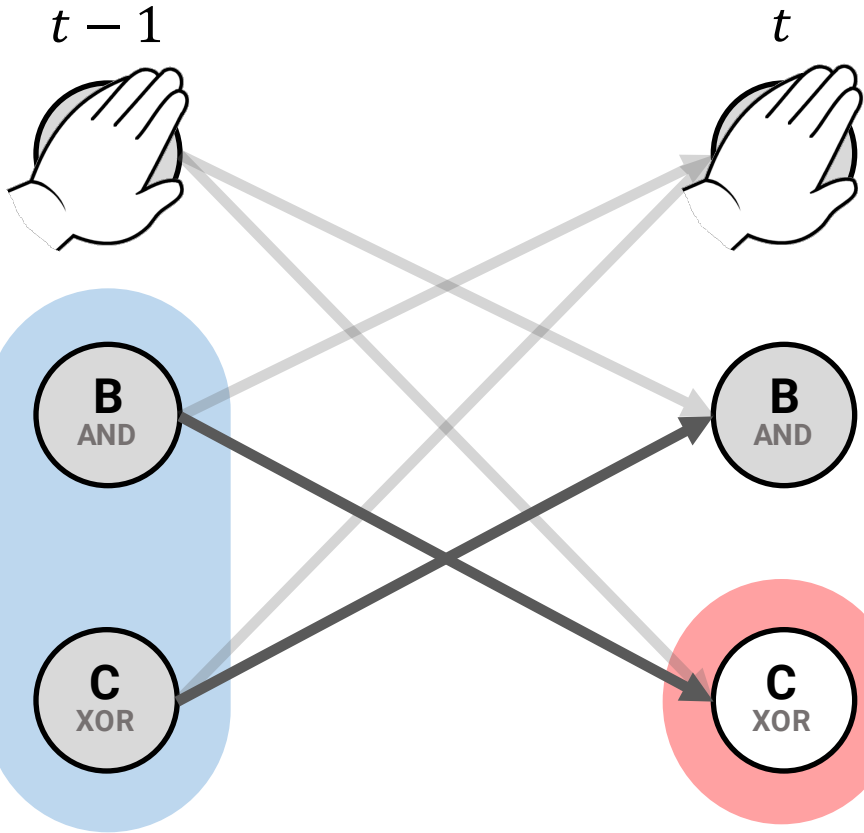

Now we marginalize over the current states of elements outside the mechanism (**A** and **B**)

|                |                                                                                      | Current state                                                                        |               |               |               |
|----------------|--------------------------------------------------------------------------------------|--------------------------------------------------------------------------------------|---------------|---------------|---------------|
|                |                                                                                      | B                                                                                    | C             | B             | C             |
| Previous state | B                                                                                    | C                                                                                    |               |               |               |
|                | 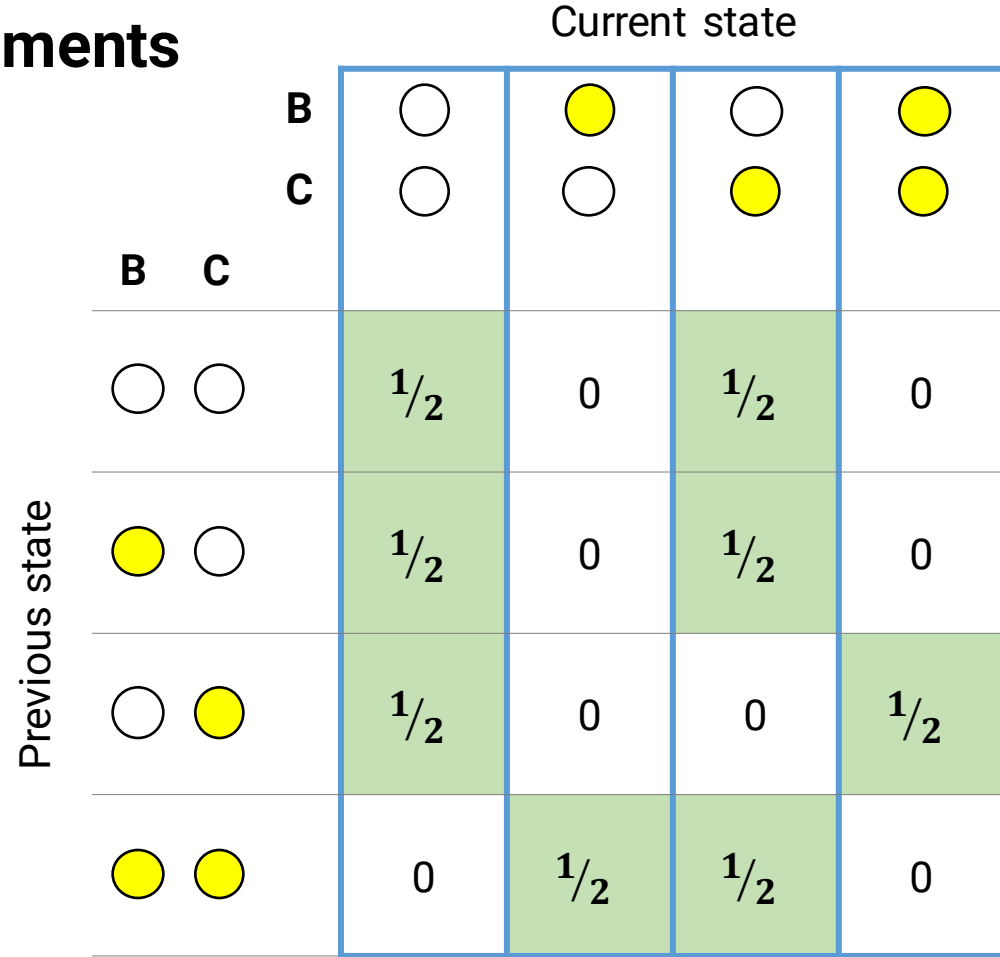  | 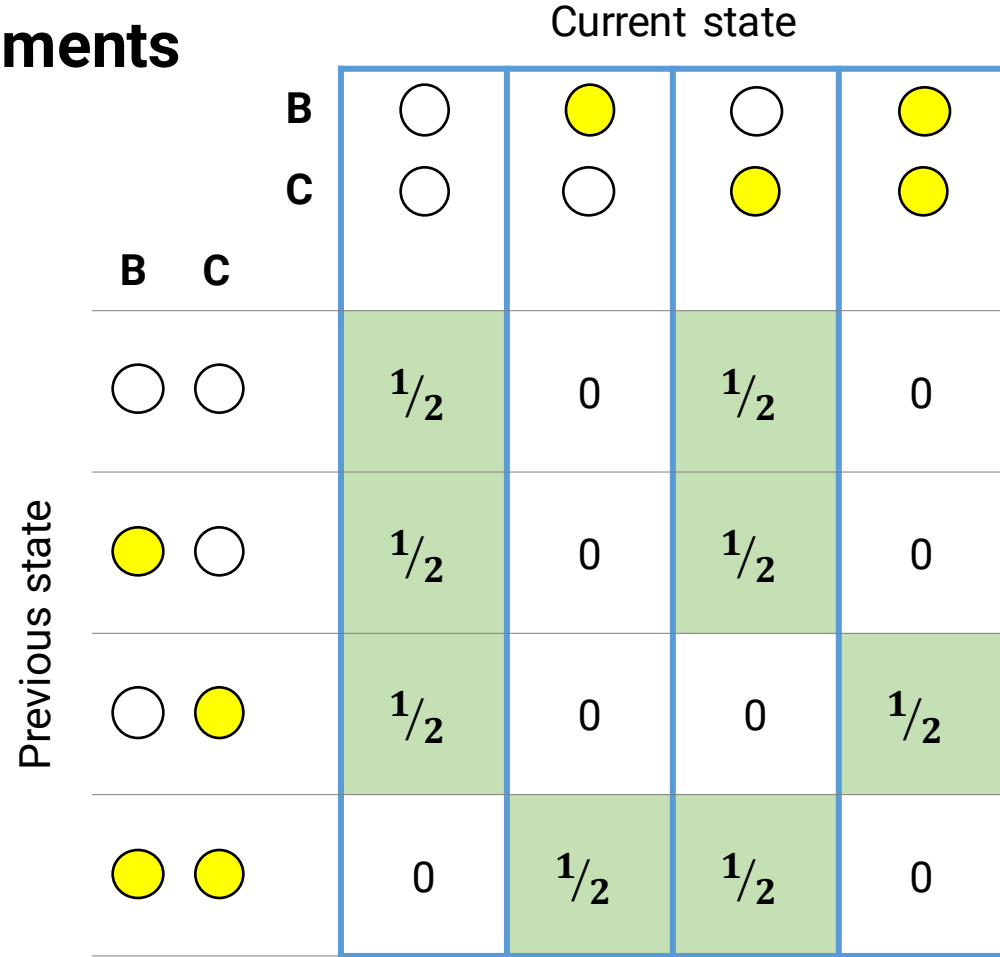  | $\frac{1}{2}$ | 0             | $\frac{1}{2}$ |
|                | 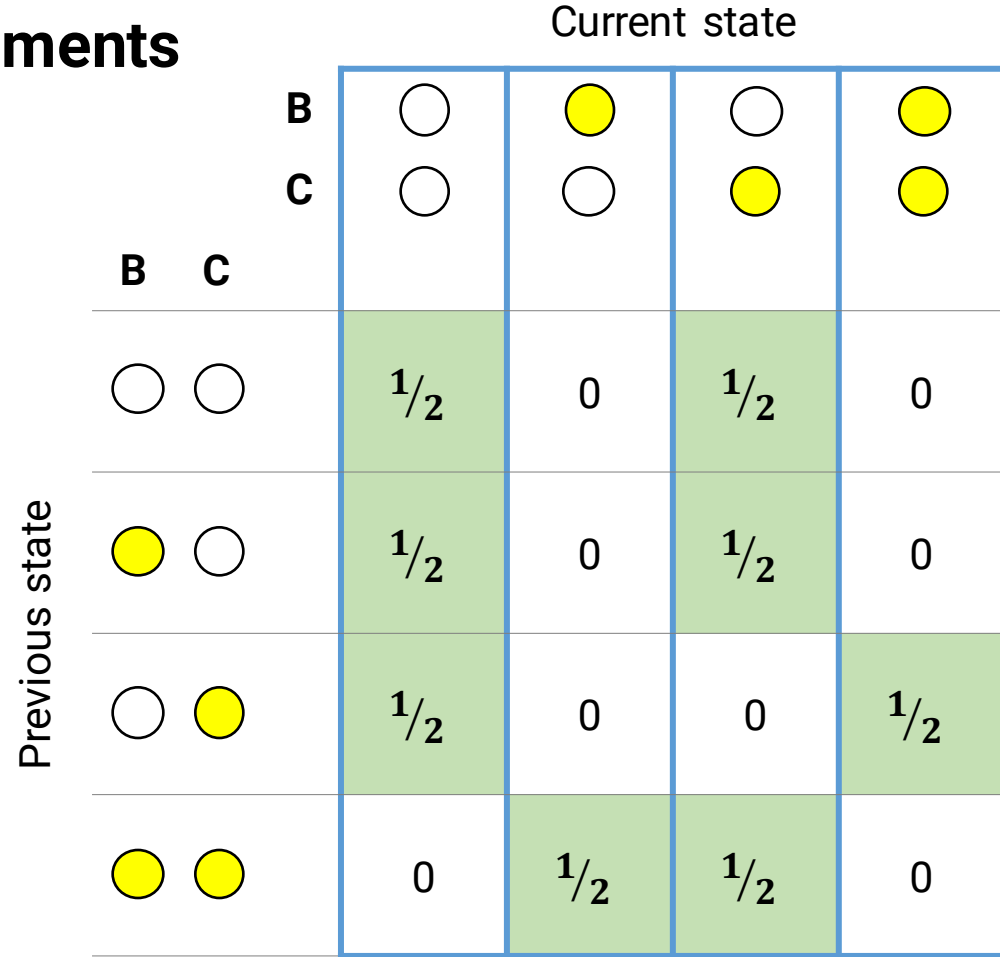  | 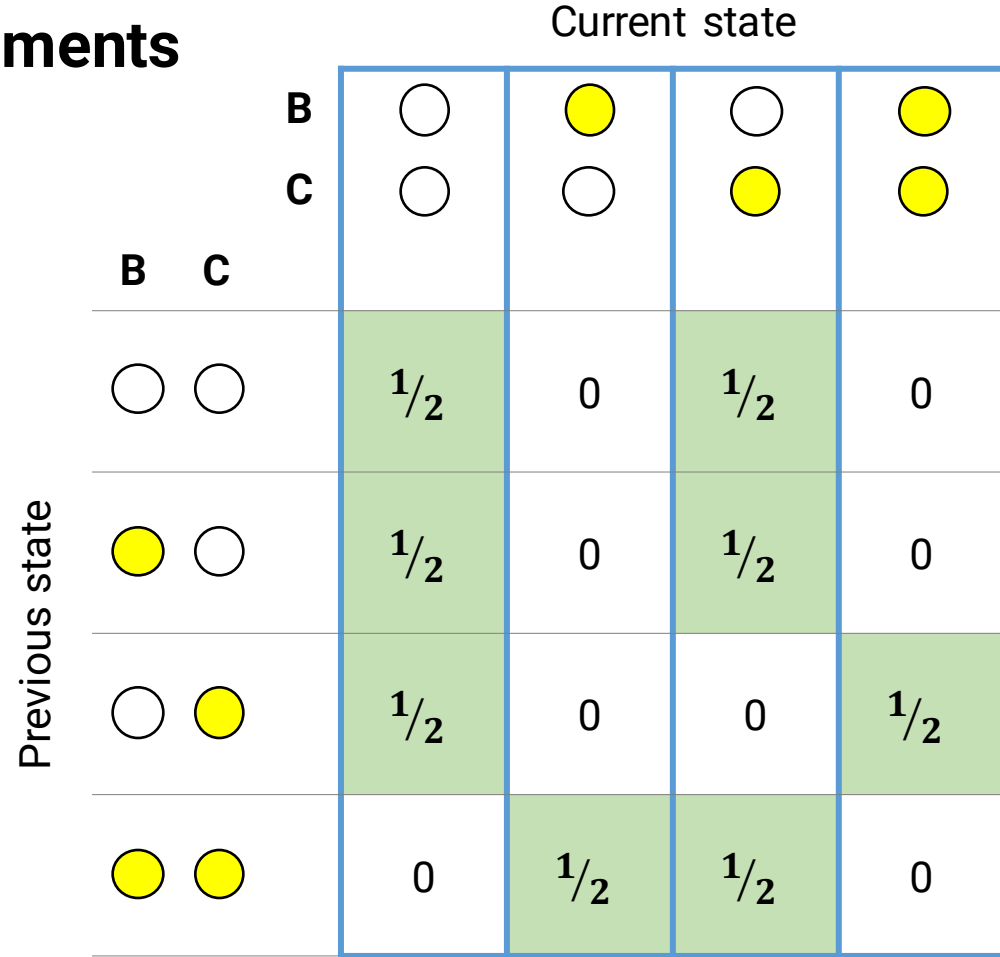  | $\frac{1}{2}$ | 0             | $\frac{1}{2}$ |
|                | 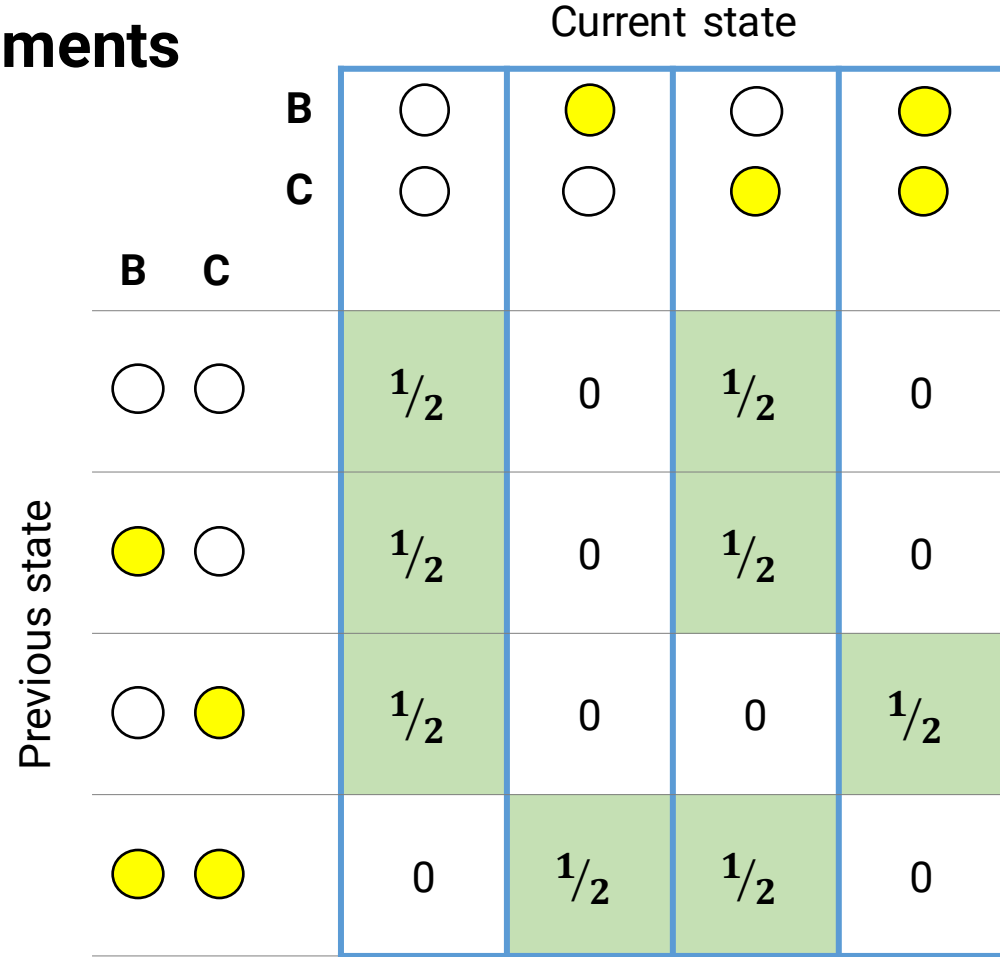  | 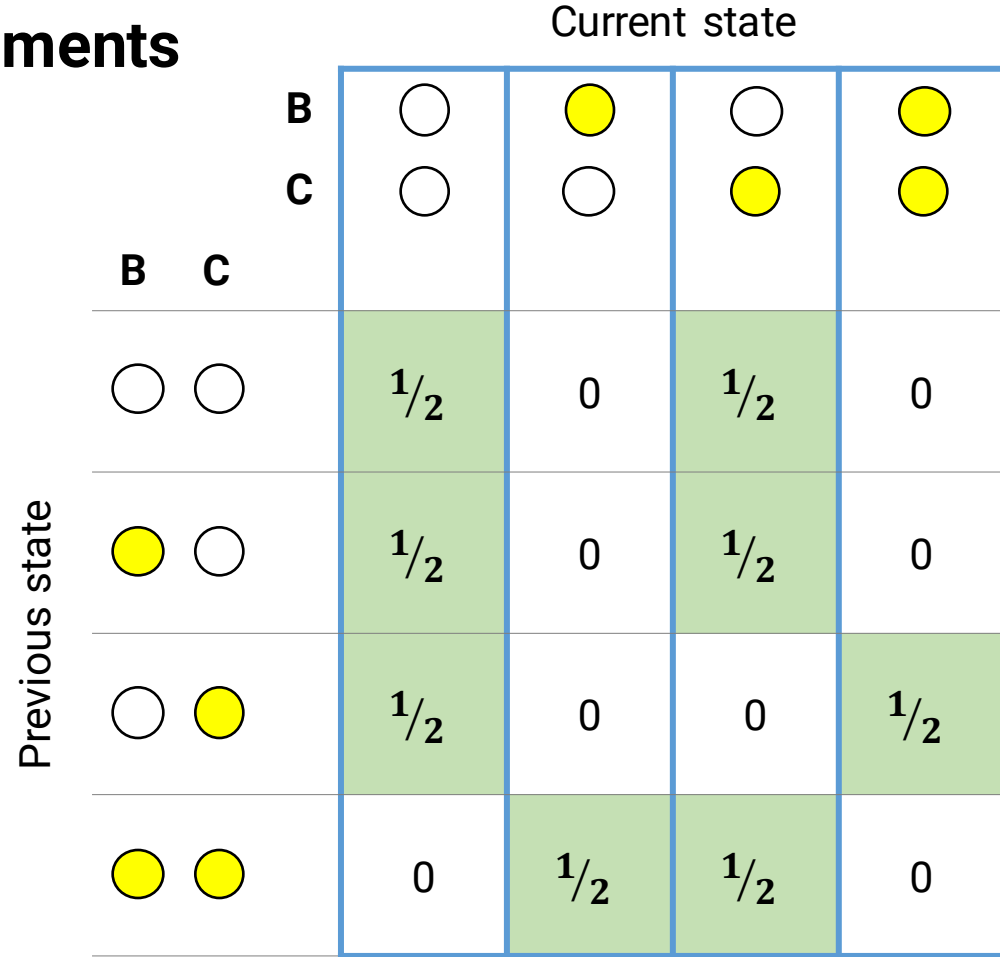  | $\frac{1}{2}$ | 0             | $\frac{1}{2}$ |
|                | 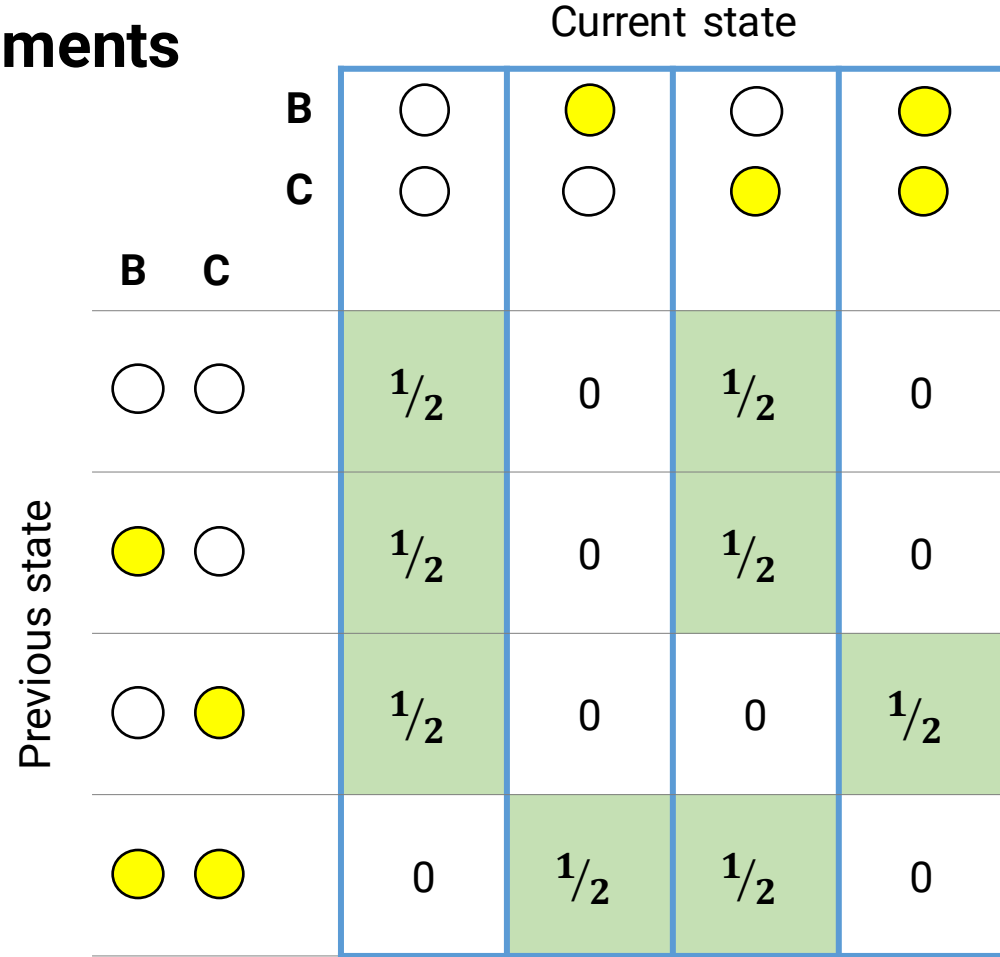 | 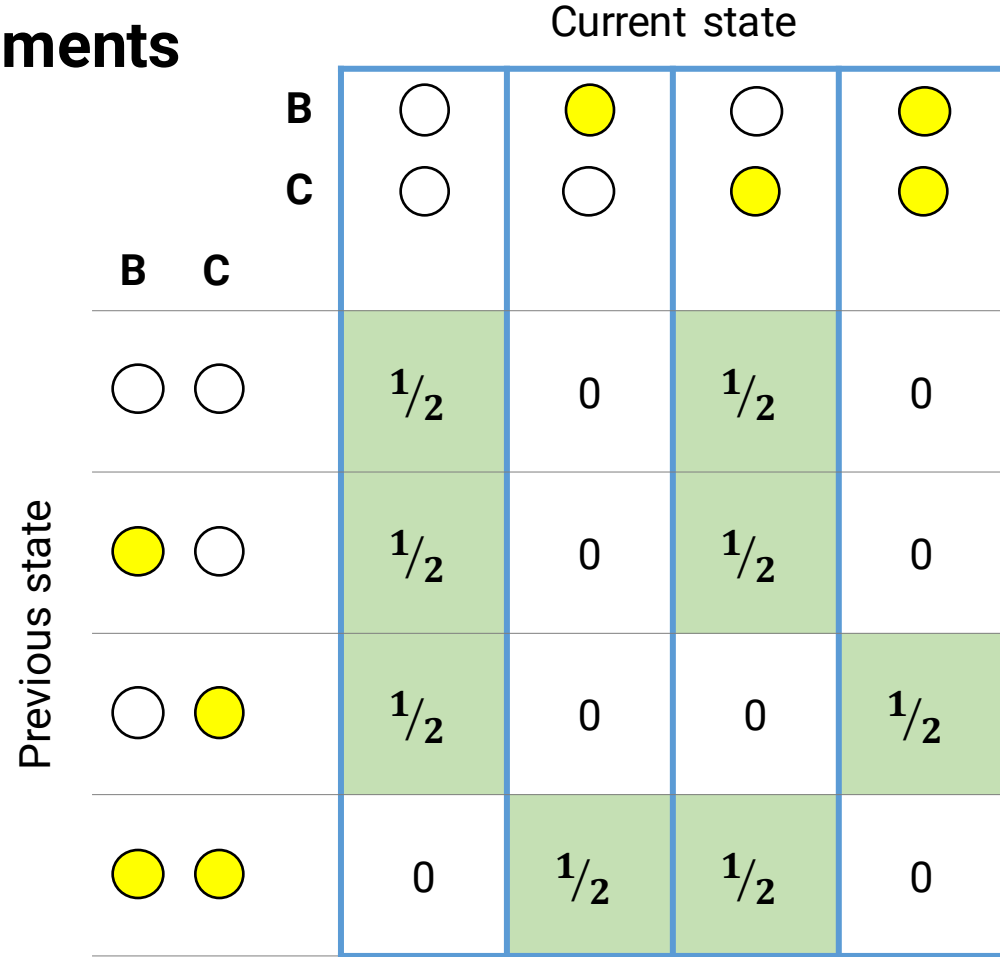 | 0             | $\frac{1}{2}$ | $\frac{1}{2}$ |

## Calculating a cause repertoire:

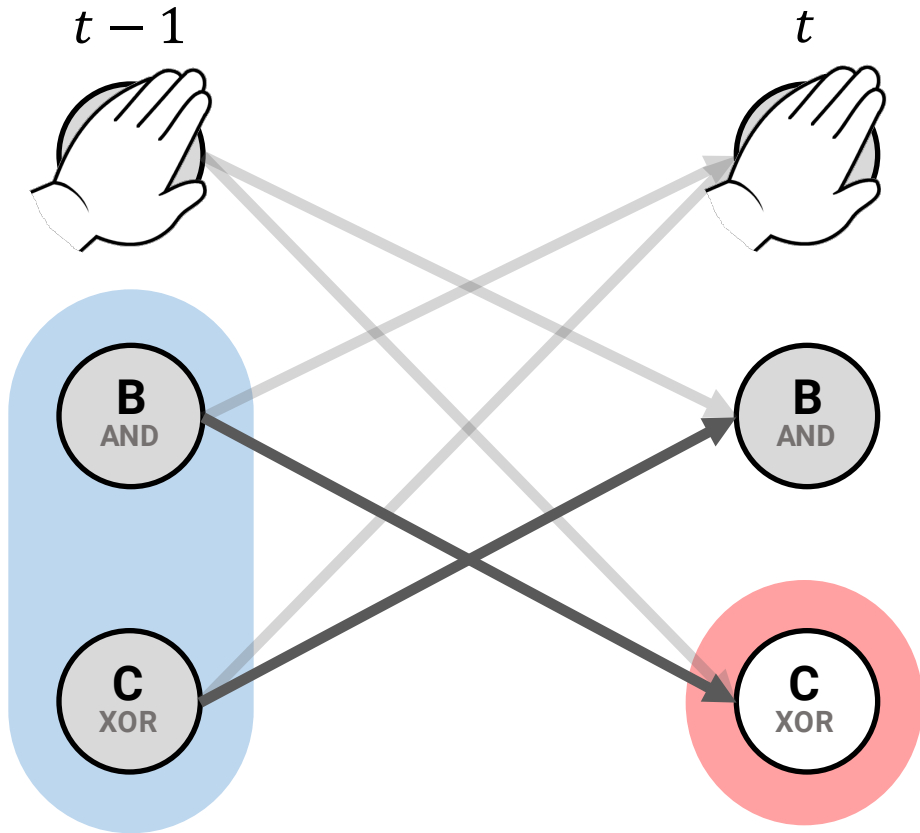

| Previous state                                                                       |                                                                                      |               | Current state  |                                                                                     |                                                                                     |                                                                                     |                                                                                     |
|--------------------------------------------------------------------------------------|--------------------------------------------------------------------------------------|---------------|----------------|-------------------------------------------------------------------------------------|-------------------------------------------------------------------------------------|-------------------------------------------------------------------------------------|-------------------------------------------------------------------------------------|
|                                                                                      |                                                                                      |               | Previous state |                                                                                     | Current state                                                                       |                                                                                     |                                                                                     |
|                                                                                      |                                                                                      | B             | C              | B                                                                                   | C                                                                                   | B                                                                                   | C                                                                                   |
|                                                                                      |                                                                                      |               |                | 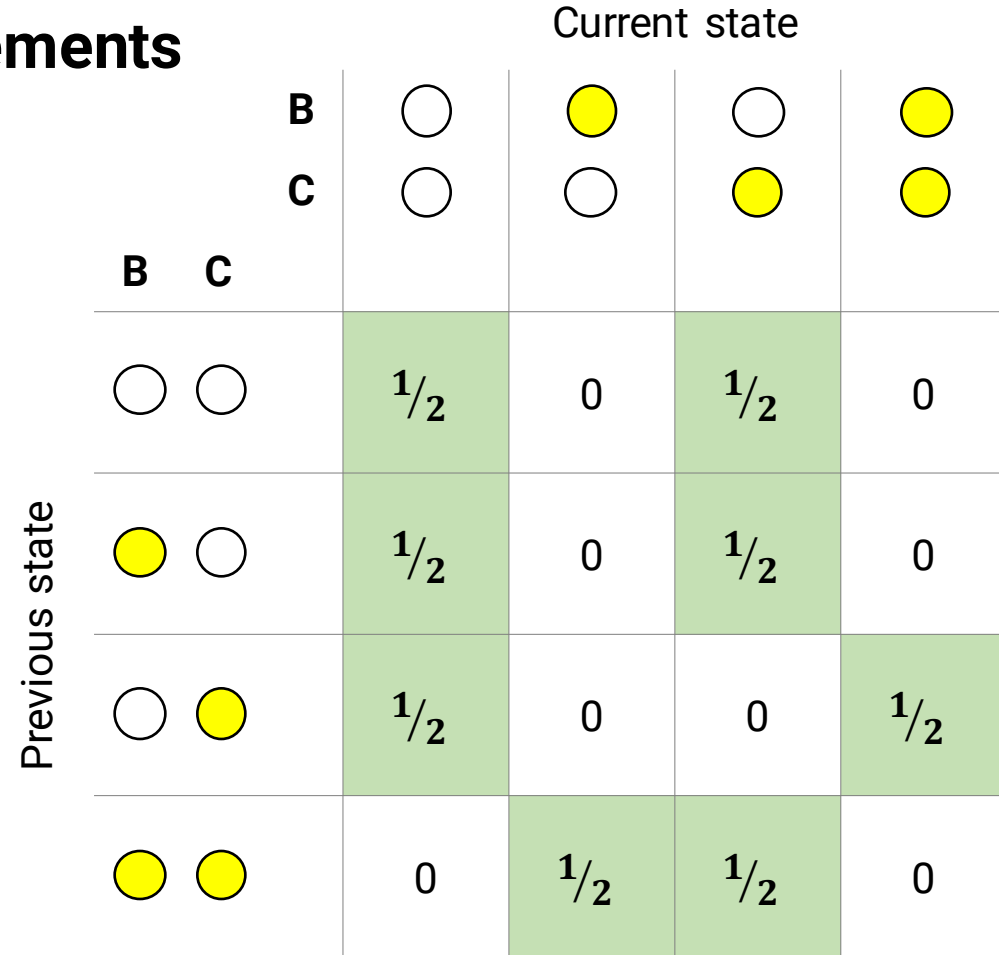 | 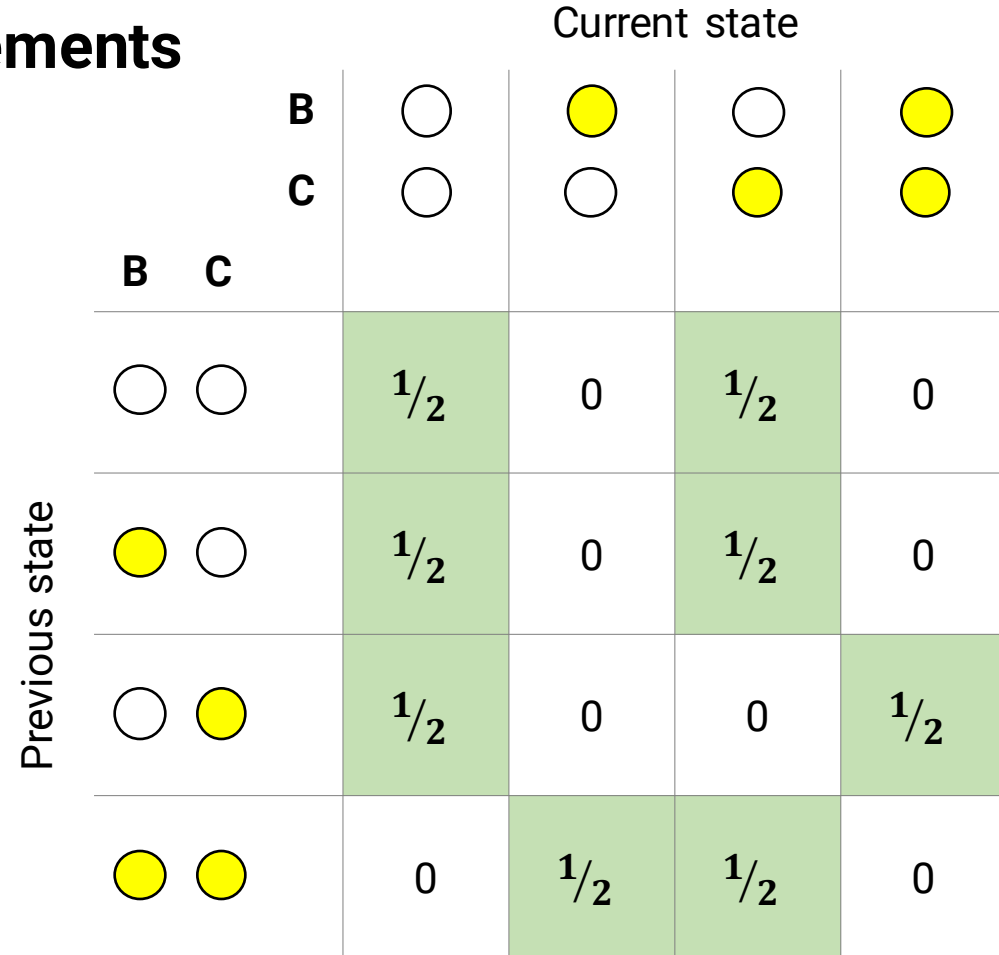 | 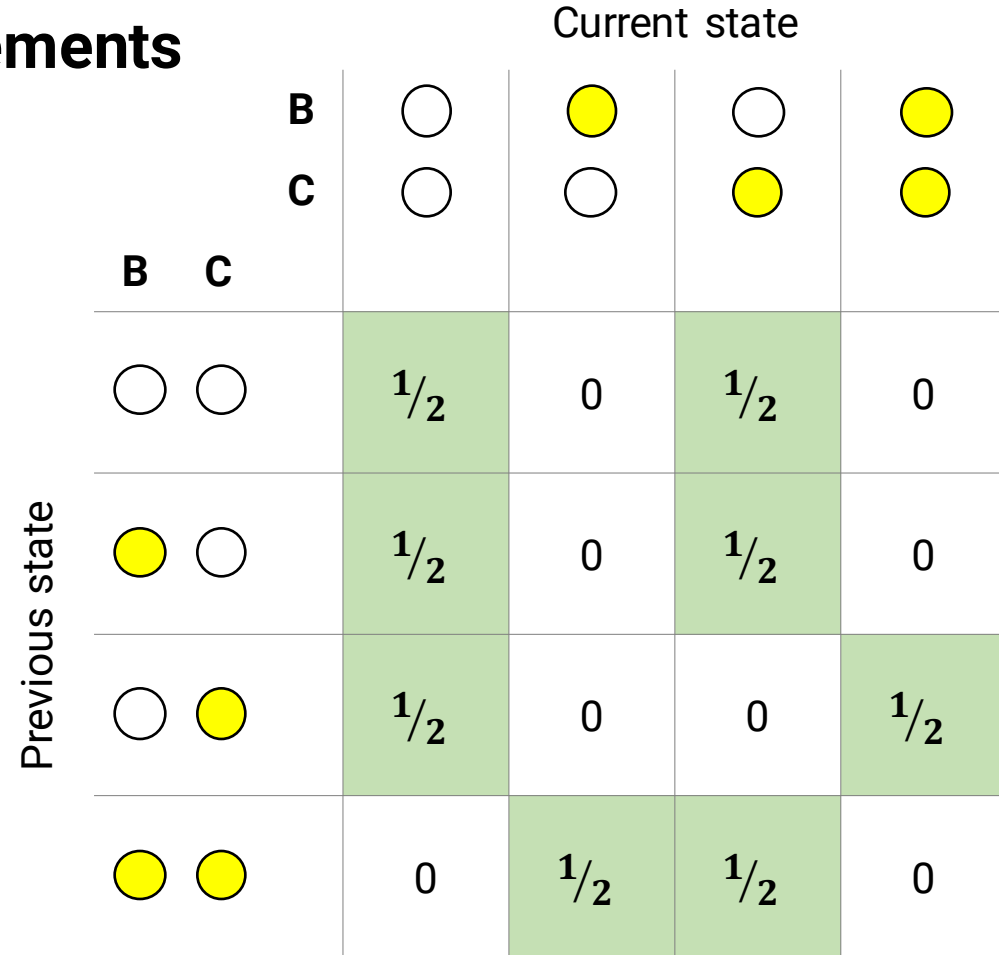 | 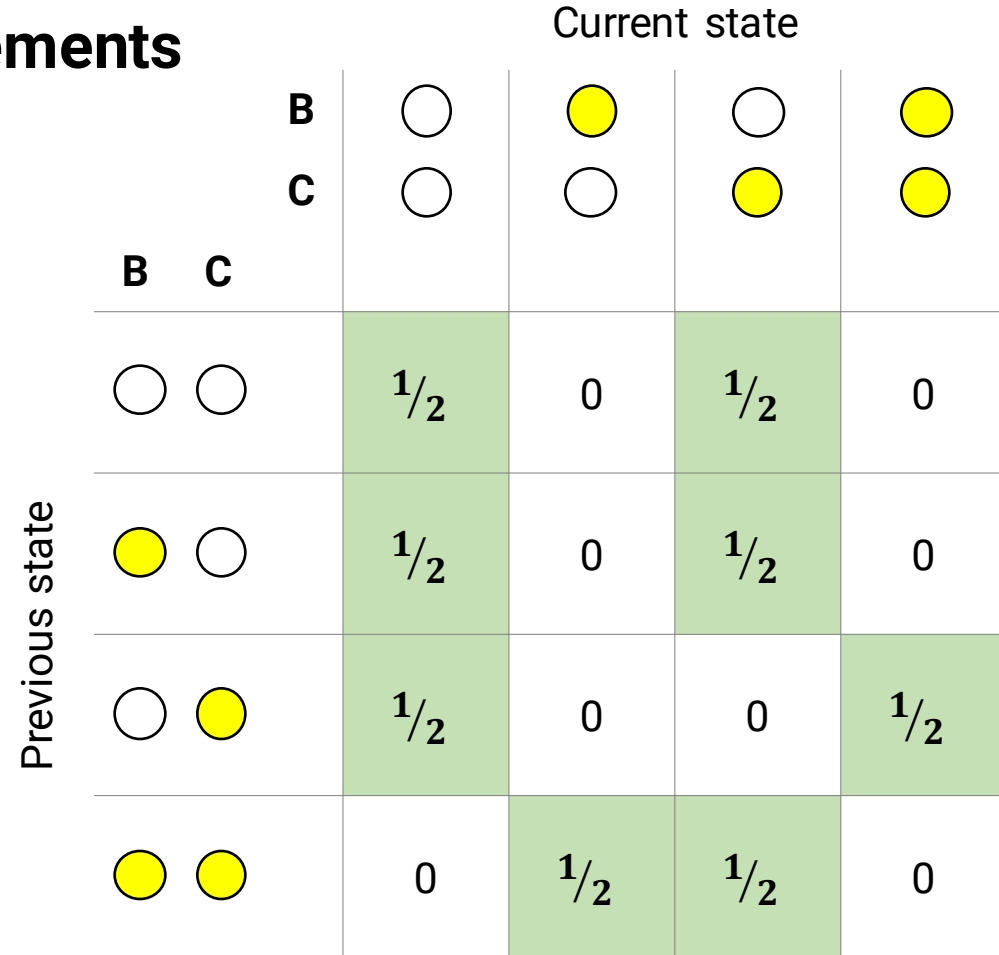 |
|                                                                                      |                                                                                      |               |                | 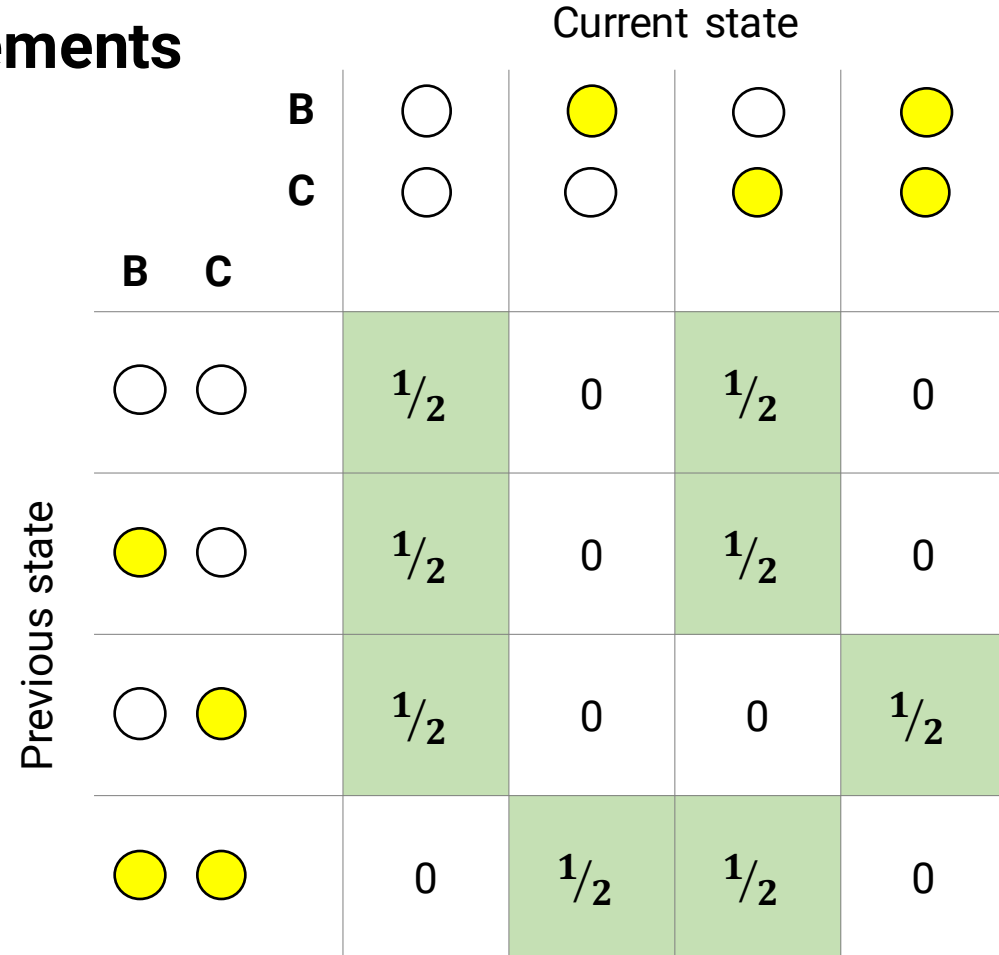 | 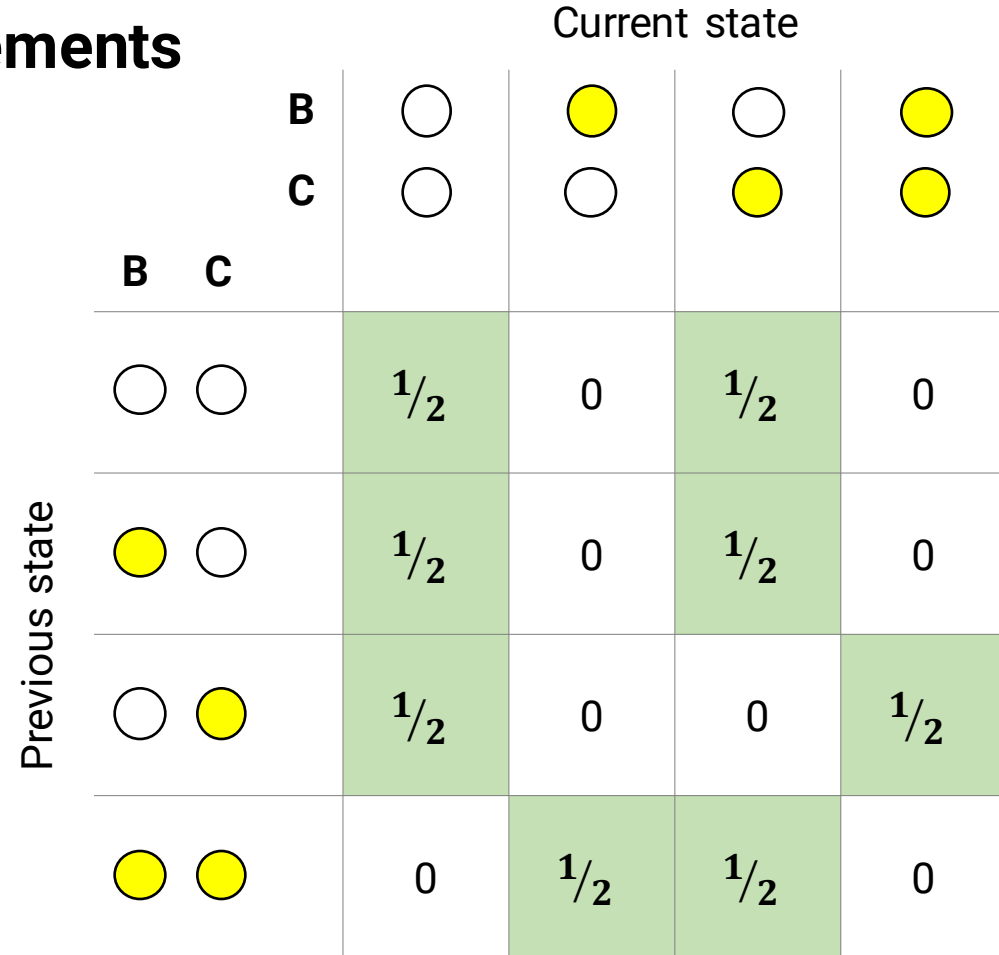 | 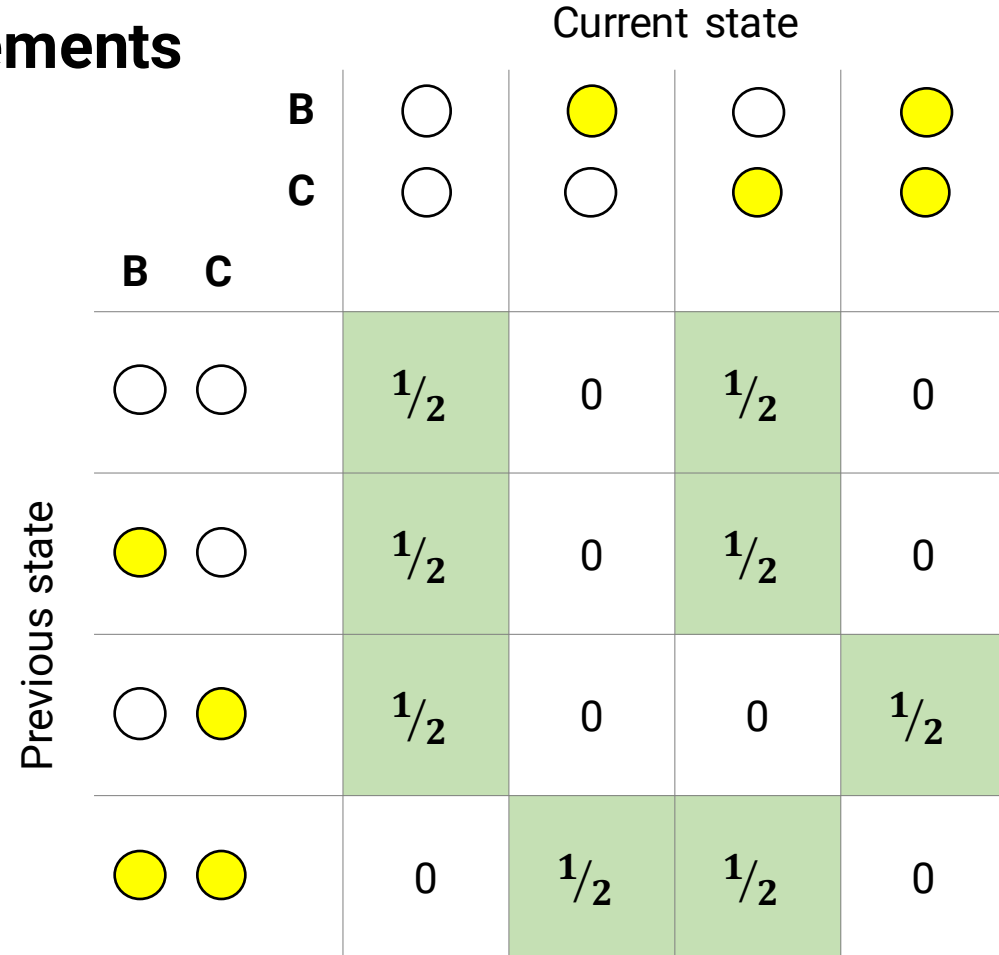 | 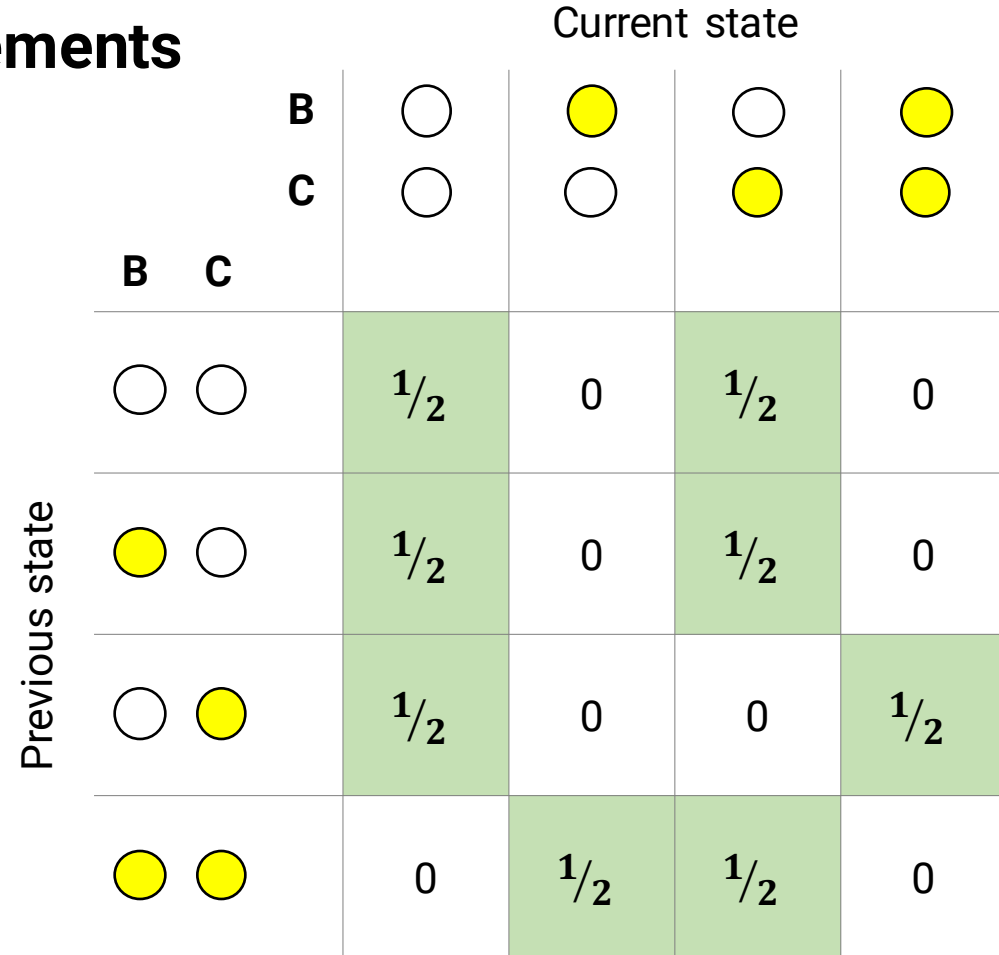 |
| 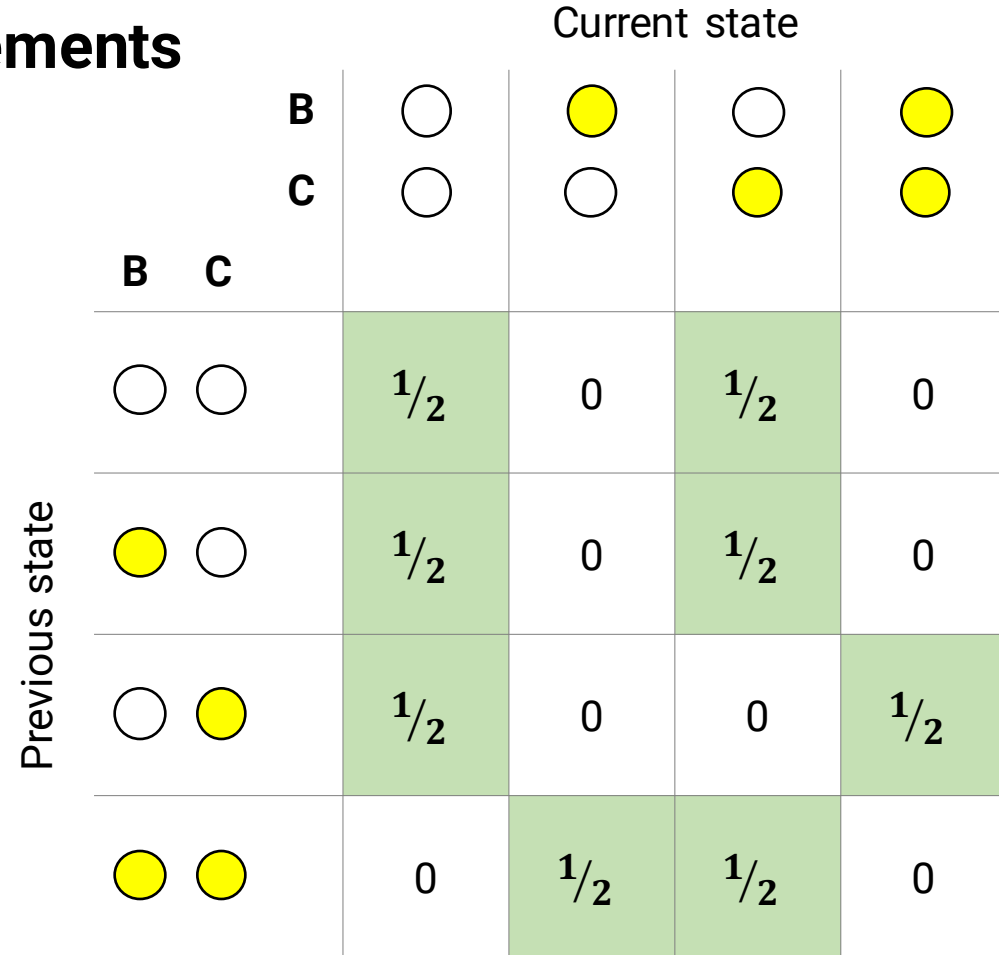  | 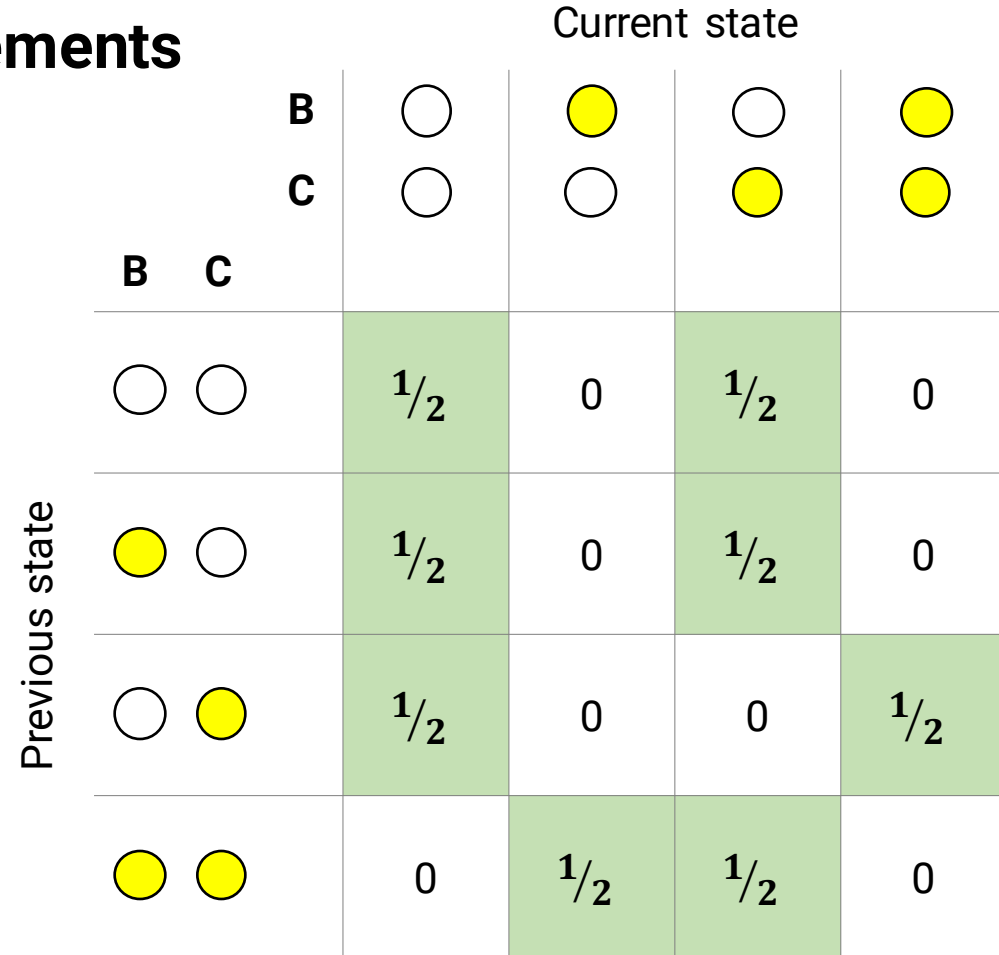  | $\frac{1}{2}$ | 0              | $\frac{1}{2}$                                                                       | 0                                                                                   |                                                                                     |                                                                                     |
| 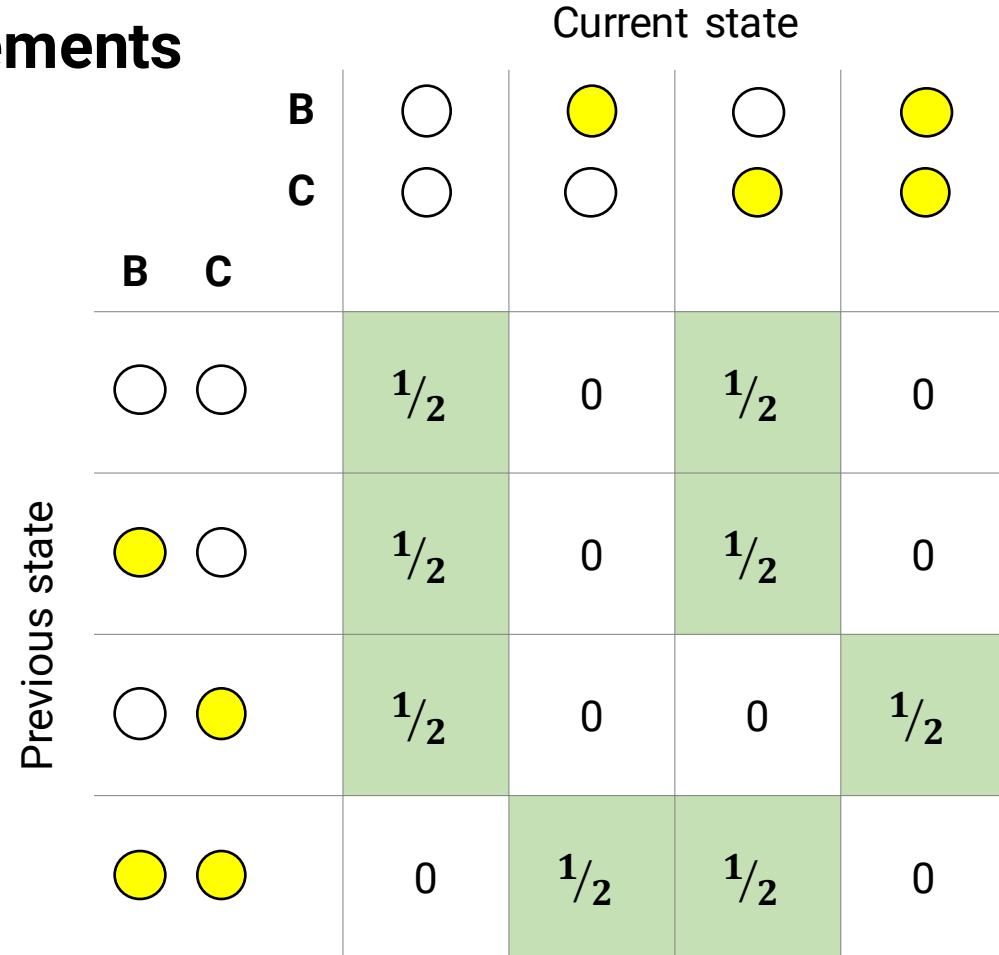  | 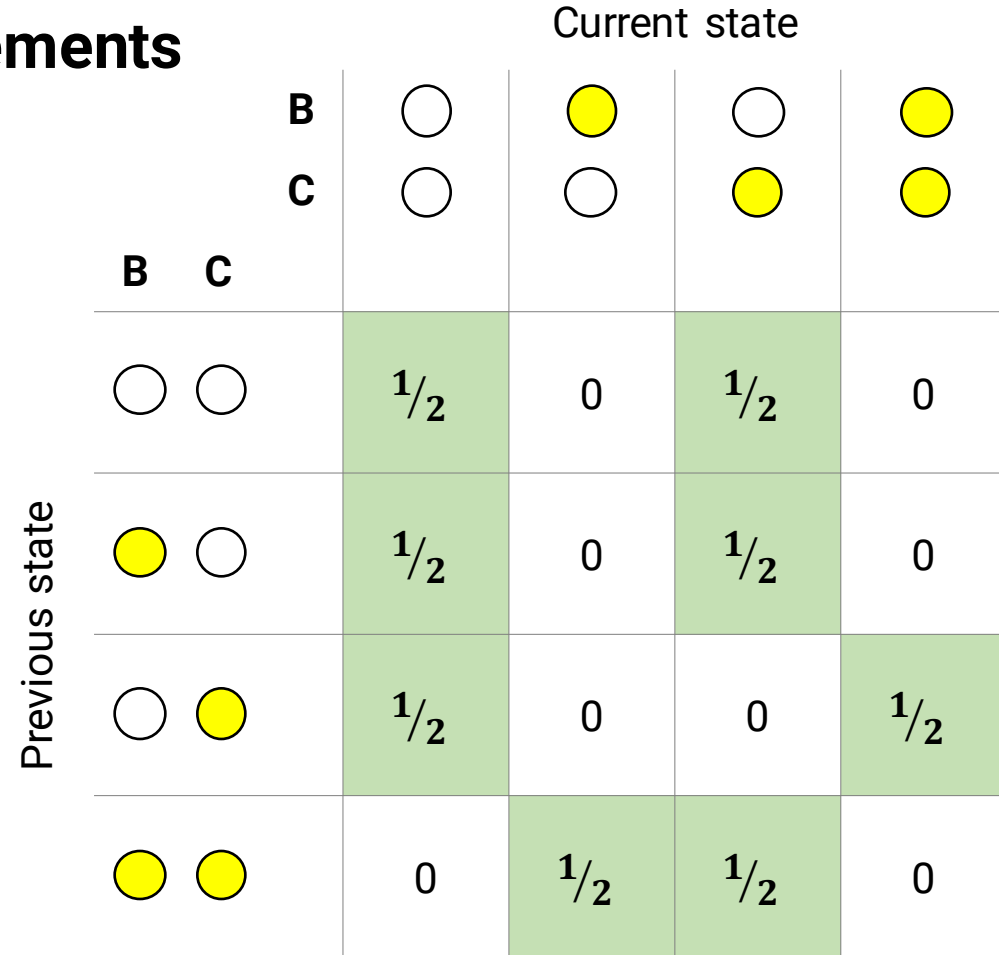  | $\frac{1}{2}$ | 0              | $\frac{1}{2}$                                                                       | 0                                                                                   |                                                                                     |                                                                                     |
| 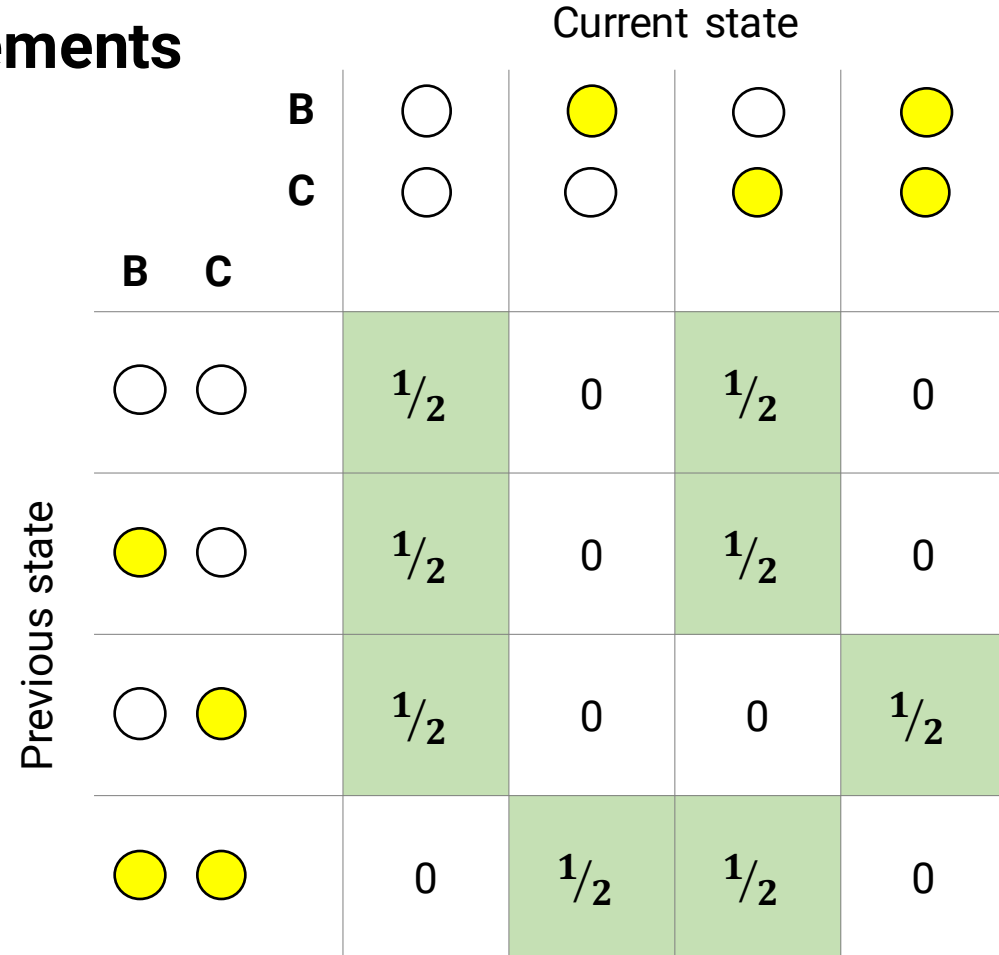  | 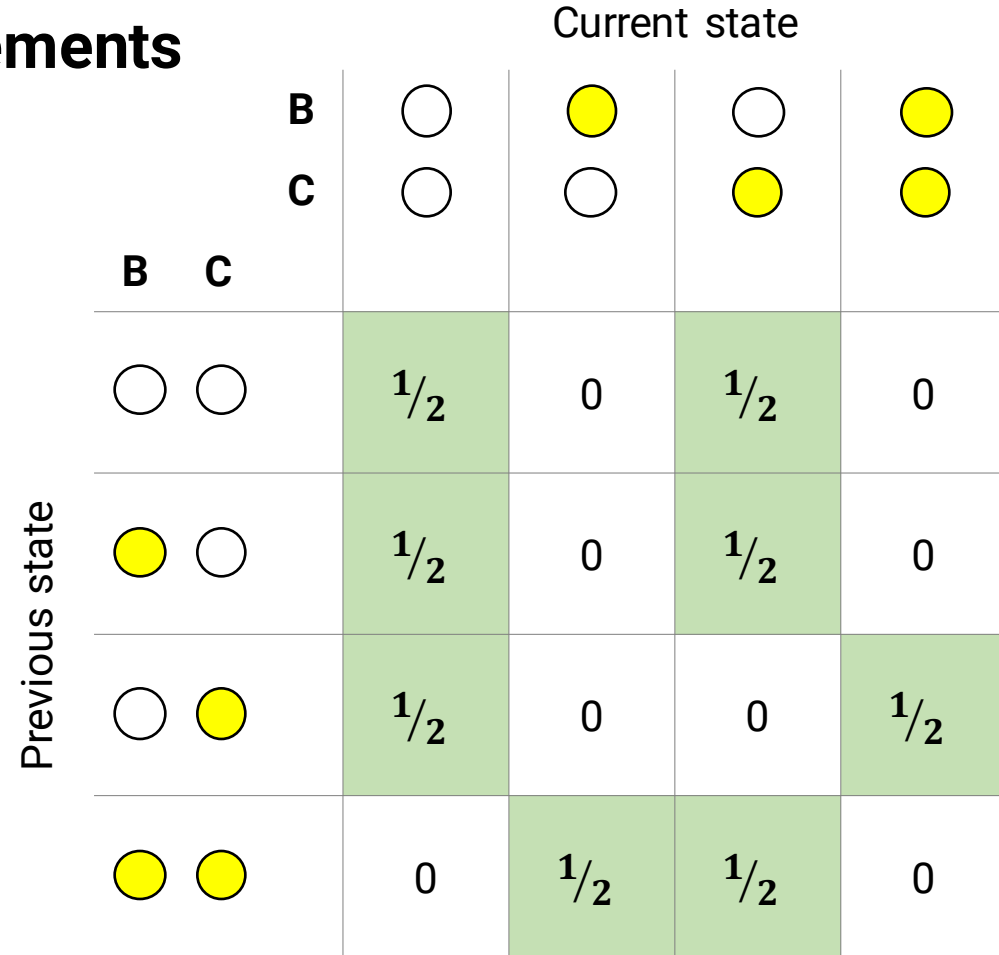  | $\frac{1}{2}$ | 0              | 0                                                                                   | $\frac{1}{2}$                                                                       |                                                                                     |                                                                                     |
| 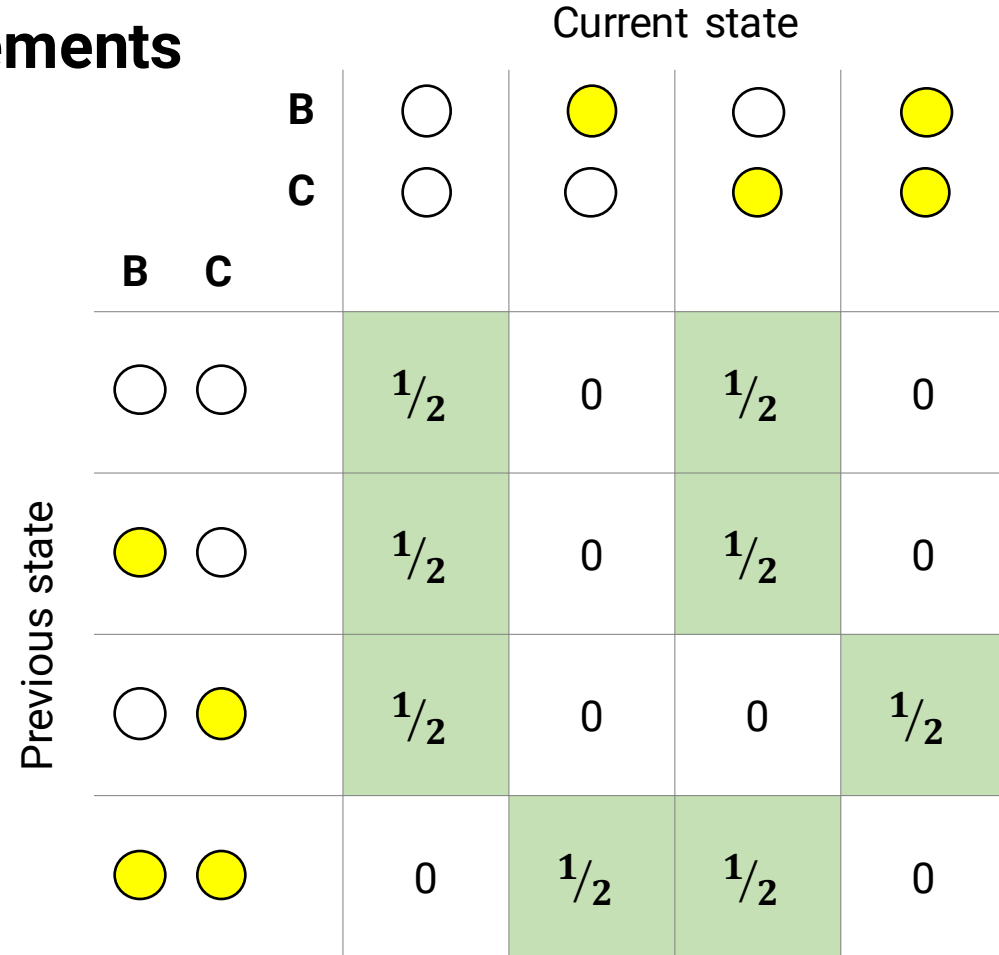 | 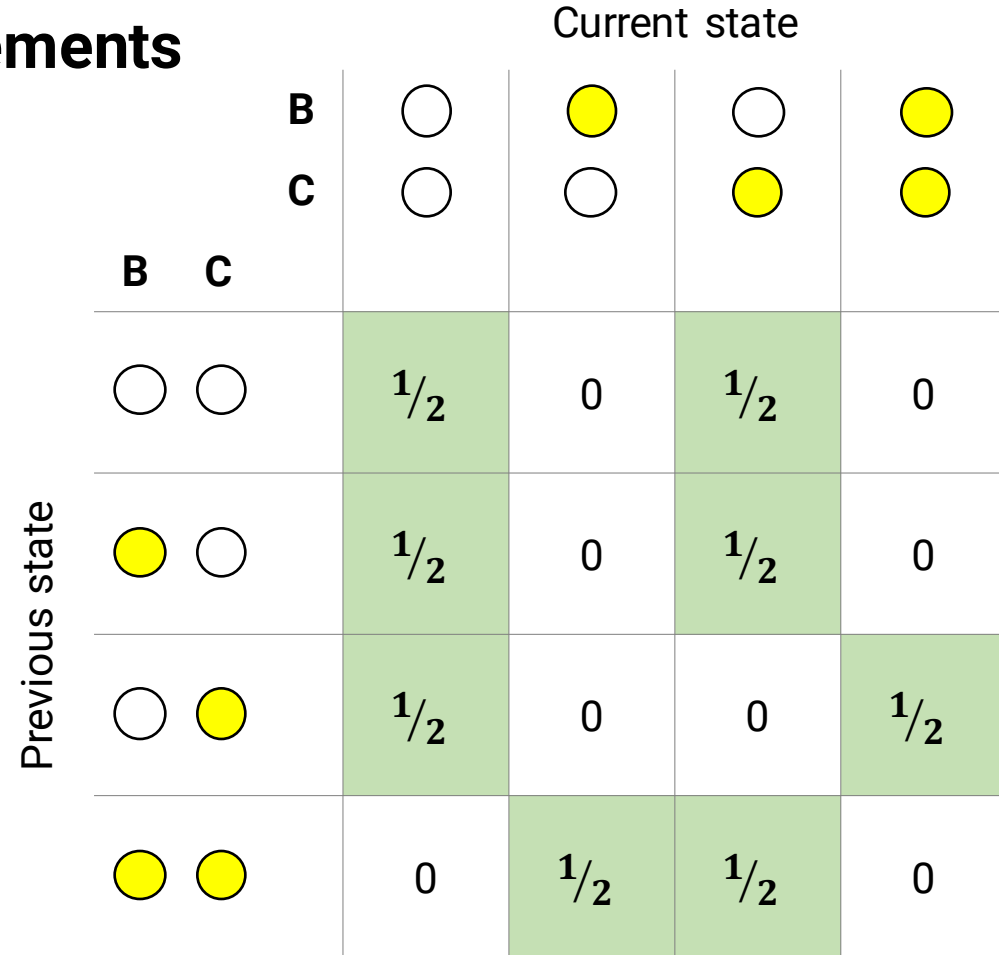 | 0             | $\frac{1}{2}$  | $\frac{1}{2}$                                                                       | 0                                                                                   |                                                                                     |                                                                                     |

Now we marginalize over the current states of elements outside the mechanism (**A** and **B**)

# Calculating a cause repertoire: Marginalizing-out non-mechanism elements

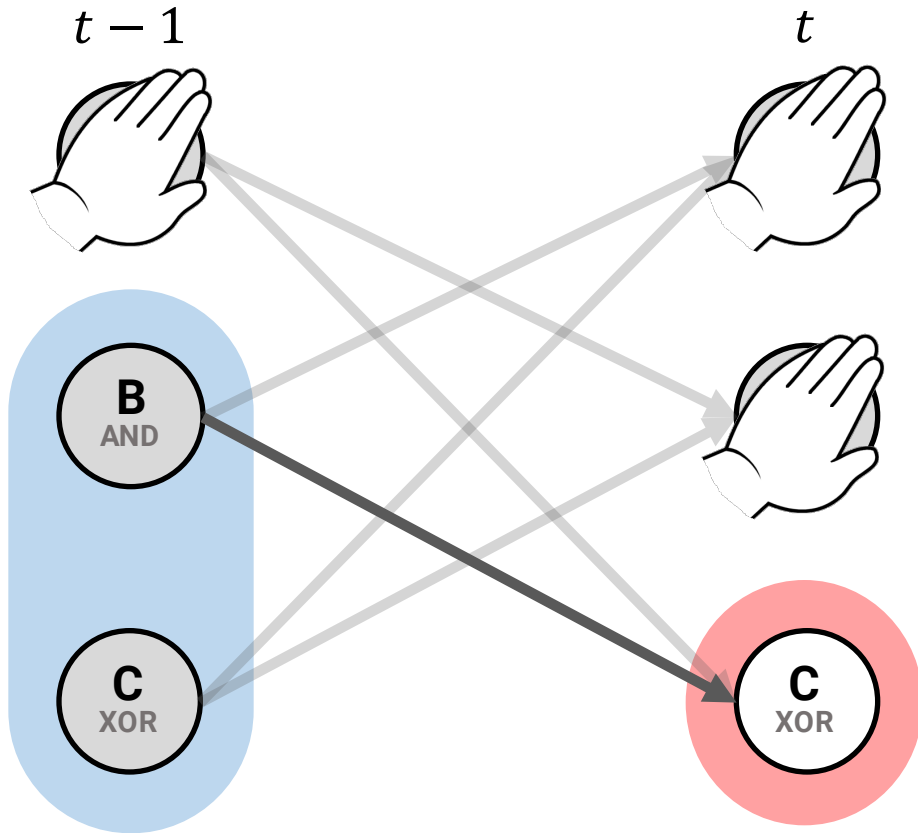

|                |   | Current state |               |               |               |
|----------------|---|---------------|---------------|---------------|---------------|
| Previous state | B | C             | B             | C             |               |
|                | B | C             |               |               |               |
|                | ○ | ○             | $\frac{1}{2}$ | 0             | $\frac{1}{2}$ |
|                | ● | ○             | $\frac{1}{2}$ | 0             | $\frac{1}{2}$ |
|                | ○ | ●             | $\frac{1}{2}$ | 0             | $\frac{1}{2}$ |
|                | ● | ●             | 0             | $\frac{1}{2}$ | $\frac{1}{2}$ |

Now we marginalize over the current states of elements outside the mechanism (**A** and **B**)





# Calculating a cause repertoire: Marginalizing-out non-mechanism elements

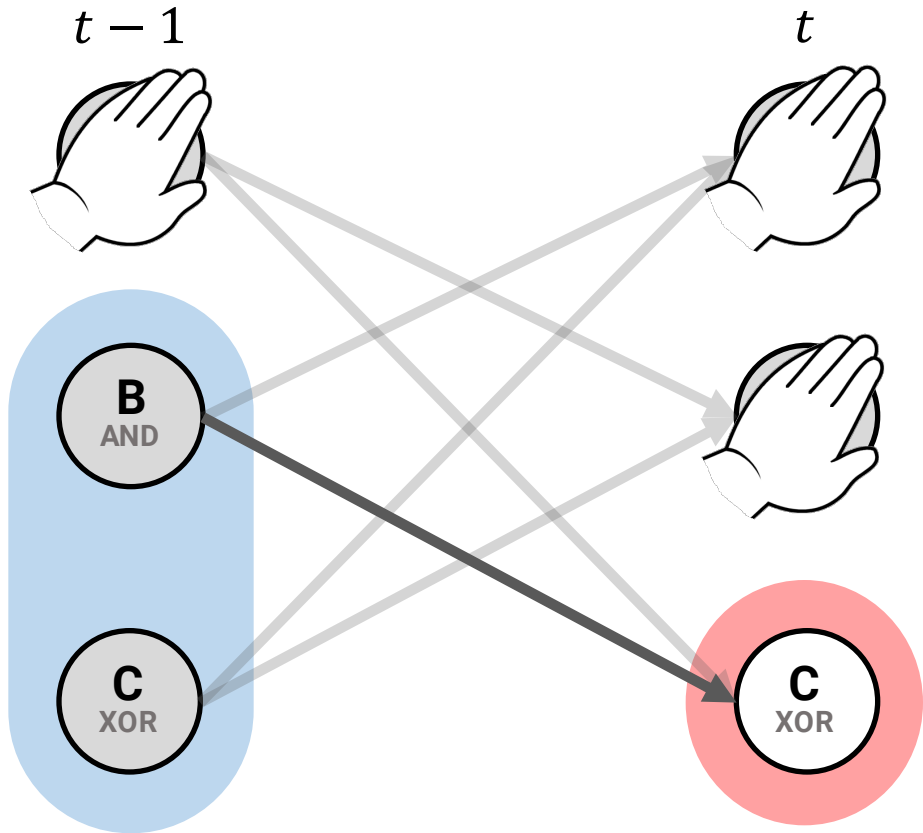

|                |                                                                                      |                                                                                      | Current state |               |               |               |  |
|----------------|--------------------------------------------------------------------------------------|--------------------------------------------------------------------------------------|---------------|---------------|---------------|---------------|--|
| Previous state |                                                                                      |                                                                                      | C             |               |               |               |  |
|                | B                                                                                    | C                                                                                    |               |               |               |               |  |
|                | 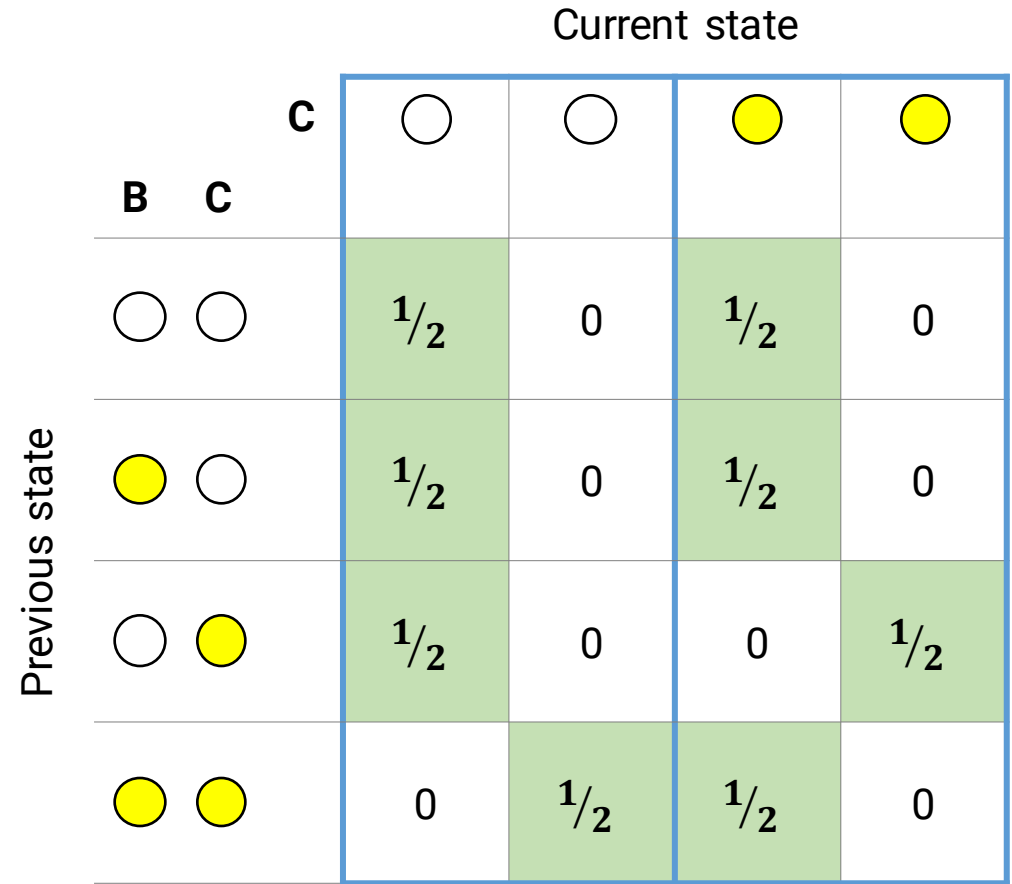  | 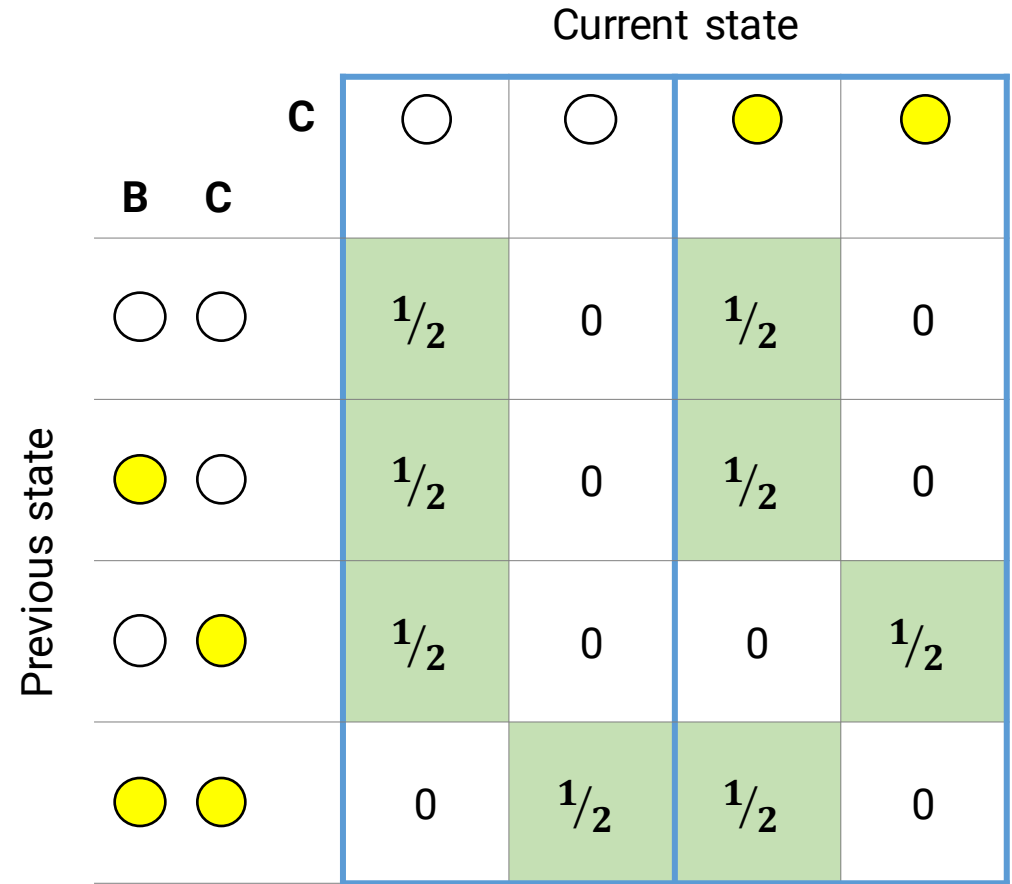  | $\frac{1}{2}$ | 0             | $\frac{1}{2}$ | 0             |  |
|                | 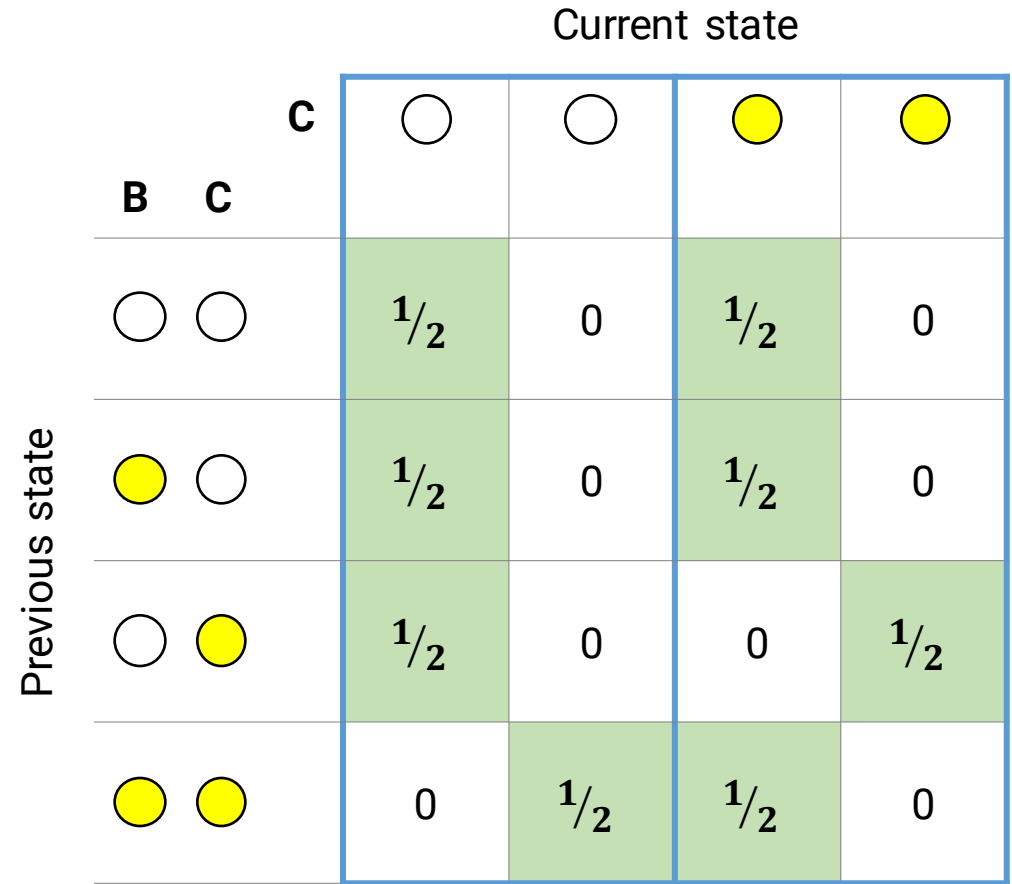  | 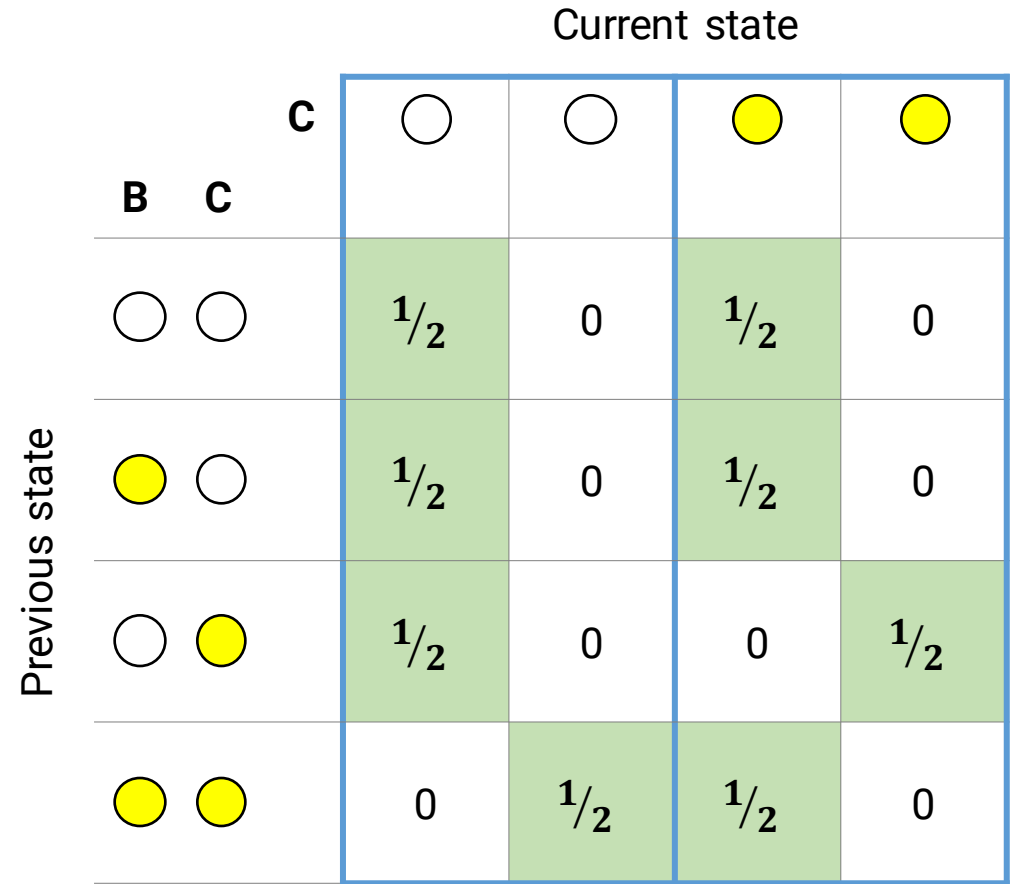  | $\frac{1}{2}$ | 0             | $\frac{1}{2}$ | 0             |  |
|                | 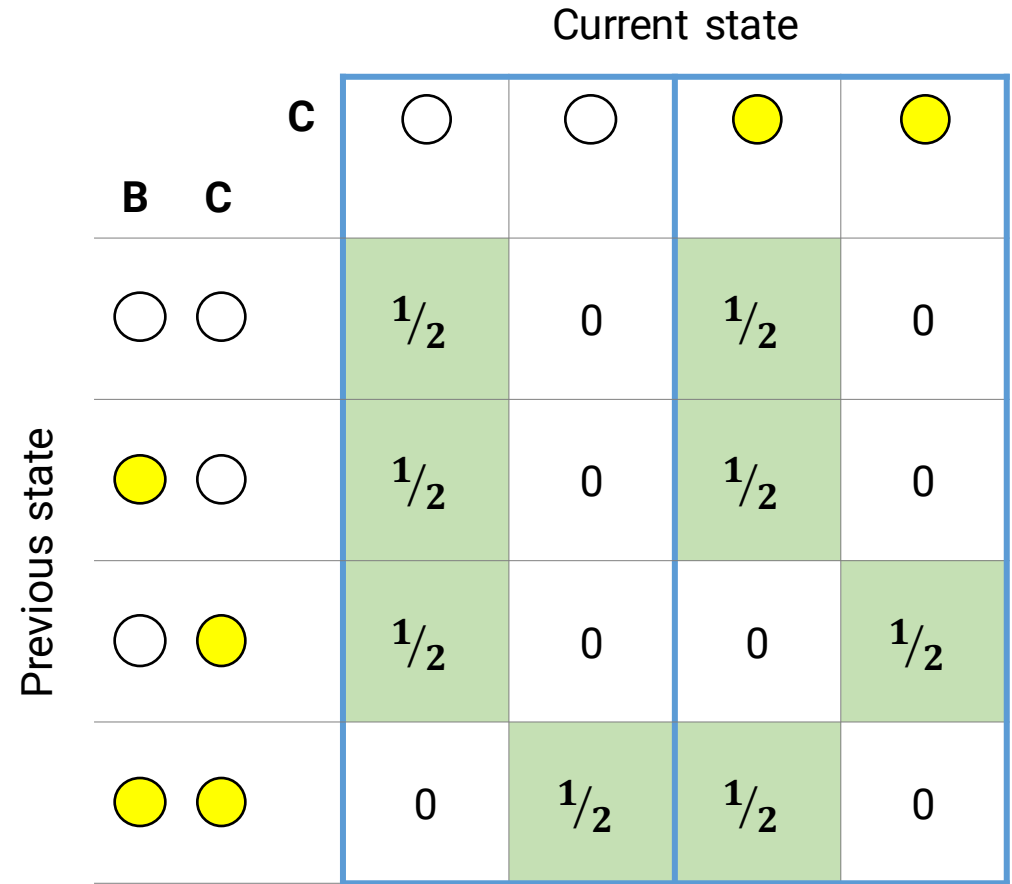  | 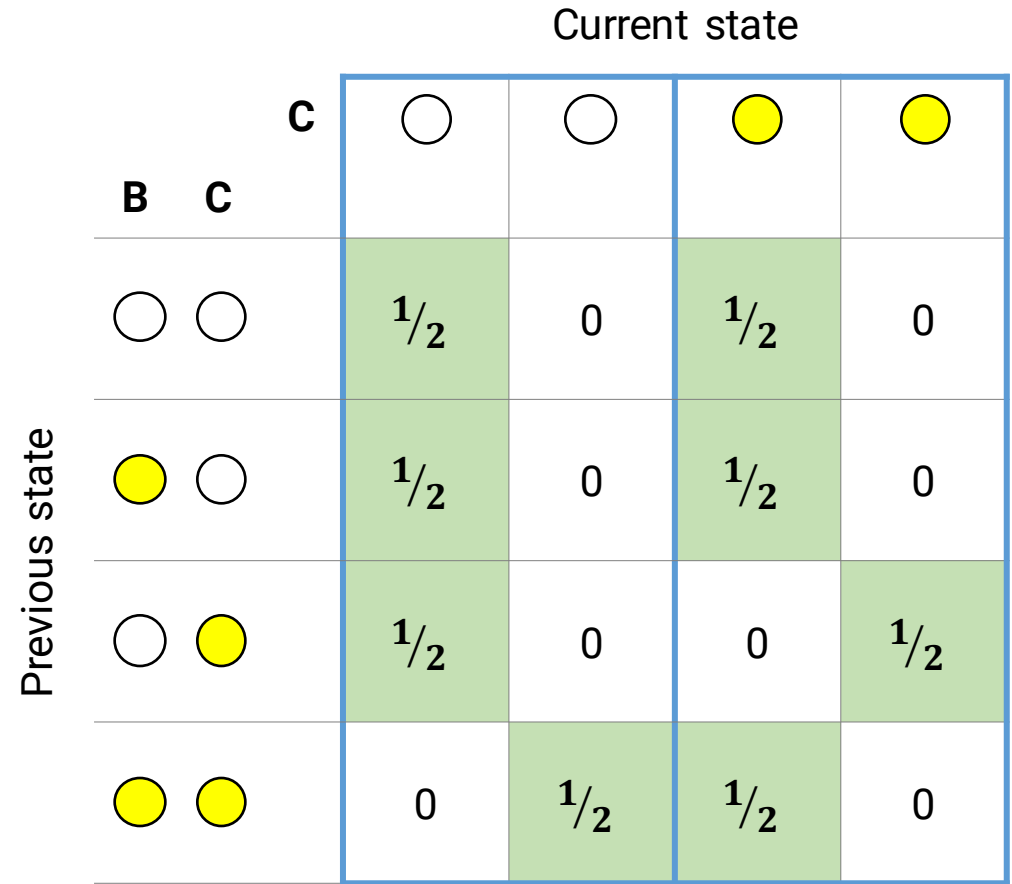  | $\frac{1}{2}$ | 0             | 0             | $\frac{1}{2}$ |  |
|                | 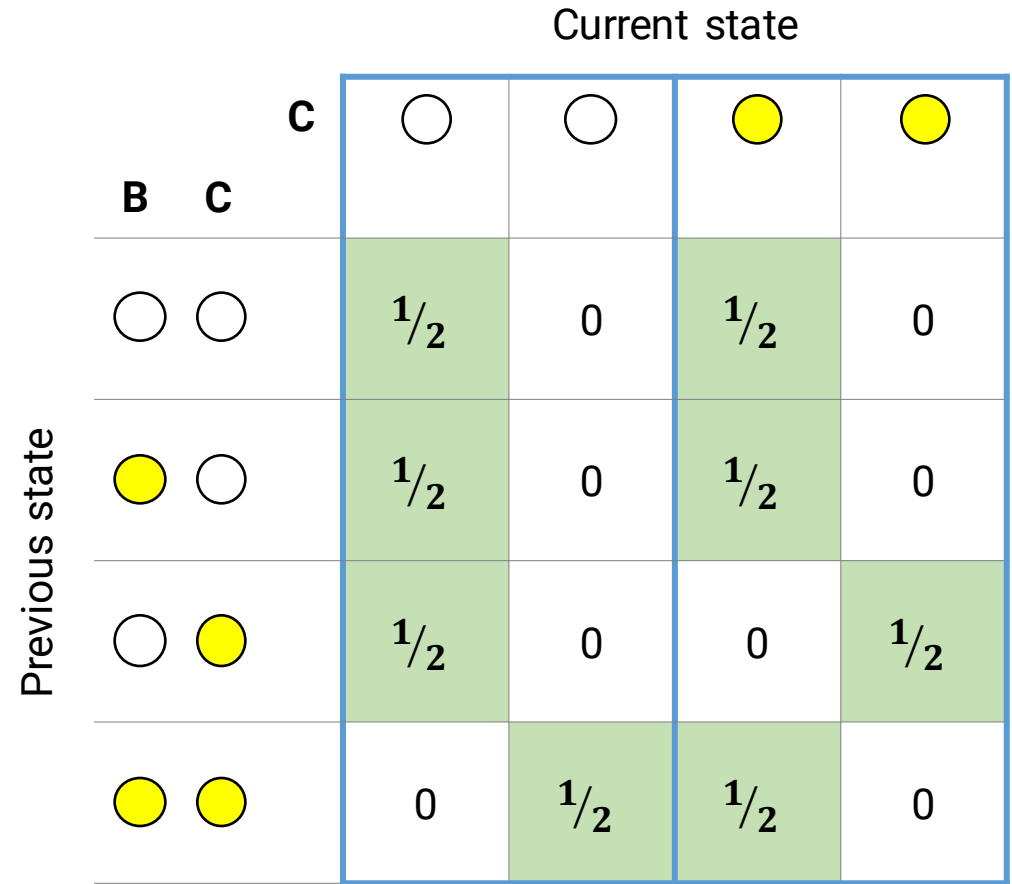 | 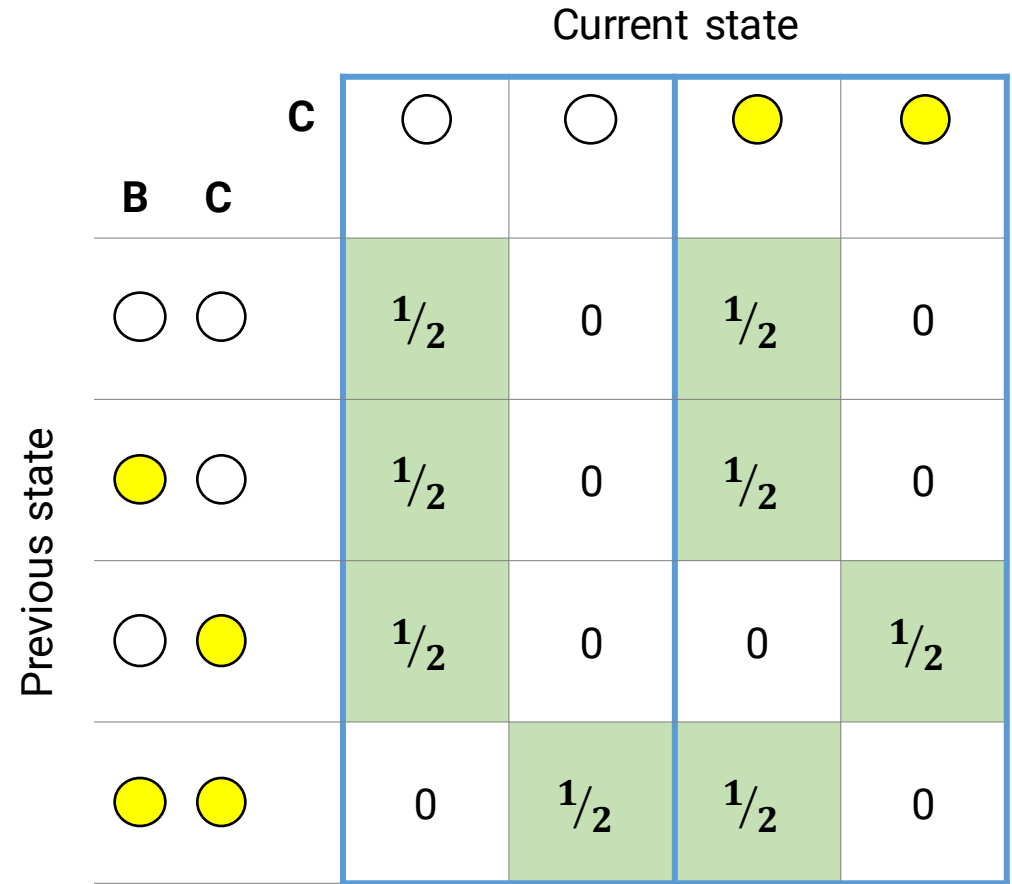 | 0             | $\frac{1}{2}$ | $\frac{1}{2}$ | 0             |  |

Now we marginalize over the current states of elements outside the mechanism (**A** and **B**)

## Calculating a cause repertoire:

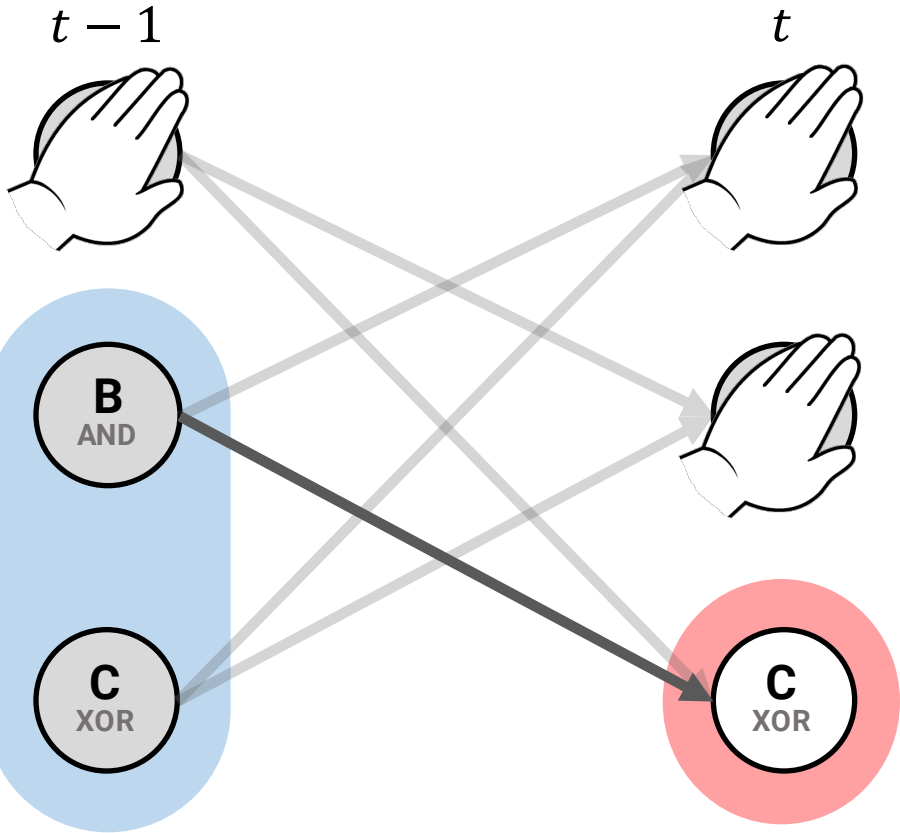

Now we marginalize over the current states of elements outside the mechanism (**A** and **B**)

|                |                                                                                      |                                                                                      | Current state |               |
|----------------|--------------------------------------------------------------------------------------|--------------------------------------------------------------------------------------|---------------|---------------|
|                |                                                                                      |                                                                                      | C             |               |
| Previous state | B                                                                                    | C                                                                                    |               |               |
|                | 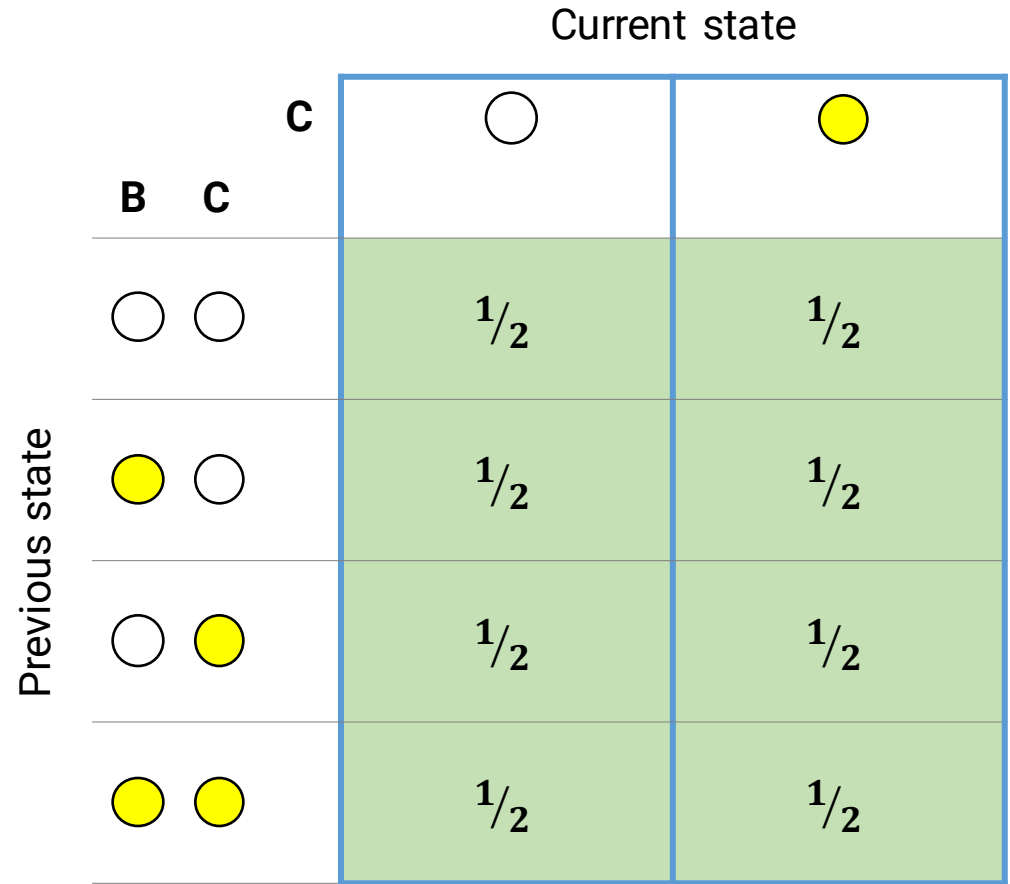  | 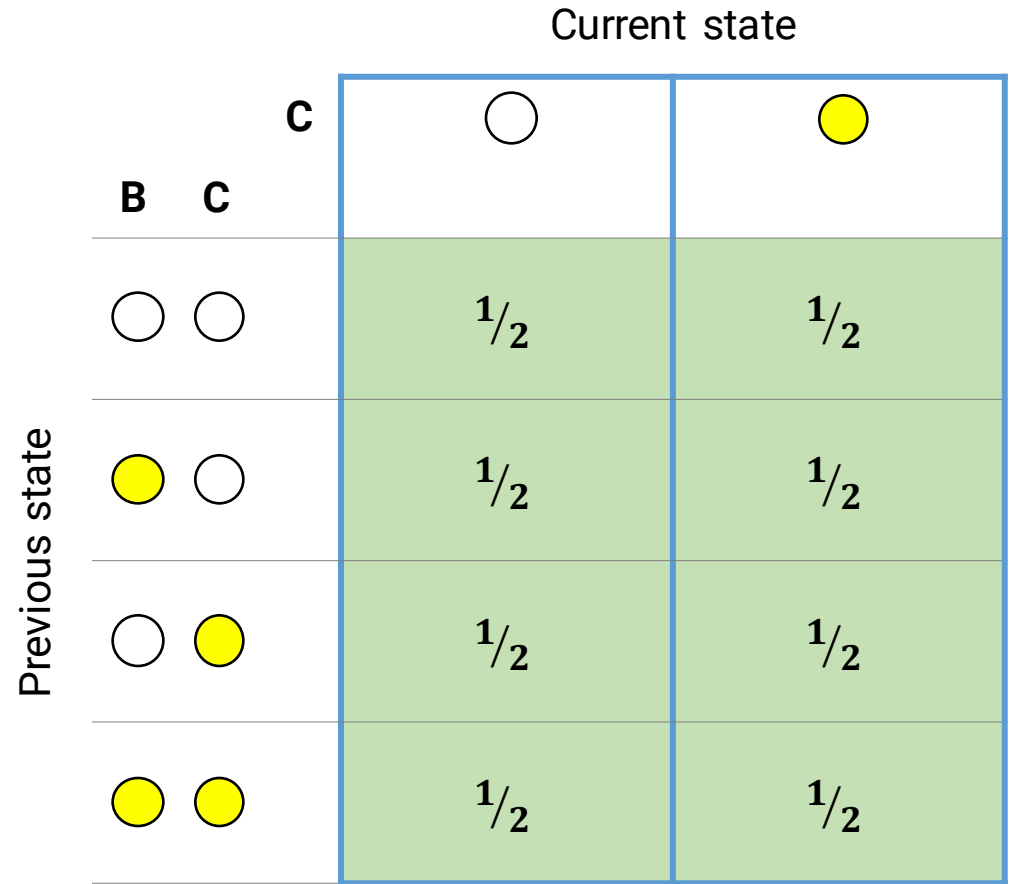  | $\frac{1}{2}$ | $\frac{1}{2}$ |
|                | 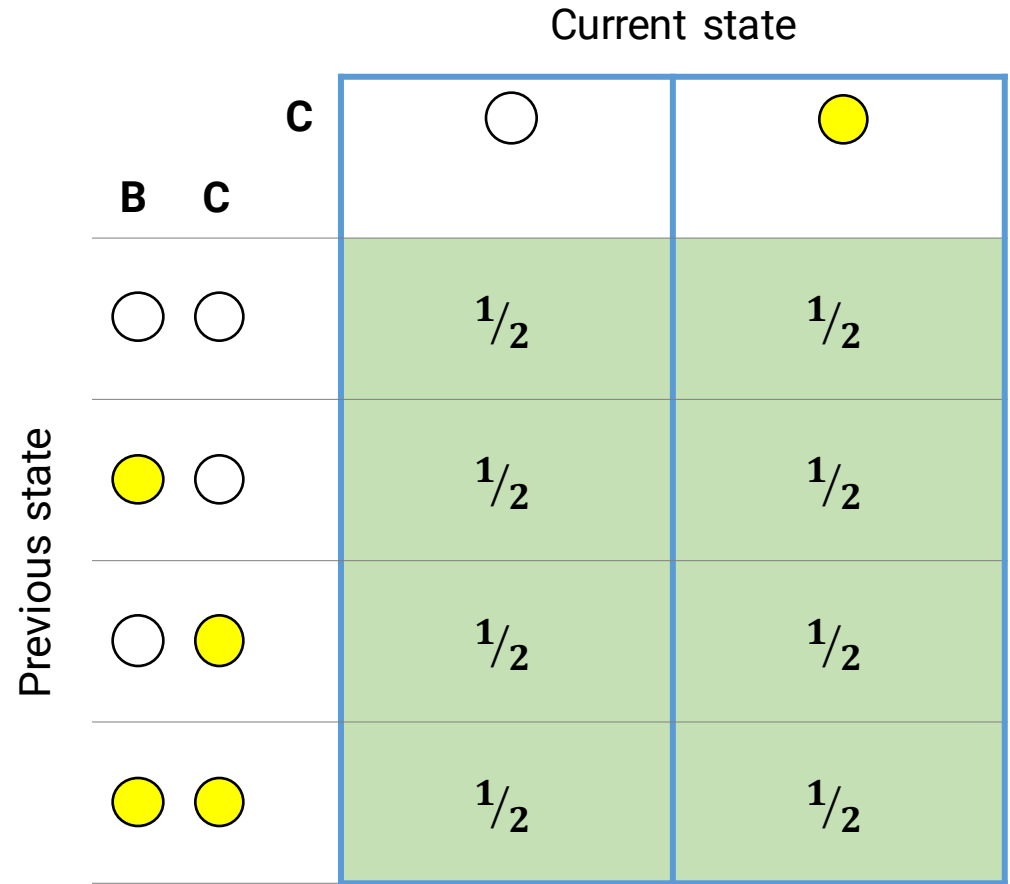  | 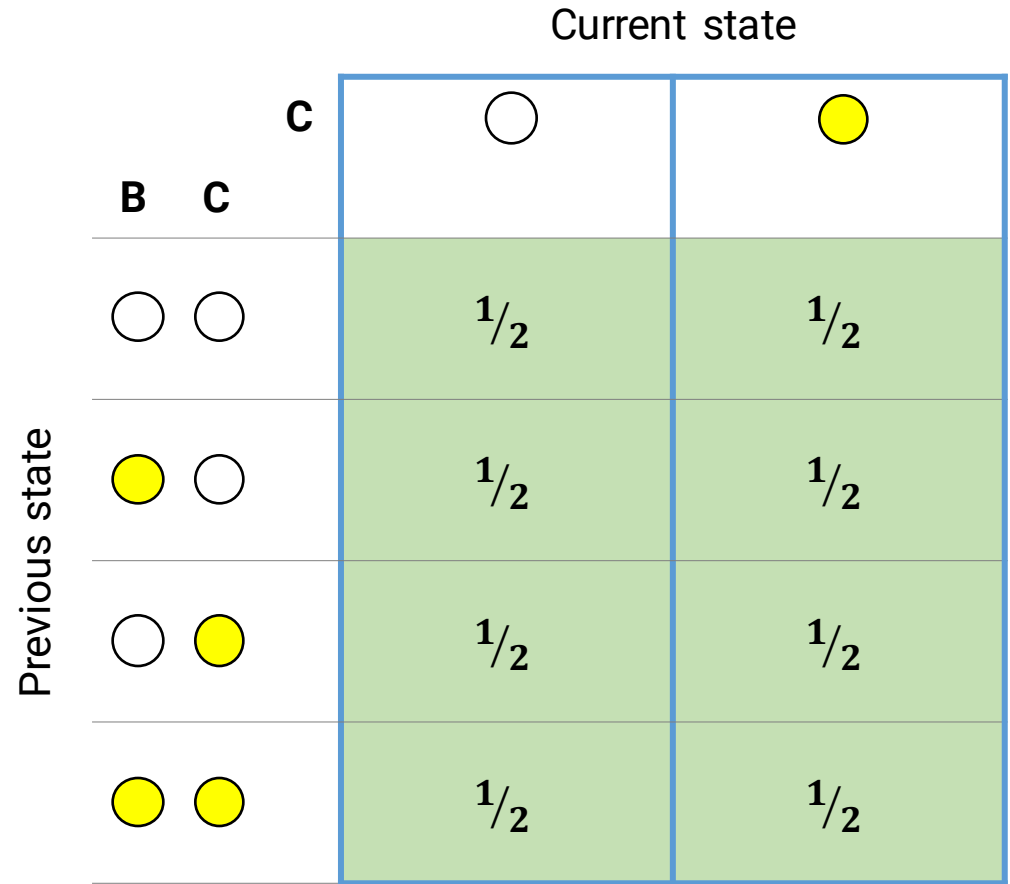  | $\frac{1}{2}$ | $\frac{1}{2}$ |
|                | 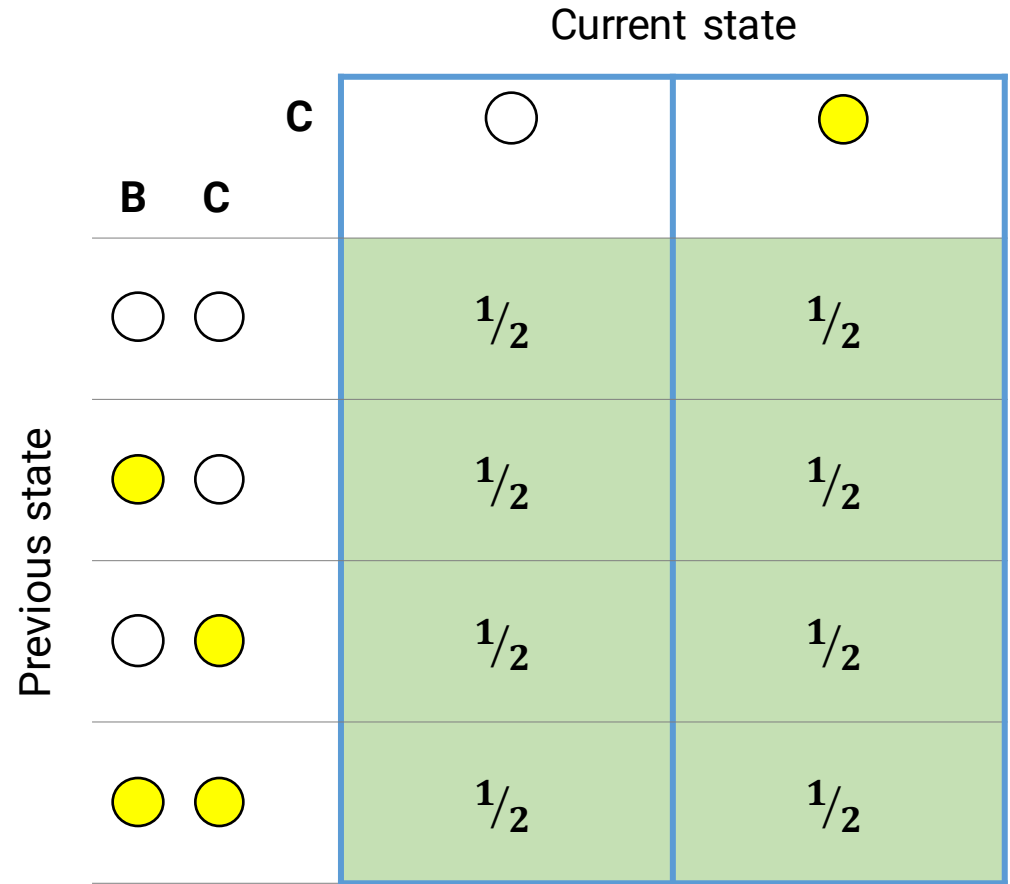  | 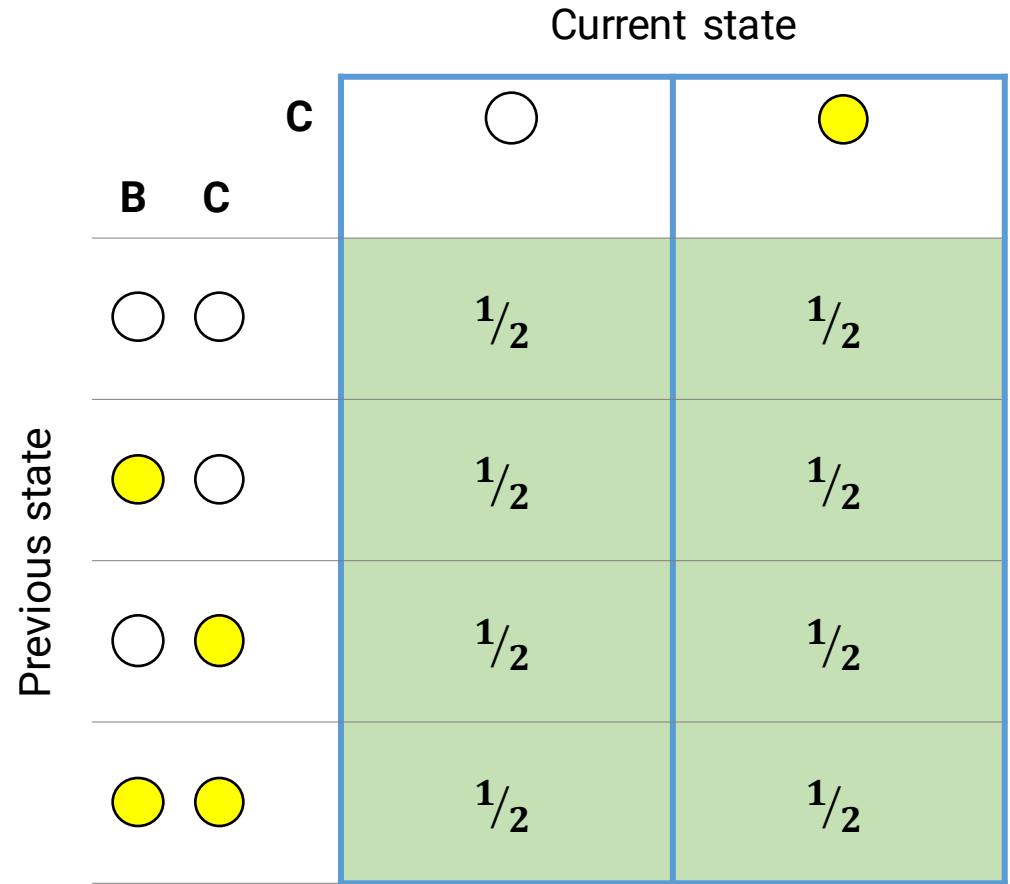  | $\frac{1}{2}$ | $\frac{1}{2}$ |
|                | 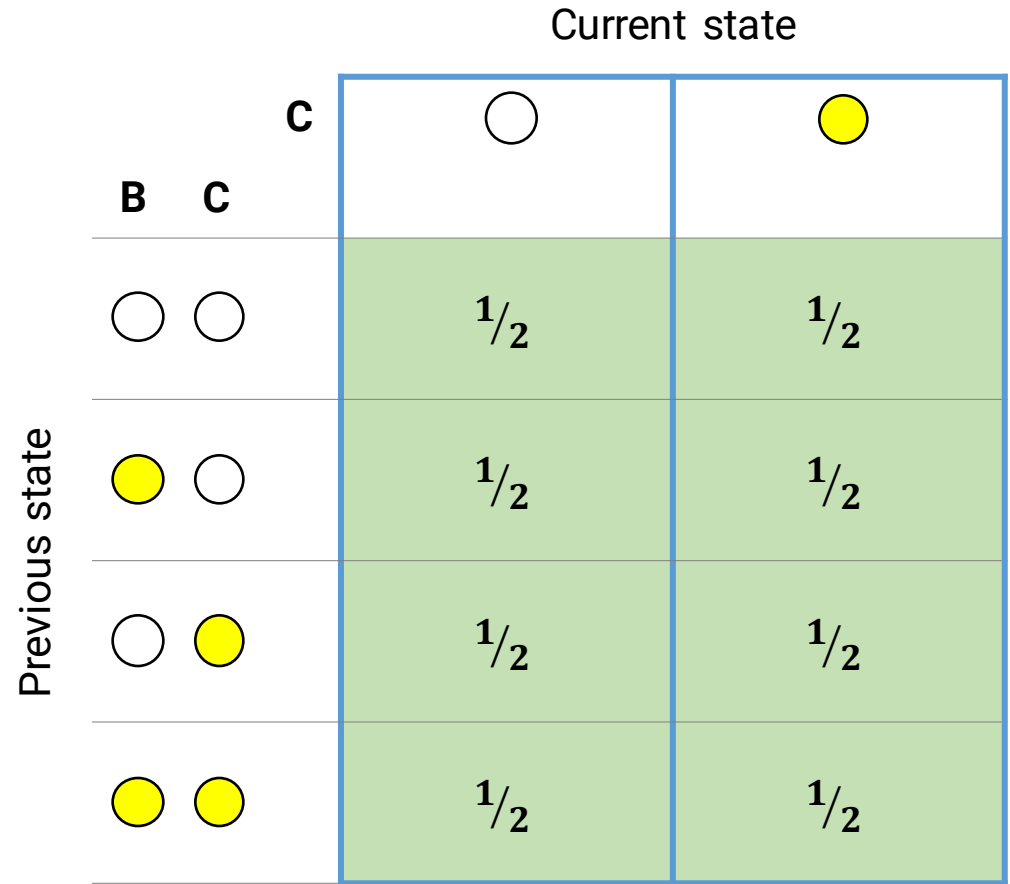 | 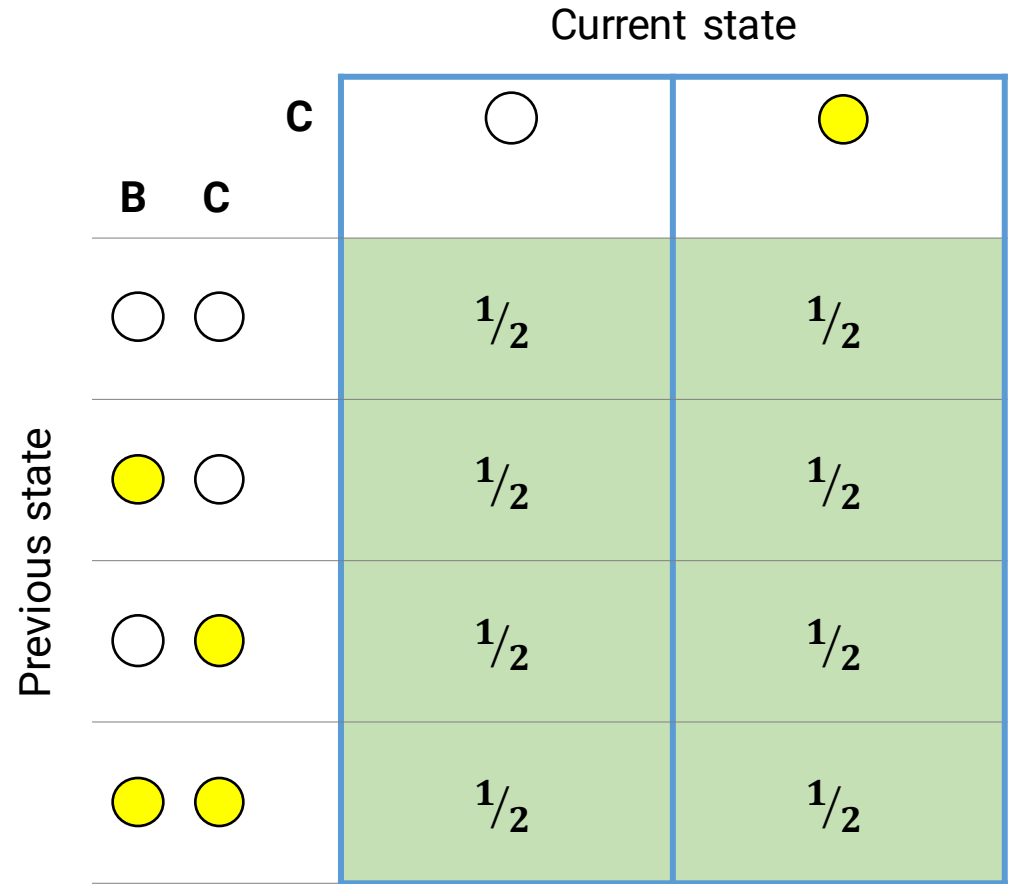 | $\frac{1}{2}$ | $\frac{1}{2}$ |

Calculating a cause repertoire:  
**Marginalizing-out non-mechanism elements**

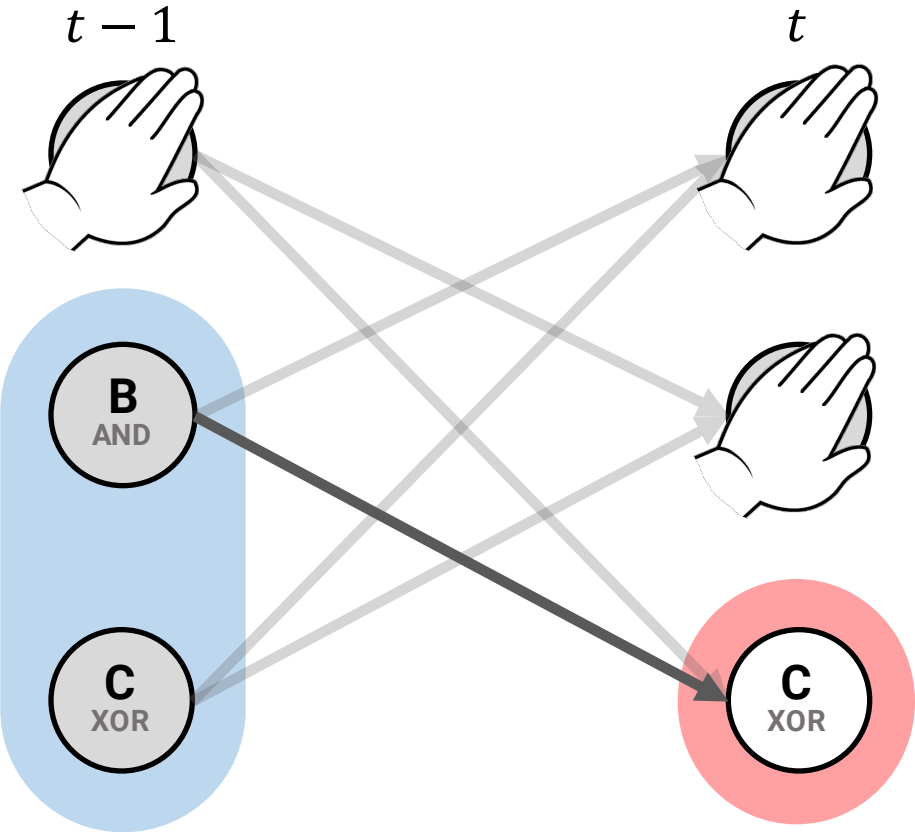

|                |     | Current state |               |
|----------------|-----|---------------|---------------|
|                |     |               |               |
| Previous state | B C |               |               |
|                |     | $\frac{1}{2}$ | $\frac{1}{2}$ |
|                |     | $\frac{1}{2}$ | $\frac{1}{2}$ |
|                |     | $\frac{1}{2}$ | $\frac{1}{2}$ |
|                |     | $\frac{1}{2}$ | $\frac{1}{2}$ |

Now we marginalize over the current states of elements outside the mechanism (**A** and **B**)

Calculating a cause repertoire:  
**Conditioning on the mechanism**

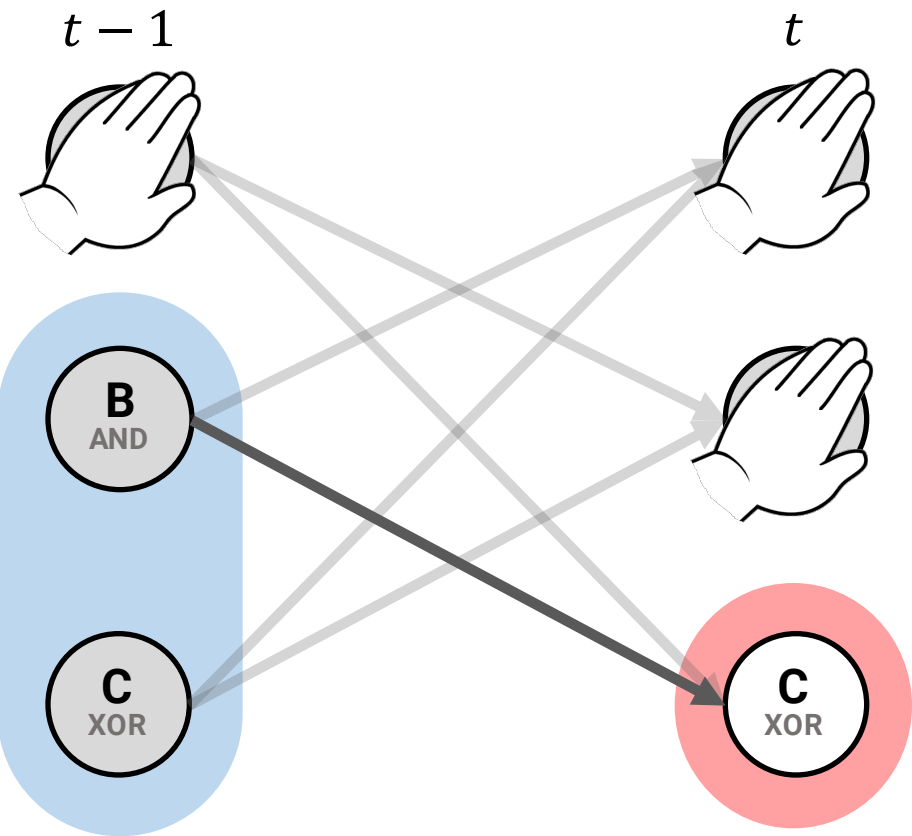

The next step is to condition on the current state of the mechanism, **C**

|                |                   | Current state |               |
|----------------|-------------------|---------------|---------------|
|                |                   | <b>C</b>      |               |
| Previous state | <b>B</b> <b>C</b> |               |               |
|                |                   | $\frac{1}{2}$ | $\frac{1}{2}$ |
|                |                   | $\frac{1}{2}$ | $\frac{1}{2}$ |
|                |                   | $\frac{1}{2}$ | $\frac{1}{2}$ |
|                |                   | $\frac{1}{2}$ | $\frac{1}{2}$ |

Calculating a cause repertoire:  
**Conditioning on the mechanism**

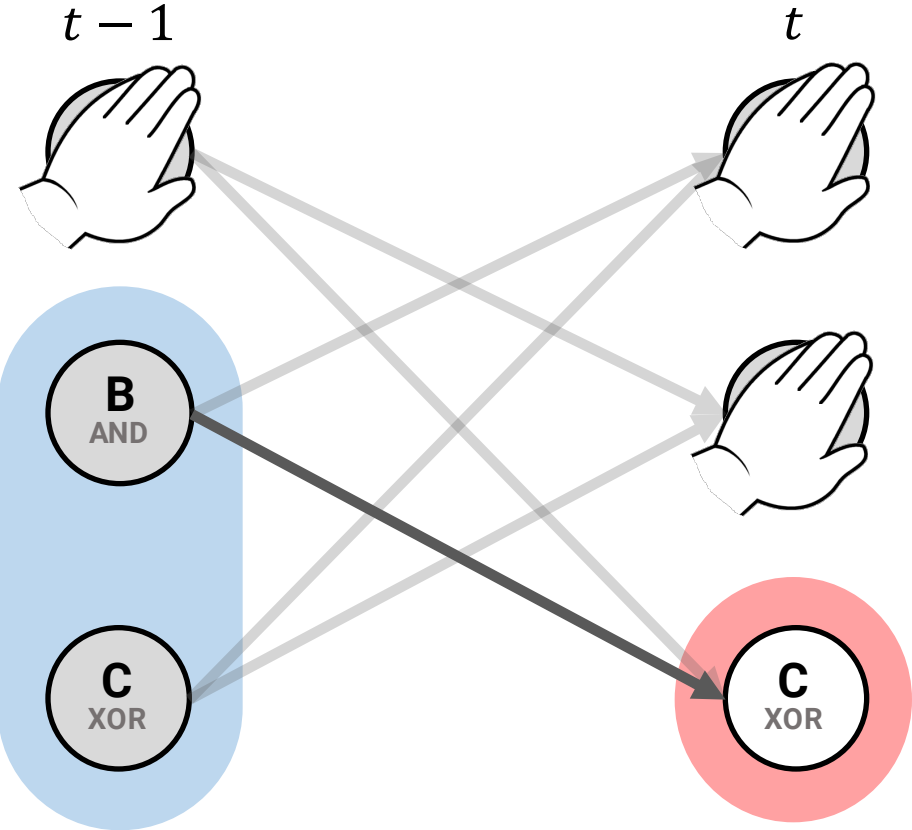

This is done by simply taking the column corresponding to **C**'s current state

|                |                   | Current state |               |
|----------------|-------------------|---------------|---------------|
|                |                   |               |               |
| Previous state | <b>B</b> <b>C</b> |               |               |
|                |                   | $\frac{1}{2}$ | $\frac{1}{2}$ |
|                |                   | $\frac{1}{2}$ | $\frac{1}{2}$ |
|                |                   | $\frac{1}{2}$ | $\frac{1}{2}$ |
|                |                   | $\frac{1}{2}$ | $\frac{1}{2}$ |

Calculating a cause repertoire:  
**Conditioning on the mechanism**

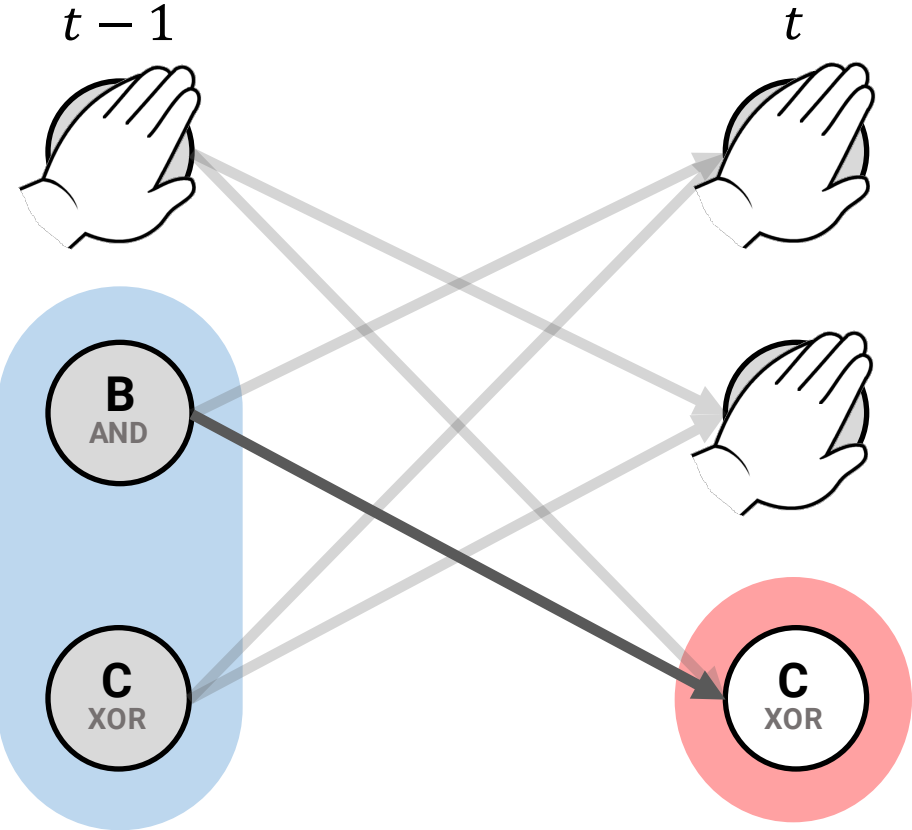

This is done by simply taking the column corresponding to **C**'s current state

|                |                                                                                      | Current state                                                                        |                                                                                     |                                                                                     |
|----------------|--------------------------------------------------------------------------------------|--------------------------------------------------------------------------------------|-------------------------------------------------------------------------------------|-------------------------------------------------------------------------------------|
|                |                                                                                      | C                                                                                    |                                                                                     |                                                                                     |
| Previous state | B                                                                                    | C                                                                                    |                                                                                     |                                                                                     |
|                |                                                                                      |                                                                                      | 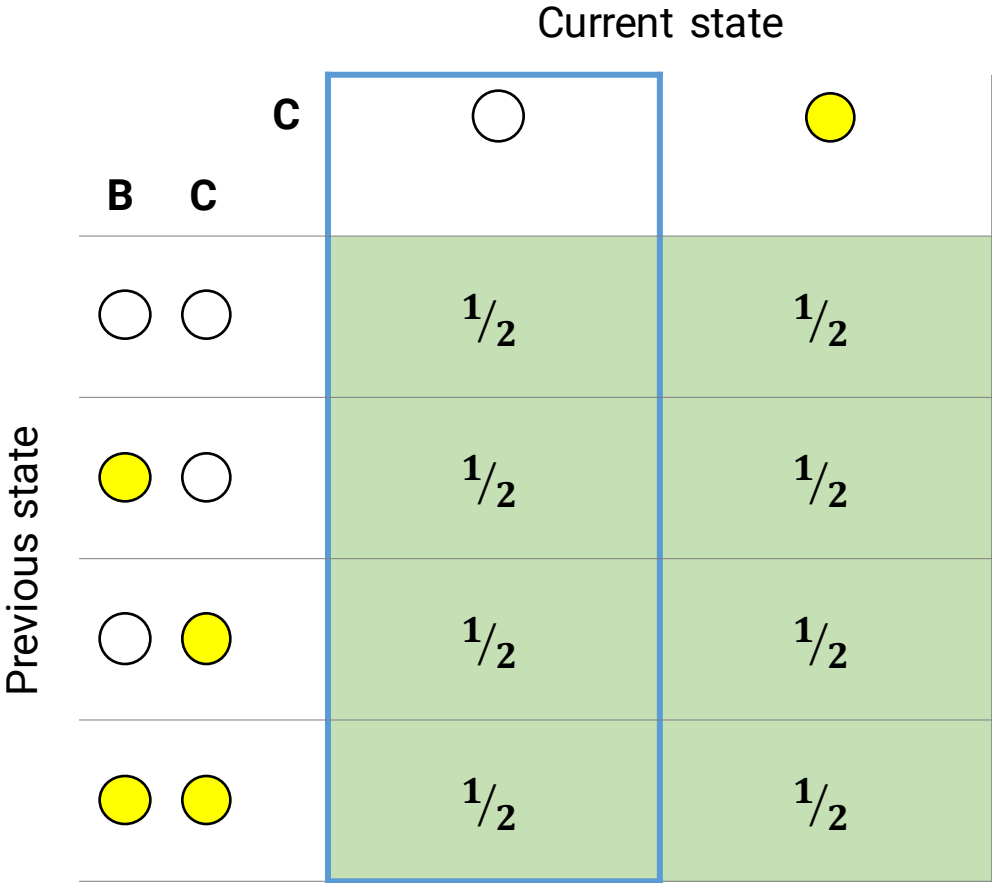 | 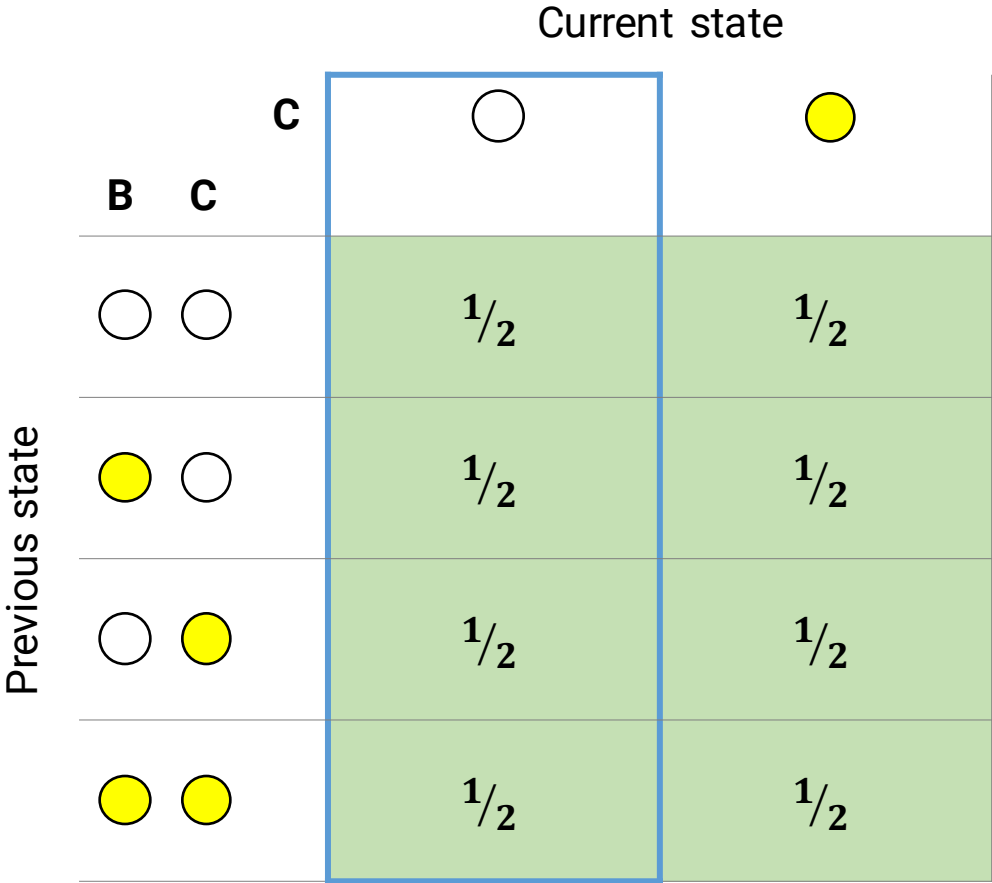 |
|                | 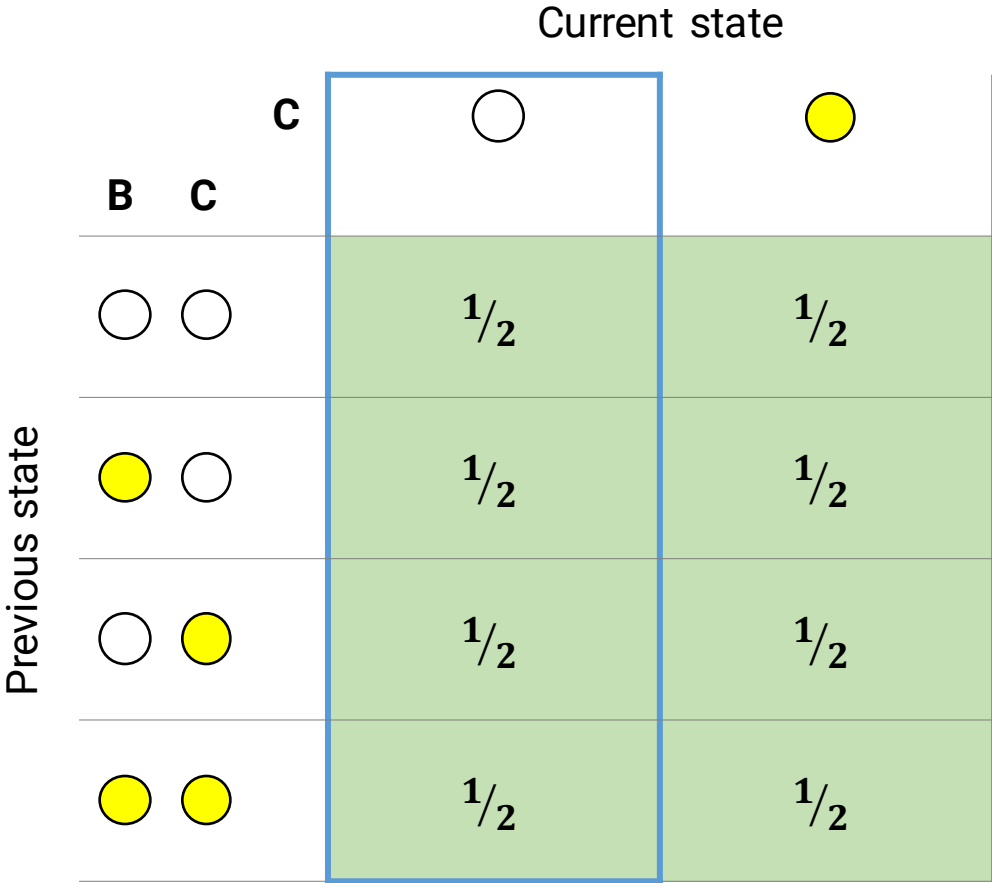  | 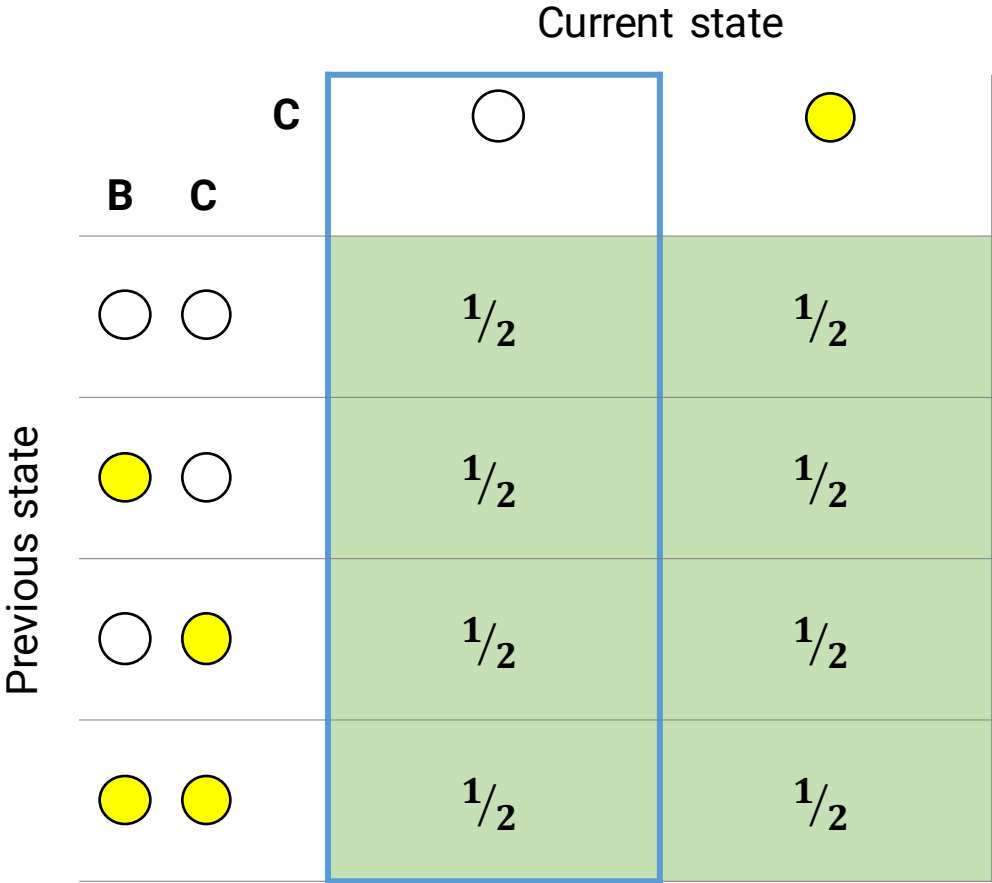  | $\frac{1}{2}$                                                                       | $\frac{1}{2}$                                                                       |
|                | 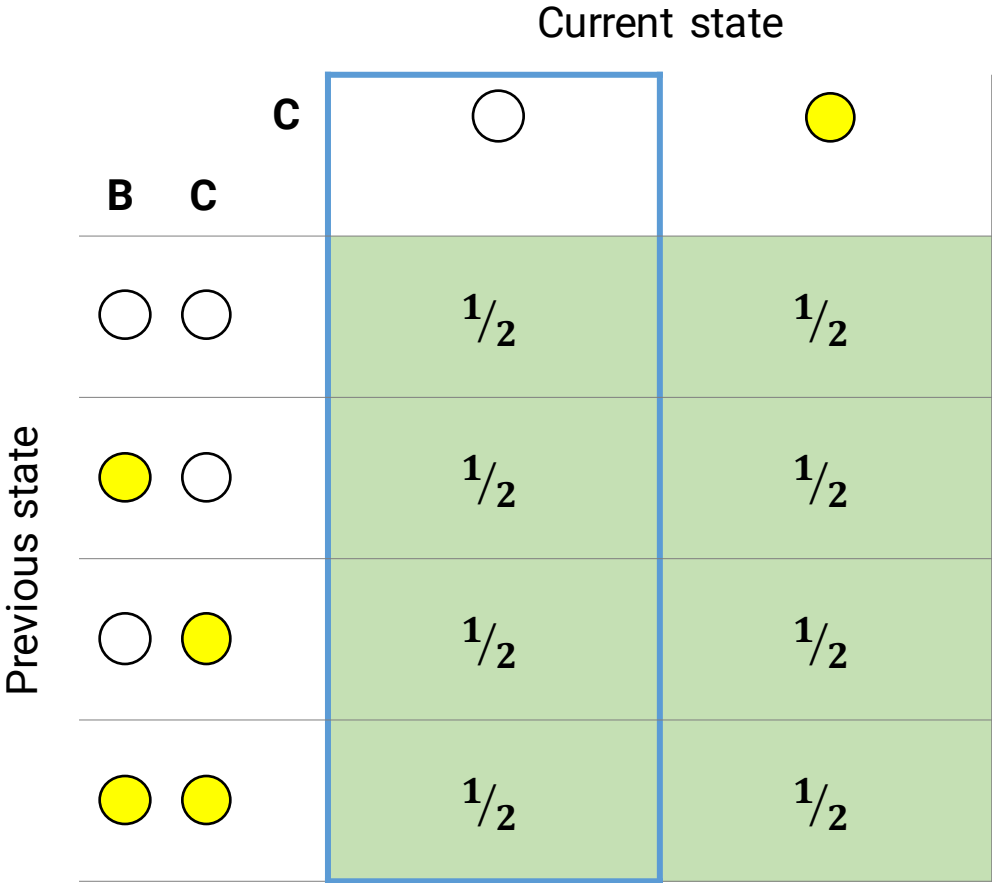  | 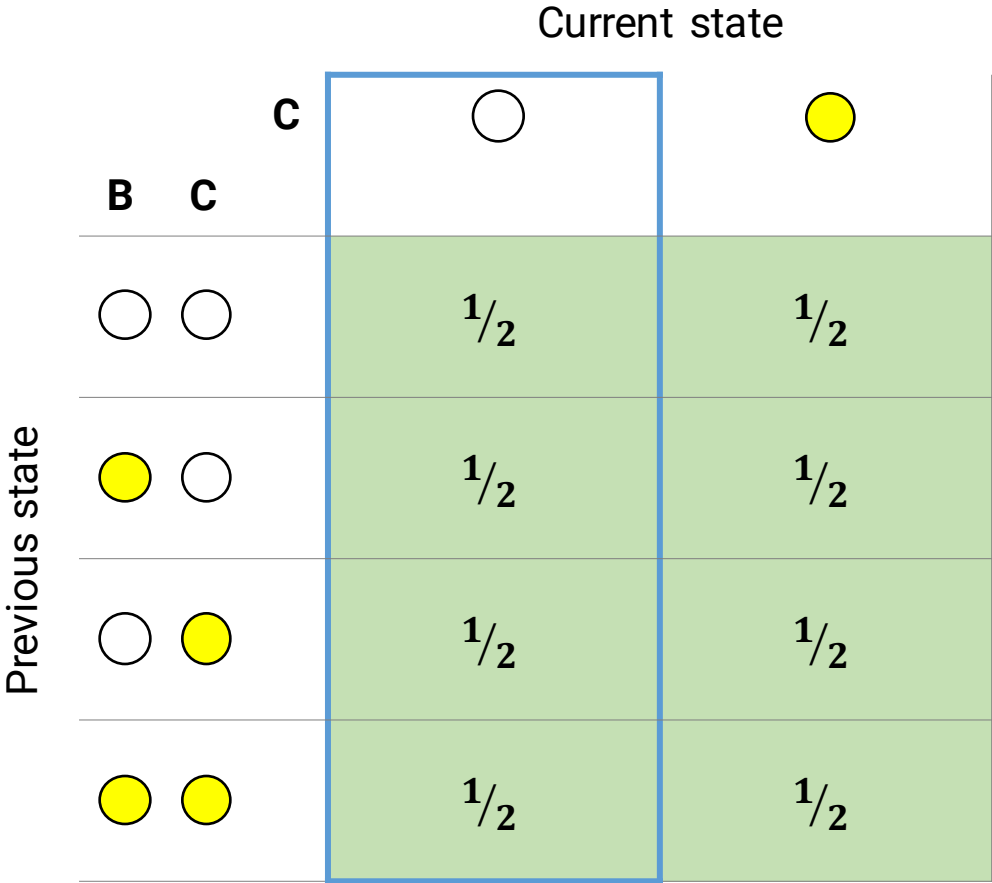  | $\frac{1}{2}$                                                                       | $\frac{1}{2}$                                                                       |
|                | 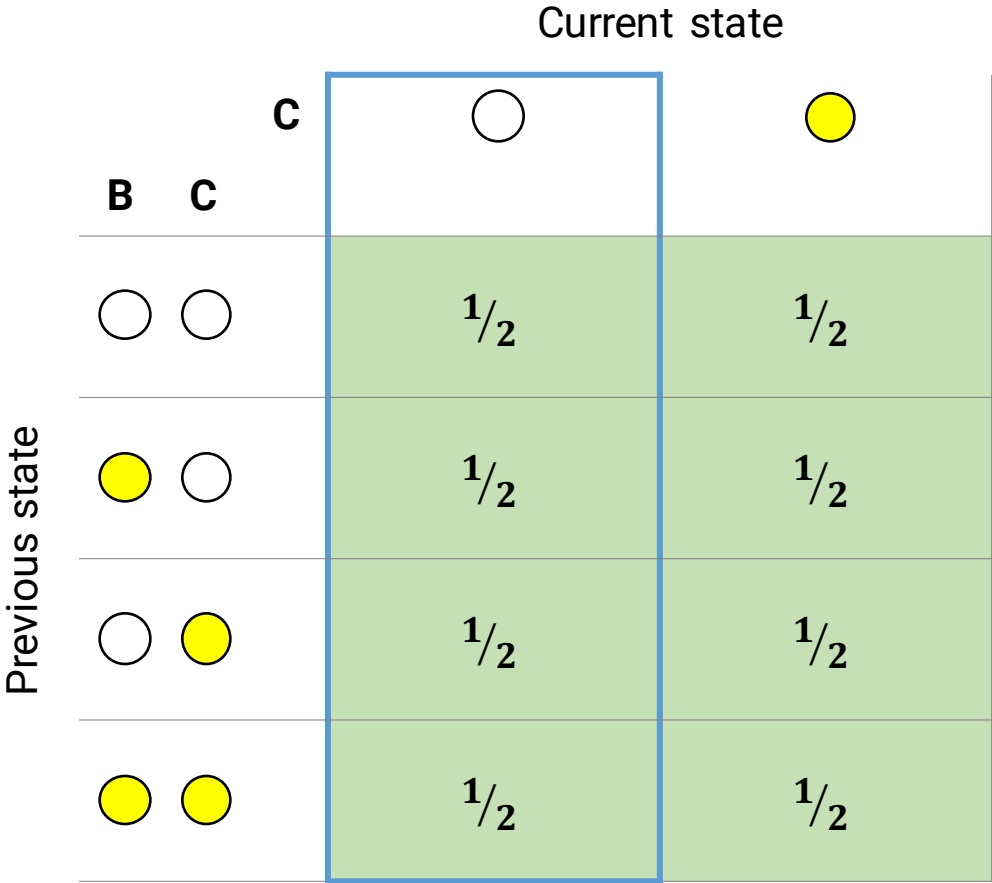  | 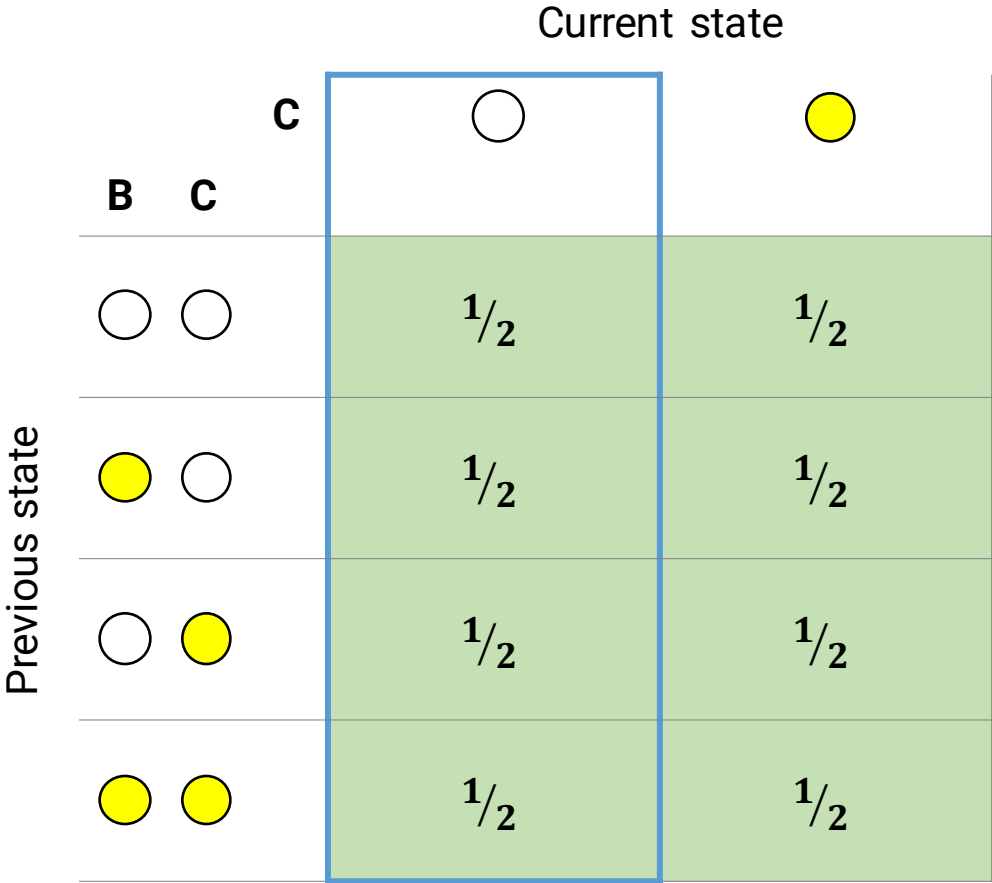  | $\frac{1}{2}$                                                                       | $\frac{1}{2}$                                                                       |
|                | 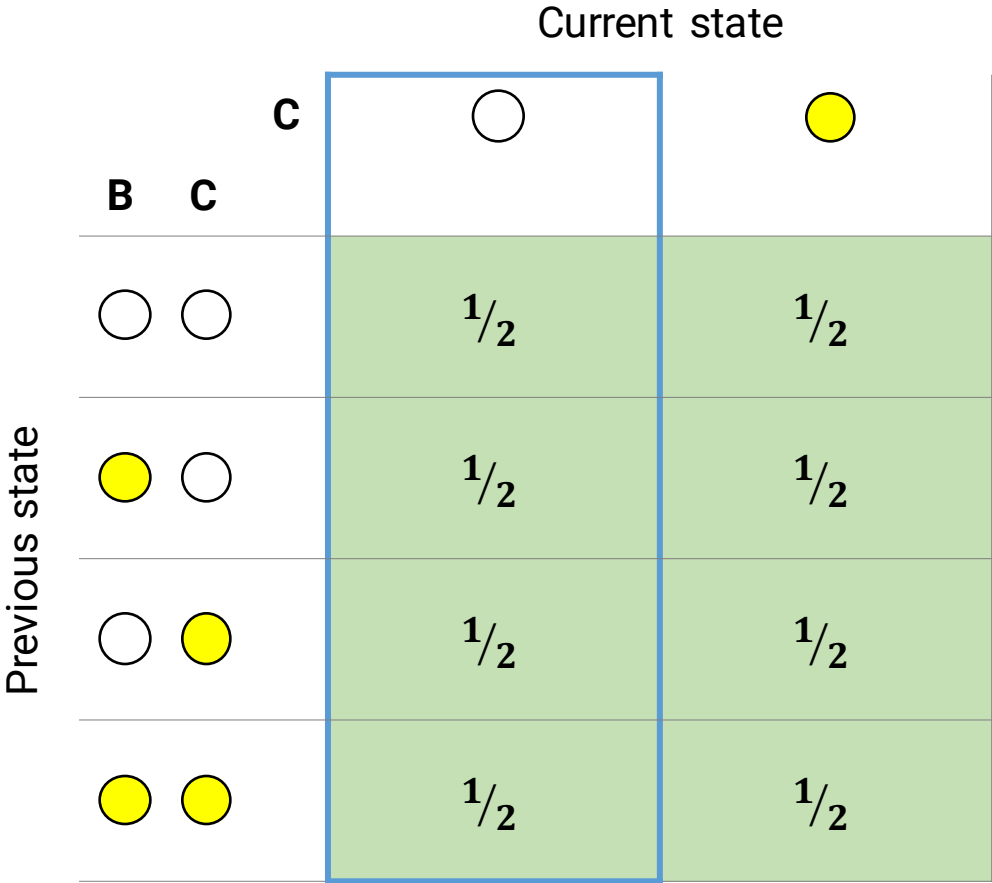 | 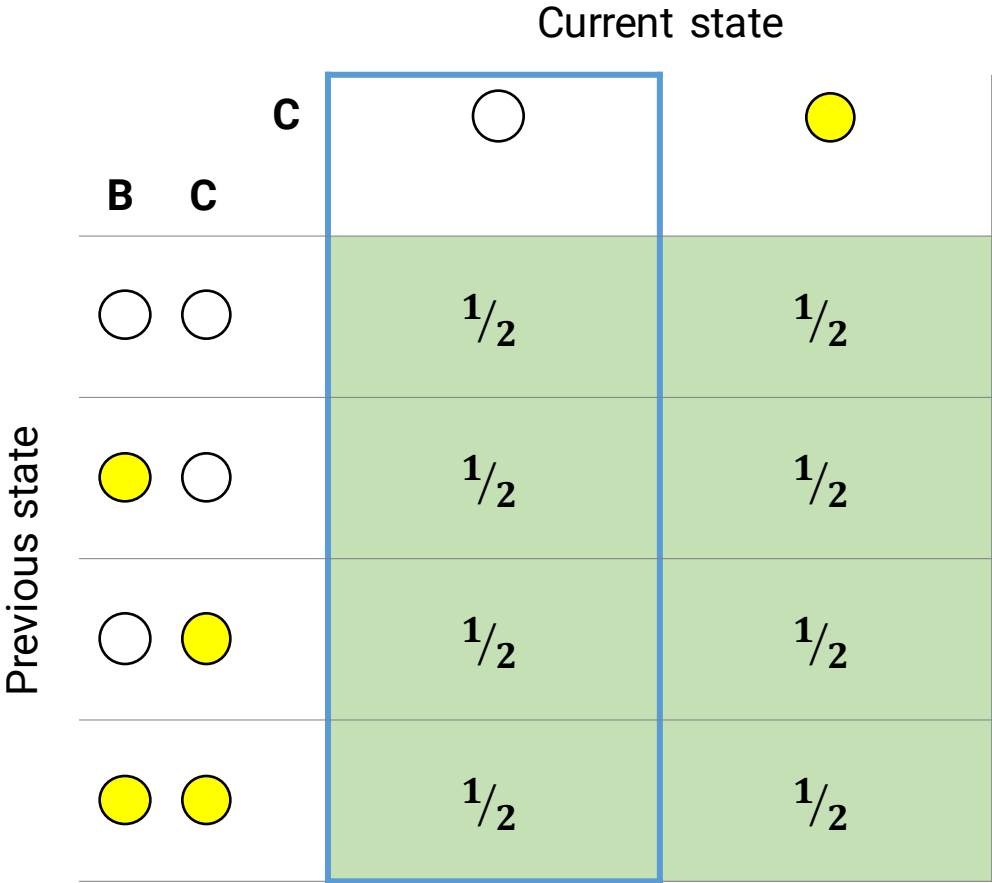 | $\frac{1}{2}$                                                                       | $\frac{1}{2}$                                                                       |

## Calculating a cause repertoire: **Conditioning on the mechanism**

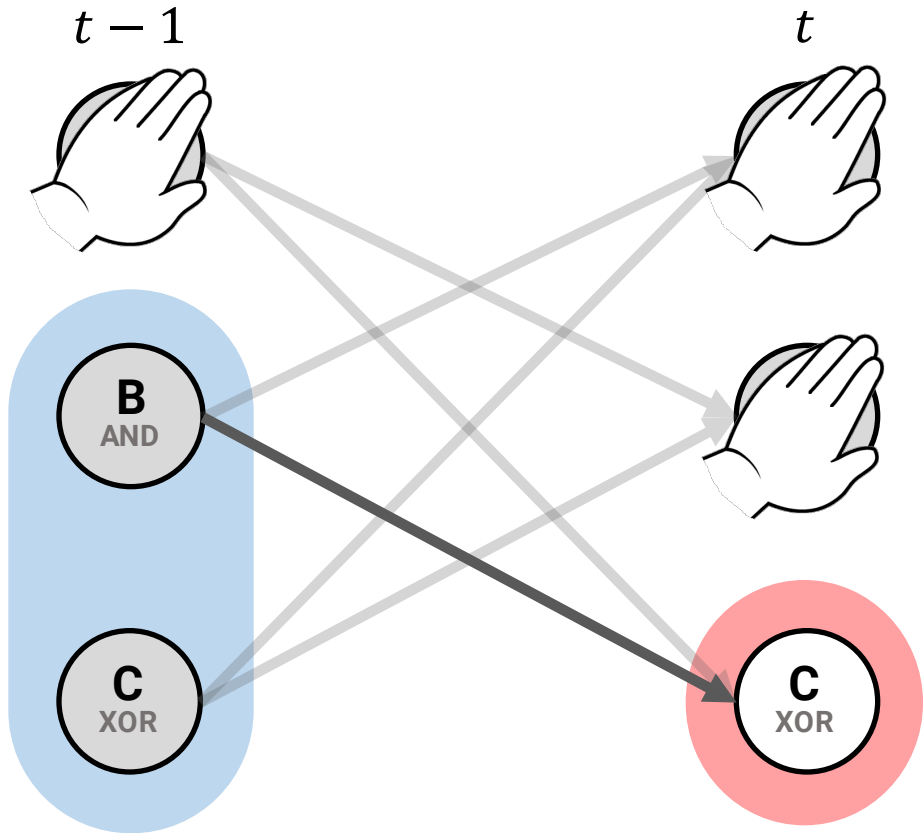

This is done by simply taking the column corresponding to **C**'s current state

| Previous state | B | C |               |
|----------------|---|---|---------------|
|                |   |   | $\frac{1}{2}$ |
|                |   |   | $\frac{1}{2}$ |
|                |   |   | $\frac{1}{2}$ |
|                |   |   | $\frac{1}{2}$ |

## Calculating a cause repertoire: Renormalizing

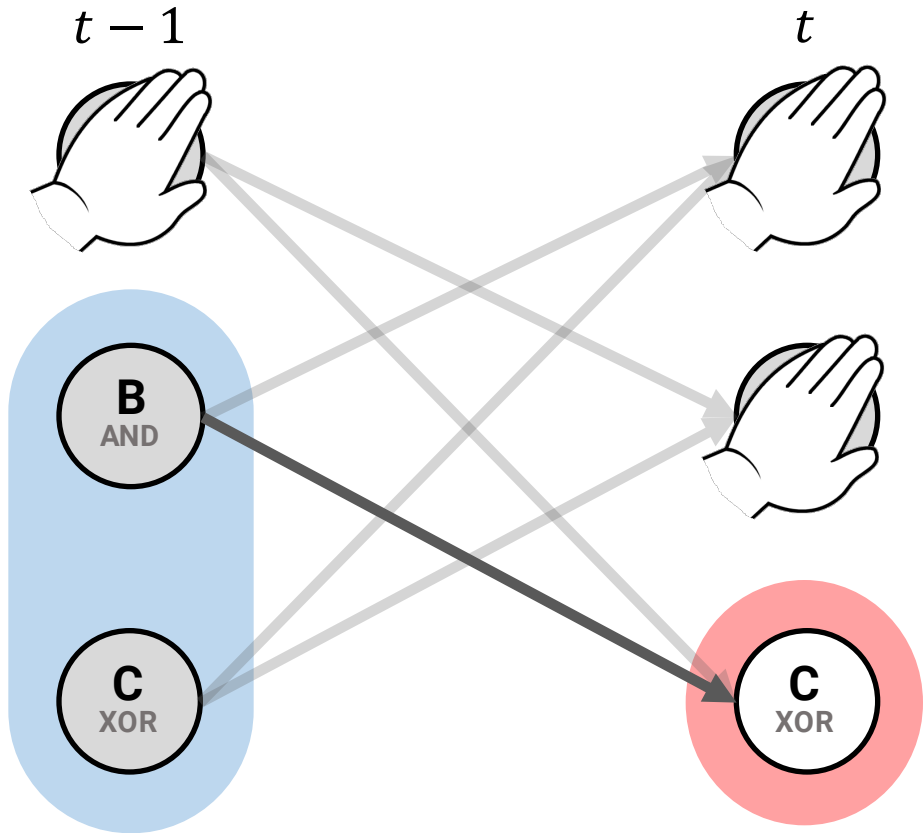

| Previous state | B | C |               |
|----------------|---|---|---------------|
|                |   |   | $\frac{1}{2}$ |
|                |   |   | $\frac{1}{2}$ |
|                |   |   | $\frac{1}{2}$ |
|                |   |   | $\frac{1}{2}$ |

And finally, we renormalize to obtain a proper distribution (not needed in this example, but required in general since columns of the TPM do not necessarily sum to 1)



Calculating a cause repertoire:  
**Renormalizing**

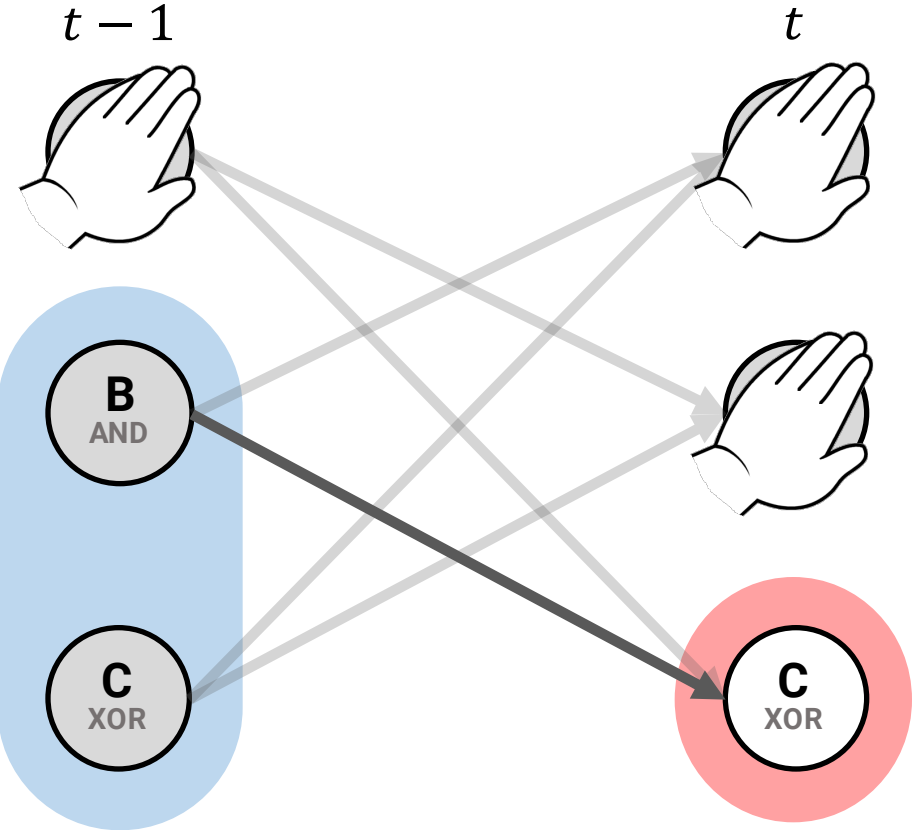

| Previous state | B | C |               |
|----------------|---|---|---------------|
|                |   |   | $\frac{1}{2}$ |
|                |   |   | $\frac{1}{2}$ |
|                |   |   | $\frac{1}{2}$ |
|                |   |   | $\frac{1}{2}$ |

This is the cause repertoire of **C** over **BC** when the system is in state (1, 0, 0)

Calculating a cause repertoire:  
**Renormalizing**

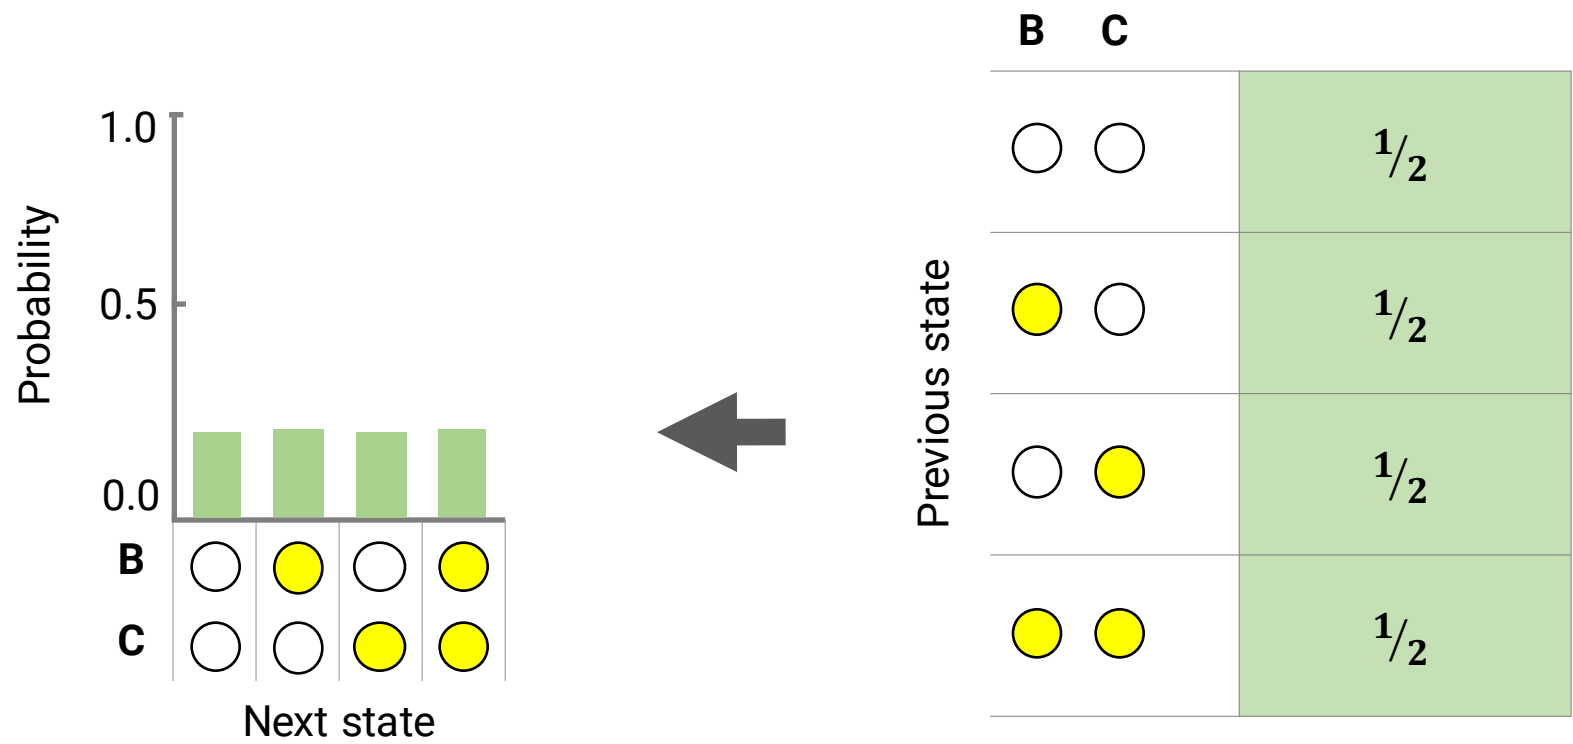

This is the cause repertoire of **C** over **BC** when the system is in state (1, 0, 0)

## Calculating a cause repertoire: Expanding to the full state-space

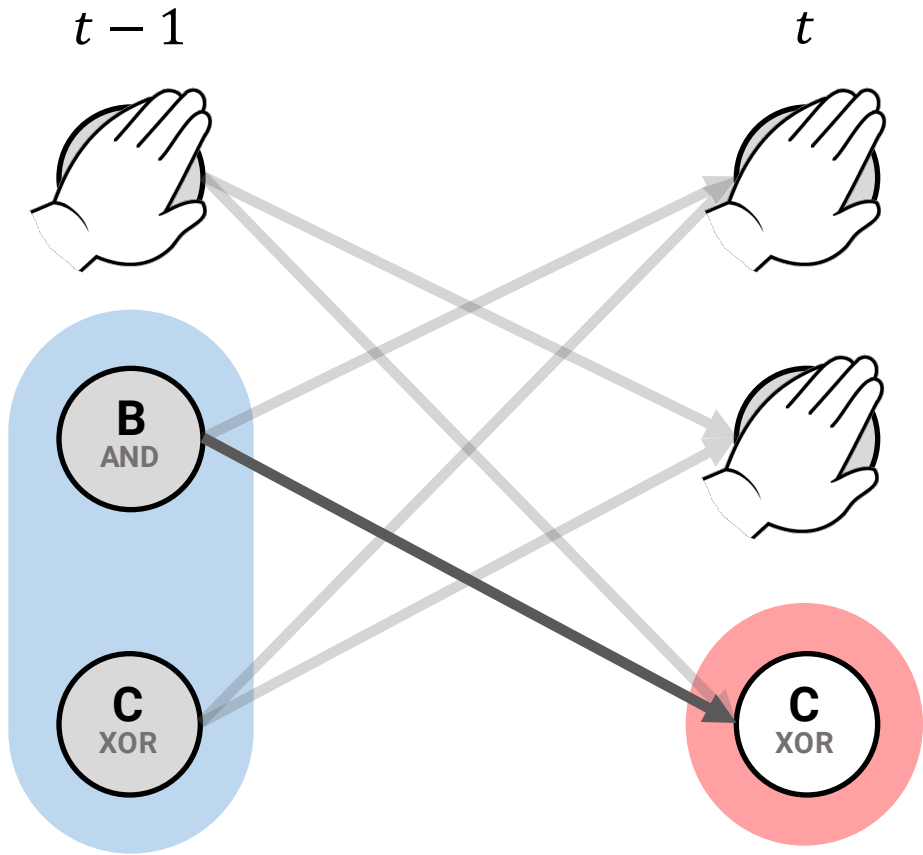

| Previous state | B | C |               |
|----------------|---|---|---------------|
|                |   |   | $\frac{1}{4}$ |
|                |   |   | $\frac{1}{4}$ |
|                |   |   | $\frac{1}{4}$ |
|                |   |   | $\frac{1}{4}$ |

Now, as with the effect repertoire, we can multiply this distribution by the unconstrained cause repertoire of the non-purview elements to get a distribution over the entire state space

## Calculating a cause repertoire: Expanding to the full state-space

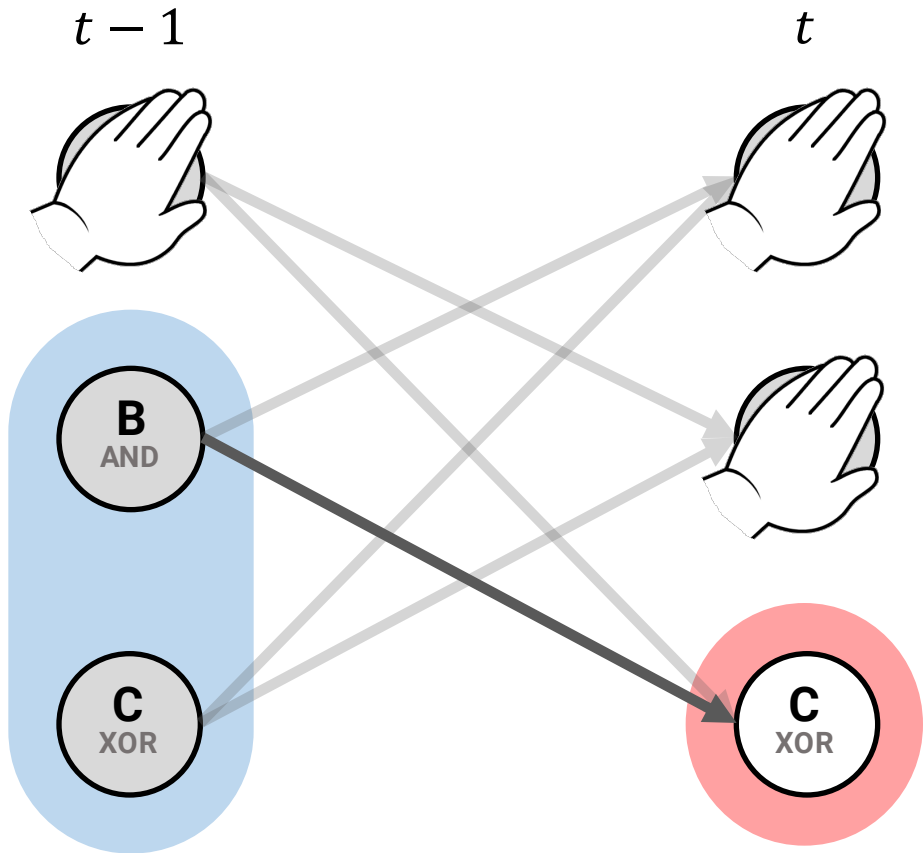

| Previous state | B | C |       |
|----------------|---|---|-------|
|                |   |   | $1/4$ |
|                |   |   | $1/4$ |
|                |   |   | $1/4$ |
|                |   |   | $1/4$ |

Recall that all previous states are equally likely in the perturbation, so the unconstrained cause repertoire of the non-mechanism elements is simply the uniform distribution

## Calculating a cause repertoire: **Expanding to the full state-space**

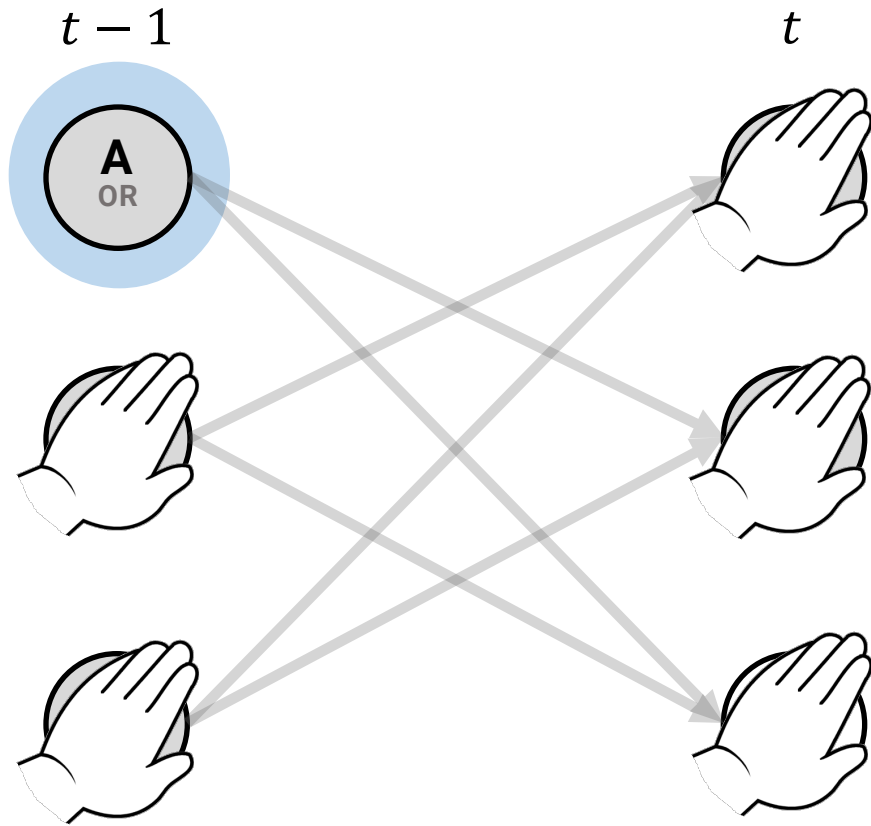

Recall that all previous states are equally likely in the perturbation, so the unconstrained cause repertoire of the non-mechanism elements is simply the uniform distribution

## Calculating a cause repertoire: Expanding to the full state-space

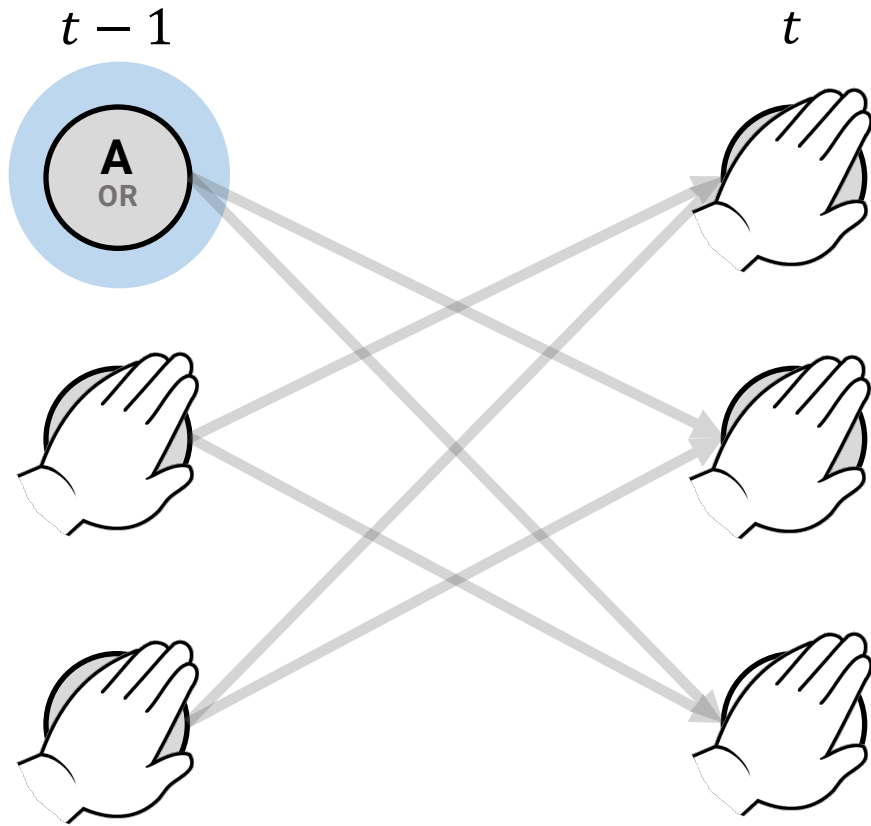

| Previous state | A |               |
|----------------|---|---------------|
|                |   |               |
| ○              |   | $\frac{1}{2}$ |
| ●              |   | $\frac{1}{2}$ |

Recall that all previous states are equally likely in the perturbation, so the unconstrained cause repertoire of the non-mechanism elements is simply the uniform distribution

# Calculating a cause repertoire: Expanding to the full state-space

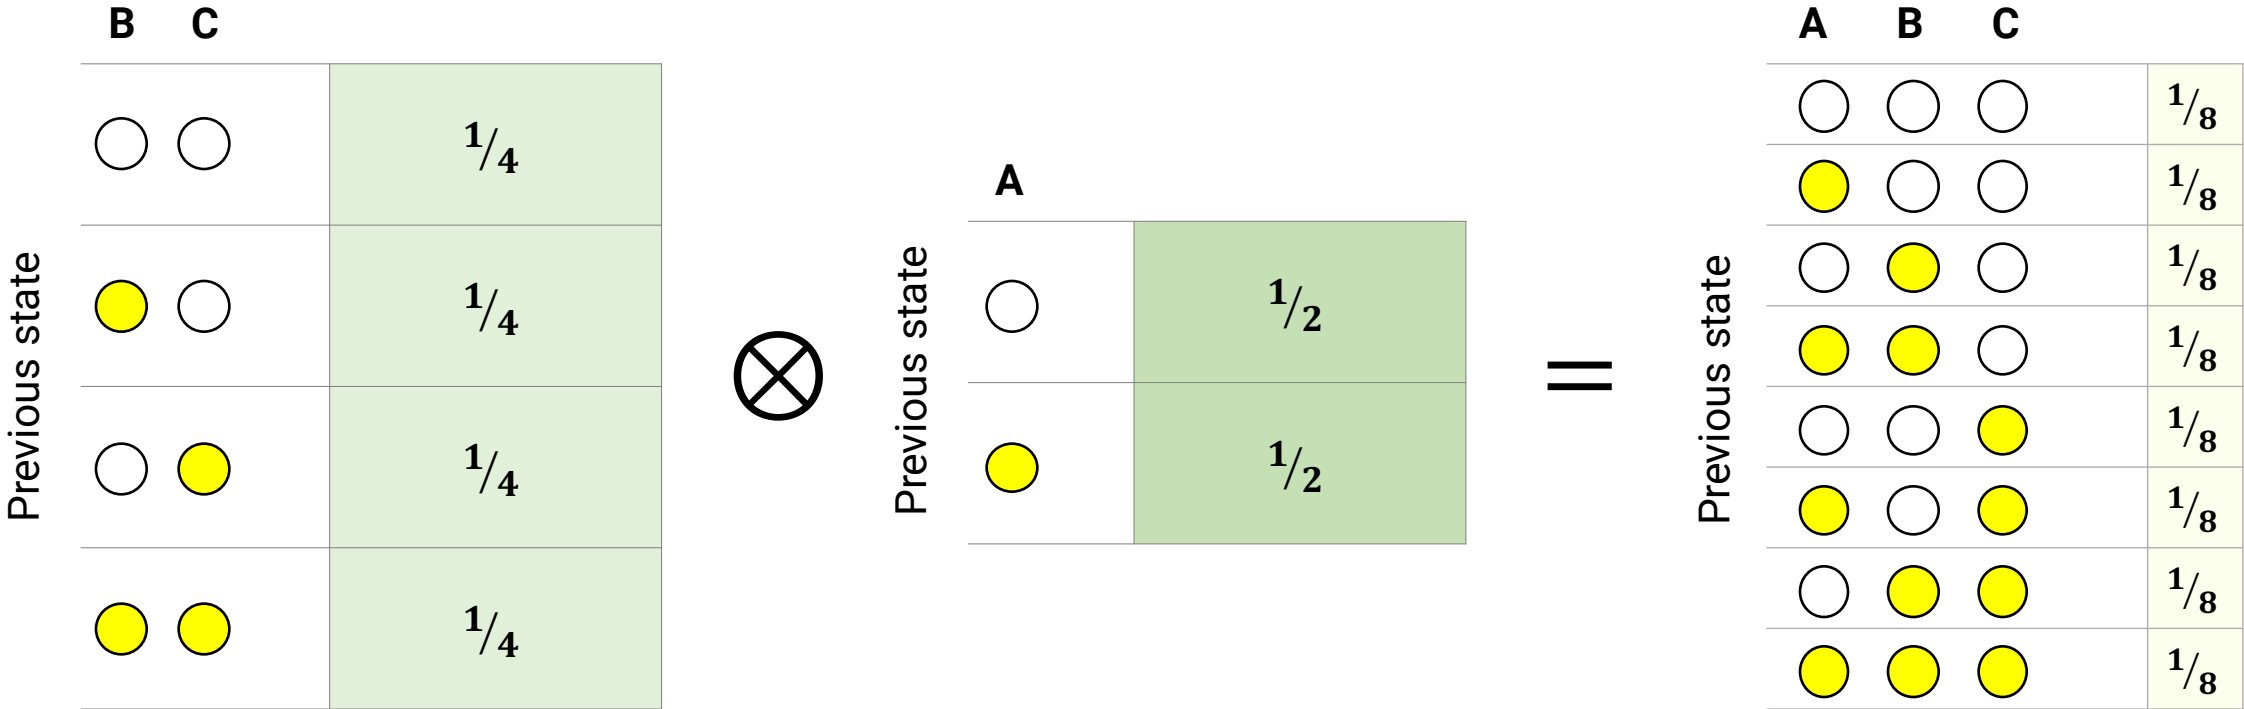

Now we can multiply the cause repertoire over the purview by the unconstrained repertoire to get the cause repertoire over the whole system’s state at  $t - 1$

Calculating a cause repertoire:  
**Expanding to the full state-space**

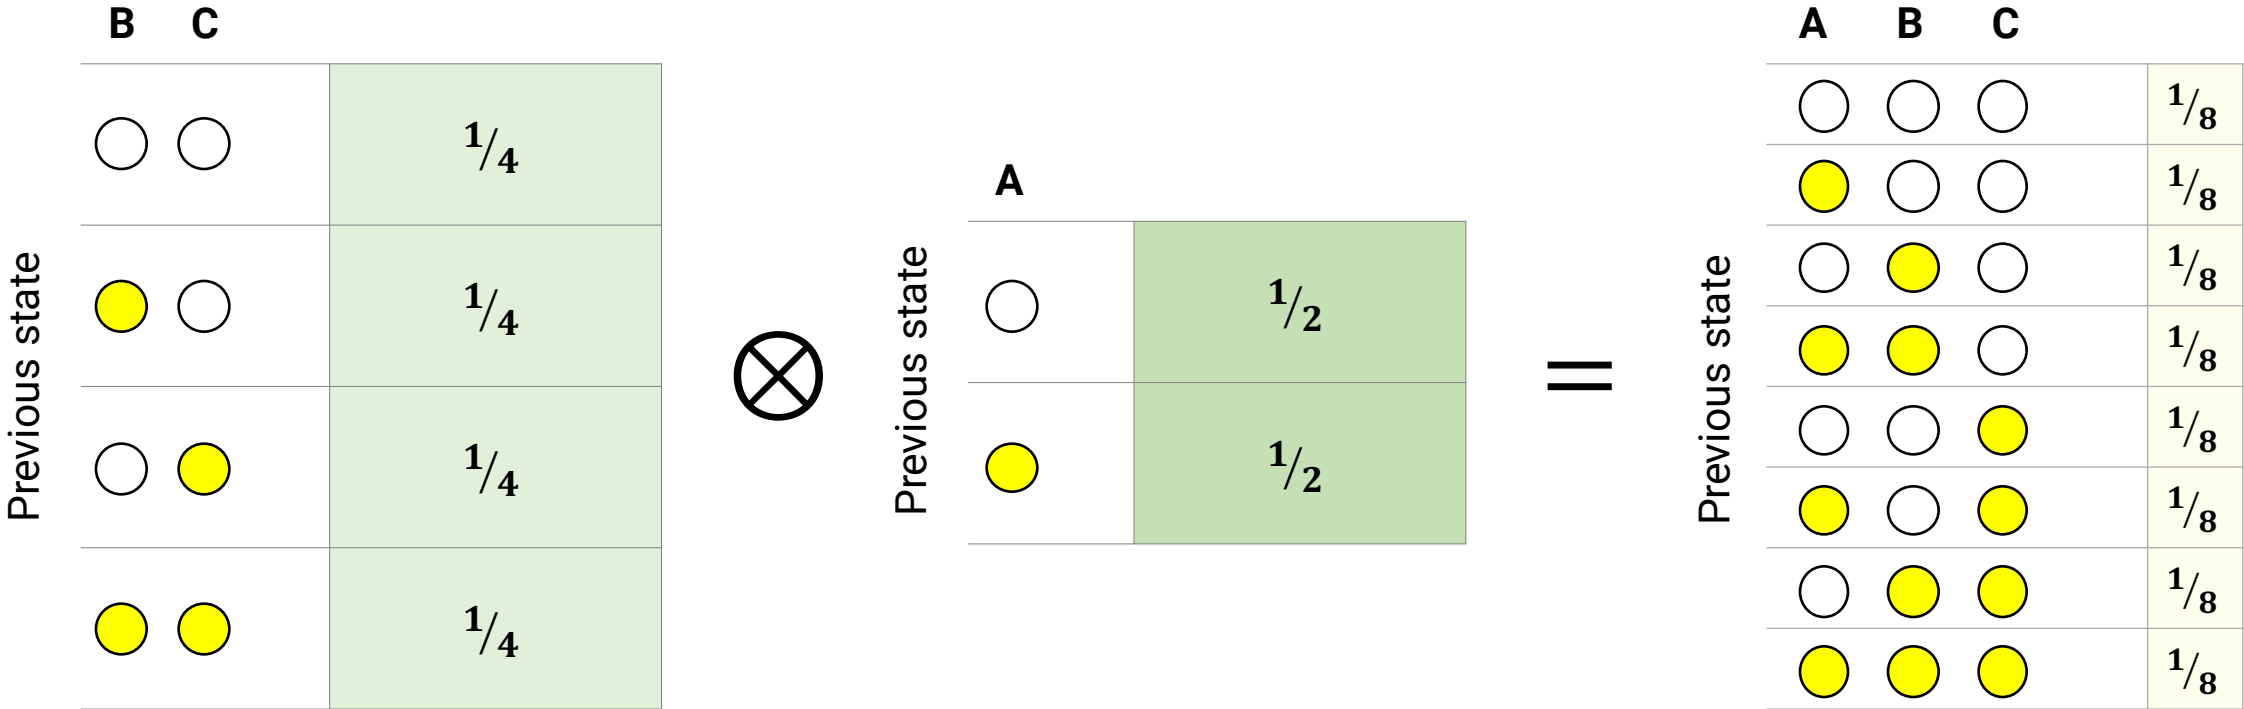

This is the expanded cause repertoire



# Calculating a cause repertoire

- Formally, the cause repertoire of a candidate mechanism  $Y$  at time  $t$  in a state  $y_0$  over the purview  $Z$  at time  $t - 1$  is the probability distribution

$$p_{\text{cause}}(\mathbf{Z}^{t-1} \mid \mathbf{Y}^t = \mathbf{y}_0).$$

- And it is obtained from Bayes rule:

$$p_{\text{cause}}(\mathbf{Z}^{t-1} \mid \mathbf{Y}^t = \mathbf{y}_0) = \frac{p(\mathbf{Y}^t = \mathbf{y}_0 \mid \mathbf{Z}^{t-1})p^{\text{uc}}(\mathbf{Z}^{t-1})}{p(\mathbf{Y}^t = \mathbf{y}_0)}.$$

- Here  $p^{\text{uc}}(\mathbf{Z}^{t-1})$  denotes the unconstrained distribution over purview states at  $t - 1$  (which is uniform, thanks to virtual elements)

# Outline

- Elements, states, and the TPM
- Background conditions
- Cause-effect repertoires
- **Integrated mechanisms:  $\varphi$**
- Concepts and cause-effect structures
- Integrated systems:  $\Phi$
- Complexes

# Integration and irreducibility

- The cause and effect repertoires quantify to what extent a candidate mechanism has selective causes and effects within the system
- Since IIT is concerned with the **intrinsic perspective** of the system, we are interested in whether or not a given candidate mechanism's causes and effects are **reducible** to the causes and effects of its parts
- If the candidate mechanism's causes and effects reduce to those of its parts, then there is nothing gained in terms of information by grouping the parts together in the first place
- The set of elements *per se* doesn't make a difference to the system

Integration and reducibility:

## An example of a reducible candidate mechanism

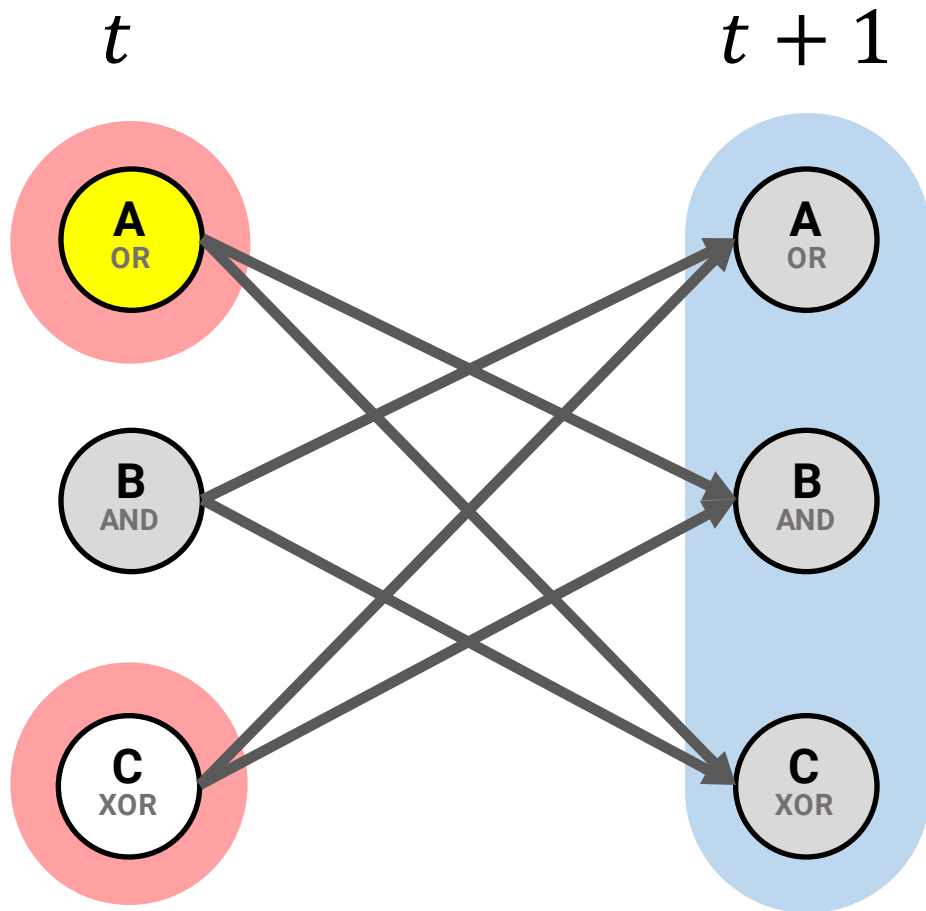

- Consider the mechanism **AC** over the purview **ABC**

Integration and reducibility:

**An example of a reducible candidate mechanism**

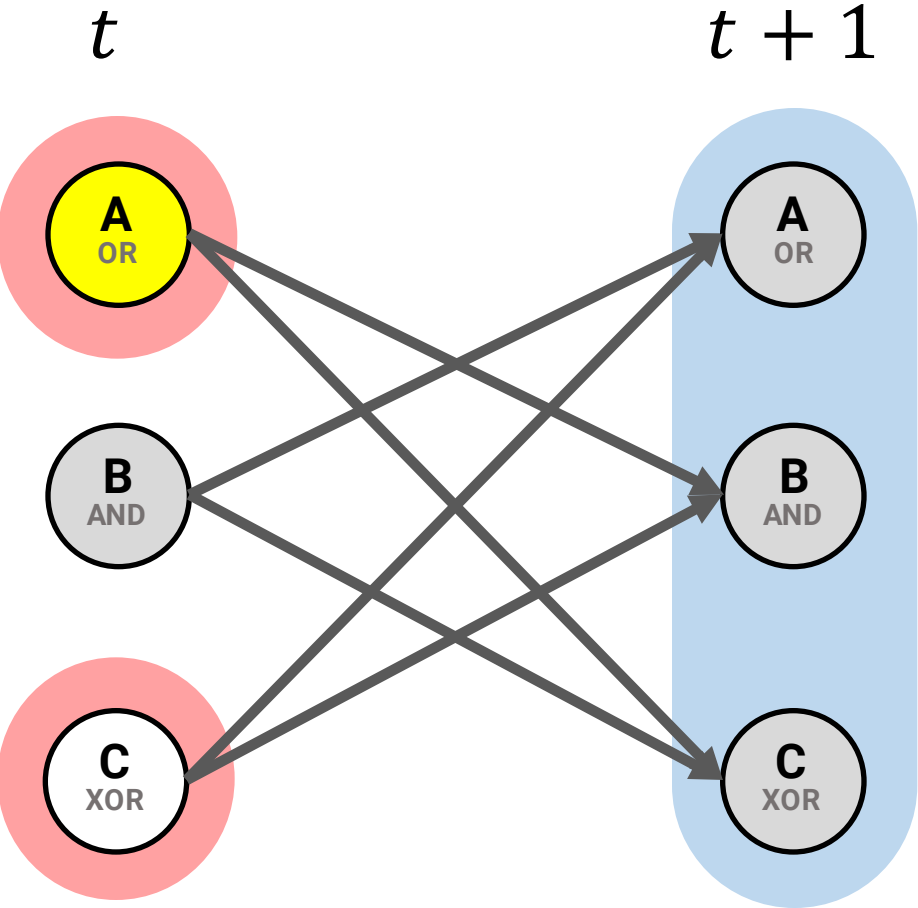

- Consider the mechanism **AC** over the purview **ABC**
- It has the following effect repertoire:

|               |   |   | Next state |     |     |     |     |     |     |     |
|---------------|---|---|------------|-----|-----|-----|-----|-----|-----|-----|
| Current state |   |   | A          |     |     |     |     |     |     |     |
|               | A | C |            |     |     |     |     |     |     |     |
|               | ● | ○ | 1/4        | 1/4 | 0   | 0   | 1/4 | 1/4 | 0   | 0   |
|               | ○ | ● | 0          | 0   | 1/4 | 1/4 | 0   | 0   | 1/4 | 1/4 |
|               | ● | ● | 0          | 0   | 0   | 0   | 0   | 0   | 0   | 0   |

Integration and reducibility:

## An example of a reducible candidate mechanism

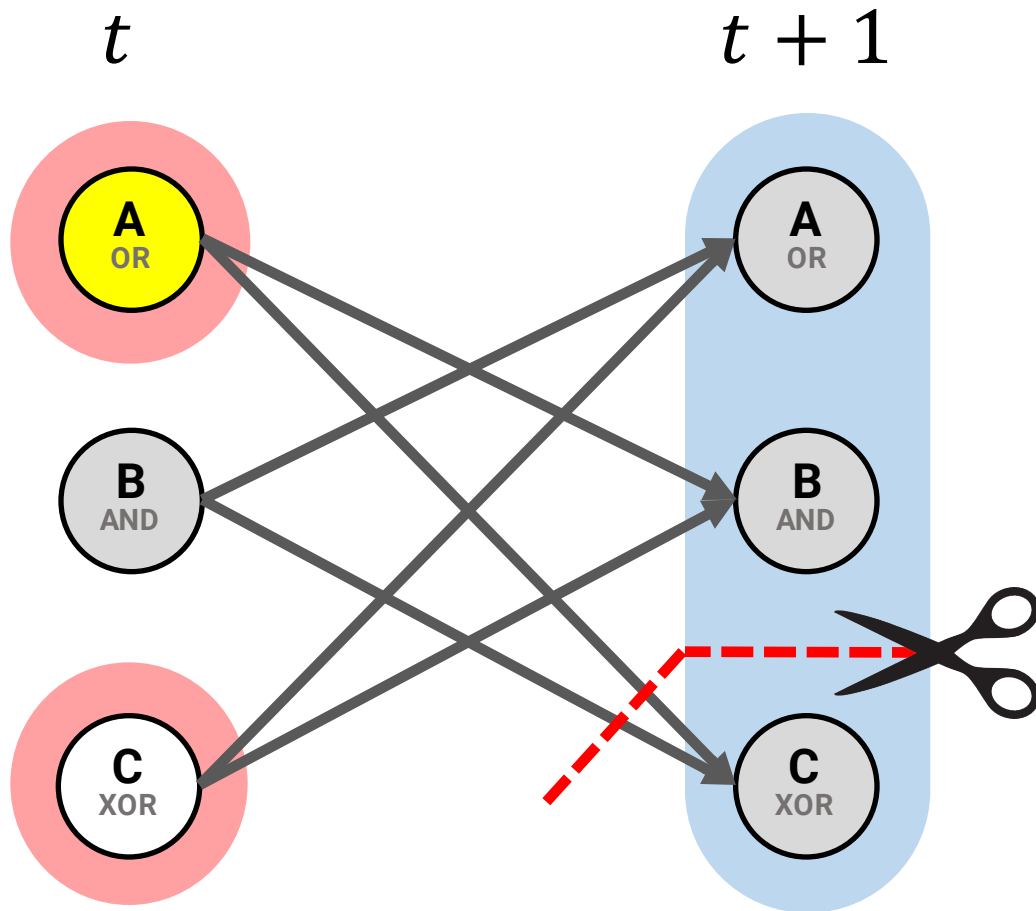

- Now we can partition the purview into **AB** and **C**
- Then we consider the effect repertoire of the mechanism **AC** over **AB** and the unconstrained repertoire of **C**
- In other words, we can separate the repertoire  $\frac{AC}{ABC}$  into  $\frac{AC}{AB}$  and  $\frac{\emptyset}{C}$

Integration and reducibility:  
**An example of a reducible mechanism**

- We calculate the unconstrained repertoire of **C**:

|   | Next state                                                                          |                                                                                     |
|---|-------------------------------------------------------------------------------------|-------------------------------------------------------------------------------------|
| C | 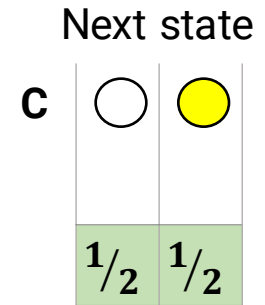 | 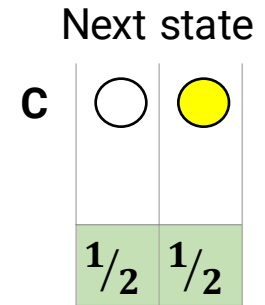 |
|   | $\frac{1}{2}$                                                                       | $\frac{1}{2}$                                                                       |

- And the repertoire **AC** over **AB**:

|   |   | Next state                                                                          |                                                                                     |                                                                                     |                                                                                     |
|---|---|-------------------------------------------------------------------------------------|-------------------------------------------------------------------------------------|-------------------------------------------------------------------------------------|-------------------------------------------------------------------------------------|
|   |   | A                                                                                   |                                                                                     | B                                                                                   |                                                                                     |
|   |   | 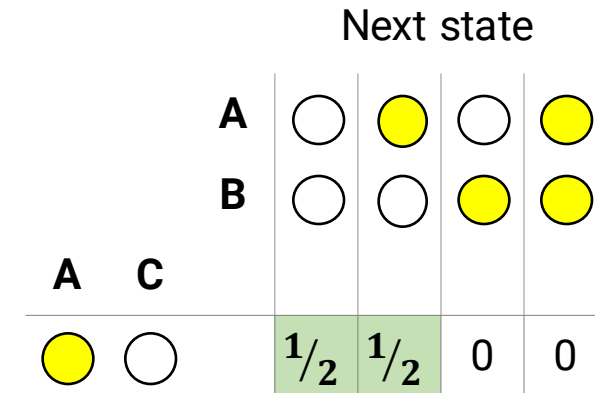 | 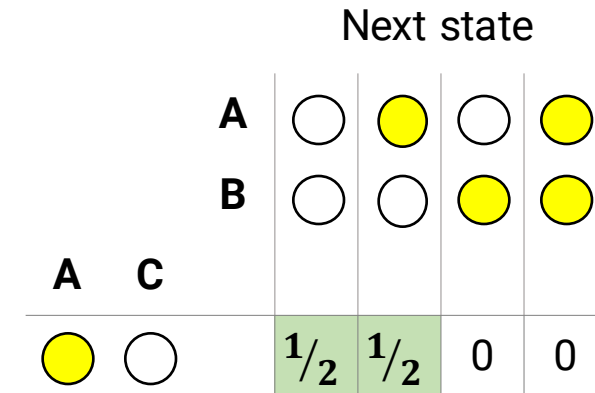 | 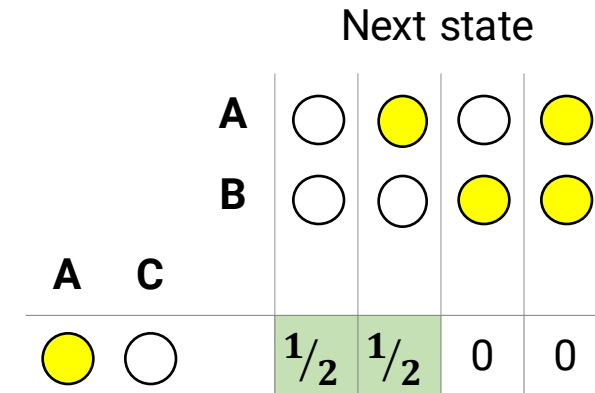 | 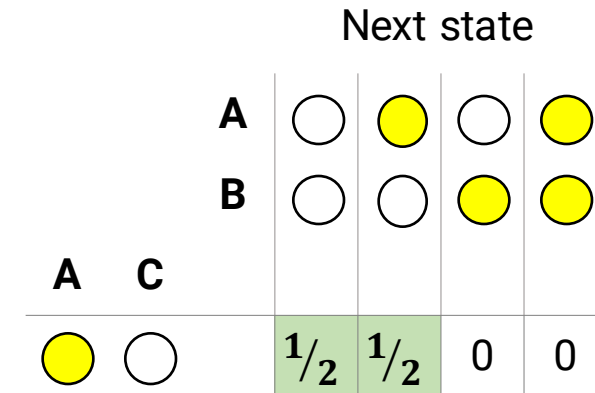 |
| A | C | 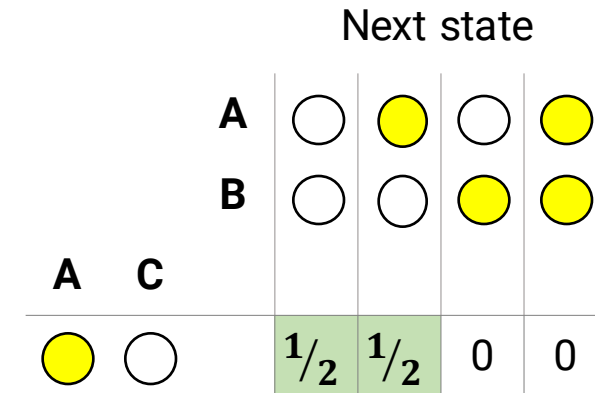 | 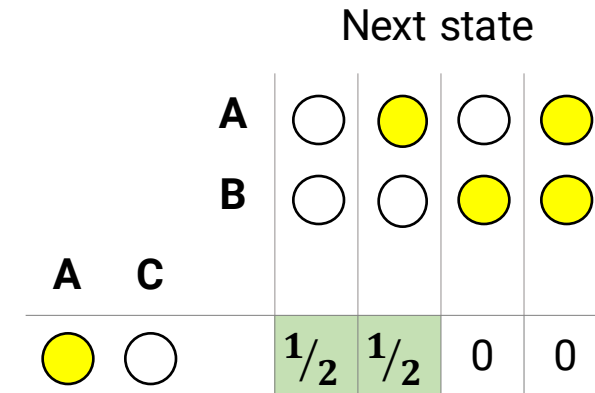 | 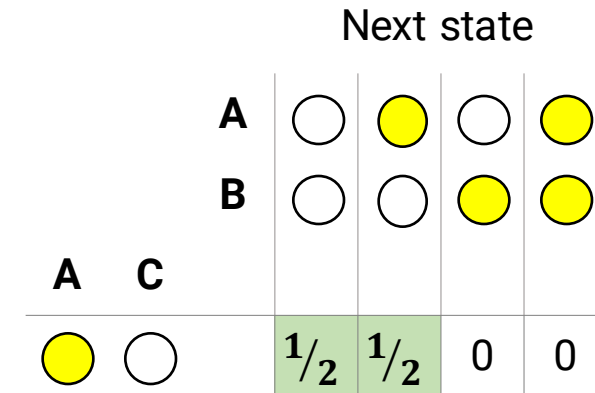 | 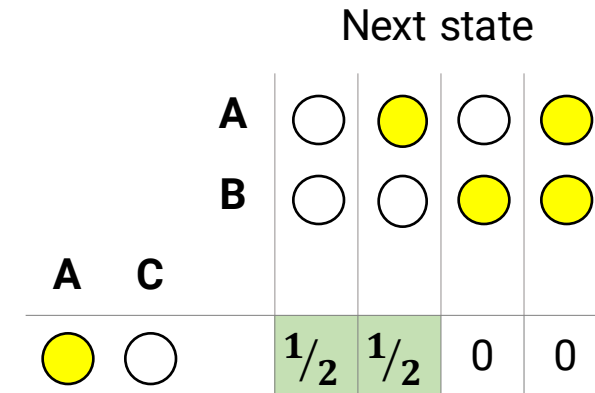 |
|   |   | $\frac{1}{2}$                                                                       | $\frac{1}{2}$                                                                       | 0                                                                                   | 0                                                                                   |

Integration and reducibility:  
**An example of a reducible mechanism**

- Now we take the tensor product to obtain a repertoire over the original purview, **ABC**:

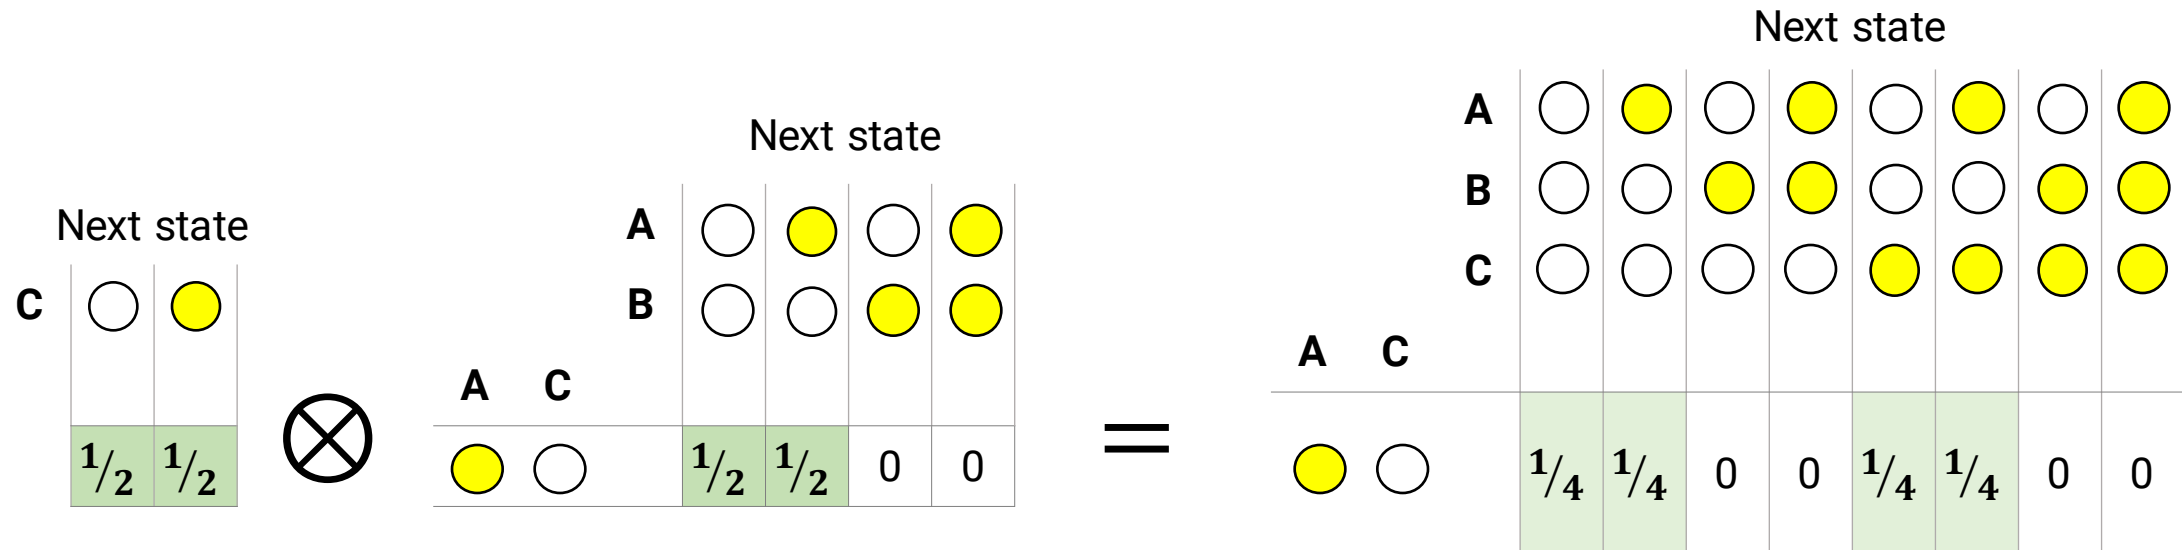



Integration and reducibility:

## An example of a reducible mechanism

- And we see that we've recovered the original effect repertoire of **AC** over **ABC**
- This means that the repertoire of  $\frac{AC}{ABC}$  can be “factored” into  $\frac{AC}{AB}$  and  $\frac{\emptyset}{C}$
- In other words, the repertoire of **AC** over **ABC** is **reducible** to that of **AC** over **AB**
- There is no information gained by including **C** in the purview

|   |   | Next state |   |     |     |   |   |     |     |   |
|---|---|------------|---|-----|-----|---|---|-----|-----|---|
| A | C | A          | B | C   | A   | B | C | A   | B   | C |
|   |   | ○          | ● | ○   | ●   | ○ | ● | ○   | ●   |   |
|   |   | ○          | ○ | ●   | ●   | ○ | ○ | ●   | ●   |   |
|   |   | ○          | ○ | ○   | ○   | ● | ● | ●   | ●   |   |
| A | C |            |   |     |     |   |   |     |     |   |
|   |   | ●          | ○ | 1/4 | 1/4 | 0 | 0 | 1/4 | 1/4 | 0 |

**Un-partitioned**

|   |   | Next state |   |               |               |   |   |               |               |   |
|---|---|------------|---|---------------|---------------|---|---|---------------|---------------|---|
| A | C | A          | B | C             | A             | B | C | A             | B             | C |
|   |   | ○          | ● | ○             | ●             | ○ | ● | ○             | ●             |   |
|   |   | ○          | ○ | ●             | ●             | ○ | ○ | ●             | ●             |   |
|   |   | ○          | ○ | ○             | ○             | ● | ● | ●             | ●             |   |
| A | C |            |   |               |               |   |   |               |               |   |
|   |   | ●          | ○ | $\frac{1}{4}$ | $\frac{1}{4}$ | 0 | 0 | $\frac{1}{4}$ | $\frac{1}{4}$ | 0 |

**Partitioned**

Integration and reducibility:

## Minimum information partition and “small-phi”

- However, note that we can try to factor the repertoire in many different ways:

$$\frac{\emptyset}{A} \times \frac{AC}{BC}$$

$$\frac{\emptyset}{B} \times \frac{AC}{AC}$$

$$\frac{\emptyset}{AB} \times \frac{AC}{C}$$

$$\frac{\emptyset}{C} \times \frac{AC}{BC}$$

$$\frac{\emptyset}{AC} \times \frac{AC}{B}$$

$$\frac{\emptyset}{BC} \times \frac{AC}{A}$$

$$\frac{\emptyset}{ABC} \times \frac{AC}{\emptyset}$$

$$\frac{A}{\emptyset} \times \frac{C}{ABC}$$

$$\frac{A}{A} \times \frac{C}{BC}$$

$$\frac{A}{B} \times \frac{C}{AC}$$

$$\frac{A}{AB} \times \frac{C}{C}$$

$$\frac{A}{C} \times \frac{C}{BC}$$

$$\frac{A}{AC} \times \frac{C}{B}$$

$$\frac{A}{BC} \times \frac{C}{A}$$

$$\frac{A}{ABC} \times \frac{C}{\emptyset}$$

Integration and reducibility:

## **Minimum information partition and “small-phi”**

- However, note that we can try to factor the repertoire in many different ways:
- We calculate the repertoire for each of these possible partitions
- Then we compare each of the partitioned repertoires to the original repertoire by calculating the distance between them
- PyPhi supports various distance measures, but we'll explore the Earth Mover's Distance (EMD) used in IIT 3.0

# Integration and reducibility: The Earth Mover's Distance

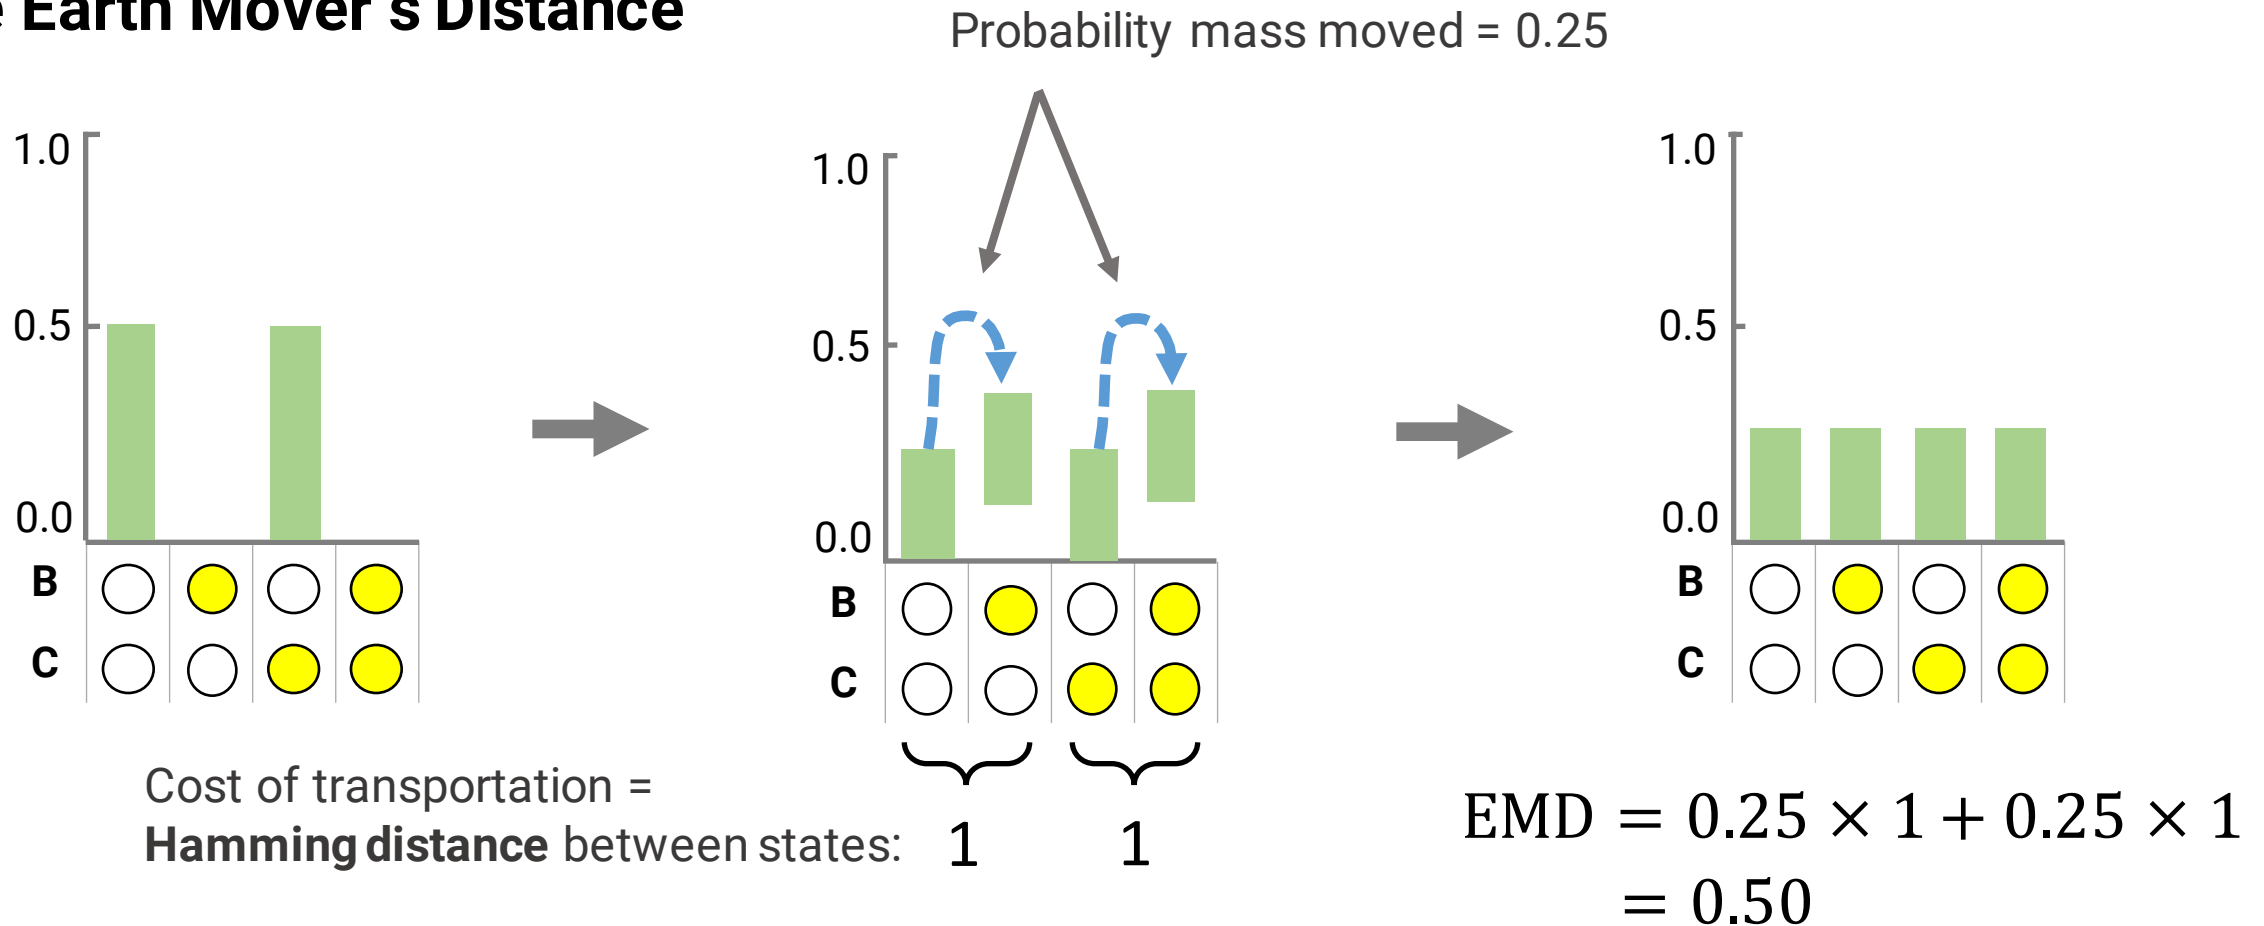

The EMD is the minimum cost of transforming one pile of “dirt” into the other, where the cost is the **amount of dirt moved** multiplied by the **distance it travels**

Integration and reducibility:

## **Minimum information partition and “small-phi”**

- The partition corresponding to the minimal distance from the original repertoire is the **minimum information partition**
- It's the partition that results in the smallest loss of information
- The EMD between the unpartitioned repertoire and the repertoire of the MIP quantifies **how irreducible** the unpartitioned repertoire is
- This quantity is called **integrated information**, denoted  $\varphi$  (“small-phi”), because it's the information that is contained in the repertoire *by virtue of considering the mechanism as an integrated whole*

# Outline

- Elements, states, and the TPM
- Background conditions
- Cause-effect repertoires
- Integrated mechanisms:  $\varphi$
- **Concepts and cause-effect structures**
- Integrated systems:  $\Phi$
- Complexes

Integration and reducibility:

## Maximally-irreducible cause-effect repertoire of mechanism ABC

Purview

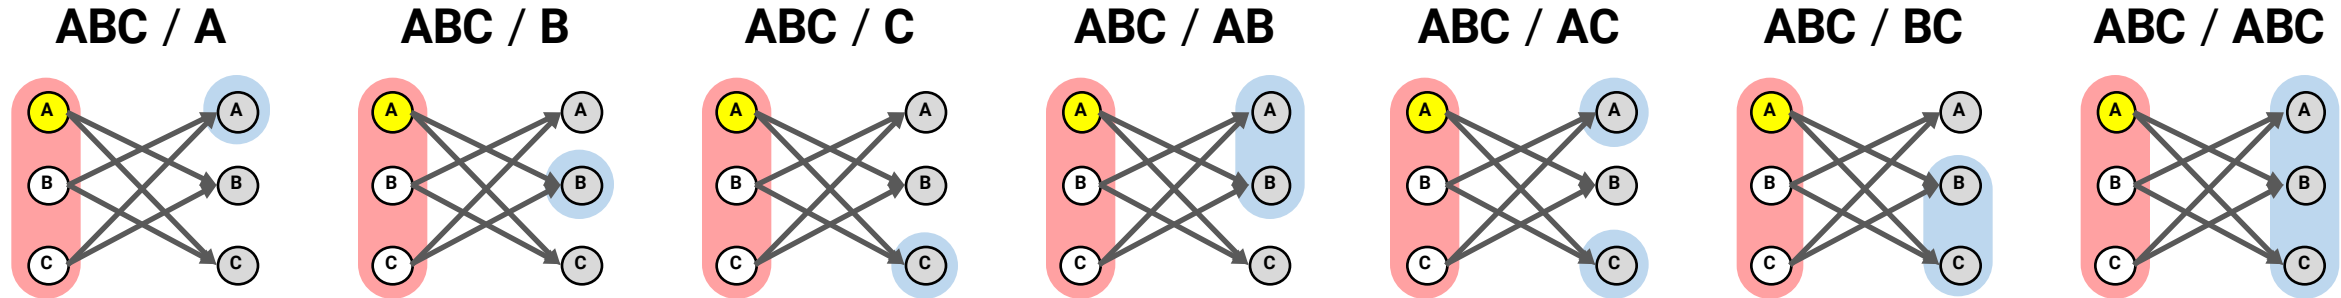

For a given candidate mechanism, we can find the cause and effect repertoires over all possible purviews (the power set of the system)

Integration and reducibility:

## Maximally-irreducible cause-effect repertoire of mechanism ABC

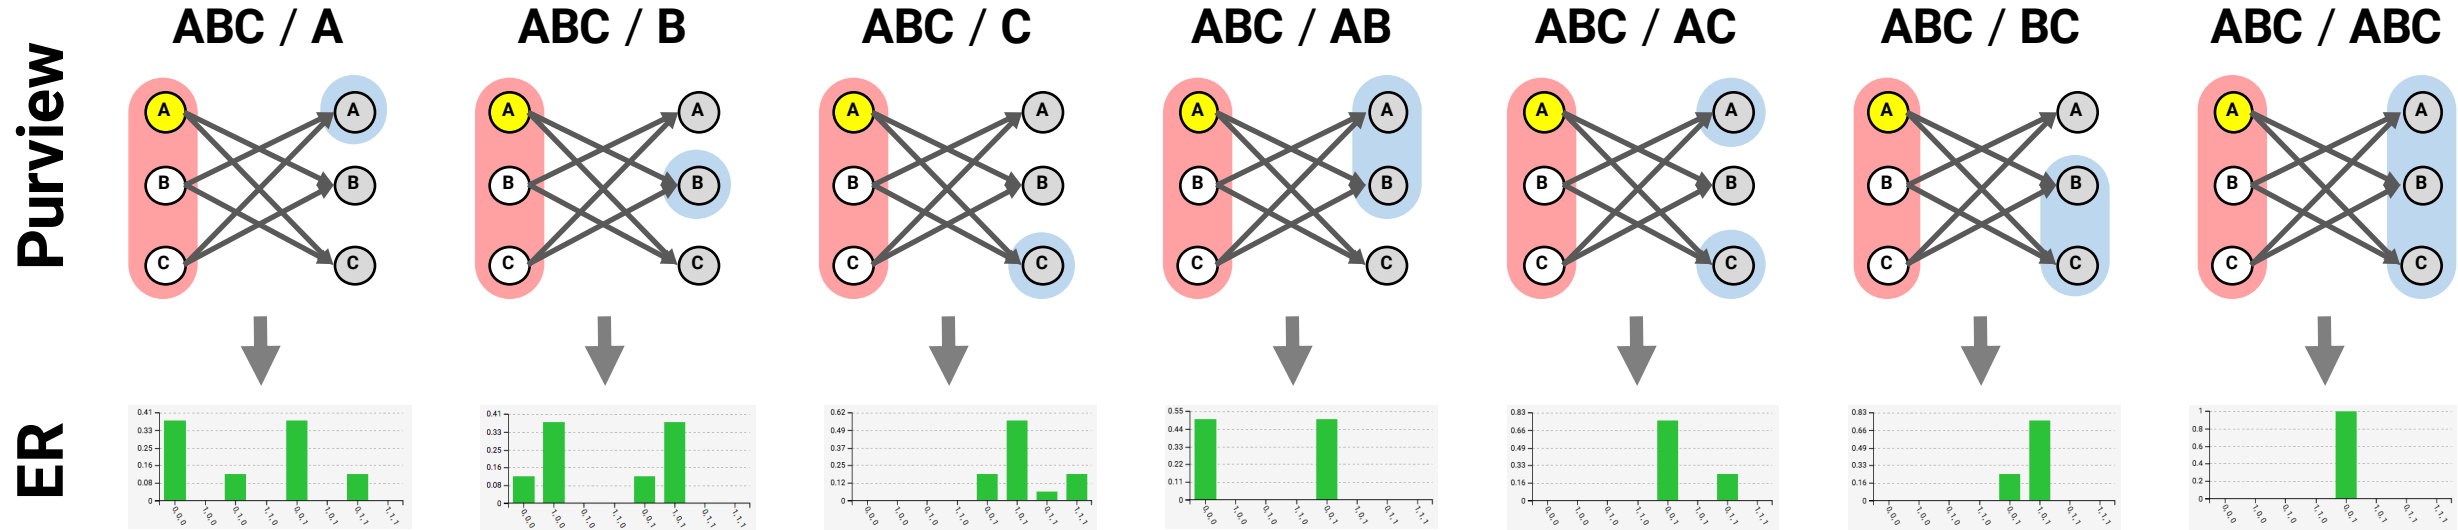

For a given candidate mechanism, we can find the cause and effect repertoires over all possible purviews (the power set of the system)



Integration and reducibility:

## Maximally-irreducible cause-effect repertoire of mechanism ABC

Purview

ABC / A

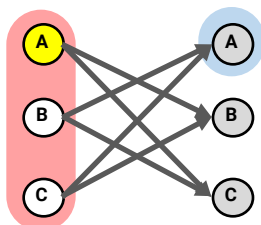

ABC / B

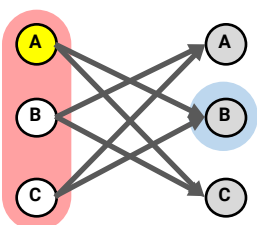

ABC / C

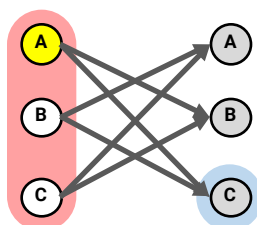

ABC / AB

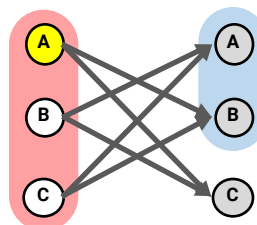

ABC / AC

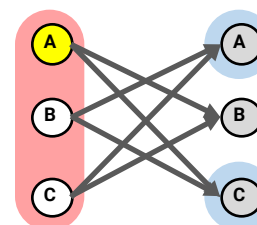

ABC / BC

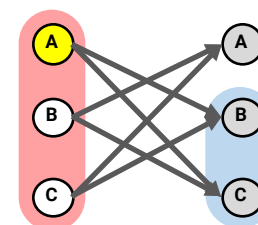

ABC / ABC

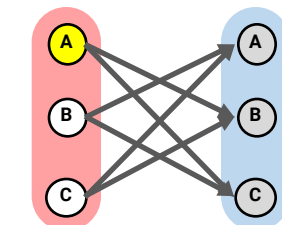

ER

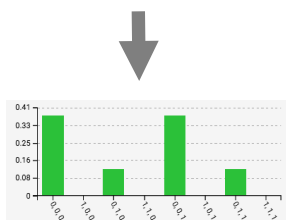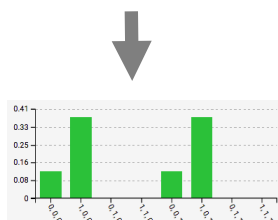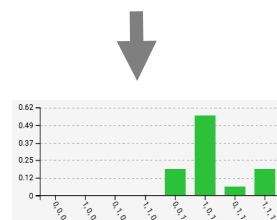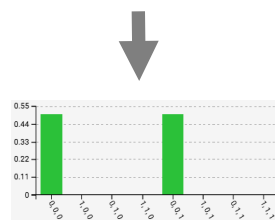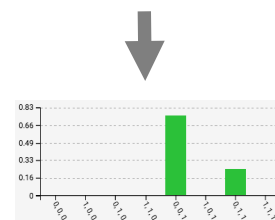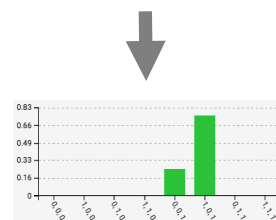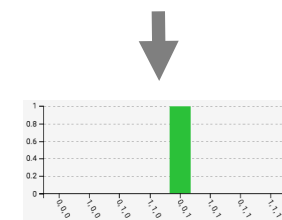

MIP

$$\frac{A}{\emptyset} \times \frac{BC}{A}$$

$$\frac{A}{\emptyset} \times \frac{BC}{B}$$

$$\frac{C}{\emptyset} \times \frac{AB}{C}$$

$$\frac{A}{\emptyset} \times \frac{BC}{AB}$$

$$\frac{\emptyset}{C} \times \frac{ABC}{A}$$

$$\frac{AB}{C} \times \frac{C}{B}$$

$$\frac{\emptyset}{B} \times \frac{ABC}{AC}$$

$\varphi$

$$\varphi = 0$$

$$\varphi = 0$$

$$\varphi = 0$$

$$\varphi = 0$$

$$\varphi = 0.5$$

$$\varphi = 0$$

$$\varphi = 0.25$$

Then we can find the MIP and  $\varphi$  value for each repertoire

Integration and reducibility:

## Maximally-irreducible cause-effect repertoire of mechanism ABC

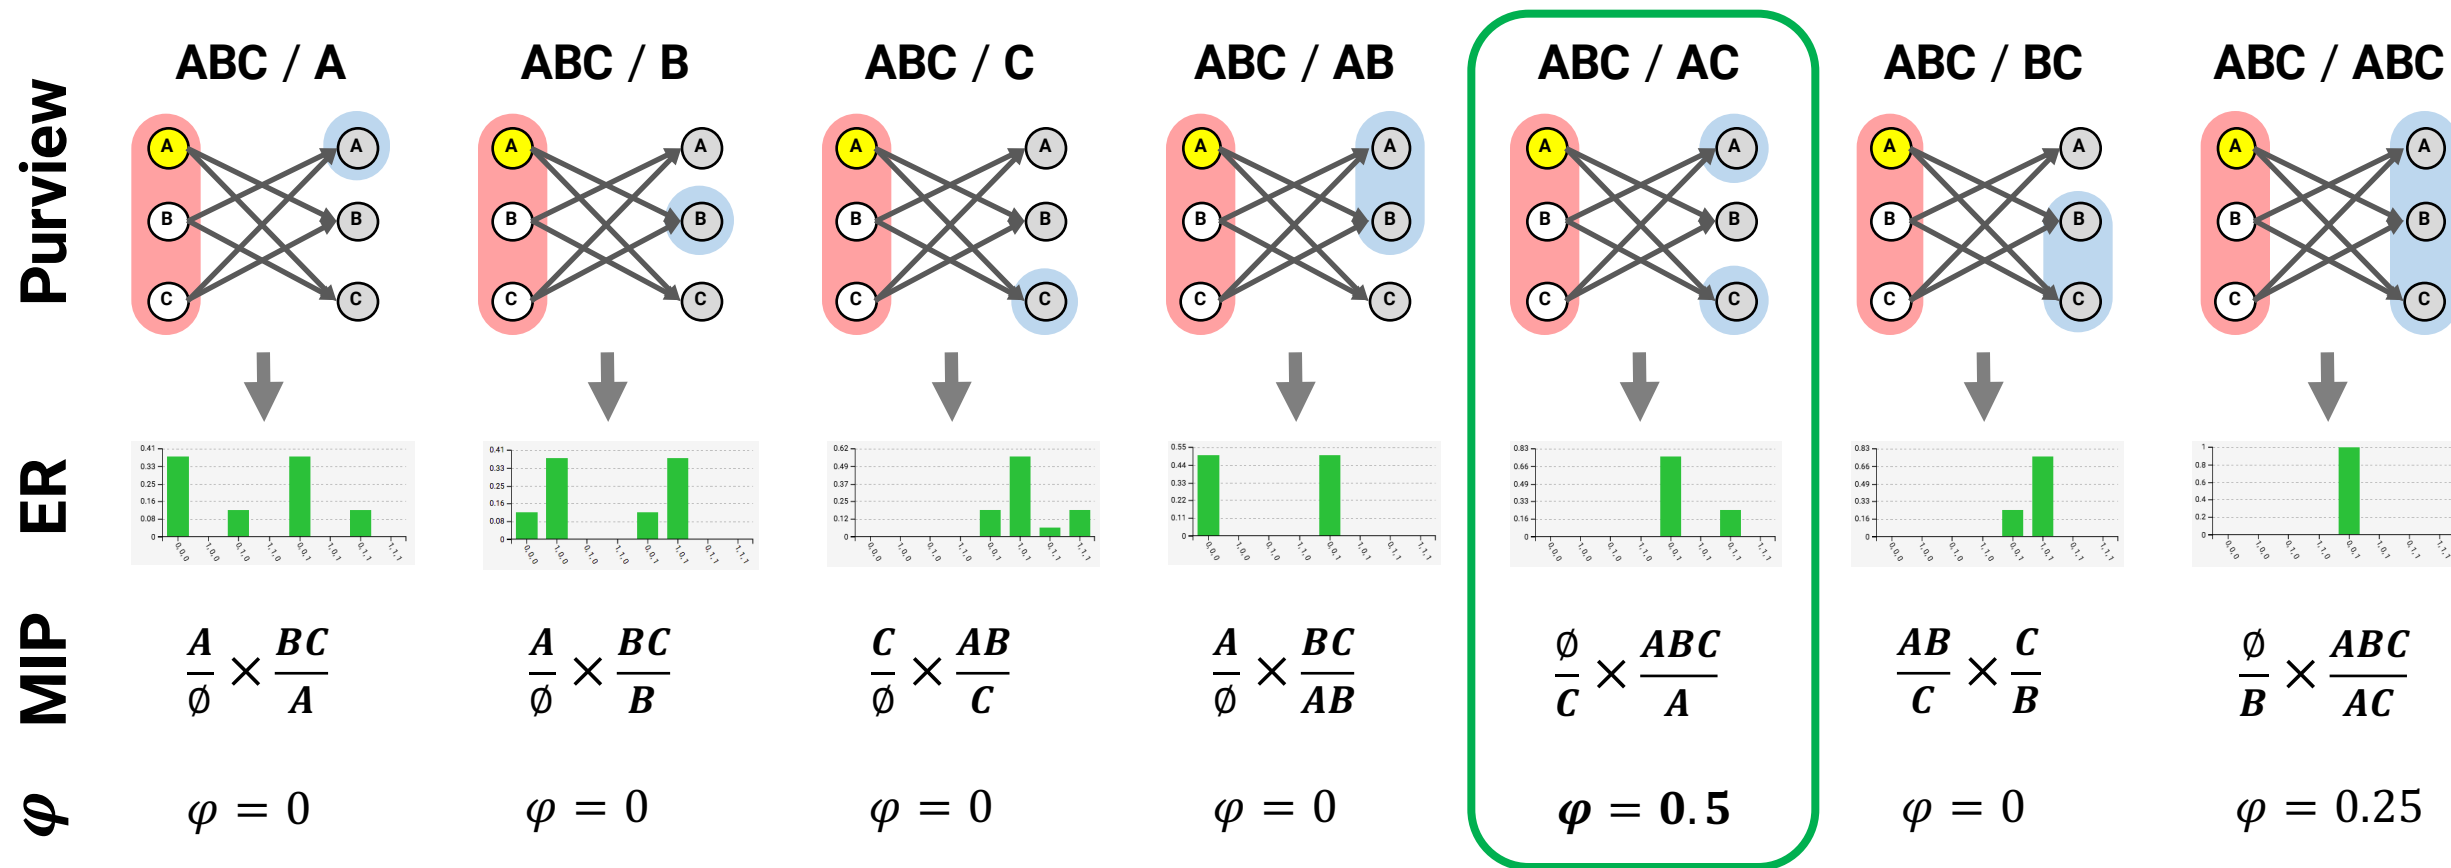

The repertoire whose MIP has the highest  $\varphi$  value ( $\varphi^{\max}$ ) is the **maximally-irreducible effect repertoire** for mechanism **ABC**  
 (the maximally-irreducible cause repertoire is defined similarly)

## Integration and reducibility: Concepts

- The maximally-irreducible cause and effect repertoires of **ABC**, and their  $\varphi_{\text{cause}}$  and  $\varphi_{\text{effect}}$  values, together form the **concept** specified by **ABC**
- The irreducibility of the concept as a whole is the minimum of its maximally-irreducible cause and effect:

$$\varphi = \min(\varphi_{\text{cause}}, \varphi_{\text{effect}})$$

### Concept specified by mechanism **ABC**

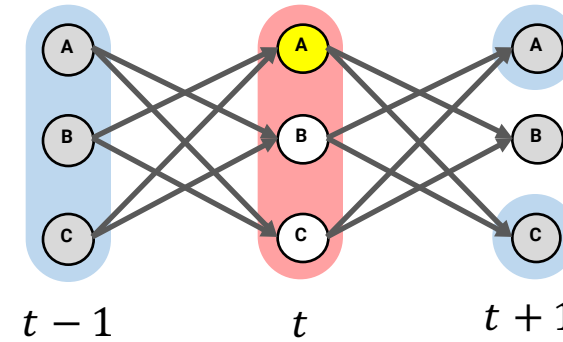

#### ABC / ABC

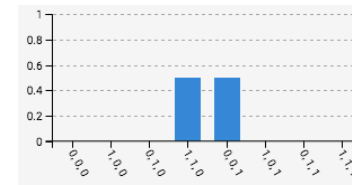

$$\frac{A}{\emptyset} \times \frac{BC}{ABC}$$

$$\varphi_{\text{cause}} = 0.5$$

Maximally-irreducible  
**cause** repertoire

#### ABC / AC

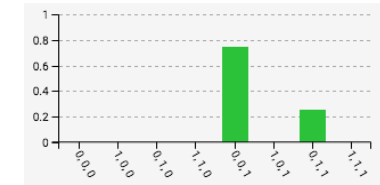

$$\frac{\emptyset}{C} \times \frac{ABC}{A}$$

$$\varphi_{\text{effect}} = 0.5$$

Maximally-irreducible  
**effect** repertoire

$$\varphi = 0.5$$

## Integration and reducibility: Cause-effect structures

- In this way we can calculate the concept specified by every candidate mechanism
- The collection of all the concepts with nonzero  $\varphi$  is the system's **cause-effect structure**:

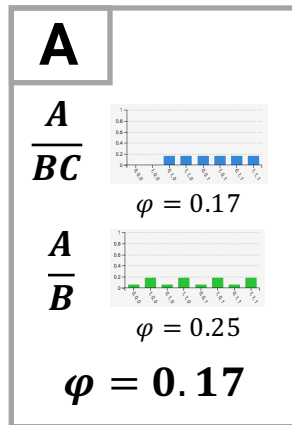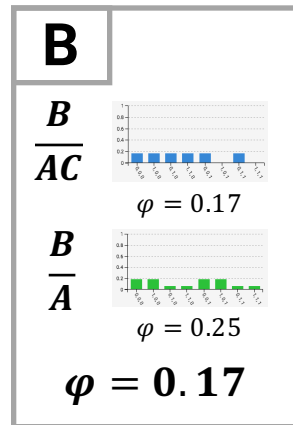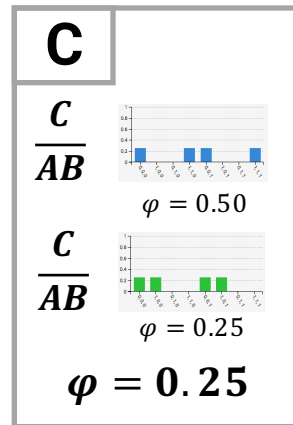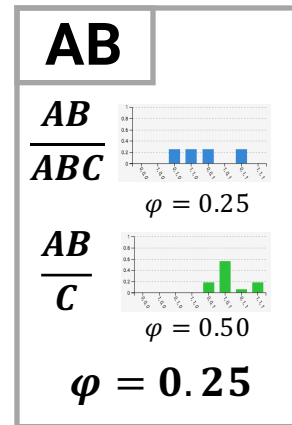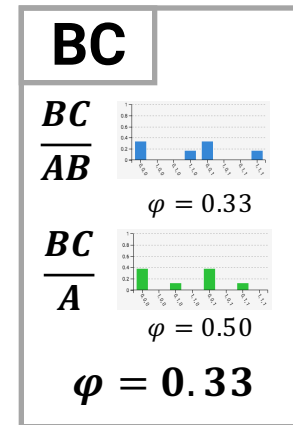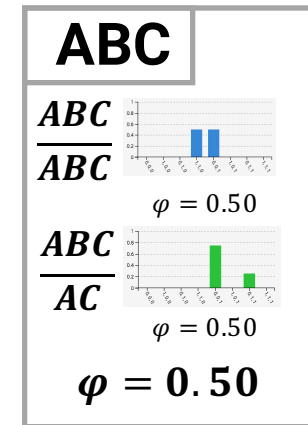

# Outline

- Elements, states, and the TPM
- Background conditions
- Cause-effect repertoires
- Integrated mechanisms:  $\varphi$
- Concepts and cause-effect structures
- **Integrated systems:  $\Phi$**
- Complexes

Integration and reducibility:

## System-level irreducibility and system cuts

- At this point, we have assessed which subsets of elements of the candidate system exist intrinsically as integrated mechanisms with irreducible cause-effect power
- But what about the system as a whole?
- We can determine whether our candidate system is an integrated, irreducible entity using the same general scheme as when calculating  $\varphi$

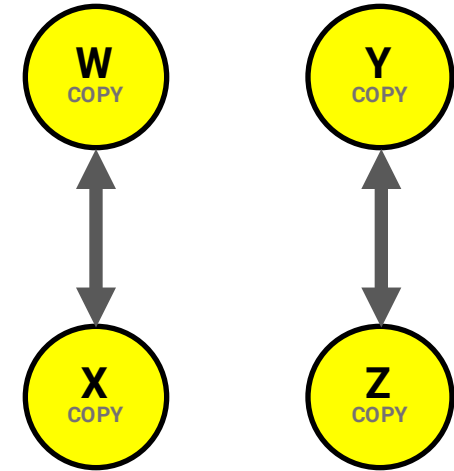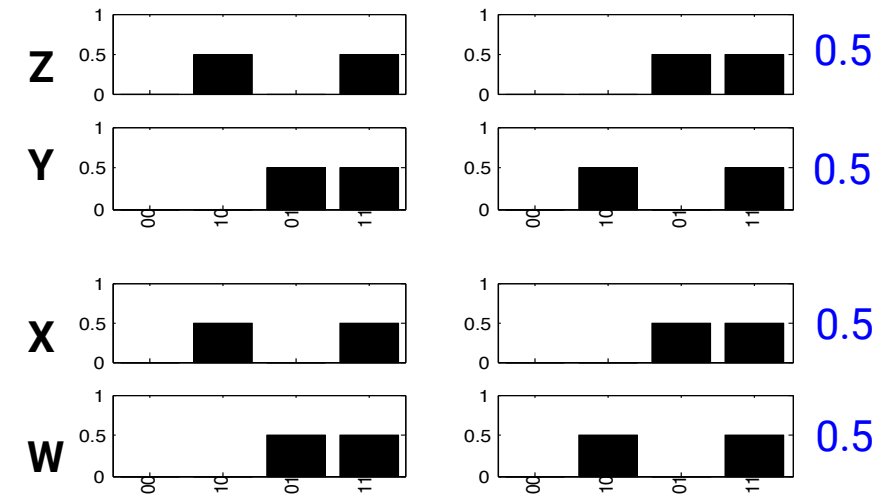

Integration and reducibility:  
**System-level irreducibility and system cuts**

- The idea is to cut the system into two groups of elements, and remove the causal link from the first group to the second (a **unidirectional cut**)
- Then we can see whether the cut “makes a difference”
- If it doesn't, then the system reduces to the two parts separated by the cut

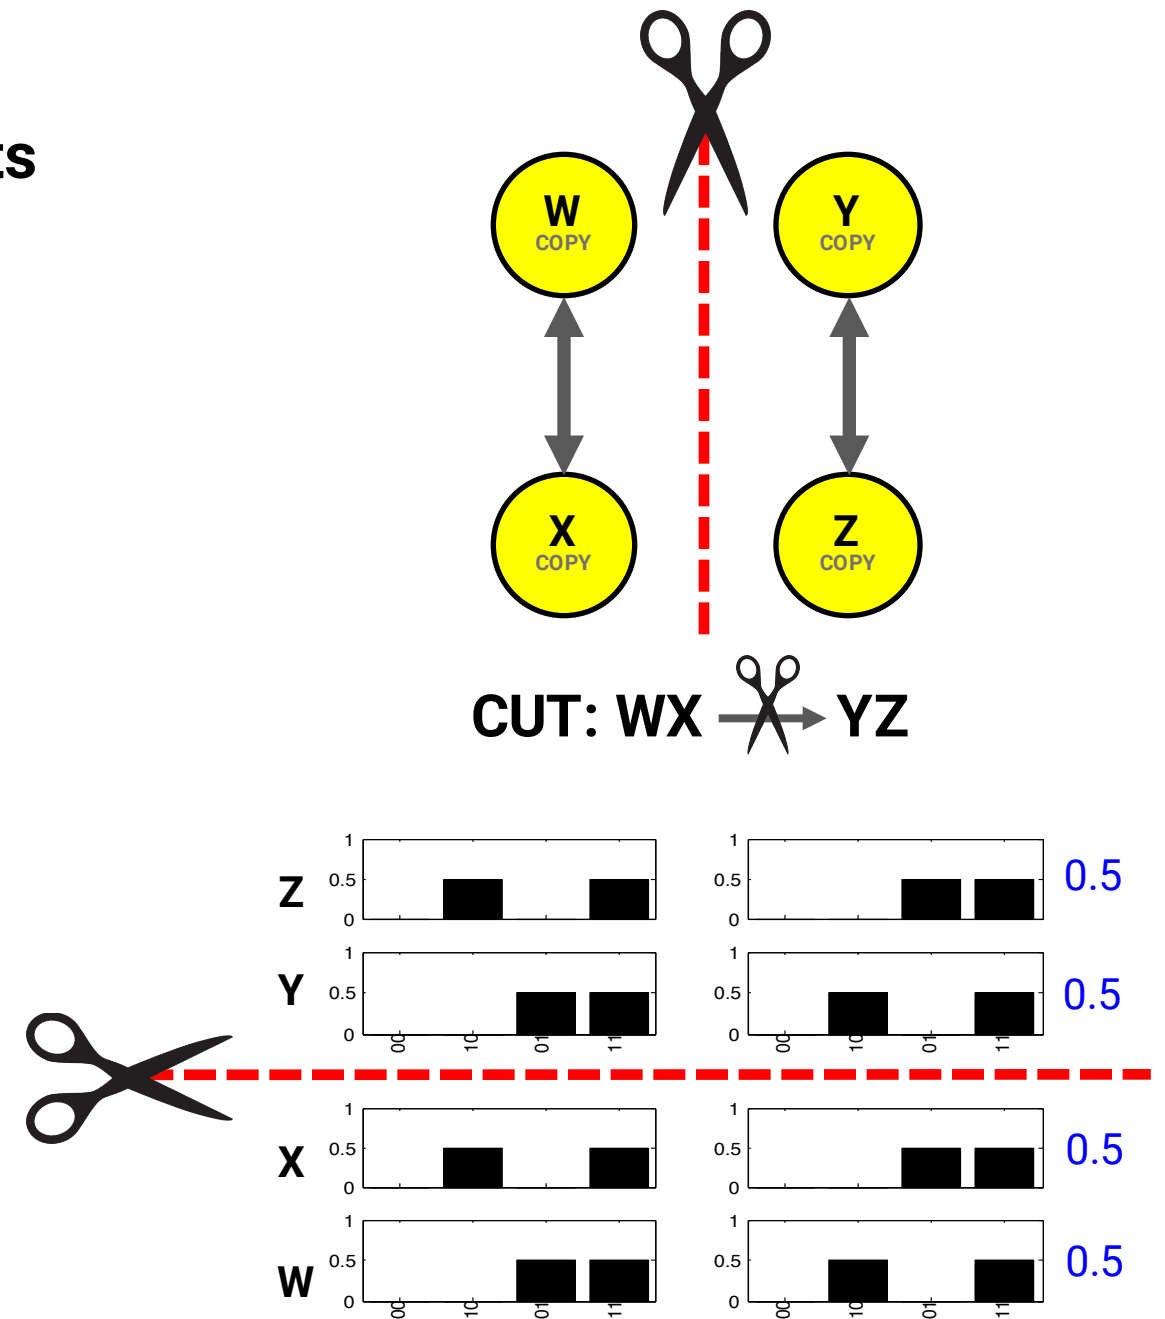

Integration and reducibility:  
**System-level irreducibility and system cuts**

- Here, we can see immediately that the cut makes no difference to the system
- The cause-effect structure is unchanged by the cut
- **WXYZ** reduces to **WX** and **YZ**

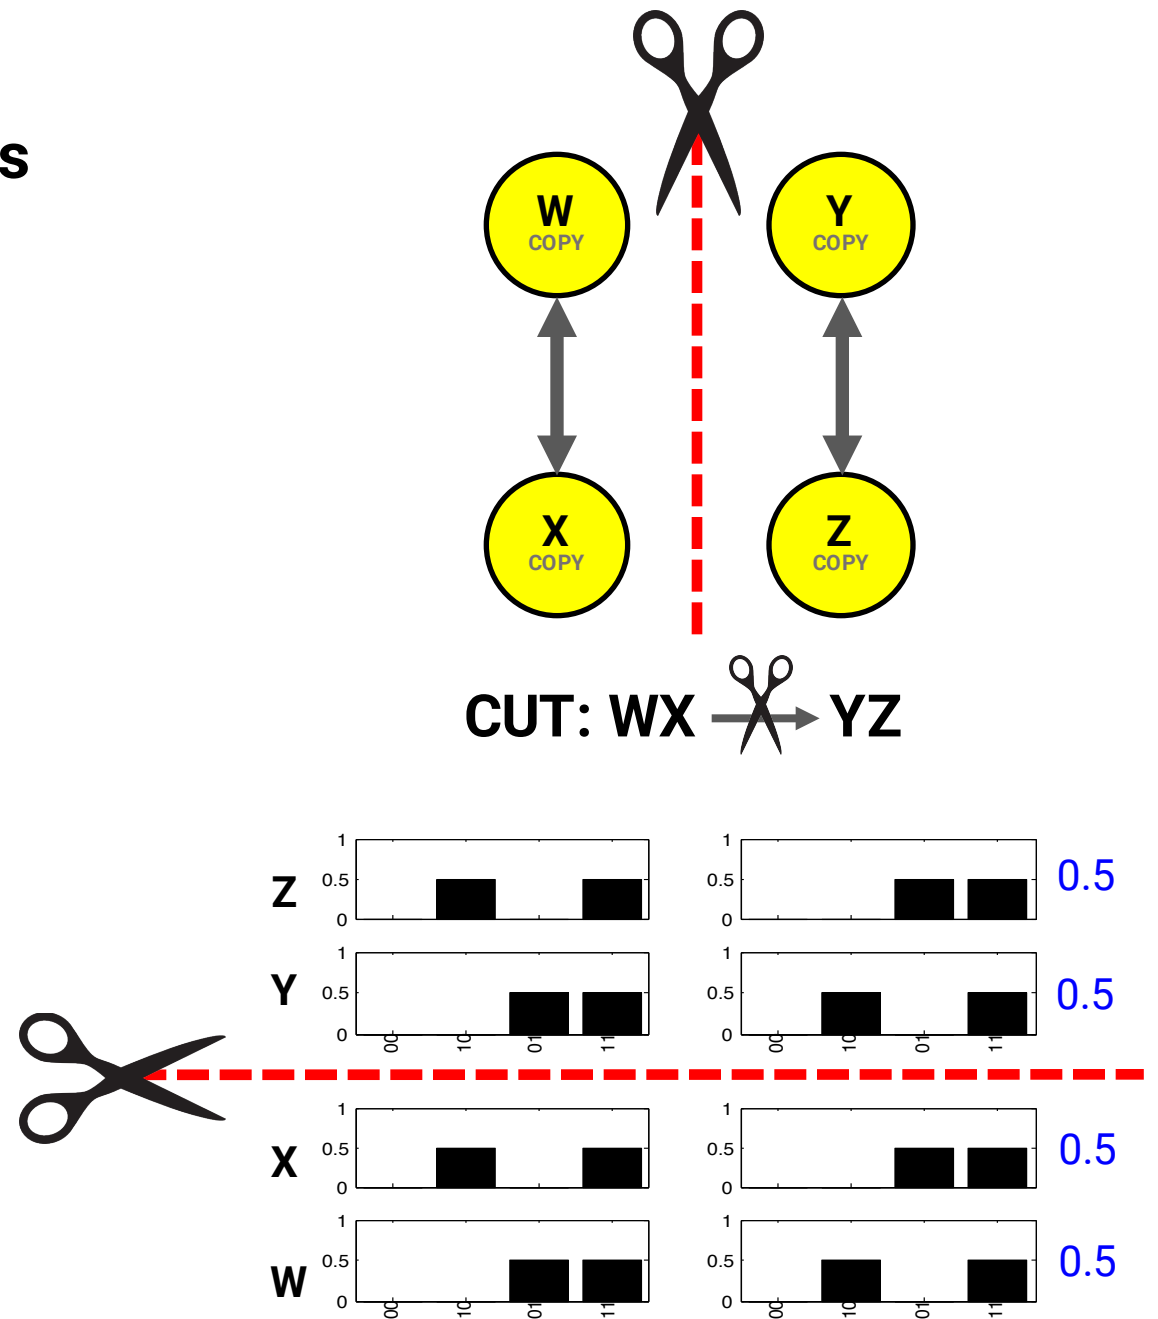



Integration and reducibility:

## System-level irreducibility and system cuts

- But what is the proper way to “remove the causal link” from one group of elements to the other when there are connections between them?
- The right way to cut a connection is to **inject noise** into it, rather than simply removing it
- In this example, the outgoing connections from **A** *independently* provide random input to elements **B** and **C**

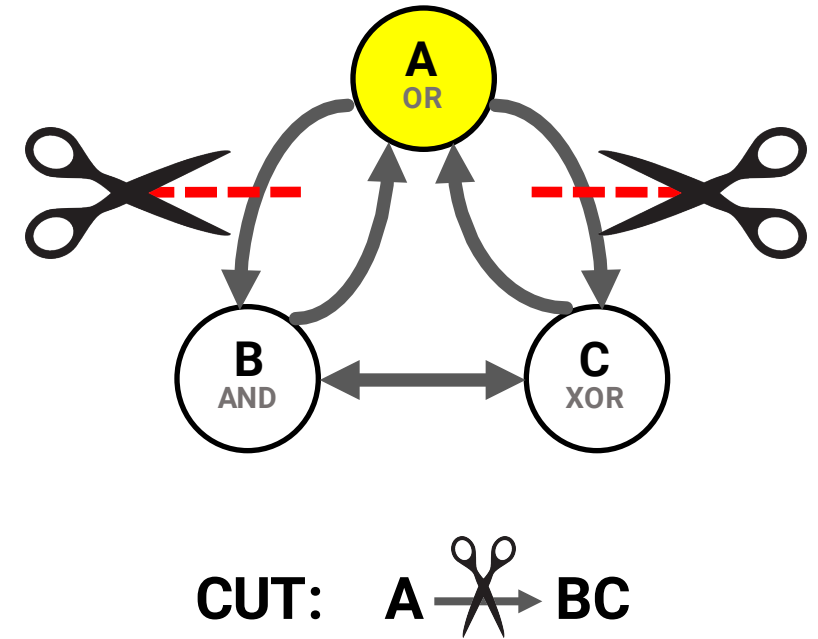

Integration and reducibility:

## **System-level irreducibility and system cuts**

- We find the TPM for each individual mechanism, and combine them to get the full TPM (again, this works because of conditional independence)
- This makes the virtual elements implicit, as usual

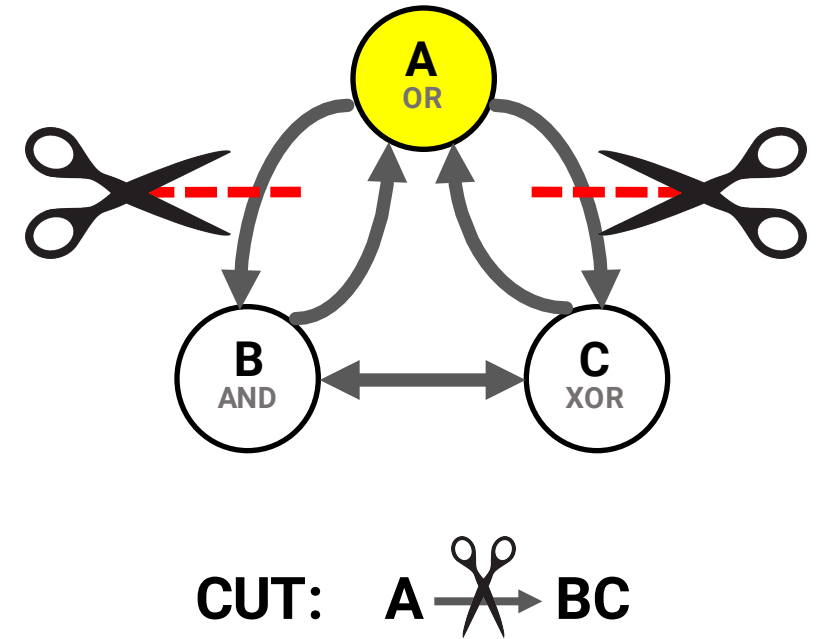

Integration and reducibility:  
**System-level irreducibility and system cuts**

Current state

|   |   | Next state |   |
|---|---|------------|---|
| B | C | A          |   |
|   |   |            |   |
| ○ | ○ | ○          | ● |

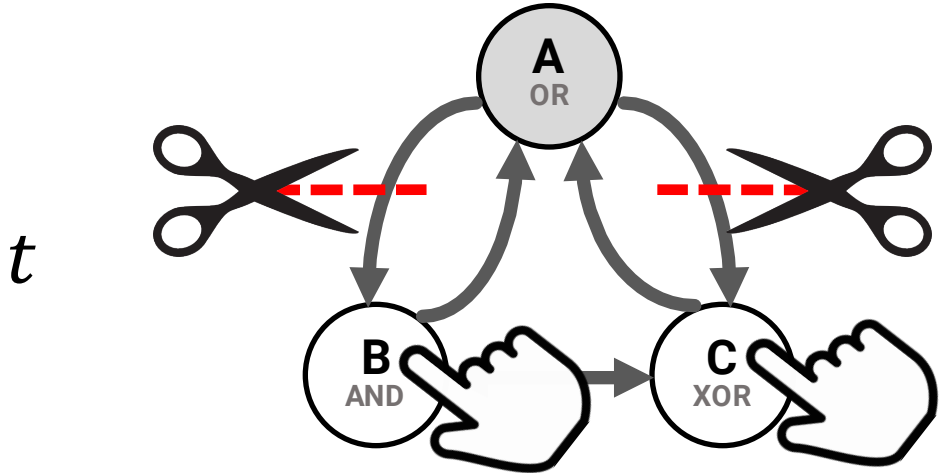

We start by finding the TPM for just **A**, which takes input from **B** and **C**

Integration and reducibility:  
**System-level irreducibility and system cuts**

|               |                                                                                                                                                                     | Next state                                                                        |                                                                                    |
|---------------|---------------------------------------------------------------------------------------------------------------------------------------------------------------------|-----------------------------------------------------------------------------------|------------------------------------------------------------------------------------|
| Current state | A                                                                                                                                                                   | 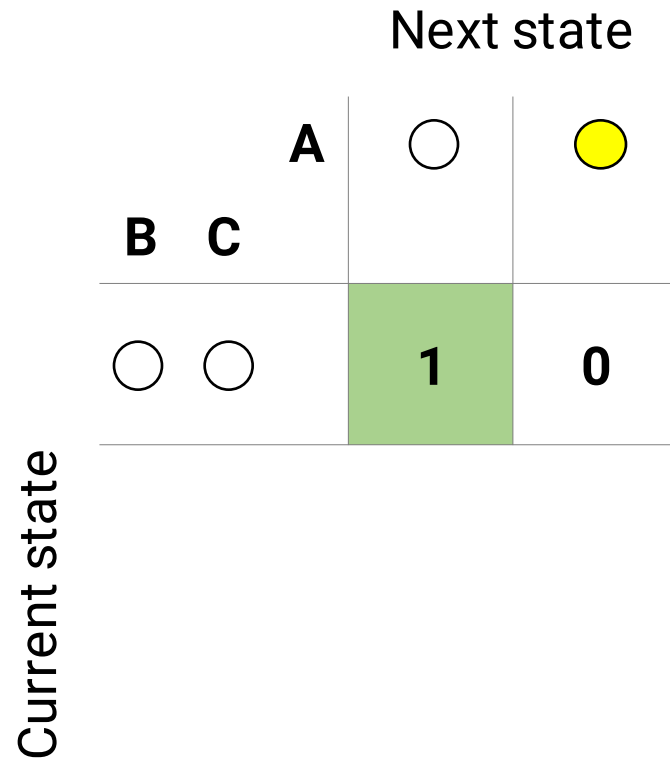 | 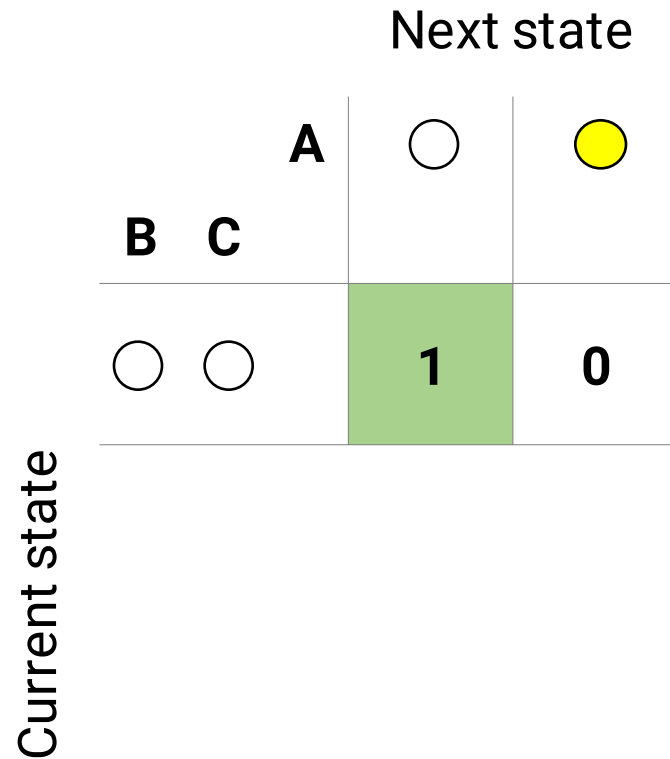 |
|               | B C                                                                                                                                                                 |                                                                                   |                                                                                    |
|               | B C                                                                                                                                                                 |                                                                                   |                                                                                    |
|               | 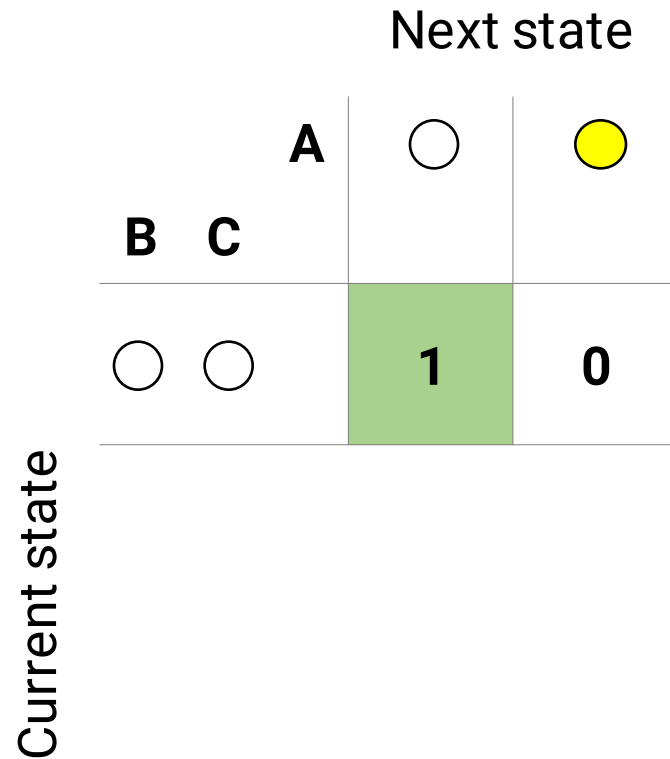 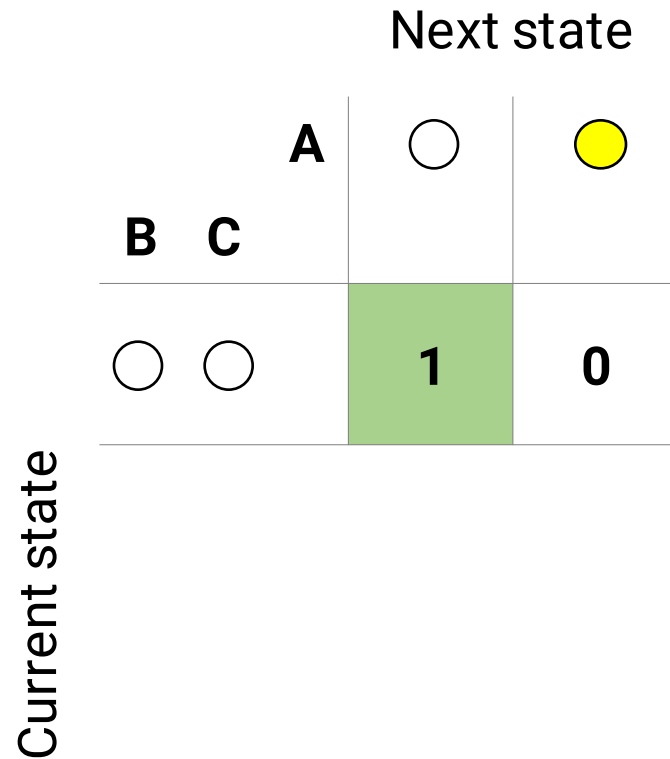 | 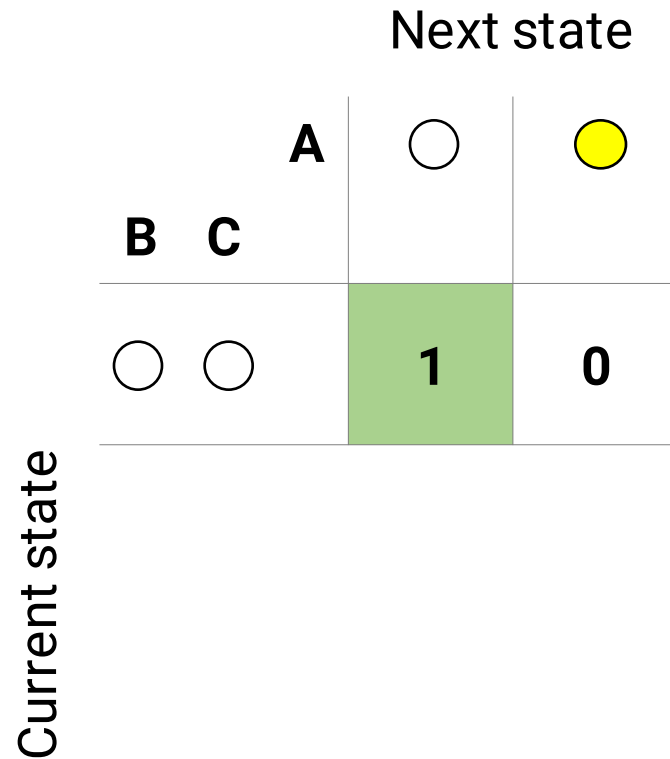 | 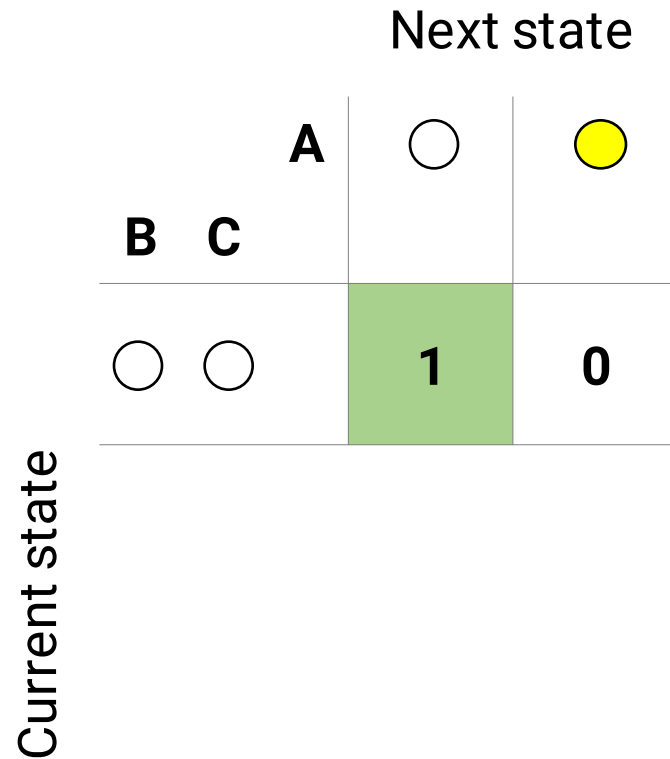 |

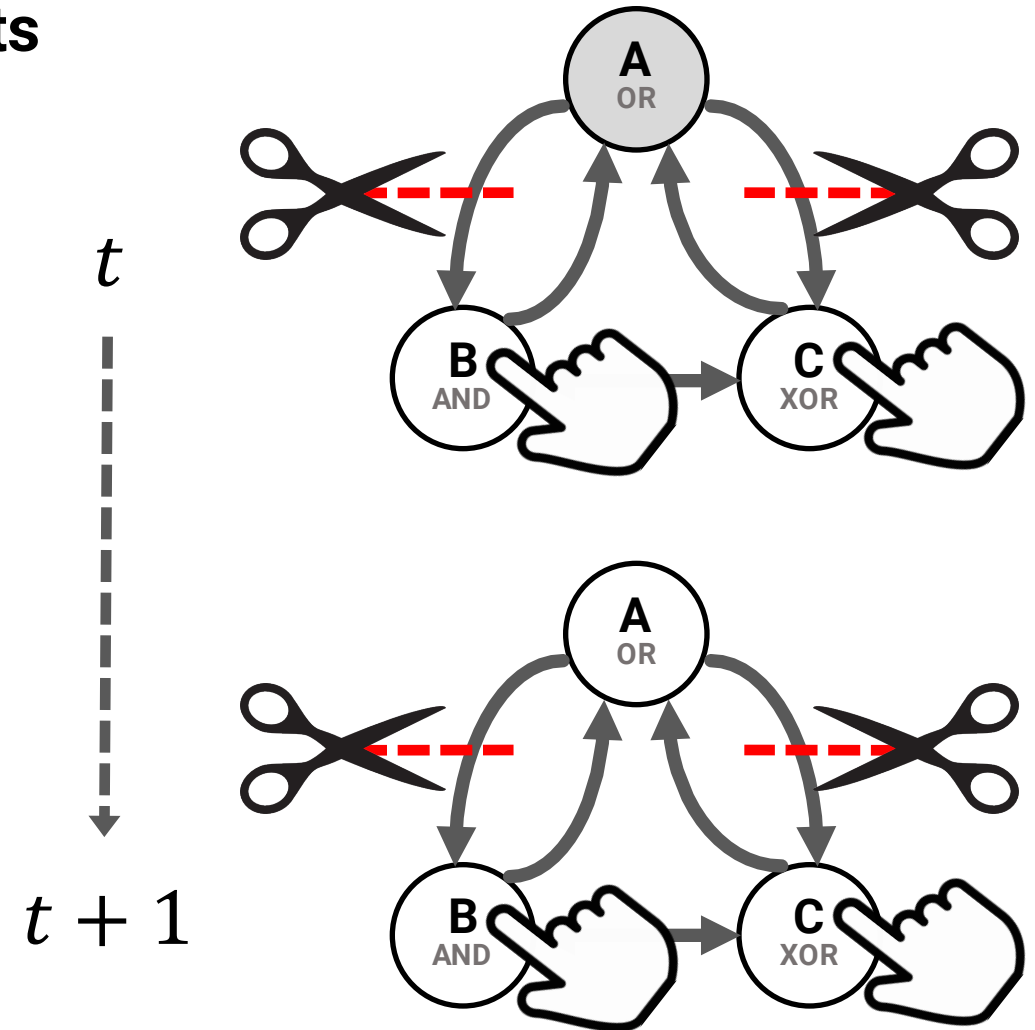

We start by finding the TPM for just **A**, which takes input from **B** and **C**

Integration and reducibility:  
**System-level irreducibility and system cuts**

|               |                                                        | Next state            |                                  |
|---------------|--------------------------------------------------------|-----------------------|----------------------------------|
| Current state | A                                                      | <input type="radio"/> | <input checked="" type="radio"/> |
|               | B C                                                    |                       |                                  |
|               | <input type="radio"/> <input type="radio"/>            | 1                     | 0                                |
|               | <input checked="" type="radio"/> <input type="radio"/> |                       |                                  |

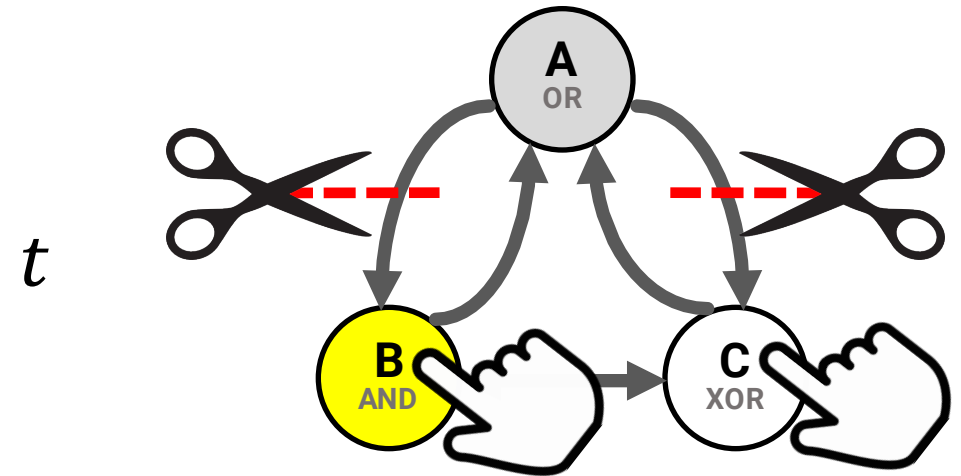

We start by finding the TPM for just **A**, which takes input from **B** and **C**

Integration and reducibility:  
**System-level irreducibility and system cuts**

|               |   | Next state |     |
|---------------|---|------------|-----|
|               |   | A          |     |
| Current state | B | C          |     |
|               | ○ | ○          | 1 0 |
|               | ● | ○          | 0 1 |

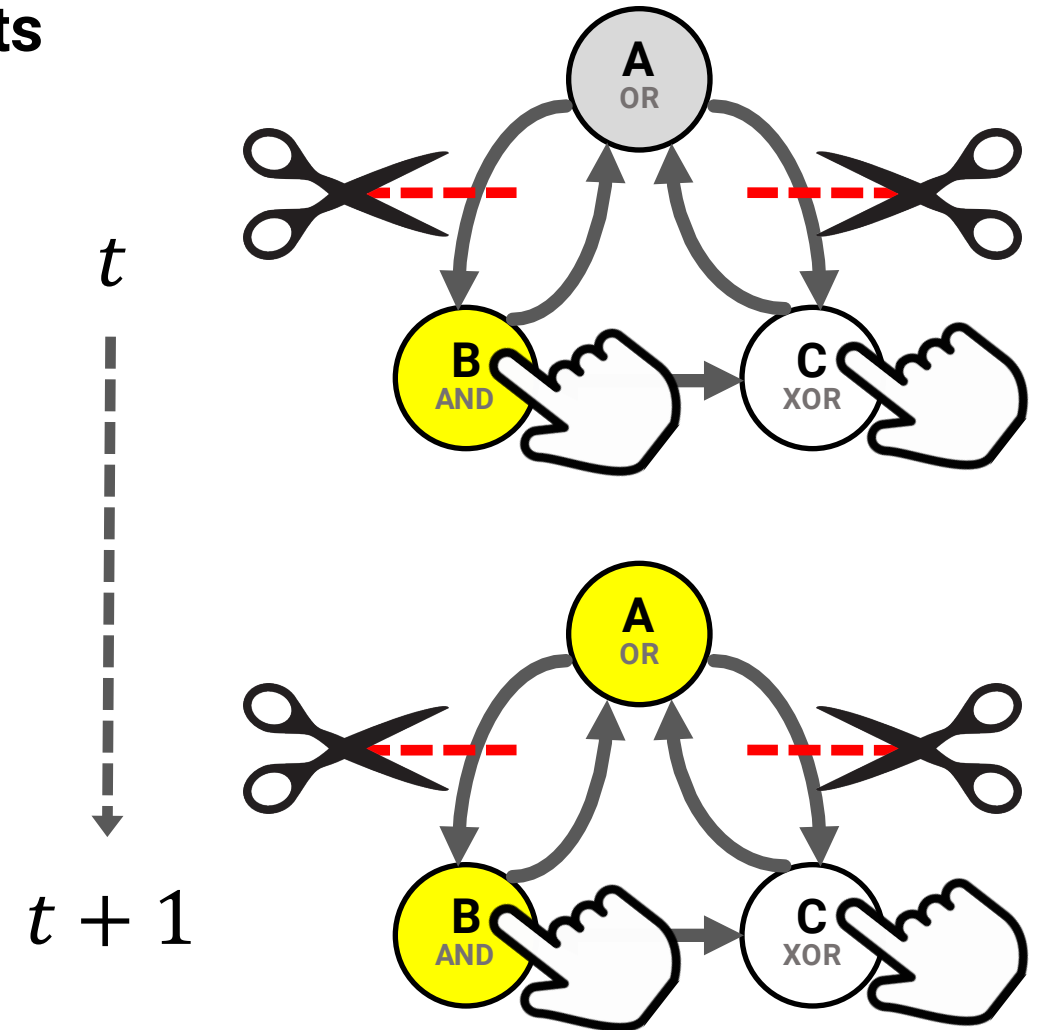

We start by finding the TPM for just **A**, which takes input from **B** and **C**

Integration and reducibility:  
**System-level irreducibility and system cuts**

|               |   |   | Next state |   |
|---------------|---|---|------------|---|
| Current state | B | C | A          |   |
|               | ○ | ○ | ○          | ● |
|               | ○ | ○ | 1          | 0 |
|               | ● | ○ | 0          | 1 |
|               | ○ | ● |            |   |

$t$

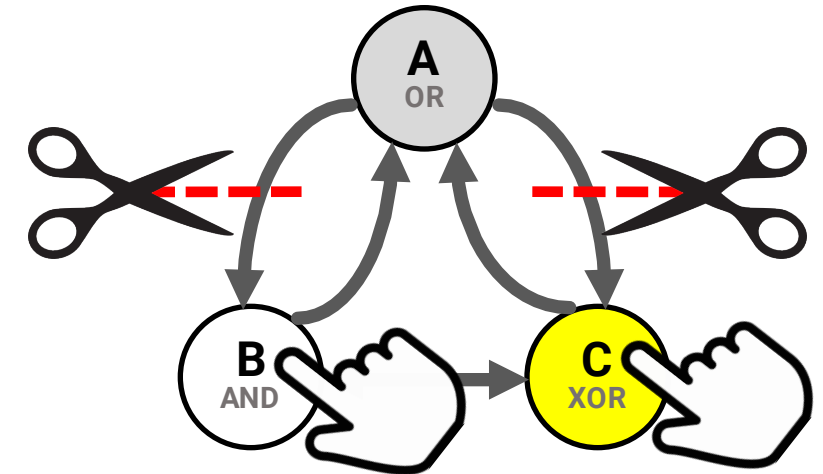

We start by finding the TPM for just **A**, which takes input from **B** and **C**

Integration and reducibility:  
**System-level irreducibility and system cuts**

|               |   |   | Next state |   |
|---------------|---|---|------------|---|
| Current state | B | C | A          |   |
|               | ○ | ○ | ○          | ● |
|               | ○ | ○ | 1          | 0 |
|               | ● | ○ | 0          | 1 |
|               | ○ | ● | 0          | 1 |

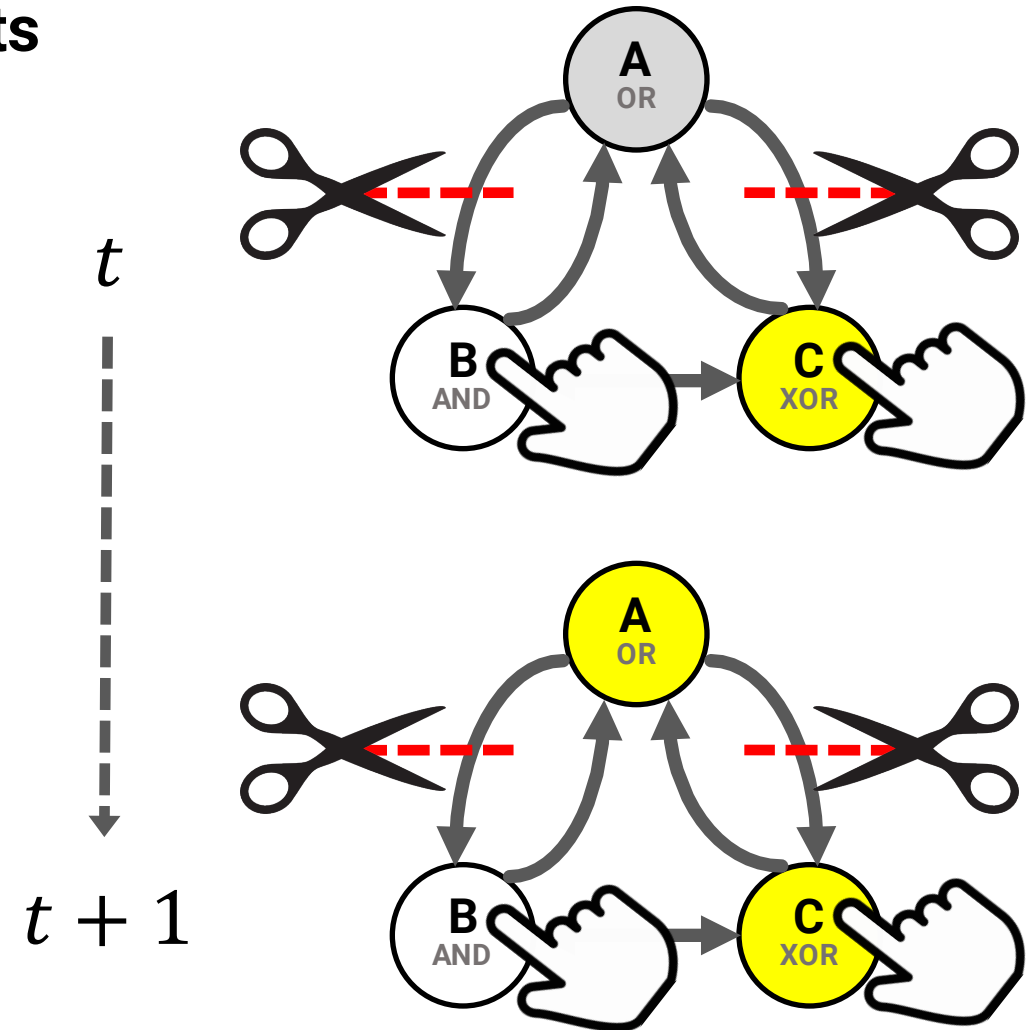

We start by finding the TPM for just **A**, which takes input from **B** and **C**



# Integration and reducibility: System-level irreducibility and system cuts

|               |     | Next state |   |
|---------------|-----|------------|---|
| Current state | A   |            |   |
|               | B C |            |   |
|               | ○ ○ | 1          | 0 |
|               | ● ○ | 0          | 1 |
|               | ○ ● | 0          | 1 |
|               | ● ● |            |   |

$t$

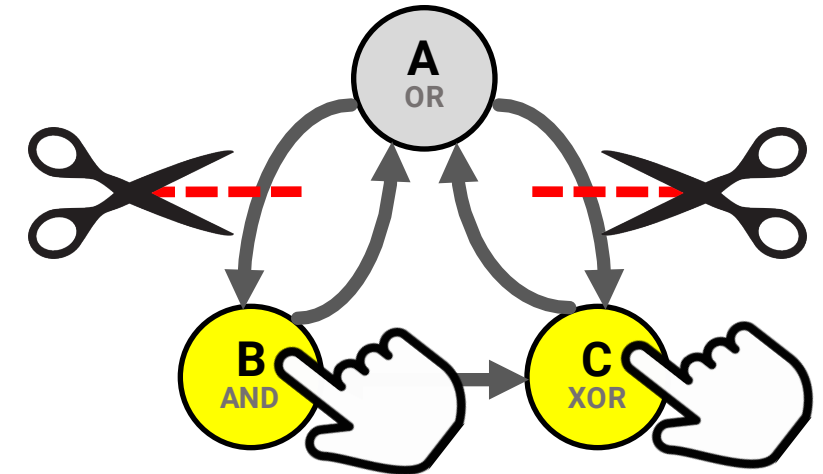

We start by finding the TPM for just **A**, which takes input from **B** and **C**

Integration and reducibility:  
**System-level irreducibility and system cuts**

|               |   |   | Next state |   |
|---------------|---|---|------------|---|
| Current state | A |   |            |   |
|               | B | C |            |   |
|               |   |   |            |   |
|               |   |   | 1          | 0 |
|               |   |   | 0          | 1 |
|               |   |   | 0          | 1 |
|               |   |   | 0          | 1 |

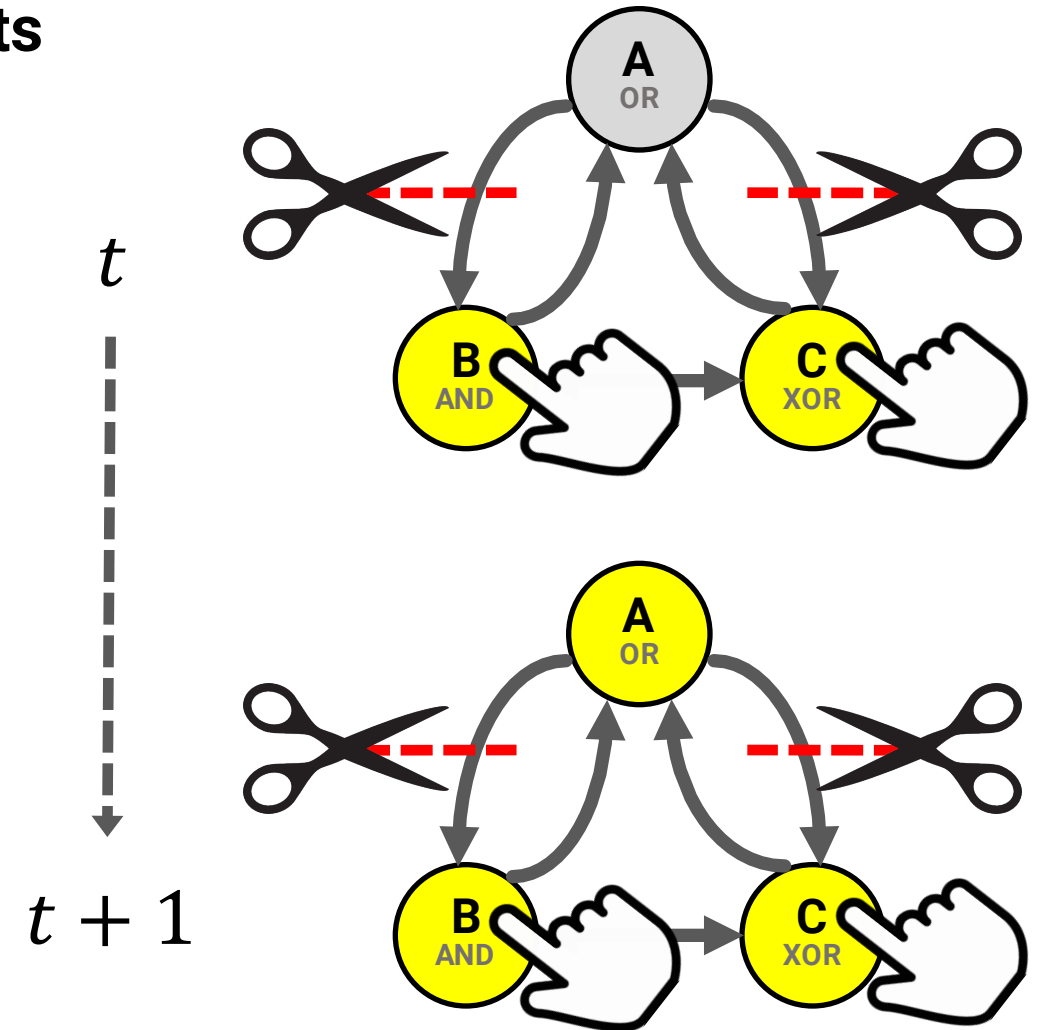

We start by finding the TPM for just **A**, which takes input from **B** and **C**

Integration and reducibility:

## System-level irreducibility and system cuts

- Next we find the TPM for **B**, which takes input from **C** and *noised* input from **A**
- We account for **A**'s noisy output by computing the TPM as if the output were not noised, then marginalizing **A** out

|               |          | Next state |   |
|---------------|----------|------------|---|
| Current state | <b>B</b> |            |   |
|               | <b>A</b> | <b>C</b>   |   |
|               | ○        | ○          | 1 |
|               | ●        | ○          | 1 |
|               | ○        | ●          | 1 |
|               | ●        | ●          | 0 |
|               |          |            |   |
|               |          | ○          | ● |
|               |          | 1          | 0 |
|               |          | 1          | 0 |
|               |          | 0          | 1 |

Integration and reducibility:

## System-level irreducibility and system cuts

- Next we find the TPM for **B**, which takes input from **C** and *noised* input from **A**
- We account for **A**'s noisy output by computing the TPM as if the output were not noised, then marginalizing **A** out

|               |                                                                                       |                                                                                       | Next state                                                                          |                                                                                     |
|---------------|---------------------------------------------------------------------------------------|---------------------------------------------------------------------------------------|-------------------------------------------------------------------------------------|-------------------------------------------------------------------------------------|
|               |                                                                                       |                                                                                       | 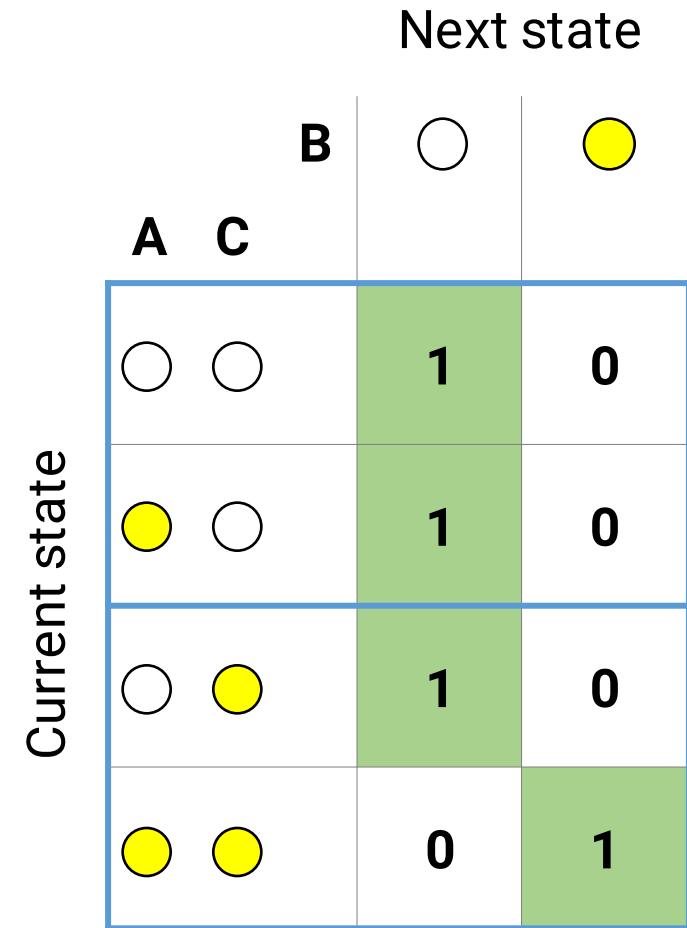 | 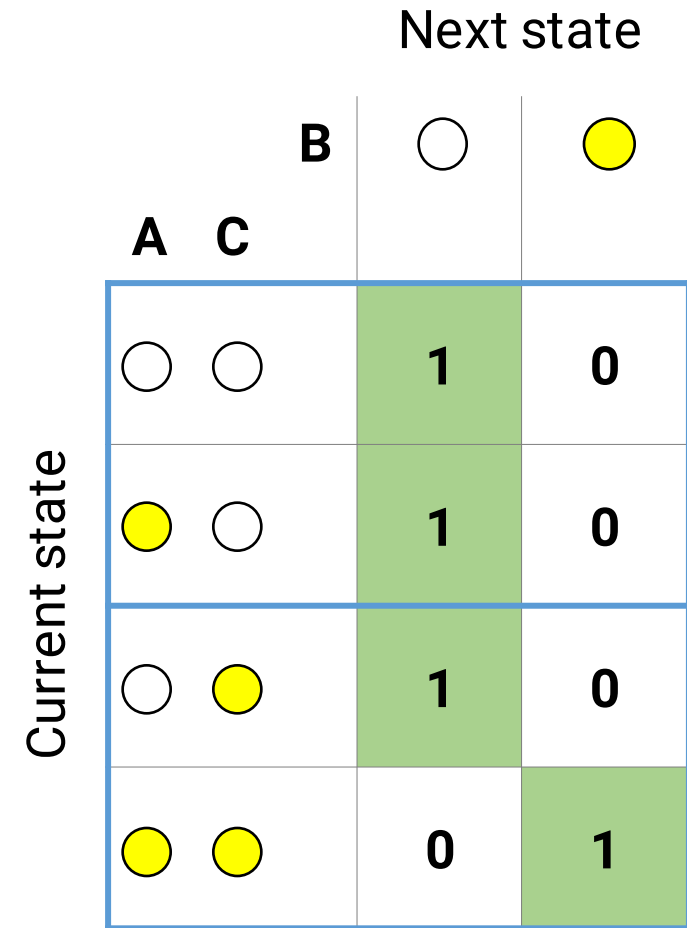 |
| Current state | A                                                                                     | C                                                                                     |                                                                                     |                                                                                     |
|               | 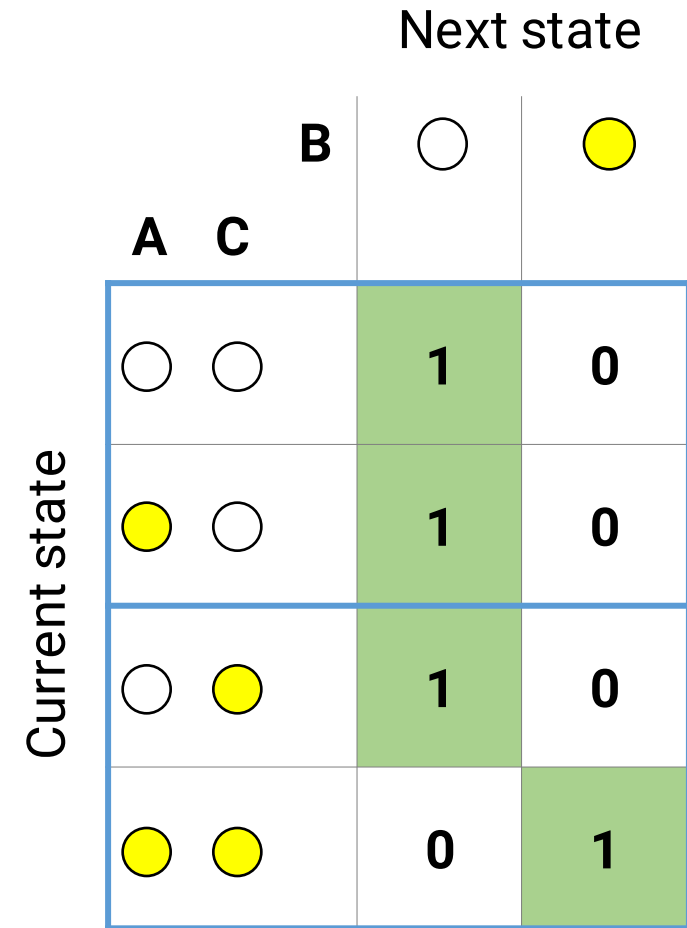   | 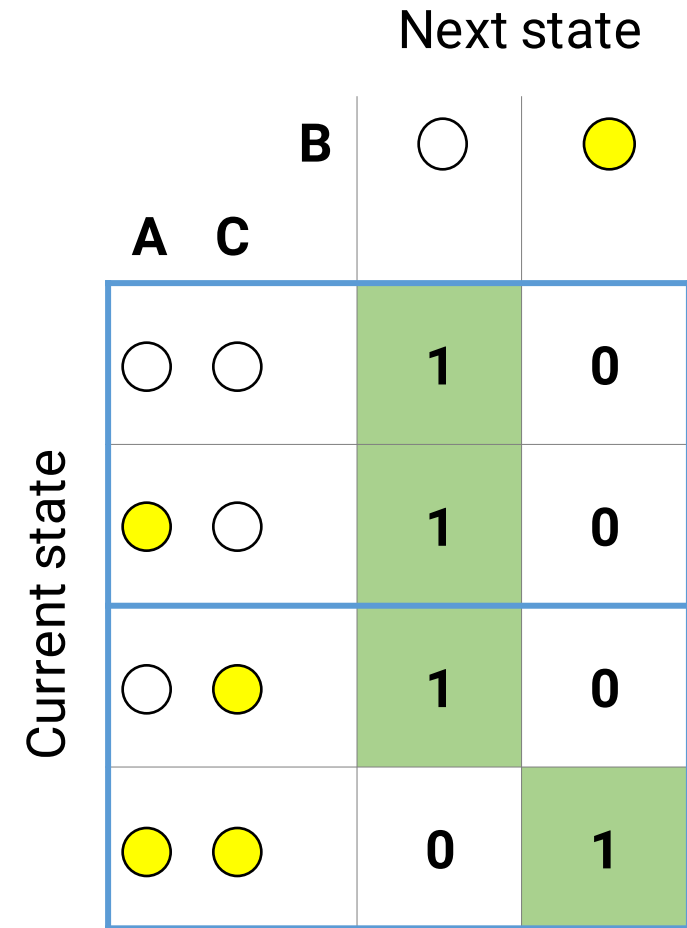   | 1                                                                                   | 0                                                                                   |
|               | 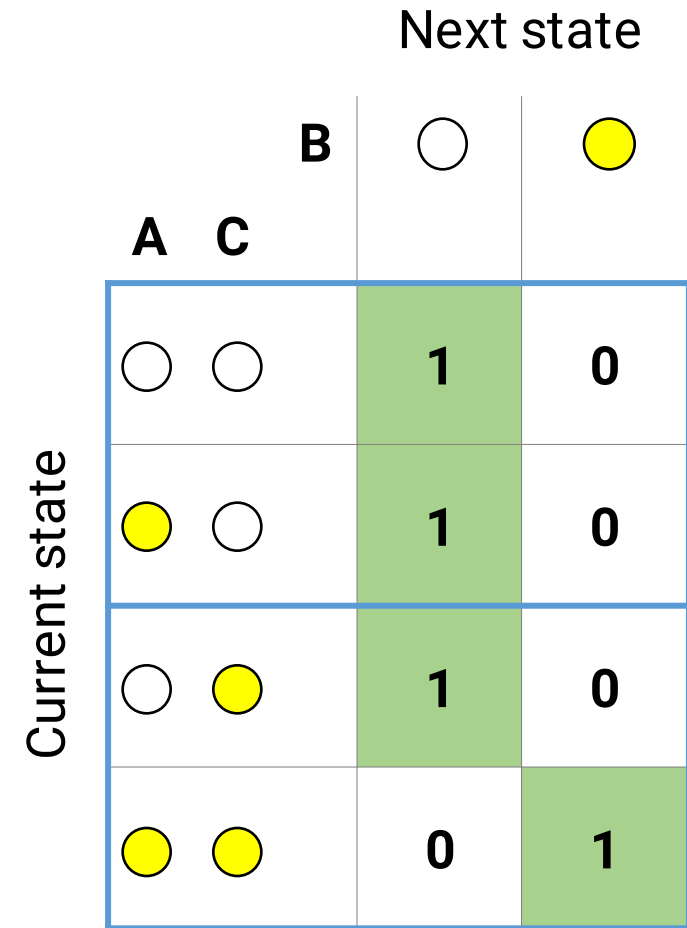   | 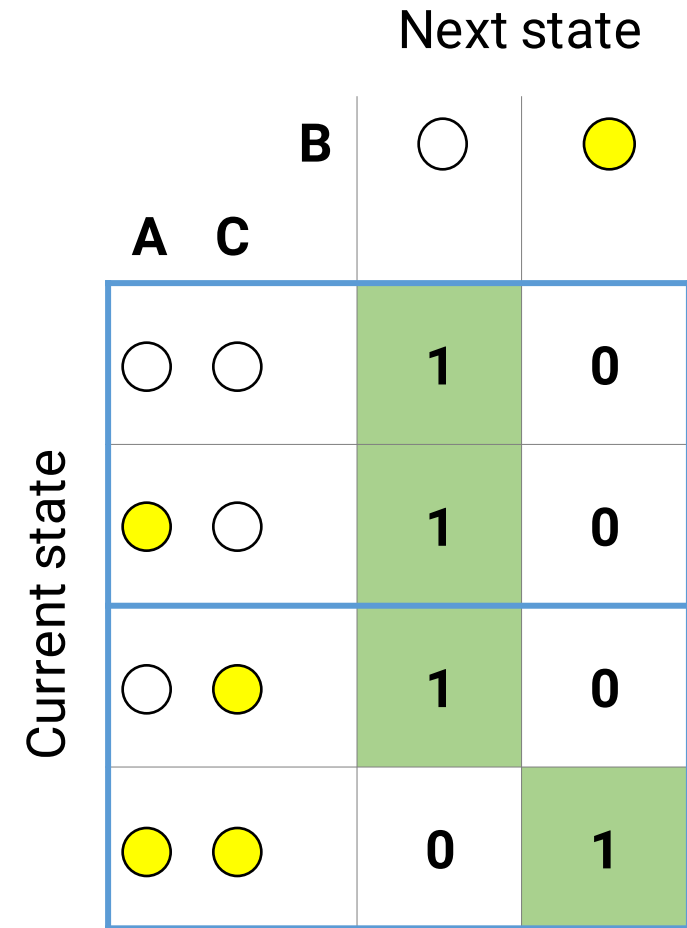   | 1                                                                                   | 0                                                                                   |
|               | 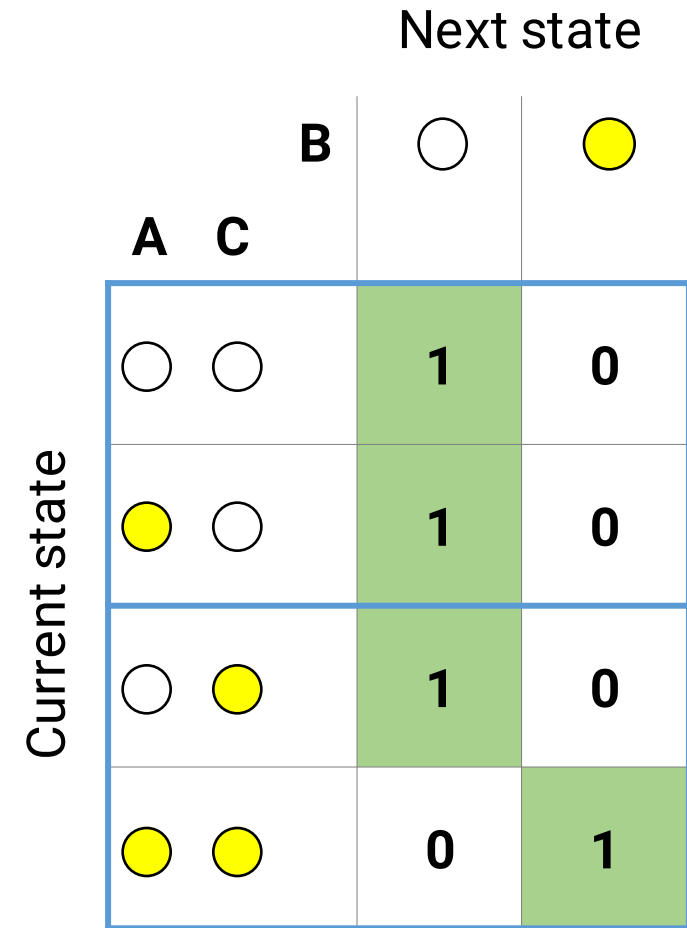   | 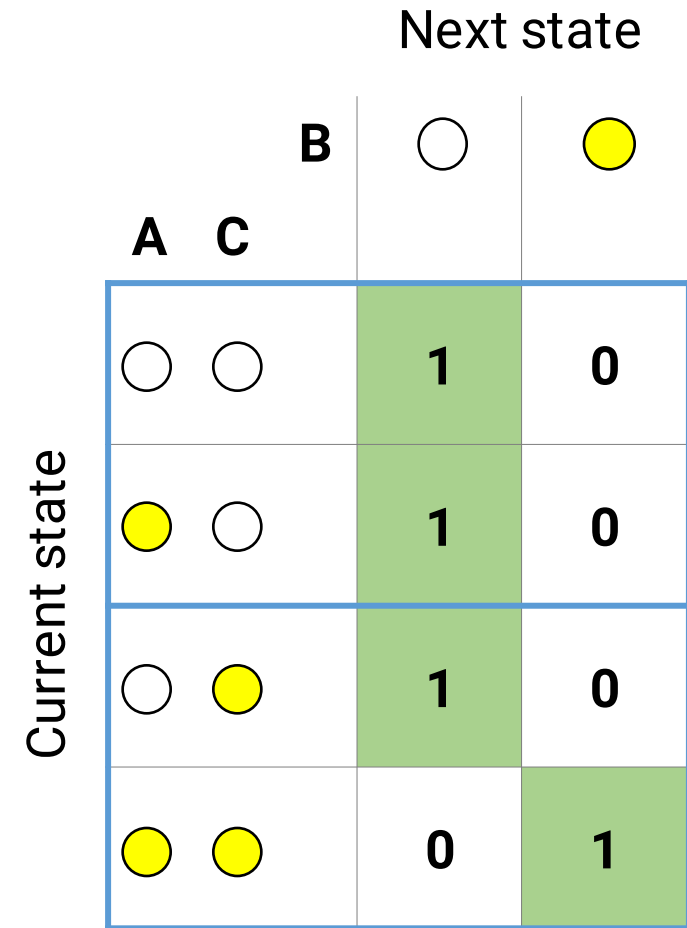   | 1                                                                                   | 0                                                                                   |
|               | 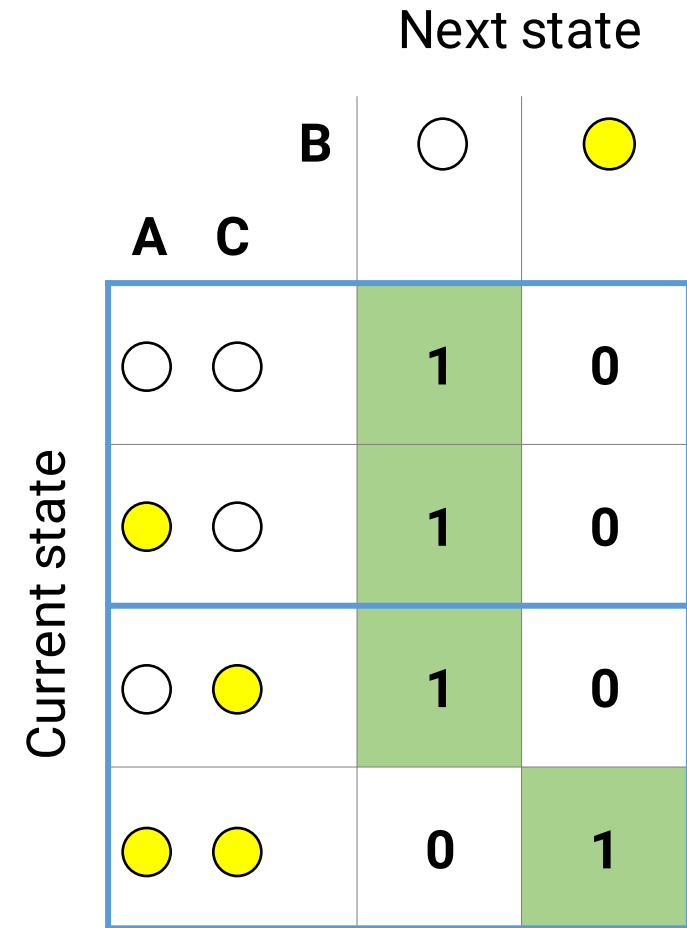 | 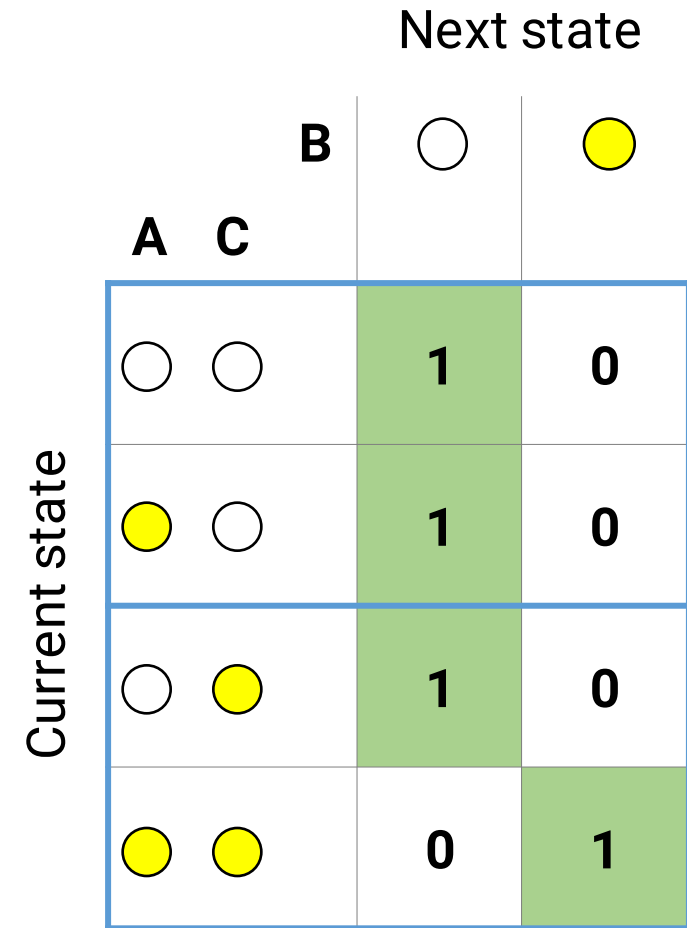 | 0                                                                                   | 1                                                                                   |

Integration and reducibility:

## System-level irreducibility and system cuts

- Next we find the TPM for **B**, which takes input from **C** and *noised* input from **A**
- We account for **A**'s noisy output by computing the TPM as if the output were not noised, then marginalizing **A** out

|               |                                                                                                                                                                           | Next state                                                                          |                                                                                     |
|---------------|---------------------------------------------------------------------------------------------------------------------------------------------------------------------------|-------------------------------------------------------------------------------------|-------------------------------------------------------------------------------------|
|               |                                                                                                                                                                           | 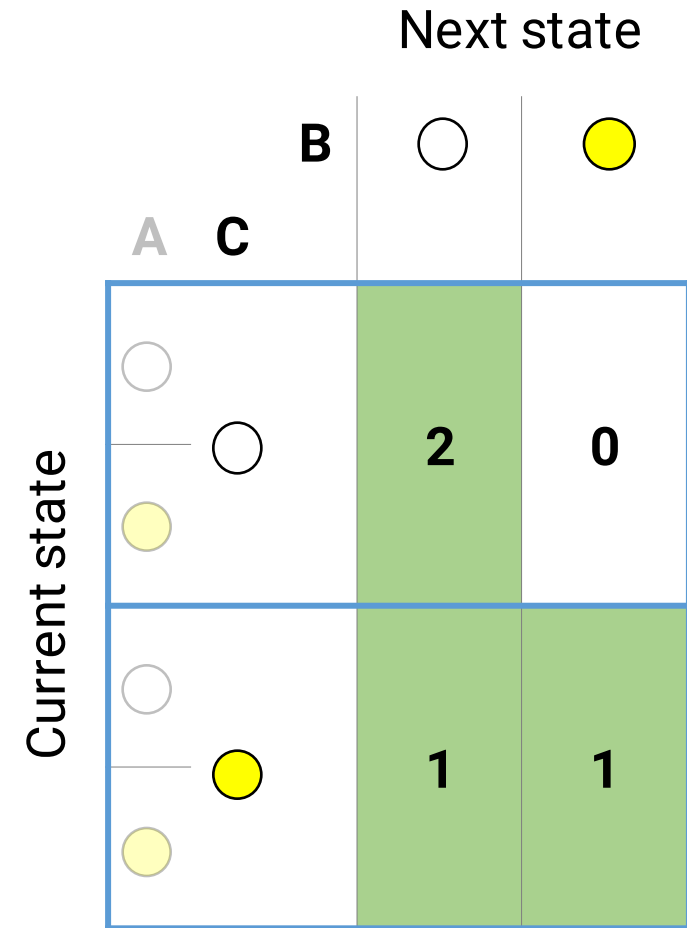 | 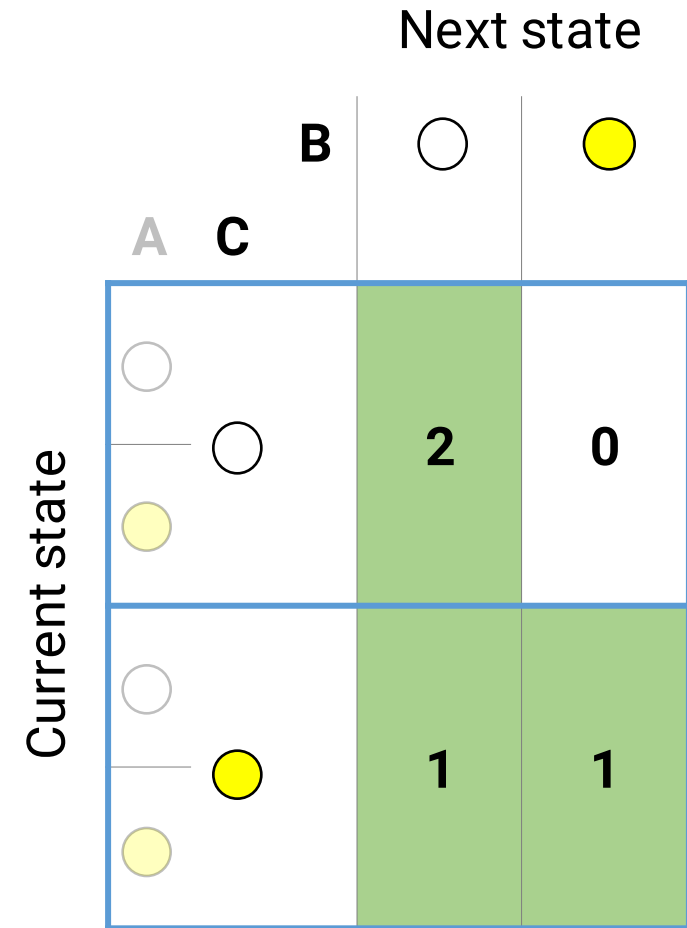 |
| Current state | <b>B</b>                                                                                                                                                                  |                                                                                     |                                                                                     |
|               | <b>A</b> <b>C</b>                                                                                                                                                         |                                                                                     |                                                                                     |
|               | 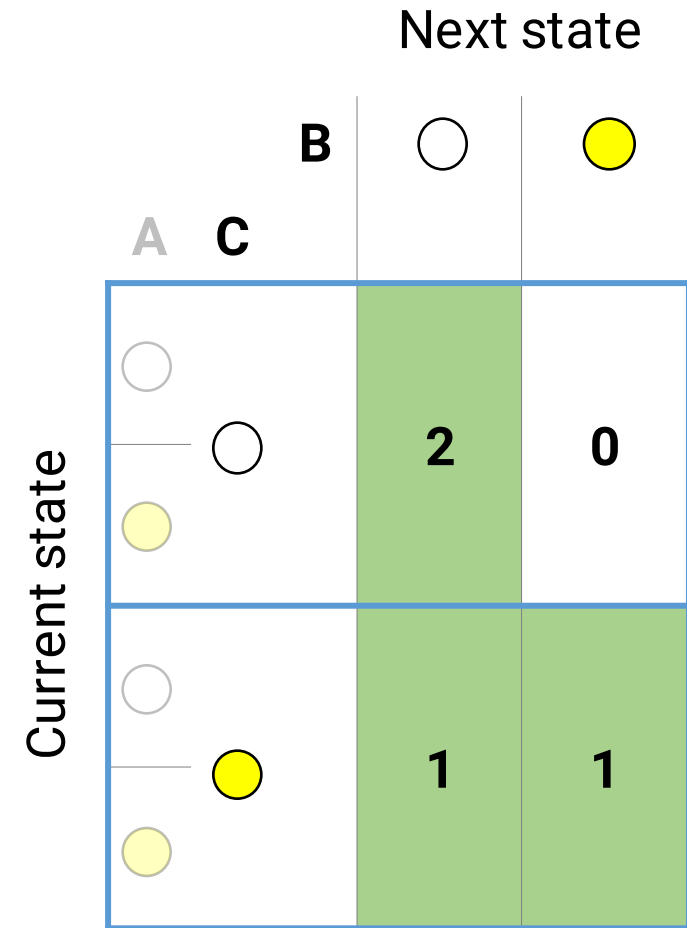 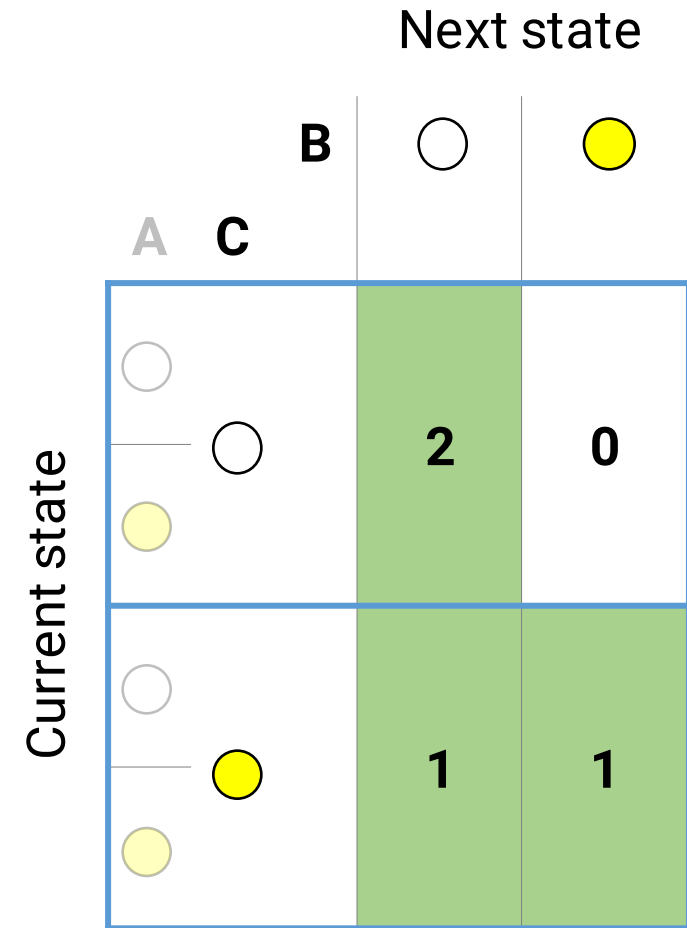   | 2                                                                                   | 0                                                                                   |
|               | 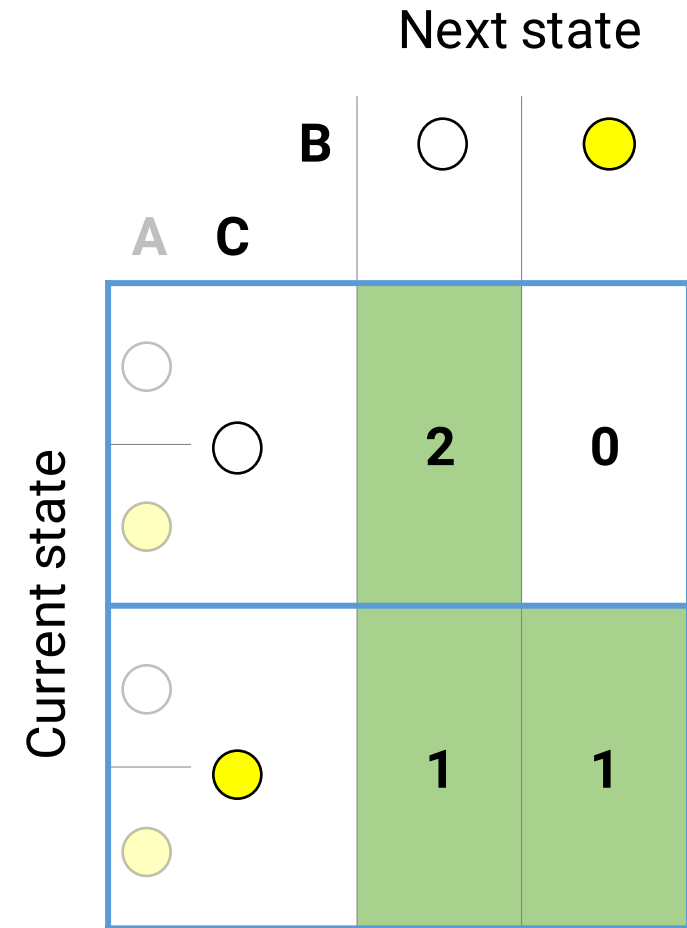 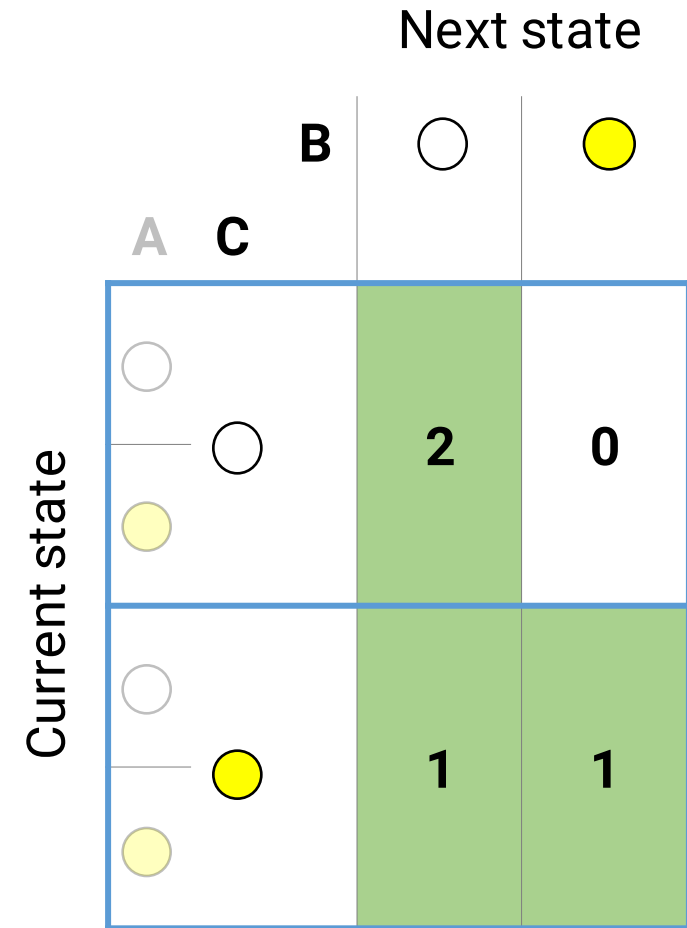   |                                                                                     |                                                                                     |
|               | 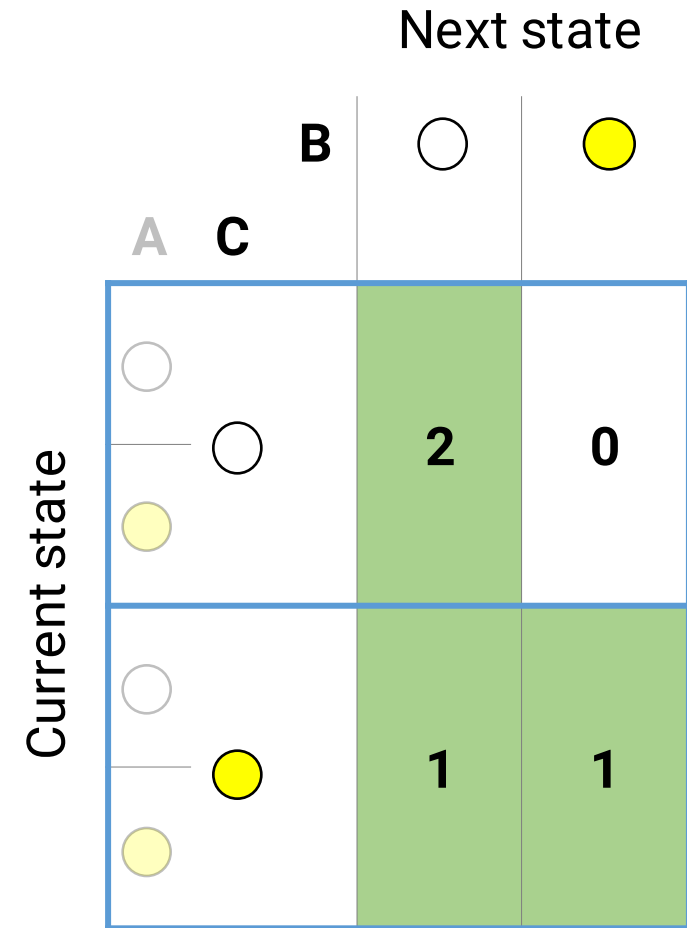 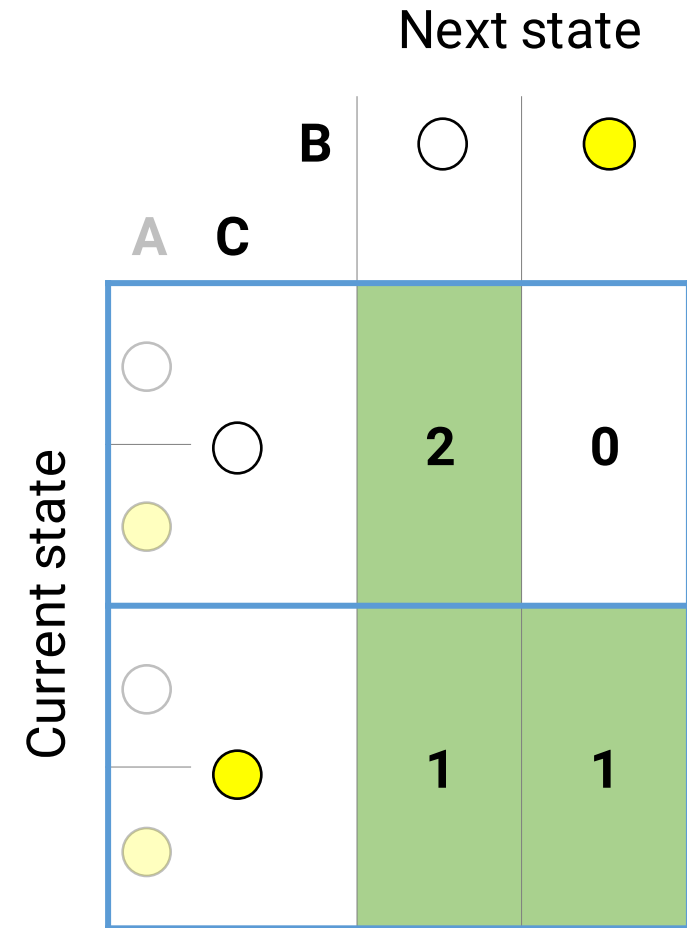   | 1                                                                                   | 1                                                                                   |
|               | 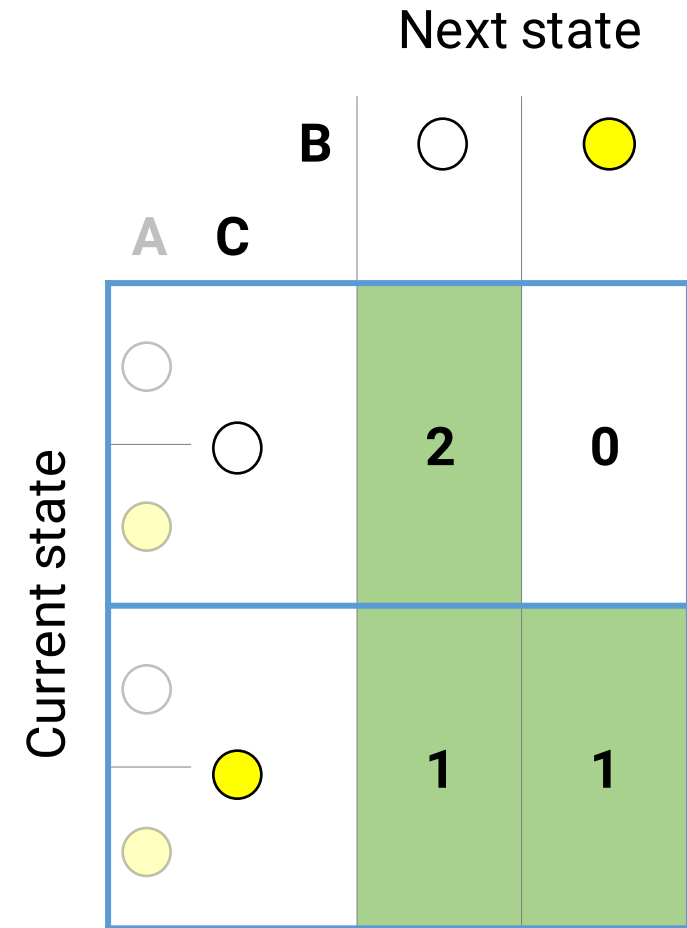 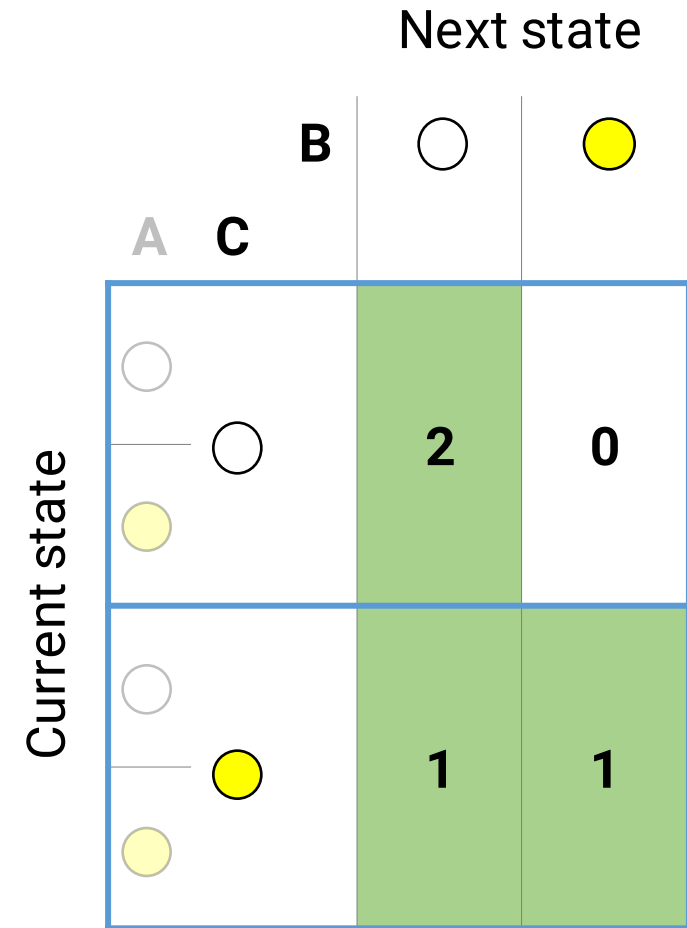 |                                                                                     |                                                                                     |

Integration and reducibility:

## System-level irreducibility and system cuts

- Next we find the TPM for **B**, which takes input from **C** and *noised* input from **A**
- We account for **A**'s noisy output by computing the TPM as if the output were not noised, then marginalizing **A** out

|               |                                                                                     | Next state                                                                          |                                                                                     |
|---------------|-------------------------------------------------------------------------------------|-------------------------------------------------------------------------------------|-------------------------------------------------------------------------------------|
|               |                                                                                     | <b>B</b>                                                                            |                                                                                     |
| Current state | <b>C</b>                                                                            | 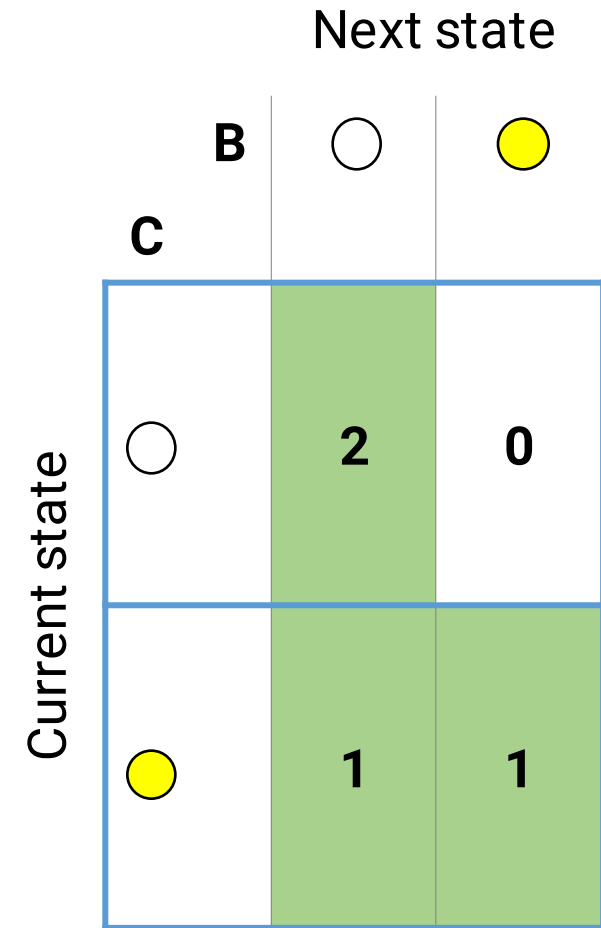 | 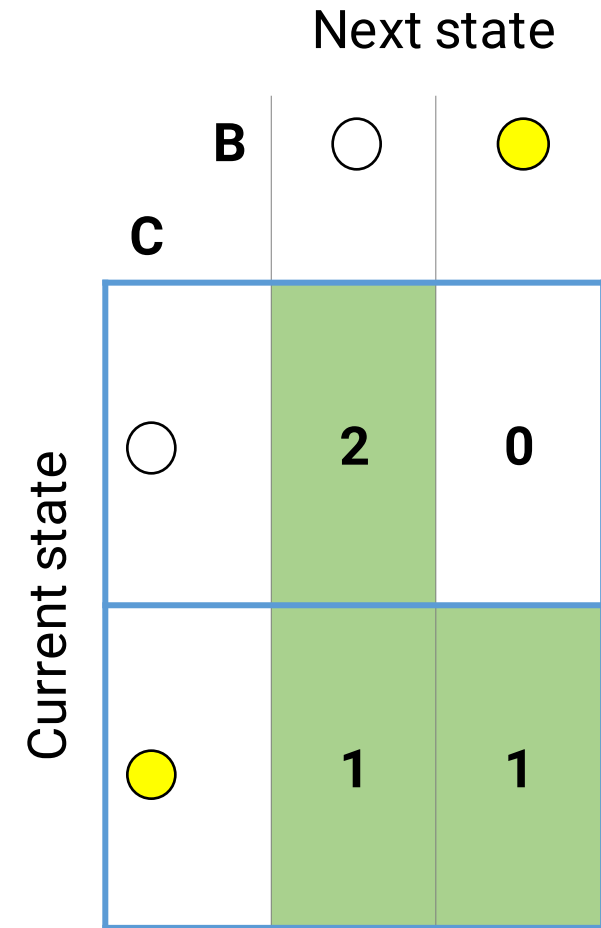 |
|               | 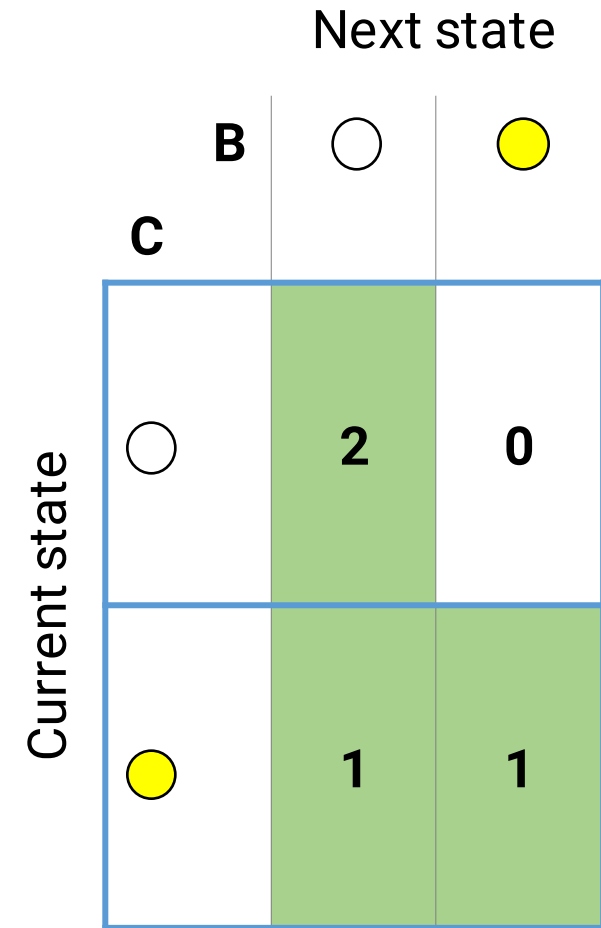 | 2                                                                                   | 0                                                                                   |
|               | 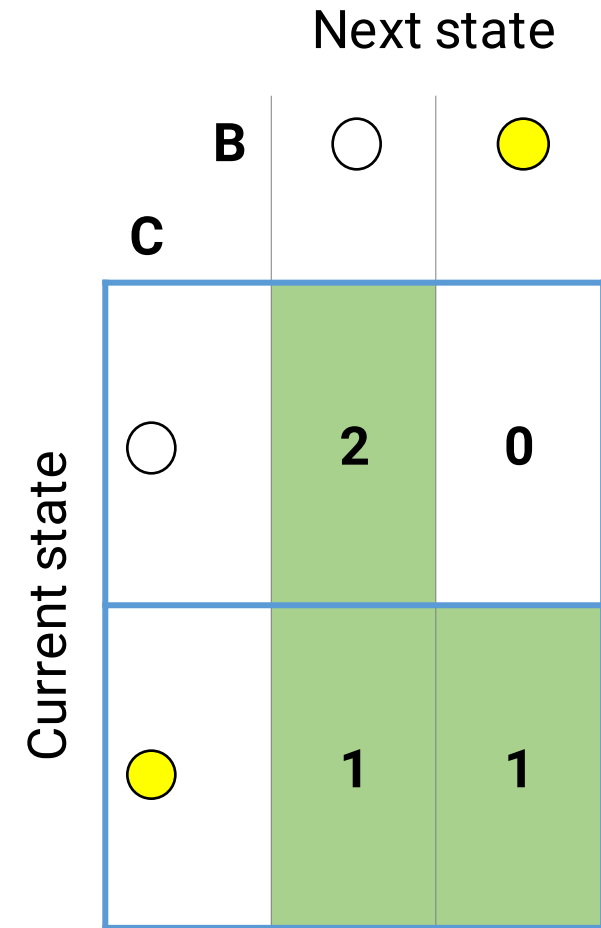 | 1                                                                                   | 1                                                                                   |

Integration and reducibility:

## System-level irreducibility and system cuts

- Next we find the TPM for **B**, which takes input from **C** and *noised* input from **A**
- We account for **A**'s noisy output by computing the TPM as if the output were not noised, then marginalizing **A** out

|               |                                                                                     | Next state                                                                          |                                                                                     |
|---------------|-------------------------------------------------------------------------------------|-------------------------------------------------------------------------------------|-------------------------------------------------------------------------------------|
|               |                                                                                     | B                                                                                   |                                                                                     |
| Current state | C                                                                                   | 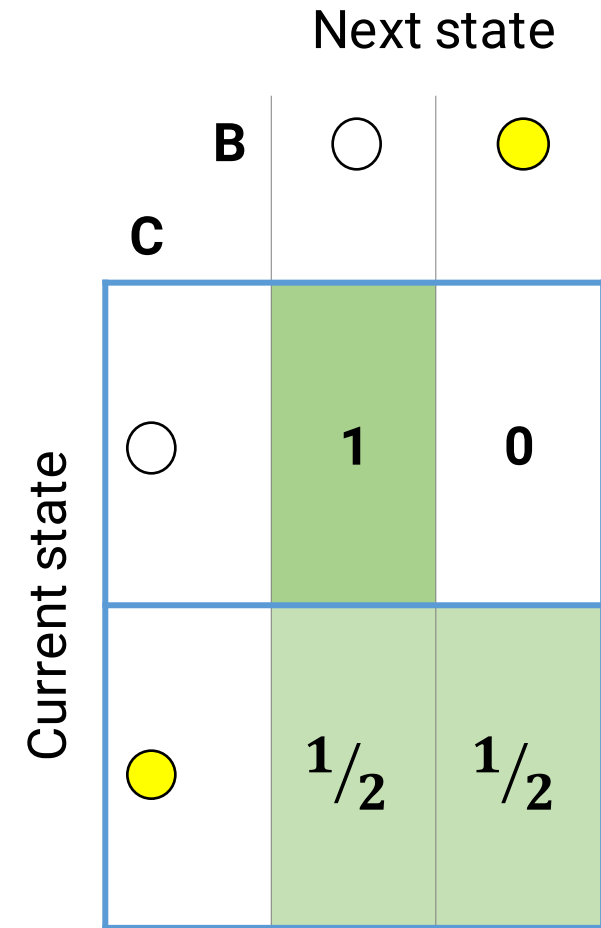 | 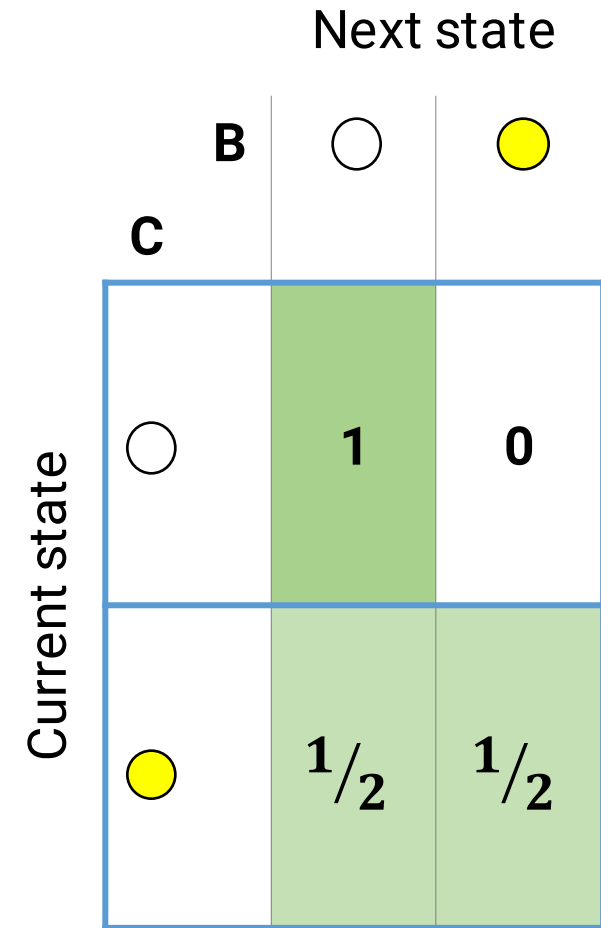 |
|               | 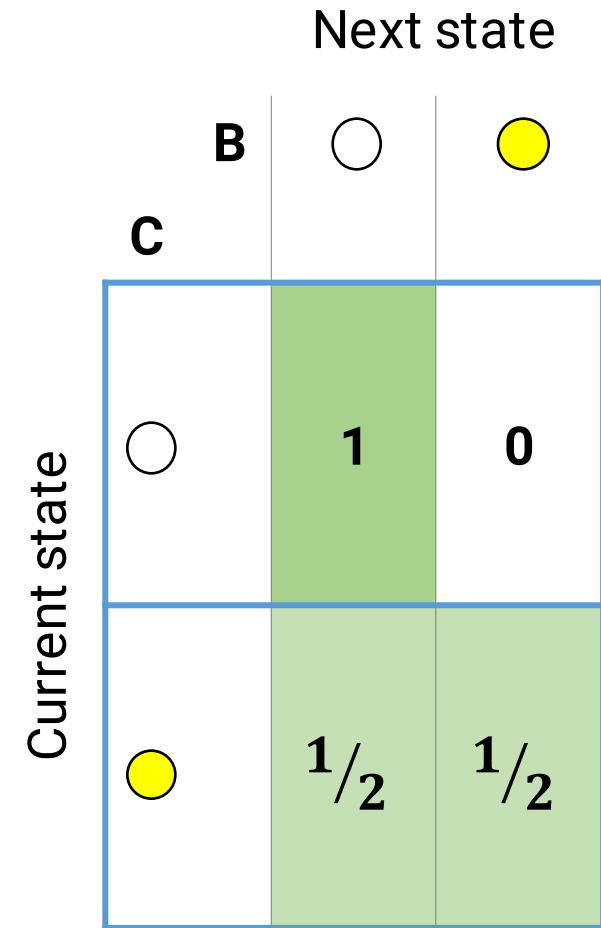 | 1                                                                                   | 0                                                                                   |
|               | 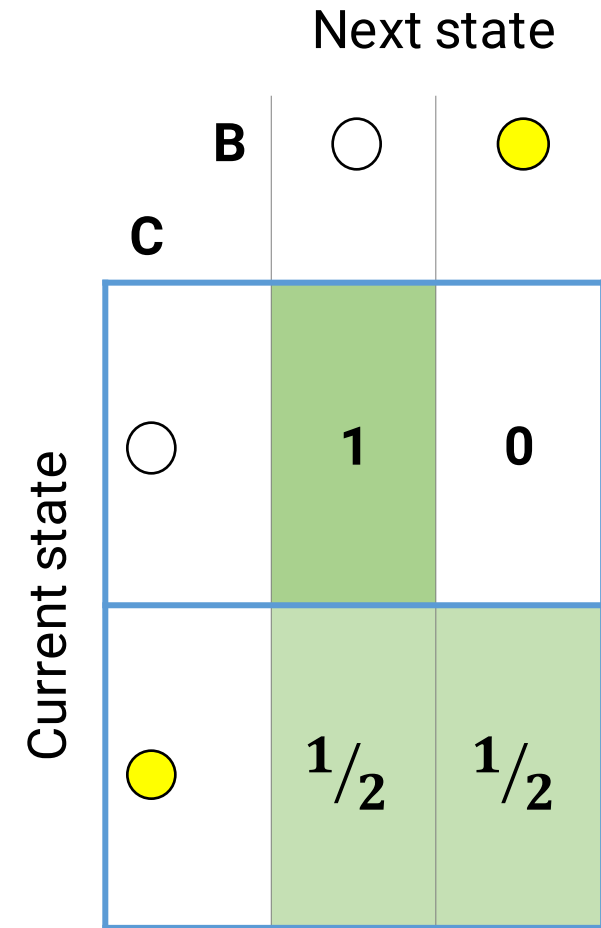 | $\frac{1}{2}$                                                                       | $\frac{1}{2}$                                                                       |

Integration and reducibility:

## System-level irreducibility and system cuts

- Next we find the TPM for **B**, which takes input from **C** and *noised* input from **A**
- We account for **A**'s noisy output by computing the TPM as if the output were not noised, then marginalizing **A** out

|               |                                                                                     | Next state                                                                          |                                                                                     |
|---------------|-------------------------------------------------------------------------------------|-------------------------------------------------------------------------------------|-------------------------------------------------------------------------------------|
|               |                                                                                     | <b>B</b>                                                                            |                                                                                     |
| Current state | <b>C</b>                                                                            | 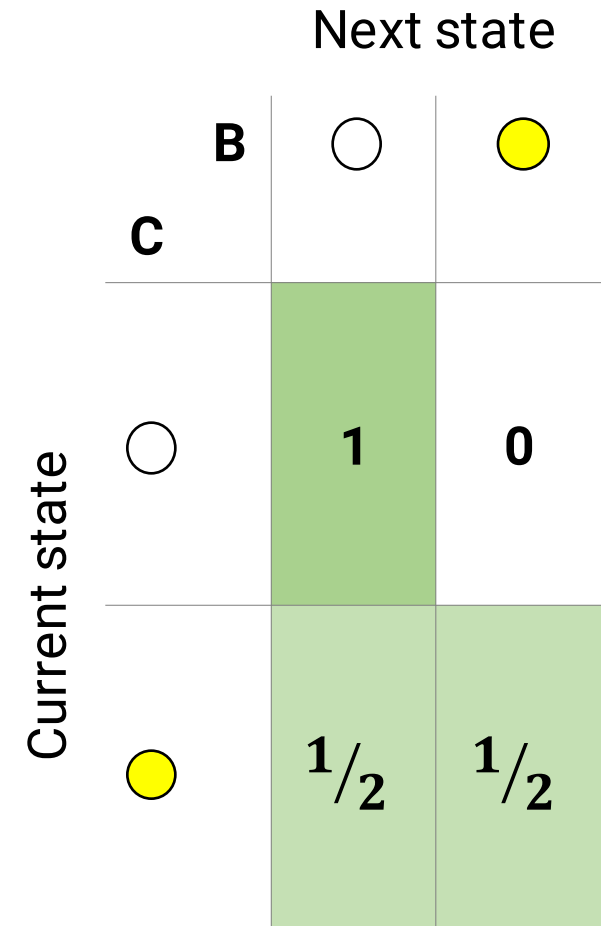 | 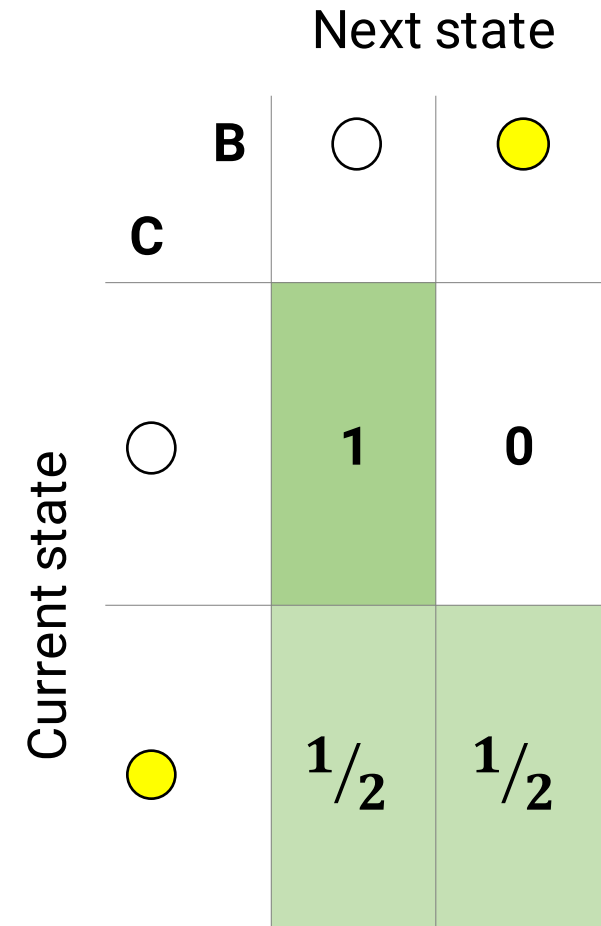 |
|               | 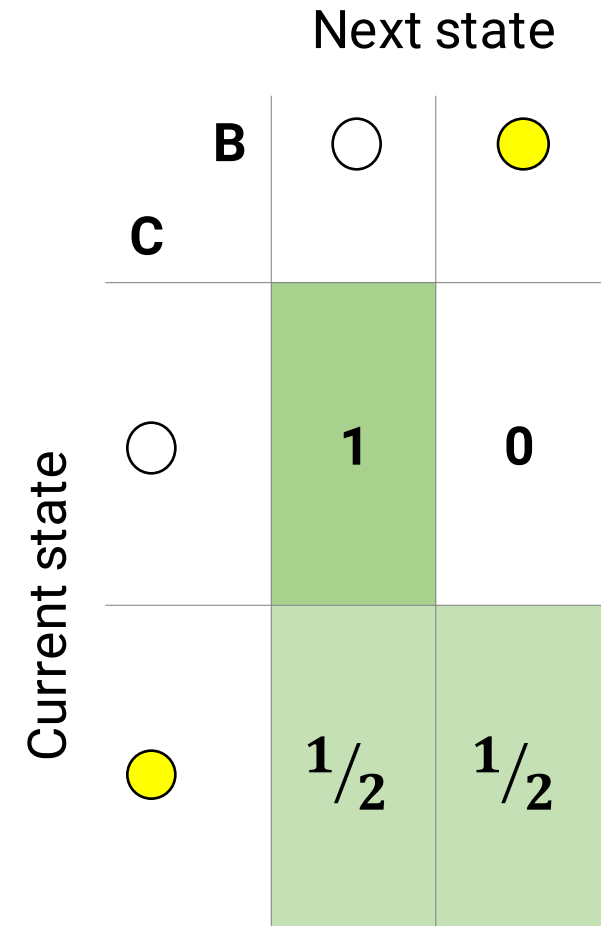 | 1                                                                                   | 0                                                                                   |
|               | 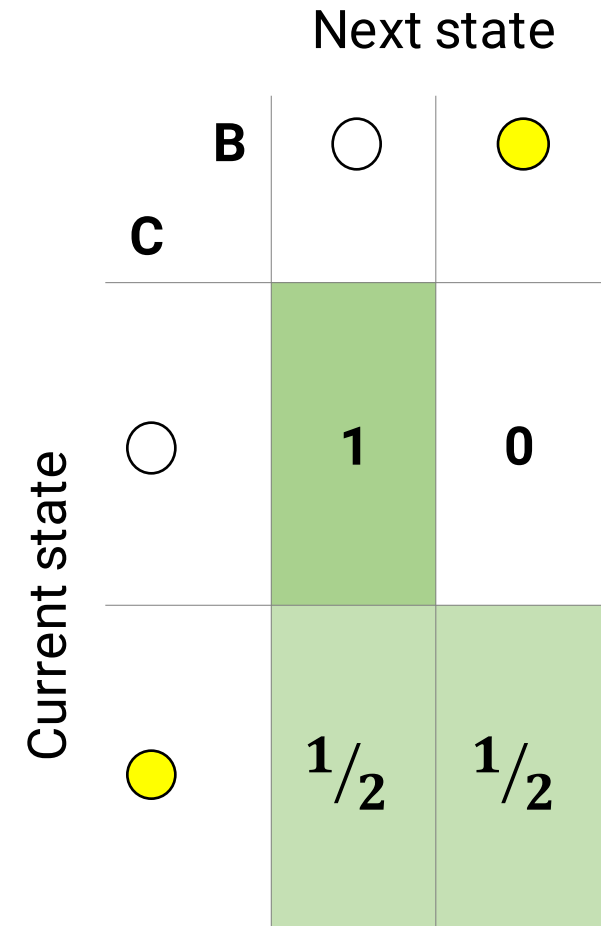 | $1/2$                                                                               | $1/2$                                                                               |



Integration and reducibility:

## System-level irreducibility and system cuts

- Finally we do the same procedure for **C**, (which only gets input from B after the cut), which results in this TPM:

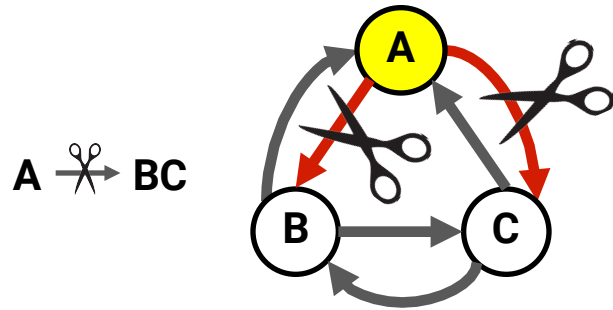

|               |                                                                                     | Next state                                                                          |                                                                                     |
|---------------|-------------------------------------------------------------------------------------|-------------------------------------------------------------------------------------|-------------------------------------------------------------------------------------|
| Current state | <b>B</b>                                                                            | <b>C</b>                                                                            |                                                                                     |
|               |                                                                                     | 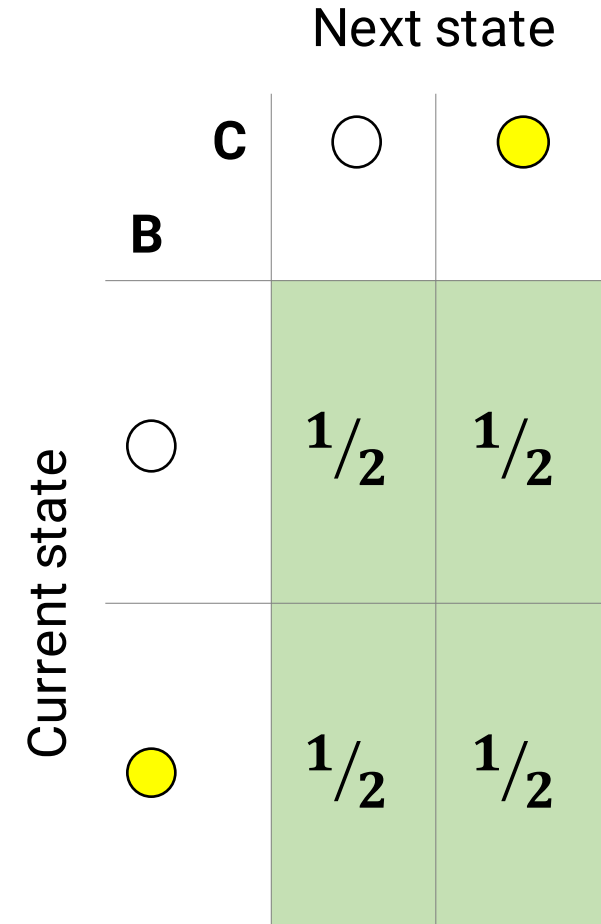 | 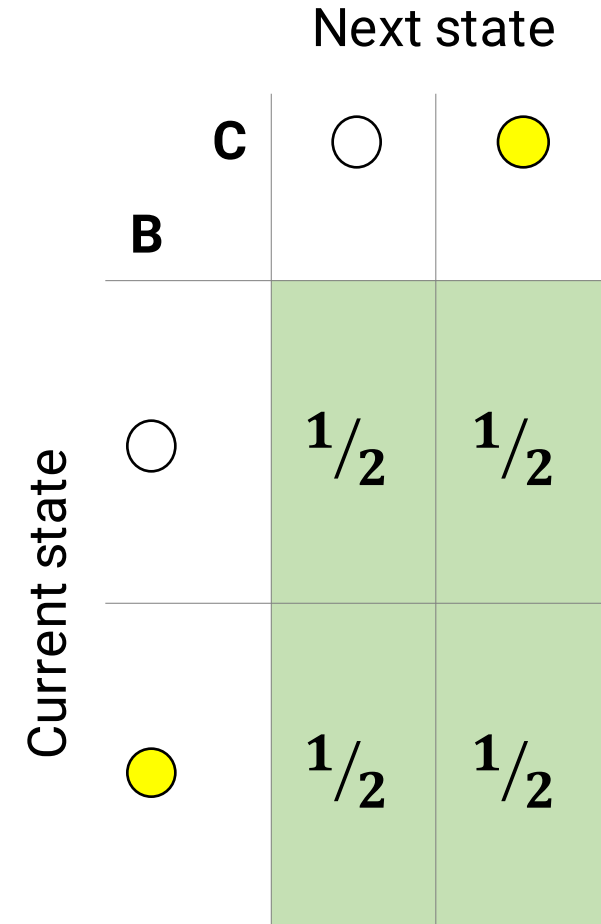 |
|               | 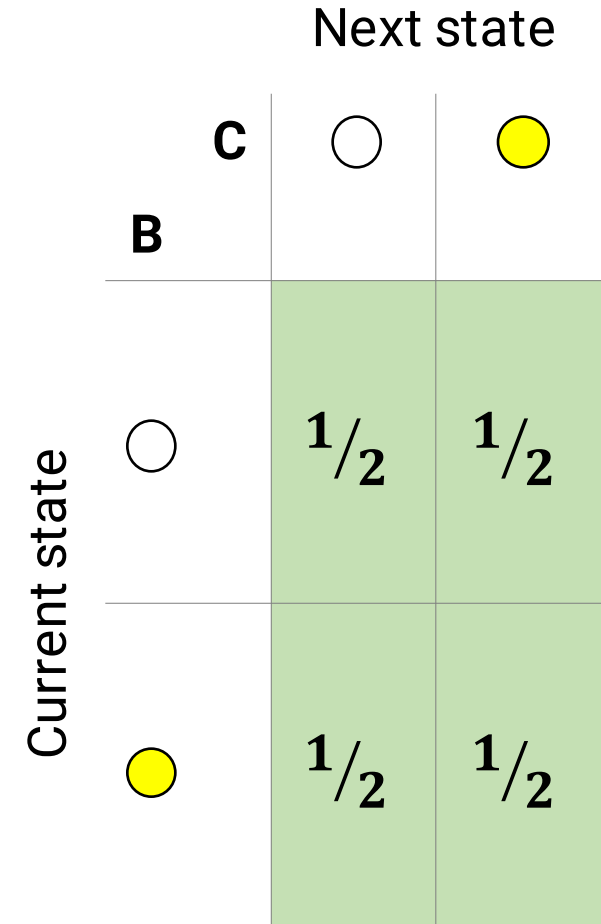 | $\frac{1}{2}$                                                                       | $\frac{1}{2}$                                                                       |
|               | 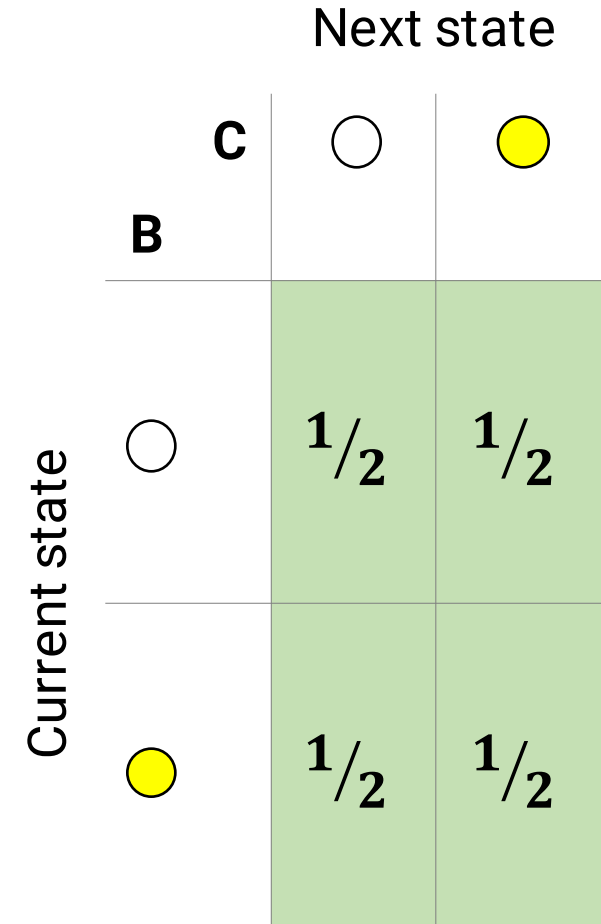 | $\frac{1}{2}$                                                                       | $\frac{1}{2}$                                                                       |

Integration and reducibility:  
**System-level irreducibility and system cuts**

Then we expand these TPMs to the full state space so they can be combined:

|   |   | A | ○ | ● |
|---|---|---|---|---|
| B | C |   |   |   |
| ○ | ○ | 1 | 0 |   |
| ● | ○ | 0 | 1 |   |
| ○ | ● | 0 | 1 |   |
| ● | ● | 0 | 1 |   |

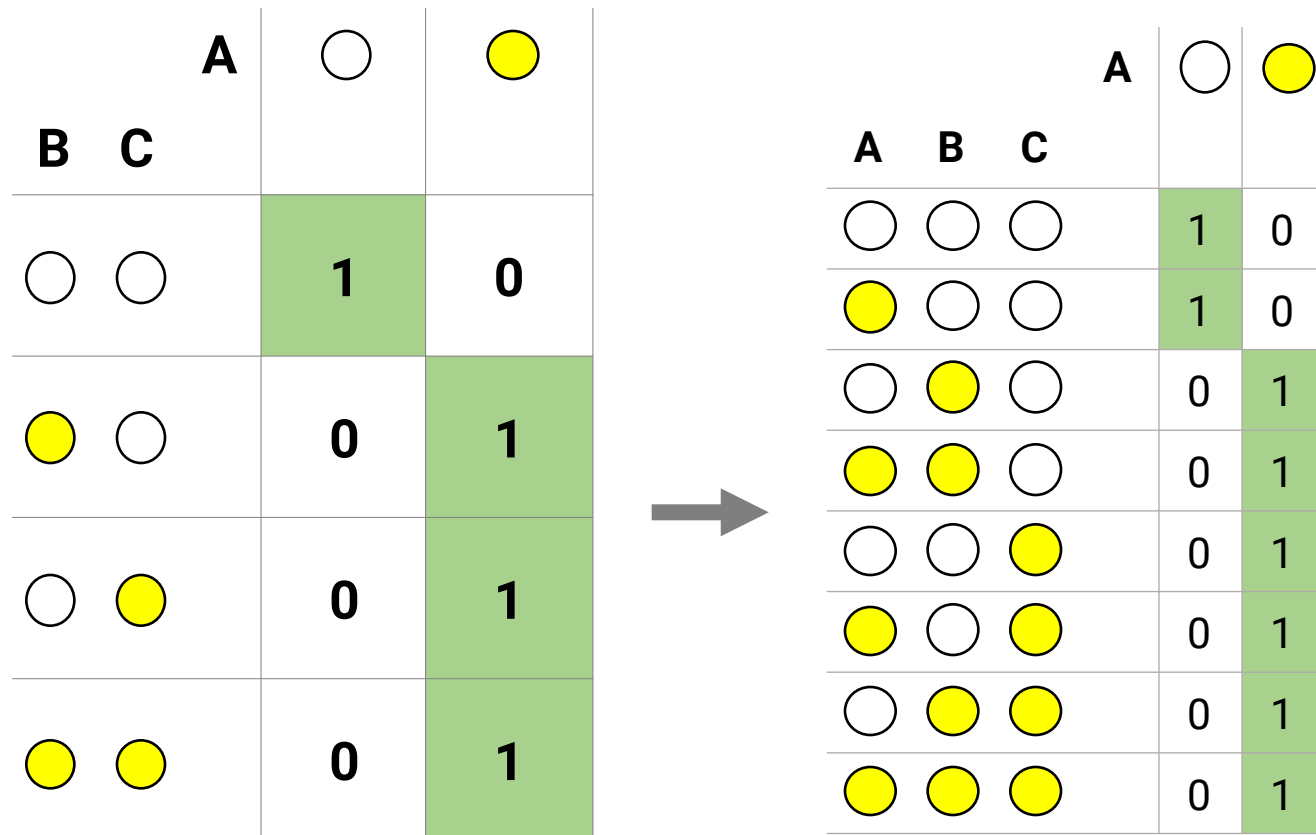

|   |   |   | A | ○ | ● |
|---|---|---|---|---|---|
| A | B | C |   |   |   |
| ○ | ○ | ○ | 1 | 0 |   |
| ● | ○ | ○ | 1 | 0 |   |
| ○ | ● | ○ | 0 | 1 |   |
| ● | ● | ○ | 0 | 1 |   |
| ○ | ○ | ● | 0 | 1 |   |
| ● | ○ | ● | 0 | 1 |   |
| ○ | ● | ● | 0 | 1 |   |
| ● | ● | ● | 0 | 1 |   |

Integration and reducibility:  
**System-level irreducibility and system cuts**

Then we expand these TPMs to the full state space so they can be combined:

|   |   | B             |               |
|---|---|---------------|---------------|
|   |   | ○             | ●             |
| C | ○ | 1             | 0             |
|   | ● | $\frac{1}{2}$ | $\frac{1}{2}$ |

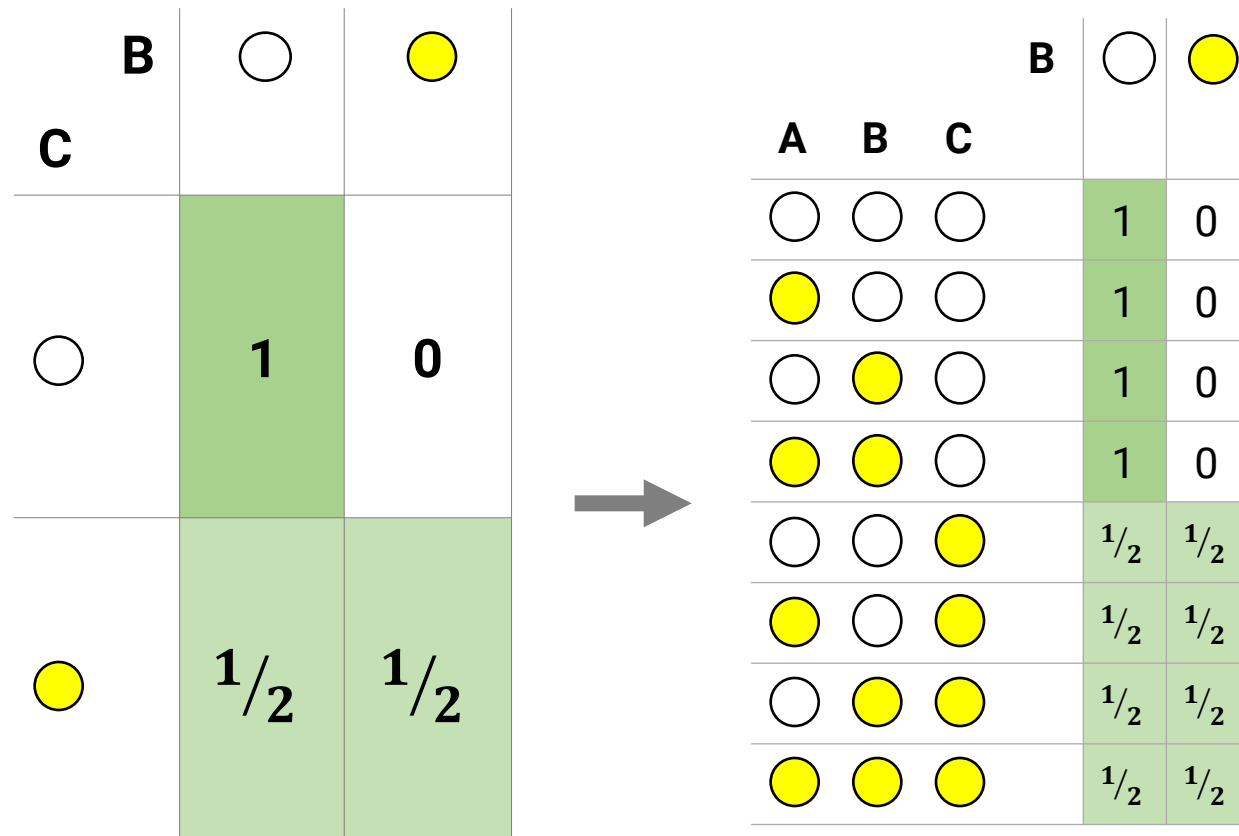

|   |   |   | B             |               |
|---|---|---|---------------|---------------|
|   |   |   | ○             | ●             |
| A | B | C |               |               |
| ○ | ○ | ○ | 1             | 0             |
| ● | ○ | ○ | 1             | 0             |
| ○ | ● | ○ | 1             | 0             |
| ● | ● | ○ | 1             | 0             |
| ○ | ○ | ● | $\frac{1}{2}$ | $\frac{1}{2}$ |
| ● | ○ | ● | $\frac{1}{2}$ | $\frac{1}{2}$ |
| ○ | ● | ● | $\frac{1}{2}$ | $\frac{1}{2}$ |
| ● | ● | ● | $\frac{1}{2}$ | $\frac{1}{2}$ |

Integration and reducibility:  
**System-level irreducibility and system cuts**

Then we expand these TPMs to the full state space so they can be combined:

|   |   | C             |               |
|---|---|---------------|---------------|
|   |   | ○             | ●             |
| B | ○ | $\frac{1}{2}$ | $\frac{1}{2}$ |
|   | ● | $\frac{1}{2}$ | $\frac{1}{2}$ |

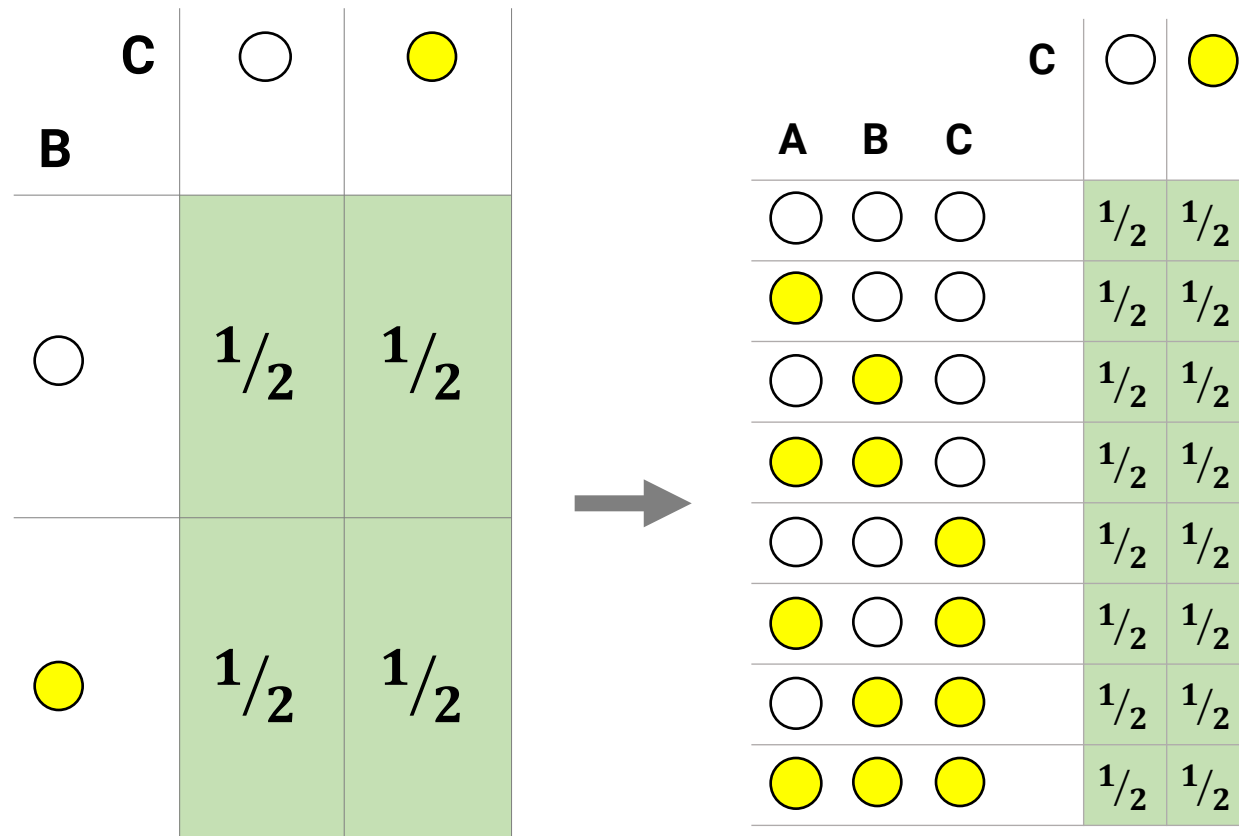

|   |   |   | C             |               |
|---|---|---|---------------|---------------|
|   |   |   | ○             | ●             |
| A | B | C |               |               |
| ○ | ○ | ○ | $\frac{1}{2}$ | $\frac{1}{2}$ |
| ● | ○ | ○ | $\frac{1}{2}$ | $\frac{1}{2}$ |
| ○ | ● | ○ | $\frac{1}{2}$ | $\frac{1}{2}$ |
| ● | ● | ○ | $\frac{1}{2}$ | $\frac{1}{2}$ |
| ○ | ○ | ● | $\frac{1}{2}$ | $\frac{1}{2}$ |
| ● | ○ | ● | $\frac{1}{2}$ | $\frac{1}{2}$ |
| ○ | ● | ● | $\frac{1}{2}$ | $\frac{1}{2}$ |
| ● | ● | ● | $\frac{1}{2}$ | $\frac{1}{2}$ |

# Integration and reducibility: System-level irreducibility and system cuts

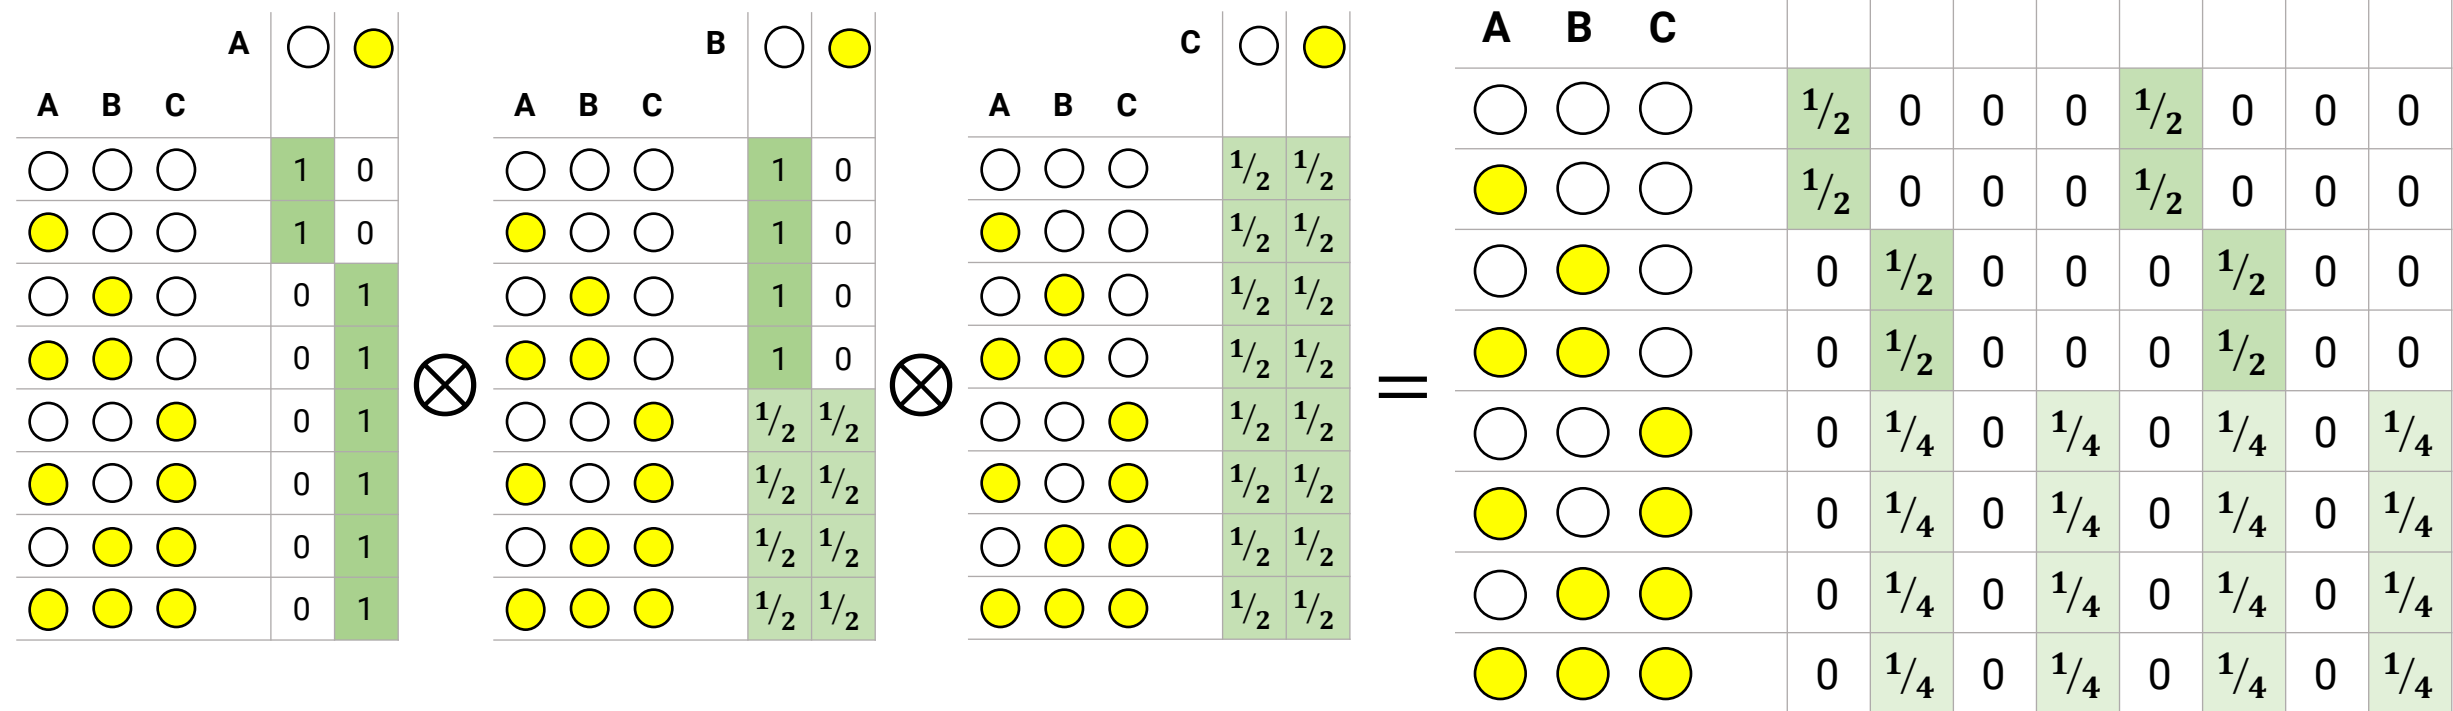

Now we can get the full TPM of the cut system by taking the tensor product of the individual TPMs

# Integration and reducibility: System-level irreducibility and system cuts

|   |   |   | A |   |   |   |   |   |   |   |
|---|---|---|---|---|---|---|---|---|---|---|
|   |   |   | A |   |   |   |   |   |   |   |
|   |   |   | B |   |   |   |   |   |   |   |
|   |   |   | C |   |   |   |   |   |   |   |
| A | B | C |   |   |   |   |   |   |   |   |
| ○ | ○ | ○ | 1 | 0 | 0 | 0 | 0 | 0 | 0 | 0 |
| ● | ○ | ○ | 0 | 0 | 0 | 0 | 1 | 0 | 0 | 0 |
| ○ | ● | ○ | 0 | 0 | 0 | 0 | 0 | 1 | 0 | 0 |
| ● | ● | ○ | 0 | 1 | 0 | 0 | 0 | 0 | 0 | 0 |
| ○ | ○ | ● | 0 | 1 | 0 | 0 | 0 | 0 | 0 | 0 |
| ● | ○ | ● | 0 | 0 | 0 | 0 | 0 | 0 | 0 | 1 |
| ○ | ● | ● | 0 | 0 | 0 | 0 | 0 | 1 | 0 | 0 |
| ● | ● | ● | 0 | 0 | 0 | 1 | 0 | 0 | 0 | 0 |

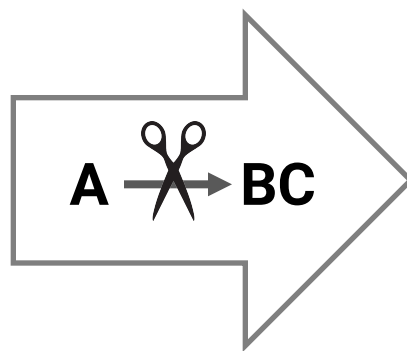

|   |   |   | A   |     |   |     |     |     |   |     |
|---|---|---|-----|-----|---|-----|-----|-----|---|-----|
|   |   |   | A   |     |   |     |     |     |   |     |
|   |   |   | B   |     |   |     |     |     |   |     |
|   |   |   | C   |     |   |     |     |     |   |     |
| A | B | C |     |     |   |     |     |     |   |     |
| ○ | ○ | ○ | 1/2 | 0   | 0 | 0   | 1/2 | 0   | 0 | 0   |
| ● | ○ | ○ | 1/2 | 0   | 0 | 0   | 1/2 | 0   | 0 | 0   |
| ○ | ● | ○ | 0   | 1/2 | 0 | 0   | 0   | 1/2 | 0 | 0   |
| ● | ● | ○ | 0   | 1/2 | 0 | 0   | 0   | 1/2 | 0 | 0   |
| ○ | ○ | ● | 0   | 1/4 | 0 | 1/4 | 0   | 1/4 | 0 | 1/4 |
| ● | ○ | ● | 0   | 1/4 | 0 | 1/4 | 0   | 1/4 | 0 | 1/4 |
| ○ | ● | ● | 0   | 1/4 | 0 | 1/4 | 0   | 1/4 | 0 | 1/4 |
| ● | ● | ● | 0   | 1/4 | 0 | 1/4 | 0   | 1/4 | 0 | 1/4 |

*In sum:* this is how the system cut  $A \not\Rightarrow BC$  changes the TPM

Integration and reducibility:

## System-level irreducibility and system cuts

- Now that we've recalculated the TPM, we can calculate the cut system's cause-effect structure
- We need to determine if the cut "makes a difference" from the intrinsic perspective of the system
- This will tell us whether the system reduces to the parts separated by the cut
- We do this by comparing the cause-effect structure of the uncut system to that of the cut system

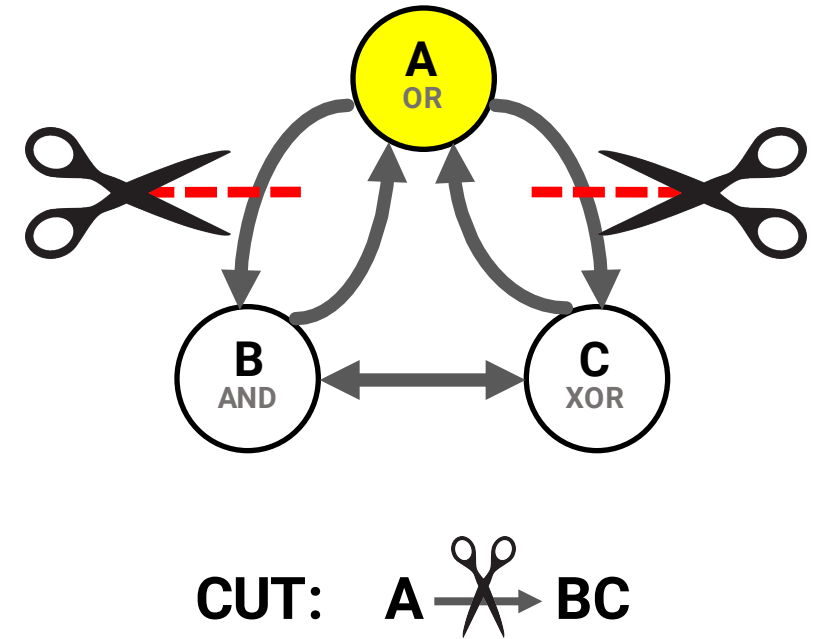

# Integration and reducibility: System-level irreducibility and system cuts

WHOLE  
SYSTEM:

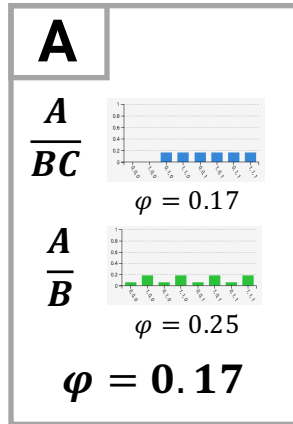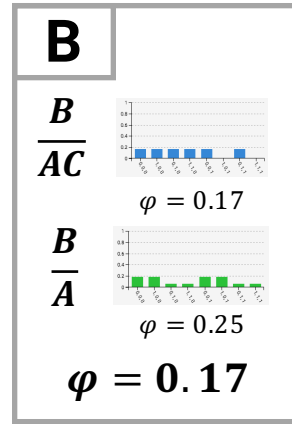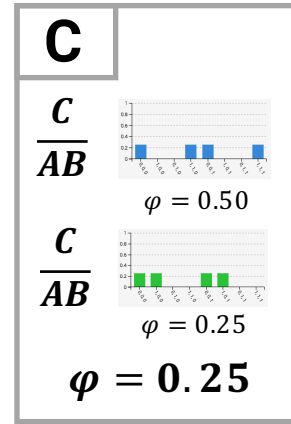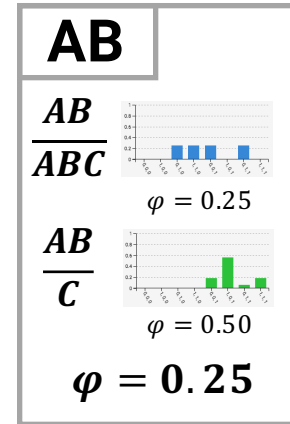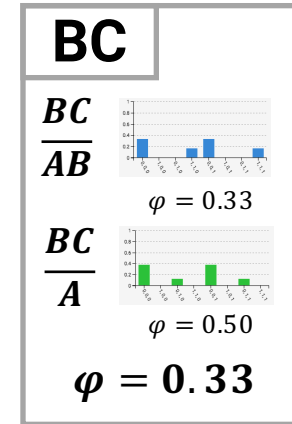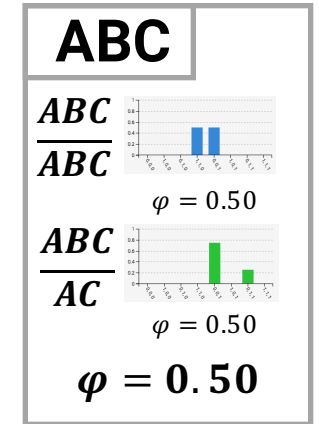

**A**

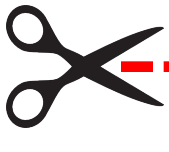

**BC**

CUT  
SYSTEM:

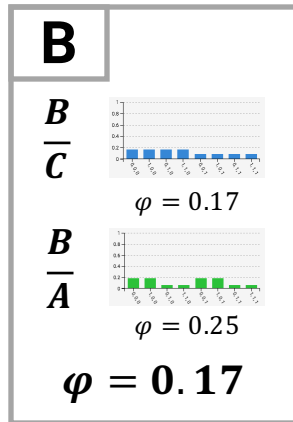

Here, we see that all the concepts except the one specified by **B** have been destroyed by the cut



# Integration and reducibility: Extended earth mover's distance

WHOLE  
SYSTEM:

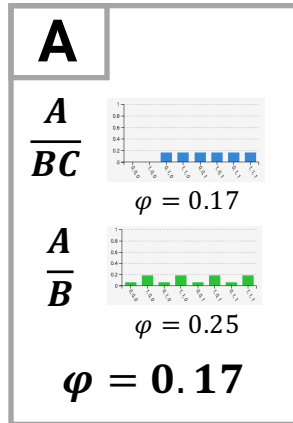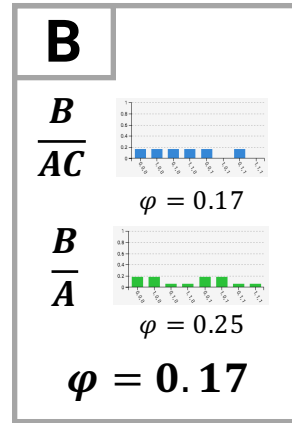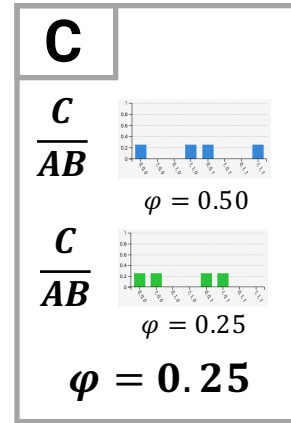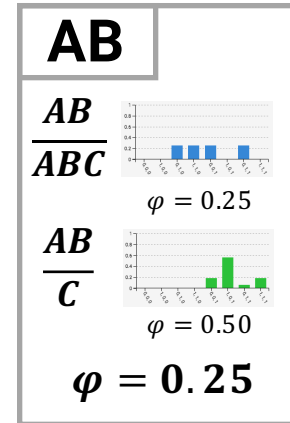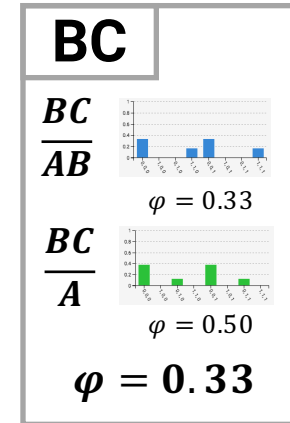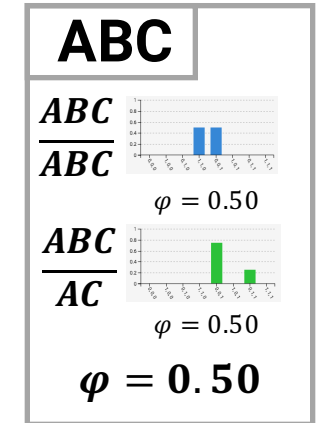

**A**

**BC**

CUT  
SYSTEM:

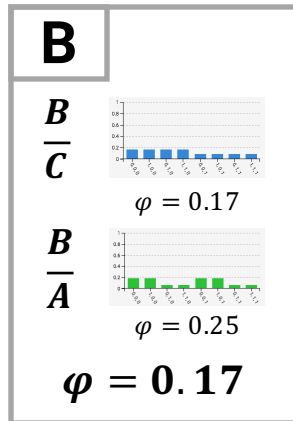

- So, we can see that this cut “makes a difference” (from the system’s intrinsic perspective), but how do we quantify that difference?
- As with calculating the  $\varphi$  of a repertoire, we can use the Earth Mover’s Distance to measure the difference between the unpartitioned and partitioned cause-effect structures

# Integration and reducibility: Extended earth mover's distance

WHOLE

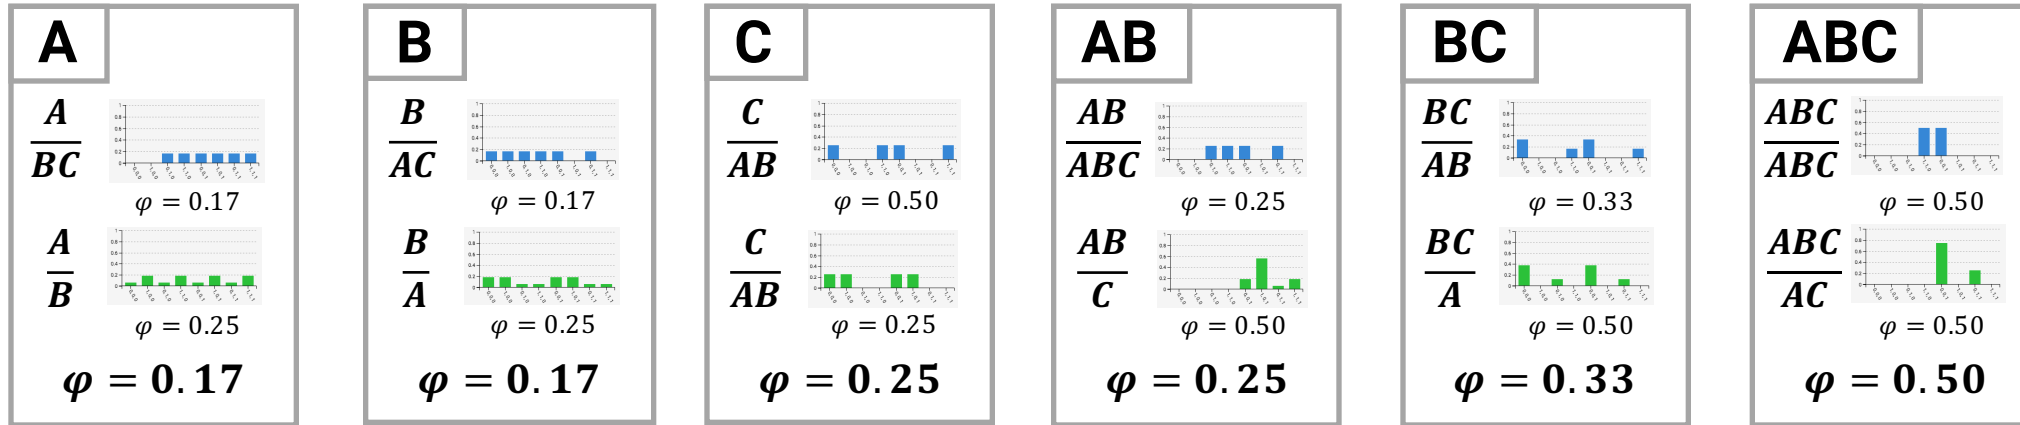

CUT

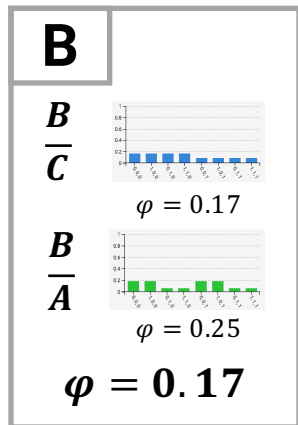

- In this case, the “earth” that we’re moving is the  $\varphi$ -value of each concept
- The cost of transporting  $\varphi$  from one concept to another is the **concept distance**
- This is the sum of the EMD between their cause repertoires and the EMD between their effect repertoires

# Integration and reducibility: Extended earth mover's distance

WHOLE

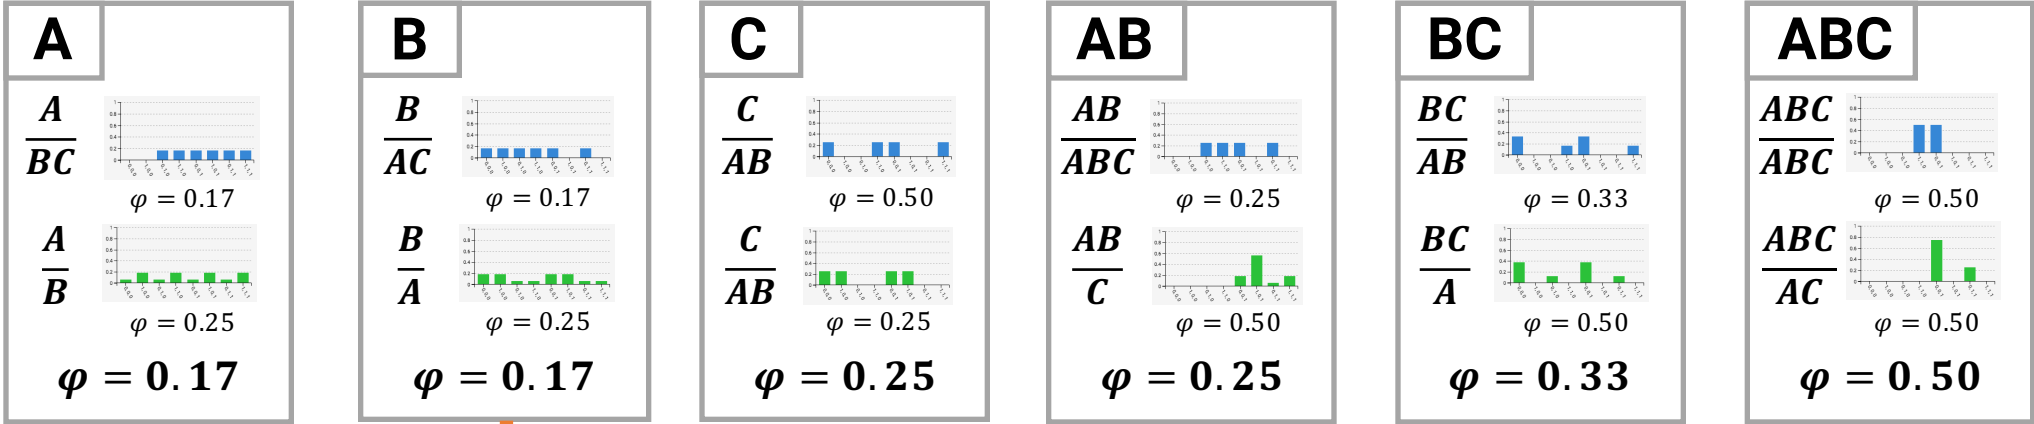

CUT

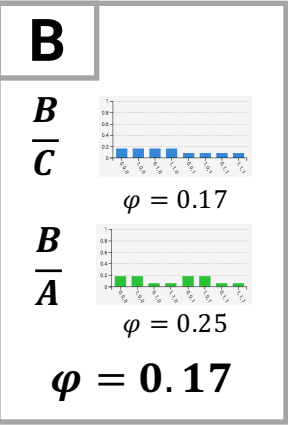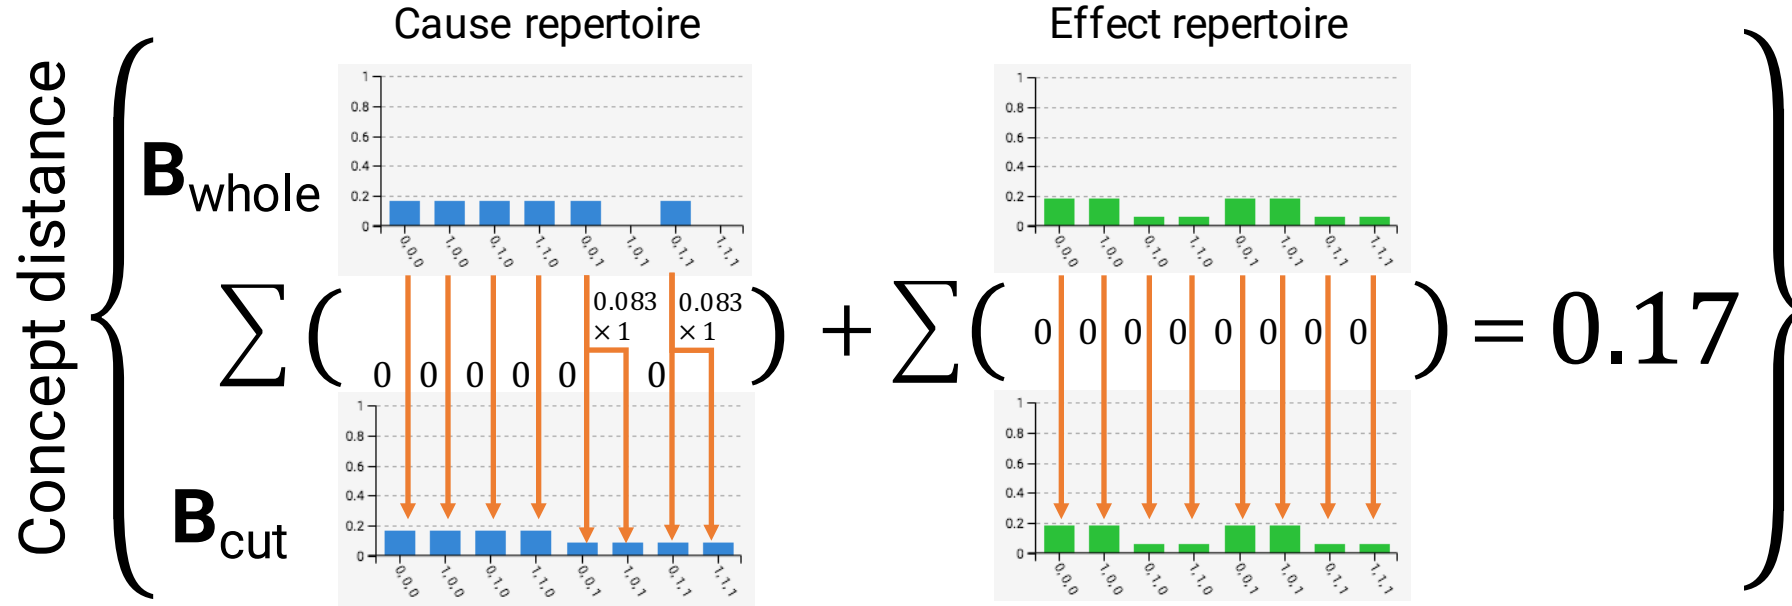

# Integration and reducibility: Extended earth mover's distance

WHOLE

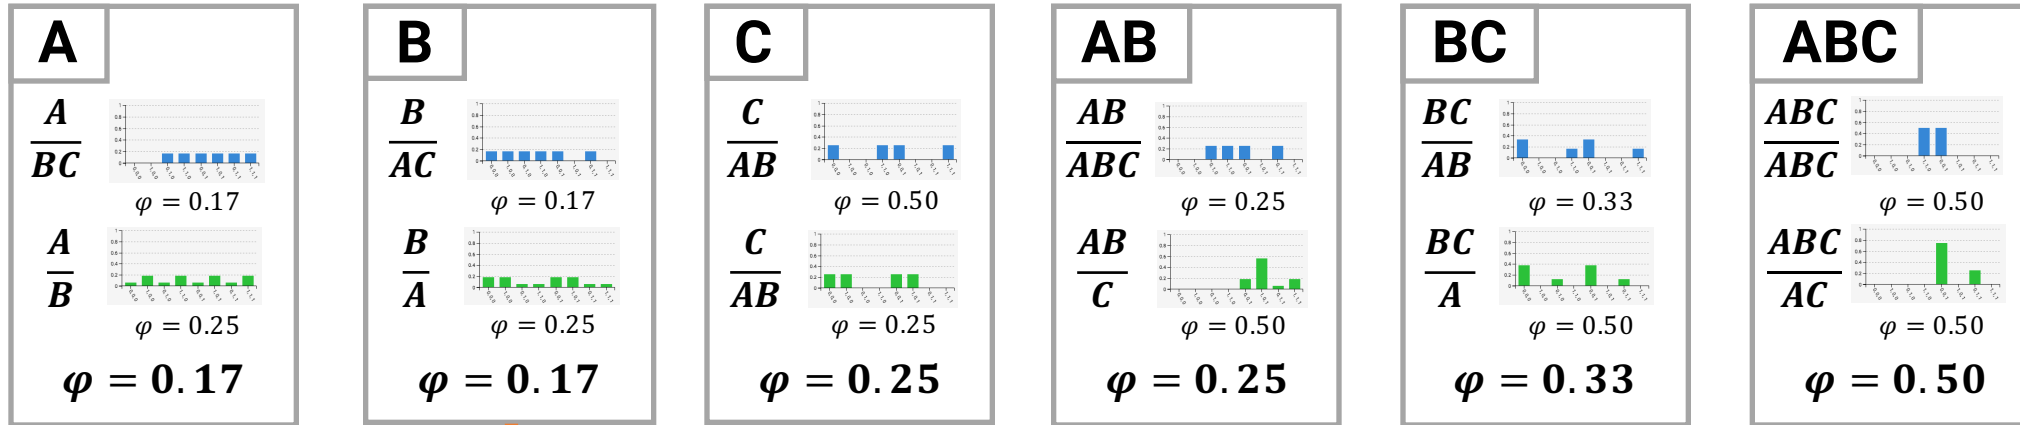

CUT

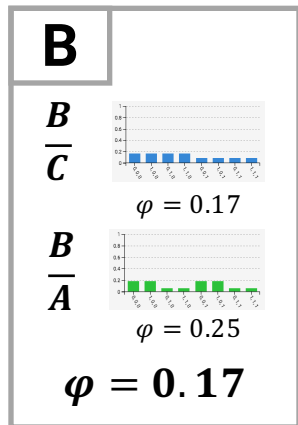

$$\underbrace{0.17}_{\text{Concept distance}} \times \underbrace{0.17}_{\varphi} = \underbrace{0.0289}_{\text{Cost of moving the } \varphi \text{ of } \mathbf{B}_{\text{whole}} \text{ to } \mathbf{B}_{\text{cut}}}$$

# Integration and reducibility: Extended earth mover's distance

WHOLE

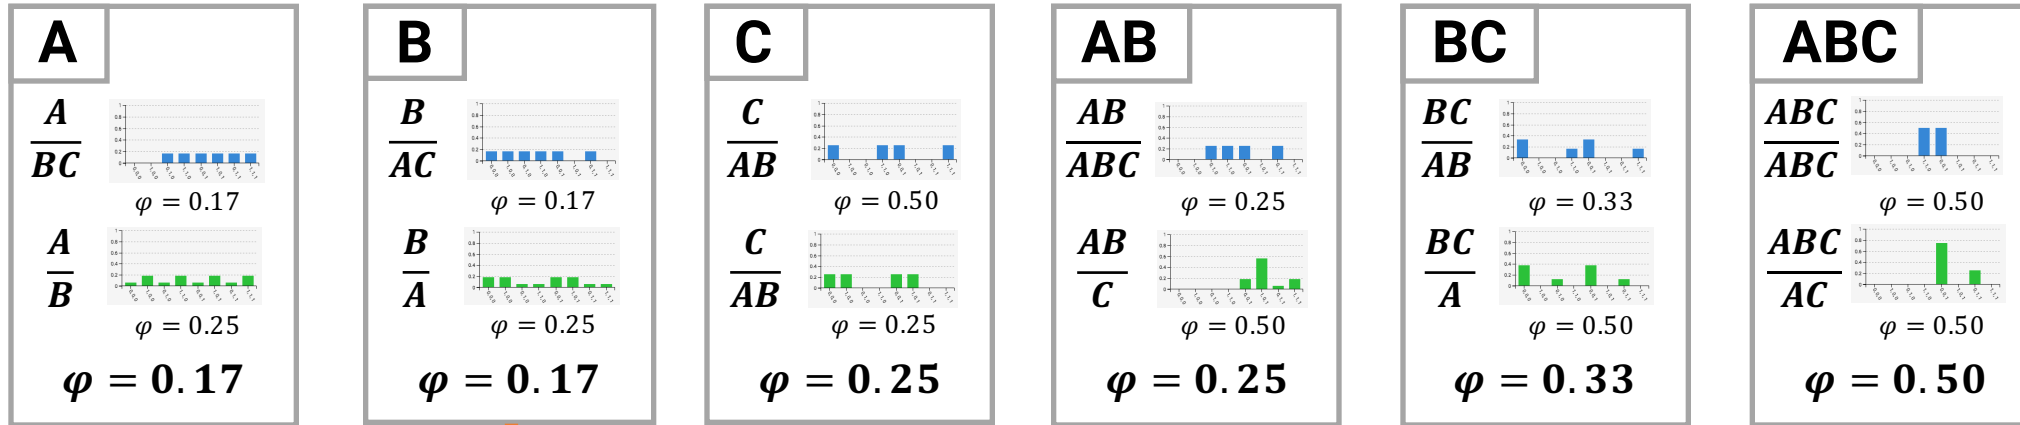

CUT

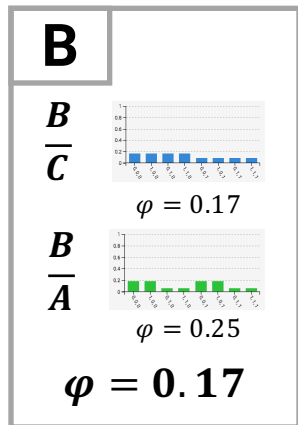

0.0289

- At this point, we've accounted for all the  $\varphi$  present in the partitioned cause-effect structure
- But we also have to account for the  $\varphi$  that disappeared when the other concepts were destroyed

# Integration and reducibility: Extended earth mover's distance

WHOLE

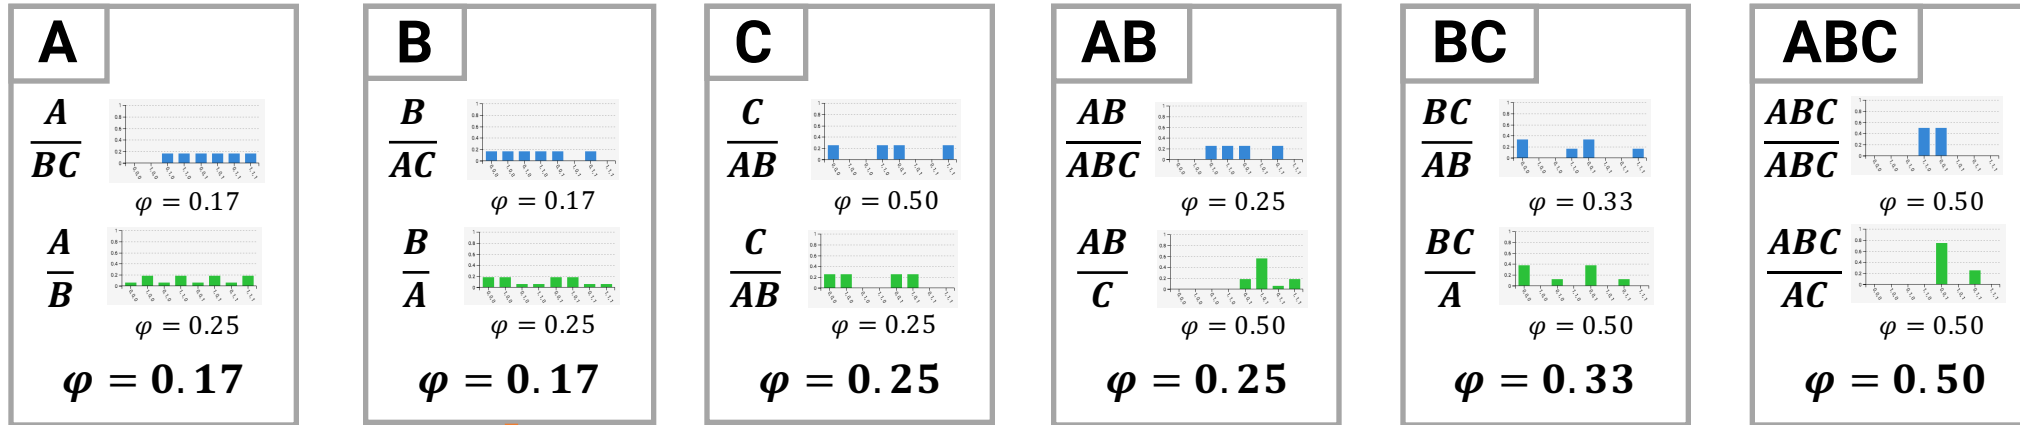

CUT

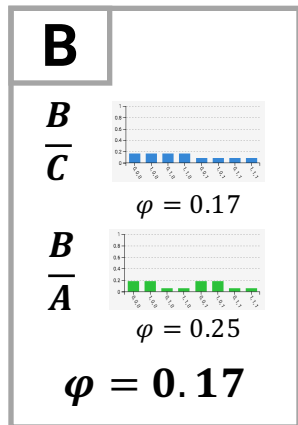

0.0289

- To do this, we transport all the “extra”  $\varphi$  to the **null concept**
- This is the concept that is specified by no mechanism (strictly speaking, it’s not a concept since it has  $\varphi = 0$ )

# Integration and reducibility: Extended earth mover's distance

WHOLE

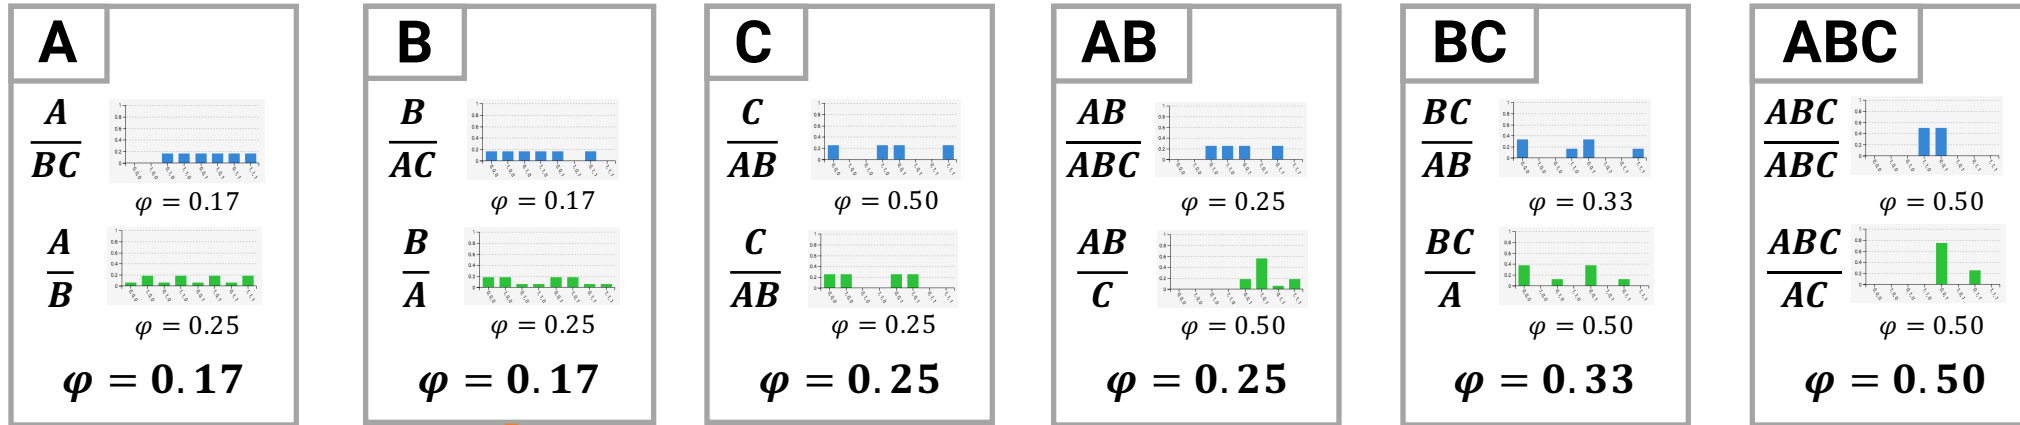

CUT

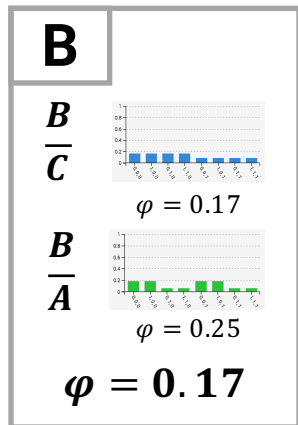

0.0289

- Since the null concept's mechanism is empty, its cause and effect repertoires are simply the unconstrained repertoires over the entire system
- So, the distance to the null concept is the sum of the distances to the unconstrained cause and effect repertoires

Integration and reducibility:  
**Extended earth mover's distance**

WHOLE

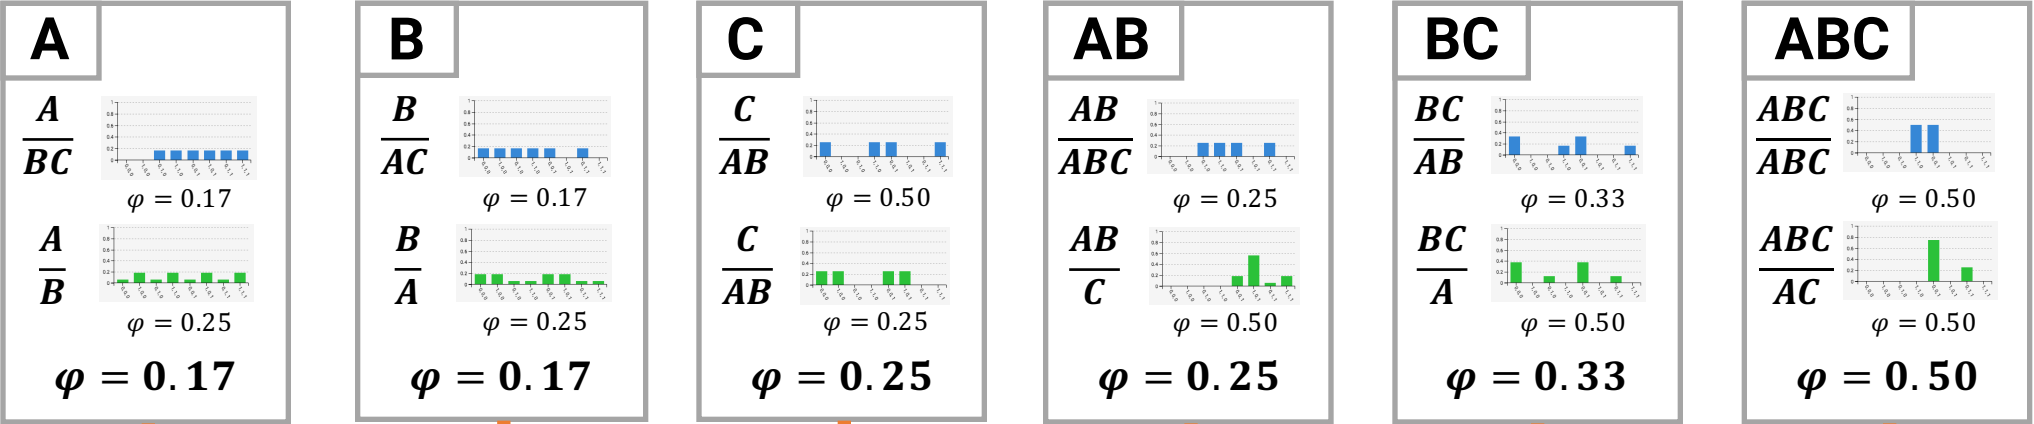

$0.583 \times \varphi_A$

$1 \times \varphi_C$

$1 \times \varphi_{AB}$

$1.25 \times \varphi_{BC}$

$2 \times \varphi_{ABC}$

CUT

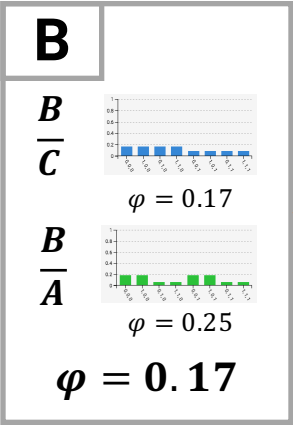

0.0289

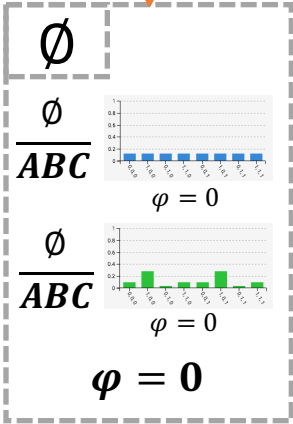

Null concept



Integration and reducibility:  
**Extended earth mover's distance**

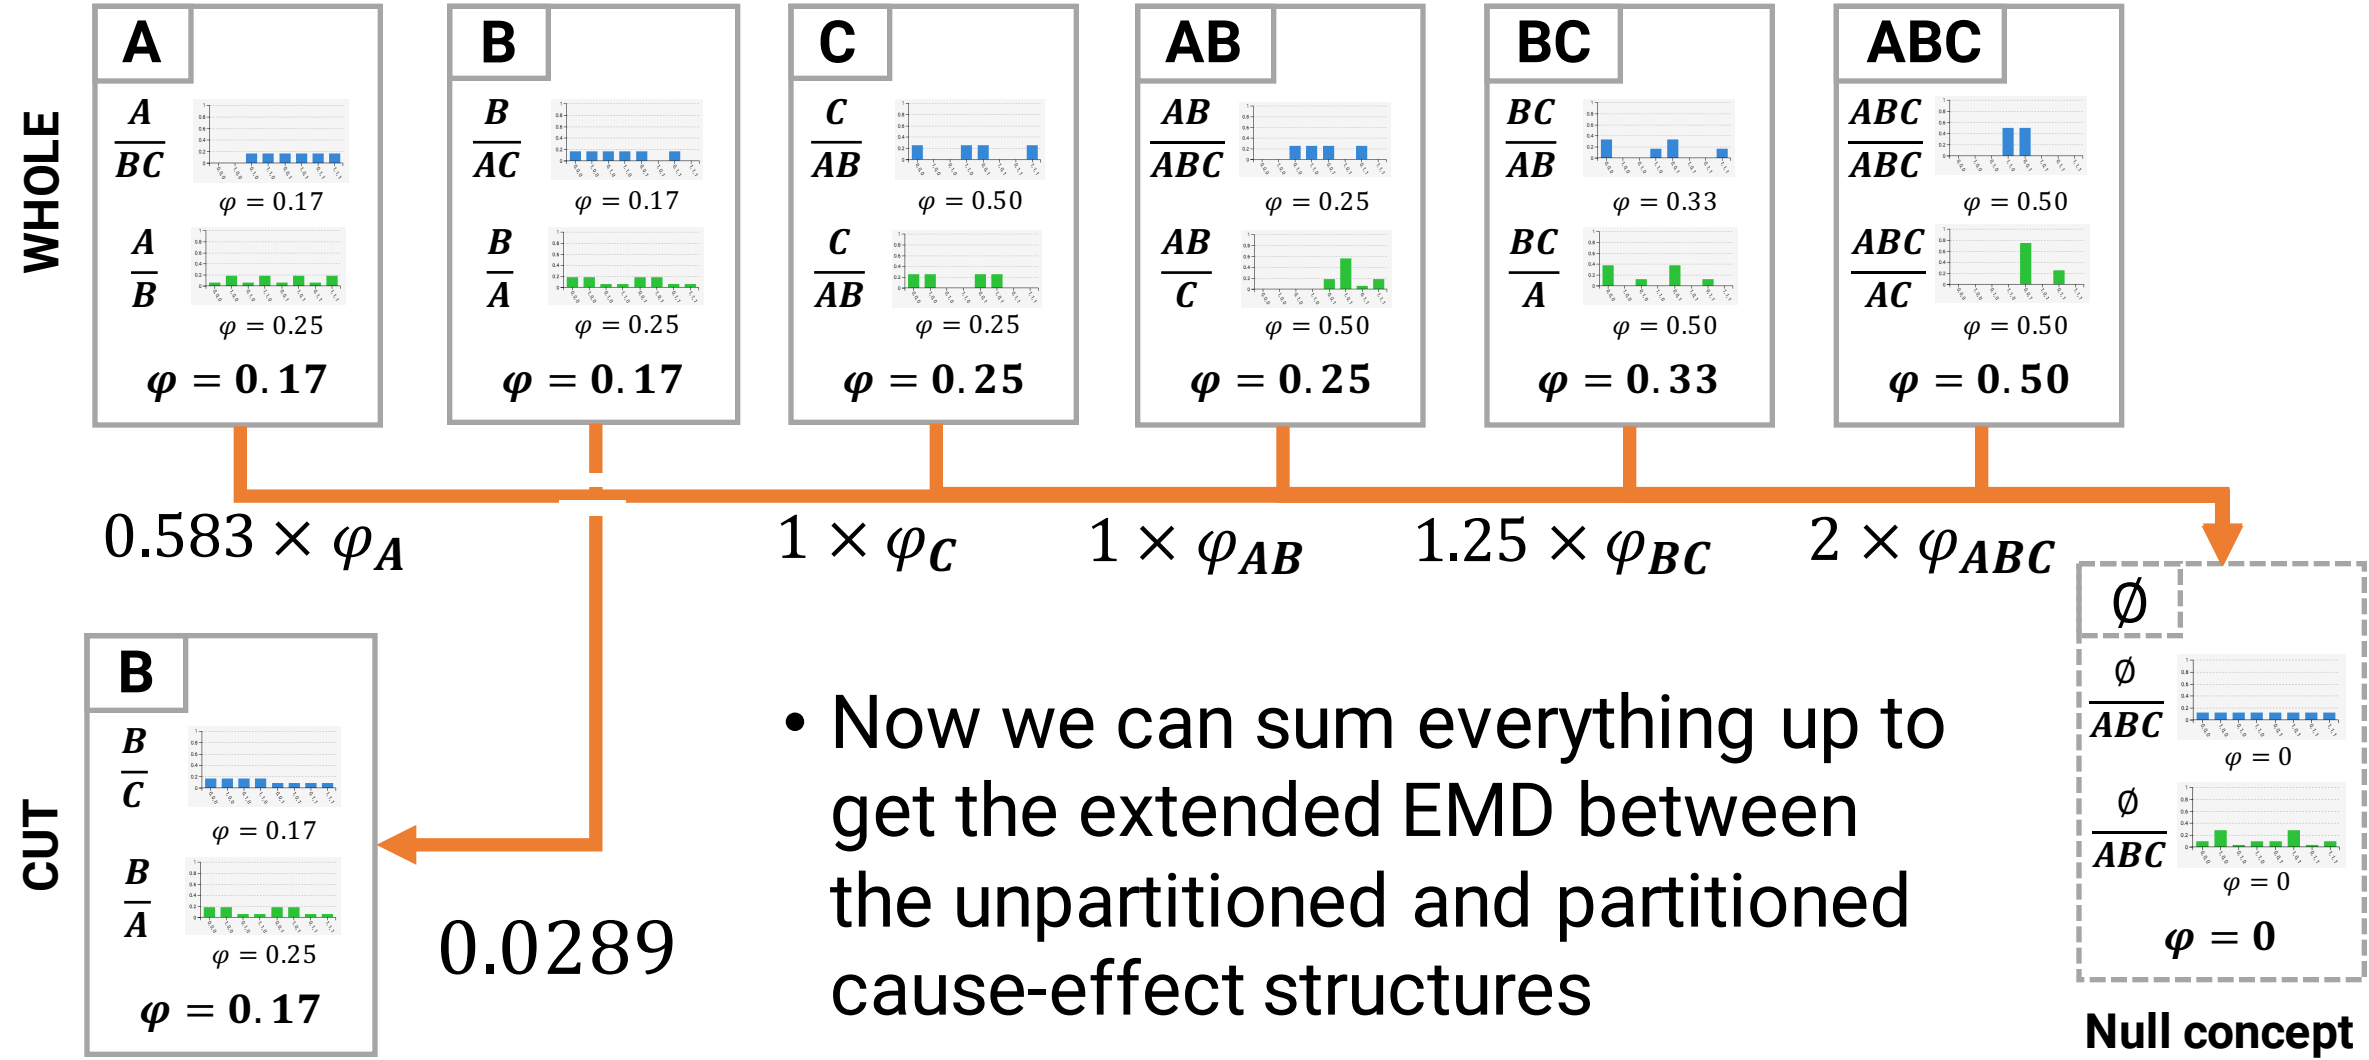

Integration and reducibility:  
**Extended earth mover's distance**

WHOLE

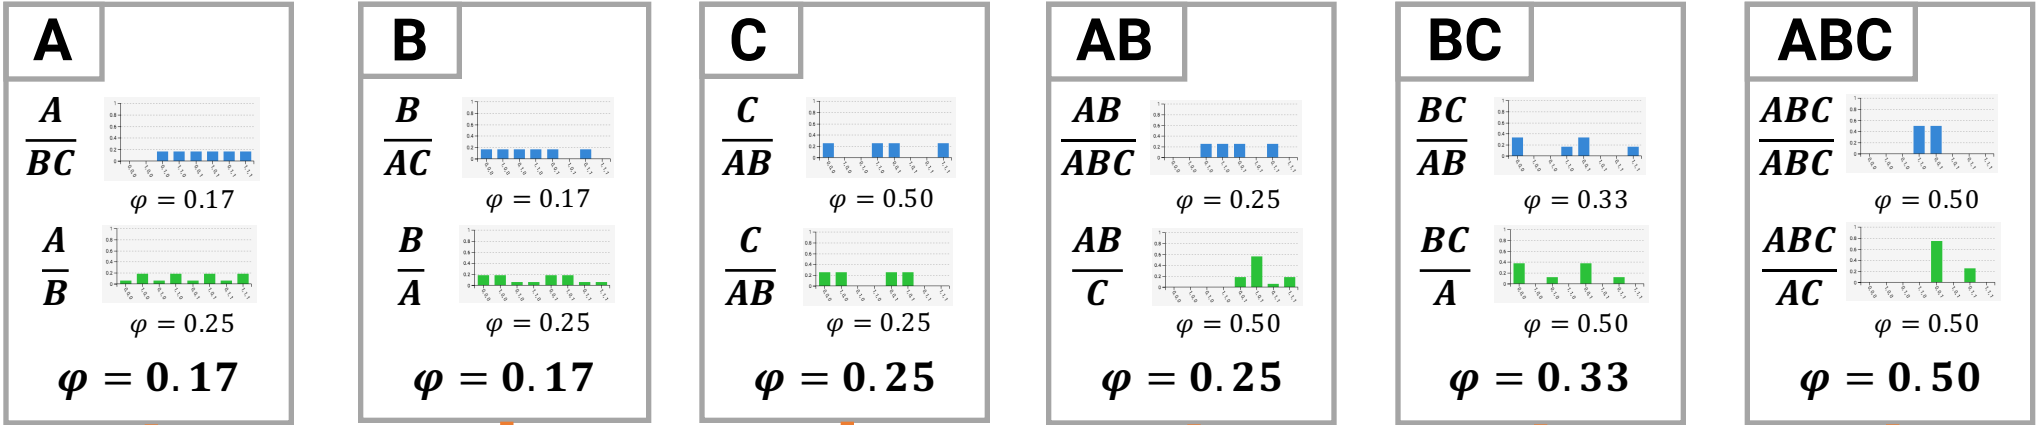

$0.583 \times \phi_A$

$1 \times \phi_C$

$1 \times \phi_{AB}$

$1.25 \times \phi_{BC}$

$2 \times \phi_{ABC}$

CUT

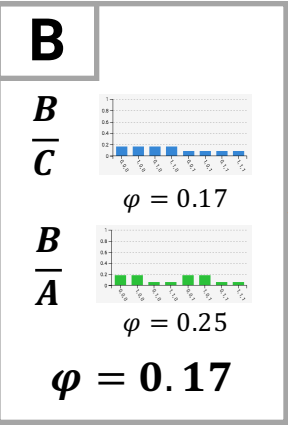

$0.097 + 0.0289 + 0.25 + 0.25 + .4125 + 1$

$= 2.0416$

$0.0289$

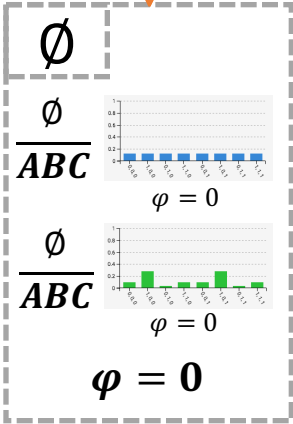

Null concept

# Integration and reducibility: Extended earth mover's distance

WHOLE

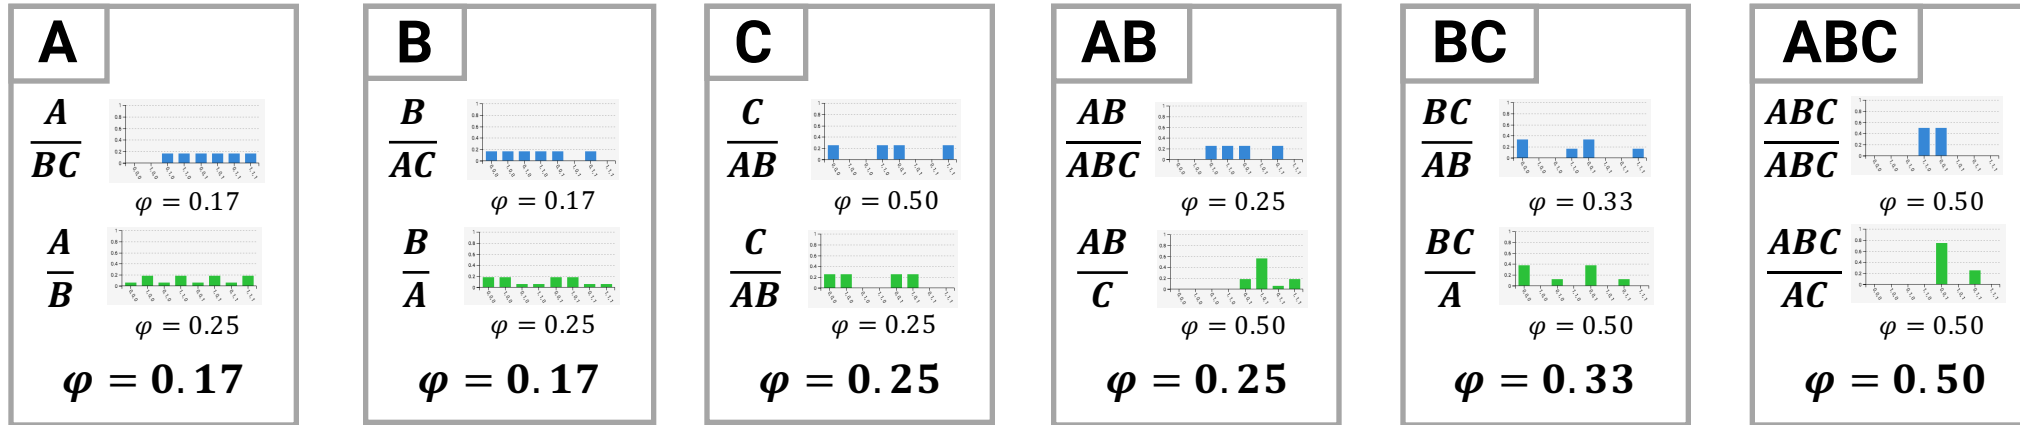

CUT

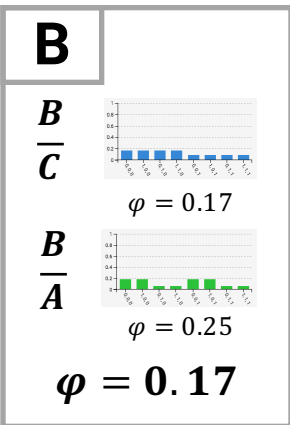

- This quantity is called **integrated conceptual information**, and is denoted  $\Phi$  (“big-phi”)
- It captures how irreducible the cause-effect structure of the system is, with respect to this particular cut

Integration and reducibility:

## System-level minimum information partition

- However, as with partitioning mechanisms, there are different ways to cut the system in two:

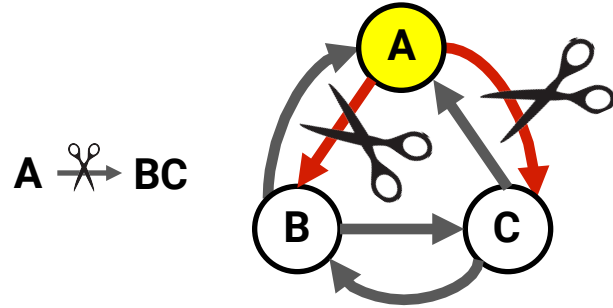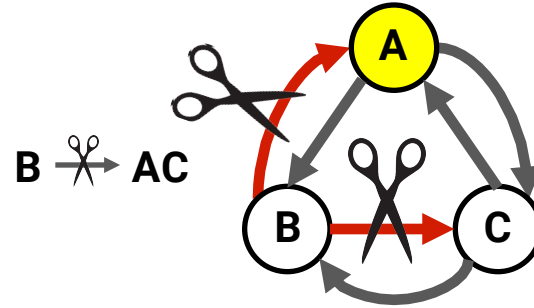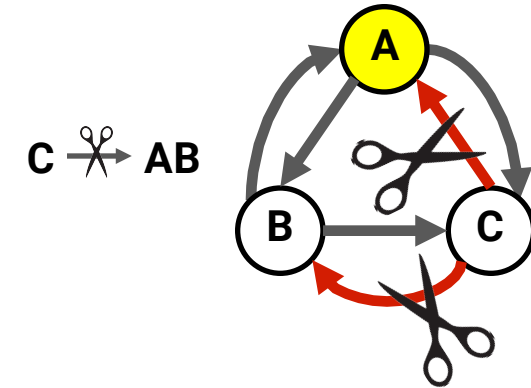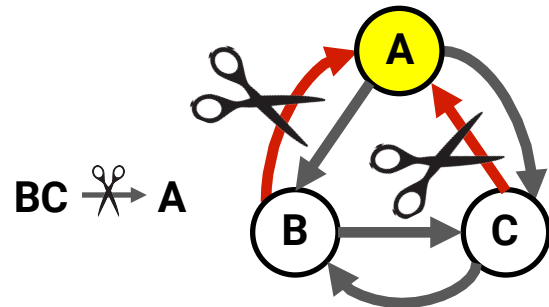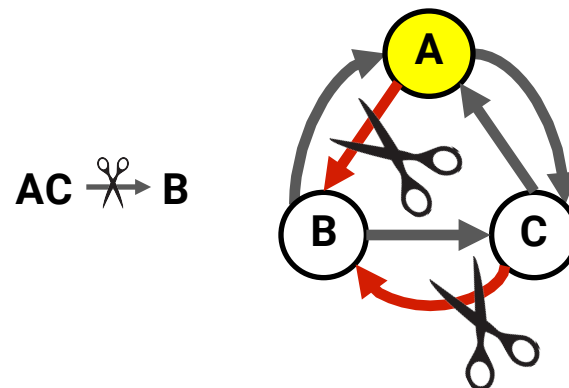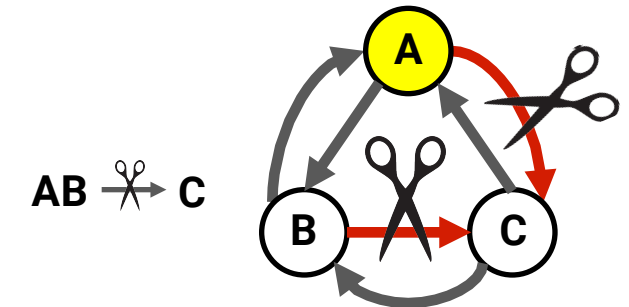

Integration and reducibility:  
**System-level minimum information partition**

- So, we perform every possible cut, determine the cause-effect structure for each of the cut systems, and calculate the  $\Phi$ -value associated with each
- The cut that yields the minimal  $\Phi$ -value is again called the **minimum information partition** (MIP) for the system

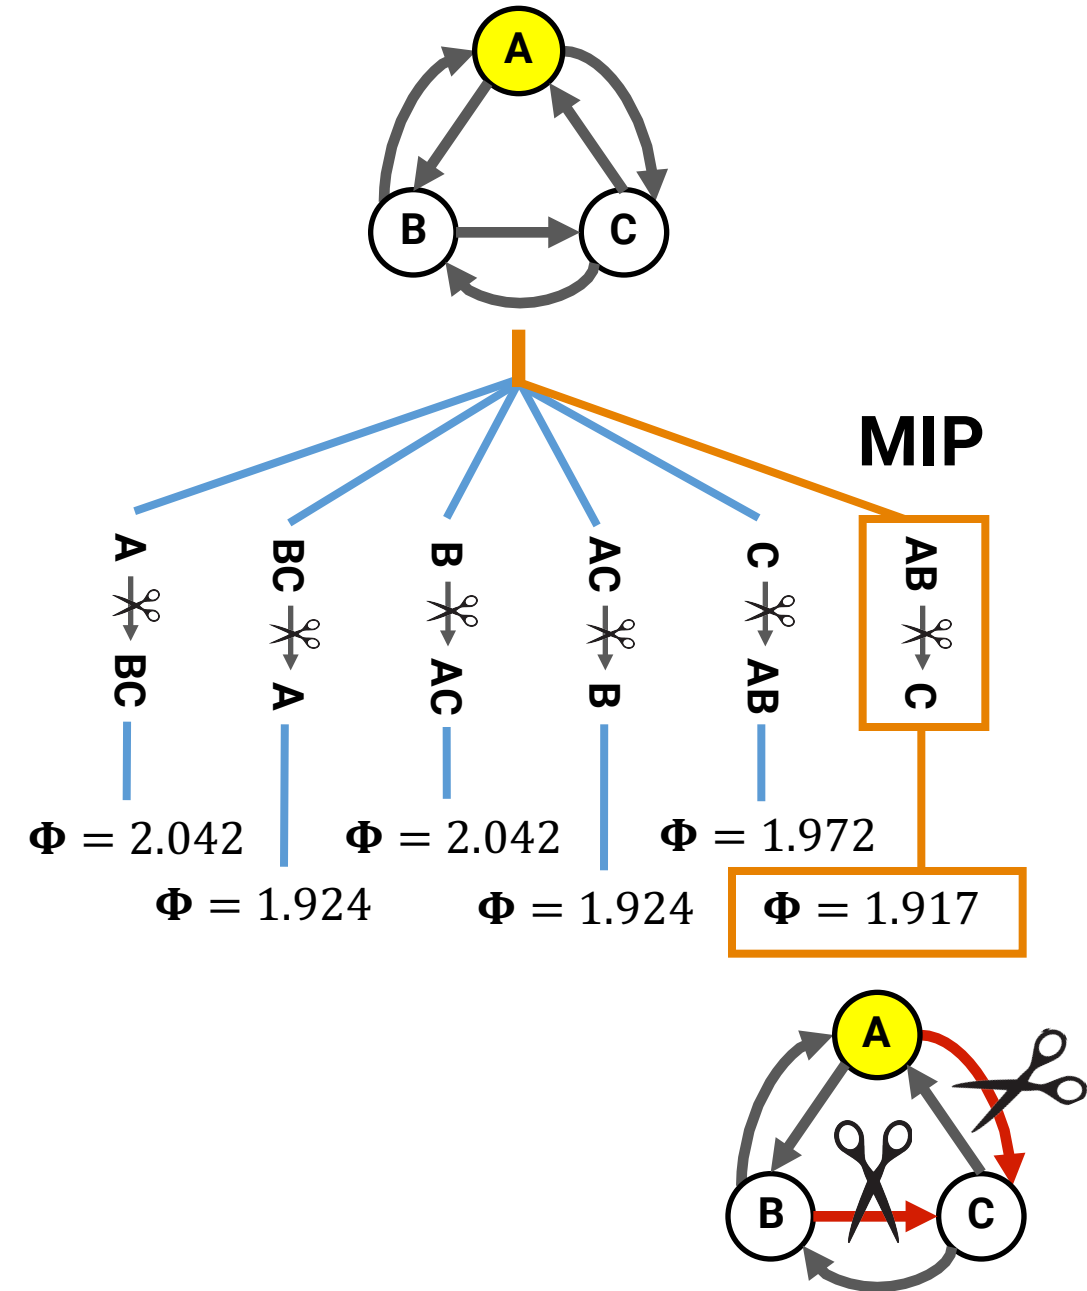

Integration and reducibility:  
**Integrated information**

- The minimal  $\Phi$ -value,  $\Phi^{\text{MIP}}$ , is the  $\Phi$  of the whole candidate system
- As with mechanisms, the cut that makes the *least difference* to the candidate system captures how intrinsically irreducible it is

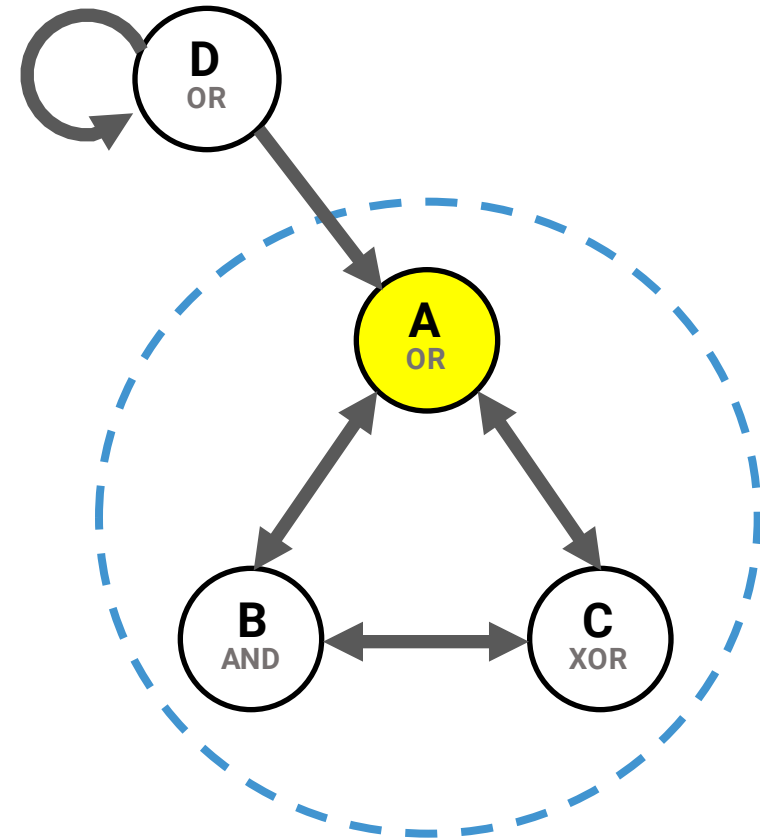

Candidate system **ABC**

$$\Phi = 1.917$$

# Outline

- Elements, states, and the TPM
- Background conditions
- Cause-effect repertoires
- Integrated mechanisms:  $\varphi$
- Concepts and cause-effect structures
- Integrated systems:  $\Phi$
- **Complexes**

Integration and reducibility:  
**Complexes**

- Now, recall that we began the analysis by choosing a candidate system to evaluate
- $\Phi$  is evaluated for each possible candidate system, and the candidate system with the maximal value,  $\Phi^{\max}$ , is called a **complex**
- For brevity we don't consider all candidate systems that include **D**, since the cut **ABC**  $\not\Rightarrow$  **D** will trivially have  $\Phi = 0$

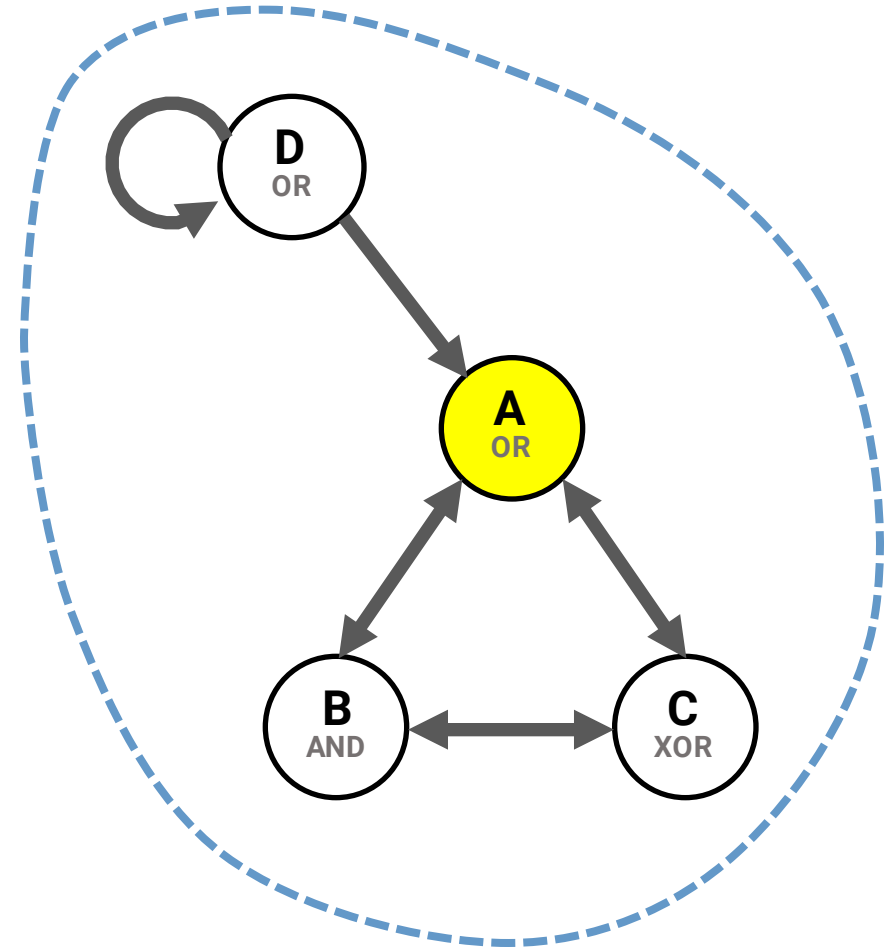

Candidate system **ABCD**

$$\Phi = 0$$



## Integration and reducibility: **Complexes**

- Now, recall that we began the analysis by choosing a candidate system to evaluate
- $\Phi$  is evaluated for each possible candidate system, and the candidate system with the maximal value,  $\Phi^{\max}$ , is called a **complex**
- For brevity we don't consider all candidate systems that include **D**, since the cut **ABC**  $\not\Rightarrow$  **D** will trivially have  $\Phi = 0$

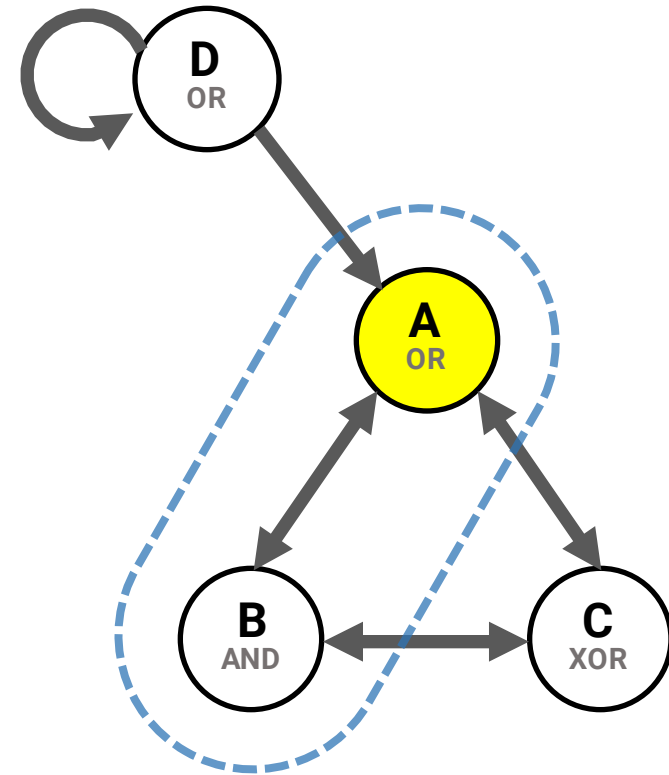

Candidate system **AB**

$$\Phi = 0$$

## Integration and reducibility: **Complexes**

- Now, recall that we began the analysis by choosing a candidate system to evaluate
- $\Phi$  is evaluated for each possible candidate system, and the candidate system with the maximal value,  $\Phi^{\max}$ , is called a **complex**
- For brevity we don't consider all candidate systems that include **D**, since the cut **ABC**  $\not\Rightarrow$  **D** will trivially have  $\Phi = 0$

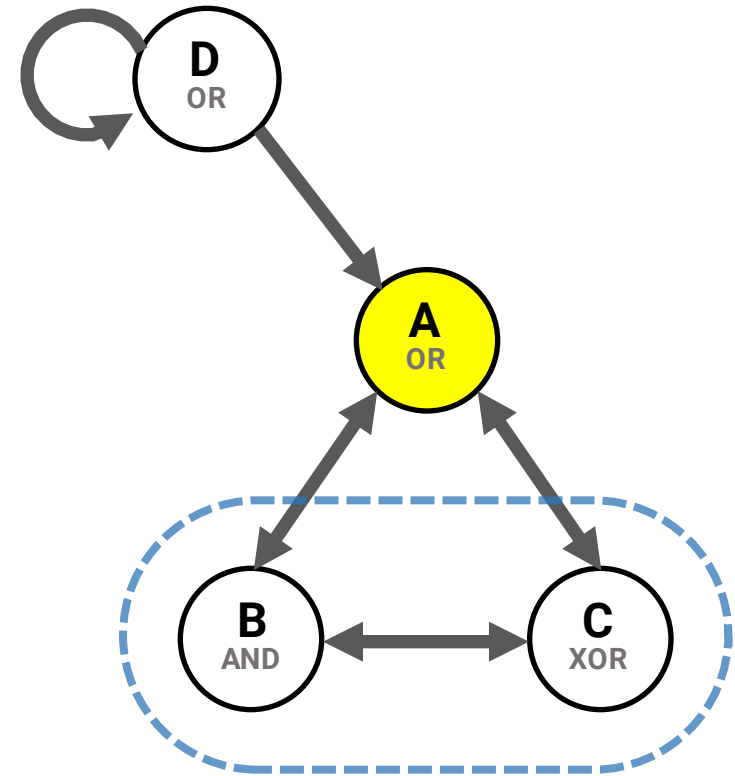

Candidate system **BC**

$$\Phi = 1.0$$

## Integration and reducibility: **Complexes**

- Now, recall that we began the analysis by choosing a subset of the network to evaluate as a candidate system
- The next step is to evaluate  $\Phi$  for every candidate system
- The system with the maximal value,  $\Phi^{\max}$ , is called a **complex**
- For brevity we don't consider all candidate systems that include **D**, since the cut **ABC**  $\nRightarrow$  **D** will trivially have  $\Phi = 0$

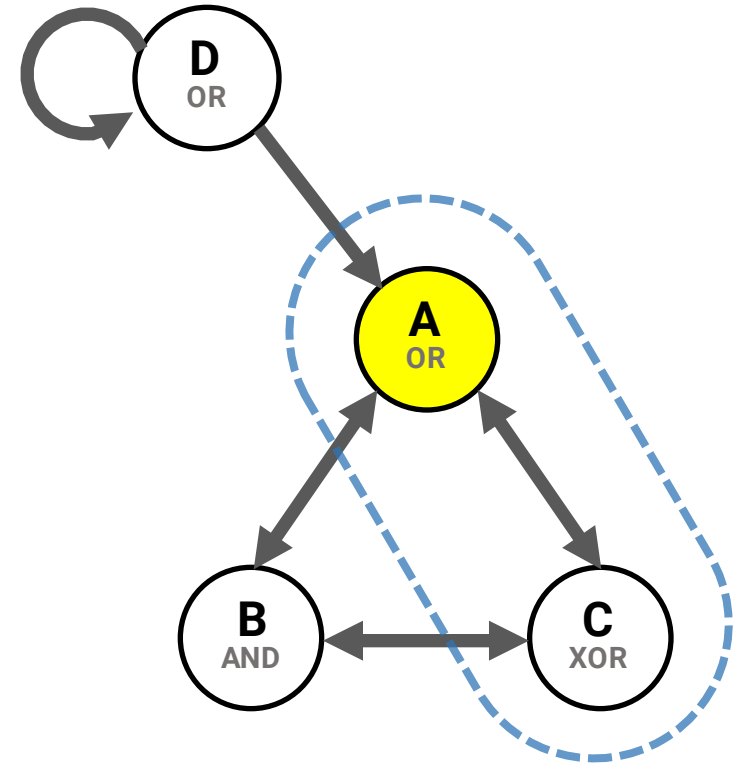

Candidate system **AC**

$$\Phi = 1.0$$

Integration and reducibility:  
**Complexes**

- The exclusion postulate of IIT dictates that only a complex exists as an integrated entity with a subjective experience
- This defines the “borders” of the physical substrate of consciousness (e.g. the brain, without the sensory or motor neurons)

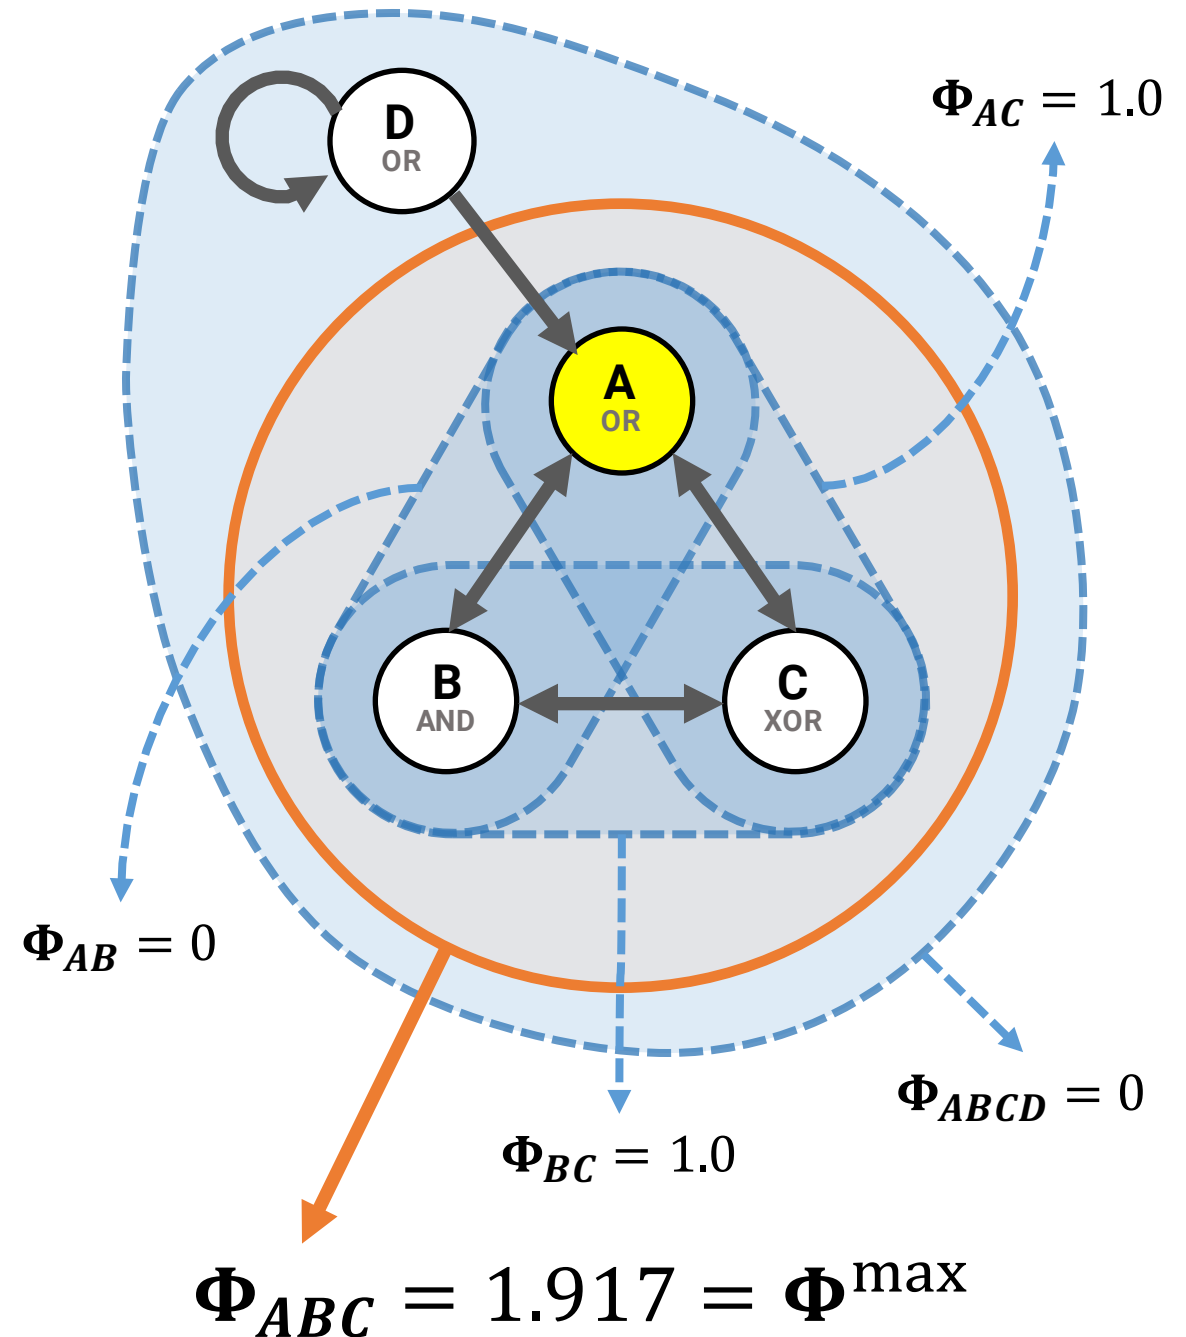

Integration and reducibility:  
**Complexes**

- Finally, note that in general, the search for the system with  $\Phi^{\max}$  must also be carried out over all spatiotemporal groupings of elements

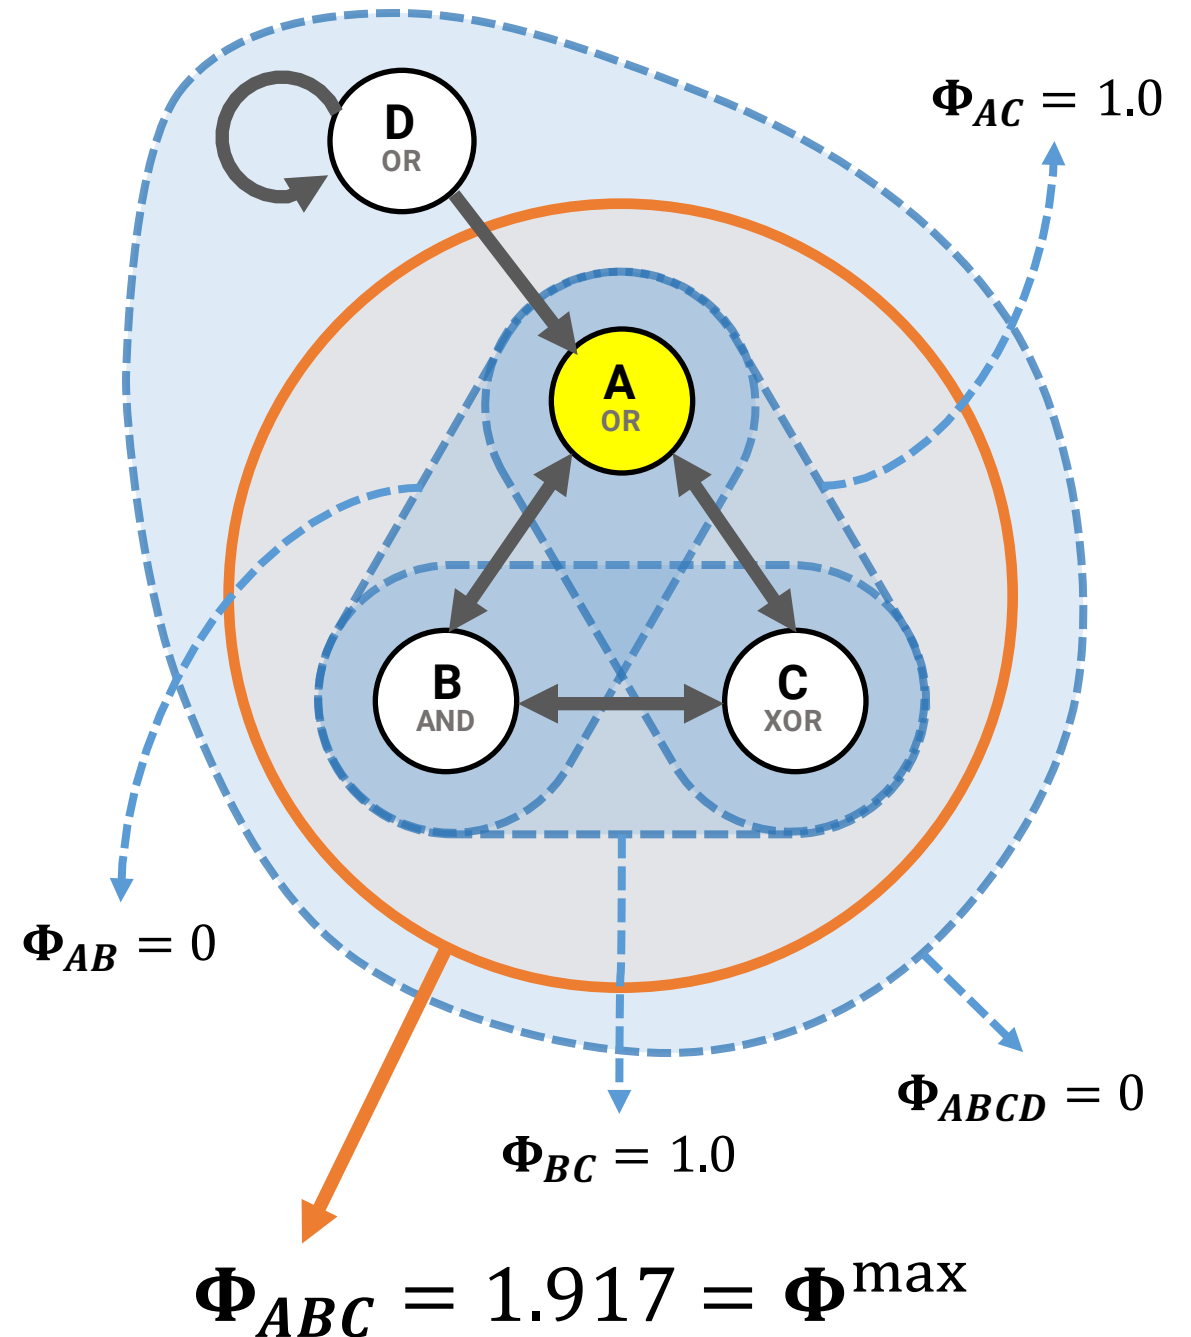

Supplement: Supplementary file 1 [file S1_Calculating_Phi.pdf]
